# Supplementary material for: Construction of nice nilpotent Lie groups
Source: arXiv:1803.09248 ancillary file (2019-02-15)
Supplement: Supplementary file 1 [file AncillaryLargeTables.pdf]

# Tables of nice nilpotent Lie groups in dimension 8 and 9

Part of “Construction of nice nilpotent Lie groups”  
by Diego Conti and Federico A. Rossi

March 24, 2018

We give the complete list of nice nilpotent Lie algebras in dimensions 8 and 9. In both tables, the columns contain the name of the nice Lie algebra, the structure equations in the nice basis and the dimensions of the upper central series (UCS).

For more details, refer to the main article.

## A Table 1 8-dimensional nice nilpotent Lie algebras

Table 1: 8-dimensional nice nilpotent Lie algebras

| Name          | $\mathfrak{g}$                                                                                                                                     | UCS Dim. |
|---------------|----------------------------------------------------------------------------------------------------------------------------------------------------|----------|
| Type: 2111111 |                                                                                                                                                    |          |
| 8654321:1     | $0, 0, e^{12}, e^{13}, e^{14}, e^{15}, e^{16}, e^{17}$                                                                                             | 1234568  |
| 8654321:2     | $0, 0, e^{12}, e^{13}, e^{14}, e^{15}, e^{16}, e^{17} + e^{23}$                                                                                    | 1234568  |
| 8654321:3     | $0, 0, e^{12}, e^{13}, e^{14}, e^{15}, e^{16} + e^{23}, e^{24} + e^{17}$                                                                           | 1234568  |
| 8654321:4     | $0, 0, -e^{12}, e^{13}, e^{14}, e^{15}, e^{16}, e^{25} + e^{34} + e^{17}$                                                                          | 1234568  |
| 8654321:5     | $0, 0, -e^{12}, -e^{13}, e^{14}, e^{15}, e^{16}, e^{36} + e^{27} + e^{45}$                                                                         | 1234568  |
| 8654321:6     | $0, 0, e^{12}, e^{13}, e^{14}, e^{15} + e^{23}, e^{24} + e^{16}, e^{25} + e^{17}$                                                                  | 1234568  |
| 8654321:7     | $0, 0, e^{12}, e^{13}, e^{14}, e^{15} + e^{23}, e^{24} + e^{16}, e^{34} + e^{17}$                                                                  | 1234568  |
| 8654321:11    | $0, 0, -e^{12}, -e^{13}, e^{14}, e^{15}, e^{16} + e^{23}, e^{36} + e^{27} + e^{45}$                                                                | 1234568  |
| 8654321:12    | $0, 0, e^{12}, e^{13}, e^{14} + e^{23}, e^{24} + e^{15}, e^{25} + e^{16}, e^{26} + e^{17}$                                                         | 1234568  |
| 8654321:14    | $0, 0, a_1 e^{12}, e^{13}, -(-1 + a_1) e^{14}, e^{15} + e^{23}, e^{24} + e^{16}, e^{25} + e^{34} + e^{17}$                                         | 1234568  |
| 8654321:15    | $0, 0, -e^{12}, e^{13}, e^{14}, 2e^{15}, e^{25} + e^{34} + e^{16}, e^{26} + e^{35} + e^{17}$                                                       | 1234568  |
| 8654321:17    | $0, 0, -e^{12}, e^{13}, e^{14}, -e^{15} + e^{23}, e^{24} + e^{16}, e^{36} + e^{27} + e^{45}$                                                       | 1234568  |
| 8654321:19    | $0, 0, e^{12}, e^{13}, e^{14} + e^{23}, e^{24} + e^{15}, e^{25} + e^{34} + 2e^{16}, e^{35} + e^{17}$                                               | 1234568  |
| 8654321:20    | $0, 0, e^{12}, -e^{13}, e^{14} + e^{23}, e^{24} - e^{15}, e^{34} + e^{16}, e^{26} + e^{35} + e^{17}$                                               | 1234568  |
| 8654321:24    | $0, 0, (1 - a_4) e^{12}, e^{13} a_4, e^{14} + e^{23}, e^{15} a_4 + e^{24}, -e^{16}(-2 + a_4) + e^{25} + e^{34}, e^{26} + e^{35} + e^{17}$          | 1234568  |
| 8654321:25    | $0, 0, -e^{12}, -e^{13}, \frac{3}{2} e^{14} - \frac{1}{2} e^{23}, \frac{1}{2} e^{24} + e^{15}, e^{25} + e^{34} + e^{16}, e^{36} + e^{27} + e^{45}$ | 1234568  |
| Type: 211121  |                                                                                                                                                    |          |
| 865431:1      | $0, 0, -e^{12}, e^{13}, e^{14}, e^{15}, e^{25} + e^{34}, e^{16}$                                                                                   | 234568   |
| 865431:2      | $0, 0, -e^{12}, e^{13}, e^{14}, e^{15}, e^{25} + e^{34}, e^{16} + e^{23}$                                                                          | 234568   |
| 865431:4      | $0, 0, -e^{12}, e^{13}, e^{14}, e^{15} + e^{23}, e^{25} + e^{34}, e^{24} + e^{16}$                                                                 | 234568   |
| 865431:7      | $0, 0, -e^{12}, e^{13}, e^{14}, 2e^{15}, e^{25} + e^{34}, e^{26} + e^{35} + e^{17}$                                                                | 134568   |
| 865431:8      | $0, 0, -e^{12}, e^{13}, e^{14}, 2e^{15} + e^{23}, e^{25} + e^{34}, e^{26} + e^{35} + e^{17}$                                                       | 134568   |
| 865431:9      | $0, 0, -e^{12}, 2e^{13}, e^{14} + e^{23}, e^{24} + 2e^{15}, e^{25} + e^{34}, e^{26} + e^{35} + e^{17}$                                             | 134568   |
| Type: 212111  |                                                                                                                                                    |          |
| 865321:1      | $0, 0, e^{12}, e^{13}, e^{23}, e^{14}, e^{16}, e^{17}$                                                                                             | 234568   |
| 865321:2a     | $0, 0, e^{12}, e^{13}, e^{23}, e^{14}, e^{16}, e^{25} + e^{17}$                                                                                    | 134568   |
| 865321:2b     | $0, 0, e^{12}, -e^{13}, e^{23}, e^{14}, e^{16}, e^{25} + e^{17}$                                                                                   | 134568   |
| 865321:3      | $0, 0, e^{12}, e^{13}, e^{23}, e^{14}, e^{25} + e^{16}, e^{35} + e^{17}$                                                                           | 124568   |
| 865321:5      | $0, 0, -e^{12}, e^{13}, e^{23}, e^{14}, e^{16}, e^{26} + e^{34} + e^{17}$                                                                          | 234568   |
| Type: 21212   |                                                                                                                                                    |          |

Table 1 – Continued to next page

Table 1 – Continued from previous page

| Name        | g                                                                                                         | UCS Dim. |
|-------------|-----------------------------------------------------------------------------------------------------------|----------|
| 86532:1     | $0, 0, -e^{12}, e^{13}, e^{23}, e^{14}, e^{16}, e^{26} + e^{34}$                                          | 34568    |
| 86532:2     | $0, 0, -e^{12}, e^{13}, e^{23}, e^{14}, e^{26} + e^{34}, e^{25} + e^{16}$                                 | 24568    |
| 86532:3     | $0, 0, e^{12}, -e^{13}, e^{23}, e^{24} - e^{15}, e^{34} + e^{16}, e^{26} + e^{35}$                        | 23568    |
| 86532:4a    | $0, 0, e^{12}, e^{13}, e^{23}, e^{25} - e^{14}, e^{26} + e^{34}, e^{35} + e^{16}$                         | 23568    |
| 86532:4b    | $0, 0, e^{12}, -e^{13}, e^{23}, e^{25} - e^{14}, e^{26} + e^{34}, e^{35} + e^{16}$                        | 23568    |
| 86532:5     | $0, 0, e^{12}, -e^{13}, e^{23}, e^{24} - e^{15}, e^{34} + e^{16}, e^{26} + e^{35} + e^{14}$               | 23568    |
| 86532:6     | $0, 0, e^{12}, -e^{13}, e^{23}, e^{24} - e^{15}, e^{25} + e^{34} + e^{16}, e^{26} + e^{35} + e^{14}$      | 23568    |
| Type: 21221 |                                                                                                           |          |
| 86531:1     | $0, 0, e^{12}, e^{13}, e^{23}, e^{14}, e^{25}, e^{16}$                                                    | 24568    |
| 86531:2     | $0, 0, e^{12}, e^{13}, e^{23}, e^{14}, e^{24} + e^{15}, e^{16}$                                           | 24568    |
| 86531:3     | $0, 0, -e^{12}, e^{13}, e^{23}, e^{14}, e^{25}, e^{26} + e^{34}$                                          | 24568    |
| 86531:4     | $0, 0, e^{12}, e^{13}, e^{23}, e^{14}, e^{24} + e^{15}, e^{25} + e^{16}$                                  | 24568    |
| 86531:5     | $0, 0, -e^{12}, e^{13}, e^{23}, e^{14}, e^{24} + e^{15}, e^{26} + e^{34}$                                 | 24568    |
| 86531:6     | $0, 0, e^{12}, e^{13}, e^{23}, e^{24} + e^{15}, e^{14}, e^{34} + e^{16}$                                  | 23568    |
| 86531:7     | $0, 0, -e^{12}, e^{13}, e^{23}, e^{24} + e^{15}, e^{14}, e^{26} + e^{35}$                                 | 23568    |
| 86531:8a    | $0, 0, e^{12}, e^{13}, e^{23}, e^{24} + e^{15}, e^{25} + e^{14}, e^{34} + e^{16}$                         | 23568    |
| 86531:8b    | $0, 0, e^{12}, -e^{13}, e^{23}, e^{24} - e^{15}, e^{25} + e^{14}, e^{34} + e^{16}$                        | 23568    |
| 86531:9a    | $0, 0, e^{12}, e^{13}, e^{23}, e^{25} - e^{14}, e^{24} + e^{15}, e^{26} + e^{34}$                         | 23568    |
| 86531:9b    | $0, 0, -e^{12}, e^{13}, e^{23}, e^{25} + e^{14}, e^{24} + e^{15}, e^{26} + e^{34}$                        | 23568    |
| 86531:10    | $0, 0, e^{12}, e^{13}, e^{23}, e^{24} + e^{15}, e^{14}, e^{25} + e^{34} + e^{16}$                         | 23568    |
| 86531:11    | $0, 0, e^{12}, e^{13}, e^{23}, e^{14}, e^{25}, e^{27} + e^{16}$                                           | 13568    |
| 86531:12    | $0, 0, e^{12}, e^{13}, e^{23}, e^{14}, e^{24} + e^{15}, e^{26} + e^{17}$                                  | 13568    |
| 86531:13a   | $0, 0, e^{12}, e^{13}, e^{23}, e^{24} + e^{15}, e^{25} + e^{14}, e^{27} + e^{16}$                         | 13568    |
| 86531:13b   | $0, 0, e^{12}, -e^{13}, e^{23}, e^{24} - e^{15}, e^{25} + e^{14}, e^{27} + e^{16}$                        | 13568    |
| 86531:14    | $0, 0, e^{12}a_1, e^{13}, e^{23}, -e^{14}(-1 + a_1), e^{24} + e^{15}, e^{26} + e^{34} + e^{17}$           | 13568    |
| 86531:15a   | $0, 0, -e^{12}, e^{13}, e^{23}, e^{14}, e^{24} + e^{15}, e^{27} + e^{35} + e^{16}$                        | 13568    |
| 86531:15b   | $0, 0, -e^{12}, e^{13}, e^{23}, -e^{14}, e^{24} + e^{15}, e^{27} + e^{35} + e^{16}$                       | 13568    |
| 86531:16a   | $0, 0, a_1e^{12}, e^{13}, e^{23}, e^{24} + e^{15}, -(-1 + a_1)e^{14} + e^{25}, e^{34} + e^{27} + e^{16}$  | 13568    |
| 86531:16b   | $0, 0, a_1e^{12}, -e^{13}, e^{23}, e^{24} - e^{15}, -(-1 + a_1)e^{14} + e^{25}, e^{34} + e^{27} + e^{16}$ | 13568    |
| Type: 31111 |                                                                                                           |          |
| 854321:1    | $0, 0, 0, e^{12}, e^{14}, e^{15}, e^{16}, e^{17}$                                                         | 234568   |
| 854321:2    | $0, 0, 0, e^{12}, e^{14}, e^{15}, e^{16}, e^{17} + e^{23}$                                                | 134568   |
| 854321:3    | $0, 0, 0, e^{12}, e^{14}, e^{15}, e^{16}, e^{24} + e^{17}$                                                | 234568   |
| 854321:4    | $0, 0, 0, -e^{12}, e^{14}, e^{15}, e^{16} + e^{23}, e^{34} + e^{17}$                                      | 124568   |
| 854321:5    | $0, 0, 0, -e^{12}, e^{14}, e^{15} + e^{23}, e^{34} + e^{16}, e^{35} + e^{17}$                             | 123568   |
| 854321:6    | $0, 0, 0, e^{12}, e^{14}, e^{15}, e^{24} + e^{16}, e^{25} + e^{17}$                                       | 234568   |
| 854321:8    | $0, 0, 0, -e^{12}, e^{14}, e^{15}, e^{16}, e^{26} + e^{17} + e^{45}$                                      | 234568   |
| 854321:11   | $0, 0, 0, -e^{12}, e^{14}, e^{15} + e^{23}, e^{34} + e^{16}, e^{24} + e^{35} + e^{17}$                    | 123568   |
| 854321:12   | $0, 0, 0, e^{12}, e^{14}, e^{24} + e^{15}, e^{25} + e^{16}, e^{45} + e^{17}$                              | 234568   |
| 854321:13   | $0, 0, 0, e^{12}, e^{14}, e^{24} + e^{15}, e^{25} + e^{16}, e^{26} + e^{17}$                              | 234568   |
| 854321:17   | $0, 0, 0, e^{12}, e^{14}, e^{24} + e^{15}, e^{25} + e^{16}, e^{45} + e^{17} + e^{23}$                     | 134568   |
| 854321:18   | $0, 0, 0, -e^{12}, e^{14} + e^{23}, e^{34} + e^{15}, e^{35} + e^{16}, e^{36} + e^{17}$                    | 123468   |
| 854321:20   | $0, 0, 0, -(-1 + a_3)e^{12}, e^{14}, e^{15}a_3 + e^{24}, e^{25} + e^{16}, e^{45} + e^{26} + e^{17}$       | 234568   |
| 854321:23   | $0, 0, 0, -e^{12}, e^{14} + e^{23}, e^{34} + e^{15}, e^{35} + e^{16}, e^{24} + e^{36} + e^{17}$           | 123468   |
| 854321:25   | $0, 0, 0, -e^{12}, e^{14} + e^{23}, e^{34} + e^{15}, e^{24} + e^{35} + e^{16}, e^{36} + e^{25} + e^{17}$  | 123468   |
| Type: 31112 |                                                                                                           |          |
| 85432:1     | $0, 0, 0, -e^{12}, e^{14}, e^{15}, e^{16}, e^{26} + e^{45}$                                               | 34568    |
| 85432:2     | $0, 0, 0, -e^{12}, e^{14}, e^{15}, e^{16}, e^{13} + e^{26} + e^{45}$                                      | 24568    |
| 85432:3     | $0, 0, 0, -e^{12}, e^{14}, e^{15}, e^{16} + e^{23}, e^{26} + e^{45}$                                      | 24568    |
| 85432:4     | $0, 0, 0, -e^{12}, e^{14}, e^{15}, e^{24} + e^{16}, e^{26} + e^{45}$                                      | 34568    |
| 85432:5     | $0, 0, 0, -e^{12}, e^{14}, e^{15} + e^{23}, e^{34} + e^{16}, e^{26} + e^{45}$                             | 23568    |
| 85432:6a    | $0, 0, 0, -e^{12}, e^{14}, e^{15}, e^{16} + e^{23}, e^{13} + e^{26} + e^{45}$                             | 24568    |
| 85432:6b    | $0, 0, 0, -e^{12}, e^{14}, e^{15}, -e^{16} + e^{23}, e^{13} + e^{26} + e^{45}$                            | 24568    |
| 85432:7     | $0, 0, 0, -e^{12}, e^{14}, e^{15}, e^{24} + e^{16}, e^{13} + e^{26} + e^{45}$                             | 24568    |
| 85432:8     | $0, 0, 0, -e^{12}, e^{14}, e^{15} + e^{23}, e^{34} + e^{16}, e^{13} + e^{26} + e^{45}$                    | 23568    |
| 85432:9     | $0, 0, 0, -e^{12}, e^{14}, e^{24} + e^{15}, e^{25} + e^{16}, e^{26} + e^{45}$                             | 34568    |
| 85432:10    | $0, 0, 0, -e^{12}, e^{14}, e^{24} + e^{15}, e^{25} + e^{16}, e^{13} + e^{26} + e^{45}$                    | 24568    |
| Type: 31211 |                                                                                                           |          |

Table 1 – Continued to next page

Table 1 – Continued from previous page

| Name        | g                                                                                                                             | UCS Dim. |
|-------------|-------------------------------------------------------------------------------------------------------------------------------|----------|
| 85421:1     | $0, 0, 0, e^{12}, e^{14}, e^{24}, e^{15}, e^{17}$                                                                             | 34568    |
| 85421:2     | $0, 0, 0, e^{12}, e^{14}, e^{24} + e^{13}, e^{15}, e^{17}$                                                                    | 24568    |
| 85421:3     | $0, 0, 0, e^{12}, e^{14}, e^{24}, e^{15}, e^{17} + e^{23}$                                                                    | 24568    |
| 85421:4a    | $0, 0, 0, e^{12}, e^{14}, e^{24} + e^{13}, e^{15}, e^{17} + e^{23}$                                                           | 24568    |
| 85421:4b    | $0, 0, 0, e^{12}, -e^{14}, e^{24} + e^{13}, e^{15}, e^{17} + e^{23}$                                                          | 24568    |
| 85421:5     | $0, 0, 0, e^{12}, e^{14}, e^{24}, e^{15}, e^{26} + e^{17}$                                                                    | 24568    |
| 85421:6     | $0, 0, 0, -e^{12}, e^{14}, e^{24}, e^{15}, e^{27} + e^{45}$                                                                   | 34568    |
| 85421:7     | $0, 0, 0, -e^{12}, e^{14}, e^{24}, e^{15} + e^{23}, e^{34} + e^{17}$                                                          | 23568    |
| 85421:8     | $0, 0, 0, -e^{12}, e^{14}, e^{24} + e^{13}, e^{15}, e^{27} + e^{45}$                                                          | 24568    |
| 85421:9     | $0, 0, 0, -e^{12}, e^{14}, e^{24} + e^{13}, e^{15} + e^{23}, e^{34} + e^{17}$                                                 | 23568    |
| 85421:10    | $0, 0, 0, -e^{12}, e^{14}, e^{24}, e^{15} + e^{23}, e^{27} + e^{45}$                                                          | 23568    |
| 85421:11    | $0, 0, 0, -e^{12}, e^{14}, e^{24}, e^{15}, e^{13} + e^{27} + e^{45}$                                                          | 24568    |
| 85421:12    | $0, 0, 0, -e^{12}, e^{14}, e^{24} + e^{13}, e^{15} + e^{23}, e^{27} + e^{45}$                                                 | 23568    |
| 85421:13    | $0, 0, 0, e^{12}, e^{14}, e^{24} + e^{13}, e^{15} + e^{23}, e^{26} + e^{17}$                                                  | 13568    |
| 85421:14    | $0, 0, 0, -e^{12}, e^{14}, e^{24}, e^{15} + e^{23}, e^{13} + e^{27} + e^{45}$                                                 | 23568    |
| 85421:15    | $0, 0, 0, e^{12}, e^{14}, e^{24} + e^{13}, e^{15}, e^{26} + e^{34} + e^{17}$                                                  | 13568    |
| 85421:16    | $0, 0, 0, -e^{12}, e^{14}, e^{24}, e^{15} + e^{23}, e^{26} + e^{34} + e^{17}$                                                 | 13568    |
| 85421:17    | $0, 0, 0, (-1 + a_2)e^{12}, e^{14}, e^{24} + a_2e^{13}, e^{15} + e^{23}, e^{26} + e^{34} + e^{17}$                            | 13568    |
| 85421:18    | $0, 0, 0, e^{12}, e^{24} + e^{13}, e^{14}, e^{25} + e^{34}, e^{27} + e^{35}$                                                  | 23468    |
| 85421:19a   | $0, 0, 0, -e^{12}, e^{14} + e^{23}, e^{24} + e^{13}, e^{34} + e^{15}, e^{35} + e^{17}$                                        | 23468    |
| 85421:19b   | $0, 0, 0, -e^{12}, e^{14} + e^{23}, e^{24} - e^{13}, e^{34} + e^{15}, e^{35} + e^{17}$                                        | 23468    |
| 85421:23    | $0, 0, 0, e^{12}, e^{24} + e^{13}, e^{14}, e^{25} + e^{34}, e^{27} + e^{35} + e^{16}$                                         | 13468    |
| 85421:24    | $0, 0, 0, e^{12}, e^{24} + e^{13}, 2e^{14}, e^{25} + e^{34}, e^{45} + e^{36} + e^{17}$                                        | 13468    |
| 85421:25a   | $0, 0, 0, -e^{12}, e^{14} + e^{23}, 2e^{24} + e^{13}, e^{34} + e^{15}, e^{36} + e^{27} + e^{45}$                              | 13468    |
| 85421:25b   | $0, 0, 0, -e^{12}, -e^{14} + e^{23}, 2e^{24} + e^{13}, e^{34} + e^{15}, e^{36} + e^{27} + e^{45}$                             | 13468    |
| 85421:26    | $0, 0, 0, e^{12}, e^{14}, e^{24}, e^{25} + e^{16}, e^{45} + e^{17}$                                                           | 23568    |
| 85421:27a   | $0, 0, 0, -e^{12}, e^{14}, e^{24}, e^{26} + e^{15}, e^{27} + e^{45}$                                                          | 23568    |
| 85421:27b   | $0, 0, 0, -e^{12}, -e^{14}, e^{24}, e^{26} + e^{15}, e^{27} + e^{45}$                                                         | 23568    |
| 85421:28a   | $0, 0, 0, -e^{12}, e^{14}, e^{24}, e^{26} + e^{15}, e^{13} + e^{27} + e^{45}$                                                 | 13568    |
| 85421:28b   | $0, 0, 0, -e^{12}, -e^{14}, e^{24}, e^{26} + e^{15}, e^{13} + e^{27} + e^{45}$                                                | 13568    |
| 85421:29    | $0, 0, 0, e^{12}, e^{14}, e^{24}, e^{25} + e^{16}, e^{45} + e^{17} + e^{23}$                                                  | 13568    |
| 85421:30    | $0, 0, 0, -e^{12}, e^{14}, e^{24}, e^{25} + e^{16}, e^{27} + e^{15} + e^{46}$                                                 | 23568    |
| 85421:31    | $0, 0, 0, e^{12}, e^{14}, e^{24} + e^{13}, e^{25} + e^{16}, e^{45} + e^{17}$                                                  | 12468    |
| 85421:33    | $0, 0, 0, e^{12}, e^{14}, e^{24} + e^{13}, e^{25} + e^{16}, e^{45} + e^{17} + e^{23}$                                         | 12468    |
| 85421:34    | $0, 0, 0, -e^{12}, e^{14}, e^{24} + e^{13}, e^{25} + e^{16}, e^{27} + e^{35} + e^{46}$                                        | 12468    |
| 85421:35a   | $0, 0, 0, e^{12}, e^{24} - e^{13}, e^{14} + e^{23}, e^{25} + e^{34} - 2e^{16}, e^{45} + e^{17}$                               | 12468    |
| 85421:35b   | $0, 0, 0, e^{12}, e^{24} - e^{13}, -e^{14} + e^{23}, e^{25} + e^{34} - 2e^{16}, e^{45} + e^{17}$                              | 12468    |
| 85421:37a   | $0, 0, 0, e^{12}, e^{14} + e^{23}, e^{24} + e^{13}, e^{26} + e^{15}, e^{46} + e^{35} + e^{17}$                                | 12468    |
| 85421:37b   | $0, 0, 0, e^{12}, -e^{14} - e^{23}, e^{24} - e^{13}, e^{26} + e^{15}, e^{46} + e^{35} + e^{17}$                               | 12468    |
| 85421:38a   | $0, 0, 0, e^{12}, e^{24} + e^{13}, e^{14} + e^{23}, e^{26} + e^{15}, e^{46} + e^{35} + e^{17}$                                | 12468    |
| 85421:38b   | $0, 0, 0, e^{12}, e^{24} - e^{13}, e^{14} + e^{23}, e^{26} + e^{15}, e^{46} + e^{35} + e^{17}$                                | 12468    |
| 85421:39a   | $0, 0, 0, e^{12}, 2e^{14}, e^{24} + e^{13}, e^{26} + e^{34} + e^{15}, e^{46} + e^{35} + e^{17}$                               | 12468    |
| 85421:39b   | $0, 0, 0, e^{12}, 2e^{14}, e^{24} + e^{13}, e^{26} + e^{34} - e^{15}, e^{46} + e^{35} + e^{17}$                               | 12468    |
| 85421:40a   | $0, 0, 0, -e^{12}, e^{14}, e^{24} - e^{13}, e^{26} + e^{34} + e^{15}, e^{36} + e^{27} + e^{45}$                               | 12468    |
| 85421:40b   | $0, 0, 0, -e^{12}, -e^{14}, e^{24} - e^{13}, e^{26} + e^{34} + e^{15}, e^{36} + e^{27} + e^{45}$                              | 12468    |
| 85421:41a   | $0, 0, 0, e^{12}, e^{14}(1 + a_3) + (-1 + a_3)e^{23}, e^{13}a_3 + e^{24}, e^{26} + e^{34} + e^{15}, e^{46} + e^{35} + e^{17}$ | 12468    |
| 85421:41b   | $0, 0, 0, e^{12}, e^{14}(1 + a_3) - (-1 + a_3)e^{23}, e^{13}a_3 + e^{24}, e^{26} + e^{34} - e^{15}, e^{46} + e^{35} + e^{17}$ | 12468    |
| Type: 32111 |                                                                                                                               |          |
| 85321:1     | $0, 0, 0, e^{12}, e^{13}, e^{14}, e^{16}, e^{17}$                                                                             | 24568    |
| 85321:2     | $0, 0, 0, e^{12}, e^{13}, e^{24}, e^{26}, e^{27}$                                                                             | 24568    |
| 85321:3     | $0, 0, 0, e^{12}, e^{13}, e^{14}, e^{16}, e^{35} + e^{17}$                                                                    | 13568    |
| 85321:4a    | $0, 0, 0, e^{12}, e^{13}, e^{24}, e^{26}, e^{27} + e^{35}$                                                                    | 13568    |
| 85321:4b    | $0, 0, 0, -e^{12}, e^{13}, e^{24}, e^{26}, e^{27} + e^{35}$                                                                   | 13568    |
| 85321:5     | $0, 0, 0, e^{12}, e^{13}, e^{14}, e^{16}, e^{17} + e^{23}$                                                                    | 24568    |
| 85321:6     | $0, 0, 0, e^{12}, e^{13}, e^{24}, e^{26}, e^{27} + e^{15}$                                                                    | 13568    |
| 85321:7     | $0, 0, 0, e^{12}, e^{13}, e^{14}, e^{16}, e^{24} + e^{17}$                                                                    | 24568    |
| 85321:8     | $0, 0, 0, e^{12}, e^{13}, e^{24}, e^{26}, e^{27} + e^{14}$                                                                    | 24568    |
| 85321:9     | $0, 0, 0, -e^{12}, e^{13}, e^{14}, e^{16}, e^{46} + e^{27}$                                                                   | 24568    |

Table 1 – Continued to next page

Table 1 – Continued from previous page

| Name       | g                                                                                                                       | UCS Dim. |
|------------|-------------------------------------------------------------------------------------------------------------------------|----------|
| 85321:10   | $0, 0, 0, e^{12}, e^{13}, e^{24}, e^{26}, e^{17} + e^{46}$                                                              | 24568    |
| 85321:11   | $0, 0, 0, -e^{12}, e^{13}, e^{14}, e^{16} + e^{23}, e^{34} + e^{17}$                                                    | 23568    |
| 85321:12   | $0, 0, 0, e^{12}, e^{13}, e^{14}, e^{16} + e^{23}, e^{25} + e^{17}$                                                     | 13568    |
| 85321:13a  | $0, 0, 0, e^{12}, e^{13}, e^{14}, e^{16}, e^{24} + e^{35} + e^{17}$                                                     | 13568    |
| 85321:13b  | $0, 0, 0, -e^{12}, e^{13}, e^{14}, e^{16}, e^{24} + e^{35} + e^{17}$                                                    | 13568    |
| 85321:14   | $0, 0, 0, e^{12}, e^{13}, e^{14}, e^{16}, e^{25} + e^{34} + e^{17}$                                                     | 13568    |
| 85321:15a  | $0, 0, 0, e^{12}, e^{13}, e^{24}, e^{26}, e^{27} + e^{35} + e^{14}$                                                     | 13568    |
| 85321:15b  | $0, 0, 0, -e^{12}, e^{13}, e^{24}, e^{26}, e^{27} + e^{35} + e^{14}$                                                    | 13568    |
| 85321:16   | $0, 0, 0, -e^{12}, e^{13}, e^{14}, e^{16} + e^{23}, e^{46} + e^{27}$                                                    | 23568    |
| 85321:17a  | $0, 0, 0, -e^{12}, e^{13}, e^{14}, e^{16}, e^{46} + e^{27} + e^{35}$                                                    | 13568    |
| 85321:17b  | $0, 0, 0, -e^{12}, -e^{13}, e^{14}, e^{16}, e^{46} + e^{27} + e^{35}$                                                   | 13568    |
| 85321:18   | $0, 0, 0, e^{12}, e^{13}, e^{24}, e^{26}, e^{35} + e^{17} + e^{46}$                                                     | 13568    |
| 85321:19   | $0, 0, 0, e^{12}, e^{13}, e^{24}, e^{26}, e^{17} + e^{23} + e^{46}$                                                     | 24568    |
| 85321:20   | $0, 0, 0, e^{12}, e^{13}, e^{14}, e^{24} + e^{16}, e^{26} + e^{17}$                                                     | 24568    |
| 85321:21   | $0, 0, 0, e^{12}, e^{13}, e^{24}, e^{26} + e^{14}, e^{27} + e^{16}$                                                     | 24568    |
| 85321:22   | $0, 0, 0, (-1 + a_2)e^{12}, a_2e^{13}, e^{14}, e^{16} + e^{23}, e^{25} + e^{34} + e^{17}$                               | 13568    |
| 85321:23   | $0, 0, 0, -e^{12}, e^{13}, e^{14}, e^{16}, e^{46} + e^{27} + e^{15}$                                                    | 13568    |
| 85321:24   | $0, 0, 0, -e^{12}, e^{13}, e^{14}, e^{24} + e^{16}, e^{46} + e^{27}$                                                    | 24568    |
| 85321:25   | $0, 0, 0, e^{12}, e^{13}, e^{24}, e^{26} + e^{14}, e^{17} + e^{46}$                                                     | 24568    |
| 85321:26a  | $0, 0, 0, -e^{12}, e^{13}, e^{14}, e^{16} + e^{23}, e^{46} + e^{27} + e^{35}$                                           | 13568    |
| 85321:26b  | $0, 0, 0, -e^{12}, -e^{13}, e^{14}, e^{16} + e^{23}, e^{46} + e^{27} + e^{35}$                                          | 13568    |
| 85321:27a  | $0, 0, 0, -e^{12}, e^{13}, e^{14}, e^{16} + e^{23}, e^{46} + e^{27} + e^{15}$                                           | 13568    |
| 85321:27b  | $0, 0, 0, -e^{12}, -e^{13}, e^{14}, e^{16} + e^{23}, e^{46} + e^{27} + e^{15}$                                          | 13568    |
| 85321:28   | $0, 0, 0, e^{12}, e^{13}, e^{14}, e^{24} + e^{16}, e^{26} + e^{35} + e^{17}$                                            | 13568    |
| 85321:29a  | $0, 0, 0, e^{12}, e^{13}, e^{24}, e^{26} + e^{14}, e^{27} + e^{35} + e^{16}$                                            | 13568    |
| 85321:29b  | $0, 0, 0, -e^{12}, e^{13}, e^{24}, e^{26} + e^{14}, e^{27} + e^{35} + e^{16}$                                           | 13568    |
| 85321:30a  | $0, 0, 0, -e^{12}, e^{13}, e^{14}, e^{24} + e^{16}, e^{46} + e^{27} + e^{35}$                                           | 13568    |
| 85321:30b  | $0, 0, 0, -e^{12}, -e^{13}, e^{14}, e^{24} + e^{16}, e^{46} + e^{27} + e^{35}$                                          | 13568    |
| 85321:31   | $0, 0, 0, e^{12}, e^{13}, e^{24}, e^{26} + e^{14}, e^{35} + e^{17} + e^{46}$                                            | 13568    |
| 85321:32   | $0, 0, 0, e^{12}, e^{13}, e^{24}, e^{26} + e^{14}, e^{17} + e^{23} + e^{46}$                                            | 24568    |
| 85321:33   | $0, 0, 0, -e^{12}, e^{13}, e^{14} + e^{23}, e^{34} + e^{16}, e^{36} + e^{17}$                                           | 23468    |
| 85321:34   | $0, 0, 0, -e^{12}, e^{13}, e^{14}, e^{24} + e^{16}, e^{46} + e^{27} + e^{15}$                                           | 13568    |
| 85321:36   | $0, 0, 0, e^{12}, e^{13}, e^{24}, e^{26} + e^{15}, e^{17} + e^{46}$                                                     | 12468    |
| 85321:39   | $0, 0, 0, e^{12}, e^{13}, e^{24}, e^{26} + e^{15}, e^{35} + e^{17} + e^{46}$                                            | 12468    |
| 85321:40   | $0, 0, 0, -e^{12}, e^{13}, e^{14} + e^{23}, e^{34} + e^{16}, e^{24} + e^{36} + e^{17}$                                  | 23468    |
| 85321:42   | $0, 0, 0, e^{12}, -e^{13}, e^{14} + e^{23}, e^{25} + e^{34} - 2e^{16}, e^{17} + e^{45}$                                 | 12468    |
| 85321:43   | $0, 0, 0, e^{12}, e^{13}, e^{24}, e^{26} + e^{15}, e^{17} + e^{23} + e^{46}$                                            | 12468    |
| 85321:45   | $0, 0, 0, e^{12}, e^{13}, e^{14} + e^{23}, e^{25} + e^{16}, e^{36} + e^{17} + e^{45}$                                   | 12468    |
| 85321:46   | $0, 0, 0, e^{12}, e^{13}, 2e^{14}, e^{25} + e^{34} + e^{16}, e^{36} + e^{17} + e^{45}$                                  | 12468    |
| 85321:47   | $0, 0, 0, -e^{12}, -2e^{13}, e^{14} - e^{23}, e^{25} + e^{34} + e^{16}, e^{46} + e^{27}$                                | 12468    |
| 85321:48   | $0, 0, 0, e^{12}, (-1 + a_3)e^{13}, e^{23} + e^{14}, a_3, (-2 + a_3)e^{16} + e^{25} + e^{34}, e^{36} + e^{17} + e^{45}$ | 12468    |
| 85321:49a  | $0, 0, 0, -e^{12}, -2e^{13}, e^{14} - e^{23}, e^{25} + e^{34} + e^{16}, e^{46} + e^{27} + e^{35}$                       | 12468    |
| 85321:49b  | $0, 0, 0, -e^{12}, -2e^{13}, -e^{14} - e^{23}, e^{25} + e^{34} + e^{16}, e^{46} + e^{27} + e^{35}$                      | 12468    |
| 85321:50   | $0, 0, 0, -e^{12}, -2e^{13}, e^{14} - e^{23}, e^{25} + e^{34} + e^{16}, e^{46} + e^{27} + e^{15}$                       | 12468    |
| Type: 2123 |                                                                                                                         |          |
| 8653:1     | $0, 0, e^{12}, e^{13}, e^{23}, e^{14}, e^{25}, e^{24} + e^{15}$                                                         | 3568     |
| Type: 3122 |                                                                                                                         |          |
| 8542:1     | $0, 0, 0, e^{12}, e^{14}, e^{24}, e^{15}, e^{26}$                                                                       | 3568     |
| 8542:2     | $0, 0, 0, e^{12}, e^{14}, e^{24}, e^{15}, e^{13} + e^{26}$                                                              | 2568     |
| 8542:3     | $0, 0, 0, e^{12}, e^{14}, e^{24}, e^{15}, e^{25} + e^{16}$                                                              | 3568     |
| 8542:4     | $0, 0, 0, e^{12}, e^{14}, e^{24}, e^{15} + e^{23}, e^{13} + e^{26}$                                                     | 2568     |
| 8542:5     | $0, 0, 0, e^{12}, e^{14}, e^{24}, e^{15} + e^{23}, e^{25} + e^{16}$                                                     | 2568     |
| 8542:6     | $0, 0, 0, e^{12}, e^{14}, e^{24} + e^{13}, e^{15}, e^{26} + e^{34}$                                                     | 2468     |
| 8542:7a    | $0, 0, 0, e^{12}, e^{14}, e^{24}, e^{25} + e^{16}, e^{26} + e^{15}$                                                     | 3568     |
| 8542:7b    | $0, 0, 0, e^{12}, -e^{14}, e^{24}, e^{25} - e^{16}, e^{26} + e^{15}$                                                    | 3568     |
| 8542:8     | $0, 0, 0, e^{12}, e^{14}, e^{24} + e^{13}, e^{15}, e^{25} + e^{16}$                                                     | 2468     |
| 8542:9     | $0, 0, 0, e^{12}, e^{14}, e^{24} + e^{13}, e^{15} + e^{23}, e^{26} + e^{34}$                                            | 2468     |
| 8542:10    | $0, 0, 0, e^{12}, e^{14}, e^{24} + e^{13}, e^{15} + e^{23}, e^{25} + e^{16}$                                            | 2468     |

Table 1 – Continued to next page

Table 1 – Continued from previous page

| Name       | g                                                                                                            | UCS Dim. |
|------------|--------------------------------------------------------------------------------------------------------------|----------|
| 8542:11    | $0, 0, 0, e^{12}, e^{24} + e^{13}, e^{14}, e^{25} + e^{34}, e^{26} + e^{15}$                                 | 2468     |
| 8542:12a   | $0, 0, 0, -e^{12}, e^{14} + e^{23}, e^{24} + e^{13}, e^{34} + e^{15}, e^{25} + e^{16}$                       | 2468     |
| 8542:12b   | $0, 0, 0, -e^{12}, e^{14} + e^{23}, e^{24} - e^{13}, e^{34} + e^{15}, e^{25} + e^{16}$                       | 2468     |
| 8542:13a   | $0, 0, 0, e^{12}, e^{14} + e^{23}, e^{24} + e^{13}, e^{25} + e^{16}, e^{26} + e^{15}$                        | 2468     |
| 8542:13b   | $0, 0, 0, e^{12}, -e^{14} + e^{23}, e^{24} + e^{13}, e^{25} - e^{16}, e^{26} + e^{15}$                       | 2468     |
| 8542:14a   | $0, 0, 0, e^{12}, e^{14}, e^{24} + e^{13}, e^{25} + e^{16}, e^{26} + e^{34} + e^{15}$                        | 2468     |
| 8542:14b   | $0, 0, 0, e^{12}, -e^{14}, e^{24} + e^{13}, e^{25} - e^{16}, e^{26} + e^{34} + e^{15}$                       | 2468     |
| 8542:15a   | $0, 0, 0, (-1 + a_2)e^{12}, e^{13}a_2 + e^{24}, e^{14} + e^{23}, e^{26} + e^{15}, e^{25} + e^{34} + e^{16}$  | 2468     |
| 8542:15b   | $0, 0, 0, (-1 + a_2)e^{12}, e^{13}a_2 + e^{24}, -e^{14} + e^{23}, e^{26} - e^{15}, e^{25} + e^{34} + e^{16}$ | 2468     |
| Type: 3221 |                                                                                                              |          |
| 8531:1     | $0, 0, 0, e^{12}, e^{13}, e^{14}, e^{24}, e^{16}$                                                            | 3568     |
| 8531:2     | $0, 0, 0, e^{12}, e^{13}, e^{24}, e^{14}, e^{26}$                                                            | 3568     |
| 8531:3     | $0, 0, 0, e^{12}, e^{13}, e^{14}, e^{35}, e^{16}$                                                            | 2468     |
| 8531:4     | $0, 0, 0, e^{12}, e^{13}, e^{24}, e^{35}, e^{26}$                                                            | 2468     |
| 8531:5     | $0, 0, 0, e^{12}, e^{13}, e^{24}, e^{14} + e^{23}, e^{26}$                                                   | 3568     |
| 8531:6     | $0, 0, 0, e^{12}, e^{13}, e^{14}, e^{15}, e^{16}$                                                            | 2468     |
| 8531:7     | $0, 0, 0, e^{12}, e^{13}, e^{24}, e^{15}, e^{26}$                                                            | 2468     |
| 8531:8     | $0, 0, 0, e^{12}, e^{13}, e^{14}, e^{24}, e^{16} + e^{23}$                                                   | 3568     |
| 8531:9     | $0, 0, 0, e^{12}, e^{13}, e^{14}, e^{15} + e^{23}, e^{16}$                                                   | 2468     |
| 8531:10    | $0, 0, 0, e^{12}, e^{13}, e^{24}, e^{15} + e^{23}, e^{26}$                                                   | 2468     |
| 8531:11    | $0, 0, 0, e^{12}, e^{13}, e^{14}, e^{35}, e^{16} + e^{23}$                                                   | 2468     |
| 8531:12a   | $0, 0, 0, e^{12}, e^{13}, e^{14}, e^{24} + e^{35}, e^{16}$                                                   | 2468     |
| 8531:12b   | $0, 0, 0, -e^{12}, e^{13}, e^{14}, e^{24} + e^{35}, e^{16}$                                                  | 2468     |
| 8531:13    | $0, 0, 0, e^{12}, e^{13}, e^{14}, e^{25} + e^{34}, e^{16}$                                                   | 2468     |
| 8531:14    | $0, 0, 0, e^{12}, e^{13}, e^{24}, e^{35} + e^{14}, e^{26}$                                                   | 2468     |
| 8531:15    | $0, 0, 0, e^{12}, e^{13}, e^{24}, e^{25} + e^{34}, e^{26}$                                                   | 2468     |
| 8531:16    | $0, 0, 0, e^{12}, e^{13}, e^{14}, e^{15}, e^{35} + e^{16}$                                                   | 2468     |
| 8531:17    | $0, 0, 0, e^{12}, e^{13}, e^{24}, e^{15}, e^{26} + e^{35}$                                                   | 2468     |
| 8531:18    | $0, 0, 0, e^{12}, e^{13}, e^{24}, e^{35}, e^{26} + e^{15}$                                                   | 2468     |
| 8531:19    | $0, 0, 0, e^{12}, e^{13}, e^{14}, e^{15}, e^{16} + e^{23}$                                                   | 2468     |
| 8531:20    | $0, 0, 0, e^{12}, e^{13}, e^{14}, e^{24} + e^{15}, e^{16}$                                                   | 2468     |
| 8531:21    | $0, 0, 0, e^{12}, e^{13}, e^{14}, e^{24}, e^{35} + e^{16}$                                                   | 2468     |
| 8531:22    | $0, 0, 0, e^{12}, e^{13}, e^{24}, e^{14}, e^{26} + e^{35}$                                                   | 2468     |
| 8531:23    | $0, 0, 0, e^{12}, e^{13}, e^{14}, e^{35}, e^{24} + e^{16}$                                                   | 2468     |
| 8531:24    | $0, 0, 0, e^{12}, e^{13}, e^{24}, e^{35}, e^{26} + e^{14}$                                                   | 2468     |
| 8531:25a   | $0, 0, 0, e^{12}, e^{13}, e^{14}, e^{15} + e^{23}, e^{35} + e^{16}$                                          | 2468     |
| 8531:25b   | $0, 0, 0, -e^{12}, e^{13}, e^{14}, e^{15} + e^{23}, e^{35} + e^{16}$                                         | 2468     |
| 8531:26a   | $0, 0, 0, e^{12}, e^{13}, e^{24}, e^{15} + e^{23}, e^{26} + e^{35}$                                          | 2468     |
| 8531:26b   | $0, 0, 0, -e^{12}, e^{13}, e^{24}, e^{15} + e^{23}, e^{26} + e^{35}$                                         | 2468     |
| 8531:27    | $0, 0, 0, e^{12}, e^{13}, e^{14} + e^{23}, e^{35}, e^{25} + e^{16}$                                          | 2468     |
| 8531:28    | $0, 0, 0, e^{12}, e^{13}, e^{14}, e^{25} + e^{34}, e^{35} + e^{16}$                                          | 2468     |
| 8531:29    | $0, 0, 0, e^{12}, e^{13}, e^{24}, e^{25} + e^{34}, e^{26} + e^{35}$                                          | 2468     |
| 8531:30    | $0, 0, 0, -e^{12}, e^{13}, e^{14} + e^{23}, e^{35}, e^{34} + e^{16}$                                         | 2468     |
| 8531:31    | $0, 0, 0, e^{12}, e^{13}, e^{24}, e^{14}, e^{26} + e^{15}$                                                   | 2468     |
| 8531:32    | $0, 0, 0, e^{12}, e^{13}, e^{14}, e^{15}, e^{24} + e^{16}$                                                   | 2468     |
| 8531:33    | $0, 0, 0, e^{12}, e^{13}, e^{24}, e^{15}, e^{26} + e^{14}$                                                   | 2468     |
| 8531:34a   | $0, 0, 0, e^{12}, e^{13}, e^{14}, e^{24} + e^{35}, e^{16} + e^{23}$                                          | 2468     |
| 8531:34b   | $0, 0, 0, -e^{12}, e^{13}, e^{14}, e^{24} + e^{35}, e^{16} + e^{23}$                                         | 2468     |
| 8531:35    | $0, 0, 0, e^{12}, e^{13}, e^{14}, e^{25} + e^{34}, e^{16} + e^{23}$                                          | 2468     |
| 8531:36    | $0, 0, 0, e^{12}, e^{13}, e^{24}, e^{14} + e^{23}, e^{26} + e^{35}$                                          | 2468     |
| 8531:37    | $0, 0, 0, e^{12}, e^{13}, e^{14} + e^{23}, e^{15}, e^{25} + e^{16}$                                          | 2468     |
| 8531:38    | $0, 0, 0, e^{12}, e^{13}, e^{14}, e^{24} + e^{15}, e^{35} + e^{16}$                                          | 2468     |
| 8531:39    | $0, 0, 0, e^{12}, e^{13}, e^{24}, e^{35} + e^{14}, e^{26} + e^{15}$                                          | 2468     |
| 8531:40    | $0, 0, 0, e^{12}, e^{13}, e^{24}, e^{25} + e^{34}, e^{26} + e^{15}$                                          | 2468     |
| 8531:41    | $0, 0, 0, -e^{12}, e^{13}, e^{14} + e^{23}, e^{24}, e^{34} + e^{16}$                                         | 3468     |
| 8531:42    | $0, 0, 0, -e^{12}, e^{13}, e^{14} + e^{23}, e^{15}, e^{34} + e^{16}$                                         | 2468     |
| 8531:43    | $0, 0, 0, e^{12}, e^{13}, e^{14}, e^{35}, e^{25} + e^{34} + e^{16}$                                          | 2468     |
| 8531:44a   | $0, 0, 0, e^{12}, e^{13}, e^{14}, e^{24} + e^{15}, e^{16} + e^{23}$                                          | 2468     |

Table 1 – Continued to next page

Table 1 – Continued from previous page

| Name     | g                                                                                                    | UCS Dim. |
|----------|------------------------------------------------------------------------------------------------------|----------|
| 8531:44b | $0, 0, 0, e^{12}, -e^{13}, e^{14}, e^{24} + e^{15}, e^{16} + e^{23}$                                 | 2468     |
| 8531:45  | $0, 0, 0, e^{12}, e^{13}, e^{24}, e^{14} + e^{23}, e^{26} + e^{15}$                                  | 2468     |
| 8531:46  | $0, 0, 0, e^{12}, a_1 e^{13}, e^{14}, e^{15} + e^{23}, e^{24} + e^{16}$                              | 2468     |
| 8531:47  | $0, 0, 0, e^{12}, e^{13}, e^{24}, e^{15} + e^{23}, e^{26} + e^{14}$                                  | 2468     |
| 8531:48  | $0, 0, 0, e^{12}, e^{13}, e^{14} + e^{23}, e^{24}, e^{25} + e^{16}$                                  | 2468     |
| 8531:49a | $0, 0, 0, e^{12}, e^{13}, e^{14}, e^{15}, e^{24} + e^{35} + e^{16}$                                  | 2468     |
| 8531:49b | $0, 0, 0, -e^{12}, e^{13}, e^{14}, e^{15}, e^{24} + e^{35} + e^{16}$                                 | 2468     |
| 8531:50  | $0, 0, 0, e^{12}, e^{13}, e^{14}, e^{15}, e^{25} + e^{34} + e^{16}$                                  | 2468     |
| 8531:51  | $0, 0, 0, e^{12}, e^{13}, e^{24}, e^{15}, e^{26} + e^{35} + e^{14}$                                  | 2468     |
| 8531:52  | $0, 0, 0, e^{12}, e^{13}, e^{14}, e^{25} + e^{34}, e^{24} + e^{16}$                                  | 2468     |
| 8531:53  | $0, 0, 0, e^{12}, e^{13}, e^{24}, e^{25} + e^{34}, e^{26} + e^{14}$                                  | 2468     |
| 8531:54a | $0, 0, 0, e^{12}, e^{13}, e^{14} + e^{23}, e^{24} + e^{35}, e^{25} + e^{16}$                         | 2468     |
| 8531:54b | $0, 0, 0, -e^{12}, e^{13}, e^{14} + e^{23}, e^{24} + e^{35}, e^{25} + e^{16}$                        | 2468     |
| 8531:55  | $0, 0, 0, e^{12}(-1 + a_2), a_2 e^{13}, e^{14} + e^{23}, e^{35}, e^{25} + e^{34} + e^{16}$           | 2468     |
| 8531:56a | $0, 0, 0, -e^{12}, e^{13}, e^{14} + e^{23}, e^{24} + e^{35}, e^{34} + e^{16}$                        | 2468     |
| 8531:56b | $0, 0, 0, -e^{12}, -e^{13}, e^{14} + e^{23}, e^{24} + e^{35}, e^{34} + e^{16}$                       | 2468     |
| 8531:57  | $0, 0, 0, e^{12}, e^{13}, e^{14}, e^{24}, e^{25} + e^{34} + e^{16}$                                  | 2468     |
| 8531:58a | $0, 0, 0, e^{12}, e^{13} a_1, e^{14}, e^{15} + e^{23}, e^{24} + e^{35} + e^{16}$                     | 2468     |
| 8531:58b | $0, 0, 0, -e^{12}, e^{13} a_1, e^{14}, e^{15} + e^{23}, e^{24} + e^{35} + e^{16}$                    | 2468     |
| 8531:59  | $0, 0, 0, e^{12}, e^{13}, e^{14}, e^{15} + e^{23}, e^{25} + e^{34} + e^{16}$                         | 2468     |
| 8531:60a | $0, 0, 0, e^{12}, e^{13}, e^{24}, e^{15} + e^{23}, e^{26} + e^{35} + e^{14}$                         | 2468     |
| 8531:60b | $0, 0, 0, -e^{12}, e^{13}, e^{24}, e^{15} + e^{23}, e^{26} + e^{35} + e^{14}$                        | 2468     |
| 8531:61  | $0, 0, 0, e^{12}, e^{13}, e^{14} + e^{23}, e^{24} + e^{15}, e^{25} + e^{16}$                         | 2468     |
| 8531:62  | $0, 0, 0, e^{12} a_1, e^{13}(1 + a_1), e^{14} + e^{23}, e^{15}, e^{25} + e^{34} + e^{16}$            | 2468     |
| 8531:63  | $0, 0, 0, -e^{12}, e^{13}, e^{14} + e^{23}, e^{24} + e^{15}, e^{34} + e^{16}$                        | 2468     |
| 8531:64a | $0, 0, 0, e^{12}, e^{13}, e^{14}, e^{24} + e^{35}, e^{25} + e^{34} + e^{16}$                         | 2468     |
| 8531:64b | $0, 0, 0, e^{12}, e^{13}, e^{14}, -e^{24} + e^{35}, e^{25} + e^{34} + e^{16}$                        | 2468     |
| 8531:65a | $0, 0, 0, e^{12}, e^{13}, e^{14}, e^{25} + e^{34}, e^{24} + e^{35} + e^{16}$                         | 2468     |
| 8531:65b | $0, 0, 0, -e^{12}, e^{13}, e^{14}, -e^{25} + e^{34}, e^{24} + e^{35} + e^{16}$                       | 2468     |
| 8531:66  | $0, 0, 0, e^{12}, e^{13}, e^{24}, e^{25} + e^{34}, e^{26} + e^{35} + e^{14}$                         | 2468     |
| 8531:67  | $0, 0, 0, e^{12}, e^{13}, e^{14}, e^{24} + e^{15}, e^{25} + e^{34} + e^{16}$                         | 2468     |
| 8531:68  | $0, 0, 0, e^{12} a_1, e^{13}(1 + a_1), e^{14} + e^{23}, e^{24}, e^{25} + e^{34} + e^{16}$            | 2468     |
| 8531:69a | $0, 0, 0, e^{12} a_1, (1 + a_1) e^{13}, e^{14} + e^{23}, e^{24} + e^{35}, e^{25} + e^{34} + e^{16}$  | 2468     |
| 8531:69b | $0, 0, 0, e^{12} a_1, (1 + a_1) e^{13}, e^{14} + e^{23}, -e^{24} + e^{35}, e^{25} + e^{34} + e^{16}$ | 2468     |
| 8531:70  | $0, 0, 0, e^{12}(-1 + a_2), a_2 e^{13}, e^{14} + e^{23}, e^{24} + e^{15}, e^{25} + e^{34} + e^{16}$  | 2468     |
| 8531:71a | $0, 0, 0, e^{12}, e^{13}, e^{14}, e^{24}, e^{27} + e^{16}$                                           | 2568     |
| 8531:71b | $0, 0, 0, e^{12}, e^{13}, -e^{14}, e^{24}, e^{27} + e^{16}$                                          | 2568     |
| 8531:72  | $0, 0, 0, e^{12}, e^{13}, e^{14}, e^{24}, e^{26} + e^{17}$                                           | 2568     |
| 8531:73  | $0, 0, 0, e^{12}, e^{13}, e^{24}, e^{14} + e^{23}, e^{27} + e^{16}$                                  | 2468     |
| 8531:74a | $0, 0, 0, e^{12}, e^{13}, e^{14}, e^{24}, e^{27} + e^{35} + e^{16}$                                  | 1468     |
| 8531:74b | $0, 0, 0, e^{12}, e^{13}, -e^{14}, e^{24}, e^{27} + e^{35} + e^{16}$                                 | 1468     |
| 8531:75  | $0, 0, 0, e^{12}, e^{13}, e^{14}, e^{24}, e^{26} + e^{35} + e^{17}$                                  | 1468     |
| 8531:76a | $0, 0, 0, -e^{12}, e^{13}, e^{24}, e^{14} + e^{23}, e^{26} + e^{34} + e^{17}$                        | 2468     |
| 8531:76b | $0, 0, 0, -e^{12}, e^{13}, e^{24}, -e^{14} + e^{23}, e^{26} + e^{34} + e^{17}$                       | 2468     |
| 8531:77  | $0, 0, 0, e^{12}, e^{13}, e^{24}, e^{14} + e^{23}, e^{27} + e^{35} + e^{16}$                         | 1468     |
| 8531:87  | $0, 0, 0, e^{12}, e^{13}, e^{24}, e^{15}, e^{26} + e^{17}$                                           | 1358     |
| 8531:88  | $0, 0, 0, e^{12}, e^{13}, e^{24}, e^{35}, e^{37} + e^{26}$                                           | 1358     |
| 8531:89  | $0, 0, 0, e^{12}, e^{13}, e^{14}, e^{24} + e^{15}, e^{26} + e^{17}$                                  | 1358     |
| 8531:90  | $0, 0, 0, e^{12}, e^{13}, e^{24}, e^{25} + e^{34}, e^{36} + e^{27}$                                  | 1358     |
| 8531:91  | $0, 0, 0, e^{12}, e^{13}, e^{14}, e^{35}, e^{24} + e^{37} + e^{16}$                                  | 1358     |
| 8531:92  | $0, 0, 0, e^{12}, e^{13}, e^{24}, e^{35}, e^{37} + e^{26} + e^{14}$                                  | 1358     |
| 8531:93  | $0, 0, 0, -e^{12}, e^{13}, e^{14}, e^{15}, e^{36} + e^{27} + e^{45}$                                 | 1358     |
| 8531:94  | $0, 0, 0, e^{12}, e^{13}, e^{14} + e^{23}, e^{24} + e^{15}, e^{26} + e^{17}$                         | 1358     |
| 8531:95a | $0, 0, 0, e^{12}, e^{13}, e^{25} + e^{34}, e^{24} + e^{35}, e^{37} + e^{26}$                         | 1358     |
| 8531:95b | $0, 0, 0, -e^{12}, e^{13}, -e^{25} + e^{34}, e^{24} + e^{35}, e^{37} + e^{26}$                       | 1358     |
| 8531:96  | $0, 0, 0, -e^{12}, e^{13}, e^{24}, e^{15} + e^{23}, e^{26} + e^{34} + e^{17}$                        | 1358     |
| 8531:97  | $0, 0, 0, e^{12}, e^{13}, e^{24}, e^{25} + e^{34}, e^{36} + e^{27} + e^{14}$                         | 1358     |
| 8531:98  | $0, 0, 0, e^{12}, e^{13}, e^{14}, e^{24} + e^{15}, e^{26} + e^{35} + e^{17}$                         | 1358     |

Table 1 – Continued to next page

Table 1 – Continued from previous page

| Name       | g                                                                                         | UCS Dim. |
|------------|-------------------------------------------------------------------------------------------|----------|
| 8531:99    | $0, 0, 0, e^{12}, e^{13}, e^{24}, e^{25} + e^{34}, e^{36} + e^{27} + e^{15}$              | 1358     |
| 8531:100   | $0, 0, 0, -e^{12}, e^{13}, e^{14}, e^{15} + e^{23}, e^{45} + e^{36} + e^{27}$             | 1358     |
| 8531:101   | $0, 0, 0, -e^{12}, e^{13}, e^{14}, e^{24} + e^{15}, e^{45} + e^{36} + e^{27}$             | 1358     |
| 8531:103   | $0, 0, 0, e^{12}, e^{13}, 2e^{14}, e^{25} + e^{34}, e^{36} + e^{17} + e^{45}$             | 1358     |
| 8531:104   | $0, 0, 0, a_1 e^{12}, e^{13}, e^{14} + e^{23}, e^{24} + e^{15}, e^{26} + e^{35} + e^{17}$ | 1358     |
| 8531:105a  | $0, 0, 0, e^{12}, e^{13}, e^{25} + e^{34}, e^{24} + e^{35}, e^{37} + e^{26} + e^{14}$     | 1358     |
| 8531:105b  | $0, 0, 0, -e^{12}, e^{13}, -e^{25} + e^{34}, e^{24} + e^{35}, e^{37} + e^{26} + e^{14}$   | 1358     |
| 8531:106a  | $0, 0, 0, e^{12}, e^{13}, e^{25} + e^{34}, e^{24} + e^{35}, e^{36} + e^{27} + e^{14}$     | 1358     |
| 8531:106b  | $0, 0, 0, e^{12}, e^{13}, e^{25} + e^{34}, -e^{24} + e^{35}, e^{36} + e^{27} + e^{14}$    | 1358     |
| 8531:107   | $0, 0, 0, -e^{12}, e^{13}, e^{14} + e^{23}, e^{24} + e^{15}, e^{45} + e^{36} + e^{27}$    | 1358     |
| 8531:108   | $0, 0, 0, e^{12}, e^{13}, 2e^{14} + e^{23}, e^{25} + e^{34}, e^{36} + e^{17} + e^{45}$    | 1358     |
| 8531:109   | $0, 0, 0, -e^{12}, -e^{13}, e^{24} + 2e^{15}, e^{25} + e^{34}, e^{45} + e^{26} + e^{17}$  | 1358     |
| 8531:110   | $0, 0, 0, -e^{12}, e^{13}, e^{24} + e^{15}, e^{35} + e^{14}, e^{45} + e^{37} + e^{26}$    | 1358     |
| Type: 3311 |                                                                                           |          |
| 8521:1     | $0, 0, 0, e^{12}, e^{13}, e^{23}, e^{14}, e^{17}$                                         | 3568     |
| 8521:2     | $0, 0, 0, e^{12}, e^{13}, e^{23}, e^{14}, e^{24} + e^{17}$                                | 3568     |
| 8521:3     | $0, 0, 0, e^{12}, e^{13}, e^{23}, e^{14}, e^{35} + e^{17}$                                | 2468     |
| 8521:4     | $0, 0, 0, e^{12}, e^{13}, e^{23}, e^{24}, e^{27} + e^{35}$                                | 2468     |
| 8521:5     | $0, 0, 0, e^{12}, e^{13}, e^{23}, e^{24}, e^{27} + e^{15}$                                | 2468     |
| 8521:6a    | $0, 0, 0, e^{12}, e^{13}, e^{23}, e^{14}, e^{24} + e^{35} + e^{17}$                       | 2468     |
| 8521:6b    | $0, 0, 0, -e^{12}, e^{13}, e^{23}, e^{14}, e^{24} + e^{35} + e^{17}$                      | 2468     |
| 8521:7     | $0, 0, 0, e^{12}, e^{13}, e^{23}, e^{14}, e^{25} + e^{34} + e^{17}$                       | 2468     |
| 8521:8     | $0, 0, 0, e^{12}, e^{13}, e^{23}, e^{24}, e^{27} + e^{35} + e^{14}$                       | 2468     |
| 8521:9     | $0, 0, 0, e^{12}, e^{13}, e^{23}, e^{14}, e^{26} + e^{35} + e^{17}$                       | 1468     |
| 8521:12    | $0, 0, 0, e^{12}, -e^{13}, e^{23}, e^{25} + e^{34} - 2e^{16}, e^{17} + e^{45}$            | 1258     |
| 8521:13    | $0, 0, 0, -e^{12}, -2e^{13}, -e^{23}, e^{25} + e^{34} + e^{16}, e^{27} + e^{15} + e^{46}$ | 1258     |
| Type: 323  |                                                                                           |          |
| 853:1      | $0, 0, 0, e^{12}, e^{13}, e^{14}, e^{24}, e^{15}$                                         | 358      |
| 853:2      | $0, 0, 0, e^{12}, e^{13}, e^{14}, e^{24}, e^{35}$                                         | 358      |
| 853:3      | $0, 0, 0, e^{12}, e^{13}, e^{14}, e^{24}, e^{15} + e^{23}$                                | 358      |
| 853:4      | $0, 0, 0, e^{12}, e^{13}, e^{24}, e^{14} + e^{23}, e^{15}$                                | 358      |
| 853:5      | $0, 0, 0, e^{12}, e^{13}, e^{24}, e^{14} + e^{23}, e^{35}$                                | 358      |
| 853:6      | $0, 0, 0, e^{12}, e^{13}, e^{14}, e^{24}, e^{25} + e^{34}$                                | 358      |
| 853:7a     | $0, 0, 0, e^{12}, e^{13}, e^{14}, e^{15}, e^{24} + e^{35}$                                | 358      |
| 853:7b     | $0, 0, 0, -e^{12}, e^{13}, e^{14}, e^{15}, e^{24} + e^{35}$                               | 358      |
| 853:8      | $0, 0, 0, e^{12}, e^{13}, e^{14}, e^{15}, e^{25} + e^{34}$                                | 358      |
| 853:9      | $0, 0, 0, e^{12}, e^{13}, e^{24}, e^{15}, e^{35} + e^{14}$                                | 358      |
| 853:10     | $0, 0, 0, e^{12}, e^{13}, e^{24}, e^{15}, e^{25} + e^{34}$                                | 358      |
| 853:11     | $0, 0, 0, e^{12}, e^{13}, e^{24}, e^{35}, e^{25} + e^{34}$                                | 358      |
| 853:12     | $0, 0, 0, e^{12}, e^{13}, e^{24}, e^{14} + e^{23}, e^{25} + e^{34}$                       | 358      |
| 853:13a    | $0, 0, 0, e^{12}, e^{13}, e^{14}, e^{15} + e^{23}, e^{24} + e^{35}$                       | 358      |
| 853:13b    | $0, 0, 0, -e^{12}, e^{13}, e^{14}, e^{15} + e^{23}, e^{24} + e^{35}$                      | 358      |
| 853:14     | $0, 0, 0, e^{12}, e^{13}, e^{14}, e^{15} + e^{23}, e^{25} + e^{34}$                       | 358      |
| 853:15     | $0, 0, 0, e^{12}, e^{13}, e^{24}, e^{15} + e^{23}, e^{35} + e^{14}$                       | 358      |
| 853:16     | $0, 0, 0, e^{12}, e^{13}, e^{24}, e^{15} + e^{23}, e^{25} + e^{34}$                       | 358      |
| 853:17     | $0, 0, 0, e^{12}, e^{13}, e^{14}, e^{24} + e^{15}, e^{25} + e^{34}$                       | 358      |
| 853:18a    | $0, 0, 0, e^{12}, e^{13}, e^{14}, e^{25} + e^{34}, e^{24} + e^{35}$                       | 358      |
| 853:18b    | $0, 0, 0, -e^{12}, e^{13}, e^{14}, -e^{25} + e^{34}, e^{24} + e^{35}$                     | 358      |
| 853:19     | $0, 0, 0, e^{12}, e^{13}, e^{24}, e^{35} + e^{14}, e^{25} + e^{34}$                       | 358      |
| 853:20     | $0, 0, 0, e^{12}, e^{13}, e^{14} + e^{23}, e^{24} + e^{15}, e^{25} + e^{34}$              | 358      |
| 853:21a    | $0, 0, 0, e^{12}, e^{13}, e^{14} + e^{23}, e^{25} + e^{34}, e^{24} + e^{35}$              | 358      |
| 853:21b    | $0, 0, 0, -e^{12}, e^{13}, e^{14} + e^{23}, -e^{25} + e^{34}, e^{24} + e^{35}$            | 358      |
| 853:22     | $0, 0, 0, e^{12}, e^{13}, e^{24} + e^{15}, e^{35} + e^{14}, e^{25} + e^{34}$              | 358      |
| Type: 332  |                                                                                           |          |
| 852:1      | $0, 0, 0, e^{12}, e^{13}, e^{23}, e^{14}, e^{24}$                                         | 468      |
| 852:2      | $0, 0, 0, e^{12}, e^{13}, e^{23}, e^{14}, e^{15}$                                         | 358      |
| 852:3      | $0, 0, 0, e^{12}, e^{13}, e^{23}, e^{24}, e^{15}$                                         | 358      |
| 852:4      | $0, 0, 0, e^{12}, e^{13}, e^{23}, e^{24}, e^{35}$                                         | 358      |

Table 1 – Continued to next page

Table 1 – Continued from previous page

| Name        | g                                                                                                  | UCS Dim. |
|-------------|----------------------------------------------------------------------------------------------------|----------|
| 852:5       | $0, 0, 0, e^{12}, e^{13}, e^{23}, e^{14}, e^{24} + e^{15}$                                         | 358      |
| 852:6a      | $0, 0, 0, e^{12}, e^{13}, e^{23}, e^{14}, e^{24} + e^{35}$                                         | 358      |
| 852:6b      | $0, 0, 0, -e^{12}, e^{13}, e^{23}, e^{14}, e^{24} + e^{35}$                                        | 358      |
| 852:7       | $0, 0, 0, e^{12}, e^{13}, e^{23}, e^{14}, e^{25} + e^{34}$                                         | 358      |
| 852:8       | $0, 0, 0, e^{12}, e^{13}, e^{23}, e^{24}, e^{35} + e^{14}$                                         | 358      |
| 852:9       | $0, 0, 0, e^{12}, e^{13}, e^{23}, e^{24}, e^{25} + e^{34}$                                         | 358      |
| 852:10      | $0, 0, 0, e^{12}, e^{13}, e^{23}, e^{24} + e^{15}, e^{35} + e^{14}$                                | 358      |
| 852:11      | $0, 0, 0, e^{12}, e^{13}, e^{23}, e^{24} + e^{15}, e^{25} + e^{34}$                                | 358      |
| 852:12a     | $0, 0, 0, e^{12}, e^{13}, e^{23}, e^{25} + e^{34}, e^{24} + e^{35}$                                | 358      |
| 852:12b     | $0, 0, 0, -e^{12}, e^{13}, e^{23}, -e^{25} + e^{34}, e^{24} + e^{35}$                              | 358      |
| 852:13a     | $0, 0, 0, e^{12}, e^{13}, e^{23}, e^{14}, e^{26} + e^{15}$                                         | 258      |
| 852:13b     | $0, 0, 0, e^{12}, -e^{13}, e^{23}, e^{14}, e^{26} + e^{15}$                                        | 258      |
| 852:14      | $0, 0, 0, e^{12}, e^{13}, e^{23}, e^{14}, e^{25} + e^{16}$                                         | 258      |
| 852:15      | $0, 0, 0, e^{12}, e^{13}, e^{23}, e^{14}, e^{36} + e^{15}$                                         | 258      |
| 852:16      | $0, 0, 0, e^{12}, e^{13}, e^{23}, e^{14}, e^{26} + e^{35}$                                         | 258      |
| 852:17      | $0, 0, 0, e^{12}, e^{13}, e^{23}, e^{14}, e^{24} + e^{36} + e^{15}$                                | 258      |
| 852:18      | $0, 0, 0, (-1 + a_2)e^{12}, e^{13}, a_2e^{23}, e^{14}, e^{25} + e^{34} + e^{16}$                   | 258      |
| 852:19      | $0, 0, 0, e^{12}, e^{13}, e^{23}, e^{24} + e^{15}, e^{26} + e^{14}$                                | 258      |
| 852:20a     | $0, 0, 0, e^{12}, e^{13}, e^{23}, e^{24} + e^{15}, e^{36} + e^{14}$                                | 258      |
| 852:20b     | $0, 0, 0, -e^{12}, e^{13}, e^{23}, e^{24} + e^{15}, e^{36} + e^{14}$                               | 258      |
| 852:21      | $0, 0, 0, -e^{12}, e^{13}, e^{23}, e^{24} + e^{15}, e^{34} + e^{16}$                               | 258      |
| 852:22      | $0, 0, 0, -e^{12}, e^{13}, e^{23}, e^{35} + e^{14}, e^{34} + e^{16}$                               | 258      |
| 852:23      | $0, 0, 0, e^{12}, a_1e^{13}, e^{23}, e^{35} + e^{14}, e^{24} + e^{36}$                             | 258      |
| 852:24a     | $0, 0, 0, e^{12}, e^{13}, e^{23}, e^{24} + e^{35}, e^{36} + e^{14}$                                | 258      |
| 852:24b     | $0, 0, 0, e^{12}, -e^{13}, e^{23}, e^{24} + e^{35}, e^{36} + e^{14}$                               | 258      |
| 852:24c     | $0, 0, 0, -e^{12}, -e^{13}, e^{23}, e^{24} + e^{35}, e^{36} + e^{14}$                              | 258      |
| 852:25a     | $0, 0, 0, e^{12}, e^{13}, e^{23}, e^{25} + e^{34}, e^{36} + e^{14}$                                | 258      |
| 852:25b     | $0, 0, 0, -e^{12}, -e^{13}, e^{23}, e^{25} + e^{34}, e^{36} + e^{14}$                              | 258      |
| 852:26      | $0, 0, 0, a_1e^{12}, e^{13}, e^{23}, e^{24} + e^{15}, e^{26} + e^{35} + e^{14}$                    | 258      |
| 852:27      | $0, 0, 0, e^{12}a_1, (1 + a_1)e^{13}, e^{23}, e^{24} + e^{15}, e^{25} + e^{34} + e^{16}$           | 258      |
| 852:28a     | $0, 0, 0, (-1 + a_2)e^{12}, a_2e^{13}, e^{23}, e^{24} + e^{35}, e^{25} + e^{34} + e^{16}$          | 258      |
| 852:28b     | $0, 0, 0, (-1 + a_2)e^{12}, a_2e^{13}, e^{23}, -e^{24} + e^{35}, e^{25} + e^{34} + e^{16}$         | 258      |
| 852:29      | $0, 0, 0, e^{12}, e^{13}, e^{23}, e^{25} + e^{34}, e^{24} + e^{36} + e^{15}$                       | 258      |
| 852:30      | $0, 0, 0, a_1e^{12}, e^{13}a_2, e^{23}, e^{26} + e^{35} + e^{14}, e^{24} + e^{36} + e^{15}$        | 258      |
| 852:31      | $0, 0, 0, (-1 + a_2)e^{12}, a_2e^{13}, e^{23}, e^{25} + e^{34} + e^{16}, e^{24} + e^{36} + e^{15}$ | 258      |
| Type: 41111 |                                                                                                    |          |
| 84321:1     | $0, 0, 0, 0, e^{12}, e^{15}, e^{16}, e^{17}$                                                       | 34568    |
| 84321:2     | $0, 0, 0, 0, e^{12}, e^{15}, e^{16}, e^{34} + e^{17}$                                              | 14568    |
| 84321:3     | $0, 0, 0, 0, e^{12}, e^{15}, e^{16}, e^{17} + e^{23}$                                              | 24568    |
| 84321:4     | $0, 0, 0, 0, e^{12}, e^{15}, e^{16}, e^{25} + e^{17}$                                              | 34568    |
| 84321:5     | $0, 0, 0, 0, -e^{12}, e^{15}, e^{16}, e^{56} + e^{27}$                                             | 34568    |
| 84321:6     | $0, 0, 0, 0, -e^{12}, e^{15}, e^{16} + e^{23}, e^{35} + e^{17}$                                    | 23568    |
| 84321:7     | $0, 0, 0, 0, e^{12}, e^{15}, e^{16}, e^{25} + e^{34} + e^{17}$                                     | 14568    |
| 84321:8     | $0, 0, 0, 0, -e^{12}, e^{15}, e^{16}, e^{34} + e^{27} + e^{56}$                                    | 14568    |
| 84321:9     | $0, 0, 0, 0, -e^{12}, e^{15}, e^{16} + e^{23}, e^{27} + e^{56}$                                    | 23568    |
| 84321:10    | $0, 0, 0, 0, -e^{12}, e^{15}, e^{16}, e^{13} + e^{27} + e^{56}$                                    | 24568    |
| 84321:11    | $0, 0, 0, 0, -e^{12}, e^{15}, e^{16} + e^{23}, e^{24} + e^{35} + e^{17}$                           | 13568    |
| 84321:12    | $0, 0, 0, 0, e^{12}, e^{15}, e^{25} + e^{16}, e^{26} + e^{17}$                                     | 34568    |
| 84321:13    | $0, 0, 0, 0, -e^{12}, e^{15}, e^{16} + e^{23}, e^{34} + e^{27} + e^{56}$                           | 13568    |
| 84321:14    | $0, 0, 0, 0, -e^{12}, e^{15}, e^{25} + e^{16}, e^{27} + e^{56}$                                    | 34568    |
| 84321:15    | $0, 0, 0, 0, e^{12}, e^{15}, e^{25} + e^{16}, e^{26} + e^{34} + e^{17}$                            | 14568    |
| 84321:16    | $0, 0, 0, 0, -e^{12}, e^{15}, e^{16} + e^{23}, e^{13} + e^{27} + e^{56}$                           | 23568    |
| 84321:17    | $0, 0, 0, 0, -e^{12}, e^{15}, e^{16} + e^{23}, e^{27} + e^{14} + e^{56}$                           | 13568    |
| 84321:18    | $0, 0, 0, 0, -e^{12}, e^{15}, e^{25} + e^{16}, e^{34} + e^{27} + e^{56}$                           | 14568    |
| 84321:19    | $0, 0, 0, 0, -e^{12}, e^{15}, e^{25} + e^{16}, e^{13} + e^{27} + e^{56}$                           | 24568    |
| 84321:20    | $0, 0, 0, 0, -e^{12}, e^{15} + e^{23}, e^{35} + e^{16}, e^{36} + e^{17}$                           | 23468    |
| 84321:22    | $0, 0, 0, 0, -e^{12}, e^{15} + e^{23}, e^{35} + e^{16}, e^{24} + e^{36} + e^{17}$                  | 13468    |
| 84321:27    | $0, 0, 0, 0, -e^{12}, e^{15} + e^{23}, e^{35} + e^{16}, e^{36} + e^{25} + e^{17}$                  | 23468    |

Table 1 – Continued to next page



Table 1 – Continued from previous page

| Name     | g                                                                                              | UCS Dim. |
|----------|------------------------------------------------------------------------------------------------|----------|
| 84321:29 | $0, 0, 0, 0, -e^{12}, e^{15} + e^{23}, e^{24} + e^{35} + e^{16}, e^{36} + e^{17} + e^{45}$     | 12468    |
|          | Type: 4121                                                                                     |          |
| 8431:1   | $0, 0, 0, 0, e^{12}, e^{15}, e^{25}, e^{16}$                                                   | 4568     |
| 8431:2   | $0, 0, 0, 0, e^{12}, e^{15}, e^{25} + e^{34}, e^{16}$                                          | 2568     |
| 8431:3   | $0, 0, 0, 0, e^{12}, e^{15}, e^{13} + e^{25}, e^{16}$                                          | 3568     |
| 8431:4   | $0, 0, 0, 0, e^{12}, e^{15}, e^{25}, e^{34} + e^{16}$                                          | 2568     |
| 8431:5   | $0, 0, 0, 0, e^{12}, e^{15}, e^{25}, e^{16} + e^{23}$                                          | 3568     |
| 8431:6   | $0, 0, 0, 0, e^{12}, e^{15}, e^{13} + e^{25}, e^{34} + e^{16}$                                 | 2568     |
| 8431:7   | $0, 0, 0, 0, e^{12}, e^{15}, e^{25} + e^{34}, e^{16} + e^{23}$                                 | 2568     |
| 8431:8   | $0, 0, 0, 0, e^{12}, e^{15}, e^{13} + e^{25}, e^{16} + e^{23}$                                 | 3568     |
| 8431:9   | $0, 0, 0, 0, e^{12}, e^{15}, e^{13} + e^{25}, e^{24} + e^{16}$                                 | 2568     |
| 8431:10  | $0, 0, 0, 0, e^{12}, e^{13} + e^{25}, e^{15}, e^{26} + e^{35}$                                 | 3468     |
| 8431:11  | $0, 0, 0, 0, e^{12}, e^{13} + e^{25}, e^{34} + e^{15}, e^{26} + e^{35}$                        | 2468     |
| 8431:12a | $0, 0, 0, 0, -e^{12}, e^{15} + e^{23}, e^{13} + e^{25}, e^{35} + e^{16}$                       | 3468     |
| 8431:12b | $0, 0, 0, 0, -e^{12}, -e^{15} + e^{23}, e^{13} + e^{25}, e^{35} + e^{16}$                      | 3468     |
| 8431:13  | $0, 0, 0, 0, -e^{12}, e^{15} + e^{23}, e^{25} + e^{14}, e^{35} + e^{16}$                       | 2468     |
| 8431:14  | $0, 0, 0, 0, e^{12}, e^{13} + e^{25}, e^{15}, e^{26} + e^{35} + e^{14}$                        | 2468     |
| 8431:15a | $0, 0, 0, 0, e^{12}, e^{13} + e^{25}, e^{34} + e^{15}, e^{26} + e^{35} + e^{14}$               | 2468     |
| 8431:15b | $0, 0, 0, 0, e^{12}, e^{13} + e^{25}, e^{34} - e^{15}, e^{26} + e^{35} + e^{14}$               | 2468     |
| 8431:16  | $0, 0, 0, 0, -e^{12}, e^{15} + e^{23}, e^{25} + e^{14}, e^{24} + e^{35} + e^{16}$              | 2468     |
| 8431:17a | $0, 0, 0, 0, -e^{12}, e^{15} + e^{23}, e^{13} + e^{25}, e^{24} + e^{35} + e^{16}$              | 2468     |
| 8431:17b | $0, 0, 0, 0, -e^{12}, -e^{15} + e^{23}, e^{13} + e^{25}, e^{24} + e^{35} + e^{16}$             | 2468     |
| 8431:18a | $0, 0, 0, 0, e^{12}, e^{15}, e^{25}, e^{27} + e^{16}$                                          | 3568     |
| 8431:18b | $0, 0, 0, 0, e^{12}, -e^{15}, e^{25}, e^{27} + e^{16}$                                         | 3568     |
| 8431:19  | $0, 0, 0, 0, e^{12}, e^{15}, e^{25}, e^{26} + e^{17}$                                          | 3568     |
| 8431:20a | $0, 0, 0, 0, e^{12}, e^{15}, e^{25}, e^{34} + e^{27} + e^{16}$                                 | 1568     |
| 8431:20b | $0, 0, 0, 0, e^{12}, -e^{15}, e^{25}, e^{34} + e^{27} + e^{16}$                                | 1568     |
| 8431:21  | $0, 0, 0, 0, e^{12}, e^{15}, e^{25}, e^{26} + e^{34} + e^{17}$                                 | 1568     |
| 8431:22  | $0, 0, 0, 0, e^{12}, e^{15}, e^{13} + e^{25}, e^{26} + e^{17}$                                 | 2468     |
| 8431:23  | $0, 0, 0, 0, e^{12}, e^{15}, e^{13} + e^{25}, e^{26} + e^{34} + e^{17}$                        | 1468     |
| 8431:24a | $0, 0, 0, 0, e^{12}, e^{15} + e^{23}, e^{13} + e^{25}, e^{27} + e^{16}$                        | 2468     |
| 8431:24b | $0, 0, 0, 0, e^{12}, -e^{15} + e^{23}, e^{13} + e^{25}, e^{27} + e^{16}$                       | 2468     |
| 8431:25a | $0, 0, 0, 0, e^{12}, e^{13} + e^{25}, e^{15} + e^{23}, e^{27} + e^{16}$                        | 2468     |
| 8431:25b | $0, 0, 0, 0, e^{12}, -e^{13} + e^{25}, e^{15} + e^{23}, e^{27} + e^{16}$                       | 2468     |
| 8431:26a | $0, 0, 0, 0, e^{12}, e^{15}, e^{13} + e^{25}, e^{27} + e^{35} + e^{16}$                        | 2468     |
| 8431:26b | $0, 0, 0, 0, e^{12}, -e^{15}, e^{13} + e^{25}, e^{27} + e^{35} + e^{16}$                       | 2468     |
| 8431:27a | $0, 0, 0, 0, e^{12}, e^{15} + e^{23}, e^{13} + e^{25}, e^{34} + e^{27} + e^{16}$               | 1468     |
| 8431:27b | $0, 0, 0, 0, e^{12}, -e^{15} + e^{23}, e^{13} + e^{25}, e^{34} + e^{27} + e^{16}$              | 1468     |
| 8431:28a | $0, 0, 0, 0, e^{12}, e^{15} + e^{23}, e^{13} + e^{25}, e^{26} + e^{34} + e^{17}$               | 1468     |
| 8431:28b | $0, 0, 0, 0, e^{12}, e^{15} + e^{23}, -e^{13} + e^{25}, e^{26} + e^{34} + e^{17}$              | 1468     |
| 8431:29  | $0, 0, 0, 0, e^{12}, e^{13} + e^{25}, e^{24} + e^{15}, e^{27} + e^{16}$                        | 1368     |
| 8431:30a | $0, 0, 0, 0, (-1 + a_2)e^{12}, e^{15} + e^{23}, e^{13}a_2 + e^{25}, e^{27} + e^{35} + e^{16}$  | 2468     |
| 8431:30b | $0, 0, 0, 0, (-1 + a_2)e^{12}, -e^{15} + e^{23}, e^{13}a_2 + e^{25}, e^{27} + e^{35} + e^{16}$ | 2468     |
| 8431:31  | $0, 0, 0, 0, a_1e^{12}, e^{15} + e^{23}, e^{25} + e^{14}, e^{26} + e^{34} + e^{17}$            | 1368     |
|          | Type: 4211                                                                                     |          |
| 8421:1   | $0, 0, 0, 0, e^{12}, e^{34}, e^{15}, e^{17}$                                                   | 2568     |
| 8421:2   | $0, 0, 0, 0, e^{12}, e^{13}, e^{15}, e^{17}$                                                   | 3568     |
| 8421:3   | $0, 0, 0, 0, e^{12}, e^{13}, e^{25}, e^{27}$                                                   | 3568     |
| 8421:4   | $0, 0, 0, 0, e^{12}, e^{13}, e^{15}, e^{34} + e^{17}$                                          | 2568     |
| 8421:5   | $0, 0, 0, 0, e^{12}, e^{13}, e^{25}, e^{34} + e^{27}$                                          | 2568     |
| 8421:6   | $0, 0, 0, 0, e^{12}, e^{24} + e^{13}, e^{15}, e^{17}$                                          | 2568     |
| 8421:7   | $0, 0, 0, 0, e^{12}, e^{34}, e^{15}, e^{17} + e^{23}$                                          | 2568     |
| 8421:8   | $0, 0, 0, 0, e^{12}, e^{13}, e^{15}, e^{17} + e^{23}$                                          | 3568     |
| 8421:9   | $0, 0, 0, 0, e^{12}, e^{13}, e^{15}, e^{24} + e^{17}$                                          | 2568     |
| 8421:10  | $0, 0, 0, 0, e^{12}, e^{13}, e^{25}, e^{27} + e^{14}$                                          | 2568     |
| 8421:11a | $0, 0, 0, 0, e^{12}, e^{24} + e^{13}, e^{15}, e^{34} + e^{17}$                                 | 2568     |
| 8421:11b | $0, 0, 0, 0, -e^{12}, e^{24} + e^{13}, e^{15}, e^{34} + e^{17}$                                | 2568     |
| 8421:12  | $0, 0, 0, 0, e^{12}, e^{34}, e^{15}, e^{25} + e^{17}$                                          | 2568     |

Table 1 – Continued to next page

Table 1 – Continued from previous page

| Name      | g                                                                                             | UCS Dim. |
|-----------|-----------------------------------------------------------------------------------------------|----------|
| 8421:13   | $0, 0, 0, 0, e^{12}, e^{24} + e^{13}, e^{15}, e^{17} + e^{23}$                                | 2568     |
| 8421:14   | $0, 0, 0, 0, e^{12}, e^{13}, e^{15}, e^{25} + e^{17}$                                         | 3568     |
| 8421:15   | $0, 0, 0, 0, e^{12}, e^{13}, e^{25}, e^{27} + e^{15}$                                         | 3568     |
| 8421:16   | $0, 0, 0, 0, e^{12}, e^{13}, e^{15}, e^{36} + e^{17}$                                         | 2468     |
| 8421:17   | $0, 0, 0, 0, e^{12}, e^{13}, e^{25}, e^{36} + e^{27}$                                         | 2468     |
| 8421:18   | $0, 0, 0, 0, e^{12}, e^{13}, e^{15}, e^{25} + e^{34} + e^{17}$                                | 2568     |
| 8421:19   | $0, 0, 0, 0, e^{12}, e^{13}, e^{25}, e^{34} + e^{27} + e^{15}$                                | 2568     |
| 8421:20   | $0, 0, 0, 0, e^{12}, e^{24} + e^{13}, e^{15}, e^{25} + e^{17}$                                | 2568     |
| 8421:21   | $0, 0, 0, 0, -e^{12}, e^{34}, e^{15} + e^{23}, e^{35} + e^{17}$                               | 2468     |
| 8421:22   | $0, 0, 0, 0, e^{12}, e^{13}, e^{25}, e^{27} + e^{16}$                                         | 2468     |
| 8421:23   | $0, 0, 0, 0, e^{12}, e^{34}, e^{15}, e^{36} + e^{17}$                                         | 1368     |
| 8421:24a  | $0, 0, 0, 0, e^{12}, e^{24} + e^{13}, e^{15}, e^{25} + e^{34} + e^{17}$                       | 2568     |
| 8421:24b  | $0, 0, 0, 0, -e^{12}, e^{24} + e^{13}, e^{15}, e^{25} + e^{34} + e^{17}$                      | 2568     |
| 8421:25   | $0, 0, 0, 0, -e^{12}, e^{13}, e^{15} + e^{23}, e^{35} + e^{17}$                               | 3468     |
| 8421:26   | $0, 0, 0, 0, -e^{12}, e^{13}, e^{24} + e^{15}, e^{45} + e^{17}$                               | 2468     |
| 8421:27   | $0, 0, 0, 0, e^{12}, e^{13}, e^{25} + e^{14}, e^{27} + e^{45}$                                | 2468     |
| 8421:28   | $0, 0, 0, 0, e^{12}, e^{13}, e^{15}, e^{24} + e^{36} + e^{17}$                                | 1468     |
| 8421:29   | $0, 0, 0, 0, e^{12}, e^{13}, e^{25}, e^{36} + e^{27} + e^{14}$                                | 1468     |
| 8421:30   | $0, 0, 0, 0, e^{12}, e^{13}, e^{25}, e^{34} + e^{27} + e^{16}$                                | 1468     |
| 8421:31   | $0, 0, 0, 0, e^{12}, e^{13}, e^{15} + e^{23}, e^{26} + e^{17}$                                | 2468     |
| 8421:32   | $0, 0, 0, 0, e^{12}, -e^{13}, e^{34} + e^{15}, e^{17} + e^{46}$                               | 1368     |
| 8421:33   | $0, 0, 0, 0, -e^{12}, e^{24} + e^{13}, e^{15} + e^{23}, e^{35} + e^{17}$                      | 2468     |
| 8421:34   | $0, 0, 0, 0, e^{12}, e^{34}, e^{13} + e^{25}, e^{27} + e^{35} + e^{14}$                       | 2468     |
| 8421:35   | $0, 0, 0, 0, e^{12}, e^{34}, e^{15}, e^{46} + e^{17} + e^{23}$                                | 1368     |
| 8421:36a  | $0, 0, 0, 0, e^{12}, e^{13}, e^{15}, e^{36} + e^{25} + e^{17}$                                | 2468     |
| 8421:36b  | $0, 0, 0, 0, -e^{12}, e^{13}, e^{15}, e^{36} + e^{25} + e^{17}$                               | 2468     |
| 8421:37   | $0, 0, 0, 0, e^{12}, e^{13}, e^{15}, e^{26} + e^{35} + e^{17}$                                | 2468     |
| 8421:38   | $0, 0, 0, 0, e^{12}, e^{13}, e^{25}, e^{36} + e^{27} + e^{15}$                                | 2468     |
| 8421:39   | $0, 0, 0, 0, -e^{12}, e^{13}, e^{24} + e^{15}, e^{17} + e^{23} + e^{45}$                      | 2468     |
| 8421:40   | $0, 0, 0, 0, -e^{12}, e^{13}, e^{15} + e^{23}, e^{24} + e^{35} + e^{17}$                      | 2468     |
| 8421:41   | $0, 0, 0, 0, e^{12}, e^{13}, e^{15} + e^{23}, e^{26} + e^{34} + e^{17}$                       | 1468     |
| 8421:42   | $0, 0, 0, 0, e^{12}, e^{14} + e^{23}, e^{34} + e^{15}, e^{36} + e^{17}$                       | 1368     |
| 8421:43   | $0, 0, 0, 0, e^{12}, e^{34}, e^{15}, e^{36} + e^{25} + e^{17}$                                | 1368     |
| 8421:44   | $0, 0, 0, 0, e^{12}, -e^{13}, e^{34} + e^{15}, e^{46} + e^{17} + e^{23}$                      | 1368     |
| 8421:45   | $0, 0, 0, 0, (-1 + a_2)e^{12}, e^{13}a_2, e^{15} + e^{23}, e^{26} + e^{35} + e^{17}$          | 2468     |
| 8421:46   | $0, 0, 0, 0, -e^{12}, e^{34}, e^{15} + e^{23}, e^{46} + e^{35} + e^{17}$                      | 1368     |
| 8421:47   | $0, 0, 0, 0, e^{12}, e^{14} + e^{23}, e^{13} + e^{25}, e^{27} + e^{16}$                       | 1368     |
| 8421:48   | $0, 0, 0, 0, e^{12}, -e^{13}, e^{34} + e^{15}, e^{46} + e^{25} + e^{17}$                      | 1368     |
| 8421:49   | $0, 0, 0, 0, -e^{12}, e^{13}, e^{24} + e^{15}, e^{45} + e^{36} + e^{17}$                      | 1368     |
| 8421:50   | $0, 0, 0, 0, e^{12}, e^{13}, e^{25} + e^{14}, e^{36} + e^{27} + e^{45}$                       | 1368     |
| 8421:51   | $0, 0, 0, 0, e^{12}, e^{24} - e^{13}, e^{34} + e^{15}, e^{46} + e^{17} + e^{23}$              | 1368     |
| 8421:52   | $0, 0, 0, 0, e^{12}, e^{24} + e^{13}, e^{15}, e^{26} + e^{35} + e^{17}$                       | 1368     |
| 8421:53   | $0, 0, 0, 0, e^{12}, e^{13}, e^{25} + e^{14}, e^{27} + e^{16} + e^{45}$                       | 1368     |
| 8421:54a  | $0, 0, 0, 0, e^{12}, e^{14} + e^{23}, e^{13} + e^{25}, e^{34} + e^{27} + e^{16}$              | 1368     |
| 8421:54b  | $0, 0, 0, 0, -e^{12}, e^{14} + e^{23}, e^{13} + e^{25}, e^{34} + e^{27} + e^{16}$             | 1368     |
| 8421:55   | $0, 0, 0, 0, e^{12}, e^{14} + e^{23}, e^{34} + e^{15}, e^{36} + e^{25} + e^{17}$              | 1368     |
| 8421:56   | $0, 0, 0, 0, e^{12}(-1 + a_2), e^{14} + e^{23}, a_2e^{13} + e^{25}, e^{27} + e^{35} + e^{16}$ | 1368     |
| Type: 422 |                                                                                               |          |
| 842:1     | $0, 0, 0, 0, e^{12}, e^{13}, e^{15}, e^{25}$                                                  | 468      |
| 842:2     | $0, 0, 0, 0, e^{12}, e^{34}, e^{15}, e^{25}$                                                  | 368      |
| 842:3     | $0, 0, 0, 0, e^{12}, e^{13}, e^{25}, e^{15} + e^{23}$                                         | 468      |
| 842:4     | $0, 0, 0, 0, e^{12}, e^{13}, e^{15}, e^{25} + e^{34}$                                         | 368      |
| 842:5     | $0, 0, 0, 0, e^{12}, e^{13}, e^{25}, e^{34} + e^{15}$                                         | 368      |
| 842:6     | $0, 0, 0, 0, e^{12}, e^{24} + e^{13}, e^{15}, e^{25}$                                         | 368      |
| 842:7     | $0, 0, 0, 0, e^{12}, e^{34}, e^{15}, e^{13} + e^{25}$                                         | 368      |
| 842:8     | $0, 0, 0, 0, e^{12}, e^{13}, e^{15}, e^{25} + e^{14}$                                         | 368      |
| 842:9     | $0, 0, 0, 0, e^{12}, e^{13}, e^{25}, e^{24} + e^{15}$                                         | 368      |
| 842:10    | $0, 0, 0, 0, e^{12}, e^{24} + e^{13}, e^{15}, e^{25} + e^{34}$                                | 368      |

Table 1 – Continued to next page

Table 1 – *Continued from previous page*

| Name    | g                                                                       | UCS Dim. |
|---------|-------------------------------------------------------------------------|----------|
| 842:11  | $0, 0, 0, 0, e^{12}, e^{13}, e^{15} + e^{23}, e^{25} + e^{34}$          | 368      |
| 842:12  | $0, 0, 0, 0, e^{12}, e^{13}, e^{25} + e^{14}, e^{34} + e^{15}$          | 368      |
| 842:13  | $0, 0, 0, 0, e^{12}, e^{13}, e^{24} + e^{15}, e^{25} + e^{34}$          | 368      |
| 842:14  | $0, 0, 0, 0, e^{12}, e^{14} + e^{23}, e^{15}, e^{13} + e^{25}$          | 368      |
| 842:15a | $0, 0, 0, 0, e^{12}, e^{34}, e^{15} + e^{23}, e^{13} + e^{25}$          | 368      |
| 842:15b | $0, 0, 0, 0, e^{12}, e^{34}, -e^{15} + e^{23}, e^{13} + e^{25}$         | 368      |
| 842:16  | $0, 0, 0, 0, e^{12}, e^{34}, e^{15} + e^{23}, e^{25} + e^{14}$          | 368      |
| 842:17  | $0, 0, 0, 0, e^{12}, e^{13}, e^{15} + e^{23}, e^{25} + e^{14}$          | 368      |
| 842:18a | $0, 0, 0, 0, e^{12}, e^{13}, e^{24} + e^{15}, e^{25} + e^{14}$          | 368      |
| 842:18b | $0, 0, 0, 0, e^{12}, e^{13}, e^{24} - e^{15}, e^{25} + e^{14}$          | 368      |
| 842:19  | $0, 0, 0, 0, e^{12}, e^{14} + e^{23}, e^{13} + e^{25}, e^{34} + e^{15}$ | 368      |
| 842:20  | $0, 0, 0, 0, e^{12}, e^{24} + e^{13}, e^{15} + e^{23}, e^{25} + e^{14}$ | 368      |
| 842:21  | $0, 0, 0, 0, e^{12}, e^{13}, e^{15}, e^{16}$                            | 358      |
| 842:22  | $0, 0, 0, 0, e^{12}, e^{13}, e^{25}, e^{16}$                            | 358      |
| 842:23  | $0, 0, 0, 0, e^{12}, e^{13}, e^{25}, e^{36}$                            | 358      |
| 842:24  | $0, 0, 0, 0, e^{12}, e^{13}, e^{15}, e^{16} + e^{23}$                   | 358      |
| 842:25  | $0, 0, 0, 0, e^{12}, e^{13}, e^{25}, e^{16} + e^{23}$                   | 358      |
| 842:26  | $0, 0, 0, 0, e^{12}, e^{13}, e^{15}, e^{24} + e^{16}$                   | 258      |
| 842:27  | $0, 0, 0, 0, e^{12}, e^{13}, e^{25}, e^{24} + e^{16}$                   | 258      |
| 842:28  | $0, 0, 0, 0, e^{12}, e^{13}, e^{15}, e^{36} + e^{14}$                   | 258      |
| 842:29  | $0, 0, 0, 0, e^{12}, e^{13}, e^{15}, e^{34} + e^{16}$                   | 258      |
| 842:30  | $0, 0, 0, 0, e^{12}, e^{13}, e^{15}, e^{24} + e^{36}$                   | 258      |
| 842:31  | $0, 0, 0, 0, e^{12}, e^{13}, e^{25}, e^{36} + e^{14}$                   | 258      |
| 842:32  | $0, 0, 0, 0, e^{12}, e^{13}, e^{25}, e^{34} + e^{16}$                   | 258      |
| 842:33  | $0, 0, 0, 0, e^{12}, e^{13}, e^{25}, e^{24} + e^{36}$                   | 258      |
| 842:34  | $0, 0, 0, 0, e^{12}, e^{13}, e^{15}, e^{25} + e^{16}$                   | 358      |
| 842:35a | $0, 0, 0, 0, e^{12}, e^{13}, e^{15}, e^{36} + e^{25}$                   | 358      |
| 842:35b | $0, 0, 0, 0, -e^{12}, e^{13}, e^{15}, e^{36} + e^{25}$                  | 358      |
| 842:36  | $0, 0, 0, 0, e^{12}, e^{13}, e^{15}, e^{26} + e^{35}$                   | 358      |
| 842:37  | $0, 0, 0, 0, e^{12}, e^{13}, e^{25}, e^{36} + e^{15}$                   | 358      |
| 842:38  | $0, 0, 0, 0, e^{12}, e^{13}, e^{25}, e^{26} + e^{35}$                   | 358      |
| 842:39  | $0, 0, 0, 0, e^{12}, e^{13}, e^{25} + e^{14}, e^{24} + e^{16}$          | 258      |
| 842:40a | $0, 0, 0, 0, e^{12}, e^{13}, e^{24} + e^{15}, e^{36} + e^{14}$          | 258      |
| 842:40b | $0, 0, 0, 0, -e^{12}, e^{13}, e^{24} + e^{15}, e^{36} + e^{14}$         | 258      |
| 842:41  | $0, 0, 0, 0, e^{12}a_1, e^{13}, e^{24} + e^{15}, e^{34} + e^{16}$       | 258      |
| 842:42  | $0, 0, 0, 0, e^{12}, e^{13}, e^{25} + e^{14}, e^{24} + e^{36}$          | 258      |
| 842:43a | $0, 0, 0, 0, e^{12}, e^{13}, e^{34} + e^{15}, e^{24} + e^{16}$          | 258      |
| 842:43b | $0, 0, 0, 0, -e^{12}, e^{13}, e^{34} + e^{15}, e^{24} + e^{16}$         | 258      |
| 842:44  | $0, 0, 0, 0, e^{12}, e^{13}, e^{25} + e^{34}, e^{24} + e^{16}$          | 258      |
| 842:45  | $0, 0, 0, 0, e^{12}, e^{13}, e^{25} + e^{34}, e^{24} + e^{36}$          | 258      |
| 842:46  | $0, 0, 0, 0, e^{12}, e^{13}, e^{15} + e^{23}, e^{24} + e^{16}$          | 258      |
| 842:47  | $0, 0, 0, 0, e^{12}, e^{13}, e^{15} + e^{23}, e^{36} + e^{14}$          | 258      |
| 842:48  | $0, 0, 0, 0, e^{12}, e^{13}, e^{15} + e^{23}, e^{34} + e^{16}$          | 258      |
| 842:49  | $0, 0, 0, 0, e^{12}, e^{13}, e^{15} + e^{23}, e^{24} + e^{36}$          | 258      |
| 842:50  | $0, 0, 0, 0, e^{12}, e^{13}, e^{15} + e^{23}, e^{25} + e^{16}$          | 358      |
| 842:51a | $0, 0, 0, 0, e^{12}, e^{13}, e^{15} + e^{23}, e^{36} + e^{25}$          | 358      |
| 842:51b | $0, 0, 0, 0, -e^{12}, e^{13}, e^{15} + e^{23}, e^{36} + e^{25}$         | 358      |
| 842:52  | $0, 0, 0, 0, e^{12}, e^{13}, e^{15} + e^{23}, e^{26} + e^{35}$          | 358      |
| 842:53a | $0, 0, 0, 0, e^{12}, e^{13}, e^{15}, e^{36} + e^{25} + e^{14}$          | 258      |
| 842:53b | $0, 0, 0, 0, -e^{12}, e^{13}, e^{15}, e^{36} + e^{25} + e^{14}$         | 258      |
| 842:54  | $0, 0, 0, 0, e^{12}, e^{13}, e^{15}, e^{26} + e^{35} + e^{14}$          | 258      |
| 842:55  | $0, 0, 0, 0, e^{12}, e^{13}, e^{15}, e^{25} + e^{34} + e^{16}$          | 258      |
| 842:56  | $0, 0, 0, 0, e^{12}, e^{13}, e^{25}, e^{24} + e^{36} + e^{15}$          | 258      |
| 842:57  | $0, 0, 0, 0, e^{12}, e^{13}, e^{25}, e^{26} + e^{35} + e^{14}$          | 258      |
| 842:58  | $0, 0, 0, 0, e^{12}, e^{13}, e^{24} + e^{15}, e^{25} + e^{16}$          | 258      |
| 842:59  | $0, 0, 0, 0, e^{12}, e^{13}, e^{25} + e^{14}, e^{36} + e^{15}$          | 258      |
| 842:60a | $0, 0, 0, 0, e^{12}, e^{13}, e^{24} + e^{15}, e^{36} + e^{25}$          | 258      |
| 842:60b | $0, 0, 0, 0, -e^{12}, e^{13}, e^{24} + e^{15}, e^{36} + e^{25}$         | 258      |

Table 1 – *Continued to next page*

Table 1 – Continued from previous page

| Name    | $g$                                                                                  | UCS Dim. |
|---------|--------------------------------------------------------------------------------------|----------|
| 842:61  | $0, 0, 0, 0, e^{12}, e^{13}, e^{25} + e^{14}, e^{26} + e^{35}$                       | 258      |
| 842:62  | $0, 0, 0, 0, e^{12}, e^{13}, e^{24} + e^{15}, e^{26} + e^{35}$                       | 258      |
| 842:63  | $0, 0, 0, 0, e^{12}, e^{13}, e^{34} + e^{15}, e^{25} + e^{16}$                       | 258      |
| 842:64a | $0, 0, 0, 0, e^{12}, e^{13}, e^{34} + e^{15}, e^{36} + e^{25}$                       | 258      |
| 842:64b | $0, 0, 0, 0, -e^{12}, e^{13}, e^{34} + e^{15}, e^{36} + e^{25}$                      | 258      |
| 842:65  | $0, 0, 0, 0, e^{12}, e^{13}, e^{34} + e^{15}, e^{26} + e^{35}$                       | 258      |
| 842:66  | $0, 0, 0, 0, e^{12}, e^{13}, e^{25} + e^{34}, e^{36} + e^{15}$                       | 258      |
| 842:67  | $0, 0, 0, 0, e^{12}, e^{13}, e^{25} + e^{34}, e^{26} + e^{35}$                       | 258      |
| 842:68  | $0, 0, 0, 0, e^{12}, e^{13}, e^{25} + e^{16}, e^{36} + e^{15}$                       | 358      |
| 842:69  | $0, 0, 0, 0, e^{12}, e^{13}, e^{25} + e^{16}, e^{26} + e^{35}$                       | 358      |
| 842:70a | $0, 0, 0, 0, e^{12}, e^{13}, e^{26} + e^{35}, e^{36} + e^{25}$                       | 358      |
| 842:70b | $0, 0, 0, 0, -e^{12}, e^{13}, -e^{26} + e^{35}, e^{36} + e^{25}$                     | 358      |
| 842:71a | $0, 0, 0, 0, e^{12}, e^{13}, e^{25} + e^{14}, e^{24} + e^{36} + e^{15}$              | 258      |
| 842:71b | $0, 0, 0, 0, e^{12}, e^{13}, e^{25} - e^{14}, e^{24} + e^{36} + e^{15}$              | 258      |
| 842:72a | $0, 0, 0, 0, e^{12}, e^{13}, e^{24} + e^{15}, e^{36} + e^{25} + e^{14}$              | 258      |
| 842:72b | $0, 0, 0, 0, e^{12}, e^{13}, e^{24} - e^{15}, e^{36} + e^{25} + e^{14}$              | 258      |
| 842:72c | $0, 0, 0, 0, -e^{12}, e^{13}, e^{24} + e^{15}, e^{36} + e^{25} + e^{14}$             | 258      |
| 842:72d | $0, 0, 0, 0, -e^{12}, e^{13}, e^{24} - e^{15}, e^{36} + e^{25} + e^{14}$             | 258      |
| 842:73  | $0, 0, 0, 0, e^{12}, e^{13}, e^{24} + e^{15}, e^{26} + e^{35} + e^{14}$              | 258      |
| 842:74  | $0, 0, 0, 0, e^{12} a_1, e^{13}, e^{24} + e^{15}, e^{25} + e^{34} + e^{16}$          | 258      |
| 842:75a | $0, 0, 0, 0, e^{12}, e^{13}, e^{34} + e^{15}, e^{36} + e^{25} + e^{14}$              | 258      |
| 842:75b | $0, 0, 0, 0, -e^{12}, e^{13}, e^{34} + e^{15}, e^{36} + e^{25} + e^{14}$             | 258      |
| 842:76a | $0, 0, 0, 0, e^{12}, e^{13}, e^{34} + e^{15}, e^{26} + e^{35} + e^{14}$              | 258      |
| 842:76b | $0, 0, 0, 0, e^{12}, e^{13}, e^{34} - e^{15}, e^{26} + e^{35} + e^{14}$              | 258      |
| 842:77  | $0, 0, 0, 0, e^{12}, e^{13}, e^{25} + e^{34}, e^{24} + e^{36} + e^{15}$              | 258      |
| 842:78  | $0, 0, 0, 0, e^{12}, e^{13}, e^{25} + e^{34}, e^{26} + e^{35} + e^{14}$              | 258      |
| 842:79a | $0, 0, 0, 0, e^{12}, e^{13}, e^{15} + e^{23}, e^{36} + e^{25} + e^{14}$              | 258      |
| 842:79b | $0, 0, 0, 0, -e^{12}, e^{13}, e^{15} + e^{23}, e^{36} + e^{25} + e^{14}$             | 258      |
| 842:80  | $0, 0, 0, 0, e^{12}, e^{13}, e^{15} + e^{23}, e^{26} + e^{35} + e^{14}$              | 258      |
| 842:81  | $0, 0, 0, 0, e^{12}, e^{13}, e^{15} + e^{23}, e^{25} + e^{34} + e^{16}$              | 258      |
| 842:82  | $0, 0, 0, 0, e^{12}, e^{13}, e^{25} + e^{16}, e^{24} + e^{36} + e^{15}$              | 258      |
| 842:83  | $0, 0, 0, 0, e^{12}, e^{13}, e^{25} + e^{16}, e^{26} + e^{35} + e^{14}$              | 258      |
| 842:84a | $0, 0, 0, 0, e^{12}, e^{13}, e^{36} + e^{25}, e^{26} + e^{35} + e^{14}$              | 258      |
| 842:84b | $0, 0, 0, 0, e^{12}, e^{13}, e^{36} - e^{25}, e^{26} + e^{35} + e^{14}$              | 258      |
| 842:85a | $0, 0, 0, 0, e^{12}, e^{13}, e^{26} + e^{35}, e^{36} + e^{25} + e^{14}$              | 258      |
| 842:85b | $0, 0, 0, 0, -e^{12}, e^{13}, -e^{26} + e^{35}, e^{36} + e^{25} + e^{14}$            | 258      |
| 842:86  | $0, 0, 0, 0, e^{12}, e^{13}, e^{26} + e^{35}, e^{24} + e^{36} + e^{15}$              | 258      |
| 842:87  | $0, 0, 0, 0, e^{12}, e^{13}, e^{26} + e^{35} + e^{14}, e^{24} + e^{36} + e^{15}$     | 258      |
| 842:88  | $0, 0, 0, 0, e^{12} a_1, e^{13}, e^{25} + e^{34} + e^{16}, e^{24} + e^{36} + e^{15}$ | 258      |
| 842:89  | $0, 0, 0, 0, e^{12}, e^{13}, e^{34}, e^{15}, e^{36}$                                 | 248      |
| 842:90  | $0, 0, 0, 0, e^{12}, e^{13}, e^{34}, e^{13} + e^{25}, e^{36}$                        | 248      |
| 842:91  | $0, 0, 0, 0, e^{12}, e^{13}, e^{34}, e^{15}, e^{23} + e^{46}$                        | 248      |
| 842:92  | $0, 0, 0, 0, e^{12}, e^{13}, e^{34}, e^{15}, e^{36} + e^{25}$                        | 248      |
| 842:93  | $0, 0, 0, 0, -e^{12}, e^{14} + e^{23}, e^{15}, e^{35} + e^{16}$                      | 248      |
| 842:94  | $0, 0, 0, 0, e^{12}, e^{24} + e^{13}, e^{15}, e^{26} + e^{35}$                       | 248      |
| 842:95  | $0, 0, 0, 0, e^{12}, e^{34}, e^{15} + e^{23}, e^{13} + e^{46}$                       | 248      |
| 842:96  | $0, 0, 0, 0, e^{12}, e^{34}, e^{15} + e^{23}, e^{36} + e^{14}$                       | 248      |
| 842:97  | $0, 0, 0, 0, e^{12}, e^{34}, e^{13} + e^{25}, e^{36} + e^{15}$                       | 248      |
| 842:98  | $0, 0, 0, 0, e^{12}, e^{34}, e^{15}, e^{46} + e^{13} + e^{25}$                       | 248      |
| 842:99  | $0, 0, 0, 0, e^{12}, e^{34}, e^{13} + e^{25}, e^{15} + e^{46}$                       | 248      |
| 842:100 | $0, 0, 0, 0, e^{12}, e^{34}, e^{36} + e^{15}, e^{46} + e^{25}$                       | 248      |
| 842:101 | $0, 0, 0, 0, -e^{12}, e^{14} + e^{23}, e^{13} + e^{25}, e^{35} + e^{16}$             | 248      |
| 842:102 | $0, 0, 0, 0, e^{12}, e^{24} + e^{13}, e^{15}, e^{26} + e^{35} + e^{14}$              | 248      |
| 842:103 | $0, 0, 0, 0, -e^{12}, e^{24} + e^{13}, e^{15}, e^{45} + e^{16} + e^{23}$             | 248      |
| 842:104 | $0, 0, 0, 0, -e^{12}, e^{24} + e^{13}, e^{15} + e^{23}, e^{45} + e^{16}$             | 248      |
| 842:105 | $0, 0, 0, 0, -e^{12}, e^{14} + e^{23}, e^{34} + e^{15}, e^{35} + e^{16}$             | 248      |
| 842:106 | $0, 0, 0, 0, e^{12}, e^{24} + e^{13}, e^{34} + e^{15}, e^{26} + e^{35}$              | 248      |
| 842:107 | $0, 0, 0, 0, -e^{12}, -e^{14} + e^{23}, e^{35} + e^{16}, e^{26} + e^{45}$            | 248      |

Table 1 – Continued to next page

Table 1 – Continued from previous page

| Name      | g                                                                                                   | UCS Dim. |
|-----------|-----------------------------------------------------------------------------------------------------|----------|
| 842:108a  | $0, 0, 0, 0, e^{12}, e^{34}, e^{13} + e^{25}, e^{46} + e^{15} + e^{23}$                             | 248      |
| 842:108b  | $0, 0, 0, 0, e^{12}, e^{34}, -e^{13} + e^{25}, e^{15} + e^{23} + e^{46}$                            | 248      |
| 842:109   | $0, 0, 0, 0, e^{12}, e^{34}, e^{13} + e^{25}, e^{24} + e^{36} + e^{15}$                             | 248      |
| 842:110   | $0, 0, 0, 0, e^{12}, e^{34}, e^{36} + e^{15}, e^{13} + e^{25} + e^{46}$                             | 248      |
| 842:111a  | $0, 0, 0, 0, e^{14} + e^{23}, e^{24} + e^{13}, e^{25} + e^{16}, e^{26} + e^{15}$                    | 248      |
| 842:111b  | $0, 0, 0, 0, -e^{14} + e^{23}, e^{24} + e^{13}, e^{25} - e^{16}, e^{26} + e^{15}$                   | 248      |
| 842:112a  | $0, 0, 0, 0, e^{14} + e^{23}, e^{24} + e^{13}, e^{26} + e^{15}, e^{46} + e^{35}$                    | 248      |
| 842:112b  | $0, 0, 0, 0, -e^{14} - e^{23}, e^{24} - e^{13}, e^{26} + e^{15}, e^{35} + e^{46}$                   | 248      |
| 842:113   | $0, 0, 0, 0, -e^{12}, e^{14} + e^{23}, e^{13} + e^{25}, e^{24} + e^{35} + e^{16}$                   | 248      |
| 842:114a  | $0, 0, 0, 0, e^{12}, e^{24} + e^{13}, e^{34} + e^{15}, e^{26} + e^{35} + e^{14}$                    | 248      |
| 842:114b  | $0, 0, 0, 0, e^{12}, e^{24} + e^{13}, e^{34} - e^{15}, e^{26} + e^{35} + e^{14}$                    | 248      |
| 842:115   | $0, 0, 0, 0, -e^{12}, e^{24} + e^{13}, e^{34} + e^{15}, e^{16} + e^{23} + e^{45}$                   | 248      |
| 842:116   | $0, 0, 0, 0, -e^{12}, -e^{14} + e^{23}, e^{35} + e^{16}, e^{13} + e^{26} + e^{45}$                  | 248      |
| 842:117   | $0, 0, 0, 0, e^{12}, e^{34}, e^{24} + e^{36} + e^{15}, e^{46} + e^{13} + e^{25}$                    | 248      |
| 842:118a  | $0, 0, 0, 0, e^{14} + e^{23}, e^{24} + e^{13}, e^{26} + e^{15}, e^{12} + e^{35} + e^{46}$           | 248      |
| 842:118b  | $0, 0, 0, 0, -e^{14} - e^{23}, e^{24} - e^{13}, e^{26} + e^{15}, e^{46} + e^{12} + e^{35}$          | 248      |
| 842:119a  | $0, 0, 0, 0, e^{14} + e^{23}, e^{24} + e^{13}, e^{26} + e^{15}, e^{25} + e^{34} + e^{16}$           | 248      |
| 842:119b  | $0, 0, 0, 0, e^{14} + e^{23}, e^{24} - e^{13}, e^{26} - e^{15}, e^{25} + e^{34} + e^{16}$           | 248      |
| 842:120   | $0, 0, 0, 0, -e^{12}, e^{24} - e^{13}, e^{16} + e^{23} + e^{45}, e^{26} + e^{35} + e^{14}$          | 248      |
| 842:121a  | $0, 0, 0, 0, -e^{24} + e^{13}, e^{12} + e^{34}, e^{36} + e^{25} + e^{14}, e^{46} + e^{15} + e^{23}$ | 248      |
| 842:121b  | $0, 0, 0, 0, e^{24} - e^{13}, -e^{12} + e^{34}, e^{36} + e^{25} + e^{14}, e^{15} + e^{23} + e^{46}$ | 248      |
| Type: 431 |                                                                                                     |          |
| 841:1     | $0, 0, 0, 0, e^{12}, e^{13}, e^{23}, e^{15}$                                                        | 468      |
| 841:2     | $0, 0, 0, 0, e^{12}, e^{13}, e^{34}, e^{15}$                                                        | 368      |
| 841:3     | $0, 0, 0, 0, e^{12}, e^{13}, e^{34}, e^{25}$                                                        | 368      |
| 841:4     | $0, 0, 0, 0, e^{12}, e^{13}, e^{14}, e^{15}$                                                        | 368      |
| 841:5     | $0, 0, 0, 0, e^{12}, e^{13}, e^{14}, e^{25}$                                                        | 368      |
| 841:6     | $0, 0, 0, 0, e^{12}, e^{13}, e^{24}, e^{15}$                                                        | 368      |
| 841:7     | $0, 0, 0, 0, e^{12}, e^{34}, e^{24} + e^{13}, e^{15}$                                               | 368      |
| 841:8     | $0, 0, 0, 0, e^{12}, e^{13}, e^{23}, e^{34} + e^{15}$                                               | 368      |
| 841:9     | $0, 0, 0, 0, e^{12}, e^{13}, e^{14} + e^{23}, e^{15}$                                               | 368      |
| 841:10    | $0, 0, 0, 0, e^{12}, e^{13}, e^{14} + e^{23}, e^{25}$                                               | 368      |
| 841:11    | $0, 0, 0, 0, e^{12}, e^{13}, e^{34}, e^{15} + e^{23}$                                               | 368      |
| 841:12    | $0, 0, 0, 0, e^{12}, e^{13}, e^{14}, e^{34} + e^{15}$                                               | 368      |
| 841:13    | $0, 0, 0, 0, e^{12}, e^{13}, e^{14}, e^{25} + e^{34}$                                               | 368      |
| 841:14    | $0, 0, 0, 0, e^{12}, e^{13}, e^{24}, e^{34} + e^{15}$                                               | 368      |
| 841:15    | $0, 0, 0, 0, e^{12}, e^{13}, e^{34}, e^{25} + e^{14}$                                               | 368      |
| 841:16    | $0, 0, 0, 0, e^{12}, e^{13}, e^{34}, e^{24} + e^{15}$                                               | 368      |
| 841:17    | $0, 0, 0, 0, e^{12}, e^{13}, e^{23}, e^{25} + e^{14}$                                               | 368      |
| 841:18    | $0, 0, 0, 0, e^{12}, e^{13}, e^{14}, e^{15} + e^{23}$                                               | 368      |
| 841:19    | $0, 0, 0, 0, e^{12}, e^{13}, e^{24}, e^{15} + e^{23}$                                               | 368      |
| 841:20    | $0, 0, 0, 0, e^{12}, e^{13}, e^{14} + e^{23}, e^{34} + e^{15}$                                      | 368      |
| 841:21    | $0, 0, 0, 0, e^{12}, e^{13}, e^{14} + e^{23}, e^{25} + e^{34}$                                      | 368      |
| 841:22a   | $0, 0, 0, 0, e^{12}, e^{14} + e^{23}, e^{24} + e^{13}, e^{15}$                                      | 368      |
| 841:22b   | $0, 0, 0, 0, e^{12}, -e^{14} + e^{23}, e^{24} + e^{13}, e^{15}$                                     | 368      |
| 841:23    | $0, 0, 0, 0, e^{12}, e^{34}, e^{14} + e^{23}, e^{13} + e^{25}$                                      | 368      |
| 841:24    | $0, 0, 0, 0, e^{12}, e^{13}, e^{14} + e^{23}, e^{24} + e^{15}$                                      | 368      |
| 841:25a   | $0, 0, 0, 0, e^{12}, e^{14} + e^{23}, e^{24} + e^{13}, e^{34} + e^{15}$                             | 368      |
| 841:25b   | $0, 0, 0, 0, e^{12}, -e^{14} + e^{23}, e^{24} + e^{13}, e^{34} + e^{15}$                            | 368      |
| 841:26    | $0, 0, 0, 0, e^{12}, e^{13}, e^{23}, e^{25} + e^{16}$                                               | 358      |
| 841:27a   | $0, 0, 0, 0, e^{12}, e^{13}, e^{23}, e^{36} + e^{25}$                                               | 358      |
| 841:27b   | $0, 0, 0, 0, -e^{12}, e^{13}, e^{23}, e^{36} + e^{25}$                                              | 358      |
| 841:28    | $0, 0, 0, 0, e^{12}, e^{13}, e^{23}, e^{26} + e^{35}$                                               | 358      |
| 841:29    | $0, 0, 0, 0, e^{12}, e^{13}, e^{14}, e^{25} + e^{16}$                                               | 258      |
| 841:30    | $0, 0, 0, 0, e^{12}, e^{13}, e^{24}, e^{25} + e^{16}$                                               | 258      |
| 841:31a   | $0, 0, 0, 0, e^{12}, e^{13}, e^{14}, e^{36} + e^{25}$                                               | 258      |
| 841:31b   | $0, 0, 0, 0, -e^{12}, e^{13}, e^{14}, e^{36} + e^{25}$                                              | 258      |
| 841:32    | $0, 0, 0, 0, e^{12}, e^{13}, e^{14}, e^{26} + e^{35}$                                               | 258      |

Table 1 – Continued to next page

Table 1 – Continued from previous page

| Name    | g                                                                                      | UCS Dim. |
|---------|----------------------------------------------------------------------------------------|----------|
| 841:33  | $0, 0, 0, 0, e^{12}, e^{13}, e^{24}, e^{36} + e^{15}$                                  | 258      |
| 841:34a | $0, 0, 0, 0, e^{12}, e^{13}, e^{24}, e^{36} + e^{25}$                                  | 258      |
| 841:34b | $0, 0, 0, 0, -e^{12}, e^{13}, e^{24}, e^{36} + e^{25}$                                 | 258      |
| 841:35  | $0, 0, 0, 0, e^{12}, e^{13}, e^{24}, e^{26} + e^{35}$                                  | 258      |
| 841:36  | $0, 0, 0, 0, e^{12}, e^{13}, e^{14} + e^{23}, e^{25} + e^{16}$                         | 258      |
| 841:37a | $0, 0, 0, 0, e^{12}, e^{13}, e^{14} + e^{23}, e^{36} + e^{25}$                         | 258      |
| 841:37b | $0, 0, 0, 0, -e^{12}, e^{13}, e^{14} + e^{23}, e^{36} + e^{25}$                        | 258      |
| 841:38  | $0, 0, 0, 0, e^{12}, e^{13}, e^{14} + e^{23}, e^{26} + e^{35}$                         | 258      |
| 841:39  | $0, 0, 0, 0, e^{12}, e^{13}, e^{14}, e^{24} + e^{36} + e^{15}$                         | 258      |
| 841:40a | $0, 0, 0, 0, e^{12}, e^{13}, e^{24}, e^{36} + e^{25} + e^{14}$                         | 258      |
| 841:40b | $0, 0, 0, 0, -e^{12}, e^{13}, e^{24}, e^{36} + e^{25} + e^{14}$                        | 258      |
| 841:41  | $0, 0, 0, 0, e^{12}, e^{13}, e^{24}, e^{26} + e^{35} + e^{14}$                         | 258      |
| 841:42  | $0, 0, 0, 0, e^{12}, e^{13}, e^{24}, e^{25} + e^{34} + e^{16}$                         | 258      |
| 841:43a | $0, 0, 0, 0, e^{12}, e^{13}, e^{23}, e^{36} + e^{25} + e^{14}$                         | 258      |
| 841:43b | $0, 0, 0, 0, -e^{12}, e^{13}, e^{23}, e^{36} + e^{25} + e^{14}$                        | 258      |
| 841:44  | $0, 0, 0, 0, e^{12}, e^{13}, e^{23}, e^{24} + e^{36} + e^{15}$                         | 258      |
| 841:45  | $0, 0, 0, 0, e^{12}, e^{13}, e^{23}, e^{26} + e^{35} + e^{14}$                         | 258      |
| 841:46  | $0, 0, 0, 0, e^{12}, e^{13}, e^{14} + e^{23}, e^{24} + e^{36} + e^{15}$                | 258      |
| 841:47  | $0, 0, 0, 0, e^{12}, e^{13}, e^{23}, e^{25} + e^{37} + e^{16}$                         | 258      |
| 841:48  | $0, 0, 0, 0, (-1 + a_2)e^{12}, e^{13}, a_2, e^{23}, e^{26} + e^{35} + e^{17}$          | 258      |
| 841:49  | $0, 0, 0, 0, e^{12}, e^{34}, e^{13}, e^{36} + e^{15}$                                  | 248      |
| 841:50  | $0, 0, 0, 0, e^{12}, e^{34}, e^{13}, e^{36} + e^{25}$                                  | 248      |
| 841:51  | $0, 0, 0, 0, e^{12}, e^{34}, e^{13}, e^{25} + e^{46}$                                  | 248      |
| 841:52  | $0, 0, 0, 0, e^{12}, e^{34}, e^{24} + e^{13}, e^{36} + e^{15}$                         | 248      |
| 841:53  | $0, 0, 0, 0, e^{12}, e^{34}, e^{14} + e^{23}, e^{36} + e^{15}$                         | 248      |
| 841:54  | $0, 0, 0, 0, -e^{12}, e^{14} + e^{23}, e^{13}, e^{35} + e^{16}$                        | 248      |
| 841:55  | $0, 0, 0, 0, e^{12}, e^{14} + e^{23}, e^{13}, e^{45} + e^{26}$                         | 248      |
| 841:56  | $0, 0, 0, 0, -e^{12}, e^{14} + e^{23}, e^{34}, e^{35} + e^{16}$                        | 248      |
| 841:57  | $0, 0, 0, 0, e^{12}, e^{34}, e^{13}, e^{46} + e^{15} + e^{23}$                         | 248      |
| 841:58  | $0, 0, 0, 0, e^{12}, e^{34}, e^{13}, e^{24} + e^{36} + e^{15}$                         | 248      |
| 841:59a | $0, 0, 0, 0, -e^{12}, e^{14} + e^{23}, e^{24} + e^{13}, e^{35} + e^{16}$               | 248      |
| 841:59b | $0, 0, 0, 0, -e^{12}, -e^{14} + e^{23}, e^{24} + e^{13}, e^{35} + e^{16}$              | 248      |
| 841:60a | $0, 0, 0, 0, e^{14} + e^{23}, e^{24} + e^{13}, e^{12}, e^{26} + e^{15}$                | 248      |
| 841:60b | $0, 0, 0, 0, -e^{14} + e^{23}, e^{24} + e^{13}, e^{12}, e^{26} + e^{15}$               | 248      |
| 841:61a | $0, 0, 0, 0, e^{14} + e^{23}, e^{24} + e^{13}, e^{12}, e^{46} + e^{35}$                | 248      |
| 841:61b | $0, 0, 0, 0, e^{14} - e^{23}, e^{24} + e^{13}, e^{12}, e^{46} + e^{35}$                | 248      |
| 841:62  | $0, 0, 0, 0, e^{12}, e^{34}, e^{24} + e^{13}, e^{46} + e^{15} + e^{23}$                | 248      |
| 841:63  | $0, 0, 0, 0, -e^{12}, e^{14} + e^{23}, e^{13}, e^{24} + e^{35} + e^{16}$               | 248      |
| 841:64  | $0, 0, 0, 0, e^{12}, e^{24} + e^{13}, e^{34}, e^{26} + e^{35} + e^{14}$                | 248      |
| 841:65a | $0, 0, 0, 0, e^{14} + e^{23}, e^{24} + e^{13}, e^{12} + e^{34}, e^{26} + e^{15}$       | 248      |
| 841:65b | $0, 0, 0, 0, -e^{14} + e^{23}, e^{24} + e^{13}, e^{12} + e^{34}, e^{26} + e^{15}$      | 248      |
| 841:65c | $0, 0, 0, 0, -e^{14} + e^{23}, e^{24} + e^{13}, -e^{12} + e^{34}, e^{26} + e^{15}$     | 248      |
| 841:66a | $0, 0, 0, 0, e^{14} + e^{23}, e^{24} + e^{13}, e^{12}, e^{26} + e^{34} + e^{15}$       | 248      |
| 841:66b | $0, 0, 0, 0, -e^{14} + e^{23}, e^{24} + e^{13}, e^{12}, e^{26} + e^{34} + e^{15}$      | 248      |
| 841:67a | $0, 0, 0, 0, e^{12}, e^{13}, e^{14}, e^{36} + e^{25} + e^{17}$                         | 148      |
| 841:67b | $0, 0, 0, 0, -e^{12}, e^{13}, e^{14}, e^{36} + e^{25} + e^{17}$                        | 148      |
| 841:68  | $0, 0, 0, 0, e^{12}, e^{13}, e^{14}, e^{26} + e^{35} + e^{17}$                         | 148      |
| 841:69  | $0, 0, 0, 0, e^{12}, e^{13}, e^{24}, e^{36} + e^{27} + e^{15}$                         | 148      |
| 841:70a | $0, 0, 0, 0, e^{12}, e^{13}, e^{14}, e^{47} + e^{36} + e^{25}$                         | 148      |
| 841:70b | $0, 0, 0, 0, e^{12}, -e^{13}, e^{14}, e^{36} + e^{25} + e^{47}$                        | 148      |
| 841:71  | $0, 0, 0, 0, e^{12}, e^{13}, e^{14}, e^{47} + e^{26} + e^{35}$                         | 148      |
| 841:72a | $0, 0, 0, 0, e^{12}, e^{13}, e^{24}, e^{47} + e^{36} + e^{15}$                         | 148      |
| 841:72b | $0, 0, 0, 0, -e^{12}, e^{13}, e^{24}, e^{36} + e^{15} + e^{47}$                        | 148      |
| 841:73  | $0, 0, 0, 0, -e^{12}, e^{13}, e^{24}, e^{36} + e^{17} + e^{45}$                        | 148      |
| 841:74  | $0, 0, 0, 0, (-1 + a_2)e^{12}, e^{13}, a_2, e^{14} + e^{23}, e^{26} + e^{35} + e^{17}$ | 148      |
| 841:75a | $0, 0, 0, 0, e^{12}, e^{13}, e^{14} + e^{23}, e^{27} + e^{16} + e^{45}$                | 148      |
| 841:75b | $0, 0, 0, 0, e^{12}, -e^{13}, e^{14} + e^{23}, e^{27} + e^{16} + e^{45}$               | 148      |
| 841:76  | $0, 0, 0, 0, e^{12}, e^{13}, e^{14} + e^{23}, e^{25} + e^{37} + e^{46}$                | 148      |

Table 1 – Continued to next page

Table 1 – Continued from previous page

| Name       | g                                                                                                     | UCS Dim. |
|------------|-------------------------------------------------------------------------------------------------------|----------|
| 841:77     | $0, 0, 0, 0, e^{12}, e^{34}, e^{24} + e^{13}, e^{37} + e^{26} + e^{15}$                               | 148      |
| 841:78a    | $0, 0, 0, 0, (-1 + a_2)e^{12}, e^{14} + e^{23}, e^{24} + a_2e^{13}, e^{27} + e^{35} + e^{16}$         | 148      |
| 841:78b    | $0, 0, 0, 0, (-1 + a_2)e^{12}, -e^{14} + e^{23}, e^{24} + a_2e^{13}, e^{27} + e^{35} + e^{16}$        | 148      |
| 841:79a    | $0, 0, 0, 0, e^{12}, e^{14} + e^{23}, e^{24} + e^{13}, e^{36} + e^{15} + e^{47}$                      | 148      |
| 841:79b    | $0, 0, 0, 0, e^{12}, e^{14} - e^{23}, e^{24} + e^{13}, e^{36} + e^{15} + e^{47}$                      | 148      |
| 841:79c    | $0, 0, 0, 0, -e^{12}, e^{14} + e^{23}, e^{24} + e^{13}, e^{36} + e^{15} + e^{47}$                     | 148      |
| 841:80a    | $0, 0, 0, 0, e^{12}, e^{14} + e^{23}, e^{24} + e^{13}, e^{37} + e^{15} + e^{46}$                      | 148      |
| 841:80b    | $0, 0, 0, 0, e^{12}, -e^{14} + e^{23}, e^{24} + e^{13}, e^{37} + e^{15} + e^{46}$                     | 148      |
| 841:81a    | $0, 0, 0, 0, e^{14} + e^{23}, (1 + a_2)e^{13} + e^{24}, a_2e^{12} + e^{34}, e^{37} + e^{26} + e^{15}$ | 148      |
| 841:81b    | $0, 0, 0, 0, e^{14} + e^{23}, (1 + a_2)e^{13} - e^{24}, a_2e^{12} + e^{34}, e^{37} + e^{26} + e^{15}$ | 148      |
| Type: 44   |                                                                                                       |          |
| 84:1       | $0, 0, 0, 0, e^{12}, e^{13}, e^{23}, e^{14}$                                                          | 48       |
| 84:2       | $0, 0, 0, 0, e^{12}, e^{13}, e^{24}, e^{34}$                                                          | 48       |
| 84:3       | $0, 0, 0, 0, e^{12}, e^{13}, e^{24}, e^{14} + e^{23}$                                                 | 48       |
| 84:4a      | $0, 0, 0, 0, e^{12}, e^{34}, e^{14} + e^{23}, e^{24} + e^{13}$                                        | 48       |
| 84:4b      | $0, 0, 0, 0, e^{12}, e^{34}, -e^{14} + e^{23}, e^{24} + e^{13}$                                       | 48       |
| Type: 5111 |                                                                                                       |          |
| 8321:1     | $0, 0, 0, 0, 0, e^{12}, e^{16}, e^{17}$                                                               | 4568     |
| 8321:2     | $0, 0, 0, 0, 0, e^{12}, e^{16}, e^{34} + e^{17}$                                                      | 2568     |
| 8321:3     | $0, 0, 0, 0, 0, e^{12}, e^{16}, e^{17} + e^{23}$                                                      | 3568     |
| 8321:4     | $0, 0, 0, 0, 0, e^{12}, e^{16}, e^{26} + e^{17}$                                                      | 4568     |
| 8321:5     | $0, 0, 0, 0, 0, e^{12}, e^{16}, e^{17} + e^{23} + e^{45}$                                             | 1568     |
| 8321:6     | $0, 0, 0, 0, 0, e^{12}, e^{16}, e^{26} + e^{34} + e^{17}$                                             | 2568     |
| 8321:7     | $0, 0, 0, 0, 0, -e^{12}, e^{16} + e^{23}, e^{36} + e^{17}$                                            | 3468     |
| 8321:8     | $0, 0, 0, 0, 0, -e^{12}, e^{16} + e^{23}, e^{45} + e^{36} + e^{17}$                                   | 1468     |
| 8321:9     | $0, 0, 0, 0, 0, e^{12}, e^{13} + e^{26}, e^{36} + e^{27} + e^{14}$                                    | 2468     |
| Type: 512  |                                                                                                       |          |
| 832:1      | $0, 0, 0, 0, 0, e^{12}, e^{16}, e^{26}$                                                               | 568      |
| 832:2      | $0, 0, 0, 0, 0, e^{12}, e^{16}, e^{13} + e^{26}$                                                      | 468      |
| 832:3      | $0, 0, 0, 0, 0, e^{12}, e^{16}, e^{26} + e^{34}$                                                      | 368      |
| 832:4a     | $0, 0, 0, 0, 0, e^{12}, e^{16} + e^{23}, e^{13} + e^{26}$                                             | 468      |
| 832:4b     | $0, 0, 0, 0, 0, e^{12}, -e^{16} + e^{23}, e^{13} + e^{26}$                                            | 468      |
| 832:5      | $0, 0, 0, 0, 0, e^{12}, e^{13} + e^{26}, e^{34} + e^{16}$                                             | 368      |
| 832:6      | $0, 0, 0, 0, 0, e^{12}, e^{34} + e^{16}, e^{26} + e^{35}$                                             | 268      |
| 832:7      | $0, 0, 0, 0, 0, e^{12}, e^{16} + e^{23}, e^{26} + e^{14}$                                             | 368      |
| 832:8      | $0, 0, 0, 0, 0, e^{12}, e^{16}, e^{13} + e^{26} + e^{45}$                                             | 268      |
| 832:9      | $0, 0, 0, 0, 0, e^{12}, e^{13} + e^{26}, e^{45} + e^{16}$                                             | 268      |
| 832:10     | $0, 0, 0, 0, 0, e^{12}, e^{34} + e^{16}, e^{13} + e^{26} + e^{45}$                                    | 268      |
| 832:11a    | $0, 0, 0, 0, 0, e^{12}, e^{13} + e^{26}, e^{45} + e^{16} + e^{23}$                                    | 268      |
| 832:11b    | $0, 0, 0, 0, 0, e^{12}, -e^{13} + e^{26}, e^{16} + e^{23} + e^{45}$                                   | 268      |
| 832:12     | $0, 0, 0, 0, 0, e^{12}, e^{13} + e^{26}, e^{24} + e^{35} + e^{16}$                                    | 268      |
| 832:13     | $0, 0, 0, 0, 0, e^{12}, e^{24} + e^{35} + e^{16}, e^{13} + e^{26} + e^{45}$                           | 268      |
| Type: 521  |                                                                                                       |          |
| 831:1      | $0, 0, 0, 0, 0, e^{12}, e^{13}, e^{16}$                                                               | 468      |
| 831:2      | $0, 0, 0, 0, 0, e^{12}, e^{13}, e^{26}$                                                               | 468      |
| 831:3      | $0, 0, 0, 0, 0, e^{12}, e^{34}, e^{16}$                                                               | 368      |
| 831:4      | $0, 0, 0, 0, 0, e^{12}, e^{13}, e^{16} + e^{23}$                                                      | 468      |
| 831:5      | $0, 0, 0, 0, 0, e^{12}, e^{13}, e^{34} + e^{16}$                                                      | 368      |
| 831:6      | $0, 0, 0, 0, 0, e^{12}, e^{13}, e^{26} + e^{34}$                                                      | 368      |
| 831:7      | $0, 0, 0, 0, 0, e^{12}, e^{24} + e^{13}, e^{16}$                                                      | 368      |
| 831:8      | $0, 0, 0, 0, 0, e^{12}, e^{34}, e^{13} + e^{26}$                                                      | 368      |
| 831:9      | $0, 0, 0, 0, 0, e^{12}, e^{34}, e^{35} + e^{16}$                                                      | 268      |
| 831:10     | $0, 0, 0, 0, 0, e^{12}, e^{13} + e^{45}, e^{16}$                                                      | 268      |
| 831:11     | $0, 0, 0, 0, 0, e^{12}, e^{45} + e^{13}, e^{26}$                                                      | 268      |
| 831:12     | $0, 0, 0, 0, 0, e^{12}, e^{13}, e^{26} + e^{14}$                                                      | 368      |
| 831:13     | $0, 0, 0, 0, 0, e^{12}, e^{13}, e^{24} + e^{16}$                                                      | 368      |
| 831:14     | $0, 0, 0, 0, 0, e^{12}, e^{13}, e^{16} + e^{45}$                                                      | 268      |
| 831:15     | $0, 0, 0, 0, 0, e^{12}, e^{13}, e^{45} + e^{26}$                                                      | 268      |

Table 1 – Continued to next page

Table 1 – Continued from previous page

| Name     | g                                                                            | UCS Dim. |
|----------|------------------------------------------------------------------------------|----------|
| 831:16   | $0, 0, 0, 0, 0, e^{12}, e^{34}, e^{26} + e^{15}$                             | 268      |
| 831:17   | $0, 0, 0, 0, 0, e^{12}, e^{24} + e^{13}, e^{34} + e^{16}$                    | 368      |
| 831:18   | $0, 0, 0, 0, 0, e^{12}, e^{13} + e^{45}, e^{34} + e^{16}$                    | 268      |
| 831:19   | $0, 0, 0, 0, 0, e^{12}, e^{45} + e^{13}, e^{26} + e^{34}$                    | 268      |
| 831:20   | $0, 0, 0, 0, 0, e^{12}, e^{14} + e^{23}, e^{13} + e^{26}$                    | 368      |
| 831:21   | $0, 0, 0, 0, 0, e^{12}, e^{24} + e^{13}, e^{35} + e^{16}$                    | 268      |
| 831:22   | $0, 0, 0, 0, 0, e^{12}, e^{14} + e^{23}, e^{35} + e^{16}$                    | 268      |
| 831:23   | $0, 0, 0, 0, 0, e^{12}, e^{34}, e^{45} + e^{13} + e^{26}$                    | 268      |
| 831:24   | $0, 0, 0, 0, 0, e^{12}, e^{35} + e^{14}, e^{13} + e^{26}$                    | 268      |
| 831:25   | $0, 0, 0, 0, 0, e^{12}, e^{45} + e^{13}, e^{16} + e^{23}$                    | 268      |
| 831:26   | $0, 0, 0, 0, 0, e^{12}, e^{35} + e^{14}, e^{16} + e^{23}$                    | 268      |
| 831:27   | $0, 0, 0, 0, 0, e^{12}, e^{13}, e^{26} + e^{35} + e^{14}$                    | 268      |
| 831:28   | $0, 0, 0, 0, 0, e^{12}, e^{13}, e^{16} + e^{23} + e^{45}$                    | 268      |
| 831:29   | $0, 0, 0, 0, 0, e^{12}, e^{13}, e^{24} + e^{35} + e^{16}$                    | 268      |
| 831:30   | $0, 0, 0, 0, 0, e^{12}, e^{24} + e^{13}, e^{26} + e^{15}$                    | 268      |
| 831:31a  | $0, 0, 0, 0, 0, e^{12}, e^{45} + e^{13}, e^{26} + e^{35} + e^{14}$           | 268      |
| 831:31b  | $0, 0, 0, 0, 0, e^{12}, -e^{13} + e^{45}, e^{26} + e^{35} + e^{14}$          | 268      |
| 831:32   | $0, 0, 0, 0, 0, e^{12}, e^{45} + e^{13}, e^{24} + e^{35} + e^{16}$           | 268      |
| 831:33   | $0, 0, 0, 0, 0, e^{12}, e^{24} + e^{13}, e^{26} + e^{35} + e^{14}$           | 268      |
| 831:34   | $0, 0, 0, 0, 0, e^{12}, e^{24} + e^{13}, e^{26} + e^{34} + e^{15}$           | 268      |
| 831:35   | $0, 0, 0, 0, 0, e^{12}, e^{13}, e^{26} + e^{17}$                             | 358      |
| 831:36a  | $0, 0, 0, 0, 0, e^{12}, e^{13}, e^{37} + e^{26}$                             | 358      |
| 831:36b  | $0, 0, 0, 0, 0, -e^{12}, e^{13}, e^{37} + e^{26}$                            | 358      |
| 831:37   | $0, 0, 0, 0, 0, e^{12}, e^{13}, e^{36} + e^{27}$                             | 358      |
| 831:38a  | $0, 0, 0, 0, 0, e^{12}, e^{13}, e^{37} + e^{26} + e^{14}$                    | 258      |
| 831:38b  | $0, 0, 0, 0, 0, -e^{12}, e^{13}, e^{37} + e^{26} + e^{14}$                   | 258      |
| 831:39   | $0, 0, 0, 0, 0, e^{12}, e^{13}, e^{24} + e^{37} + e^{16}$                    | 258      |
| 831:40   | $0, 0, 0, 0, 0, e^{12}, e^{13}, e^{36} + e^{27} + e^{14}$                    | 258      |
| 831:41   | $0, 0, 0, 0, 0, e^{12}, e^{13}, e^{26} + e^{17} + e^{45}$                    | 158      |
| 831:42a  | $0, 0, 0, 0, 0, e^{12}, e^{13}, e^{45} + e^{37} + e^{26}$                    | 158      |
| 831:42b  | $0, 0, 0, 0, 0, -e^{12}, e^{13}, e^{37} + e^{26} + e^{45}$                   | 158      |
| 831:43   | $0, 0, 0, 0, 0, e^{12}, e^{13}, e^{45} + e^{36} + e^{27}$                    | 158      |
| 831:44   | $0, 0, 0, 0, 0, e^{12}, e^{34}, e^{37} + e^{16}$                             | 248      |
| 831:45   | $0, 0, 0, 0, 0, -e^{12}, e^{14} + e^{23}, e^{36} + e^{17}$                   | 248      |
| 831:46   | $0, 0, 0, 0, 0, e^{12}, e^{34}, e^{13} + e^{26} + e^{47}$                    | 248      |
| 831:47   | $0, 0, 0, 0, 0, e^{12}, e^{34}, e^{37} + e^{26} + e^{15}$                    | 148      |
| 831:48a  | $0, 0, 0, 0, 0, e^{14} + e^{23}, e^{24} + e^{13}, e^{27} + e^{16}$           | 248      |
| 831:48b  | $0, 0, 0, 0, 0, -e^{14} + e^{23}, e^{24} + e^{13}, e^{27} + e^{16}$          | 248      |
| 831:49   | $0, 0, 0, 0, 0, e^{12}, e^{24} + e^{13}, e^{36} + e^{27} + e^{14}$           | 248      |
| 831:50   | $0, 0, 0, 0, 0, e^{12}, e^{24} + e^{13}, e^{36} + e^{27} + e^{15}$           | 148      |
| 831:51   | $0, 0, 0, 0, 0, -e^{12}, e^{24} + e^{13}, e^{46} + e^{35} + e^{17}$          | 148      |
| 831:52a  | $0, 0, 0, 0, 0, e^{24} + e^{13}, -e^{12} + e^{34}, e^{47} + e^{16} + e^{23}$ | 248      |
| 831:52b  | $0, 0, 0, 0, 0, e^{24} - e^{13}, -e^{12} + e^{34}, e^{47} + e^{16} + e^{23}$ | 248      |
| 831:53a  | $0, 0, 0, 0, 0, e^{24} + e^{13}, e^{12} + e^{34}, e^{37} + e^{26} + e^{15}$  | 148      |
| 831:53b  | $0, 0, 0, 0, 0, -e^{24} + e^{13}, e^{12} + e^{34}, e^{37} + e^{26} + e^{15}$ | 148      |
| 831:54a  | $0, 0, 0, 0, 0, e^{24} + e^{13}, e^{12} + e^{34}, e^{36} + e^{27} + e^{15}$  | 148      |
| 831:54b  | $0, 0, 0, 0, 0, e^{24} - e^{13}, e^{12} + e^{34}, e^{36} + e^{27} + e^{15}$  | 148      |
| 831:55   | $0, 0, 0, 0, 0, e^{14} + e^{23}, e^{13} + e^{25}, e^{27} + e^{16}$           | 138      |
| 831:56   | $0, 0, 0, 0, 0, e^{24} + e^{13}, e^{12} + e^{35}, e^{37} + e^{26} + e^{14}$  | 138      |
| 831:57   | $0, 0, 0, 0, 0, e^{14} + e^{23}, e^{13} + e^{25}, e^{27} + e^{16} + e^{45}$  | 138      |
| Type: 53 |                                                                              |          |
| 83:1     | $0, 0, 0, 0, 0, e^{12}, e^{13}, e^{23}$                                      | 58       |
| 83:2     | $0, 0, 0, 0, 0, e^{12}, e^{13}, e^{14}$                                      | 48       |
| 83:3     | $0, 0, 0, 0, 0, e^{12}, e^{13}, e^{24}$                                      | 48       |
| 83:4     | $0, 0, 0, 0, 0, e^{12}, e^{13}, e^{14} + e^{23}$                             | 48       |
| 83:5     | $0, 0, 0, 0, 0, e^{12}, e^{34}, e^{24} + e^{13}$                             | 48       |
| 83:6a    | $0, 0, 0, 0, 0, e^{12}, e^{14} + e^{23}, e^{24} + e^{13}$                    | 48       |
| 83:6b    | $0, 0, 0, 0, 0, e^{12}, -e^{14} + e^{23}, e^{24} + e^{13}$                   | 48       |

Table 1 – Continued to next page



Table 1 – Continued from previous page

| Name      | g                                                                   | UCS Dim. |
|-----------|---------------------------------------------------------------------|----------|
| 83:7a     | $0, 0, 0, 0, 0, e^{14} + e^{23}, e^{24} + e^{13}, e^{12} + e^{34}$  | 48       |
| 83:7b     | $0, 0, 0, 0, 0, e^{14} + e^{23}, e^{24} - e^{13}, e^{12} + e^{34}$  | 48       |
| 83:8      | $0, 0, 0, 0, 0, e^{12}, e^{13}, e^{45}$                             | 38       |
| 83:9      | $0, 0, 0, 0, 0, e^{12}, e^{13}, e^{25} + e^{14}$                    | 38       |
| 83:10     | $0, 0, 0, 0, 0, e^{12}, e^{13}, e^{45} + e^{23}$                    | 38       |
| 83:11     | $0, 0, 0, 0, 0, e^{12}, e^{13}, e^{24} + e^{35}$                    | 38       |
| 83:12     | $0, 0, 0, 0, 0, e^{12}, e^{34}, e^{13} + e^{25}$                    | 38       |
| 83:13     | $0, 0, 0, 0, 0, e^{12}, e^{14} + e^{23}, e^{13} + e^{25}$           | 38       |
| 83:14     | $0, 0, 0, 0, 0, e^{12}, e^{14} + e^{23}, e^{45} + e^{13}$           | 38       |
| 83:15     | $0, 0, 0, 0, 0, e^{12}, e^{24} + e^{13}, e^{34} + e^{15}$           | 38       |
| 83:16a    | $0, 0, 0, 0, 0, e^{24} + e^{13}, e^{12} + e^{34}, e^{15}$           | 38       |
| 83:16b    | $0, 0, 0, 0, 0, e^{24} - e^{13}, e^{12} + e^{34}, e^{15}$           | 38       |
| 83:17     | $0, 0, 0, 0, 0, e^{12}, e^{35} + e^{14}, e^{45} + e^{23}$           | 38       |
| 83:18a    | $0, 0, 0, 0, 0, e^{14} + e^{23}, e^{24} + e^{13}, e^{12} + e^{35}$  | 38       |
| 83:18b    | $0, 0, 0, 0, 0, -e^{14} + e^{23}, e^{24} + e^{13}, e^{12} + e^{35}$ | 38       |
| 83:19     | $0, 0, 0, 0, 0, e^{14} + e^{23}, e^{13} + e^{25}, e^{12} + e^{45}$  | 38       |
| 83:20     | $0, 0, 0, 0, 0, e^{24} + e^{13}, e^{15} + e^{23}, e^{25} + e^{14}$  | 38       |
| Type: 611 |                                                                     |          |
| 821:1     | $0, 0, 0, 0, 0, 0, e^{12}, e^{17}$                                  | 568      |
| 821:2     | $0, 0, 0, 0, 0, 0, e^{12}, e^{13} + e^{27}$                         | 468      |
| 821:3     | $0, 0, 0, 0, 0, 0, e^{12}, e^{34} + e^{17}$                         | 368      |
| 821:4     | $0, 0, 0, 0, 0, 0, e^{12}, e^{45} + e^{13} + e^{27}$                | 268      |
| 821:5     | $0, 0, 0, 0, 0, 0, e^{12}, e^{34} + e^{17} + e^{56}$                | 168      |
| Type: 62  |                                                                     |          |
| 82:1      | $0, 0, 0, 0, 0, 0, e^{12}, e^{13}$                                  | 58       |
| 82:2      | $0, 0, 0, 0, 0, 0, e^{12}, e^{34}$                                  | 48       |
| 82:3      | $0, 0, 0, 0, 0, 0, e^{12}, e^{24} + e^{13}$                         | 48       |
| 82:4a     | $0, 0, 0, 0, 0, 0, e^{24} + e^{13}, e^{12} + e^{34}$                | 48       |
| 82:4b     | $0, 0, 0, 0, 0, 0, e^{24} - e^{13}, e^{12} + e^{34}$                | 48       |
| 82:5      | $0, 0, 0, 0, 0, 0, e^{12}, e^{13} + e^{45}$                         | 38       |
| 82:6      | $0, 0, 0, 0, 0, 0, e^{24} + e^{13}, e^{12} + e^{35}$                | 38       |
| 82:7      | $0, 0, 0, 0, 0, 0, e^{12}, e^{34} + e^{56}$                         | 28       |
| 82:8      | $0, 0, 0, 0, 0, 0, e^{12}, e^{56} + e^{24} + e^{13}$                | 28       |
| 82:9      | $0, 0, 0, 0, 0, 0, e^{24} + e^{13}, e^{12} + e^{56}$                | 28       |
| 82:10     | $0, 0, 0, 0, 0, 0, e^{24} + e^{13}, e^{26} + e^{15}$                | 28       |
| 82:11a    | $0, 0, 0, 0, 0, 0, e^{12} + e^{34}, e^{24} + e^{13} + e^{56}$       | 28       |
| 82:11b    | $0, 0, 0, 0, 0, 0, -e^{12} + e^{34}, e^{56} + e^{24} + e^{13}$      | 28       |
| 82:12     | $0, 0, 0, 0, 0, 0, e^{12} + e^{34}, e^{13} + e^{25} + e^{46}$       | 28       |
| 82:13     | $0, 0, 0, 0, 0, 0, e^{13} + e^{25}, e^{56} + e^{12} + e^{34}$       | 28       |
| Type: 71  |                                                                     |          |
| 81:1      | $0, 0, 0, 0, 0, 0, 0, e^{12}$                                       | 68       |
| 81:2      | $0, 0, 0, 0, 0, 0, 0, e^{12} + e^{34}$                              | 48       |
| 81:3      | $0, 0, 0, 0, 0, 0, 0, e^{12} + e^{34} + e^{56}$                     | 28       |
| Type: 8   |                                                                     |          |
| 8:1       | $0, 0, 0, 0, 0, 0, 0, 0$                                            | 8        |

End of Table 1

## B Table 2 9-dimensional nice nilpotent Lie algebras

Table 2: 9-dimensional nice nilpotent Lie algebras

| Name           | $\mathfrak{g}$                                                                                                                                                                                                                                                                                                                      | UCS Dim. |
|----------------|-------------------------------------------------------------------------------------------------------------------------------------------------------------------------------------------------------------------------------------------------------------------------------------------------------------------------------------|----------|
| Type: 21111111 |                                                                                                                                                                                                                                                                                                                                     |          |
| 97654321:1     | $0, 0, e^{12}, e^{13}, e^{14}, e^{15}, e^{16}, e^{17}, e^{18}$                                                                                                                                                                                                                                                                      | 12345679 |
| 97654321:2     | $0, 0, e^{12}, e^{13}, e^{14}, e^{15}, e^{16}, e^{17}, e^{23} + e^{18}$                                                                                                                                                                                                                                                             | 12345679 |
| 97654321:3     | $0, 0, e^{12}, e^{13}, e^{14}, e^{15}, e^{16}, e^{17} + e^{23}, e^{18} + e^{24}$                                                                                                                                                                                                                                                    | 12345679 |
| 97654321:4     | $0, 0, -e^{12}, e^{13}, e^{14}, e^{15}, e^{16}, e^{17}, e^{34} + e^{18} + e^{25}$                                                                                                                                                                                                                                                   | 12345679 |
| 97654321:5     | $0, 0, e^{12}, e^{13}, e^{14}, e^{15}, e^{16} + e^{23}, e^{17} + e^{24}, e^{18} + e^{25}$                                                                                                                                                                                                                                           | 12345679 |
| 97654321:6     | $0, 0, e^{12}, e^{13}, e^{14}, e^{15}, e^{23} + e^{16}, e^{24} + e^{17}, e^{18} + e^{34}$                                                                                                                                                                                                                                           | 12345679 |
| 97654321:8     | $0, 0, -e^{12}, -e^{13}, e^{14}, e^{15}, e^{16}, e^{17}, e^{18} + e^{27} + e^{45} + e^{36}$                                                                                                                                                                                                                                         | 12345679 |
| 97654321:9     | $0, 0, e^{12}, e^{13}, e^{14}, e^{15} + e^{23}, e^{16} + e^{24}, e^{17} + e^{25}, e^{18} + e^{26}$                                                                                                                                                                                                                                  | 12345679 |
| 97654321:12    | $0, 0, e^{12}a_1, e^{13}, -e^{14}(-1 + a_1), e^{15}, e^{23} + e^{16}, e^{24} + e^{17}, e^{34} + e^{25} + e^{18}$                                                                                                                                                                                                                    | 12345679 |
| 97654321:13    | $0, 0, -e^{12}, e^{13}, e^{14}, 2e^{15}, e^{16}, e^{17} + e^{25} + e^{34}, e^{35} + e^{18} + e^{26}$                                                                                                                                                                                                                                | 12345679 |
| 97654321:15    | $0, 0, e^{12}, e^{13}, e^{14}, e^{15} + e^{23}, e^{16} + e^{24}, 2e^{17} + e^{34} + e^{25}, e^{18} + e^{35}$                                                                                                                                                                                                                        | 12345679 |
| 97654321:16    | $0, 0, e^{12}, e^{13}, e^{14} + e^{23}, e^{15} + e^{24}, e^{16} + e^{25}, e^{17} + e^{26}, e^{18} + e^{27}$                                                                                                                                                                                                                         | 12345679 |
| 97654321:21    | $0, 0, e^{12}, e^{13}, e^{14}, -e^{15} + e^{23}, e^{16} + e^{24}, e^{17} + e^{34}, e^{18} + e^{35} + e^{26}$                                                                                                                                                                                                                        | 12345679 |
| 97654321:24    | $0, 0, e^{12}, 3e^{13}, -e^{14}, -2e^{15}, e^{16} + e^{34} + e^{25}, -e^{17} + e^{26} + e^{35}, e^{18} + e^{36} + e^{45}$                                                                                                                                                                                                           | 12345679 |
| 97654321:25    | $0, 0, (-1 + a_5)e^{12}, e^{13}, e^{14}, e^{23} - (-2 + a_5)e^{15}, e^{24} + e^{16}, e^{17}a_5 + e^{34} + e^{25}, e^{35} + e^{26} + e^{18}$                                                                                                                                                                                         | 12345679 |
| 97654321:31    | $0, 0, e^{12}, e^{13}, e^{14} - e^{23}, -e^{15} + e^{24}, e^{16} + e^{34}, e^{17} + e^{35} + e^{26}, e^{18} + e^{27} + e^{45}$                                                                                                                                                                                                      | 12345679 |
| 97654321:40    | $0, 0, e^{12}, \frac{1}{2}e^{13}, \frac{3}{2}e^{14} + e^{23}, \frac{1}{2}e^{15} + e^{24}, \frac{5}{2}e^{16} + e^{34} + e^{25}, \frac{3}{2}e^{17} + e^{35} + e^{26}, e^{18} + e^{36} + e^{45}$                                                                                                                                       | 12345679 |
| 97654321:42    | $0, 0, e^{12}, \frac{3}{5}e^{13}, e^{14} - 3e^{23}, \frac{2}{5}e^{15} - 2e^{24}, -e^{16} + e^{34} + e^{25}, e^{17} + e^{35}, e^{18} + e^{27} + e^{36} + e^{45}$                                                                                                                                                                     | 12345679 |
| 97654321:43(*) | $0, 0, -\frac{2(a_8-1)a_8}{(a_8+2)(2a_8-1)}e^{12}, \frac{a_8-1}{2a_8-1}e^{13}, \frac{3a_8^2}{(a_8+2)(2a_8-1)}e^{14} + (-1 + a_8)e^{23}, \frac{a_8}{2a_8-1}e^{15} + a_8e^{24},$<br>$\frac{5a_8-2}{2a_8^2+3a_8-2}e^{16} + e^{34} + e^{25}, \frac{3a_8^2}{(a_8+2)(2a_8-1)}e^{17} + e^{35} + e^{26}, e^{18} + e^{27} + e^{36} + e^{45}$ | 12345679 |
| Type: 2111112  |                                                                                                                                                                                                                                                                                                                                     |          |
| 9765432:1      | $0, 0, -e^{12}, -e^{13}, e^{14}, e^{15}, e^{16}, e^{17}, e^{27} + e^{45} + e^{36}$                                                                                                                                                                                                                                                  | 2345679  |
| 9765432:2      | $0, 0, -e^{12}, -e^{13}, e^{14}, e^{15}, e^{16}, e^{17} + e^{23}, e^{45} + e^{36} + e^{27}$                                                                                                                                                                                                                                         | 2345679  |
| 9765432:4      | $0, 0, -e^{12}, e^{13}, e^{14}, -e^{15}, e^{16} + e^{23}, e^{17} + e^{24}, e^{27} + e^{36} + e^{45}$                                                                                                                                                                                                                                | 2345679  |
| 9765432:5      | $0, 0, -e^{12}, -e^{13}, e^{14}, e^{15}, e^{16}, e^{17} + e^{34} + e^{25}, e^{27} + e^{45} + e^{36}$                                                                                                                                                                                                                                | 2345679  |
| 9765432:6      | $0, 0, -e^{12}, e^{13}, e^{14}, e^{23} - e^{15}, e^{24} + e^{16}, e^{17} + e^{25}, e^{36} + e^{45} + e^{27}$                                                                                                                                                                                                                        | 2345679  |
| 9765432:7      | $0, 0, e^{12}, -e^{13}, e^{14}, e^{15} + e^{23}, e^{24} - e^{16}, e^{34} + e^{17}, e^{36} + e^{27} + e^{45}$                                                                                                                                                                                                                        | 2345679  |
| 9765432:12     | $0, 0, -e^{12}a_1, e^{13}a_1, e^{14}(1 + a_1), e^{23} - e^{15}a_1, e^{24} + e^{16}a_1, e^{17} + e^{25} + e^{34}, e^{36} + e^{45} + e^{27}$                                                                                                                                                                                          | 2345679  |
| 9765432:16(*)  | $0, 0, -\frac{2}{3}e^{12}, -\frac{5}{3}e^{13}, -\frac{1}{2}e^{23} + e^{14}, \frac{5}{3}e^{15} + \frac{1}{2}e^{24}, \frac{2}{3}e^{16} + e^{25} + e^{34}, e^{26} + e^{17} + e^{35}, e^{45} + e^{27} + e^{36}$                                                                                                                         | 2345679  |
| Type: 2112111  |                                                                                                                                                                                                                                                                                                                                     |          |
| 9765421:1      | $0, 0, -e^{12}, e^{13}, e^{14}, e^{15}, e^{25} + e^{34}, e^{16}, e^{18}$                                                                                                                                                                                                                                                            | 2345679  |
| 9765421:2      | $0, 0, -e^{12}, e^{13}, e^{14}, e^{15}, e^{25} + e^{34}, e^{16}, e^{23} + e^{18}$                                                                                                                                                                                                                                                   | 2345679  |
| 9765421:3      | $0, 0, -e^{12}, e^{13}, e^{14}, e^{15}, e^{25} + e^{34}, e^{16} + e^{23}, e^{18} + e^{24}$                                                                                                                                                                                                                                          | 2345679  |
| 9765421:6      | $0, 0, -e^{12}, -e^{13}, e^{14}, e^{15}, e^{34} + e^{25}, e^{16}, e^{28} + e^{45} + e^{36}$                                                                                                                                                                                                                                         | 2345679  |
| 9765421:9      | $0, 0, -e^{12}, -e^{13}, e^{14}, e^{15}, e^{25} + e^{34}, e^{23} + e^{16}, e^{45} + e^{28} + e^{36}$                                                                                                                                                                                                                                | 2345679  |
| 9765421:13     | $0, 0, -e^{12}, e^{13}, e^{14}, e^{23} - e^{15}, e^{25} + e^{34}, e^{24} + e^{16}, e^{36} + e^{45} + e^{28}$                                                                                                                                                                                                                        | 2345679  |
| 9765421:16     | $0, 0, -e^{12}, e^{13}, e^{14}, e^{25} + e^{34}, 2e^{15}, e^{35} + e^{27} + e^{16}, e^{36} + e^{28}$                                                                                                                                                                                                                                | 1245679  |
| 9765421:18     | $0, 0, -e^{12}, e^{13}, e^{14}, e^{25} + e^{34}, e^{23} + 2e^{15}, e^{35} + e^{27} + e^{16}, e^{36} + e^{28}$                                                                                                                                                                                                                       | 1245679  |
| 9765421:19     | $0, 0, e^{12}, 3e^{13}, -e^{14}, -2e^{15}, e^{34} + e^{25}, e^{26} + e^{35} - e^{17}, e^{36} + e^{45} + e^{18}$                                                                                                                                                                                                                     | 1245679  |
| 9765421:20     | $0, 0, -e^{12}, e^{13}, e^{14}, 2e^{15}, e^{25} + e^{34}, e^{35} + e^{17} + e^{26}, e^{37} + e^{16} + e^{28}$                                                                                                                                                                                                                       | 1245679  |
| 9765421:21     | $0, 0, -e^{12}, 2e^{13}, e^{23} + e^{14}, e^{25} + e^{34}, e^{24} + 2e^{15}, e^{35} + e^{27} + e^{16}, e^{36} + e^{28}$                                                                                                                                                                                                             | 1245679  |
| 9765421:22     | $0, 0, e^{12}, 3e^{13}, -e^{14}, -2e^{15} + e^{23}, e^{34} + e^{25}, e^{26} + e^{35} - e^{17}, e^{36} + e^{45} + e^{18}$                                                                                                                                                                                                            | 1245679  |
| 9765421:25     | $0, 0, e^{12}, 3e^{13}, -e^{14} - \frac{3}{5}e^{23}, -2e^{15} + \frac{2}{5}e^{24}, e^{34} + e^{25}, e^{26} + e^{35} - e^{17}, e^{27} + e^{36} + e^{45} + e^{18}$                                                                                                                                                                    | 1245679  |
| Type: 2121111  |                                                                                                                                                                                                                                                                                                                                     |          |
| 9764321:1      | $0, 0, e^{12}, e^{13}, e^{23}, e^{14}, e^{16}, e^{17}, e^{18}$                                                                                                                                                                                                                                                                      | 2345679  |
| 9764321:2      | $0, 0, e^{12}, e^{13}, e^{23}, e^{14}, e^{16}, e^{17}, e^{25} + e^{18}$                                                                                                                                                                                                                                                             | 1345679  |
| 9764321:3a     | $0, 0, e^{12}, e^{13}, e^{23}, e^{14}, e^{16}, e^{25} + e^{17}, e^{18} + e^{35}$                                                                                                                                                                                                                                                    | 1245679  |
| 9764321:3b     | $0, 0, e^{12}, -e^{13}, e^{23}, e^{14}, e^{16}, e^{17} + e^{25}, e^{18} + e^{35}$                                                                                                                                                                                                                                                   | 1245679  |
| 9764321:4      | $0, 0, -e^{12}, e^{13}, e^{23}, e^{14}, e^{16}, e^{17}, e^{18} + e^{26} + e^{34}$                                                                                                                                                                                                                                                   | 2345679  |
| 9764321:5      | $0, 0, -e^{12}, -e^{13}, e^{23}, e^{14}, e^{16}, e^{17}, e^{28} + e^{37} + e^{46}$                                                                                                                                                                                                                                                  | 2345679  |
| 9764321:6a     | $0, 0, -e^{12}, -e^{13}, e^{23}, e^{14}, e^{16}, e^{17} + e^{25}, e^{28} + e^{46} + e^{37}$                                                                                                                                                                                                                                         | 1245679  |

Table 2 – Continued to next page

Table 2 – Continued from previous page

| Name         | $\mathfrak{g}$                                                                                                                                           | UCS Dim. |
|--------------|----------------------------------------------------------------------------------------------------------------------------------------------------------|----------|
| 9764321:6b   | $0, 0, -e^{12}, -e^{13}, e^{23}, -e^{14}, e^{16}, e^{25} + e^{17}, e^{37} + e^{46} + e^{28}$                                                             | 1245679  |
| 9764321:13   | $0, 0, -e^{12}, e^{13}, e^{23}, e^{14}, 2e^{16}, e^{17} + e^{26} + e^{34}, e^{27} + e^{18} + e^{36}$                                                     | 2345679  |
| Type: 211122 |                                                                                                                                                          |          |
| 976542:3     | $0, 0, -e^{12}, e^{13}, e^{14}, 2e^{15}, e^{25} + e^{34}, e^{16}, e^{17} + e^{26} + e^{35}$                                                              | 245679   |
| 976542:5     | $0, 0, -e^{12}, e^{13}, e^{14}, 2e^{15}, e^{25} + e^{34}, e^{16} + e^{23}, e^{17} + e^{26} + e^{35}$                                                     | 245679   |
| 976542:6     | $0, 0, -e^{12}, e^{13}, e^{14}, 2e^{15} + e^{23}, e^{25} + e^{34}, e^{16} + e^{24}, e^{17} + e^{26} + e^{35}$                                            | 245679   |
| Type: 212121 |                                                                                                                                                          |          |
| 976431:1     | $0, 0, -e^{12}, e^{13}, e^{23}, e^{14}, e^{16}, e^{26} + e^{34}, e^{17}$                                                                                 | 345679   |
| 976431:2a    | $0, 0, -e^{12}, e^{13}, e^{23}, e^{14}, e^{16}, e^{26} + e^{34}, e^{17} + e^{25}$                                                                        | 245679   |
| 976431:2b    | $0, 0, -e^{12}, -e^{13}, e^{23}, e^{14}, e^{16}, e^{26} + e^{34}, e^{17} + e^{25}$                                                                       | 245679   |
| 976431:5     | $0, 0, e^{12}, e^{13}, e^{23}, -e^{14}, e^{16} + e^{25}, e^{26} + e^{34}, e^{35} + e^{17}$                                                               | 235679   |
| 976431:7     | $0, 0, -e^{12}, e^{13}, e^{23}, e^{14}, 2e^{16}, e^{26} + e^{34}, e^{18} + e^{27} + e^{36}$                                                              | 245679   |
| 976431:8     | $0, 0, -e^{12}, e^{13}, e^{23}, e^{14}, e^{34} + e^{26}, e^{25} + 2e^{16}, e^{17} + e^{28} + e^{36}$                                                     | 135679   |
| 976431:13    | $0, 0, e^{12}, e^{13}, -e^{23}, e^{24} - e^{15}, e^{16} + e^{34}, e^{35} + e^{26}, e^{45} + e^{27} + e^{18}$                                             | 134679   |
| 976431:14a   | $0, 0, e^{12}, e^{13}, -e^{23}, e^{25} - e^{14}, e^{34} + e^{26}, e^{35} + e^{16}, e^{27} + e^{45} + e^{18}$                                             | 134679   |
| 976431:14b   | $0, 0, -e^{12}, e^{13}, -e^{23}, e^{14} + e^{25}, e^{26} + e^{34}, e^{35} - e^{16}, e^{45} + e^{27} + e^{18}$                                            | 134679   |
| 976431:17    | $0, 0, e^{12}, e^{13}, -e^{23}, -e^{15} + e^{24}, e^{16} + e^{34}, e^{14} + e^{26} + e^{35}, e^{18} + e^{27} + e^{45}$                                   | 134679   |
| 976431:20    | $0, 0, e^{12}, e^{13}, -e^{23}, -e^{15} + e^{24}, e^{26} + e^{35} + e^{14}, e^{16} + e^{25} + e^{34}, e^{28} + e^{17} + e^{45}$                          | 134679   |
| Type: 212211 |                                                                                                                                                          |          |
| 976421:1     | $0, 0, e^{12}, e^{13}, e^{23}, e^{14}, e^{25}, e^{16}, e^{18}$                                                                                           | 245679   |
| 976421:2     | $0, 0, e^{12}, e^{13}, e^{23}, e^{14}, e^{15} + e^{24}, e^{16}, e^{18}$                                                                                  | 245679   |
| 976421:3a    | $0, 0, e^{12}, e^{13}, e^{23}, e^{14}, e^{15} + e^{24}, e^{16}, e^{25} + e^{18}$                                                                         | 245679   |
| 976421:3b    | $0, 0, e^{12}, e^{13}, e^{23}, -e^{14}, e^{15} + e^{24}, e^{16}, e^{18} + e^{25}$                                                                        | 245679   |
| 976421:4     | $0, 0, e^{12}, e^{13}, e^{23}, e^{14}, e^{25}, e^{16}, e^{27} + e^{18}$                                                                                  | 135679   |
| 976421:6     | $0, 0, -e^{12}, e^{13}, e^{23}, e^{14}, e^{25}, e^{16}, e^{34} + e^{18} + e^{26}$                                                                        | 245679   |
| 976421:7     | $0, 0, e^{12}, e^{13}, e^{23}, e^{14}, e^{15} + e^{24}, e^{16} + e^{25}, e^{18} + e^{35}$                                                                | 235679   |
| 976421:9     | $0, 0, -e^{12}, e^{13}, e^{23}, e^{14}, e^{15} + e^{24}, e^{16}, e^{18} + e^{26} + e^{34}$                                                               | 245679   |
| 976421:10    | $0, 0, e^{12}, e^{13}, e^{23}, e^{14}, e^{24} + e^{15}, e^{25} + e^{16}, e^{27} + e^{18}$                                                                | 135679   |
| 976421:11    | $0, 0, -e^{12}, e^{13}, e^{23}, e^{14}, e^{15} + e^{24}, e^{16}, e^{27} + e^{18} + e^{35}$                                                               | 135679   |
| 976421:14    | $0, 0, -e^{12}(-1 + a_3), a_3e^{13}, e^{23}, e^{14}, a_3e^{15} + e^{24}, e^{16} + e^{25}, e^{18} + e^{27} + e^{35}$                                      | 135679   |
| 976421:21    | $0, 0, e^{12}, e^{13}, e^{23}, e^{14}, e^{15} + e^{24}, e^{26} + e^{34} + 2e^{17}, e^{36} + e^{18}$                                                      | 124679   |
| 976421:23    | $0, 0, e^{12}, e^{13}, e^{23}, e^{14}, e^{15} + e^{24}, e^{26} + e^{34} + 2e^{17}, e^{36} + e^{18} + e^{25}$                                             | 124679   |
| 976421:25    | $0, 0, -e^{12}, -e^{13}, -\frac{1}{2}e^{23}, e^{15} + \frac{1}{2}e^{24}, \frac{3}{2}e^{14}, e^{34} + e^{27} + e^{16}, e^{45} + e^{36} + e^{28}$          | 124679   |
| 976421:28a   | $0, 0, -e^{12}, e^{13}, -\frac{1}{2}e^{23}, -e^{15} + \frac{1}{2}e^{24}, e^{25} + \frac{3}{2}e^{14}, e^{27} + e^{16} + e^{34}, e^{28} + e^{45} + e^{36}$ | 124679   |
| 976421:28b   | $0, 0, -e^{12}, -e^{13}, -\frac{1}{2}e^{23}, e^{15} + \frac{1}{2}e^{24}, e^{25} + \frac{3}{2}e^{14}, e^{27} + e^{16} + e^{34}, e^{28} + e^{36} + e^{45}$ | 124679   |
| 976421:29    | $0, 0, -e^{12}, -e^{13}, -\frac{1}{2}e^{23}, \frac{3}{2}e^{14}, e^{15} + \frac{1}{2}e^{24}, e^{17} + e^{26} + e^{34}, e^{28} + e^{16} + e^{45} + e^{37}$ | 124679   |
| Type: 21222  |                                                                                                                                                          |          |
| 97642:1      | $0, 0, -e^{12}, e^{13}, e^{23}, e^{14}, e^{25}, e^{16}, e^{26} + e^{34}$                                                                                 | 35679    |
| 97642:2      | $0, 0, -e^{12}, e^{13}, e^{23}, e^{14}, e^{15} + e^{24}, e^{16}, e^{26} + e^{34}$                                                                        | 35679    |
| 97642:3      | $0, 0, -e^{12}, e^{13}, e^{23}, e^{14}, e^{15} + e^{24}, e^{26} + e^{34}, e^{25} + e^{16}$                                                               | 35679    |
| 97642:4      | $0, 0, e^{12}, -e^{13}, e^{23}, -e^{15} + e^{24}, e^{14}, e^{34} + e^{16}, e^{26} + e^{35}$                                                              | 34679    |
| 97642:5a     | $0, 0, e^{12}, -e^{13}, e^{23}, e^{24} - e^{15}, e^{25} + e^{14}, e^{34} + e^{16}, e^{26} + e^{35}$                                                      | 34679    |
| 97642:5b     | $0, 0, e^{12}, -e^{13}, e^{23}, e^{24} - e^{15}, e^{25} - e^{14}, e^{34} + e^{16}, e^{35} + e^{26}$                                                      | 34679    |
| 97642:6a     | $0, 0, e^{12}, e^{13}, e^{23}, e^{25} - e^{14}, e^{15} + e^{24}, e^{34} + e^{26}, e^{35} + e^{16}$                                                       | 34679    |
| 97642:6b     | $0, 0, e^{12}, -e^{13}, e^{23}, e^{25} - e^{14}, e^{24} - e^{15}, e^{26} + e^{34}, e^{16} + e^{35}$                                                      | 34679    |
| 97642:7      | $0, 0, e^{12}, -e^{13}, e^{23}, -e^{15} + e^{24}, e^{14}, e^{26} + e^{35}, e^{34} + e^{16} + e^{25}$                                                     | 34679    |
| 97642:8      | $0, 0, e^{12}, e^{13}, e^{23}, e^{14}, e^{25}, e^{16}, e^{27}$                                                                                           | 24679    |
| 97642:9      | $0, 0, -e^{12}, e^{13}, e^{23}, e^{14}, e^{25}, e^{34} + e^{26}, e^{27}$                                                                                 | 24679    |
| 97642:10     | $0, 0, e^{12}, e^{13}, e^{23}, e^{14}, e^{24} + e^{15}, e^{16}, e^{17} + e^{26}$                                                                         | 24679    |
| 97642:11     | $0, 0, e^{12}, e^{13}, e^{23}, e^{14}, e^{15} + e^{24}, e^{16}, e^{17} + e^{34}$                                                                         | 24679    |
| 97642:12     | $0, 0, -e^{12}, e^{13}, e^{23}, e^{14}, e^{24} + e^{15}, e^{16}, e^{27} + e^{35}$                                                                        | 24679    |
| 97642:13     | $0, 0, -e^{12}, e^{13}, e^{23}, e^{14}, e^{25}, e^{26} + e^{34}, e^{16} + e^{27}$                                                                        | 24679    |
| 97642:14     | $0, 0, e^{12}, e^{13}, e^{23}, -e^{14}, e^{25}, e^{34} + e^{26}, e^{17} + e^{35}$                                                                        | 24679    |
| 97642:15     | $0, 0, e^{12}, e^{13}, e^{23}, e^{14}, e^{24} + e^{15}, e^{25} + e^{16}, e^{26} + e^{17}$                                                                | 24679    |
| 97642:16     | $0, 0, e^{12}, e^{13}, e^{23}, e^{14}, e^{15} + e^{24}, e^{16}, e^{17} + e^{25} + e^{34}$                                                                | 24679    |
| 97642:17     | $0, 0, e^{12}, e^{13}, e^{23}, e^{14}, e^{24} + e^{15}, e^{25} + e^{16}, e^{34} + e^{17}$                                                                | 24679    |
| 97642:18     | $0, 0, -e^{12}, e^{13}, e^{23}, e^{14}, e^{15} + e^{24}, e^{25} + e^{16}, e^{35} + e^{27}$                                                               | 24679    |

Table 2 – Continued to next page

Table 2 – Continued from previous page

| Name          | $\mathfrak{g}$                                                                                                                                                     | UCS Dim. |
|---------------|--------------------------------------------------------------------------------------------------------------------------------------------------------------------|----------|
| 97642:19      | $0, 0, -(-1 + a_3)e^{12}, e^{13}, e^{23}, e^{14}a_3, e^{24} + e^{15}, e^{16}, e^{26} + e^{34} + e^{17}$                                                            | 24679    |
| 97642:20      | $0, 0, -e^{12}, e^{13}, e^{23}, e^{14}, e^{15} + e^{24}, e^{34} + e^{26}, e^{27} + e^{35}$                                                                         | 24679    |
| 97642:21      | $0, 0, -e^{12}, e^{13}, e^{23}, e^{15} + e^{24}, e^{14}, e^{26} + e^{35}, e^{16} + e^{27}$                                                                         | 24679    |
| 97642:22a     | $0, 0, e^{12}, e^{13}, e^{23}, e^{24} + e^{15}, e^{25} + e^{14}, e^{34} + e^{16}, e^{35} + e^{17}$                                                                 | 24679    |
| 97642:22b     | $0, 0, e^{12}, -e^{13}, e^{23}, e^{24} - e^{15}, e^{25} + e^{14}, e^{16} + e^{34}, e^{17} + e^{35}$                                                                | 24679    |
| 97642:23a     | $0, 0, e^{12}, e^{13}, e^{23}, e^{24} + e^{15}, e^{25} + e^{14}, e^{34} + e^{16}, e^{26} + e^{17}$                                                                 | 24679    |
| 97642:23b     | $0, 0, e^{12}, e^{13}, e^{23}, e^{24} + e^{15}, e^{25} - e^{14}, e^{34} + e^{16}, e^{26} + e^{17}$                                                                 | 24679    |
| 97642:24a     | $0, 0, e^{12}, e^{13}, e^{23}, -e^{14} + e^{25}, e^{15} + e^{24}, e^{26} + e^{34}, e^{27} + e^{16}$                                                                | 24679    |
| 97642:24b     | $0, 0, -e^{12}, e^{13}, e^{23}, e^{25} + e^{14}, e^{24} + e^{15}, e^{26} + e^{34}, e^{27} + e^{16}$                                                                | 24679    |
| 97642:25a     | $0, 0, e^{12}, e^{13}, e^{23}, e^{24} + e^{15}, e^{25} + e^{14}, e^{26} + e^{17}, e^{27} + e^{16}$                                                                 | 24679    |
| 97642:25b     | $0, 0, e^{12}, -e^{13}, e^{23}, e^{24} - e^{15}, e^{25} + e^{14}, -e^{17} + e^{26}, e^{16} + e^{27}$                                                               | 24679    |
| 97642:26      | $0, 0, -(-1 + a_3)e^{12}, e^{13}, e^{23}, e^{14}a_3, e^{15} + e^{24}, e^{16} + e^{25}, e^{17} + e^{26} + e^{34}$                                                   | 24679    |
| 97642:27a     | $0, 0, e^{12}, -e^{13}, e^{23}, -e^{14}, -e^{15} + e^{24}, e^{26} + e^{34}, e^{27} + e^{16} + e^{35}$                                                              | 24679    |
| 97642:27b     | $0, 0, -e^{12}, e^{13}, e^{23}, e^{14}, e^{15} + e^{24}, e^{26} + e^{34}, e^{16} + e^{27} + e^{35}$                                                                | 24679    |
| 97642:28a     | $0, 0, -e^{12}, e^{13}, e^{23}, e^{14}, e^{15} + e^{24}, e^{17} + e^{26}, e^{35} + e^{27} + e^{16}$                                                                | 24679    |
| 97642:28b     | $0, 0, -e^{12}, e^{13}, e^{23}, -e^{14}, e^{15} + e^{24}, -e^{17} + e^{26}, e^{27} + e^{35} + e^{16}$                                                              | 24679    |
| 97642:29a     | $0, 0, e^{12}, -e^{13}, e^{23}, e^{24} - e^{15}, e^{14}, e^{16} + e^{34}, e^{17} + e^{26} + e^{35}$                                                                | 24679    |
| 97642:29b     | $0, 0, e^{12}, -e^{13}, e^{23}, -e^{15} + e^{24}, -e^{14}, e^{34} + e^{16}, e^{26} + e^{35} + e^{17}$                                                              | 24679    |
| 97642:30      | $0, 0, -e^{12}a_1, e^{13}a_1, e^{23}, e^{15}a_1 + e^{24}, e^{14}(1 + a_1), e^{26} + e^{35}, e^{27} + e^{16} + e^{34}$                                              | 24679    |
| 97642:31a     | $0, 0, -(-1 + a_2)e^{12}, e^{13}a_2, e^{23}, e^{24} + e^{15}a_2, e^{14} + e^{25}, e^{34} - (-1 + a_2)e^{16}, e^{17} + e^{26} + e^{35}$                             | 24679    |
| 97642:31b     | $0, 0, -(-1 + a_2)e^{12}, e^{13}a_2, e^{23}, e^{24} + e^{15}a_2, -e^{14} + e^{25}, e^{34} - (-1 + a_2)e^{16}, e^{17} + e^{26} + e^{35}$                            | 24679    |
| 97642:32a     | $0, 0, e^{12}, e^{13}a_3, e^{23}, e^{25}(1 + a_3) - e^{14}, e^{24} + e^{15}a_3, e^{34} + e^{26}, e^{35} + e^{27} + e^{16}$                                         | 24679    |
| 97642:32b     | $0, 0, -e^{12}, e^{13}a_3, e^{23}, e^{14} + (-1 + a_3)e^{25}, e^{24} + e^{15}a_3, e^{26} + e^{34}, e^{16} + e^{27} + e^{35}$                                       | 24679    |
| 97642:33a     | $0, 0, -e^{12}(-1 + a_2), e^{13}, e^{23}, e^{25} + a_2e^{14}, e^{15} + e^{24}, e^{16} + e^{27}, e^{17} + e^{26} + e^{34}$                                          | 24679    |
| 97642:33b     | $0, 0, -e^{12}(-1 + a_2), -e^{13}, e^{23}, e^{25} + a_2e^{14}, e^{24} - e^{15}, e^{27} - e^{16}, e^{26} + e^{34} + e^{17}$                                         | 24679    |
| 97642:34a     | $0, 0, e^{12}, -e^{13}, e^{23}, e^{24} - e^{15}, e^{14}, e^{16} + e^{34} + e^{25}, e^{17} + e^{26} + e^{35}$                                                       | 24679    |
| 97642:34b     | $0, 0, e^{12}, -e^{13}, e^{23}, -e^{15} + e^{24}, -e^{14}, e^{34} + e^{16} + e^{25}, e^{26} + e^{35} + e^{17}$                                                     | 24679    |
| 97642:35a     | $0, 0, e^{12}, -e^{13}, e^{23}, e^{14}a_2, -e^{15} + e^{24}, e^{26} + e^{34} + (1 + a_2)e^{17}, e^{16} + e^{27} + e^{35}$                                          | 24679    |
| 97642:35b     | $0, 0, -e^{12}, e^{13}, e^{23}, e^{14}a_2, e^{15} + e^{24}, e^{26} + e^{34} + (-1 + a_2)e^{17}, e^{16} + e^{27} + e^{35}$                                          | 24679    |
| 97642:36a(*)  | $0, 0, e^{12}a_1, e^{13}, e^{23}, -(-1 + a_1)(e^{15} + e^{24}),$<br>$(-a_1 + a_4 - a_1a_4)e^{14} + e^{25}, e^{16}a_4 + e^{34} + e^{27}, e^{17} + e^{26} + e^{35}$  | 24679    |
| 97642:36b(*)  | $0, 0, e^{12}a_1, -e^{13}, e^{23}, -(e^{15} - e^{24})(-1 + a_1),$<br>$(-a_1 - a_4 + a_1a_4)e^{14} + e^{25}, e^{16}a_4 + e^{34} + e^{27}, e^{26} + e^{17} + e^{35}$ | 24679    |
| Type: 3111111 |                                                                                                                                                                    |          |
| 9654321:1     | $0, 0, 0, e^{12}, e^{14}, e^{15}, e^{16}, e^{17}, e^{18}$                                                                                                          | 2345679  |
| 9654321:2     | $0, 0, 0, e^{12}, e^{14}, e^{15}, e^{16}, e^{17}, e^{18} + e^{23}$                                                                                                 | 1345679  |
| 9654321:3     | $0, 0, 0, e^{12}, e^{14}, e^{15}, e^{16}, e^{17}, e^{18} + e^{24}$                                                                                                 | 2345679  |
| 9654321:4     | $0, 0, 0, -e^{12}, e^{14}, e^{15}, e^{16}, e^{17} + e^{23}, e^{34} + e^{18}$                                                                                       | 1245679  |
| 9654321:5     | $0, 0, 0, -e^{12}, e^{14}, e^{15}, e^{23} + e^{16}, e^{34} + e^{17}, e^{18} + e^{35}$                                                                              | 1235679  |
| 9654321:6     | $0, 0, 0, e^{12}, e^{14}, e^{15}, e^{16}, e^{17} + e^{24}, e^{18} + e^{25}$                                                                                        | 2345679  |
| 9654321:7     | $0, 0, 0, -e^{12}, e^{14}, e^{15} + e^{23}, e^{34} + e^{16}, e^{35} + e^{17}, e^{18} + e^{36}$                                                                     | 1234679  |
| 9654321:8     | $0, 0, 0, -e^{12}, e^{14}, e^{15}, e^{16}, e^{17}, e^{26} + e^{18} + e^{45}$                                                                                       | 2345679  |
| 9654321:9     | $0, 0, 0, -e^{12}, -e^{14}, e^{15}, e^{16}, e^{17}, e^{56} + e^{47} + e^{28}$                                                                                      | 2345679  |
| 9654321:10    | $0, 0, 0, -e^{12}, e^{14}, e^{15}, e^{16} + e^{23}, e^{17} + e^{34}, e^{18} + e^{35} + e^{24}$                                                                     | 1235679  |
| 9654321:11    | $0, 0, 0, e^{12}, e^{14}, e^{15}, e^{16} + e^{24}, e^{25} + e^{17}, e^{26} + e^{18}$                                                                               | 2345679  |
| 9654321:12    | $0, 0, 0, -e^{12}, -e^{14}, e^{15}, e^{16}, e^{17} + e^{23}, e^{28} + e^{56} + e^{47}$                                                                             | 1245679  |
| 9654321:13    | $0, 0, 0, e^{12}, e^{14}, e^{15}, e^{16} + e^{24}, e^{17} + e^{25}, e^{18} + e^{45}$                                                                               | 2345679  |
| 9654321:17    | $0, 0, 0, -e^{12}, -e^{14}, e^{15}, e^{16}, e^{17}, e^{56} + e^{47} + e^{28} + e^{13}$                                                                             | 1345679  |
| 9654321:18    | $0, 0, 0, -e^{12}, -e^{14}, e^{15}, e^{16}, e^{24} + e^{17}, e^{28} + e^{56} + e^{47}$                                                                             | 2345679  |
| 9654321:20    | $0, 0, 0, -e^{12}, e^{14}, e^{23} + e^{15}, e^{16} + e^{34}, e^{17} + e^{35}, e^{18} + e^{36} + e^{24}$                                                            | 1234679  |
| 9654321:23    | $0, 0, 0, -e^{12}, -e^{14}, e^{15}, e^{16}, e^{17} + e^{23}, e^{28} + e^{13} + e^{56} + e^{47}$                                                                    | 1245679  |
| 9654321:24    | $0, 0, 0, e^{12}, e^{14}, e^{15}, e^{16} + e^{24}, e^{17} + e^{25}, e^{45} + e^{18} + e^{23}$                                                                      | 1345679  |
| 9654321:27    | $0, 0, 0, e^{12}, e^{14}, e^{15} + e^{24}, e^{25} + e^{16}, e^{17} + e^{26}, e^{18} + e^{27}$                                                                      | 2345679  |
| 9654321:29    | $0, 0, 0, -e^{12}, e^{14}, e^{15} - e^{23}, e^{34} - e^{16}, e^{35} + e^{17}, e^{28} + e^{47} + e^{56}$                                                            | 1234679  |
| 9654321:31    | $0, 0, 0, -e^{12}, -e^{14}, e^{15}, e^{16}, e^{24} + e^{17}, e^{13} + e^{28} + e^{56} + e^{47}$                                                                    | 1345679  |
| 9654321:32    | $0, 0, 0, -(-1 + a_3)e^{12}, e^{14}, e^{15}a_3, e^{16} + e^{24}, e^{17} + e^{25}, e^{18} + e^{45} + e^{26}$                                                        | 2345679  |
| 9654321:35    | $0, 0, 0, -e^{12}, e^{14}, e^{15}, 2e^{16}, e^{26} + e^{45} + e^{17}, e^{27} + e^{46} + e^{18}$                                                                    | 2345679  |
| 9654321:37    | $0, 0, 0, -e^{12}, e^{14}, e^{15}, e^{24} - e^{16}, e^{25} + e^{17}, e^{47} + e^{56} + e^{28}$                                                                     | 2345679  |

Table 2 – Continued to next page

Table 2 – Continued from previous page

| Name         | $\mathfrak{g}$                                                                                                                                              | UCS Dim. |
|--------------|-------------------------------------------------------------------------------------------------------------------------------------------------------------|----------|
| 9654321:41   | $0, 0, 0, -e^{12}, e^{14}, e^{23} + e^{15}, e^{16} + e^{34}, e^{17} + e^{35} + e^{24}, e^{18} + e^{36} + e^{25}$                                            | 1234679  |
| 9654321:45   | $0, 0, 0, -e^{12}, e^{14} + e^{23}, e^{15} + e^{34}, e^{35} + e^{16}, e^{36} + e^{17}, e^{37} + e^{18}$                                                     | 1234579  |
| 9654321:47   | $0, 0, 0, -e^{12}, e^{14}, e^{15} - e^{23}, -e^{16} + e^{34}, e^{17} + e^{35}, e^{13} + e^{47} + e^{56} + e^{28}$                                           | 1234679  |
| 9654321:51   | $0, 0, 0, e^{12}, e^{14}, e^{15} + e^{24}, e^{25} + e^{16}, e^{26} + 2e^{17} + e^{45}, e^{18} + e^{46}$                                                     | 2345679  |
| 9654321:52   | $0, 0, 0, -e^{12}, e^{14}, e^{15} - e^{23}, -e^{16} + e^{34}, e^{17} + e^{35} + e^{24}, e^{47} + e^{56} + e^{28}$                                           | 1234679  |
| 9654321:53   | $0, 0, 0, -e^{12}, e^{14}, e^{15}, -e^{16} + e^{24}, e^{17} + e^{25}, e^{13} + e^{47} + e^{56} + e^{28}$                                                    | 1345679  |
| 9654321:54   | $0, 0, 0, e^{12}, -e^{14}, e^{15} + e^{24}, -e^{16} + e^{25}, e^{17} + e^{45}, e^{27} + e^{18} + e^{46}$                                                    | 2345679  |
| 9654321:61   | $0, 0, 0, e^{12}, e^{14}, e^{15} + e^{24}, e^{25} + e^{16}, e^{26} + 2e^{17} + e^{45}, e^{23} + e^{18} + e^{46}$                                            | 1345679  |
| 9654321:62   | $0, 0, 0, -e^{12}, e^{14}, e^{15} - e^{23}, -e^{16} + e^{34}, e^{17} + e^{35} + e^{24}, e^{13} + e^{47} + e^{56} + e^{28}$                                  | 1234679  |
| 9654321:65   | $0, 0, 0, -e^{12}, e^{23} + e^{14}, e^{34} + e^{15}, e^{16} + e^{35}, e^{17} + e^{36}, e^{18} + e^{37} + e^{24}$                                            | 1234579  |
| 9654321:70   | $0, 0, 0, (-1 + a_5)e^{12}, -e^{14}(-2 + a_5), e^{15} + e^{24}, e^{25} - e^{16}(-2 + a_5), e^{26} + e^{45} + e^{17}a_5, e^{18} + e^{46} + e^{27}$           | 2345679  |
| 9654321:72   | $0, 0, 0, -e^{12}, -e^{14}, \frac{3}{2}e^{15} - \frac{1}{2}e^{24}, e^{16} + \frac{1}{2}e^{25}, e^{45} + e^{17} + e^{26}, e^{56} + e^{47} + e^{28}$          | 2345679  |
| 9654321:78   | $0, 0, 0, -e^{12}, e^{23} + e^{14}, e^{34} + e^{15}, e^{16} + e^{35}, e^{17} + e^{36} + e^{24}, e^{18} + e^{37} + e^{25}$                                   | 1234579  |
| 9654321:80   | $0, 0, 0, -e^{12}, -e^{14}, \frac{3}{2}e^{15} - \frac{1}{2}e^{24}, e^{16} + \frac{1}{2}e^{25}, e^{45} + e^{17} + e^{26}, e^{56} + e^{47} + e^{28} + e^{13}$ | 1345679  |
| 9654321:88   | $0, 0, 0, -e^{12}, e^{23} + e^{14}, e^{34} + e^{15}, e^{16} + e^{35} + e^{24}, e^{17} + e^{36} + e^{25}, e^{18} + e^{26} + e^{37}$                          | 1234579  |
| Type: 311121 |                                                                                                                                                             |          |
| 965431:1     | $0, 0, 0, -e^{12}, e^{14}, e^{15}, e^{16}, e^{26} + e^{45}, e^{17}$                                                                                         | 345679   |
| 965431:2     | $0, 0, 0, -e^{12}, e^{14}, e^{15}, e^{16}, e^{45} + e^{26} + e^{13}, e^{17}$                                                                                | 245679   |
| 965431:3     | $0, 0, 0, -e^{12}, e^{14}, e^{15}, e^{16}, e^{26} + e^{45}, e^{17} + e^{23}$                                                                                | 245679   |
| 965431:4     | $0, 0, 0, -e^{12}, e^{14}, e^{15}, e^{16}, e^{13} + e^{26} + e^{45}, e^{17} + e^{23}$                                                                       | 245679   |
| 965431:5     | $0, 0, 0, -e^{12}, e^{14}, e^{15}, e^{16}, e^{26} + e^{45}, e^{24} + e^{17}$                                                                                | 345679   |
| 965431:6     | $0, 0, 0, -e^{12}, e^{14}, e^{15}, e^{16} + e^{23}, e^{45} + e^{26}, e^{17} + e^{34}$                                                                       | 235679   |
| 965431:8     | $0, 0, 0, -e^{12}, e^{14}, e^{15}, e^{16}, e^{45} + e^{26} + e^{13}, e^{17} + e^{24}$                                                                       | 245679   |
| 965431:9a    | $0, 0, 0, -e^{12}, e^{14}, e^{15}, e^{16} + e^{23}, e^{13} + e^{26} + e^{45}, e^{17} + e^{34}$                                                              | 235679   |
| 965431:9b    | $0, 0, 0, -e^{12}, e^{14}, e^{15}, e^{23} - e^{16}, e^{26} + e^{13} + e^{45}, e^{34} + e^{17}$                                                              | 235679   |
| 965431:12    | $0, 0, 0, -e^{12}, e^{14}, e^{23} + e^{15}, e^{34} + e^{16}, e^{26} + e^{45}, e^{35} + e^{17}$                                                              | 234679   |
| 965431:13    | $0, 0, 0, -e^{12}, e^{14}, e^{15}, e^{16} + e^{24}, e^{26} + e^{45}, e^{17} + e^{25}$                                                                       | 345679   |
| 965431:17    | $0, 0, 0, -e^{12}, e^{14}, e^{23} + e^{15}, e^{16} + e^{34}, e^{26} + e^{45} + e^{13}, e^{17} + e^{35}$                                                     | 234679   |
| 965431:18    | $0, 0, 0, -e^{12}, e^{14}, e^{15}, e^{16} + e^{24}, e^{26} + e^{13} + e^{45}, e^{17} + e^{25}$                                                              | 245679   |
| 965431:22    | $0, 0, 0, -e^{12}, e^{14}, e^{15} + e^{23}, e^{34} + e^{16}, e^{26} + e^{45}, e^{35} + e^{24} + e^{17}$                                                     | 234679   |
| 965431:25    | $0, 0, 0, -e^{12}, e^{14}, e^{15} + e^{23}, e^{16} + e^{34}, e^{13} + e^{26} + e^{45}, e^{17} + e^{35} + e^{24}$                                            | 234679   |
| 965431:39    | $0, 0, 0, -e^{12}, e^{14}, e^{15}, 2e^{16}, e^{26} + e^{45}, e^{46} + e^{27} + e^{18}$                                                                      | 245679   |
| 965431:40    | $0, 0, 0, -e^{12}, e^{14}, e^{15}, 2e^{16}, e^{26} + e^{45} + e^{13}, e^{46} + e^{27} + e^{18}$                                                             | 135679   |
| 965431:41    | $0, 0, 0, -e^{12}, e^{14}, e^{15}, e^{23} + 2e^{16}, e^{26} + e^{45}, e^{46} + e^{27} + e^{18}$                                                             | 135679   |
| 965431:42a   | $0, 0, 0, -e^{12}, e^{14}, e^{15}, 2e^{16} + e^{23}, e^{13} + e^{26} + e^{45}, e^{18} + e^{46} + e^{27}$                                                    | 135679   |
| 965431:42b   | $0, 0, 0, -e^{12}, e^{14}, e^{15}, 2e^{16} + e^{23}, -e^{13} + e^{26} + e^{45}, e^{18} + e^{46} + e^{27}$                                                   | 135679   |
| 965431:43    | $0, 0, 0, -e^{12}, e^{14}, e^{15}, e^{24} + 2e^{16}, e^{26} + e^{45}, e^{46} + e^{27} + e^{18}$                                                             | 245679   |
| 965431:45    | $0, 0, 0, -e^{12}, e^{14}, e^{15}, e^{24} + 2e^{16}, e^{26} + e^{45} + e^{13}, e^{46} + e^{27} + e^{18}$                                                    | 135679   |
| 965431:47    | $0, 0, 0, -e^{12}, 2e^{14}, e^{15} + e^{24}, 2e^{16} + e^{25}, e^{26} + e^{45}, e^{18} + e^{46} + e^{27}$                                                   | 245679   |
| 965431:48    | $0, 0, 0, -e^{12}, 2e^{14}, e^{24} + e^{15}, e^{25} + 2e^{16}, e^{26} + e^{45} + e^{13}, e^{46} + e^{27} + e^{18}$                                          | 135679   |
| Type: 312111 |                                                                                                                                                             |          |
| 965321:1     | $0, 0, 0, e^{12}, e^{14}, e^{24}, e^{15}, e^{17}, e^{18}$                                                                                                   | 345679   |
| 965321:2     | $0, 0, 0, e^{12}, e^{14}, e^{13} + e^{24}, e^{15}, e^{17}, e^{18}$                                                                                          | 245679   |
| 965321:3     | $0, 0, 0, e^{12}, e^{14}, e^{24}, e^{15}, e^{17}, e^{23} + e^{18}$                                                                                          | 245679   |
| 965321:4a    | $0, 0, 0, e^{12}, e^{14}, e^{24}, e^{15}, e^{17}, e^{18} + e^{26}$                                                                                          | 245679   |
| 965321:4b    | $0, 0, 0, e^{12}, -e^{14}, e^{24}, e^{15}, e^{17}, e^{26} + e^{18}$                                                                                         | 245679   |
| 965321:5     | $0, 0, 0, e^{12}, e^{14}, e^{24} + e^{13}, e^{15}, e^{17}, e^{18} + e^{23}$                                                                                 | 245679   |
| 965321:6     | $0, 0, 0, -e^{12}, e^{14}, e^{24}, e^{15}, e^{17} + e^{23}, e^{18} + e^{34}$                                                                                | 235679   |
| 965321:7a    | $0, 0, 0, -e^{12}, e^{14}, e^{24} + e^{13}, e^{15}, e^{23} + e^{17}, e^{34} + e^{18}$                                                                       | 235679   |
| 965321:7b    | $0, 0, 0, -e^{12}, -e^{14}, e^{24} + e^{13}, e^{15}, e^{17} + e^{23}, e^{34} + e^{18}$                                                                      | 235679   |
| 965321:8a    | $0, 0, 0, e^{12}, e^{14}, e^{13} + e^{24}, e^{15}, e^{17} + e^{23}, e^{18} + e^{26}$                                                                        | 135679   |
| 965321:8b    | $0, 0, 0, e^{12}, -e^{14}, e^{24} + e^{13}, e^{15}, e^{17} + e^{23}, e^{18} + e^{26}$                                                                       | 135679   |
| 965321:9     | $0, 0, 0, -e^{12}, e^{14}, e^{24}, e^{23} + e^{15}, e^{34} + e^{17}, e^{35} + e^{18}$                                                                       | 234679   |
| 965321:10a   | $0, 0, 0, e^{12}, e^{14}, e^{13} + e^{24}, e^{15}, e^{17}, e^{26} + e^{18} + e^{34}$                                                                        | 135679   |
| 965321:10b   | $0, 0, 0, e^{12}, -e^{14}, e^{24} + e^{13}, e^{15}, e^{17}, e^{18} + e^{26} + e^{34}$                                                                       | 135679   |
| 965321:11a   | $0, 0, 0, -e^{12}, e^{14}, e^{24}, e^{15}, e^{17} + e^{23}, e^{18} + e^{34} + e^{26}$                                                                       | 135679   |
| 965321:11b   | $0, 0, 0, -e^{12}, -e^{14}, e^{24}, e^{15}, e^{17} + e^{23}, e^{26} + e^{34} + e^{18}$                                                                      | 135679   |
| 965321:12    | $0, 0, 0, -e^{12}, e^{14}, e^{13} + e^{24}, e^{15} + e^{23}, e^{34} + e^{17}, e^{18} + e^{35}$                                                              | 234679   |

Table 2 – Continued to next page

Table 2 – Continued from previous page

| Name         | $\mathfrak{g}$                                                                                                               | UCS Dim. |
|--------------|------------------------------------------------------------------------------------------------------------------------------|----------|
| 965321:13    | $0, 0, 0, e^{12}, e^{14}, e^{24}, e^{15}, e^{17} + e^{26}, e^{46} + e^{18}$                                                  | 235679   |
| 965321:15    | $0, 0, 0, -e^{12}, e^{14}, e^{24}, e^{15}, e^{17}, e^{45} + e^{18} + e^{27}$                                                 | 345679   |
| 965321:16a   | $0, 0, 0, e^{12}a_1, e^{14}, e^{13}(1 + a_1) + e^{24}, e^{15}, e^{17} + e^{23}, e^{18} + e^{26} + e^{34}$                    | 135679   |
| 965321:16b   | $0, 0, 0, e^{12}a_1, -e^{14}, e^{13}(1 + a_1) + e^{24}, e^{15}, e^{17} + e^{23}, e^{18} + e^{34} + e^{26}$                   | 135679   |
| 965321:18a   | $0, 0, 0, -e^{12}, e^{14}, e^{24}, e^{23} + e^{15}, e^{17} + e^{34}, e^{18} + e^{26} + e^{35}$                               | 134679   |
| 965321:18b   | $0, 0, 0, -e^{12}, e^{14}, e^{24}, -e^{15} + e^{23}, e^{17} + e^{34}, e^{18} + e^{35} + e^{26}$                              | 134679   |
| 965321:20    | $0, 0, 0, -e^{12}, e^{14}, e^{13} + e^{24}, e^{15}, e^{17}, e^{18} + e^{27} + e^{45}$                                        | 245679   |
| 965321:21    | $0, 0, 0, e^{12}, e^{14}, e^{24}, e^{15}, e^{17} + e^{26}, e^{23} + e^{46} + e^{18}$                                         | 135679   |
| 965321:29    | $0, 0, 0, e^{12}, e^{14}, e^{24} - e^{13}, e^{23} + e^{15}, -2e^{17} + e^{26} + e^{34}, e^{46} + e^{18}$                     | 124679   |
| 965321:32    | $0, 0, 0, e^{12}, e^{13} + e^{24}, e^{14}, e^{34} + e^{25}, e^{27} + e^{35}, e^{28} + e^{37}$                                | 234579   |
| 965321:33    | $0, 0, 0, e^{12}, e^{14}, e^{13} + e^{24}, e^{15} + e^{23}, e^{26} + e^{17}, e^{18} + e^{46} + e^{35}$                       | 124679   |
| 965321:35    | $0, 0, 0, e^{12}, e^{14}, e^{24}, e^{15} + e^{23}, e^{34} - e^{17} + e^{26}, e^{46} + e^{35} + e^{18}$                       | 124679   |
| 965321:36    | $0, 0, 0, e^{12}, 2e^{14}, e^{13} + e^{24}, e^{15}, e^{17} + e^{34} + e^{26}, e^{18} + e^{46} + e^{35}$                      | 124679   |
| 965321:37a   | $0, 0, 0, -e^{12}, e^{23} + e^{14}, e^{24} + e^{13}, e^{34} + e^{15}, e^{17} + e^{35}, e^{18} + e^{37}$                      | 234579   |
| 965321:37b   | $0, 0, 0, -e^{12}, e^{14} + e^{23}, -e^{13} + e^{24}, e^{15} + e^{34}, e^{35} + e^{17}, e^{37} + e^{18}$                     | 234579   |
| 965321:40a   | $0, 0, 0, e^{12}, e^{13} + e^{24}, e^{14}, e^{34} + e^{25}, e^{27} + e^{35}, e^{28} + e^{37} + e^{16}$                       | 134579   |
| 965321:40b   | $0, 0, 0, e^{12}, e^{13} + e^{24}, -e^{14}, e^{25} + e^{34}, e^{27} + e^{35}, e^{37} + e^{16} + e^{28}$                      | 134579   |
| 965321:45    | $0, 0, 0, -e^{12}, e^{24} - e^{13}, e^{14}, e^{25} + e^{34}, e^{16} + e^{27} + e^{35}, e^{46} + e^{28} + e^{37}$             | 124579   |
| Type: 321111 |                                                                                                                              |          |
| 964321:1     | $0, 0, 0, e^{12}, e^{13}, e^{14}, e^{16}, e^{17}, e^{18}$                                                                    | 245679   |
| 964321:2     | $0, 0, 0, e^{12}, e^{13}, e^{24}, e^{26}, e^{27}, e^{28}$                                                                    | 245679   |
| 964321:3     | $0, 0, 0, e^{12}, e^{13}, e^{14}, e^{16}, e^{17}, e^{18} + e^{35}$                                                           | 135679   |
| 964321:4     | $0, 0, 0, e^{12}, e^{13}, e^{24}, e^{26}, e^{27}, e^{28} + e^{35}$                                                           | 135679   |
| 964321:5     | $0, 0, 0, e^{12}, e^{13}, e^{14}, e^{16}, e^{17}, e^{18} + e^{23}$                                                           | 245679   |
| 964321:6     | $0, 0, 0, e^{12}, e^{13}, e^{24}, e^{26}, e^{27}, e^{28} + e^{15}$                                                           | 135679   |
| 964321:7     | $0, 0, 0, e^{12}, e^{13}, e^{14}, e^{16}, e^{17}, e^{24} + e^{18}$                                                           | 245679   |
| 964321:8     | $0, 0, 0, e^{12}, e^{13}, e^{24}, e^{26}, e^{27}, e^{14} + e^{28}$                                                           | 245679   |
| 964321:9     | $0, 0, 0, e^{12}, e^{13}, e^{14}, e^{16}, e^{17} + e^{23}, e^{18} + e^{25}$                                                  | 135679   |
| 964321:10    | $0, 0, 0, -e^{12}, e^{13}, e^{14}, e^{16}, e^{17} + e^{23}, e^{18} + e^{34}$                                                 | 235679   |
| 964321:11a   | $0, 0, 0, e^{12}, e^{13}, e^{14}, e^{16}, e^{17}, e^{35} + e^{18} + e^{24}$                                                  | 135679   |
| 964321:11b   | $0, 0, 0, -e^{12}, e^{13}, e^{14}, e^{16}, e^{17}, e^{35} + e^{24} + e^{18}$                                                 | 135679   |
| 964321:12    | $0, 0, 0, e^{12}, e^{13}, e^{14}, e^{16}, e^{17}, e^{25} + e^{18} + e^{34}$                                                  | 135679   |
| 964321:13    | $0, 0, 0, e^{12}, e^{13}, e^{24}, e^{26}, e^{27}, e^{14} + e^{35} + e^{28}$                                                  | 135679   |
| 964321:14    | $0, 0, 0, -e^{12}, e^{13}, e^{14}, e^{16} + e^{23}, e^{17} + e^{34}, e^{18} + e^{36}$                                        | 234679   |
| 964321:16    | $0, 0, 0, e^{12}a_1, e^{13}(1 + a_1), e^{14}, e^{16}, e^{23} + e^{17}, e^{18} + e^{34} + e^{25}$                             | 135679   |
| 964321:17    | $0, 0, 0, e^{12}, e^{13}, e^{14}, e^{16}, e^{17} + e^{24}, e^{18} + e^{26}$                                                  | 245679   |
| 964321:18    | $0, 0, 0, e^{12}, e^{13}, e^{24}, e^{26}, e^{27} + e^{14}, e^{28} + e^{16}$                                                  | 245679   |
| 964321:21    | $0, 0, 0, e^{12}, -e^{13}, e^{14}, e^{16} + e^{23}, e^{25} + e^{34} - 2e^{17}, e^{18} + e^{45}$                              | 124679   |
| 964321:22    | $0, 0, 0, -e^{12}, e^{13}, e^{14}, e^{16}, e^{17}, e^{27} + e^{18} + e^{46}$                                                 | 245679   |
| 964321:23    | $0, 0, 0, e^{12}, e^{13}, e^{24}, e^{26}, e^{27}, e^{28} + e^{17} + e^{46}$                                                  | 245679   |
| 964321:24    | $0, 0, 0, e^{12}, e^{13}, e^{14}, e^{16}, e^{24} + e^{17}, e^{35} + e^{26} + e^{18}$                                         | 135679   |
| 964321:25    | $0, 0, 0, e^{12}, e^{13}, e^{24}, e^{26}, e^{27} + e^{14}, e^{35} + e^{16} + e^{28}$                                         | 135679   |
| 964321:29    | $0, 0, 0, e^{12}, e^{13}, e^{14}, e^{23} + e^{16}, e^{25} + e^{17}, e^{36} + e^{45} + e^{18}$                                | 124679   |
| 964321:31    | $0, 0, 0, e^{12}, e^{13}, 2e^{14}, e^{16}, e^{17} + e^{34} + e^{25}, e^{18} + e^{36} + e^{45}$                               | 124679   |
| 964321:33a   | $0, 0, 0, -e^{12}, e^{13}, e^{14}, e^{16}, e^{17}, e^{27} + e^{18} + e^{35} + e^{46}$                                        | 135679   |
| 964321:33b   | $0, 0, 0, -e^{12}, -e^{13}, e^{14}, e^{16}, e^{17}, e^{18} + e^{27} + e^{46} + e^{35}$                                       | 135679   |
| 964321:34    | $0, 0, 0, e^{12}, e^{13}, e^{24}, e^{26}, e^{27}, e^{17} + e^{46} + e^{35} + e^{28}$                                         | 135679   |
| 964321:36    | $0, 0, 0, -e^{12}, e^{13}, e^{14}, e^{23} + e^{16}, e^{17} + e^{34}, e^{18} + e^{24} + e^{36}$                               | 234679   |
| 964321:38    | $0, 0, 0, e^{12}, e^{13}, e^{14}, e^{16} + e^{24}, e^{17} + e^{26}, e^{18} + e^{46}$                                         | 245679   |
| 964321:39    | $0, 0, 0, -e^{12}, e^{13}, e^{24}, e^{14} + e^{26}, e^{27} + e^{16}, e^{28} + e^{46}$                                        | 245679   |
| 964321:40    | $0, 0, 0, e^{12}, e^{13}, e^{14}, e^{16} + e^{24}, e^{17} + e^{26}, e^{18} + e^{27}$                                         | 245679   |
| 964321:41    | $0, 0, 0, e^{12}, e^{13}, e^{24}, e^{26} + e^{14}, e^{27} + e^{16}, e^{28} + e^{17}$                                         | 245679   |
| 964321:45    | $0, 0, 0, e^{12}, e^{13}a_2, e^{14}(1 + a_2), e^{16} + e^{23}, e^{25} + e^{34} + (-1 + a_2)e^{17}, e^{18} + e^{45} + e^{36}$ | 124679   |
| 964321:47a   | $0, 0, 0, e^{12}, e^{13}, e^{14}, e^{16} + e^{24}, e^{17} + e^{26}, e^{18} + e^{35} + e^{46}$                                | 135679   |
| 964321:47b   | $0, 0, 0, e^{12}, -e^{13}, e^{14}, e^{24} + e^{16}, e^{26} + e^{17}, e^{35} + e^{18} + e^{46}$                               | 135679   |
| 964321:48    | $0, 0, 0, -e^{12}, e^{13}, e^{24}, e^{14} + e^{26}, e^{27} + e^{16}, e^{28} + e^{46} + e^{35}$                               | 135679   |
| 964321:49a   | $0, 0, 0, e^{12}, e^{13}, e^{14}, e^{24} + e^{16}, e^{26} + e^{17}, e^{18} + e^{27} + e^{35}$                                | 135679   |

Table 2 – Continued to next page

Table 2 – Continued from previous page

| Name        | $\mathfrak{g}$                                                                                                                   | UCS Dim. |
|-------------|----------------------------------------------------------------------------------------------------------------------------------|----------|
| 964321:49b  | $0, 0, 0, -e^{12}, e^{13}, e^{14}, e^{16} + e^{24}, e^{17} + e^{26}, e^{18} + e^{27} + e^{35}$                                   | 135679   |
| 964321:50   | $0, 0, 0, e^{12}, e^{13}, e^{24}, e^{26} + e^{14}, e^{27} + e^{16}, e^{35} + e^{17} + e^{28}$                                    | 135679   |
| 964321:57   | $0, 0, 0, e^{12}, e^{13}, e^{14}, e^{16} + e^{24}, e^{17} + e^{26}, e^{46} + e^{18} + e^{23}$                                    | 245679   |
| 964321:58   | $0, 0, 0, -e^{12}, e^{13}, e^{24}, e^{14} + e^{26}, e^{16} + e^{27}, e^{15} + e^{46} + e^{28}$                                   | 135679   |
| 964321:59   | $0, 0, 0, -e^{12}, e^{13}, e^{14} + e^{23}, e^{16} + e^{34}, e^{17} + e^{36}, e^{18} + e^{37}$                                   | 234579   |
| 964321:64   | $0, 0, 0, a_1 e^{12}, e^{13}, e^{14}, e^{24} - e^{16}(-1 + a_1), e^{26} + e^{17}, e^{18} + e^{46} + e^{27}$                      | 245679   |
| 964321:65   | $0, 0, 0, -(-1 + a_3)e^{12}, e^{13}, e^{24}, e^{14} a_3 + e^{26}, e^{16} a_3 + e^{27}, e^{17} + e^{28} + e^{46}$                 | 245679   |
| 964321:68a  | $0, 0, 0, e^{12} a_1, e^{13}, e^{14}, -(-1 + a_1)e^{16} + e^{24}, e^{17} + e^{26}, e^{46} + e^{18} + e^{27} + e^{35}$            | 135679   |
| 964321:68b  | $0, 0, 0, e^{12} a_1, -e^{13}, e^{14}, -(-1 + a_1)e^{16} + e^{24}, e^{17} + e^{26}, e^{46} + e^{18} + e^{27} + e^{35}$           | 135679   |
| 964321:69   | $0, 0, 0, e^{12} a_1, e^{13}, e^{24}, -(-1 + a_1)e^{14} + e^{26}, -(-1 + a_1)e^{16} + e^{27}, e^{28} + e^{17} + e^{35} + e^{46}$ | 135679   |
| 964321:71   | $0, 0, 0, -e^{12}, e^{13}, e^{14} + e^{23}, e^{16} + e^{34}, e^{17} + e^{36}, e^{18} + e^{24} + e^{37}$                          | 234579   |
| 964321:76   | $0, 0, 0, -e^{12}, e^{13}, e^{14} + e^{23}, e^{34} + e^{16}, e^{36} + e^{17} + e^{24}, e^{37} + e^{18} + e^{26}$                 | 234579   |
| Type: 21231 |                                                                                                                                  |          |
| 97641:1     | $0, 0, e^{12}, e^{13}, e^{23}, e^{14}, e^{25}, e^{15} + e^{24}, e^{16}$                                                          | 35679    |
| 97641:2     | $0, 0, -e^{12}, e^{13}, e^{23}, e^{14}, e^{25}, e^{24} + e^{15}, e^{26} + e^{34}$                                                | 35679    |
| 97641:3     | $0, 0, e^{12}, e^{13}, e^{23}, e^{15} + e^{24}, e^{14}, e^{25}, e^{34} + e^{16}$                                                 | 34679    |
| 97641:4     | $0, 0, e^{12}, e^{13}, e^{23}, e^{14}, e^{25}, e^{15} + e^{24}, e^{16} + e^{27}$                                                 | 24679    |
| 97641:5     | $0, 0, e^{12}, e^{13}, e^{23}, e^{14}, e^{24} + e^{15}, e^{25}, e^{26} + e^{17}$                                                 | 24679    |
| 97641:6     | $0, 0, -(-1 + a_3)e^{12}, e^{13}, e^{23}, e^{14} a_3, e^{15} + e^{24}, e^{25}, e^{17} + e^{26} + e^{34}$                         | 24679    |
| 97641:7a    | $0, 0, -e^{12}, e^{13}, e^{23}, e^{14}, e^{15} + e^{24}, e^{25}, e^{35} + e^{27} + e^{16}$                                       | 24679    |
| 97641:7b    | $0, 0, -e^{12}, e^{13}, e^{23}, -e^{14}, e^{15} + e^{24}, e^{25}, e^{16} + e^{27} + e^{35}$                                      | 24679    |
| Type: 31212 |                                                                                                                                  |          |
| 96532:1     | $0, 0, 0, -e^{12}, e^{14}, e^{24}, e^{15}, e^{17}, e^{45} + e^{27}$                                                              | 45679    |
| 96532:2     | $0, 0, 0, -e^{12}, e^{14}, e^{24} + e^{13}, e^{15}, e^{17}, e^{45} + e^{27}$                                                     | 35679    |
| 96532:3     | $0, 0, 0, -e^{12}, e^{14}, e^{24}, e^{15}, e^{17}, e^{27} + e^{45} + e^{13}$                                                     | 35679    |
| 96532:4     | $0, 0, 0, -e^{12}, e^{14}, e^{24}, e^{15}, e^{17} + e^{23}, e^{27} + e^{45}$                                                     | 35679    |
| 96532:5a    | $0, 0, 0, -e^{12}, e^{14}, e^{13} + e^{24}, e^{15}, e^{17} + e^{23}, e^{27} + e^{45}$                                            | 35679    |
| 96532:5b    | $0, 0, 0, -e^{12}, -e^{14}, e^{24} + e^{13}, e^{15}, e^{23} + e^{17}, e^{45} + e^{27}$                                           | 35679    |
| 96532:6     | $0, 0, 0, -e^{12}, e^{14}, e^{24}, e^{15}, e^{45} + e^{27}, e^{26} + e^{17}$                                                     | 35679    |
| 96532:7     | $0, 0, 0, -e^{12}, e^{14}, e^{24}, e^{15} + e^{23}, e^{17} + e^{34}, e^{27} + e^{45}$                                            | 34679    |
| 96532:8a    | $0, 0, 0, -e^{12}, e^{14}, e^{24}, e^{15}, e^{23} + e^{17}, e^{13} + e^{45} + e^{27}$                                            | 35679    |
| 96532:8b    | $0, 0, 0, -e^{12}, e^{14}, e^{24}, e^{15}, -e^{17} + e^{23}, e^{27} + e^{45} + e^{13}$                                           | 35679    |
| 96532:9     | $0, 0, 0, -e^{12}, e^{14}, e^{24} + e^{13}, e^{15} + e^{23}, e^{17} + e^{34}, e^{27} + e^{45}$                                   | 34679    |
| 96532:10    | $0, 0, 0, -e^{12}, e^{14}, e^{24}, e^{15}, e^{13} + e^{45} + e^{27}, e^{17} + e^{26}$                                            | 25679    |
| 96532:11    | $0, 0, 0, -e^{12}, e^{14}, e^{24}, e^{15} + e^{23}, e^{17} + e^{34}, e^{13} + e^{45} + e^{27}$                                   | 34679    |
| 96532:12    | $0, 0, 0, -e^{12}, e^{14}, e^{13} + e^{24}, e^{15} + e^{23}, e^{45} + e^{27}, e^{17} + e^{26}$                                   | 24679    |
| 96532:13    | $0, 0, 0, -e^{12}, e^{14}, e^{24} - e^{13}, e^{15}, e^{27} + e^{45}, e^{17} + e^{26} + e^{34}$                                   | 24679    |
| 96532:14    | $0, 0, 0, -e^{12}, e^{14}, e^{24}, e^{15} + e^{23}, e^{45} + e^{27}, e^{34} + e^{17} + e^{26}$                                   | 24679    |
| 96532:15    | $0, 0, 0, -e^{12} a_3, e^{14}, e^{24} - (-1 + a_3)e^{13}, e^{15} a_3 + e^{23}, e^{45} + e^{27}, e^{26} + e^{17} + e^{34}$        | 24679    |
| 96532:17a   | $0, 0, 0, -e^{12}, e^{14}, e^{24}, e^{15} + e^{23}, e^{13} + e^{45} + e^{27}, e^{26} + e^{17} + e^{34}$                          | 24679    |
| 96532:17b   | $0, 0, 0, -e^{12}, -e^{14}, e^{24}, e^{15} + e^{23}, e^{45} + e^{27} + e^{13}, e^{34} + e^{17} + e^{26}$                         | 24679    |
| 96532:20    | $0, 0, 0, e^{12}, e^{24} + e^{13}, 2e^{14}, e^{25} + e^{34}, e^{27} + e^{35}, e^{36} + e^{17} + e^{45}$                          | 24579    |
| 96532:22a   | $0, 0, 0, -e^{12}, e^{14} + e^{23}, e^{13} + 2e^{24}, e^{15} + e^{34}, e^{17} + e^{35}, e^{45} + e^{27} + e^{36}$                | 24579    |
| 96532:22b   | $0, 0, 0, -e^{12}, e^{14} + e^{23}, -e^{13} + 2e^{24}, e^{15} + e^{34}, e^{17} + e^{35}, e^{45} + e^{27} + e^{36}$               | 24579    |
| 96532:23    | $0, 0, 0, e^{12}, e^{24} + e^{13}, 2e^{14}, e^{25} + e^{34}, e^{27} + e^{35} + e^{16}, e^{45} + e^{36} + e^{17}$                 | 24579    |
| 96532:25    | $0, 0, 0, e^{12}, -e^{14}, e^{24}, -e^{16} + e^{25}, e^{45} + e^{17}, e^{46} + e^{27}$                                           | 34679    |
| 96532:26a   | $0, 0, 0, e^{12}, e^{14}, e^{24}, -e^{15} + e^{26}, e^{45} + e^{27}, e^{46} + e^{17}$                                            | 34679    |
| 96532:26b   | $0, 0, 0, e^{12}, -e^{14}, e^{24}, e^{26} - e^{15}, e^{27} + e^{45}, e^{46} + e^{17}$                                            | 34679    |
| 96532:27    | $0, 0, 0, e^{12}, -e^{14}, e^{24}, -e^{16} + e^{25}, e^{17} + e^{45}, e^{27} + e^{46} + e^{13}$                                  | 24679    |
| 96532:28a   | $0, 0, 0, e^{12}, e^{14}, e^{24}, -e^{15} + e^{26}, e^{27} + e^{45}, e^{17} + e^{46} + e^{23}$                                   | 24679    |
| 96532:28b   | $0, 0, 0, e^{12}, -e^{14}, e^{24}, e^{26} - e^{15}, e^{27} + e^{45}, e^{46} + e^{23} + e^{17}$                                   | 24679    |
| 96532:29    | $0, 0, 0, e^{12}, -e^{14}, e^{24}, -e^{16} + e^{25}, e^{17} + e^{45}, e^{27} + e^{46} + e^{15}$                                  | 34679    |
| 96532:30a   | $0, 0, 0, e^{12}, e^{14}, e^{24}, e^{26} - e^{15}, e^{45} + e^{27} + a_3 e^{13}, e^{46} + e^{17} + e^{23}$                       | 24679    |
| 96532:30b   | $0, 0, 0, e^{12}, -e^{14}, e^{24}, -e^{15} + e^{26}, e^{27} + e^{45} + a_3 e^{13}, e^{17} + e^{46} + e^{23}$                     | 24679    |
| 96532:31a   | $0, 0, 0, e^{12}, -e^{14}, e^{24}, -e^{16} + e^{25}, e^{17} + e^{45} + e^{23}, e^{27} + e^{46} + e^{13}$                         | 24679    |
| 96532:31b   | $0, 0, 0, -e^{12}, e^{14}, e^{24}, e^{16} + e^{25}, e^{45} + e^{23} - e^{17}, e^{27} + e^{13} + e^{46}$                          | 24679    |
| 96532:32    | $0, 0, 0, e^{12}, -e^{14}, e^{24}, -e^{16} + e^{25}, e^{17} + e^{45} + e^{23}, e^{27} + e^{46} + e^{15}$                         | 24679    |
| 96532:33    | $0, 0, 0, e^{12}, -e^{14}, e^{24}, e^{25} - e^{16}, e^{26} + e^{17} + e^{45}, e^{27} + e^{15} + e^{46}$                          | 34679    |

Table 2 – Continued to next page

Table 2 – Continued from previous page

| Name        | $\mathfrak{g}$                                                                                                                                                            | UCS Dim. |
|-------------|---------------------------------------------------------------------------------------------------------------------------------------------------------------------------|----------|
| 96532:34    | $0, 0, 0, e^{12}, -e^{14}, e^{24} - e^{13}, e^{25} - e^{16}, e^{17} + e^{45}, e^{27} + e^{35} + e^{46}$                                                                   | 23579    |
| 96532:37    | $0, 0, 0, e^{12}, -e^{14}, e^{24} - e^{13}, -e^{16} + e^{25}, e^{17} + e^{23} + e^{45}, e^{27} + e^{35} + e^{46}$                                                         | 23579    |
| 96532:38a   | $0, 0, 0, e^{12}, 3e^{24} - e^{13}, e^{14} + 2e^{23}, -e^{16} + e^{25} + e^{34}, e^{17} + e^{45}, e^{27} + e^{35} + e^{46}$                                               | 23579    |
| 96532:38b   | $0, 0, 0, e^{12}, 3e^{24} - e^{13}, -e^{14} + 2e^{23}, -e^{16} + e^{25} + e^{34}, e^{45} + e^{17}, e^{46} + e^{27} + e^{35}$                                              | 23579    |
| 96532:40a   | $0, 0, 0, e^{12}, e^{14} + e^{23}, -e^{13} + e^{24}, e^{26} - e^{15}, e^{17} + e^{46} - e^{35}, e^{27} + e^{45} + e^{36}$                                                 | 23579    |
| 96532:40b   | $0, 0, 0, e^{12}, e^{23} - e^{14}, e^{24} - e^{13}, -e^{15} + e^{26}, e^{35} + e^{46} + e^{17}, e^{36} + e^{45} + e^{27}$                                                 | 23579    |
| 96532:41a   | $0, 0, 0, e^{12}, -e^{24} + e^{13}, e^{14} + e^{23}, e^{26} - e^{15}, -e^{35} + e^{17} + e^{46}, e^{36} + e^{27} + e^{45}$                                                | 23579    |
| 96532:41b   | $0, 0, 0, e^{12}, e^{24} - e^{13}, e^{23} - e^{14}, -e^{15} + e^{26}, e^{35} + e^{46} + e^{17}, e^{36} + e^{45} + e^{27}$                                                 | 23579    |
| 96532:42a   | $0, 0, 0, e^{12}, e^{14}, e^{24} + e^{13}, e^{26} + e^{34} - e^{15}, e^{17} + e^{46} + 2e^{35}, e^{27} + e^{36} + e^{45}$                                                 | 23579    |
| 96532:42b   | $0, 0, 0, e^{12}, -e^{14}, e^{24} + e^{13}, e^{26} + e^{34} - e^{15}, e^{17} + e^{46} - 2e^{35}, e^{27} + e^{36} + e^{45}$                                                | 23579    |
| 96532:43a   | $0, 0, 0, e^{12}, e^{14} - (-1 + a_2)e^{23}, -e^{24}(-2 + a_2) + e^{13}a_2,$<br>$e^{26} - e^{15} + e^{34}, e^{17} + e^{46} + (1 + a_2)e^{35}, e^{45} + e^{27} + e^{36}$   | 23579    |
| 96532:43b   | $0, 0, 0, e^{12}, -e^{14} - (-1 + a_2)e^{23}, -e^{24}(-2 + a_2) + e^{13}a_2,$<br>$-e^{15} + e^{26} + e^{34}, e^{46} + e^{17} - (1 + a_2)e^{35}, e^{36} + e^{45} + e^{27}$ | 23579    |
| Type: 31221 |                                                                                                                                                                           |          |
| 96531:1     | $0, 0, 0, e^{12}, e^{14}, e^{24}, e^{15}, e^{26}, e^{17}$                                                                                                                 | 35679    |
| 96531:2     | $0, 0, 0, e^{12}, e^{14}, e^{24}, e^{15}, e^{13} + e^{26}, e^{17}$                                                                                                        | 25679    |
| 96531:3     | $0, 0, 0, e^{12}, e^{14}, e^{24}, e^{15}, e^{26}, e^{17} + e^{23}$                                                                                                        | 25679    |
| 96531:4     | $0, 0, 0, e^{12}, e^{14}, e^{24}, e^{15}, e^{25} + e^{16}, e^{17}$                                                                                                        | 35679    |
| 96531:5     | $0, 0, 0, e^{12}, e^{14}, e^{24} + e^{13}, e^{15}, e^{26} + e^{34}, e^{17}$                                                                                               | 24679    |
| 96531:6     | $0, 0, 0, e^{12}, e^{14}, e^{24}, e^{15}, e^{13} + e^{26}, e^{17} + e^{23}$                                                                                               | 25679    |
| 96531:7     | $0, 0, 0, -e^{12}, e^{14}, e^{24}, e^{15}, e^{26}, e^{45} + e^{27}$                                                                                                       | 35679    |
| 96531:8     | $0, 0, 0, e^{12}, e^{14}, e^{24} + e^{13}, e^{15}, e^{25} + e^{16}, e^{17}$                                                                                               | 24679    |
| 96531:9     | $0, 0, 0, -e^{12}, e^{14}, e^{24}, e^{15} + e^{23}, e^{26}, e^{17} + e^{34}$                                                                                              | 24679    |
| 96531:10    | $0, 0, 0, e^{12}, e^{14}, e^{24}, e^{15}, e^{16} + e^{25}, e^{17} + e^{23}$                                                                                               | 25679    |
| 96531:11a   | $0, 0, 0, e^{12}, e^{14}, e^{24} + e^{13}, e^{15}, e^{34} + e^{26}, e^{23} + e^{17}$                                                                                      | 24679    |
| 96531:11b   | $0, 0, 0, e^{12}, -e^{14}, e^{24} + e^{13}, e^{15}, e^{26} + e^{34}, e^{17} + e^{23}$                                                                                     | 24679    |
| 96531:12    | $0, 0, 0, -e^{12}, e^{14}, e^{24}, e^{15}, e^{26} + e^{13}, e^{27} + e^{45}$                                                                                              | 25679    |
| 96531:13    | $0, 0, 0, e^{12}, e^{14}, e^{24}, e^{15}, e^{16} + e^{25}, e^{17} + e^{26}$                                                                                               | 35679    |
| 96531:14    | $0, 0, 0, -e^{12}, e^{14}, e^{24}, e^{23} + e^{15}, e^{13} + e^{26}, e^{17} + e^{34}$                                                                                     | 24679    |
| 96531:15    | $0, 0, 0, -e^{12}, e^{14}, e^{24}, e^{15} + e^{23}, e^{26}, e^{45} + e^{27}$                                                                                              | 24679    |
| 96531:16    | $0, 0, 0, -e^{12}, e^{14}, e^{24}, e^{15}, e^{26}, e^{27} + e^{45} + e^{13}$                                                                                              | 25679    |
| 96531:17a   | $0, 0, 0, e^{12}, e^{14}, e^{24} + e^{13}, e^{15}, e^{16} + e^{25}, e^{17} + e^{23}$                                                                                      | 24679    |
| 96531:17b   | $0, 0, 0, e^{12}, e^{14}, -e^{13} + e^{24}, e^{15}, e^{16} + e^{25}, e^{17} + e^{23}$                                                                                     | 24679    |
| 96531:18    | $0, 0, 0, -e^{12}, e^{14}, e^{24}, e^{15}, e^{25} + e^{16}, e^{27} + e^{45}$                                                                                              | 35679    |
| 96531:19    | $0, 0, 0, -e^{12}, e^{14}, e^{24}, e^{15} + e^{23}, e^{25} + e^{16}, e^{17} + e^{34}$                                                                                     | 24679    |
| 96531:20    | $0, 0, 0, -e^{12}, e^{14}, e^{24}, e^{15} + e^{23}, e^{13} + e^{26}, e^{45} + e^{27}$                                                                                     | 24679    |
| 96531:21    | $0, 0, 0, -e^{12}, e^{14}, -e^{13} + e^{24}, e^{15}, e^{34} + e^{26}, e^{45} + e^{27}$                                                                                    | 24679    |
| 96531:22    | $0, 0, 0, -e^{12}, e^{14}, e^{24}, e^{23} + e^{15}, e^{26}, e^{13} + e^{45} + e^{27}$                                                                                     | 24679    |
| 96531:23    | $0, 0, 0, -e^{12}, e^{14}, e^{13} + e^{24}, e^{15} + e^{23}, e^{25} + e^{16}, e^{17} + e^{34}$                                                                            | 24679    |
| 96531:24    | $0, 0, 0, -e^{12}, e^{14}, e^{13} + e^{24}, e^{15}, e^{25} + e^{16}, e^{27} + e^{45}$                                                                                     | 24679    |
| 96531:25    | $0, 0, 0, -e^{12}, e^{14}, e^{24}, e^{15} + e^{23}, e^{25} + e^{16}, e^{45} + e^{27}$                                                                                     | 24679    |
| 96531:26    | $0, 0, 0, -e^{12}, e^{14}, e^{24} - e^{13}, e^{23} + e^{15}, e^{26} + e^{34}, e^{45} + e^{27}$                                                                            | 24679    |
| 96531:27    | $0, 0, 0, e^{12}, e^{14}, e^{24} + e^{13}, e^{15} + e^{23}, e^{25} + e^{16}, e^{26} + e^{17}$                                                                             | 24679    |
| 96531:28    | $0, 0, 0, -e^{12}, e^{14}, e^{24}, e^{15}, e^{25} + e^{16}, e^{45} + e^{27} + e^{13}$                                                                                     | 25679    |
| 96531:29    | $0, 0, 0, e^{12}, e^{24} + e^{13}, e^{14}, e^{25} + e^{34}, e^{16}, e^{27} + e^{35}$                                                                                      | 24579    |
| 96531:30    | $0, 0, 0, -e^{12}, e^{14}, e^{24}, e^{15} + e^{23}, e^{25} + e^{16}, e^{34} + e^{17} + e^{26}$                                                                            | 24679    |
| 96531:31    | $0, 0, 0, e^{12}, e^{14}, e^{24} + e^{13}, e^{15}, e^{25} + e^{16}, e^{26} + e^{34} + e^{17}$                                                                             | 24679    |
| 96531:32    | $0, 0, 0, -e^{12}, e^{14}, e^{13} + e^{24}, e^{15} + e^{23}, e^{25} + e^{16}, e^{27} + e^{45}$                                                                            | 24679    |
| 96531:33    | $0, 0, 0, -e^{12}, e^{14}, e^{24}, e^{15} + e^{23}, e^{25} + e^{16}, e^{13} + e^{45} + e^{27}$                                                                            | 24679    |
| 96531:34    | $0, 0, 0, e^{12}, e^{24} + e^{13}, e^{14}, e^{25} + e^{34}, e^{16} + e^{23}, e^{27} + e^{35}$                                                                             | 24579    |
| 96531:36    | $0, 0, 0, a_1 e^{12}, e^{14}, (1 + a_1)e^{13} + e^{24}, e^{15} + e^{23}, e^{16} + e^{25}, e^{17} + e^{26} + e^{34}$                                                       | 24679    |
| 96531:38    | $0, 0, 0, e^{12}, e^{24} + e^{13}, e^{14}, e^{25} + e^{34}, e^{26} + e^{15}, e^{27} + e^{35}$                                                                             | 24579    |
| 96531:39    | $0, 0, 0, e^{12}, e^{24} + e^{13}, 2e^{14}, e^{25} + e^{34}, e^{16}, e^{45} + e^{36} + e^{17}$                                                                            | 24579    |
| 96531:42a   | $0, 0, 0, -e^{12}, e^{14} + e^{23}, e^{13} + e^{24}, e^{34} + e^{15}, e^{25} + e^{16}, e^{17} + e^{35}$                                                                   | 24579    |
| 96531:42b   | $0, 0, 0, -e^{12}, e^{14} + e^{23}, -e^{13} + e^{24}, e^{15} + e^{34}, e^{25} + e^{16}, e^{17} + e^{35}$                                                                  | 24579    |
| 96531:43    | $0, 0, 0, e^{12}, e^{24} + e^{13}, 2e^{14}, e^{25} + e^{34}, e^{16} + e^{23}, e^{36} + e^{17} + e^{45}$                                                                   | 24579    |
| 96531:44    | $0, 0, 0, e^{12}, e^{24} + e^{13}, e^{14}, e^{25} + e^{34}, e^{26} + e^{15}, e^{27} + e^{35} + e^{16}$                                                                    | 24579    |

Table 2 – Continued to next page



Table 2 – Continued from previous page

| Name      | $\mathfrak{g}$                                                                                                                                     | UCS Dim. |
|-----------|----------------------------------------------------------------------------------------------------------------------------------------------------|----------|
| 96531:46  | $0, 0, 0, e^{12}, e^{24} + e^{13}, 2e^{14}, e^{25} + e^{34}, e^{26} + 2e^{15}, e^{36} + e^{17} + e^{45}$                                           | 24579    |
| 96531:48a | $0, 0, 0, -e^{12}, 2e^{14} + e^{23}, e^{13} + 2e^{24}, e^{34} + e^{15}, e^{25} + e^{16}, e^{27} + e^{45} + e^{36}$                                 | 24579    |
| 96531:48b | $0, 0, 0, -e^{12}, 2e^{14} + e^{23}, -e^{13} + 2e^{24}, e^{34} + e^{15}, e^{25} + e^{16}, e^{27} + e^{45} + e^{36}$                                | 24579    |
| 96531:49  | $0, 0, 0, e^{12}, e^{14}, e^{24}, e^{25} + e^{16}, e^{15}, e^{17} + e^{45}$                                                                        | 34679    |
| 96531:50  | $0, 0, 0, -e^{12}, e^{14}, e^{24}, e^{25} + e^{16}, e^{15}, e^{46} + e^{27}$                                                                       | 34679    |
| 96531:51  | $0, 0, 0, e^{12}, e^{14}, e^{24}, e^{25} + e^{16}, e^{15} + e^{23}, e^{45} + e^{17}$                                                               | 24679    |
| 96531:52  | $0, 0, 0, -e^{12}, e^{14}, e^{24}, e^{25} + e^{16}, e^{15} + e^{23}, e^{46} + e^{27}$                                                              | 24679    |
| 96531:53  | $0, 0, 0, e^{12}, e^{14}, e^{24}, e^{25} + e^{16}, e^{15}, e^{17} + e^{23} + e^{45}$                                                               | 24679    |
| 96531:54  | $0, 0, 0, -e^{12}, e^{14}, e^{24}, e^{25} + e^{16}, e^{15}, e^{46} + e^{27} + e^{13}$                                                              | 24679    |
| 96531:55a | $0, 0, 0, e^{12}, e^{14}, e^{24}, e^{25} + e^{16}, e^{26} + e^{15}, e^{45} + e^{17}$                                                               | 34679    |
| 96531:55b | $0, 0, 0, e^{12}, -e^{14}, e^{24}, -e^{16} + e^{25}, e^{15} + e^{26}, e^{17} + e^{45}$                                                             | 34679    |
| 96531:56a | $0, 0, 0, e^{12}, e^{14}, e^{24}, e^{26} - e^{15}, e^{16} + e^{25}, e^{27} + e^{45}$                                                               | 34679    |
| 96531:56b | $0, 0, 0, -e^{12}, e^{14}, e^{24}, e^{15} + e^{26}, e^{16} + e^{25}, e^{27} + e^{45}$                                                              | 34679    |
| 96531:57  | $0, 0, 0, -e^{12}, e^{14}, e^{24}, e^{25} + e^{16}, e^{15} + e^{23}, e^{13} + e^{46} + e^{27}$                                                     | 24679    |
| 96531:58  | $0, 0, 0, e^{12}, e^{14}, e^{24}, e^{16} + e^{25}, e^{15}, e^{17} + e^{26} + e^{45}$                                                               | 34679    |
| 96531:59  | $0, 0, 0, e^{12}, e^{14}, e^{24} + e^{13}, e^{25} + e^{16}, e^{15}, e^{17} + e^{45}$                                                               | 23579    |
| 96531:60a | $0, 0, 0, e^{12}, e^{14}, e^{24}, e^{16} + e^{25}, e^{15} + e^{26}, e^{45} + e^{17} + e^{23}$                                                      | 24679    |
| 96531:60b | $0, 0, 0, e^{12}, -e^{14}, e^{24}, -e^{16} + e^{25}, e^{26} + e^{15}, e^{17} + e^{45} + e^{23}$                                                    | 24679    |
| 96531:61a | $0, 0, 0, e^{12}, e^{14}, e^{24}, e^{26} - e^{15}, e^{25} + e^{16}, e^{27} + e^{45} + e^{13}$                                                      | 24679    |
| 96531:61b | $0, 0, 0, -e^{12}, e^{14}, e^{24}, e^{26} + e^{15}, e^{25} + e^{16}, e^{13} + e^{27} + e^{45}$                                                     | 24679    |
| 96531:62  | $0, 0, 0, e^{12}, e^{14}, e^{24}, e^{16} + e^{25}, e^{15} + e^{23}, e^{17} + e^{26} + e^{45}$                                                      | 24679    |
| 96531:63  | $0, 0, 0, e^{12}, e^{14}, e^{24} + e^{13}, e^{25} + e^{16}, e^{15} + e^{23}, e^{45} + e^{17}$                                                      | 23579    |
| 96531:64  | $0, 0, 0, e^{12}, e^{24} + e^{13}, e^{14}, e^{15} + e^{26}, e^{25} + e^{34}, e^{46} + e^{17}$                                                      | 23579    |
| 96531:65  | $0, 0, 0, e^{12}, e^{14}, e^{24} + e^{13}, e^{16} + e^{25}, e^{15}, e^{45} + e^{17} + e^{23}$                                                      | 23579    |
| 96531:66  | $0, 0, 0, -e^{12}, e^{14}, e^{13} + e^{24}, e^{25} + e^{16}, e^{15}, e^{46} + e^{27} + e^{35}$                                                     | 23579    |
| 96531:67  | $0, 0, 0, e^{12}, e^{24} + e^{13}, e^{14}, e^{26} + e^{15}, e^{25} + e^{34}, e^{17} + e^{23} + e^{46}$                                             | 23579    |
| 96531:68  | $0, 0, 0, -e^{12}, e^{14}, e^{13} + e^{24}, e^{25} + e^{16}, e^{15} + e^{23}, e^{46} + e^{27} + e^{35}$                                            | 23579    |
| 96531:69a | $0, 0, 0, e^{12}, e^{14}, e^{24} + e^{13}, e^{25} + e^{16}, e^{26} + e^{34} + e^{15}, e^{17} + e^{45}$                                             | 23579    |
| 96531:69b | $0, 0, 0, e^{12}, -e^{14}, e^{24} + e^{13}, -e^{16} + e^{25}, e^{15} + e^{26} + e^{34}, e^{17} + e^{45}$                                           | 23579    |
| 96531:70  | $0, 0, 0, -e^{12}, -e^{24} - e^{13}, -e^{14}, e^{15} + e^{26}, e^{25} + e^{34}, e^{36} + e^{45} + e^{27}$                                          | 23579    |
| 96531:72a | $0, 0, 0, e^{12}, e^{14} + e^{23}, e^{24} + e^{13}, e^{16} + e^{25}, -e^{15} + e^{34}, e^{17} + e^{36} + e^{45}$                                   | 23579    |
| 96531:72b | $0, 0, 0, e^{12}, e^{14} + e^{23}, e^{24} - e^{13}, e^{16} + e^{25}, -e^{15} + e^{34}, e^{45} + e^{17} + e^{36}$                                   | 23579    |
| 96531:73a | $0, 0, 0, e^{12}, -e^{23} - e^{14}, e^{24} - e^{13}, -e^{16} + e^{25}, e^{15} + e^{34}, e^{35} + e^{46} + e^{27}$                                  | 23579    |
| 96531:73b | $0, 0, 0, -e^{12}, e^{14} + e^{23}, e^{24} + e^{13}, e^{25} + e^{16}, e^{34} + e^{15}, e^{27} + e^{35} + e^{46}$                                   | 23579    |
| 96531:74a | $0, 0, 0, e^{12}, e^{24} - e^{13}, e^{23} + e^{14}, e^{34} + e^{25} - 2e^{16}, e^{26} + e^{15}, e^{45} + e^{17}$                                   | 23579    |
| 96531:74b | $0, 0, 0, e^{12}, e^{24} - e^{13}, e^{23} - e^{14}, e^{34} + e^{25} - 2e^{16}, e^{26} - e^{15}, e^{45} + e^{17}$                                   | 23579    |
| 96531:75a | $0, 0, 0, e^{12}, e^{14}, e^{24} + e^{13}, e^{25} + e^{16}, e^{26} + e^{34} + e^{15}, e^{17} + e^{23} + e^{45}$                                    | 23579    |
| 96531:75b | $0, 0, 0, e^{12}, -e^{14}, e^{24} + e^{13}, -e^{16} + e^{25}, e^{15} + e^{26} + e^{34}, e^{45} + e^{17} + e^{23}$                                  | 23579    |
| 96531:77a | $0, 0, 0, e^{12}, e^{14}, -e^{24} + e^{13}, -e^{16} + e^{25}, e^{15} + e^{26} + e^{34}, e^{46} + e^{27} + e^{35}$                                  | 23579    |
| 96531:77b | $0, 0, 0, -e^{12}, -e^{14}, -e^{24} - e^{13}, e^{16} + e^{25}, e^{15} + e^{26} + e^{34}, e^{27} + e^{35} + e^{46}$                                 | 23579    |
| 96531:78a | $0, 0, 0, e^{12}, e^{14} + e^{23}, e^{24} + e^{13}, e^{25} + e^{16}, e^{26} + e^{15}, e^{36} + e^{17} + e^{45}$                                    | 23579    |
| 96531:78b | $0, 0, 0, e^{12}, -e^{14} + e^{23}, e^{24} + e^{13}, -e^{16} + e^{25}, e^{15} + e^{26}, e^{17} + e^{36} + e^{45}$                                  | 23579    |
| 96531:79a | $0, 0, 0, e^{12}, e^{24} + e^{13}, e^{14} + e^{23}, e^{25} + e^{16}, e^{26} + e^{15}, e^{36} + e^{17} + e^{45}$                                    | 23579    |
| 96531:79b | $0, 0, 0, -e^{12}, -e^{24} - e^{13}, -e^{14} + e^{23}, -e^{16} + e^{25}, e^{15} + e^{26}, e^{17} + e^{36} + e^{45}$                                | 23579    |
| 96531:80a | $0, 0, 0, e^{12}, 2e^{14}, e^{24} + e^{13}, e^{26} + e^{34} + e^{15}, e^{25} + 2e^{16}, e^{35} + e^{17} + e^{46}$                                  | 23579    |
| 96531:80b | $0, 0, 0, e^{12}, 2e^{14}, e^{24} + e^{13}, e^{26} + e^{34} - e^{15}, e^{25} + 2e^{16}, e^{35} + e^{17} + e^{46}$                                  | 23579    |
| 96531:81a | $0, 0, 0, e^{12}, e^{14}, e^{24} + e^{13}, -e^{15} + e^{26} + e^{34}, e^{16} + e^{25}, e^{45} + e^{36} + e^{27}$                                   | 23579    |
| 96531:81b | $0, 0, 0, -e^{12}, e^{14}, -e^{13} + e^{24}, e^{26} + e^{15} + e^{34}, e^{16} + e^{25}, e^{27} + e^{36} + e^{45}$                                  | 23579    |
| 96531:82a | $0, 0, 0, e^{12}, e^{24} + (1 + a_4)e^{13}, e^{14} + e^{23}, e^{26} + e^{15}, e^{25} + e^{34} + e^{16}, a_4, e^{35} + e^{17} + e^{46}$             | 23579    |
| 96531:82b | $0, 0, 0, e^{12}, e^{24} + (1 + a_4)e^{13}, -e^{14} + e^{23}, -e^{15} + e^{26}, e^{25} + e^{34} + e^{16}, a_4, e^{46} + e^{17} + e^{35}$           | 23579    |
| 96531:83a | $0, 0, 0, e^{12}, (-1 + a_5)e^{13} + e^{24}a_5, e^{23} + e^{14}a_5, e^{16}(-2 + a_5) + e^{25} + e^{34}, e^{26} + e^{15}, e^{36} + e^{17} + e^{45}$ | 23579    |
| 96531:83b | $0, 0, 0, e^{12}, e^{24}a_5 - e^{13}(1 + a_5), e^{23} - e^{14}a_5, e^{34} + e^{25} - (2 + a_5)e^{16}, e^{26} - e^{15}, e^{36} + e^{45} + e^{17}$   | 23579    |
| 96531:84  | $0, 0, 0, e^{12}, e^{14}, e^{24}, e^{15}, e^{26}, e^{17} + e^{28}$                                                                                 | 24679    |
| 96531:85  | $0, 0, 0, e^{12}, e^{14}, e^{24}, e^{15}, e^{25} + e^{16}, e^{18} + e^{27}$                                                                        | 24679    |
| 96531:86  | $0, 0, 0, e^{12}, e^{14}, e^{24}, e^{15} + e^{23}, e^{13} + e^{26}, e^{17} + e^{28}$                                                               | 13679    |
| 96531:87  | $0, 0, 0, e^{12}, e^{14}, e^{24}, e^{15}, e^{13} + e^{26}, e^{28} + e^{17} + e^{34}$                                                               | 13679    |
| 96531:88  | $0, 0, 0, e^{12}, e^{14}, e^{24}, e^{15} + e^{23}, e^{25} + e^{16}, e^{18} + e^{27}$                                                               | 13679    |
| 96531:89  | $0, 0, 0, e^{12}a_1, e^{14}, e^{24}, e^{15} + e^{23}, e^{26} + (1 + a_1)e^{13}, e^{17} + e^{28} + e^{34}$                                          | 13679    |

Table 2 – Continued to next page

Table 2 – Continued from previous page

| Name          | $\mathfrak{g}$                                                                                                                                                                                  | UCS Dim. |
|---------------|-------------------------------------------------------------------------------------------------------------------------------------------------------------------------------------------------|----------|
| 96531:90a     | $0, 0, 0, e^{12}, e^{14}, e^{24}, e^{25} + e^{16}, e^{26} + e^{15}, e^{17} + e^{28}$                                                                                                            | 24679    |
| 96531:90b     | $0, 0, 0, e^{12}, -e^{14}, e^{24}, e^{25} - e^{16}, e^{26} + e^{15}, e^{17} + e^{28}$                                                                                                           | 24679    |
| 96531:91      | $0, 0, 0, e^{12}a_1, e^{14}, e^{24}, -(-1 + a_1)e^{15}, e^{25} + e^{16}, e^{18} + e^{45} + e^{27}$                                                                                              | 24679    |
| 96531:92a     | $0, 0, 0, -e^{12}, e^{14}, e^{24}, e^{15}, e^{25} + e^{16}, e^{17} + e^{28} + e^{46}$                                                                                                           | 24679    |
| 96531:92b     | $0, 0, 0, -e^{12}, e^{14}, e^{24}, -e^{15}, e^{25} + e^{16}, e^{46} + e^{17} + e^{28}$                                                                                                          | 24679    |
| 96531:93      | $0, 0, 0, e^{12}, e^{14}, e^{24} + e^{13}, e^{15}, e^{25} + e^{16}, e^{18} + e^{27}$                                                                                                            | 13579    |
| 96531:94      | $0, 0, 0, e^{12}a_1, e^{14}, e^{24}, -(-1 + a_1)e^{15} + e^{23}, e^{16} + e^{25}, e^{18} + e^{27} + e^{45}$                                                                                     | 13679    |
| 96531:95      | $0, 0, 0, e^{12}, e^{14}, e^{24} + e^{13}, e^{15} + e^{23}, e^{16} + e^{25}, e^{18} + e^{27}$                                                                                                   | 13579    |
| 96531:96      | $0, 0, 0, e^{12}, e^{24} + e^{13}, e^{14}, e^{25} + e^{34}, e^{16}, e^{18} + e^{27} + e^{35}$                                                                                                   | 13579    |
| 96531:97a     | $0, 0, 0, e^{12}a_1, e^{14}, e^{24}, e^{16} + e^{25}, e^{26} - (-1 + a_1)e^{15}, e^{45} + e^{28} + e^{17}$                                                                                      | 24679    |
| 96531:97b     | $0, 0, 0, e^{12}a_1, -e^{14}, e^{24}, -e^{16} + e^{25}, e^{26} - (-1 + a_1)e^{15}, e^{17} + e^{28} + e^{45}$                                                                                    | 24679    |
| 96531:98      | $0, 0, 0, -(-1 + a_3)e^{12}, e^{14}, e^{24} + e^{13}, e^{15}a_3, e^{16} + e^{25}, e^{45} + e^{18} + e^{27}$                                                                                     | 13579    |
| 96531:99a     | $0, 0, 0, e^{12}, e^{14} + e^{23}, e^{24} + e^{13}, e^{16} + e^{25}, e^{15} + e^{26}, e^{28} + e^{17}$                                                                                          | 13579    |
| 96531:99b     | $0, 0, 0, e^{12}, e^{23} - e^{14}, e^{24} + e^{13}, e^{25} - e^{16}, e^{26} + e^{15}, e^{28} + e^{17}$                                                                                          | 13579    |
| 96531:100     | $0, 0, 0, e^{12}, e^{24} + e^{13}, e^{14}, e^{25} + e^{34}, e^{15} + e^{26}, e^{28} + e^{17} + e^{36}$                                                                                          | 13579    |
| 96531:101     | $0, 0, 0, -(-1 + a_3)e^{12}, e^{14}, e^{24} + e^{13}, e^{23} + e^{15}a_3, e^{16} + e^{25}, e^{18} + e^{27} + e^{45}$                                                                            | 13579    |
| 96531:102     | $0, 0, 0, -e^{12}, e^{24} - e^{13}, 2e^{14}, e^{25} + e^{34}, 2e^{15} + e^{26}, e^{45} + e^{28} + e^{17}$                                                                                       | 13579    |
| 96531:103a    | $0, 0, 0, -e^{12}, e^{14} + e^{23}, e^{13} + e^{24}, e^{15} + e^{34}, e^{25} + e^{16}, e^{18} + e^{27} + e^{36}$                                                                                | 13579    |
| 96531:103b    | $0, 0, 0, -e^{12}, e^{14} + e^{23}, -e^{13} + e^{24}, e^{34} + e^{15}, e^{25} + e^{16}, e^{36} + e^{18} + e^{27}$                                                                               | 13579    |
| 96531:104a    | $0, 0, 0, -e^{12}, e^{14}, e^{13} + e^{24}, e^{15}, e^{25} + e^{16}, e^{17} + e^{28} + e^{46} + e^{35}$                                                                                         | 13579    |
| 96531:104b    | $0, 0, 0, -e^{12}, e^{14}, e^{13} + e^{24}, -e^{15}, e^{25} + e^{16}, e^{46} + e^{35} + e^{17} + e^{28}$                                                                                        | 13579    |
| 96531:105a    | $0, 0, 0, \frac{1}{2}e^{12}, e^{14} - e^{23}, e^{24} + e^{13}, \frac{1}{2}e^{15} + e^{34}, e^{16} + e^{25}, e^{45} + e^{18} + e^{27}$                                                           | 13579    |
| 96531:105b    | $0, 0, 0, \frac{1}{2}e^{12}, e^{14} - e^{23}, e^{24} - e^{13}, \frac{1}{2}e^{15} + e^{34}, e^{16} + e^{25}, e^{18} + e^{27} + e^{45}$                                                           | 13579    |
| 96531:106a    | $0, 0, 0, e^{12}, e^{23} - e^{14}, e^{24} - e^{13}, -e^{15} + e^{34}, -e^{16} + e^{25}, e^{28} + e^{17} + e^{46}$                                                                               | 13579    |
| 96531:106b    | $0, 0, 0, -e^{12}, e^{23} + e^{14}, e^{24} - e^{13}, e^{34} + e^{15}, e^{25} + e^{16}, e^{46} + e^{28} + e^{17}$                                                                                | 13579    |
| 96531:107a    | $0, 0, 0, e^{12}, e^{14}, e^{24} + e^{13}, e^{16} + e^{25}, e^{15} + e^{26} + e^{34}, e^{18} + e^{27} + e^{35}$                                                                                 | 13579    |
| 96531:107b    | $0, 0, 0, e^{12}, e^{14}, e^{24} + e^{13}, e^{16} + e^{25}, -e^{15} + e^{26} + e^{34}, e^{18} + e^{27} + e^{35}$                                                                                | 13579    |
| 96531:108a    | $0, 0, 0, e^{12}, e^{24} + e^{13}, e^{14}, e^{15} + e^{26}, e^{16} + e^{25} + e^{34}, e^{28} + e^{17} + e^{35}$                                                                                 | 13579    |
| 96531:108b    | $0, 0, 0, e^{12}, e^{24} + e^{13}, -e^{14}, e^{26} - e^{15}, e^{34} + e^{25} + e^{16}, e^{35} + e^{28} + e^{17}$                                                                                | 13579    |
| 96531:109(*)  | $0, 0, 0, (-1 + a_3)e^{12}, (-1 + a_3)e^{13} - \frac{a_3}{a_3-2}e^{24}, e^{14}a_3, e^{25} + e^{34}, -(-2 + a_3)e^{15} + e^{26}, e^{45} + e^{28} + e^{17} + e^{36}$                              | 13579    |
| 96531:110a    | $0, 0, 0, e^{12}, e^{24} + e^{13}, e^{14}, e^{25} + e^{34}, e^{15} + e^{26}, e^{18} + e^{27} + e^{35} + e^{46}$                                                                                 | 13579    |
| 96531:110b    | $0, 0, 0, e^{12}, e^{24} + e^{13}, -e^{14}, e^{25} + e^{34}, e^{26} - e^{15}, e^{27} + e^{35} + e^{18} + e^{46}$                                                                                | 13579    |
| 96531:111a    | $0, 0, 0, -e^{12}, e^{24} - e^{13}, 2e^{14}, 2e^{15} + e^{26}, e^{16} + e^{25} + e^{34}, e^{45} + e^{27} + e^{18}$                                                                              | 13579    |
| 96531:111b    | $0, 0, 0, -e^{12}, e^{24} - e^{13}, 2e^{14}, 2e^{15} + e^{26}, -e^{16} + e^{25} + e^{34}, e^{45} + e^{27} + e^{18}$                                                                             | 13579    |
| 96531:112a    | $0, 0, 0, e^{12}a_1, e^{24} + (1 + a_1)e^{13}, e^{14} + e^{23}, e^{15} + e^{26}, e^{16} + e^{25} + e^{34}, e^{28} + e^{17} + e^{35}$                                                            | 13579    |
| 96531:112b    | $0, 0, 0, e^{12}a_1, e^{24} + (1 + a_1)e^{13}, -e^{14} + e^{23}, e^{26} - e^{15}, e^{25} + e^{34} + e^{16}, e^{35} + e^{17} + e^{28}$                                                           | 13579    |
| 96531:113a    | $0, 0, 0, -e^{12}a_1, (e^{14} + e^{23})a_1, e^{24} + (-1 + a_1)e^{13}, e^{34} + e^{15}, e^{25} + e^{16}a_1, e^{46} + e^{35} + e^{17} + e^{28}$                                                  | 13579    |
| 96531:113b    | $0, 0, 0, e^{12}a_1, (e^{23} - e^{14})a_1, e^{24} - (1 + a_1)e^{13}, e^{34} - e^{15}, e^{25} - e^{16}a_1, e^{17} + e^{28} + e^{46} + e^{35}$                                                    | 13579    |
| 96531:114a(*) | $0, 0, 0, a_1e^{12}, \frac{a_1}{a_1-1}e^{23} + \frac{2a_1-1}{a_1-1}e^{14}, e^{13} + \frac{2a_1-1}{a_1-1}e^{24}, e^{34} - e^{15}(-1 + a_1), e^{16} + e^{25}, e^{36} + e^{18} + e^{27} + e^{45}$  | 13579    |
| 96531:114b(*) | $0, 0, 0, a_1e^{12}, \frac{a_1}{a_1-1}e^{23} + \frac{2a_1-1}{a_1-1}e^{14}, -e^{13} + \frac{2a_1-1}{a_1-1}e^{24}, e^{34} - e^{15}(-1 + a_1), e^{16} + e^{25}, e^{45} + e^{36} + e^{18} + e^{27}$ | 13579    |
| 96531:115a    | $0, 0, 0, -(1 + a_5)e^{12}, e^{24} - e^{13}, e^{23}a_5 + e^{14}(2 + a_5), e^{26} + e^{15}(2 + a_5), e^{16} + e^{25} + e^{34}, e^{45} + e^{27} + e^{18}$                                         | 13579    |
| 96531:115b    | $0, 0, 0, (a_5 - 1)e^{12}, e^{24} - e^{13}, e^{23}a_5 - e^{14}(a_5 - 2), e^{26} - e^{15}(a_5 - 2), e^{34} + e^{25} - e^{16}, e^{27} + e^{45} + e^{18}$                                          | 13579    |
| 96531:116a    | $0, 0, 0, -(-1 + a_2)e^{12}, e^{14} + e^{23}, e^{13}a_2 + e^{24}, e^{16} + e^{25}, e^{15}a_2 + e^{26}, e^{28} + e^{17} + e^{36} + e^{45}$                                                       | 13579    |
| 96531:116b    | $0, 0, 0, -(-1 + a_2)e^{12}, -e^{14} + e^{23}, e^{13}a_2 + e^{24}, e^{25} - e^{16}, e^{15}a_2 + e^{26}, e^{36} + e^{17} + e^{28} + e^{45}$                                                      | 13579    |
| 96531:117a    | $0, 0, 0, e^{12}a_2, e^{14}, e^{24} + e^{13}a_2, e^{16} + e^{25}, -(-1 + a_2)e^{15} + e^{26} + e^{34}, e^{28} + e^{17} + e^{36} + e^{45}$                                                       | 13579    |
| 96531:117b    | $0, 0, 0, e^{12}a_2, -e^{14}, e^{24} + e^{13}a_2, e^{25} - e^{16}, -(-1 + a_2)e^{15} + e^{26} + e^{34}, e^{36} + e^{17} + e^{28} + e^{45}$                                                      | 13579    |
| 96531:118a(*) | $0, 0, 0, e^{12}a_3, e^{14}(1 + a_3), \frac{a_3+1}{1-a_3}e^{24} + e^{13}a_3, e^{25} - (-1 + a_3)e^{16}, e^{15} + e^{26} + e^{34}, e^{18} + e^{27} + e^{35} + e^{46}$                            | 13579    |
| 96531:118b(*) | $0, 0, 0, e^{12}a_3, e^{14}(1 + a_3), \frac{a_3+1}{1-a_3}e^{24} + e^{13}a_3, e^{25} - (-1 + a_3)e^{16}, -e^{15} + e^{26} + e^{34}, e^{46} + e^{18} + e^{27} + e^{35}$                           | 13579    |
| 96531:119a(*) | $0, 0, 0, e^{12}a_1, (-a_1a_6 + a_1 + a_6)e^{13} + e^{24}(1 + a_6), a_6e^{23} + e^{14}, e^{26} + \frac{1}{a_6+1}e^{15}, -(-1 + a_1)e^{16} + e^{25} + e^{34}, e^{28} + e^{17} + e^{35} + e^{46}$ | 13579    |

Table 2 – Continued to next page

Table 2 – Continued from previous page

| Name          | $\mathfrak{g}$                                                                                                                                                                                       | UCS Dim. |
|---------------|------------------------------------------------------------------------------------------------------------------------------------------------------------------------------------------------------|----------|
| 96531:119b(*) | $0, 0, 0, e^{12}a_1, (-a_1a_6 + a_1 + a_6)e^{13} + e^{24}(1 + a_6), a_6e^{23} - e^{14},$<br>$e^{26} - \frac{1}{a_6+1}e^{15}, -(-1 + a_1)e^{16} + e^{25} + e^{34}, e^{28} + e^{17} + e^{35} + e^{46}$ | 13579    |
|               | Type: 32112                                                                                                                                                                                          |          |
| 96432:1       | $0, 0, 0, -e^{12}, e^{13}, e^{14}, e^{16}, e^{17}, e^{46} + e^{27}$                                                                                                                                  | 35679    |
| 96432:2       | $0, 0, 0, e^{12}, e^{13}, e^{24}, e^{26}, e^{27}, e^{46} + e^{17}$                                                                                                                                   | 35679    |
| 96432:3a      | $0, 0, 0, -e^{12}, e^{13}, e^{14}, e^{16}, e^{17}, e^{27} + e^{46} + e^{35}$                                                                                                                         | 24679    |
| 96432:3b      | $0, 0, 0, -e^{12}, -e^{13}, e^{14}, e^{16}, e^{17}, e^{27} + e^{35} + e^{46}$                                                                                                                        | 24679    |
| 96432:4       | $0, 0, 0, e^{12}, e^{13}, e^{24}, e^{26}, e^{27}, e^{46} + e^{17} + e^{35}$                                                                                                                          | 24679    |
| 96432:5       | $0, 0, 0, -e^{12}, e^{13}, e^{14}, e^{16}, e^{35} + e^{17}, e^{46} + e^{27}$                                                                                                                         | 24679    |
| 96432:6a      | $0, 0, 0, e^{12}, e^{13}, e^{24}, e^{26}, e^{27} + e^{35}, e^{46} + e^{17}$                                                                                                                          | 24679    |
| 96432:6b      | $0, 0, 0, e^{12}, -e^{13}, e^{24}, e^{26}, e^{27} + e^{35}, e^{17} + e^{46}$                                                                                                                         | 24679    |
| 96432:7       | $0, 0, 0, e^{12}, e^{13}, e^{24}, e^{26}, e^{27}, e^{46} + e^{17} + e^{23}$                                                                                                                          | 35679    |
| 96432:8       | $0, 0, 0, -e^{12}, e^{13}, e^{14}, e^{16}, e^{23} + e^{17}, e^{46} + e^{27}$                                                                                                                         | 35679    |
| 96432:9       | $0, 0, 0, -e^{12}, e^{13}, e^{14}, e^{16}, e^{17}, e^{27} + e^{46} + e^{15}$                                                                                                                         | 24679    |
| 96432:10      | $0, 0, 0, e^{12}, e^{13}, e^{24}, e^{26}, e^{15} + e^{27}, e^{46} + e^{17}$                                                                                                                          | 24679    |
| 96432:11      | $0, 0, 0, -e^{12}, e^{13}, e^{14}, e^{16}, e^{17} + e^{24}, e^{46} + e^{27}$                                                                                                                         | 35679    |
| 96432:12      | $0, 0, 0, e^{12}, e^{13}, e^{24}, e^{26}, e^{27} + e^{14}, e^{46} + e^{17}$                                                                                                                          | 35679    |
| 96432:13a     | $0, 0, 0, -e^{12}, e^{13}, e^{14}, e^{16}, e^{23} + e^{17}, e^{46} + e^{27} + e^{35}$                                                                                                                | 24679    |
| 96432:13b     | $0, 0, 0, -e^{12}, -e^{13}, e^{14}, e^{16}, e^{17} + e^{23}, e^{27} + e^{35} + e^{46}$                                                                                                               | 24679    |
| 96432:14a     | $0, 0, 0, e^{12}, e^{13}, e^{24}, e^{26}, e^{27} + e^{35}, e^{46} + e^{17} + e^{23}$                                                                                                                 | 24679    |
| 96432:14b     | $0, 0, 0, e^{12}, -e^{13}, e^{24}, e^{26}, e^{35} + e^{27}, e^{46} + e^{23} + e^{17}$                                                                                                                | 24679    |
| 96432:15      | $0, 0, 0, e^{12}, e^{13}, e^{24}, e^{26}, e^{27} + e^{15}, e^{35} + e^{17} + e^{46}$                                                                                                                 | 24679    |
| 96432:16      | $0, 0, 0, -e^{12}, e^{13}, e^{14}, e^{16}, e^{17} + e^{35}, e^{15} + e^{27} + e^{46}$                                                                                                                | 24679    |
| 96432:17      | $0, 0, 0, -e^{12}, e^{13}, e^{14}, e^{23} + e^{16}, e^{17} + e^{34}, e^{27} + e^{46}$                                                                                                                | 34679    |
| 96432:18      | $0, 0, 0, -e^{12}, e^{13}, e^{14}, e^{23} + e^{16}, e^{25} + e^{17}, e^{46} + e^{27}$                                                                                                                | 24679    |
| 96432:19      | $0, 0, 0, -e^{12}, e^{13}, e^{14}, e^{16}, e^{17} + e^{23}, e^{27} + e^{15} + e^{46}$                                                                                                                | 24679    |
| 96432:20      | $0, 0, 0, e^{12}, e^{13}, e^{24}, e^{26}, e^{15} + e^{27}, e^{17} + e^{46} + e^{23}$                                                                                                                 | 24679    |
| 96432:21a     | $0, 0, 0, -e^{12}, e^{13}, e^{14}, e^{16}, e^{17} + e^{35} + e^{24}, e^{27} + e^{46}$                                                                                                                | 24679    |
| 96432:21b     | $0, 0, 0, -e^{12}, -e^{13}, e^{14}, e^{16}, e^{17} + e^{35} + e^{24}, e^{27} + e^{46}$                                                                                                               | 24679    |
| 96432:22      | $0, 0, 0, -e^{12}, -e^{13}, e^{14}, e^{16}, e^{17} + e^{25} + e^{34}, e^{46} + e^{27}$                                                                                                               | 24679    |
| 96432:23a     | $0, 0, 0, e^{12}, e^{13}, e^{24}, e^{26}, e^{27} + e^{35} + e^{14}, e^{46} + e^{17}$                                                                                                                 | 24679    |
| 96432:23b     | $0, 0, 0, e^{12}, -e^{13}, e^{24}, e^{26}, e^{35} + e^{14} + e^{27}, e^{17} + e^{46}$                                                                                                                | 24679    |
| 96432:24a     | $0, 0, 0, -e^{12}, e^{13}, e^{14}, e^{16}, e^{17} + e^{24}, e^{46} + e^{35} + e^{27}$                                                                                                                | 24679    |
| 96432:24b     | $0, 0, 0, -e^{12}, -e^{13}, e^{14}, e^{16}, e^{24} + e^{17}, e^{35} + e^{46} + e^{27}$                                                                                                               | 24679    |
| 96432:25a     | $0, 0, 0, e^{12}, e^{13}, e^{24}, e^{26}, e^{27} + e^{14}, e^{35} + e^{17} + e^{46}$                                                                                                                 | 24679    |
| 96432:25b     | $0, 0, 0, e^{12}, -e^{13}, e^{24}, e^{26}, e^{14} + e^{27}, e^{46} + e^{35} + e^{17}$                                                                                                                | 24679    |
| 96432:26a     | $0, 0, 0, -e^{12}, e^{13}, e^{14}, e^{23} + e^{16}, e^{17} + e^{25}, e^{46} + e^{35} + e^{27}$                                                                                                       | 24679    |
| 96432:26b     | $0, 0, 0, -e^{12}, e^{13}, -e^{14}, e^{23} + e^{16}, e^{25} + e^{17}, e^{46} + e^{27} + e^{35}$                                                                                                      | 24679    |
| 96432:27a     | $0, 0, 0, -e^{12}, e^{13}, e^{14}, e^{23} + e^{16}, e^{17} + e^{34}, e^{27} + e^{46} + e^{35}$                                                                                                       | 24679    |
| 96432:27b     | $0, 0, 0, -e^{12}, -e^{13}, e^{14}, e^{23} + e^{16}, e^{17} + e^{34}, e^{27} + e^{46} + e^{35}$                                                                                                      | 24679    |
| 96432:28      | $0, 0, 0, e^{12}, e^{13}, e^{24}, e^{26}, e^{14} + e^{27}, e^{17} + e^{23} + e^{46}$                                                                                                                 | 35679    |
| 96432:29      | $0, 0, 0, -e^{12}, e^{13}, e^{14}, e^{16}, e^{24} + e^{17}, e^{46} + e^{15} + e^{27}$                                                                                                                | 24679    |
| 96432:30a     | $0, 0, 0, -e^{12}, -e^{13}, e^{14}, e^{16}, e^{17} + e^{25} + e^{34}, e^{27} + e^{35} + e^{46}$                                                                                                      | 24679    |
| 96432:30b     | $0, 0, 0, -e^{12}, -e^{13}, -e^{14}, e^{16}, e^{17} + e^{25} + e^{34}, e^{35} + e^{46} + e^{27}$                                                                                                     | 24679    |
| 96432:31a     | $0, 0, 0, -e^{12}, e^{13}, e^{14}, e^{23} + e^{16}, e^{17} + e^{25}, e^{27} + e^{46} + e^{15}$                                                                                                       | 24679    |
| 96432:31b     | $0, 0, 0, -e^{12}, -e^{13}, e^{14}, e^{23} + e^{16}, -e^{17} + e^{25}, e^{46} + e^{15} + e^{27}$                                                                                                     | 24679    |
| 96432:32      | $0, 0, 0, -e^{12}, e^{13}, e^{14}, e^{16} + e^{24}, e^{26} + e^{17}, e^{46} + e^{27}$                                                                                                                | 35679    |
| 96432:33      | $0, 0, 0, e^{12}, e^{13}, e^{24}, e^{14} + e^{26}, e^{16} + e^{27}, e^{46} + e^{17}$                                                                                                                 | 35679    |
| 96432:34      | $0, 0, 0, (-1 + a_2)e^{12}, e^{13}a_2, e^{14}, -(-1 + a_2)e^{16} + e^{23}, e^{17} + e^{34} + e^{25}, e^{27} + e^{46}$                                                                                | 24679    |
| 96432:35a     | $0, 0, 0, -e^{12}, e^{13}, e^{14}, e^{23} + e^{16}, e^{17} + e^{34}, e^{15} + e^{46} + e^{27}$                                                                                                       | 24679    |
| 96432:35b     | $0, 0, 0, -e^{12}, -e^{13}, e^{14}, e^{23} + e^{16}, e^{34} + e^{17}, e^{46} + e^{27} + e^{15}$                                                                                                      | 24679    |
| 96432:36a     | $0, 0, 0, e^{12}, e^{13}, e^{24}, e^{26}, e^{27} + e^{35} + e^{14}, e^{17} + e^{23} + e^{46}$                                                                                                        | 24679    |
| 96432:36b     | $0, 0, 0, e^{12}, -e^{13}, e^{24}, e^{26}, e^{14} + e^{27} + e^{35}, e^{46} + e^{23} + e^{17}$                                                                                                       | 24679    |
| 96432:37a     | $0, 0, 0, -e^{12}, e^{13}, e^{14}, e^{16}, e^{17} + e^{24} + e^{35}, e^{27} + e^{15} + e^{46}$                                                                                                       | 24679    |
| 96432:37b     | $0, 0, 0, -e^{12}, -e^{13}, e^{14}, e^{16}, e^{35} + e^{24} + e^{17}, e^{46} + e^{15} + e^{27}$                                                                                                      | 24679    |
| 96432:38a     | $0, 0, 0, -e^{12}, -e^{13}, e^{14}, e^{16}, e^{17} + e^{25} + e^{34}, e^{15} + e^{27} + e^{46}$                                                                                                      | 24679    |
| 96432:38b     | $0, 0, 0, -e^{12}, -e^{13}, e^{14}, e^{16}, -e^{17} + e^{25} + e^{34}, e^{46} + e^{15} + e^{27}$                                                                                                     | 24679    |

Table 2 – Continued to next page

Table 2 – Continued from previous page

| Name        | $\mathfrak{g}$                                                                                                              | UCS Dim. |
|-------------|-----------------------------------------------------------------------------------------------------------------------------|----------|
| 96432:39a   | $0, 0, 0, -e^{12}a_3, -(-1 + a_3)e^{13}, e^{14}, e^{23} + e^{16}a_3, e^{17} + e^{34} + e^{25}, e^{27} + e^{46} + e^{35}$    | 24679    |
| 96432:39b   | $0, 0, 0, -e^{12}a_3, -(-1 + a_3)e^{13}, -e^{14}, e^{23} + e^{16}a_3, e^{25} + e^{17} + e^{34}, e^{46} + e^{27} + e^{35}$   | 24679    |
| 96432:40    | $0, 0, 0, -e^{12}, e^{13}, e^{14}, e^{16} + e^{24}, e^{27} + e^{46}, e^{17} + e^{35} + e^{26}$                              | 24679    |
| 96432:41a   | $0, 0, 0, e^{12}, e^{13}, e^{24}, e^{14} + e^{26}, e^{46} + e^{17}, e^{16} + e^{27} + e^{35}$                               | 24679    |
| 96432:41b   | $0, 0, 0, e^{12}, -e^{13}, e^{24}, e^{26} + e^{14}, e^{46} + e^{17}, e^{27} + e^{35} + e^{16}$                              | 24679    |
| 96432:42a   | $0, 0, 0, -e^{12}, e^{13}, e^{14}, e^{16} + e^{24}, e^{17} + e^{26}, e^{27} + e^{46} + e^{35}$                              | 24679    |
| 96432:42b   | $0, 0, 0, -e^{12}, -e^{13}, e^{14}, e^{16} + e^{24}, e^{17} + e^{26}, e^{27} + e^{46} + e^{35}$                             | 24679    |
| 96432:43    | $0, 0, 0, e^{12}, e^{13}, e^{24}, e^{14} + e^{26}, e^{16} + e^{27}, e^{17} + e^{35} + e^{46}$                               | 24679    |
| 96432:44    | $0, 0, 0, e^{12}, e^{13}, e^{24}, e^{26} + e^{14}, e^{27} + e^{16}, e^{46} + e^{17} + e^{23}$                               | 35679    |
| 96432:45a   | $0, 0, 0, e^{12}, e^{13}a_1, e^{14}, -e^{16} + e^{23}, (-1 + a_1)e^{17} + e^{34} + e^{25}, e^{15} + e^{46} + e^{27}$        | 24679    |
| 96432:45b   | $0, 0, 0, -e^{12}, e^{13}a_1, e^{14}, e^{16} + e^{23}, e^{17}(1 + a_1) + e^{25} + e^{34}, e^{46} + e^{15} + e^{27}$         | 24679    |
| 96432:46    | $0, 0, 0, -e^{12}, e^{13}, e^{14}, e^{16} + e^{24}, e^{17} + e^{26}, e^{27} + e^{15} + e^{46}$                              | 24679    |
| 96432:48a   | $0, 0, 0, e^{12}, e^{13}, e^{24}, e^{26} + e^{14}, e^{46} + e^{17} + e^{23}, e^{27} + e^{35} + e^{16}$                      | 24679    |
| 96432:48b   | $0, 0, 0, e^{12}, -e^{13}, e^{24}, e^{14} + e^{26}, e^{46} + e^{17} + e^{23}, e^{16} + e^{27} + e^{35}$                     | 24679    |
| 96432:49    | $0, 0, 0, -e^{12}, e^{13}, e^{14}, e^{16} + e^{24}, e^{17} + e^{35} + e^{26}, e^{27} + e^{46} + e^{15}$                     | 24679    |
| 96432:58    | $0, 0, 0, e^{12}, 2e^{13}, 3e^{14} - e^{23}, -e^{16} + e^{25} + e^{34}, e^{27} + e^{46}, e^{17} + e^{36} + e^{45}$          | 23579    |
| 96432:59a   | $0, 0, 0, e^{12}, 2e^{13}, e^{14} - e^{23}, e^{25} + e^{34} - e^{16}, e^{45} + 3e^{36} + e^{17}, e^{46} + e^{27} + e^{35}$  | 23579    |
| 96432:59b   | $0, 0, 0, e^{12}, 2e^{13}, -e^{14} - e^{23}, e^{25} + e^{34} - e^{16}, e^{45} - 3e^{36} + e^{17}, e^{46} + e^{27} + e^{35}$ | 23579    |
| 96432:60    | $0, 0, 0, e^{12}, 2e^{13}, 3e^{14} - e^{23}, -e^{16} + e^{25} + e^{34}, e^{15} + e^{27} + e^{46}, e^{17} + e^{36} + e^{45}$ | 23579    |
| Type: 32211 |                                                                                                                             |          |
| 96421:1     | $0, 0, 0, e^{12}, e^{13}, e^{14}, e^{35}, e^{16}, e^{18}$                                                                   | 24679    |
| 96421:2     | $0, 0, 0, e^{12}, e^{13}, e^{24}, e^{35}, e^{26}, e^{28}$                                                                   | 24679    |
| 96421:3     | $0, 0, 0, e^{12}, e^{13}, e^{14}, e^{15}, e^{16}, e^{18}$                                                                   | 24679    |
| 96421:4     | $0, 0, 0, e^{12}, e^{13}, e^{24}, e^{15}, e^{26}, e^{28}$                                                                   | 24679    |
| 96421:5     | $0, 0, 0, e^{12}, e^{13}, e^{14}, e^{24}, e^{16}, e^{18}$                                                                   | 35679    |
| 96421:6     | $0, 0, 0, e^{12}, e^{13}, e^{24}, e^{14}, e^{26}, e^{28}$                                                                   | 35679    |
| 96421:7     | $0, 0, 0, e^{12}, e^{13}, e^{14}, e^{23} + e^{15}, e^{16}, e^{18}$                                                          | 24679    |
| 96421:8     | $0, 0, 0, e^{12}, e^{13}, e^{24}, e^{15} + e^{23}, e^{26}, e^{28}$                                                          | 24679    |
| 96421:9     | $0, 0, 0, e^{12}, e^{13}, e^{14}, e^{35}, e^{16}, e^{18} + e^{23}$                                                          | 24679    |
| 96421:10a   | $0, 0, 0, e^{12}, e^{13}, e^{14}, e^{35} + e^{24}, e^{16}, e^{18}$                                                          | 24679    |
| 96421:10b   | $0, 0, 0, -e^{12}, e^{13}, e^{14}, e^{35} + e^{24}, e^{16}, e^{18}$                                                         | 24679    |
| 96421:11    | $0, 0, 0, e^{12}, e^{13}, e^{14}, e^{25} + e^{34}, e^{16}, e^{18}$                                                          | 24679    |
| 96421:12    | $0, 0, 0, e^{12}, e^{13}, e^{24}, e^{35} + e^{14}, e^{26}, e^{28}$                                                          | 24679    |
| 96421:13    | $0, 0, 0, e^{12}, e^{13}, e^{24}, e^{34} + e^{25}, e^{26}, e^{28}$                                                          | 24679    |
| 96421:14    | $0, 0, 0, e^{12}, e^{13}, e^{14}, e^{15}, e^{16}, e^{18} + e^{35}$                                                          | 24679    |
| 96421:15a   | $0, 0, 0, e^{12}, e^{13}, e^{24}, e^{15}, e^{26}, e^{28} + e^{35}$                                                          | 24679    |
| 96421:15b   | $0, 0, 0, -e^{12}, e^{13}, e^{24}, e^{15}, e^{26}, e^{35} + e^{28}$                                                         | 24679    |
| 96421:16    | $0, 0, 0, e^{12}, e^{13}, e^{24}, e^{35}, e^{26}, e^{15} + e^{28}$                                                          | 24679    |
| 96421:17    | $0, 0, 0, e^{12}, e^{13}, e^{24}, e^{14} + e^{23}, e^{26}, e^{28}$                                                          | 35679    |
| 96421:18    | $0, 0, 0, e^{12}, e^{13}, e^{14}, e^{15}, e^{16}, e^{23} + e^{18}$                                                          | 24679    |
| 96421:19    | $0, 0, 0, e^{12}, e^{13}, e^{14}, e^{24} + e^{15}, e^{16}, e^{18}$                                                          | 24679    |
| 96421:20    | $0, 0, 0, e^{12}, e^{13}, e^{14}, e^{15} + e^{23}, e^{16}, e^{18} + e^{35}$                                                 | 24679    |
| 96421:21a   | $0, 0, 0, e^{12}, e^{13}, e^{24}, e^{15} + e^{23}, e^{26}, e^{28} + e^{35}$                                                 | 24679    |
| 96421:21b   | $0, 0, 0, -e^{12}, e^{13}, e^{24}, e^{15} + e^{23}, e^{26}, e^{28} + e^{35}$                                                | 24679    |
| 96421:22    | $0, 0, 0, e^{12}, e^{13}, e^{14}, e^{24}, e^{16}, e^{35} + e^{18}$                                                          | 24679    |
| 96421:23a   | $0, 0, 0, e^{12}, e^{13}, e^{24}, e^{14}, e^{26}, e^{35} + e^{28}$                                                          | 24679    |
| 96421:23b   | $0, 0, 0, -e^{12}, e^{13}, e^{24}, e^{14}, e^{26}, e^{35} + e^{28}$                                                         | 24679    |
| 96421:24    | $0, 0, 0, e^{12}, e^{13}, e^{14}, e^{35}, e^{16}, e^{18} + e^{24}$                                                          | 24679    |
| 96421:25    | $0, 0, 0, e^{12}, e^{13}, e^{24}, e^{35}, e^{26}, e^{14} + e^{28}$                                                          | 24679    |
| 96421:26    | $0, 0, 0, e^{12}, e^{13}, e^{14}, e^{25} + e^{34}, e^{16}, e^{18} + e^{35}$                                                 | 24679    |
| 96421:27a   | $0, 0, 0, e^{12}, e^{13}, e^{24}, e^{34} + e^{25}, e^{26}, e^{35} + e^{28}$                                                 | 24679    |
| 96421:27b   | $0, 0, 0, e^{12}, e^{13}, -e^{24}, e^{25} + e^{34}, e^{26}, e^{35} + e^{28}$                                                | 24679    |
| 96421:28    | $0, 0, 0, e^{12}, e^{13}, e^{14}, e^{35}, e^{23} + e^{16}, e^{25} + e^{18}$                                                 | 24679    |
| 96421:29    | $0, 0, 0, -e^{12}, e^{13}, e^{14}, e^{35}, e^{16} + e^{23}, e^{18} + e^{34}$                                                | 24679    |
| 96421:30    | $0, 0, 0, -e^{12}, e^{13}, e^{14}, e^{35}, e^{16}, e^{46} + e^{28}$                                                         | 24679    |
| 96421:31    | $0, 0, 0, e^{12}, e^{13}, e^{24}, e^{35}, e^{26}, e^{46} + e^{18}$                                                          | 24679    |
| 96421:32    | $0, 0, 0, e^{12}, e^{13}, e^{14}, e^{24}, e^{16}, e^{18} + e^{23}$                                                          | 35679    |
| 96421:33a   | $0, 0, 0, e^{12}, e^{13}, e^{14}, e^{35} + e^{24}, e^{16}, e^{18} + e^{23}$                                                 | 24679    |

Table 2 – Continued to next page

Table 2 – Continued from previous page

| Name      | $\mathfrak{g}$                                                                                    | UCS Dim. |
|-----------|---------------------------------------------------------------------------------------------------|----------|
| 96421:33b | $0, 0, 0, -e^{12}, e^{13}, e^{14}, e^{35} + e^{24}, e^{16}, e^{18} + e^{23}$                      | 24679    |
| 96421:34  | $0, 0, 0, e^{12}, e^{13}, e^{14}, e^{25} + e^{34}, e^{16}, e^{18} + e^{23}$                       | 24679    |
| 96421:35  | $0, 0, 0, e^{12}, e^{13}, e^{24}, e^{14}, e^{26}, e^{15} + e^{28}$                                | 24679    |
| 96421:36  | $0, 0, 0, e^{12}, e^{13}, e^{14}, e^{15}, e^{16}, e^{24} + e^{18}$                                | 24679    |
| 96421:37  | $0, 0, 0, e^{12}, e^{13}, e^{24}, e^{15}, e^{26}, e^{28} + e^{14}$                                | 24679    |
| 96421:38a | $0, 0, 0, e^{12}, e^{13}, e^{24}, e^{14} + e^{23}, e^{26}, e^{35} + e^{28}$                       | 24679    |
| 96421:38b | $0, 0, 0, -e^{12}, e^{13}, e^{24}, e^{23} + e^{14}, e^{26}, e^{28} + e^{35}$                      | 24679    |
| 96421:39  | $0, 0, 0, e^{12}, e^{13}, e^{14}, e^{15} + e^{24}, e^{16}, e^{18} + e^{35}$                       | 24679    |
| 96421:40  | $0, 0, 0, e^{12}, e^{13}, e^{24}, e^{14} + e^{35}, e^{26}, e^{28} + e^{15}$                       | 24679    |
| 96421:41  | $0, 0, 0, e^{12}, e^{13}, e^{24}, e^{25} + e^{34}, e^{26}, e^{28} + e^{15}$                       | 24679    |
| 96421:42  | $0, 0, 0, e^{12}, e^{13}, e^{14}, e^{15}, e^{23} + e^{16}, e^{25} + e^{18}$                       | 24679    |
| 96421:43  | $0, 0, 0, e^{12}, e^{13}, e^{14}, e^{35}, e^{16}, e^{18} + e^{34} + e^{25}$                       | 24679    |
| 96421:44  | $0, 0, 0, -e^{12}, e^{13}, e^{14}, e^{15}, e^{16} + e^{23}, e^{18} + e^{34}$                      | 24679    |
| 96421:45  | $0, 0, 0, -e^{12}, e^{13}, e^{14}, e^{15}, e^{16}, e^{46} + e^{28}$                               | 24679    |
| 96421:46  | $0, 0, 0, e^{12}, e^{13}, e^{24}, e^{15}, e^{26}, e^{46} + e^{18}$                                | 24679    |
| 96421:47  | $0, 0, 0, -e^{12}, e^{13}, e^{14}, e^{35}, e^{16} + e^{23}, e^{28} + e^{46}$                      | 24679    |
| 96421:48  | $0, 0, 0, e^{12}, e^{13}, e^{14}, e^{24}, e^{16}, e^{27} + e^{18}$                                | 25679    |
| 96421:49  | $0, 0, 0, e^{12}, e^{13}, e^{24}, e^{14}, e^{26}, e^{28} + e^{17}$                                | 25679    |
| 96421:50  | $0, 0, 0, e^{12}, e^{13}, e^{14}, e^{15} + e^{24}, e^{16}, e^{18} + e^{23}$                       | 24679    |
| 96421:51  | $0, 0, 0, e^{12}, e^{13}, e^{24}, e^{14} + e^{23}, e^{26}, e^{15} + e^{28}$                       | 24679    |
| 96421:52  | $0, 0, 0, e^{12}, e^{13}, e^{14}, e^{23} + e^{15}, e^{16}, e^{24} + e^{18}$                       | 24679    |
| 96421:53  | $0, 0, 0, e^{12}, e^{13}, e^{24}, e^{15} + e^{23}, e^{26}, e^{14} + e^{28}$                       | 24679    |
| 96421:54  | $0, 0, 0, -e^{12}, e^{13}, e^{14}, e^{24}, e^{16}, e^{28} + e^{46}$                               | 35679    |
| 96421:55  | $0, 0, 0, e^{12}, e^{13}, e^{24}, e^{14}, e^{26}, e^{18} + e^{46}$                                | 35679    |
| 96421:56a | $0, 0, 0, e^{12}, e^{13}, e^{14}, e^{15}, e^{16}, e^{35} + e^{18} + e^{24}$                       | 24679    |
| 96421:56b | $0, 0, 0, -e^{12}, e^{13}, e^{14}, e^{15}, e^{16}, e^{18} + e^{35} + e^{24}$                      | 24679    |
| 96421:57  | $0, 0, 0, e^{12}, e^{13}, e^{14}, e^{15}, e^{16}, e^{25} + e^{18} + e^{34}$                       | 24679    |
| 96421:58a | $0, 0, 0, e^{12}, e^{13}, e^{24}, e^{15}, e^{26}, e^{14} + e^{35} + e^{28}$                       | 24679    |
| 96421:58b | $0, 0, 0, -e^{12}, e^{13}, e^{24}, e^{15}, e^{26}, e^{28} + e^{35} + e^{14}$                      | 24679    |
| 96421:59  | $0, 0, 0, e^{12}, e^{13}, e^{14}, e^{25} + e^{34}, e^{16}, e^{18} + e^{24}$                       | 24679    |
| 96421:60  | $0, 0, 0, e^{12}, e^{13}, e^{24}, e^{25} + e^{34}, e^{26}, e^{28} + e^{14}$                       | 24679    |
| 96421:61  | $0, 0, 0, -e^{12}, e^{13}, e^{14}, e^{24}, e^{16} + e^{23}, e^{34} + e^{18}$                      | 34679    |
| 96421:62  | $0, 0, 0, e^{12}, e^{13}, e^{14}, e^{24}, e^{23} + e^{16}, e^{18} + e^{25}$                       | 24679    |
| 96421:63  | $0, 0, 0, -e^{12}, e^{13}, e^{14}, e^{15} + e^{23}, e^{16}, e^{28} + e^{46}$                      | 24679    |
| 96421:64  | $0, 0, 0, e^{12}, e^{13}, e^{24}, e^{15} + e^{23}, e^{26}, e^{46} + e^{18}$                       | 24679    |
| 96421:65  | $0, 0, 0, e^{12}, e^{13}, e^{24}, e^{35}, e^{26}, e^{23} + e^{46} + e^{18}$                       | 24679    |
| 96421:66a | $0, 0, 0, e^{12}, e^{13}, e^{14}, e^{24} + e^{35}, e^{23} + e^{16}, e^{25} + e^{18}$              | 24679    |
| 96421:66b | $0, 0, 0, -e^{12}, e^{13}, e^{14}, e^{35} + e^{24}, e^{16} + e^{23}, e^{25} + e^{18}$             | 24679    |
| 96421:67  | $0, 0, 0, e^{12}(-1 + a_2), e^{13}a_2, e^{14}, e^{35}, e^{23} + e^{16}, e^{34} + e^{18} + e^{25}$ | 24679    |
| 96421:68a | $0, 0, 0, -e^{12}, e^{13}, e^{14}, e^{35} + e^{24}, e^{23} + e^{16}, e^{18} + e^{34}$             | 24679    |
| 96421:68b | $0, 0, 0, -e^{12}, -e^{13}, e^{14}, e^{24} + e^{35}, e^{16} + e^{23}, e^{18} + e^{34}$            | 24679    |
| 96421:69a | $0, 0, 0, -e^{12}, e^{13}, e^{14}, e^{35} + e^{24}, e^{16}, e^{46} + e^{28}$                      | 24679    |
| 96421:69b | $0, 0, 0, -e^{12}, -e^{13}, e^{14}, e^{24} + e^{35}, e^{16}, e^{28} + e^{46}$                     | 24679    |
| 96421:70  | $0, 0, 0, -e^{12}, -e^{13}, e^{14}, e^{25} + e^{34}, e^{16}, e^{28} + e^{46}$                     | 24679    |
| 96421:71  | $0, 0, 0, e^{12}, e^{13}, e^{24}, e^{14} + e^{35}, e^{26}, e^{18} + e^{46}$                       | 24679    |
| 96421:72  | $0, 0, 0, e^{12}, e^{13}, e^{24}, e^{25} + e^{34}, e^{26}, e^{46} + e^{18}$                       | 24679    |
| 96421:73a | $0, 0, 0, -e^{12}, e^{13}, e^{14}, e^{15}, e^{16}, e^{28} + e^{35} + e^{46}$                      | 24679    |
| 96421:73b | $0, 0, 0, -e^{12}, -e^{13}, e^{14}, e^{15}, e^{16}, e^{46} + e^{35} + e^{28}$                     | 24679    |
| 96421:74  | $0, 0, 0, e^{12}, e^{13}, e^{24}, e^{15}, e^{26}, e^{35} + e^{46} + e^{18}$                       | 24679    |
| 96421:75  | $0, 0, 0, -e^{12}, e^{13}, e^{14}, e^{35}, e^{16}, e^{28} + e^{46} + e^{15}$                      | 24679    |
| 96421:76  | $0, 0, 0, -e^{12}, e^{13}, e^{14}, e^{15}, e^{16} + e^{23}, e^{28} + e^{46}$                      | 24679    |
| 96421:77  | $0, 0, 0, e^{12}, e^{13}, e^{14}, e^{35}, e^{16} + e^{24}, e^{18} + e^{26}$                       | 24679    |
| 96421:78  | $0, 0, 0, e^{12}, e^{13}, e^{24}, e^{35}, e^{14} + e^{26}, e^{16} + e^{28}$                       | 24679    |
| 96421:79  | $0, 0, 0, -e^{12}, e^{13}, e^{14}, e^{35}, e^{16} + e^{24}, e^{28} + e^{46}$                      | 24679    |
| 96421:80  | $0, 0, 0, e^{12}, e^{13}, e^{24}, e^{35}, e^{26} + e^{14}, e^{18} + e^{46}$                       | 24679    |
| 96421:81  | $0, 0, 0, e^{12}, e^{13}, e^{24}, e^{14} + e^{23}, e^{26}, e^{18} + e^{46}$                       | 35679    |
| 96421:82a | $0, 0, 0, e^{12}, e^{13}, e^{14}, e^{23} + e^{15}, e^{16}, e^{35} + e^{24} + e^{18}$              | 24679    |
| 96421:82b | $0, 0, 0, -e^{12}, e^{13}, e^{14}, e^{15} + e^{23}, e^{16}, e^{18} + e^{24} + e^{35}$             | 24679    |

Table 2 – Continued to next page

Table 2 – Continued from previous page

| Name       | $\mathfrak{g}$                                                                                               | UCS Dim. |
|------------|--------------------------------------------------------------------------------------------------------------|----------|
| 96421:83   | $0, 0, 0, e^{12}, e^{13}, e^{14}, e^{15} + e^{23}, e^{16}, e^{25} + e^{18} + e^{34}$                         | 24679    |
| 96421:84a  | $0, 0, 0, e^{12}, e^{13}, e^{24}, e^{15} + e^{23}, e^{26}, e^{28} + e^{35} + e^{14}$                         | 24679    |
| 96421:84b  | $0, 0, 0, -e^{12}, e^{13}, e^{24}, e^{15} + e^{23}, e^{26}, e^{28} + e^{14} + e^{35}$                        | 24679    |
| 96421:85   | $0, 0, 0, e^{12}, e^{13}, e^{14}, e^{24}, e^{16}, e^{18} + e^{25} + e^{34}$                                  | 24679    |
| 96421:86   | $0, 0, 0, e^{12}, e^{13}, e^{24}, e^{15}, e^{26}, e^{23} + e^{46} + e^{18}$                                  | 24679    |
| 96421:87a  | $0, 0, 0, e^{12}, e^{13}, e^{14}, e^{15} + e^{24}, e^{23} + e^{16}, e^{18} + e^{25}$                         | 24679    |
| 96421:87b  | $0, 0, 0, e^{12}, e^{13}, -e^{14}, e^{15} + e^{24}, e^{16} + e^{23}, e^{25} + e^{18}$                        | 24679    |
| 96421:88   | $0, 0, 0, e^{12}, e^{13}, e^{14}, e^{24}, e^{16}, e^{35} + e^{18} + e^{27}$                                  | 14679    |
| 96421:89a  | $0, 0, 0, e^{12}, e^{13}, e^{24}, e^{14}, e^{26}, e^{35} + e^{28} + e^{17}$                                  | 14679    |
| 96421:89b  | $0, 0, 0, -e^{12}, e^{13}, e^{24}, e^{14}, e^{26}, e^{35} + e^{28} + e^{17}$                                 | 14679    |
| 96421:90a  | $0, 0, 0, e^{12}, e^{13}, e^{14}, e^{24} + e^{35}, e^{16}, e^{18} + e^{25} + e^{34}$                         | 24679    |
| 96421:90b  | $0, 0, 0, e^{12}, e^{13}, e^{14}, e^{35} - e^{24}, e^{16}, e^{18} + e^{34} + e^{25}$                         | 24679    |
| 96421:91a  | $0, 0, 0, e^{12}, e^{13}, e^{14}, e^{25} + e^{34}, e^{16}, e^{24} + e^{18} + e^{35}$                         | 24679    |
| 96421:91b  | $0, 0, 0, -e^{12}, e^{13}, e^{14}, -e^{25} + e^{34}, e^{16}, e^{35} + e^{24} + e^{18}$                       | 24679    |
| 96421:92a  | $0, 0, 0, e^{12}, e^{13}, e^{24}, e^{25} + e^{34}, e^{26}, e^{35} + e^{14} + e^{28}$                         | 24679    |
| 96421:92b  | $0, 0, 0, e^{12}, e^{13}, -e^{24}, e^{34} + e^{25}, e^{26}, e^{14} + e^{28} + e^{35}$                        | 24679    |
| 96421:93   | $0, 0, 0, e^{12}(-1 + a_2), a_2 e^{13}, e^{14}, e^{15}, e^{16} + e^{23}, e^{25} + e^{18} + e^{34}$           | 24679    |
| 96421:94a  | $0, 0, 0, -e^{12}, e^{13}, e^{14}, e^{15} + e^{24}, e^{23} + e^{16}, e^{18} + e^{34}$                        | 24679    |
| 96421:94b  | $0, 0, 0, -e^{12}, -e^{13}, e^{14}, e^{15} + e^{24}, e^{16} + e^{23}, e^{18} + e^{34}$                       | 24679    |
| 96421:95   | $0, 0, 0, -e^{12}, e^{13}, e^{14}, e^{15} + e^{24}, e^{16}, e^{28} + e^{46}$                                 | 24679    |
| 96421:96a  | $0, 0, 0, -e^{12}, e^{13}, e^{14}, e^{23} + e^{15}, e^{16}, e^{35} + e^{46} + e^{28}$                        | 24679    |
| 96421:96b  | $0, 0, 0, -e^{12}, -e^{13}, e^{14}, e^{15} + e^{23}, e^{16}, e^{28} + e^{46} + e^{35}$                       | 24679    |
| 96421:97   | $0, 0, 0, e^{12}, e^{13}, e^{24}, e^{15} + e^{23}, e^{26}, e^{46} + e^{18} + e^{35}$                         | 24679    |
| 96421:98   | $0, 0, 0, -e^{12}, e^{13}, e^{14}, e^{24}, e^{23} + e^{16}, e^{28} + e^{46}$                                 | 34679    |
| 96421:99a  | $0, 0, 0, -e^{12}, e^{13}, e^{14}, e^{24}, e^{16}, e^{35} + e^{46} + e^{28}$                                 | 24679    |
| 96421:99b  | $0, 0, 0, -e^{12}, -e^{13}, e^{14}, e^{24}, e^{16}, e^{46} + e^{35} + e^{28}$                                | 24679    |
| 96421:100  | $0, 0, 0, e^{12}, e^{13}, e^{24}, e^{14}, e^{26}, e^{18} + e^{46} + e^{35}$                                  | 24679    |
| 96421:101  | $0, 0, 0, e^{12}, e^{13}, e^{14}, e^{15}, e^{16} + e^{24}, e^{18} + e^{26}$                                  | 24679    |
| 96421:102  | $0, 0, 0, e^{12}, e^{13}, e^{24}, e^{15}, e^{14} + e^{26}, e^{16} + e^{28}$                                  | 24679    |
| 96421:103a | $0, 0, 0, -e^{12}, -e^{13}, e^{14}, e^{25} + e^{34}, e^{16}, e^{28} + e^{35} + e^{46}$                       | 24679    |
| 96421:103b | $0, 0, 0, -e^{12}, -e^{13}, -e^{14}, e^{25} + e^{34}, e^{16}, e^{35} + e^{46} + e^{28}$                      | 24679    |
| 96421:104  | $0, 0, 0, e^{12}, e^{13}, e^{24}, e^{25} + e^{34}, e^{26}, e^{18} + e^{46} + e^{35}$                         | 24679    |
| 96421:105a | $0, 0, 0, -e^{12}, e^{13}, e^{14}, e^{24} + e^{35}, e^{23} + e^{16}, e^{28} + e^{46}$                        | 24679    |
| 96421:105b | $0, 0, 0, -e^{12}, -e^{13}, e^{14}, e^{35} + e^{24}, e^{23} + e^{16}, e^{46} + e^{28}$                       | 24679    |
| 96421:106  | $0, 0, 0, -e^{12}, -e^{13}, e^{14}, e^{25} + e^{34}, e^{16} + e^{23}, e^{28} + e^{46}$                       | 24679    |
| 96421:107a | $0, 0, 0, -e^{12}, e^{13}, e^{14}, e^{15}, e^{23} + e^{16}, e^{46} + e^{35} + e^{28}$                        | 24679    |
| 96421:107b | $0, 0, 0, -e^{12}, -e^{13}, e^{14}, e^{15}, e^{23} + e^{16}, e^{35} + e^{46} + e^{28}$                       | 24679    |
| 96421:108a | $0, 0, 0, -e^{12}, e^{13}, e^{14}, e^{35}, e^{23} + e^{16}, e^{15} + e^{46} + e^{28}$                        | 24679    |
| 96421:108b | $0, 0, 0, -e^{12}, -e^{13}, e^{14}, e^{35}, e^{16} + e^{23}, e^{15} + e^{28} + e^{46}$                       | 24679    |
| 96421:109  | $0, 0, 0, -e^{12}, e^{13}, e^{14}, e^{15}, e^{16} + e^{24}, e^{46} + e^{28}$                                 | 24679    |
| 96421:110  | $0, 0, 0, e^{12}, e^{13}, e^{24}, e^{15}, e^{14} + e^{26}, e^{18} + e^{46}$                                  | 24679    |
| 96421:111  | $0, 0, 0, e^{12}, e^{13}, e^{14}, e^{35}, e^{16}, e^{37} + e^{18}$                                           | 13579    |
| 96421:112  | $0, 0, 0, e^{12}, e^{13}, e^{24}, e^{35}, e^{26}, e^{28} + e^{37}$                                           | 13579    |
| 96421:113  | $0, 0, 0, e^{12}, e^{13}, e^{24}, e^{14}, e^{26}, e^{46} + e^{18} + e^{23}$                                  | 35679    |
| 96421:114a | $0, 0, 0, e^{12}, e^{13}, e^{14}, e^{15} + e^{24}, e^{16}, e^{25} + e^{18} + e^{34}$                         | 24679    |
| 96421:114b | $0, 0, 0, e^{12}, e^{13}, -e^{14}, e^{15} + e^{24}, e^{16}, e^{18} + e^{34} + e^{25}$                        | 24679    |
| 96421:115  | $0, 0, 0, e^{12}, e^{13}, e^{24}, e^{35} + e^{14}, e^{26}, e^{18} + e^{46} + e^{23}$                         | 24679    |
| 96421:116  | $0, 0, 0, e^{12}, e^{13}, e^{24}, e^{34} + e^{25}, e^{26}, e^{18} + e^{46} + e^{23}$                         | 24679    |
| 96421:117  | $0, 0, 0, e^{12}(-1 + a_2), a_2 e^{13}, e^{14}, e^{24}, e^{16} + e^{23}, e^{18} + e^{34} + e^{25}$           | 24679    |
| 96421:118  | $0, 0, 0, -e^{12}, e^{13}, e^{14}, e^{24}, e^{16}, e^{15} + e^{28} + e^{46}$                                 | 24679    |
| 96421:119  | $0, 0, 0, e^{12}, e^{13}, e^{24}, e^{14} + e^{23}, e^{26}, e^{18} + e^{35} + e^{46}$                         | 24679    |
| 96421:120  | $0, 0, 0, e^{12}, a_1 e^{13}, e^{14}, e^{23} + e^{15}, e^{24} + e^{16}, e^{26} + e^{18}$                     | 24679    |
| 96421:121  | $0, 0, 0, e^{12}, e^{13}, e^{24}, e^{23} + e^{15}, e^{26} + e^{14}, e^{16} + e^{28}$                         | 24679    |
| 96421:122a | $0, 0, 0, e^{12}(-1 + a_2), a_2 e^{13}, e^{14}, e^{24} + e^{35}, e^{16} + e^{23}, e^{25} + e^{18} + e^{34}$  | 24679    |
| 96421:122b | $0, 0, 0, e^{12}(-1 + a_2), a_2 e^{13}, e^{14}, -e^{24} + e^{35}, e^{16} + e^{23}, e^{25} + e^{34} + e^{18}$ | 24679    |
| 96421:123a | $0, 0, 0, -e^{12}, e^{13}, e^{14}, e^{15} + e^{24}, e^{16}, e^{28} + e^{46} + e^{35}$                        | 24679    |
| 96421:123b | $0, 0, 0, -e^{12}, -e^{13}, e^{14}, e^{24} + e^{15}, e^{16}, e^{35} + e^{46} + e^{28}$                       | 24679    |
| 96421:124a | $0, 0, 0, -e^{12}, e^{13}, e^{14}, e^{24} + e^{35}, e^{16}, e^{15} + e^{46} + e^{28}$                        | 24679    |

Table 2 – Continued to next page

Table 2 – Continued from previous page

| Name       | $\mathfrak{g}$                                                                                               | UCS Dim. |
|------------|--------------------------------------------------------------------------------------------------------------|----------|
| 96421:124b | $0, 0, 0, -e^{12}, -e^{13}, e^{14}, e^{35} + e^{24}, e^{16}, e^{15} + e^{28} + e^{46}$                       | 24679    |
| 96421:125  | $0, 0, 0, -e^{12}, -e^{13}, e^{14}, e^{25} + e^{34}, e^{16}, e^{46} + e^{15} + e^{28}$                       | 24679    |
| 96421:126a | $0, 0, 0, -e^{12}, e^{13}, e^{14}, e^{15} + e^{24}, e^{23} + e^{16}, e^{28} + e^{46}$                        | 24679    |
| 96421:126b | $0, 0, 0, -e^{12}, -e^{13}, e^{14}, e^{15} + e^{24}, e^{16} + e^{23}, e^{28} + e^{46}$                       | 24679    |
| 96421:127  | $0, 0, 0, e^{12}, e^{13}, e^{14}, e^{15}, e^{16} + e^{24}, e^{18} + e^{26} + e^{35}$                         | 24679    |
| 96421:128a | $0, 0, 0, e^{12}, e^{13}, e^{24}, e^{15}, e^{26} + e^{14}, e^{35} + e^{28} + e^{16}$                         | 24679    |
| 96421:128b | $0, 0, 0, -e^{12}, e^{13}, e^{24}, e^{15}, e^{26} + e^{14}, e^{28} + e^{35} + e^{16}$                        | 24679    |
| 96421:129  | $0, 0, 0, e^{12}, e^{13}, e^{14}, e^{34} + e^{25}, e^{16} + e^{24}, e^{18} + e^{26}$                         | 24679    |
| 96421:130  | $0, 0, 0, e^{12}, e^{13}, e^{24}, e^{34} + e^{25}, e^{26} + e^{14}, e^{28} + e^{16}$                         | 24679    |
| 96421:131a | $0, 0, 0, -e^{12}, e^{13}, e^{14}, e^{24}, e^{16} + e^{23}, e^{28} + e^{35} + e^{46}$                        | 24679    |
| 96421:131b | $0, 0, 0, -e^{12}, -e^{13}, e^{14}, e^{24}, e^{23} + e^{16}, e^{46} + e^{35} + e^{28}$                       | 24679    |
| 96421:132  | $0, 0, 0, -e^{12}, a_2 e^{13}, e^{14}, e^{23} + e^{15}, e^{24} + e^{16}, e^{46} + e^{28}$                    | 24679    |
| 96421:133  | $0, 0, 0, e^{12}, e^{13}, e^{24}, e^{23} + e^{15}, e^{26} + e^{14}, e^{18} + e^{46}$                         | 24679    |
| 96421:134  | $0, 0, 0, e^{12}, e^{13}, e^{24}, e^{35}, e^{14} + e^{26}, e^{46} + e^{23} + e^{18}$                         | 24679    |
| 96421:135a | $0, 0, 0, -e^{12}, -e^{13}, e^{14}, e^{34} + e^{25}, e^{23} + e^{16}, e^{28} + e^{46} + e^{35}$              | 24679    |
| 96421:135b | $0, 0, 0, -e^{12}, -e^{13}, -e^{14}, e^{25} + e^{34}, e^{23} + e^{16}, e^{28} + e^{46} + e^{35}$             | 24679    |
| 96421:136  | $0, 0, 0, -e^{12}, -e^{13}, e^{14}, e^{25} + e^{34}, e^{16} + e^{24}, e^{46} + e^{28}$                       | 24679    |
| 96421:137  | $0, 0, 0, e^{12}, e^{13}, e^{24}, e^{34} + e^{25}, e^{26} + e^{14}, e^{18} + e^{46}$                         | 24679    |
| 96421:138a | $0, 0, 0, -e^{12}, e^{13}, e^{14}, e^{15}, e^{24} + e^{16}, e^{35} + e^{46} + e^{28}$                        | 24679    |
| 96421:138b | $0, 0, 0, -e^{12}, -e^{13}, e^{14}, e^{15}, e^{16} + e^{24}, e^{28} + e^{46} + e^{35}$                       | 24679    |
| 96421:139  | $0, 0, 0, e^{12}, e^{13}, e^{24}, e^{15}, e^{14} + e^{26}, e^{46} + e^{18} + e^{35}$                         | 24679    |
| 96421:140  | $0, 0, 0, -e^{12}, e^{13}, e^{14}, e^{35}, e^{16} + e^{24}, e^{46} + e^{28} + e^{15}$                        | 24679    |
| 96421:141  | $0, 0, 0, -e^{12}, e^{13}, e^{23} + e^{14}, e^{35}, e^{16} + e^{34}, e^{36} + e^{18}$                        | 24579    |
| 96421:142  | $0, 0, 0, e^{12}, e^{13}, e^{14}, e^{15}, e^{16} + e^{35}, e^{18} + e^{37}$                                  | 13579    |
| 96421:143  | $0, 0, 0, -e^{12}, e^{13}, e^{24}, e^{14} + e^{23}, e^{26}, e^{17} + e^{28} + e^{34}$                        | 24679    |
| 96421:144  | $0, 0, 0, -e^{12}, e^{13}, e^{14}, e^{24}, e^{23} + e^{16}, e^{27} + e^{18} + e^{34}$                        | 24679    |
| 96421:145a | $0, 0, 0, (-1 + a_2)e^{12}, a_2 e^{13}, e^{14}, e^{24} + e^{15}, e^{16} + e^{23}, e^{25} + e^{34} + e^{18}$  | 24679    |
| 96421:145b | $0, 0, 0, (-1 + a_2)e^{12}, a_2 e^{13}, -e^{14}, e^{15} + e^{24}, e^{16} + e^{23}, e^{25} + e^{18} + e^{34}$ | 24679    |
| 96421:146  | $0, 0, 0, e^{12}, a_1 e^{13}, e^{14}, e^{15} + e^{23}, e^{24} + e^{16}, e^{18} + e^{26} + e^{35}$            | 24679    |
| 96421:147a | $0, 0, 0, e^{12}, e^{13}, e^{24}, e^{15} + e^{23}, e^{14} + e^{26}, e^{16} + e^{28} + e^{35}$                | 24679    |
| 96421:147b | $0, 0, 0, -e^{12}, e^{13}, e^{24}, e^{23} + e^{15}, e^{26} + e^{14}, e^{35} + e^{28} + e^{16}$               | 24679    |
| 96421:148a | $0, 0, 0, -e^{12}, e^{13}, e^{14}, e^{24}, e^{23} + e^{16}, e^{28} + e^{46} + e^{15}$                        | 24679    |
| 96421:148b | $0, 0, 0, -e^{12}, -e^{13}, e^{14}, e^{24}, e^{16} + e^{23}, e^{15} + e^{28} + e^{46}$                       | 24679    |
| 96421:149  | $0, 0, 0, e^{12}, e^{13}, e^{24}, e^{15}, e^{14} + e^{26}, e^{46} + e^{18} + e^{23}$                         | 24679    |
| 96421:150a | $0, 0, 0, -e^{12}, e^{13}, e^{14}, e^{24} + a_2 e^{15}, e^{23} + e^{16}, e^{35} + e^{46} + e^{28}$           | 24679    |
| 96421:150b | $0, 0, 0, -e^{12}, -e^{13}, e^{14}, e^{24} + a_2 e^{15}, e^{16} + e^{23}, e^{28} + e^{35} + e^{46}$          | 24679    |
| 96421:151a | $0, 0, 0, e^{12}, e^{13}, e^{14}, e^{35} + e^{24}, e^{23} - e^{16}, e^{46} + e^{15} + e^{28}$                | 24679    |
| 96421:151b | $0, 0, 0, e^{12}, -e^{13}, e^{14}, e^{35} + e^{24}, e^{23} - e^{16}, e^{28} + e^{46} + e^{15}$               | 24679    |
| 96421:151c | $0, 0, 0, -e^{12}, e^{13}, e^{14}, e^{35} + e^{24}, e^{23} + e^{16}, e^{15} + e^{28} + e^{46}$               | 24679    |
| 96421:151d | $0, 0, 0, -e^{12}, -e^{13}, e^{14}, e^{24} + e^{35}, e^{16} + e^{23}, e^{28} + e^{15} + e^{46}$              | 24679    |
| 96421:152a | $0, 0, 0, e^{12}, e^{13}, e^{14}, e^{25} + e^{34}, -e^{16} + e^{23}, e^{28} + e^{46} + e^{15}$               | 24679    |
| 96421:152b | $0, 0, 0, -e^{12}, -e^{13}, e^{14}, e^{25} + e^{34}, e^{16} + e^{23}, e^{15} + e^{28} + e^{46}$              | 24679    |
| 96421:153  | $0, 0, 0, e^{12}, e^{13}, e^{14}, e^{34} + e^{25}, e^{24} + e^{16}, e^{35} + e^{26} + e^{18}$                | 24679    |
| 96421:154a | $0, 0, 0, e^{12}, e^{13}, e^{24}, e^{34} + e^{25}, e^{14} + e^{26}, e^{28} + e^{35} + e^{16}$                | 24679    |
| 96421:154b | $0, 0, 0, e^{12}, e^{13}, -e^{24}, e^{25} + e^{34}, e^{26} - e^{14}, e^{28} + e^{35} + e^{16}$               | 24679    |
| 96421:155  | $0, 0, 0, -e^{12}, e^{13}, e^{23} + e^{14}, e^{15}, e^{16} + e^{34}, e^{18} + e^{36}$                        | 24579    |
| 96421:156a | $0, 0, 0, -e^{12}, e^{13}, e^{14}, e^{23} + a_2 e^{15}, e^{24} + e^{16}, e^{35} + e^{46} + e^{28}$           | 24679    |
| 96421:156b | $0, 0, 0, -e^{12}, -e^{13}, e^{14}, e^{23} + a_2 e^{15}, e^{16} + e^{24}, e^{28} + e^{35} + e^{46}$          | 24679    |
| 96421:157a | $0, 0, 0, e^{12}, e^{13}, e^{24}, e^{23} + e^{15}, e^{26} + e^{14}, e^{46} + e^{35} + e^{18}$                | 24679    |
| 96421:157b | $0, 0, 0, e^{12}, e^{13}, e^{24}, -e^{15} + e^{23}, e^{26} + e^{14}, e^{18} + e^{46} + e^{35}$               | 24679    |
| 96421:158a | $0, 0, 0, -e^{12}, -e^{13}, e^{14}, e^{34} + e^{25}, e^{16} + e^{24}, e^{46} + e^{35} + e^{28}$              | 24679    |
| 96421:158b | $0, 0, 0, -e^{12}, -e^{13}, -e^{14}, e^{34} + e^{25}, e^{16} + e^{24}, e^{28} + e^{46} + e^{35}$             | 24679    |
| 96421:159  | $0, 0, 0, e^{12}, e^{13}, e^{24}, e^{34} + e^{25}, e^{14} + e^{26}, e^{46} + e^{18} + e^{35}$                | 24679    |
| 96421:161  | $0, 0, 0, e^{12}, e^{13}, e^{24}, e^{15}, e^{26}, e^{17} + e^{28}$                                           | 13579    |
| 96421:162  | $0, 0, 0, e^{12}, e^{13}, e^{24}, e^{35}, e^{26}, e^{15} + e^{28} + e^{37}$                                  | 13579    |
| 96421:163  | $0, 0, 0, e^{12}, e^{13}, e^{24}, e^{35}, e^{15} + e^{26}, e^{18} + e^{46}$                                  | 23579    |
| 96421:164a | $0, 0, 0, e^{12}, e^{13}, e^{14}, e^{15} + e^{23}, e^{16} + e^{35}, e^{18} + e^{37}$                         | 13579    |
| 96421:164b | $0, 0, 0, -e^{12}, e^{13}, e^{14}, e^{15} + e^{23}, e^{35} + e^{16}, e^{37} + e^{18}$                        | 13579    |

Table 2 – Continued to next page

Table 2 – Continued from previous page

| Name       | $\mathfrak{g}$                                                                                            | UCS Dim. |
|------------|-----------------------------------------------------------------------------------------------------------|----------|
| 96421:165  | $0, 0, 0, -e^{12}, e^{13}, e^{23} + e^{14}, e^{24}, e^{16} + e^{34}, e^{18} + e^{36}$                     | 34579    |
| 96421:166  | $0, 0, 0, e^{12}, e^{13}, e^{24}, e^{34} + e^{25}, e^{35} + e^{26}, e^{28} + e^{37}$                      | 13579    |
| 96421:167  | $0, 0, 0, e^{12}, e^{13}, e^{24}, e^{34} + e^{25}, e^{26} + e^{14}, e^{18} + e^{46} + e^{23}$             | 24679    |
| 96421:169  | $0, 0, 0, -e^{12}, -e^{13}, e^{14}, e^{34} + e^{25}, e^{16} + e^{24}, e^{46} + e^{28} + e^{15}$           | 24679    |
| 96421:170a | $0, 0, 0, -e^{12}, e^{13}, e^{23} + e^{14}, e^{35} + e^{24}, e^{16} + e^{34}, e^{36} + e^{18}$            | 24579    |
| 96421:170b | $0, 0, 0, -e^{12}, -e^{13}, e^{23} + e^{14}, e^{35} + e^{24}, e^{16} + e^{34}, e^{18} + e^{36}$           | 24579    |
| 96421:172a | $0, 0, 0, e^{12}, e^{13}, e^{24}, e^{15}, e^{26}, e^{28} + e^{35} + e^{17}$                               | 13579    |
| 96421:172b | $0, 0, 0, -e^{12}, e^{13}, e^{24}, e^{15}, e^{26}, e^{28} + e^{17} + e^{35}$                              | 13579    |
| 96421:173  | $0, 0, 0, e^{12}, e^{13}, e^{14}, e^{35}, e^{16}, e^{24} + e^{37} + e^{18}$                               | 13579    |
| 96421:174  | $0, 0, 0, e^{12}, e^{13}, e^{24}, e^{35}, e^{26}, e^{37} + e^{28} + e^{14}$                               | 13579    |
| 96421:175  | $0, 0, 0, -e^{12}, e^{13}, e^{14}, e^{35}, e^{16}, e^{37} + e^{46} + e^{28}$                              | 13579    |
| 96421:176  | $0, 0, 0, e^{12}, e^{13}, e^{24}, e^{35}, e^{26}, e^{18} + e^{46} + e^{37}$                               | 13579    |
| 96421:177  | $0, 0, 0, e^{12}, e^{13}, e^{14}, e^{35}, e^{16} + e^{23}, e^{18} + e^{37} + e^{25}$                      | 13579    |
| 96421:179  | $0, 0, 0, -e^{12}, e^{13}, e^{14} + e^{23}, e^{15} + e^{24}, e^{34} + e^{16}, e^{18} + e^{36}$            | 24579    |
| 96421:181  | $0, 0, 0, -e^{12}, e^{13}, e^{14} + e^{23}, e^{35}, e^{16} + e^{34}, e^{24} + e^{18} + e^{36}$            | 24579    |
| 96421:185  | $0, 0, 0, e^{12}, -e^{13}, e^{14} + e^{23}, e^{35}, -2e^{16} + e^{34} + e^{25}, e^{18} + e^{45}$          | 23579    |
| 96421:186  | $0, 0, 0, e^{12}, e^{13}, e^{14} + e^{23}, e^{15}, e^{25} + e^{16}, e^{18} + e^{27}$                      | 13579    |
| 96421:187  | $0, 0, 0, e^{12}, e^{13}, e^{24}, e^{14}, e^{15} + e^{26}, e^{46} + e^{18}$                               | 23579    |
| 96421:188  | $0, 0, 0, e^{12}, e^{13}, e^{14}, e^{15}, e^{35} + e^{16}, e^{24} + e^{37} + e^{18}$                      | 13579    |
| 96421:189  | $0, 0, 0, e^{12}, e^{13}, e^{24}, e^{35}, e^{26} + e^{15}, e^{23} + e^{18} + e^{46}$                      | 23579    |
| 96421:190  | $0, 0, 0, -e^{12}, e^{13}, e^{14}, e^{35}, e^{16} + e^{23}, e^{28} + e^{37} + e^{46}$                     | 13579    |
| 96421:191  | $0, 0, 0, e^{12}, e^{13}, e^{24}, e^{14} + e^{35}, e^{15} + e^{26}, e^{18} + e^{46}$                      | 23579    |
| 96421:192  | $0, 0, 0, e^{12}, e^{13}, e^{24}, e^{34} + e^{25}, e^{26} + e^{15}, e^{46} + e^{18}$                      | 23579    |
| 96421:193  | $0, 0, 0, e^{12}, e^{13}, e^{24}, e^{15}, e^{26} + e^{35}, e^{18} + e^{37} + e^{46}$                      | 13579    |
| 96421:194a | $0, 0, 0, e^{12}, e^{13}, e^{24}, e^{35}, e^{15} + e^{26}, e^{18} + e^{46} + e^{37}$                      | 13579    |
| 96421:194b | $0, 0, 0, e^{12}, e^{13}, e^{24}, e^{35}, e^{26} - e^{15}, e^{37} + e^{18} + e^{46}$                      | 13579    |
| 96421:196  | $0, 0, 0, -e^{12}, e^{13}, e^{23} + e^{14}, e^{15}, e^{16} + e^{34}, e^{24} + e^{36} + e^{18}$            | 24579    |
| 96421:197  | $0, 0, 0, e^{12}, e^{13}, e^{24}, e^{34} + e^{25}, e^{26} + e^{35}, e^{28} + e^{37} + e^{15}$             | 13579    |
| 96421:201  | $0, 0, 0, e^{12}, -e^{13}, e^{14} + e^{23}, e^{15}, -2e^{16} + e^{25} + e^{34}, e^{45} + e^{18}$          | 23579    |
| 96421:204  | $0, 0, 0, e^{12}, e^{13}, e^{23} + e^{14}, e^{35}, e^{25} + e^{16}, e^{36} + e^{45} + e^{18}$             | 23579    |
| 96421:206  | $0, 0, 0, e^{12}, e^{13}, 2e^{14}, e^{35}, e^{34} + e^{16} + e^{25}, e^{36} + e^{45} + e^{18}$            | 23579    |
| 96421:207  | $0, 0, 0, -e^{12}, -2e^{13}, e^{14} - e^{23}, e^{35}, e^{34} + e^{25} + e^{16}, e^{28} + e^{46}$          | 23579    |
| 96421:208  | $0, 0, 0, -e^{12}, e^{13}, e^{14}, e^{15}, e^{16}, e^{28} + e^{17} + e^{46}$                              | 13579    |
| 96421:209  | $0, 0, 0, -e^{12}, e^{13}, e^{24}, e^{15} + e^{23}, e^{26}, e^{17} + e^{28} + e^{34}$                     | 13579    |
| 96421:210  | $0, 0, 0, e^{12}, e^{13}, e^{24}, e^{23} + e^{14}, e^{26} + e^{15}, e^{46} + e^{18}$                      | 23579    |
| 96421:211  | $0, 0, 0, -e^{12}, e^{13}, e^{14}, e^{35}, e^{16}, e^{37} + e^{15} + e^{46} + e^{28}$                     | 13579    |
| 96421:212  | $0, 0, 0, e^{12}, e^{13}, e^{14}, e^{35}, e^{16} + e^{24}, e^{18} + e^{26} + e^{37}$                      | 13579    |
| 96421:213  | $0, 0, 0, e^{12}, e^{13}, e^{24}, e^{35}, e^{14} + e^{26}, e^{16} + e^{28} + e^{37}$                      | 13579    |
| 96421:215  | $0, 0, 0, e^{12}, e^{13}, e^{14} + e^{23}, e^{15}, e^{16} + e^{25}, e^{27} + e^{18} + e^{35}$             | 13579    |
| 96421:216  | $0, 0, 0, e^{12}, e^{13}, e^{24}, e^{14}, e^{15} + e^{26}, e^{18} + e^{46} + e^{35}$                      | 23579    |
| 96421:217a | $0, 0, 0, e^{12}, e^{13}, e^{14}, e^{15} + e^{23}, e^{35} + e^{16}, e^{18} + e^{24} + e^{37}$             | 13579    |
| 96421:217b | $0, 0, 0, -e^{12}, e^{13}, e^{14}, e^{23} + e^{15}, e^{16} + e^{35}, e^{18} + e^{37} + e^{24}$            | 13579    |
| 96421:218  | $0, 0, 0, -e^{12}, e^{13}, e^{24}, e^{14}, e^{26} + e^{15}, e^{28} + e^{45} + e^{37}$                     | 13579    |
| 96421:219  | $0, 0, 0, -e^{12}, e^{13}, e^{14}, e^{35}, e^{16} + e^{24}, e^{28} + e^{37} + e^{46}$                     | 13579    |
| 96421:220  | $0, 0, 0, e^{12}, e^{13}, e^{24}, e^{35}, e^{14} + e^{26}, e^{37} + e^{46} + e^{18}$                      | 13579    |
| 96421:221  | $0, 0, 0, e^{12}, e^{13}, e^{24}, e^{25} + e^{34}, e^{26} + e^{35}, e^{28} + e^{14} + e^{37}$             | 13579    |
| 96421:222  | $0, 0, 0, e^{12}, e^{13}, e^{24}, e^{25} + e^{34}, e^{26} + e^{15}, e^{18} + e^{46} + e^{35}$             | 23579    |
| 96421:224a | $0, 0, 0, e^{12}, e^{13}, e^{24}, e^{15} + e^{23}, e^{26} + e^{35}, e^{46} + e^{37} + e^{18}$             | 13579    |
| 96421:224b | $0, 0, 0, e^{12}, e^{13}, -e^{24}, e^{15} + e^{23}, e^{26} + e^{35}, e^{18} + e^{46} + e^{37}$            | 13579    |
| 96421:225  | $0, 0, 0, -e^{12}, e^{13}, e^{14} + e^{23}, e^{24}, e^{16} + e^{34}, e^{18} + e^{27} + e^{36}$            | 24579    |
| 96421:228  | $0, 0, 0, e^{12}, -e^{13}, e^{14} + e^{23}, e^{24}, -2e^{16} + e^{34} + e^{25}, e^{18} + e^{45}$          | 23579    |
| 96421:229  | $0, 0, 0, e^{12}, e^{13}, e^{14} + e^{23}, e^{15}, e^{25} + e^{16}, e^{36} + e^{18} + e^{45}$             | 23579    |
| 96421:230  | $0, 0, 0, -e^{12}, e^{13}, e^{24}, e^{14} + e^{35}, e^{26} + e^{15}, e^{37} + e^{45} + e^{28}$            | 13579    |
| 96421:231  | $0, 0, 0, -e^{12}, -e^{13}, e^{14}, e^{25} + e^{34}, e^{35} + e^{16}, e^{37} + e^{46} + e^{28}$           | 13579    |
| 96421:233  | $0, 0, 0, e^{12}, e^{13}, 2e^{14}, e^{15}, e^{16} + e^{25} + e^{34}, e^{45} + e^{36} + e^{18}$            | 23579    |
| 96421:234  | $0, 0, 0, -e^{12}, e^{13}, e^{14} + e^{23}, 2e^{24}, e^{34} + e^{16}, e^{46} + e^{37} + e^{28}$           | 24579    |
| 96421:237  | $0, 0, 0, -e^{12}, -2e^{13}, -e^{23} + e^{14}, e^{15}, e^{16} + e^{25} + e^{34}, e^{28} + e^{46}$         | 23579    |
| 96421:238a | $0, 0, 0, e^{12}, -e^{13}, e^{23} + e^{14}, e^{35} + e^{24}, -2e^{16} + e^{34} + e^{25}, e^{18} + e^{45}$ | 23579    |

Table 2 – Continued to next page



Table 2 – Continued from previous page

| Name       | $\mathfrak{g}$                                                                                                                 | UCS Dim. |
|------------|--------------------------------------------------------------------------------------------------------------------------------|----------|
| 96421:238b | $0, 0, 0, e^{12}, -e^{13}, e^{14} + e^{23}, e^{35} - e^{24}, e^{34} - 2e^{16} + e^{25}, e^{45} + e^{18}$                       | 23579    |
| 96421:239  | $0, 0, 0, e^{12}, -e^{13}, e^{23} + e^{14}, e^{35}, -2e^{16} + e^{34} + e^{25}, e^{18} + e^{37} + e^{45}$                      | 13579    |
| 96421:240  | $0, 0, 0, e^{12}, (-1 + a_3)e^{13}, e^{14}a_3 + e^{23}, e^{35}, e^{25} + e^{34} + (-2 + a_3)e^{16}, e^{45} + e^{36} + e^{18}$  | 23579    |
| 96421:241  | $0, 0, 0, e^{12}, e^{13}, e^{24}, e^{14}, e^{15} + e^{26}, e^{18} + e^{23} + e^{46}$                                           | 23579    |
| 96421:242  | $0, 0, 0, -e^{12}, e^{13}, e^{14}, e^{15}, e^{23} + e^{16}, e^{46} + e^{28} + e^{17}$                                          | 13579    |
| 96421:243a | $0, 0, 0, -e^{12}, e^{13}, e^{14}, e^{15}, e^{16}, e^{17} + e^{28} + e^{46} + e^{35}$                                          | 13579    |
| 96421:243b | $0, 0, 0, -e^{12}, -e^{13}, e^{14}, e^{15}, e^{16}, e^{17} + e^{35} + e^{46}$                                                  | 13579    |
| 96421:244  | $0, 0, 0, -e^{12}, e^{13}, e^{14}, e^{15}, e^{16}, e^{18} + e^{27} + e^{45} + e^{36}$                                          | 13579    |
| 96421:245a | $0, 0, 0, e^{12}, e^{13}, e^{24}, e^{35} + e^{14}, e^{26} + e^{15}, e^{18} + e^{46} + e^{23}$                                  | 23579    |
| 96421:245b | $0, 0, 0, e^{12}, e^{13}, e^{24}, e^{35} - e^{14}, e^{26} + e^{15}, e^{18} + e^{46} + e^{23}$                                  | 23579    |
| 96421:246  | $0, 0, 0, e^{12}, e^{13}, e^{24}, e^{25} + e^{34}, e^{15} + e^{26}, e^{18} + e^{23} + e^{46}$                                  | 23579    |
| 96421:247  | $0, 0, 0, e^{12}, e^{13}, e^{14} + e^{23}, e^{24} + e^{15}, e^{25} + e^{16}, e^{27} + e^{18}$                                  | 13579    |
| 96421:248  | $0, 0, 0, e^{12}, e^{13}, e^{24}, a_2e^{14} + e^{23}, e^{15} + e^{26}, e^{46} + e^{18} + e^{35}$                               | 23579    |
| 96421:249a | $0, 0, 0, -e^{12}, e^{13}, e^{14}, e^{35}, e^{23} + e^{16}, e^{37} + e^{15} + e^{46} + e^{28}$                                 | 13579    |
| 96421:249b | $0, 0, 0, -e^{12}, -e^{13}, e^{14}, e^{35}, e^{16} + e^{23}, e^{15} + e^{28} + e^{37} + e^{46}$                                | 13579    |
| 96421:250  | $0, 0, 0, -e^{12}, -e^{13}, e^{23} + e^{14}, e^{15}, e^{16} + e^{34}, e^{45} + e^{27} + e^{18}$                                | 13579    |
| 96421:252a | $0, 0, 0, e^{12}, e^{13}, e^{14}, e^{15}, e^{16} + e^{24} + e^{35}, e^{37} + e^{18} + e^{26}$                                  | 13579    |
| 96421:252b | $0, 0, 0, -e^{12}, e^{13}, e^{14}, e^{15}, e^{24} + e^{35} + e^{16}, e^{37} + e^{26} + e^{18}$                                 | 13579    |
| 96421:253  | $0, 0, 0, e^{12}, e^{13}, e^{14}, e^{15}, e^{16} + e^{25} + e^{34}, e^{36} + e^{18} + e^{27}$                                  | 13579    |
| 96421:254  | $0, 0, 0, -e^{12}, e^{13}, e^{24}, e^{14} + e^{23}, e^{26} + e^{15}, e^{28} + e^{45} + e^{37}$                                 | 13579    |
| 96421:255  | $0, 0, 0, e^{12}, e^{13}, e^{14} + e^{23}, e^{24}, e^{25} + e^{16}, e^{36} + e^{18} + e^{45}$                                  | 23579    |
| 96421:256  | $0, 0, 0, -e^{12}, -e^{13}, e^{24}, e^{25} + e^{34}, 2e^{15} + e^{26}, e^{28} + e^{17} + e^{45}$                               | 13579    |
| 96421:257  | $0, 0, 0, -e^{12}, -e^{13}, e^{14}, 2e^{15}, e^{16} + e^{25} + e^{34}, e^{27} + e^{18} + e^{45}$                               | 13579    |
| 96421:259  | $0, 0, 0, e^{12}, e^{13}, 2e^{14}, e^{24}, e^{25} + e^{34} + e^{16}, e^{18} + e^{45} + e^{36}$                                 | 23579    |
| 96421:260  | $0, 0, 0, e^{12}, e^{13}, e^{24}, e^{15}, e^{26} + e^{35} + e^{14}, e^{37} + e^{18} + e^{46}$                                  | 13579    |
| 96421:261  | $0, 0, 0, e^{12}, -e^{13}, e^{23} + e^{14}, e^{24} + e^{15}, -2e^{16} + e^{34} + e^{25}, e^{18} + e^{45}$                      | 23579    |
| 96421:262  | $0, 0, 0, -e^{12}, -2e^{13}, -e^{23} + e^{14}, e^{24}, e^{16} + e^{25} + e^{34}, e^{28} + e^{46}$                              | 23579    |
| 96421:263  | $0, 0, 0, e^{12}, e^{13}, 2e^{14}, e^{15} + e^{23}, e^{16} + e^{25} + e^{34}, e^{36} + e^{18} + e^{45}$                        | 23579    |
| 96421:264a | $0, 0, 0, e^{12}, e^{13}, e^{14} + e^{23}, e^{24} + e^{35}, e^{16} + e^{25}, e^{36} + e^{18} + e^{45}$                         | 23579    |
| 96421:264b | $0, 0, 0, e^{12}, -e^{13}, e^{23} - e^{14}, e^{35} + e^{24}, -e^{16} + e^{25}, e^{18} + e^{36} + e^{45}$                       | 23579    |
| 96421:265a | $0, 0, 0, e^{12}, e^{13}, 2e^{14}, e^{24} + e^{35}, e^{16} + e^{25} + e^{34}, e^{36} + e^{18} + e^{45}$                        | 23579    |
| 96421:265b | $0, 0, 0, e^{12}, e^{13}, 2e^{14}, -e^{24} + e^{35}, e^{16} + e^{25} + e^{34}, e^{36} + e^{18} + e^{45}$                       | 23579    |
| 96421:266a | $0, 0, 0, -e^{12}, -2e^{13}, -e^{23} + e^{14}, e^{35} + e^{24}, e^{16} + e^{25} + e^{34}, e^{28} + e^{46}$                     | 23579    |
| 96421:266b | $0, 0, 0, -e^{12}, -2e^{13}, -e^{23} + e^{14}, e^{35} - e^{24}, e^{16} + e^{25} + e^{34}, e^{28} + e^{46}$                     | 23579    |
| 96421:267  | $0, 0, 0, e^{12}, e^{13}a_2, (1 + a_2)e^{14} + e^{23}, e^{15}, (-1 + a_2)e^{16} + e^{25} + e^{34}, e^{45} + e^{36} + e^{18}$   | 23579    |
| 96421:268a | $0, 0, 0, -e^{12}, -2e^{13}, -e^{23} + e^{14}, e^{15}, e^{16} + e^{25} + e^{34}, e^{28} + e^{35} + e^{46}$                     | 23579    |
| 96421:268b | $0, 0, 0, -e^{12}, -2e^{13}, -e^{23} - e^{14}, e^{15}, e^{16} + e^{25} + e^{34}, e^{28} + e^{35} + e^{46}$                     | 23579    |
| 96421:269  | $0, 0, 0, -e^{12}, -2e^{13}, -e^{23} + e^{14}, e^{35}, e^{16} + e^{25} + e^{34}, e^{15} + e^{28} + e^{46}$                     | 23579    |
| 96421:270a | $0, 0, 0, -e^{12}, e^{13}, -e^{23} + e^{14}, e^{35}, e^{16} - 2e^{25} + e^{34}, e^{28} + e^{37} + e^{46}$                      | 13579    |
| 96421:270b | $0, 0, 0, -e^{12}, -e^{13}, -e^{23} + e^{14}, e^{35}, e^{16} + 2e^{25} + e^{34}, e^{37} + e^{46} + e^{28}$                     | 13579    |
| 96421:271  | $0, 0, 0, -e^{12}, e^{13}, e^{14}, e^{15}, e^{16} + e^{24}, e^{46} + e^{17} + e^{28}$                                          | 13579    |
| 96421:272  | $0, 0, 0, -e^{12}, e^{13}, e^{14}, e^{23} + e^{15}, e^{16}, e^{36} + e^{45} + e^{27} + e^{18}$                                 | 13579    |
| 96421:273a | $0, 0, 0, -e^{12}, e^{13}, e^{14}, e^{15}, e^{16} + e^{23}, e^{28} + e^{17} + e^{35} + e^{46}$                                 | 13579    |
| 96421:273b | $0, 0, 0, -e^{12}, -e^{13}, e^{14}, e^{15}, e^{23} + e^{16}, e^{17} + e^{28} + e^{46} + e^{35}$                                | 13579    |
| 96421:274  | $0, 0, 0, -e^{12}, e^{13}, e^{14}, e^{35}, e^{24} + e^{16}, e^{37} + e^{46} + e^{15} + e^{28}$                                 | 13579    |
| 96421:276  | $0, 0, 0, e^{12}, e^{13}, e^{14} + e^{23}, e^{24} + e^{15}, e^{25} + e^{16}, e^{18} + e^{27} + e^{35}$                         | 13579    |
| 96421:278  | $0, 0, 0, -e^{12}, e^{13}, e^{14} + e^{23}, e^{24}, e^{25} + e^{16}, e^{46} + e^{37} + e^{28}$                                 | 13579    |
| 96421:280  | $0, 0, 0, e^{12}, e^{13}, e^{14} + e^{23}, e^{24} + e^{15}, e^{25} + e^{16}, e^{36} + e^{18} + e^{45}$                         | 23579    |
| 96421:281a | $0, 0, 0, e^{12}, a_1e^{13}, e^{14}, e^{15} + e^{23}, e^{24} + e^{35} + e^{16}, e^{18} + e^{37} + e^{26}$                      | 13579    |
| 96421:281b | $0, 0, 0, -e^{12}, a_1e^{13}, e^{14}, e^{15} + e^{23}, e^{24} + e^{35} + e^{16}, e^{37} + e^{26} + e^{18}$                     | 13579    |
| 96421:282  | $0, 0, 0, e^{12}, e^{13}, e^{14}, e^{15} + e^{23}, e^{25} + e^{34} + e^{16}, e^{18} + e^{36} + e^{27}$                         | 13579    |
| 96421:283  | $0, 0, 0, -e^{12}, -e^{13}, e^{14}, e^{24}, e^{16} + e^{25} + e^{34}, e^{28} + e^{37} + e^{46}$                                | 13579    |
| 96421:284  | $0, 0, 0, -a_1e^{12}, -e^{13}, e^{23} + e^{14}, (1 + a_1)e^{15}, e^{25} + e^{34} + e^{16}(-1 + a_1), e^{27} + e^{18} + e^{45}$ | 13579    |
| 96421:285  | $0, 0, 0, e^{12}a_1, e^{13}(1 + a_1), e^{14} + e^{23}, e^{15}, e^{25} + e^{34} + e^{16}, e^{18} + e^{36} + e^{27}$             | 13579    |
| 96421:286  | $0, 0, 0, e^{12}, e^{13}, 2e^{14}, e^{24} + e^{15}, e^{25} + e^{34} + e^{16}, e^{18} + e^{45} + e^{36}$                        | 23579    |
| 96421:287  | $0, 0, 0, -e^{12}, -e^{13}, e^{14}, 2e^{15} + e^{23}, e^{16} + e^{25} + e^{34}, e^{27} + e^{18} + e^{45}$                      | 13579    |
| 96421:288  | $0, 0, 0, -e^{12}, -e^{13}, e^{14}, e^{25} + e^{34}, e^{16} + e^{35}, e^{15} + e^{28} + e^{37} + e^{46}$                       | 13579    |
| 96421:290  | $0, 0, 0, -e^{12}, -2e^{13}, -e^{23} + e^{14}, e^{24} + e^{15}, e^{16} + e^{25} + e^{34}, e^{46} + e^{28}$                     | 23579    |

Table 2 – Continued to next page

Table 2 – Continued from previous page

| Name       | $\mathfrak{g}$                                                                                                                                                 | UCS Dim. |
|------------|----------------------------------------------------------------------------------------------------------------------------------------------------------------|----------|
| 96421:291  | $0, 0, 0, e^{12}, e^{13}, e^{24}, e^{25} + e^{34}, e^{26} + e^{35} + e^{14}, e^{37} + e^{16} + e^{28}$                                                         | 13579    |
| 96421:292  | $0, 0, 0, -e^{12}, e^{13}, e^{14} + e^{23}, 2e^{24}, e^{16} + e^{34}, e^{37} + e^{15} + e^{46} + e^{28}$                                                       | 14579    |
| 96421:293a | $0, 0, 0, e^{12}, e^{13}, e^{24}, e^{15} + e^{23}, e^{26} + e^{35} + e^{14}, e^{37} + e^{18} + e^{46}$                                                         | 13579    |
| 96421:293b | $0, 0, 0, e^{12}, e^{13}, -e^{24}, e^{15} + e^{23}, e^{14} + e^{26} + e^{35}, e^{37} + e^{18} + e^{46}$                                                        | 13579    |
| 96421:294a | $0, 0, 0, -e^{12}, e^{13}, e^{14} + e^{23}, e^{24} + e^{35}, e^{25} + e^{16}, e^{37} + e^{46} + e^{28}$                                                        | 13579    |
| 96421:294b | $0, 0, 0, -e^{12}, -e^{13}, e^{14} + e^{23}, e^{35} + e^{24}, -e^{25} + e^{16}, e^{46} + e^{37} + e^{28}$                                                      | 13579    |
| 96421:295  | $0, 0, 0, e^{12}, e^{13}(1 + a_4), e^{23} + (2 + a_4)e^{14}, e^{24}, e^{25} + e^{34} + e^{16}, a_4, e^{18} + e^{45} + e^{36}$                                  | 23579    |
| 96421:296a | $0, 0, 0, -e^{12}, -2e^{13}, -e^{23} + e^{14}, e^{24}, e^{16} + e^{25} + e^{34}, e^{35} + e^{46} + e^{28}$                                                     | 23579    |
| 96421:296b | $0, 0, 0, -e^{12}, -2e^{13}, -e^{23} - e^{14}, e^{24}, e^{16} + e^{25} + e^{34}, e^{35} + e^{46} + e^{28}$                                                     | 23579    |
| 96421:297a | $0, 0, 0, -e^{12}, e^{13}, e^{14} + e^{23}, 2e^{24} + e^{35}, e^{16} + e^{34}, e^{37} + e^{46} + e^{28}$                                                       | 13579    |
| 96421:297b | $0, 0, 0, -e^{12}, -e^{13}, e^{14} + e^{23}, e^{35} + 2e^{24}, e^{34} + e^{16}, e^{28} + e^{37} + e^{46}$                                                      | 13579    |
| 96421:298a | $0, 0, 0, -e^{12}, e^{13}, e^{14}, e^{35} + e^{24}, e^{34} - e^{25} + e^{16}, e^{46} + e^{37} + e^{28}$                                                        | 13579    |
| 96421:298b | $0, 0, 0, -e^{12}, -e^{13}, e^{14}, e^{35} + e^{24}, e^{34} + e^{25} + e^{16}, e^{28} + e^{37} + e^{46}$                                                       | 13579    |
| 96421:299a | $0, 0, 0, -e^{12}, -e^{13}, e^{14}, e^{25} + e^{34}, e^{16} + e^{35} + e^{24}, e^{28} + e^{37} + e^{46}$                                                       | 13579    |
| 96421:299b | $0, 0, 0, -e^{12}, -e^{13}, e^{14}, e^{25} + e^{34}, e^{16} + e^{35} - e^{24}, e^{28} + e^{37} + e^{46}$                                                       | 13579    |
| 96421:300a | $0, 0, 0, e^{12}, (-1 + a_3)e^{13}, e^{23} + e^{14}a_3, e^{24} + e^{35}, e^{16}(-2 + a_3) + e^{25} + e^{34}, e^{18} + e^{45} + e^{36}$                         | 23579    |
| 96421:300b | $0, 0, 0, e^{12}, (-1 + a_3)e^{13}, e^{23} + e^{14}a_3, -e^{24} + e^{35}, e^{16}(-2 + a_3) + e^{25} + e^{34}, e^{18} + e^{45} + e^{36}$                        | 23579    |
| 96421:301  | $0, 0, 0, -e^{12}, e^{13}, e^{14}, e^{15} + e^{24}, e^{16}, e^{45} + e^{18} + e^{27} + e^{36}$                                                                 | 13579    |
| 96421:302a | $0, 0, 0, -e^{12}, e^{13}, e^{14}, e^{15}, e^{16} + e^{24}, e^{46} + e^{35} + e^{17} + e^{28}$                                                                 | 13579    |
| 96421:302b | $0, 0, 0, -e^{12}, -e^{13}, e^{14}, e^{15}, e^{24} + e^{16}, e^{35} + e^{46} + e^{28} + e^{17}$                                                                | 13579    |
| 96421:303  | $0, 0, 0, -(1 + a_4)e^{12}, e^{13}, e^{14} + e^{23}, a_4e^{15}, e^{25} + e^{16}, e^{36} + e^{27} + e^{18} + e^{45}$                                            | 13579    |
| 96421:304  | $0, 0, 0, -e^{12}, -e^{13}, e^{23} + e^{14}, e^{15} + e^{24}, e^{16} + e^{34}, e^{27} + e^{18} + e^{45}$                                                       | 13579    |
| 96421:305  | $0, 0, 0, e^{12}, -e^{13}, e^{23} + e^{14}, e^{24}, e^{34} + e^{25} - 2e^{16}, e^{27} + e^{45} + e^{18}$                                                       | 13579    |
| 96421:307  | $0, 0, 0, -e^{12}, (-1 + a_3)e^{13}, e^{23} + e^{14}a_3, e^{15}, e^{34} + e^{16}, e^{18} + e^{27} + e^{45} + e^{36}$                                           | 13579    |
| 96421:308  | $0, 0, 0, e^{12}, e^{13}, e^{14}, e^{24} + e^{15}, e^{25} + e^{34} + e^{16}, e^{36} + e^{27} + e^{18}$                                                         | 13579    |
| 96421:309  | $0, 0, 0, e^{12}a_2, e^{13}a_2, e^{14}(1 + a_2), -(1 + a_2)e^{15}, e^{25} + e^{34} + e^{16}, e^{18} + e^{45} + e^{36} + e^{27}$                                | 13579    |
| 96421:310  | $0, 0, 0, -e^{12}, -2e^{13}, -e^{23} + e^{14}, e^{24}, e^{16} + e^{25} + e^{34}, e^{46} + e^{15} + e^{28}$                                                     | 23579    |
| 96421:311a | $0, 0, 0, -e^{12}, -2e^{13}, -e^{23} + e^{14}, e^{15}, e^{16} + e^{25} + e^{34}, e^{46} + e^{28} + e^{17}$                                                     | 13579    |
| 96421:311b | $0, 0, 0, -e^{12}, -2e^{13}, -e^{23} + e^{14}, -e^{15}, e^{16} + e^{25} + e^{34}, e^{46} + e^{28} + e^{17}$                                                    | 13579    |
| 96421:312  | $0, 0, 0, -e^{12}, -e^{13}, e^{14}, 2e^{15} + e^{24}, e^{16} + e^{25} + e^{34}, e^{27} + e^{18} + e^{45}$                                                      | 13579    |
| 96421:313  | $0, 0, 0, -e^{12}, e^{13}a_2, e^{14} + e^{23}(1 + a_2), e^{24}(2 + a_2), e^{25} + e^{16} + e^{34}, e^{37} + e^{46} + e^{28}$                                   | 13579    |
| 96421:314  | $0, 0, 0, e^{12}, (1 + a_4)e^{13}, (2 + a_4)e^{14} + e^{23}, e^{24} + e^{15}, e^{16}a_4 + e^{25} + e^{34}, e^{18} + e^{45} + e^{36}$                           | 23579    |
| 96421:315a | $0, 0, 0, -e^{12}, -2e^{13}, -e^{23} + e^{14}, e^{24} + e^{15}, e^{16} + e^{25} + e^{34}, e^{35} + e^{46} + e^{28}$                                            | 23579    |
| 96421:315b | $0, 0, 0, -e^{12}, -2e^{13}, -e^{23} - e^{14}, e^{24} + e^{15}, e^{16} + e^{25} + e^{34}, e^{35} + e^{46} + e^{28}$                                            | 23579    |
| 96421:316a | $0, 0, 0, -e^{12}, -2e^{13}, -e^{23} + e^{14}, e^{35} + e^{24}, e^{16} + e^{25} + e^{34}, e^{46} + e^{15} + e^{28}$                                            | 23579    |
| 96421:316b | $0, 0, 0, -e^{12}, -2e^{13}, -e^{23} + e^{14}, e^{35} - e^{24}, e^{16} + e^{25} + e^{34}, e^{46} + e^{15} + e^{28}$                                            | 23579    |
| 96421:317a | $0, 0, 0, -e^{12}, e^{13}, -e^{23} + e^{14}, e^{35}, e^{16} - 2e^{25} + e^{34}, e^{37} + e^{46} + e^{15} + e^{28}$                                             | 13579    |
| 96421:317b | $0, 0, 0, -e^{12}, -e^{13}, -e^{23} + e^{14}, e^{35}, e^{16} + 2e^{25} + e^{34}, e^{15} + e^{28} + e^{37} + e^{46}$                                            | 13579    |
| 96421:318a | $0, 0, 0, -e^{12}, e^{13}, e^{14} + (1 + a_4)e^{23}, e^{35} + e^{24}(2 + a_4), e^{16} + e^{34} + e^{25}a_4, e^{37} + e^{46} + e^{28}$                          | 13579    |
| 96421:318b | $0, 0, 0, -e^{12}, -e^{13}, e^{14} - (1 + a_4)e^{23}, -e^{24}(-2 + a_4) + e^{35}, e^{16} + e^{34} + e^{25}a_4, e^{37} + e^{46} + e^{28}$                       | 13579    |
| 96421:319  | $0, 0, 0, -e^{12}, e^{13}, e^{14} + e^{23}, e^{24}, e^{25} + e^{16}, e^{37} + e^{15} + e^{46} + e^{28}$                                                        | 13579    |
| 96421:320  | $0, 0, 0, e^{12}, e^{13}, e^{14} + e^{23}, e^{24}, e^{25} + e^{16}, e^{36} + e^{27} + e^{18} + e^{45}$                                                         | 13579    |
| 96421:321  | $0, 0, 0, -e^{12}, -e^{13}, e^{14}, e^{24}, e^{16} + e^{25} + e^{34}, e^{15} + e^{28} + e^{37} + e^{46}$                                                       | 13579    |
| 96421:322  | $0, 0, 0, e^{12}, e^{13}, 2e^{14}, e^{24}, e^{25} + e^{34} + e^{16}, e^{36} + e^{27} + e^{18} + e^{45}$                                                        | 13579    |
| 96421:323  | $0, 0, 0, e^{12}a_2, e^{13}a_2, e^{14}(1 + a_2), e^{23} - (-1 + a_2)e^{15}, e^{25} + e^{34} + e^{16}, e^{18} + e^{45} + e^{36} + e^{27}$                       | 13579    |
| 96421:324  | $0, 0, 0, -e^{12}(1 + a_4), -e^{13}, e^{23} + e^{14}, e^{24} + (2 + a_4)e^{15}, e^{25} + e^{34} + e^{16}a_4, e^{27} + e^{18} + e^{45}$                         | 13579    |
| 96421:325a | $0, 0, 0, -e^{12}, e^{13}, e^{14} + e^{23}, e^{24} + e^{35}, e^{25} + e^{16}, e^{37} + e^{15} + e^{46} + e^{28}$                                               | 13579    |
| 96421:325b | $0, 0, 0, -e^{12}, -e^{13}, e^{14} + e^{23}, e^{35} + e^{24}, -e^{25} + e^{16}, e^{46} + e^{37} + e^{28} + e^{15}$                                             | 13579    |
| 96421:326  | $0, 0, 0, (-1 + a_2)e^{12}, a_2e^{13}, e^{14} + e^{23}, e^{24} + e^{15}, e^{25} + e^{34} + e^{16}, e^{18} + e^{36} + e^{27}$                                   | 13579    |
| 96421:327a | $0, 0, 0, -e^{12}, -2e^{13}, -e^{23} + e^{14}, a_3e^{15}, e^{16} + e^{25} + e^{34}, e^{28} + e^{17} + e^{35} + e^{46}$                                         | 13579    |
| 96421:327b | $0, 0, 0, -e^{12}, -2e^{13}, -e^{23} - e^{14}, a_3e^{15}, e^{16} + e^{25} + e^{34}, e^{28} + e^{17} + e^{35} + e^{46}$                                         | 13579    |
| 96421:328  | $0, 0, 0, -(1 + a_5 - a_3)e^{12}, (-1 + a_3)e^{13}, e^{14}a_3 + e^{23}, e^{15}(2 + a_5 - a_3), a_5e^{16} + e^{25} + e^{34}, e^{18} + e^{45} + e^{36} + e^{27}$ | 13579    |
| 96421:329a | $0, 0, 0, -e^{12}, e^{13}, e^{14} + e^{23}, 2e^{24} + e^{35}, e^{16} + e^{34}, e^{37} + e^{15} + e^{46} + e^{28}$                                              | 13579    |
| 96421:329b | $0, 0, 0, -e^{12}, -e^{13}, e^{14} + e^{23}, e^{35} + 2e^{24}, e^{34} + e^{16}, e^{28} + e^{37} + e^{46} + e^{15}$                                             | 13579    |
| 96421:330a | $0, 0, 0, -e^{12}, e^{13}, e^{14}, e^{35} + e^{24}, e^{34} - e^{25} + e^{16}, e^{46} + e^{37} + e^{28} + e^{15}$                                               | 13579    |
| 96421:330b | $0, 0, 0, -e^{12}, -e^{13}, e^{14}, e^{35} + e^{24}, e^{34} + e^{25} + e^{16}, e^{28} + e^{37} + e^{46} + e^{15}$                                              | 13579    |
| 96421:331a | $0, 0, 0, -e^{12}, -e^{13}, e^{14}, e^{25} + e^{34}, e^{16} + e^{35} + e^{24}, e^{15} + e^{28} + e^{37} + e^{46}$                                              | 13579    |

Table 2 – Continued to next page

Table 2 – Continued from previous page

| Name       | $\mathfrak{g}$                                                                                                                                                    | UCS Dim. |
|------------|-------------------------------------------------------------------------------------------------------------------------------------------------------------------|----------|
| 96421:331b | $0, 0, 0, -e^{12}, -e^{13}, e^{14}, e^{25} + e^{34}, e^{16} + e^{35} - e^{24}, e^{15} + e^{28} + e^{37} + e^{46}$                                                 | 13579    |
| 96421:332  | $0, 0, 0, e^{12}a_1, e^{13}, e^{14} + e^{23}, -(-1 + a_1)e^{15} + e^{24}, e^{25} + e^{16}, e^{18} + e^{45} + e^{36} + e^{27}$                                     | 13579    |
| 96421:333  | $0, 0, 0, -e^{12}, e^{13}a_2, e^{14}(1 + a_2) + e^{23}, e^{15} + e^{24}, e^{16} + e^{34}, e^{45} + e^{18} + e^{27} + e^{36}$                                      | 13579    |
| 96421:334  | $0, 0, 0, (-1 + a_3)e^{12}, (-1 + a_3)e^{13}, e^{14}a_3, -(-2 + a_3)e^{15} + e^{24}, e^{25} + e^{34} + e^{16}, e^{18} + e^{45} + e^{36} + e^{27}$                 | 13579    |
| 96421:335  | $0, 0, 0, -e^{12}, e^{13}(-2 + a_4), e^{14} + (-1 + a_4)e^{23}, e^{24}a_4, e^{25} + e^{16} + e^{34}, e^{37} + e^{15} + e^{46} + e^{28}$                           | 13579    |
| 96421:336  | $0, 0, 0, e^{12}, (-1 + a_3)e^{13}, e^{23} + e^{14}a_3, e^{24}, e^{16}(-2 + a_3) + e^{25} + e^{34}, e^{18} + e^{45} + e^{36} + e^{27}$                            | 13579    |
| 96421:337a | $0, 0, 0, -e^{12}, e^{13}, (-1 + a_3)e^{23} + e^{14}, e^{24}a_3 + e^{35}, (-2 + a_3)e^{25} + e^{16} + e^{34}, e^{37} + e^{15} + e^{46} + e^{28}$                  | 13579    |
| 96421:337b | $0, 0, 0, -e^{12}, -e^{13}, (-1 + a_3)e^{23} + e^{14}, e^{24}a_3 + e^{35}, -(-2 + a_3)e^{25} + e^{16} + e^{34}, e^{37} + e^{15} + e^{46} + e^{28}$                | 13579    |
| 96421:338  | $0, 0, 0, (1 - a_4)e^{12}, e^{13}(-1 + a_3), a_3e^{14} + e^{23}, e^{24} + e^{15}a_4, (-2 + a_3 + a_4)e^{16} + e^{25} + e^{34}, e^{18} + e^{45} + e^{36} + e^{27}$ | 13579    |
| 96421:339  | $0, 0, 0, e^{12}, e^{13}, e^{14}, e^{24}, e^{26} + e^{17}, e^{18} + e^{46}$                                                                                       | 24679    |
| 96421:340a | $0, 0, 0, -e^{12}, e^{13}, e^{14}, e^{24}, e^{27} + e^{16}, e^{28} + e^{46}$                                                                                      | 24679    |
| 96421:340b | $0, 0, 0, -e^{12}, e^{13}, -e^{14}, e^{24}, e^{27} + e^{16}, e^{46} + e^{28}$                                                                                     | 24679    |
| 96421:341a | $0, 0, 0, e^{12}, e^{13}, e^{24}, e^{14}, e^{26} + e^{17}, e^{18} + e^{46}$                                                                                       | 24679    |
| 96421:341b | $0, 0, 0, e^{12}, e^{13}, e^{24}, -e^{14}, e^{26} + e^{17}, e^{46} + e^{18}$                                                                                      | 24679    |
| 96421:342  | $0, 0, 0, -e^{12}, e^{13}, e^{24}, e^{14}, e^{27} + e^{16}, e^{28} + e^{46}$                                                                                      | 24679    |
| 96421:343a | $0, 0, 0, e^{12}, e^{13}, e^{14}, e^{24}, e^{26} + e^{17}, e^{18} + e^{46} + e^{35}$                                                                              | 13679    |
| 96421:343b | $0, 0, 0, e^{12}, -e^{13}, e^{14}, e^{24}, e^{17} + e^{26}, e^{18} + e^{35} + e^{46}$                                                                             | 13679    |
| 96421:344a | $0, 0, 0, -e^{12}, e^{13}, e^{14}, e^{24}, e^{27} + e^{16}, e^{28} + e^{46} + e^{35}$                                                                             | 13679    |
| 96421:344b | $0, 0, 0, -e^{12}, e^{13}, -e^{14}, e^{24}, e^{27} + e^{16}, e^{28} + e^{35} + e^{46}$                                                                            | 13679    |
| 96421:344c | $0, 0, 0, -e^{12}, -e^{13}, e^{14}, e^{24}, e^{27} + e^{16}, e^{46} + e^{35} + e^{28}$                                                                            | 13679    |
| 96421:344d | $0, 0, 0, -e^{12}, -e^{13}, -e^{14}, e^{24}, e^{27} + e^{16}, e^{35} + e^{46} + e^{28}$                                                                           | 13679    |
| 96421:345a | $0, 0, 0, e^{12}, e^{13}, e^{24}, e^{14}, e^{26} + e^{17}, e^{18} + e^{46} + e^{35}$                                                                              | 13679    |
| 96421:345b | $0, 0, 0, e^{12}, e^{13}, e^{24}, -e^{14}, e^{17} + e^{26}, e^{18} + e^{46} + e^{35}$                                                                             | 13679    |
| 96421:346  | $0, 0, 0, -e^{12}, e^{13}, e^{24}, e^{14}, e^{27} + e^{16}, e^{28} + e^{46} + e^{35}$                                                                             | 13679    |
| 96421:347  | $0, 0, 0, e^{12}, e^{13}, e^{14}, e^{24}, e^{26} + e^{17}, e^{23} + e^{18} + e^{46}$                                                                              | 24679    |
| 96421:348a | $0, 0, 0, e^{12}, e^{13}, e^{24}, e^{14}, e^{17} + e^{26}, e^{18} + e^{23} + e^{46}$                                                                              | 24679    |
| 96421:348b | $0, 0, 0, e^{12}, e^{13}, e^{24}, -e^{14}, e^{26} + e^{17}, e^{46} + e^{23} + e^{18}$                                                                             | 24679    |
| 96421:349a | $0, 0, 0, -e^{12}, e^{13}, e^{14}, e^{24}, e^{16} + e^{27}, e^{15} + e^{46} + e^{28}$                                                                             | 13679    |
| 96421:349b | $0, 0, 0, -e^{12}, e^{13}, -e^{14}, e^{24}, e^{27} + e^{16}, e^{15} + e^{28} + e^{46}$                                                                            | 13679    |
| 96421:350  | $0, 0, 0, -e^{12}, e^{13}, e^{24}, e^{14}, e^{27} + e^{16}, e^{46} + e^{28} + e^{15}$                                                                             | 13679    |
| 96421:351  | $0, 0, 0, -e^{12}, e^{13}, e^{14}, e^{24}, e^{17} + e^{26}, e^{28} + e^{47} + e^{16}$                                                                             | 24679    |
| 96421:352  | $0, 0, 0, e^{12}, e^{13}, e^{14}, e^{24}, e^{17} + e^{26}, e^{46} + e^{18} + e^{27}$                                                                              | 24679    |
| 96421:353  | $0, 0, 0, -e^{12}, e^{13}, e^{24}, e^{14} + e^{23}, e^{16} + e^{27}, e^{46} + e^{28}$                                                                             | 23579    |
| 96421:354  | $0, 0, 0, -e^{12}, e^{13}, e^{14}, e^{24}, e^{17} + e^{26}, e^{28} + e^{16} + e^{35} + e^{47}$                                                                    | 13679    |
| 96421:355a | $0, 0, 0, e^{12}, e^{13}, e^{14}, e^{24}, e^{26} + e^{17}, e^{27} + e^{35} + e^{18} + e^{46}$                                                                     | 13679    |
| 96421:355b | $0, 0, 0, e^{12}, -e^{13}, e^{14}, e^{24}, e^{17} + e^{26}, e^{18} + e^{27} + e^{35} + e^{46}$                                                                    | 13679    |
| 96421:356  | $0, 0, 0, -e^{12}, e^{13}, e^{24}, e^{14} + e^{23}, e^{16} + e^{27}, e^{46} + e^{35} + e^{28}$                                                                    | 13579    |
| 96421:358  | $0, 0, 0, -e^{12}, e^{13}, e^{24}, e^{14} + e^{23}, e^{27} + e^{16}, e^{28} + e^{15} + e^{46}$                                                                    | 13579    |
| 96421:359  | $0, 0, 0, e^{12}, e^{13}, e^{24}, e^{14} + e^{23}, e^{27} + e^{16}, e^{18} + e^{47} + e^{36}$                                                                     | 23579    |
| 96421:362a | $0, 0, 0, e^{12}, e^{13}, e^{24}, e^{14} + e^{23}, -e^{17} + e^{26} + e^{34}, e^{46} + e^{37} + e^{18}$                                                           | 23579    |
| 96421:362b | $0, 0, 0, e^{12}, e^{13}, -e^{24}, e^{14} + e^{23}, -e^{17} + e^{26} + e^{34}, e^{37} + e^{18} + e^{46}$                                                          | 23579    |
| 96421:363a | $0, 0, 0, -e^{12}, e^{13}, 2e^{24}, e^{14} + e^{23}, e^{26} + e^{17} + e^{34}, e^{47} + e^{28} + e^{36}$                                                          | 23579    |
| 96421:363b | $0, 0, 0, -e^{12}, e^{13}, 2e^{24}, -e^{14} + e^{23}, e^{17} + e^{34} + e^{26}, e^{28} + e^{47} + e^{36}$                                                         | 23579    |
| 96421:364a | $0, 0, 0, -e^{12}, e^{13}, 2e^{24}, e^{14} + e^{23}, e^{26} + e^{17} + e^{34}, e^{15} + e^{47} + e^{28} + e^{36}$                                                 | 13579    |
| 96421:364b | $0, 0, 0, -e^{12}, e^{13}, 2e^{24}, -e^{14} + e^{23}, e^{17} + e^{34} + e^{26}, e^{28} + e^{47} + e^{36} + e^{15}$                                                | 13579    |
| 96421:414  | $0, 0, 0, e^{12}, e^{13}, e^{24}, e^{15}, e^{26} + e^{17}, e^{18} + e^{46}$                                                                                       | 12469    |
| 96421:415  | $0, 0, 0, e^{12}, e^{13}, e^{14}, e^{24} + e^{15}, e^{17} + e^{26}, e^{18} + e^{46}$                                                                              | 12469    |
| 96421:416  | $0, 0, 0, e^{12}, e^{13}, e^{24}, e^{15}, e^{26} + e^{17}, e^{46} + e^{23} + e^{18}$                                                                              | 12469    |
| 96421:417  | $0, 0, 0, e^{12}, e^{13}, e^{24}, e^{15}, e^{26} + e^{17}, e^{35} + e^{18} + e^{46}$                                                                              | 12469    |
| 96421:418  | $0, 0, 0, e^{12}, e^{13}, e^{24}, e^{35}, e^{26} + e^{37}, e^{46} + e^{57} + e^{18}$                                                                              | 12469    |
| 96421:421  | $0, 0, 0, e^{12}, -e^{13}, e^{25} - e^{34}, -2e^{14}, e^{16} + e^{37} + e^{45}, e^{38} + e^{56}$                                                                  | 12469    |
| 96421:422  | $0, 0, 0, e^{12}, e^{13}, e^{14}, e^{15} + e^{24}, e^{17} + e^{26}, e^{46} + e^{18} + e^{23}$                                                                     | 12469    |
| 96421:423a | $0, 0, 0, e^{12}, e^{13}, e^{14}, e^{15} + e^{24}, e^{17} + e^{26}, e^{18} + e^{46} + e^{35}$                                                                     | 12469    |
| 96421:423b | $0, 0, 0, e^{12}, -e^{13}, e^{14}, e^{15} + e^{24}, e^{17} + e^{26}, e^{46} + e^{35} + e^{18}$                                                                    | 12469    |
| 96421:424  | $0, 0, 0, e^{12}, e^{13}, e^{14}, e^{35}, e^{37} + e^{16} + e^{24}, e^{26} + e^{57} + e^{18}$                                                                     | 12469    |
| 96421:425  | $0, 0, 0, e^{12}, e^{13}, e^{24}, e^{35}, e^{14} + e^{26} + e^{37}, e^{18} + e^{57} + e^{46}$                                                                     | 12469    |
| 96421:426  | $0, 0, 0, e^{12}, e^{13}, e^{24}, e^{34} + e^{25}, e^{27} + e^{36}, e^{18} + e^{47} + e^{56}$                                                                     | 12469    |

Table 2 – Continued to next page

Table 2 – Continued from previous page

| Name       | $\mathfrak{g}$                                                                                                            | UCS Dim. |
|------------|---------------------------------------------------------------------------------------------------------------------------|----------|
| 96421:428  | $0, 0, 0, e^{12}, e^{13}, e^{24}, e^{35}, e^{26} + e^{37}, e^{57} + e^{18} + e^{46} + e^{23}$                             | 12469    |
| 96421:429  | $0, 0, 0, e^{12}, -e^{13}, e^{25} - e^{34}, -2e^{14} + e^{23}, e^{16} + e^{37} + e^{45}, e^{38} + e^{56}$                 | 12469    |
| 96421:431  | $0, 0, 0, -e^{12}, -e^{13}, e^{34} + e^{25}, 2e^{15} + e^{24}, e^{27} + e^{45} + e^{16}, e^{28} + e^{46}$                 | 12469    |
| 96421:436  | $0, 0, 0, e^{12}, -e^{13}, e^{25} - e^{34}, -2e^{14}, e^{16} + e^{37} + e^{45}, e^{38} + e^{24} + e^{56}$                 | 12469    |
| 96421:437  | $0, 0, 0, e^{12}, -e^{13}, -2e^{14}, e^{25} - e^{34}, e^{17} + e^{36} + e^{45}, e^{16} + e^{38} + e^{57}$                 | 12469    |
| 96421:438  | $0, 0, 0, e^{12}, e^{13}, e^{24}, e^{34} + e^{25}, e^{27} + e^{36} + e^{14}, e^{47} + e^{56} + e^{18}$                    | 12469    |
| 96421:439  | $0, 0, 0, e^{12}, e^{13}, e^{24}, e^{34} + e^{25}, e^{27} + e^{36} + e^{15}, e^{47} + e^{56} + e^{18}$                    | 12469    |
| 96421:440a | $0, 0, 0, e^{12}, e^{13}, e^{34} + e^{25}, e^{35} + e^{24}, e^{26} + e^{37}, e^{46} + e^{57} + e^{18}$                    | 12469    |
| 96421:440b | $0, 0, 0, e^{12}, e^{13}, -e^{34} - e^{25}, e^{35} - e^{24}, e^{26} + e^{37}, e^{18} + e^{46} + e^{57}$                   | 12469    |
| 96421:442  | $0, 0, 0, e^{12}, e^{13}, e^{24}, e^{35}, e^{26} + e^{37} + e^{14}, e^{46} + e^{23} + e^{57} + e^{18}$                    | 12469    |
| 96421:443  | $0, 0, 0, e^{12}, e^{13}, e^{24}, e^{34} + e^{25}, e^{27} + e^{36}, e^{47} + e^{56} + e^{18} + e^{23}$                    | 12469    |
| 96421:446  | $0, 0, 0, e^{12}, -e^{13}, -e^{34} + e^{25}, e^{23} - 2e^{14}, e^{16} + e^{37} + e^{45}, e^{38} + e^{56} + e^{24}$        | 12469    |
| 96421:447  | $0, 0, 0, e^{12}, e^{13}, e^{14} + e^{23}, e^{15} + e^{24}, e^{17} + e^{26} + e^{35}, e^{46} + e^{37} + e^{18}$           | 12469    |
| 96421:449a | $0, 0, 0, -e^{12}, -e^{13}, e^{25} + e^{34}, e^{24} + 2e^{15}, e^{45} + e^{27} + e^{16}, e^{35} + e^{46} + e^{28}$        | 12469    |
| 96421:449b | $0, 0, 0, -e^{12}, -e^{13}, e^{25} + e^{34}, -e^{24} + 2e^{15}, e^{45} + e^{27} + e^{16}, e^{35} + e^{46} + e^{28}$       | 12469    |
| 96421:451a | $0, 0, 0, e^{12}, e^{13}, e^{25} + e^{34}, e^{24} + e^{35}, e^{14} + e^{37} + e^{26}, e^{18} + e^{57} + e^{46}$           | 12469    |
| 96421:451b | $0, 0, 0, e^{12}, e^{13}, -e^{25} - e^{34}, -e^{24} + e^{35}, e^{37} + e^{26} + e^{14}, e^{18} + e^{57} + e^{46}$         | 12469    |
| 96421:452a | $0, 0, 0, e^{12}, e^{13}, e^{25} + e^{34}, e^{24} + e^{35}, e^{14} + e^{36} + e^{27}, e^{56} + e^{47} + e^{18}$           | 12469    |
| 96421:452b | $0, 0, 0, e^{12}, e^{13}, e^{25} + e^{34}, -e^{24} + e^{35}, e^{14} + e^{36} + e^{27}, e^{56} + e^{47} + e^{18}$          | 12469    |
| 96421:454  | $0, 0, 0, e^{12}, e^{13}, e^{24}, e^{34} + e^{25}, e^{27} + e^{36} + e^{14}, e^{23} + e^{47} + e^{56} + e^{18}$           | 12469    |
| 96421:455  | $0, 0, 0, e^{12}, e^{13}, e^{24}, e^{34} + e^{25}, e^{15} + e^{27} + e^{36}, e^{18} + e^{23} + e^{47} + e^{56}$           | 12469    |
| 96421:456a | $0, 0, 0, e^{12}, e^{13}, e^{34} + e^{25}, e^{35} + e^{24}, e^{26} + e^{37}, e^{46} + e^{23} + e^{57} + e^{18}$           | 12469    |
| 96421:456b | $0, 0, 0, e^{12}, e^{13}, -e^{34} - e^{25}, e^{35} - e^{24}, e^{26} + e^{37}, e^{46} + e^{57} + e^{18} + e^{23}$          | 12469    |
| 96421:458  | $0, 0, 0, e^{12}, -e^{13}, -2e^{14}, e^{25} - e^{34}, e^{17} + e^{36} + e^{45}, e^{16} + e^{38} + e^{24} + e^{57}$        | 12469    |
| 96421:460a | $0, 0, 0, e^{12}, e^{13}, e^{34} + e^{25}, e^{35} + e^{24}, e^{26} + e^{37} + e^{14}, e^{46} + e^{23} + e^{57} + e^{18}$  | 12469    |
| 96421:460b | $0, 0, 0, e^{12}, e^{13}, -e^{34} - e^{25}, e^{35} - e^{24}, e^{14} + e^{26} + e^{37}, e^{46} + e^{57} + e^{18} + e^{23}$ | 12469    |
| 96421:461a | $0, 0, 0, e^{12}, e^{13}, e^{34} + e^{25}, e^{35} + e^{24}, e^{27} + e^{36} + e^{14}, e^{23} + e^{47} + e^{56} + e^{18}$  | 12469    |
| 96421:461b | $0, 0, 0, e^{12}, e^{13}, e^{34} + e^{25}, e^{35} - e^{24}, e^{14} + e^{27} + e^{36}, e^{18} + e^{23} + e^{47} + e^{56}$  | 12469    |
| Type: 3222 |                                                                                                                           |          |
| 9642:1     | $0, 0, 0, e^{12}, e^{13}, e^{14}, e^{24}, e^{16}, e^{27}$                                                                 | 3679     |
| 9642:2     | $0, 0, 0, e^{12}, e^{13}, e^{24}, e^{14}, e^{26}, e^{23} + e^{17}$                                                        | 3679     |
| 9642:3     | $0, 0, 0, e^{12}, e^{13}, e^{14}, e^{24}, e^{16}, e^{26} + e^{17}$                                                        | 3679     |
| 9642:4     | $0, 0, 0, e^{12}, e^{13}, e^{24}, e^{14}, e^{26}, e^{16} + e^{27}$                                                        | 3679     |
| 9642:5     | $0, 0, 0, e^{12}, e^{13}, e^{14}, e^{24}, e^{16}, e^{35} + e^{27}$                                                        | 2579     |
| 9642:6     | $0, 0, 0, e^{12}, e^{13}, e^{24}, e^{14}, e^{26}, e^{35} + e^{17}$                                                        | 2579     |
| 9642:7     | $0, 0, 0, e^{12}, e^{13}, e^{14}, e^{24}, e^{16}, e^{27} + e^{15}$                                                        | 2579     |
| 9642:8     | $0, 0, 0, e^{12}, e^{13}, e^{14}, e^{24}, e^{23} + e^{16}, e^{26} + e^{17}$                                               | 3679     |
| 9642:9     | $0, 0, 0, -e^{12}, e^{13}, e^{24}, e^{14} + e^{23}, e^{26}, e^{17} + e^{34}$                                              | 3579     |
| 9642:10    | $0, 0, 0, e^{12}, e^{13}, e^{14}, e^{24}, e^{23} + e^{16}, e^{27} + e^{35}$                                               | 2579     |
| 9642:11a   | $0, 0, 0, e^{12}, e^{13}, e^{14}, e^{24}, e^{26} + e^{17}, e^{27} + e^{16}$                                               | 3679     |
| 9642:11b   | $0, 0, 0, e^{12}, e^{13}, -e^{14}, e^{24}, -e^{17} + e^{26}, e^{27} + e^{16}$                                             | 3679     |
| 9642:12    | $0, 0, 0, e^{12}, e^{13}, e^{24}, e^{14} + e^{23}, e^{26}, e^{17} + e^{25}$                                               | 2579     |
| 9642:13    | $0, 0, 0, e^{12}, e^{13}, e^{24}, e^{14}, e^{15} + e^{26}, e^{17} + e^{35}$                                               | 2579     |
| 9642:14    | $0, 0, 0, e^{12}, e^{13}, e^{24}, e^{14} + e^{23}, e^{26}, e^{27} + e^{16}$                                               | 3579     |
| 9642:15    | $0, 0, 0, e^{12}, e^{13}, e^{14}, e^{24}, e^{23} + e^{16}, e^{15} + e^{27}$                                               | 2579     |
| 9642:16    | $0, 0, 0, e^{12}, e^{13}, e^{24}, e^{14}, e^{26}, e^{25} + e^{34} + e^{17}$                                               | 2579     |
| 9642:17    | $0, 0, 0, e^{12}, e^{13}, e^{14}, e^{24}, e^{16}, e^{17} + e^{26} + e^{35}$                                               | 2579     |
| 9642:18    | $0, 0, 0, e^{12}, e^{13}, e^{24}, e^{14}, e^{26}, e^{16} + e^{27} + e^{35}$                                               | 2579     |
| 9642:19    | $0, 0, 0, e^{12}, e^{13}, e^{14}, e^{24}, e^{16} + e^{35}, e^{17} + e^{26}$                                               | 2579     |
| 9642:20    | $0, 0, 0, e^{12}, e^{13}, e^{24}, e^{14}, e^{26} + e^{35}, e^{27} + e^{16}$                                               | 2579     |
| 9642:21    | $0, 0, 0, e^{12}, e^{13}, e^{24}, e^{14} + e^{23}, e^{26} + e^{35}, e^{17} + e^{25}$                                      | 2579     |
| 9642:22    | $0, 0, 0, -e^{12}, e^{13}, e^{14} + e^{23}, e^{24}, e^{16} + e^{34}, e^{27} + e^{35}$                                     | 2579     |
| 9642:23    | $0, 0, 0, e^{12}, e^{13}, e^{24}, e^{14}, e^{15} + e^{26}, e^{16} + e^{27}$                                               | 2579     |
| 9642:24    | $0, 0, 0, e^{12}, e^{13}, e^{24}, e^{14} + e^{23}, e^{26} + e^{15}, e^{25} + e^{17}$                                      | 2579     |
| 9642:25    | $0, 0, 0, e^{12}a_1, e^{13}(1 + a_1), e^{24}, e^{23} + e^{14}, e^{26}, e^{17} + e^{34} + e^{25}$                          | 2579     |
| 9642:26    | $0, 0, 0, -e^{12}, e^{13}, e^{23} + e^{14}, e^{24}, e^{16} + e^{34}, e^{15} + e^{27}$                                     | 2579     |
| 9642:27    | $0, 0, 0, e^{12}, e^{13}, e^{24}, e^{14}, e^{26} + e^{35}, e^{25} + e^{34} + e^{17}$                                      | 2579     |
| 9642:28    | $0, 0, 0, e^{12}, e^{13}, e^{24}, e^{14} + e^{23}, e^{26}, e^{27} + e^{35} + e^{16}$                                      | 2579     |

Table 2 – Continued to next page

Table 2 – Continued from previous page

| Name     | $\mathfrak{g}$                                                                                                     | UCS Dim. |
|----------|--------------------------------------------------------------------------------------------------------------------|----------|
| 9642:29  | $0, 0, 0, e^{12}, e^{13}, e^{24}, e^{14} + e^{23}, e^{26} + e^{35}, e^{16} + e^{27}$                               | 2579     |
| 9642:30  | $0, 0, 0, -e^{12}, e^{13}, e^{23} + e^{14}, e^{24}, e^{16} + e^{34}, e^{17} + e^{26}$                              | 3579     |
| 9642:31  | $0, 0, 0, e^{12}, e^{13}, e^{14}, e^{24}, e^{16} + e^{23}, e^{17} + e^{26} + e^{35}$                               | 2579     |
| 9642:32  | $0, 0, 0, e^{12}, e^{13}, e^{24}, e^{14}, e^{15} + e^{26}, e^{17} + e^{25} + e^{34}$                               | 2579     |
| 9642:33  | $0, 0, 0, e^{12}, e^{13}, e^{24}, e^{14} + e^{23}, e^{15} + e^{26}, e^{16} + e^{27}$                               | 2579     |
| 9642:34  | $0, 0, 0, e^{12}, e^{13}, e^{24}, e^{14}, e^{26} + e^{15}, e^{27} + e^{35} + e^{16}$                               | 2579     |
| 9642:35  | $0, 0, 0, e^{12}, e^{13}, e^{14} + e^{23}, e^{24}, e^{16} + e^{25}, e^{26} + e^{17}$                               | 2579     |
| 9642:36  | $0, 0, 0, e^{12}a_1, e^{13}(1 + a_1), e^{24}, e^{14} + e^{23}, e^{35} + e^{26}, e^{17} + e^{34} + e^{25}$          | 2579     |
| 9642:37  | $0, 0, 0, e^{12}, e^{13}, e^{14}, e^{24}, e^{16} + e^{34} + e^{25}, e^{17} + e^{26}$                               | 2579     |
| 9642:38a | $0, 0, 0, e^{12}, e^{13}, e^{14}, e^{24}, e^{27} + e^{16}, e^{35} + e^{26} + e^{17}$                               | 2579     |
| 9642:38b | $0, 0, 0, e^{12}, e^{13}, e^{14}, e^{24}, e^{27} - e^{16}, e^{26} + e^{35} + e^{17}$                               | 2579     |
| 9642:39a | $0, 0, 0, e^{12}, e^{13}, e^{14}, e^{24}, e^{26} + e^{17}, e^{27} + e^{35} + e^{16}$                               | 2579     |
| 9642:39b | $0, 0, 0, e^{12}, e^{13}, -e^{14}, e^{24}, -e^{17} + e^{26}, e^{35} + e^{27} + e^{16}$                             | 2579     |
| 9642:40  | $0, 0, 0, e^{12}a_1, e^{13}(1 + a_1), e^{24}, e^{23} + e^{14}, e^{26} + e^{15}, e^{34} + e^{25} + e^{17}$          | 2579     |
| 9642:41  | $0, 0, 0, e^{12}, e^{13}, e^{24}, e^{23} + e^{14}, e^{26} + e^{15}, e^{16} + e^{27} + e^{35}$                      | 2579     |
| 9642:42  | $0, 0, 0, e^{12}, e^{13}, e^{14} + e^{23}, e^{24}, e^{16} + e^{25}, e^{17} + e^{26} + e^{35}$                      | 2579     |
| 9642:43  | $0, 0, 0, -e^{12}, e^{13}, e^{14} + e^{23}, e^{24}, e^{34} + e^{16}, e^{17} + e^{35} + e^{26}$                     | 2579     |
| 9642:44  | $0, 0, 0, e^{12}, e^{13}, e^{14}, e^{24}, e^{16} + e^{25} + e^{34}, e^{17} + e^{26} + e^{35}$                      | 2579     |
| 9642:45  | $0, 0, 0, (-1 + a_2)e^{12}, a_2e^{13}, e^{14} + e^{23}, e^{24}, e^{25} + e^{34} + e^{16}, e^{26} + e^{17}$         | 2579     |
| 9642:46a | $0, 0, 0, -e^{12}, e^{13}, e^{24}, e^{14} + e^{23}, e^{27} + e^{16}, e^{17} + e^{34} + e^{26}$                     | 3579     |
| 9642:46b | $0, 0, 0, -e^{12}, e^{13}, e^{24}, e^{23} - e^{14}, e^{27} - e^{16}, e^{17} + e^{26} + e^{34}$                     | 3579     |
| 9642:47  | $0, 0, 0, e^{12}a_1, e^{13}(1 + a_1), e^{14} + e^{23}, e^{24}, e^{25} + e^{34} + e^{16}, e^{26} + e^{35} + e^{17}$ | 2579     |
| 9642:48a | $0, 0, 0, e^{12}, e^{13}, e^{24}, e^{14} + e^{23}, e^{26} + e^{34} - e^{17}, e^{27} + e^{35} + e^{16}$             | 2579     |
| 9642:48b | $0, 0, 0, -e^{12}, e^{13}, e^{24}, e^{14} + e^{23}, e^{17} + e^{26} + e^{34}, e^{16} + e^{27} + e^{35}$            | 2579     |
| 9642:49  | $0, 0, 0, e^{12}, e^{13}, e^{14}, e^{15}, e^{16}, e^{17}$                                                          | 2469     |
| 9642:50  | $0, 0, 0, e^{12}, e^{13}, e^{24}, e^{15}, e^{26}, e^{17}$                                                          | 2469     |
| 9642:51  | $0, 0, 0, e^{12}, e^{13}, e^{24}, e^{35}, e^{26}, e^{37}$                                                          | 2469     |
| 9642:52  | $0, 0, 0, e^{12}, e^{13}, e^{14}, e^{15}, e^{16}, e^{17} + e^{23}$                                                 | 2469     |
| 9642:53  | $0, 0, 0, e^{12}, e^{13}, e^{24}, e^{15}, e^{26}, e^{17} + e^{23}$                                                 | 2469     |
| 9642:54  | $0, 0, 0, e^{12}, e^{13}, e^{14}, e^{15}, e^{16}, e^{17} + e^{24}$                                                 | 2469     |
| 9642:55  | $0, 0, 0, e^{12}, e^{13}, e^{14}, e^{35}, e^{16}, e^{24} + e^{37}$                                                 | 2469     |
| 9642:56  | $0, 0, 0, e^{12}, e^{13}, e^{24}, e^{35}, e^{26}, e^{37} + e^{14}$                                                 | 2469     |
| 9642:57  | $0, 0, 0, e^{12}, e^{13}, e^{14}, e^{15}, e^{24} + e^{16}, e^{17}$                                                 | 2469     |
| 9642:58  | $0, 0, 0, e^{12}, e^{13}, e^{24}, e^{15}, e^{14} + e^{26}, e^{17}$                                                 | 2469     |
| 9642:59  | $0, 0, 0, e^{12}, e^{13}, e^{14}, e^{35}, e^{16} + e^{24}, e^{37}$                                                 | 2469     |
| 9642:60  | $0, 0, 0, e^{12}, e^{13}, e^{24}, e^{35}, e^{26} + e^{14}, e^{37}$                                                 | 2469     |
| 9642:61  | $0, 0, 0, -e^{12}, e^{13}, e^{14}, e^{15} + e^{23}, e^{16}, e^{34} + e^{17}$                                       | 2469     |
| 9642:62  | $0, 0, 0, -e^{12}, e^{13}, e^{24}, e^{23} + e^{15}, e^{26}, e^{17} + e^{34}$                                       | 2469     |
| 9642:63  | $0, 0, 0, -e^{12}, e^{13}, e^{14} + e^{23}, e^{15}, e^{16} + e^{34}, e^{17}$                                       | 2469     |
| 9642:64  | $0, 0, 0, -e^{12}, e^{13}, e^{23} + e^{14}, e^{35}, e^{16} + e^{34}, e^{37}$                                       | 2469     |
| 9642:65  | $0, 0, 0, e^{12}, e^{13}, e^{14}, e^{15} + e^{24}, e^{16}, e^{17} + e^{26}$                                        | 2469     |
| 9642:66  | $0, 0, 0, e^{12}, e^{13}, e^{24}, e^{34} + e^{25}, e^{26}, e^{27} + e^{36}$                                        | 2469     |
| 9642:69  | $0, 0, 0, e^{12}, e^{13}, e^{14}, e^{15}, e^{16} + e^{23}, e^{17} + e^{24}$                                        | 2469     |
| 9642:70  | $0, 0, 0, e^{12}, e^{13}, e^{14}, e^{35}, e^{16} + e^{23}, e^{37} + e^{24}$                                        | 2469     |
| 9642:71  | $0, 0, 0, e^{12}, e^{13}, e^{14}, e^{15}, e^{16} + e^{24}, e^{17} + e^{23}$                                        | 2469     |
| 9642:72  | $0, 0, 0, e^{12}, e^{13}, e^{24}, e^{15}, e^{14} + e^{26}, e^{17} + e^{23}$                                        | 2469     |
| 9642:73a | $0, 0, 0, e^{12}, e^{13}, e^{14}, e^{15}, e^{16}, e^{17} + e^{35} + e^{24}$                                        | 2469     |
| 9642:73b | $0, 0, 0, -e^{12}, e^{13}, e^{14}, e^{15}, e^{16}, e^{35} + e^{24} + e^{17}$                                       | 2469     |
| 9642:74  | $0, 0, 0, e^{12}, e^{13}, e^{14}, e^{15}, e^{16}, e^{25} + e^{34} + e^{17}$                                        | 2469     |
| 9642:75  | $0, 0, 0, e^{12}, e^{13}, e^{24}, e^{15}, e^{26}, e^{34} + e^{17} + e^{25}$                                        | 2469     |
| 9642:76  | $0, 0, 0, e^{12}, e^{13}, e^{14}, e^{35}, e^{16}, e^{15} + e^{24} + e^{37}$                                        | 2469     |
| 9642:77  | $0, 0, 0, e^{12}, e^{13}, e^{14}, e^{15}, e^{16} + e^{24}, e^{17} + e^{35}$                                        | 2469     |
| 9642:78  | $0, 0, 0, e^{12}, e^{13}, e^{24}, e^{15}, e^{26} + e^{14}, e^{35} + e^{17}$                                        | 2469     |
| 9642:79a | $0, 0, 0, e^{12}, e^{13}, e^{24}, e^{35}, e^{14} + e^{26}, e^{37} + e^{15}$                                        | 2469     |
| 9642:79b | $0, 0, 0, e^{12}, e^{13}, e^{24}, e^{35}, e^{26} - e^{14}, e^{37} + e^{15}$                                        | 2469     |
| 9642:80  | $0, 0, 0, e^{12}, e^{13}, e^{14}, e^{15}, e^{16} + e^{35}, e^{24} + e^{17}$                                        | 2469     |
| 9642:81a | $0, 0, 0, e^{12}, e^{13}, e^{24}, e^{35}, e^{26} + e^{15}, e^{37} + e^{14}$                                        | 2469     |
| 9642:81b | $0, 0, 0, e^{12}, e^{13}, e^{24}, e^{35}, -e^{15} + e^{26}, e^{37} + e^{14}$                                       | 2469     |

Table 2 – Continued to next page

Table 2 – Continued from previous page

| Name      | $\mathfrak{g}$                                                                                                | UCS Dim. |
|-----------|---------------------------------------------------------------------------------------------------------------|----------|
| 9642:82   | $0, 0, 0, -e^{12}, e^{13}, e^{14}, e^{15}, e^{16}, e^{45} + e^{36} + e^{27}$                                  | 2469     |
| 9642:83a  | $0, 0, 0, e^{12}, e^{13}, e^{14}, e^{24} + e^{15}, e^{16} + e^{23}, e^{26} + e^{17}$                          | 2469     |
| 9642:83b  | $0, 0, 0, e^{12}, -e^{13}, e^{14}, e^{15} + e^{24}, e^{23} + e^{16}, e^{26} + e^{17}$                         | 2469     |
| 9642:84   | $0, 0, 0, (-1 + a_2)e^{12}, a_2e^{13}, e^{14}, e^{15} + e^{23}, e^{16}, e^{17} + e^{25} + e^{34}$             | 2469     |
| 9642:85   | $0, 0, 0, e^{12}a_1, (1 + a_1)e^{13}, e^{24}, e^{15} + e^{23}, e^{26}, e^{25} + e^{34} + e^{17}$              | 2469     |
| 9642:86   | $0, 0, 0, -e^{12}, a_2e^{13}, e^{14}, e^{15} + e^{23}, e^{16} + e^{24}, e^{17} + e^{34}$                      | 2469     |
| 9642:87   | $0, 0, 0, -e^{12}, e^{13}, e^{24}, e^{15} + e^{23}, e^{14} + e^{26}, e^{17} + e^{34}$                         | 2469     |
| 9642:88a  | $0, 0, 0, -e^{12}, e^{13}, e^{23} + e^{14}, e^{15}, e^{16} + e^{34}, e^{17} + e^{24}$                         | 2469     |
| 9642:88b  | $0, 0, 0, -e^{12}, -e^{13}, e^{14} + e^{23}, e^{15}, e^{34} + e^{16}, e^{17} + e^{24}$                        | 2469     |
| 9642:89a  | $0, 0, 0, -e^{12}, e^{13}, e^{23} + e^{14}, e^{35}, e^{16} + e^{34}, e^{24} + e^{37}$                         | 2469     |
| 9642:89b  | $0, 0, 0, -e^{12}, -e^{13}, e^{14} + e^{23}, e^{35}, e^{16} + e^{34}, e^{37} + e^{24}$                        | 2469     |
| 9642:90   | $0, 0, 0, e^{12}, e^{13}, a_2e^{14}, e^{23} + e^{15}, e^{16} + e^{24}, e^{17} + e^{25}$                       | 2469     |
| 9642:91   | $0, 0, 0, e^{12}, e^{13}, e^{24}, e^{23} + e^{15}, e^{26} + e^{14}, e^{25} + e^{17}$                          | 2469     |
| 9642:92a  | $0, 0, 0, -e^{12}, e^{13}, e^{14}, e^{15} + e^{23}, e^{35} + e^{16}, e^{17} + e^{34}$                         | 2469     |
| 9642:92b  | $0, 0, 0, -e^{12}, e^{13}, -e^{14}, e^{15} + e^{23}, e^{16} + e^{35}, e^{17} + e^{34}$                        | 2469     |
| 9642:93a  | $0, 0, 0, -e^{12}, e^{13}, e^{24}, e^{15} + e^{23}, e^{35} + e^{26}, e^{34} + e^{17}$                         | 2469     |
| 9642:93b  | $0, 0, 0, -e^{12}, e^{13}, e^{24}, e^{23} - e^{15}, e^{35} + e^{26}, e^{17} + e^{34}$                         | 2469     |
| 9642:97   | $0, 0, 0, e^{12}, e^{13}, e^{24}, e^{25} + e^{34}, e^{26}, e^{14} + e^{36} + e^{27}$                          | 2469     |
| 9642:98   | $0, 0, 0, e^{12}, e^{13}, e^{14}, e^{24} + e^{15}, e^{16}, e^{26} + e^{35} + e^{17}$                          | 2469     |
| 9642:99   | $0, 0, 0, e^{12}, e^{13}, e^{24}, e^{34} + e^{25}, e^{26}, e^{15} + e^{27} + e^{36}$                          | 2469     |
| 9642:100  | $0, 0, 0, e^{12}, e^{13}, e^{24}, e^{34} + e^{25}, e^{14} + e^{26}, e^{27} + e^{36}$                          | 2469     |
| 9642:101  | $0, 0, 0, e^{12}, e^{13}, e^{14}, e^{24} + e^{15}, e^{16} + e^{35}, e^{17} + e^{26}$                          | 2469     |
| 9642:102  | $0, 0, 0, e^{12}, e^{13}, e^{24}, e^{25} + e^{34}, e^{15} + e^{26}, e^{36} + e^{27}$                          | 2469     |
| 9642:103  | $0, 0, 0, e^{12}, e^{13}, e^{24}, e^{25} + e^{34}, e^{26} + e^{35}, e^{36} + e^{27}$                          | 2469     |
| 9642:104  | $0, 0, 0, -e^{12}, e^{13}, e^{14}, e^{15} + e^{23}, e^{16}, e^{45} + e^{36} + e^{27}$                         | 2469     |
| 9642:110  | $0, 0, 0, -e^{12}, e^{13}, e^{14}, e^{15} + e^{24}, e^{16}, e^{27} + e^{45} + e^{36}$                         | 2469     |
| 9642:111  | $0, 0, 0, e^{12}, e^{13}, 2e^{14}, e^{25} + e^{34}, e^{16}, e^{36} + e^{17} + e^{45}$                         | 2469     |
| 9642:113a | $0, 0, 0, e^{12}, e^{13}, e^{14}, e^{15}, e^{16} + e^{23}, e^{24} + e^{35} + e^{17}$                          | 2469     |
| 9642:113b | $0, 0, 0, -e^{12}, e^{13}, e^{14}, e^{15}, e^{23} + e^{16}, e^{17} + e^{35} + e^{24}$                         | 2469     |
| 9642:114  | $0, 0, 0, e^{12}, e^{13}, e^{14}, e^{15}, e^{23} + e^{16}, e^{34} + e^{17} + e^{25}$                          | 2469     |
| 9642:115a | $0, 0, 0, e^{12}, e^{13}, e^{14}, e^{35}, e^{16} + e^{23}, e^{15} + e^{24} + e^{37}$                          | 2469     |
| 9642:115b | $0, 0, 0, e^{12}, -e^{13}, e^{14}, e^{35}, e^{23} + e^{16}, e^{37} + e^{15} + e^{24}$                         | 2469     |
| 9642:116  | $0, 0, 0, e^{12}, e^{13}, a_2e^{14}, e^{15}, e^{16} + e^{24}, e^{17} + e^{34} + e^{25}$                       | 2469     |
| 9642:117  | $0, 0, 0, e^{12}, e^{13}, e^{24}, e^{15}, e^{26} + e^{14}, e^{17} + e^{34} + e^{25}$                          | 2469     |
| 9642:118a | $0, 0, 0, e^{12}, e^{13}, e^{14}, e^{15}, e^{16} + e^{25} + e^{34}, e^{17} + e^{24}$                          | 2469     |
| 9642:118b | $0, 0, 0, e^{12}, e^{13}, -e^{14}, e^{15}, e^{34} + e^{25} + e^{16}, e^{24} + e^{17}$                         | 2469     |
| 9642:119a | $0, 0, 0, e^{12}, e^{13}, e^{14}, e^{35}, e^{25} + e^{34} + e^{16}, e^{24} + e^{37}$                          | 2469     |
| 9642:119b | $0, 0, 0, e^{12}, e^{13}, -e^{14}, e^{35}, e^{34} + e^{16} + e^{25}, e^{37} + e^{24}$                         | 2469     |
| 9642:120  | $0, 0, 0, -e^{12}, e^{13}, e^{14}, e^{15}, e^{23} + e^{16}, e^{45} + e^{36} + e^{27}$                         | 2469     |
| 9642:121  | $0, 0, 0, -e^{12}, e^{13}, e^{14}, e^{15}, e^{16} + e^{24}, e^{45} + e^{27} + e^{36}$                         | 2469     |
| 9642:122  | $0, 0, 0, -e^{12}, e^{13}, e^{14}, e^{15}, e^{35} + e^{16}, e^{45} + e^{36} + e^{27}$                         | 2469     |
| 9642:123  | $0, 0, 0, -e^{12}, e^{13}, e^{14} + e^{23}, e^{15} + e^{24}, e^{34} + e^{16}, e^{17} + e^{26}$                | 2469     |
| 9642:124  | $0, 0, 0, e^{12}, e^{13}, e^{14} + e^{23}, e^{15} + e^{24}, e^{16} + e^{25}, e^{17} + e^{26}$                 | 2469     |
| 9642:126a | $0, 0, 0, e^{12}, e^{13}, e^{25} + e^{34}, e^{24} + e^{35}, e^{36} + e^{27}, e^{37} + e^{26}$                 | 2469     |
| 9642:126b | $0, 0, 0, -e^{12}, e^{13}, e^{34} - e^{25}, e^{35} + e^{24}, -e^{27} + e^{36}, e^{26} + e^{37}$               | 2469     |
| 9642:127a | $0, 0, 0, e^{12}, e^{13}, e^{14}, e^{15} + e^{24}, e^{16} + e^{23}, e^{17} + e^{26} + e^{35}$                 | 2469     |
| 9642:127b | $0, 0, 0, e^{12}, -e^{13}, e^{14}, e^{15} + e^{24}, e^{16} + e^{23}, e^{17} + e^{35} + e^{26}$                | 2469     |
| 9642:128  | $0, 0, 0, (-1 + a_2)e^{12}, a_2e^{13}, e^{14}a_3, e^{15} + e^{23}, e^{24} + e^{16}, e^{25} + e^{34} + e^{17}$ | 2469     |
| 9642:129  | $0, 0, 0, (-1 + a_2)e^{12}, e^{13}a_2, e^{24}, e^{15} + e^{23}, e^{26} + e^{14}, e^{25} + e^{34} + e^{17}$    | 2469     |
| 9642:130a | $0, 0, 0, -e^{12}, e^{13}, e^{23} + a_2e^{14}, e^{15}, e^{34} + e^{16}, e^{35} + e^{17} + e^{24}$             | 2469     |
| 9642:130b | $0, 0, 0, -e^{12}, -e^{13}, e^{23} + a_2e^{14}, e^{15}, e^{16} + e^{34}, e^{24} + e^{17} + e^{35}$            | 2469     |
| 9642:131a | $0, 0, 0, -e^{12}, e^{13}, e^{14} + e^{23}, e^{35}, e^{34} + e^{16}, e^{37} + e^{15} + e^{24}$                | 2469     |
| 9642:131b | $0, 0, 0, -e^{12}, -e^{13}, e^{23} + e^{14}, e^{35}, e^{16} + e^{34}, e^{24} + e^{37} + e^{15}$               | 2469     |
| 9642:132a | $0, 0, 0, -e^{12}, e^{13}, e^{14}a_2, e^{15} + e^{23}, e^{35} + e^{16} + e^{24}, e^{17} + e^{34}$             | 2469     |
| 9642:132b | $0, 0, 0, -e^{12}, -e^{13}, e^{14}a_2, e^{15} + e^{23}, e^{35} + e^{16} + e^{24}, e^{34} + e^{17}$            | 2469     |
| 9642:133a | $0, 0, 0, -e^{12}, e^{13}, e^{24}, e^{15} + e^{23}, e^{14} + e^{26} + e^{35}, e^{17} + e^{34}$                | 2469     |
| 9642:133b | $0, 0, 0, -e^{12}, e^{13}, e^{24}, -e^{15} + e^{23}, e^{26} + e^{35} + e^{14}, e^{17} + e^{34}$               | 2469     |
| 9642:134a | $0, 0, 0, (-1 + a_2)e^{12}, a_2e^{13}, e^{14} + e^{23}, e^{15}, e^{16} + e^{25} + e^{34}, e^{17} + e^{24}$    | 2469     |

Table 2 – Continued to next page

Table 2 – Continued from previous page

| Name      | $\mathfrak{g}$                                                                                                                             | UCS Dim. |
|-----------|--------------------------------------------------------------------------------------------------------------------------------------------|----------|
| 9642:134b | $0, 0, 0, (-1 + a_2)e^{12}, a_2e^{13}, -e^{14} + e^{23}, e^{15}, e^{25} + e^{34} + e^{16}, e^{24} + e^{17}$                                | 2469     |
| 9642:135a | $0, 0, 0, (-1 + a_2)e^{12}, e^{13}a_2, e^{14} + e^{23}, e^{35}, e^{16} + e^{25} + e^{34}, e^{24} + e^{37}$                                 | 2469     |
| 9642:135b | $0, 0, 0, (-1 + a_2)e^{12}, e^{13}a_2, -e^{14} + e^{23}, e^{35}, e^{25} + e^{34} + e^{16}, e^{24} + e^{37}$                                | 2469     |
| 9642:141a | $0, 0, 0, e^{12}, e^{13}, e^{14}, -e^{15} + e^{24}, e^{16} + e^{23}, e^{27} + e^{36} + e^{45}$                                             | 2469     |
| 9642:141b | $0, 0, 0, -e^{12}, e^{13}, e^{14}, e^{24} + e^{15}, e^{16} + e^{23}, e^{45} + e^{36} + e^{27}$                                             | 2469     |
| 9642:142  | $0, 0, 0, e^{12}, e^{13}, 2e^{14}, e^{25} + e^{34}, e^{16} + e^{23}, e^{17} + e^{36} + e^{45}$                                             | 2469     |
| 9642:143  | $0, 0, 0, e^{12}, e^{13}, e^{24}, e^{25} + e^{34}, e^{26} + e^{14}a_2, e^{15} + e^{36} + e^{27}$                                           | 2469     |
| 9642:144a | $0, 0, 0, e^{12}, e^{13}, e^{24}, e^{25} + e^{34}, e^{15} + e^{26}, e^{14} + e^{36} + e^{27}$                                              | 2469     |
| 9642:144b | $0, 0, 0, e^{12}, e^{13}, e^{24}, e^{25} + e^{34}, e^{26} - e^{15}, e^{36} + e^{27} + e^{14}$                                              | 2469     |
| 9642:145  | $0, 0, 0, e^{12}, e^{13}, e^{24}, e^{25} + e^{34}, e^{26} + e^{35}, e^{14} + e^{36} + e^{27}$                                              | 2469     |
| 9642:146  | $0, 0, 0, e^{12}, e^{13}, e^{14}, e^{24} + e^{15}, e^{25} + e^{34} + e^{16}, e^{26} + e^{17}$                                              | 2469     |
| 9642:147  | $0, 0, 0, e^{12}, e^{13}, e^{24}, e^{25} + e^{34}, e^{14} + e^{26} + e^{35}, e^{36} + e^{27}$                                              | 2469     |
| 9642:148  | $0, 0, 0, e^{12}, e^{13}, e^{24}, e^{25} + e^{34}, e^{26} + e^{35}, e^{36} + e^{27} + e^{15}$                                              | 2469     |
| 9642:149  | $0, 0, 0, -e^{12}a_3, e^{13}, e^{14}, e^{23} + e^{15}a_3, e^{16} + e^{24}, e^{45} + e^{36} + e^{27}$                                       | 2469     |
| 9642:150a | $0, 0, 0, -e^{12}, e^{13}, e^{14}, e^{15} + e^{23}, e^{35} + e^{16}, e^{45} + e^{36} + e^{27}$                                             | 2469     |
| 9642:150b | $0, 0, 0, -e^{12}, -e^{13}, -e^{14}, e^{15} + e^{23}, e^{16} + e^{35}, e^{27} + e^{36} + e^{45}$                                           | 2469     |
| 9642:153  | $0, 0, 0, e^{12}, e^{13}, 2e^{14}, e^{25} + e^{34}, e^{24} + e^{16}, e^{36} + e^{17} + e^{45}$                                             | 2469     |
| 9642:154  | $0, 0, 0, -e^{12}, e^{13}, e^{14}, e^{15} + e^{24}, e^{16} + e^{35}, e^{45} + e^{27} + e^{36}$                                             | 2469     |
| 9642:155  | $0, 0, 0, e^{12}, e^{13}, 2e^{14}, e^{25} + e^{34}, e^{16} + e^{35}, e^{17} + e^{36} + e^{45}$                                             | 2469     |
| 9642:157  | $0, 0, 0, -e^{12}, e^{13}, e^{14} + e^{23}, e^{15}, e^{34} + e^{16}, e^{45} + e^{36} + e^{27}$                                             | 2469     |
| 9642:158  | $0, 0, 0, -e^{12}, e^{13}, e^{14} + e^{23}, e^{15}, e^{25} + e^{16}, e^{45} + e^{36} + e^{27}$                                             | 2469     |
| 9642:161  | $0, 0, 0, -e^{12}, e^{13}, e^{14}, e^{15} + e^{24}, e^{17} + e^{26}, e^{27} + e^{45} + e^{36}$                                             | 2469     |
| 9642:163a | $0, 0, 0, e^{12}, e^{13}, a_1e^{14}, e^{15}, e^{16} + e^{25} + e^{34}, e^{17} + e^{24} + e^{35}$                                           | 2469     |
| 9642:163b | $0, 0, 0, -e^{12}, e^{13}, a_1e^{14}, e^{15}, e^{16} + e^{34} - e^{25}, e^{17} + e^{35} + e^{24}$                                          | 2469     |
| 9642:164a | $0, 0, 0, e^{12}, e^{13}, e^{24}, e^{15}, e^{14} + e^{26} + e^{35}, e^{17} + e^{25} + e^{34}$                                              | 2469     |
| 9642:164b | $0, 0, 0, e^{12}, e^{13}, e^{24}, -e^{15}, e^{35} + e^{26} + e^{14}, e^{34} + e^{25} + e^{17}$                                             | 2469     |
| 9642:165a | $0, 0, 0, -e^{12}, e^{13}, e^{14}, e^{15}, e^{35} + e^{16} + e^{24}, e^{27} + e^{45} + e^{36}$                                             | 2469     |
| 9642:165b | $0, 0, 0, -e^{12}, -e^{13}, -e^{14}, e^{15}, e^{35} + e^{24} + e^{16}, e^{36} + e^{45} + e^{27}$                                           | 2469     |
| 9642:166  | $0, 0, 0, -e^{12}, -e^{13}, -e^{14}, e^{15}, e^{16} + e^{25} + e^{34}, e^{36} + e^{45} + e^{27}$                                           | 2469     |
| 9642:167  | $0, 0, 0, -e^{12}, e^{13}, e^{14} + e^{23}, a_3e^{15} + e^{24}, e^{34} + e^{16}, e^{17} + e^{35} + e^{26}$                                 | 2469     |
| 9642:168  | $0, 0, 0, (-1 + a_2)e^{12}, e^{13}a_2, e^{14} + e^{23}, e^{24} + e^{15}, e^{25} + e^{34} + e^{16}, e^{26} + e^{17}$                        | 2469     |
| 9642:169  | $0, 0, 0, a_1e^{12}, e^{13}, e^{14} + e^{23}, e^{24} + e^{15}, e^{25} + e^{16}, e^{26} + e^{35} + e^{17}$                                  | 2469     |
| 9642:171  | $0, 0, 0, -e^{12}, e^{13}, e^{14} + e^{23}, e^{15} + e^{24}, e^{16} + e^{34}, e^{45} + e^{27} + e^{36}$                                    | 2469     |
| 9642:172  | $0, 0, 0, -e^{12}, e^{13}, e^{14} + e^{23}, e^{15} + e^{24}, e^{25} + e^{16}, e^{27} + e^{45} + e^{36}$                                    | 2469     |
| 9642:175a | $0, 0, 0, e^{12}, e^{13}, e^{25} + e^{34}, e^{24} + e^{35}, e^{37} + e^{26}, e^{36} + e^{27} + e^{14}$                                     | 2469     |
| 9642:175b | $0, 0, 0, e^{12}, e^{13}, e^{25} + e^{34}, -e^{24} + e^{35}, e^{37} - e^{26}, e^{14} + e^{36} + e^{27}$                                    | 2469     |
| 9642:176a | $0, 0, 0, e^{12}, e^{13}, e^{24} + e^{35}, e^{25} + e^{34}, e^{37} + e^{26}, e^{36} + e^{27} + e^{14}$                                     | 2469     |
| 9642:176b | $0, 0, 0, -e^{12}, e^{13}, e^{35} + e^{24}, e^{34} - e^{25}, -e^{26} + e^{37}, e^{14} + e^{27} + e^{36}$                                   | 2469     |
| 9642:177  | $0, 0, 0, -e^{12}, e^{13}, e^{14} + e^{23}, e^{15} + e^{24}, e^{26} + e^{17}, e^{45} + e^{27} + e^{36}$                                    | 2469     |
| 9642:178a | $0, 0, 0, (-1 + a_2)e^{12}, e^{13}a_2, e^{14}, e^{15} + e^{23}, a_3e^{24} + e^{35} + e^{16}, e^{25} + e^{34} + e^{17}$                     | 2469     |
| 9642:178b | $0, 0, 0, (-1 + a_2)e^{12}, e^{13}a_2, -e^{14}, e^{15} + e^{23}, a_3e^{24} + e^{35} + e^{16}, e^{25} + e^{34} + e^{17}$                    | 2469     |
| 9642:179a | $0, 0, 0, e^{12}(-1 + a_2), a_2e^{13}, e^{24}, e^{15} + e^{23}, e^{26} + e^{35} + e^{14}, e^{25} + e^{34} + e^{17}$                        | 2469     |
| 9642:179b | $0, 0, 0, e^{12}(-1 + a_2), a_2e^{13}, e^{24}, -e^{15} + e^{23}, e^{14} + e^{26} + e^{35}, e^{17} + e^{25} + e^{34}$                       | 2469     |
| 9642:182  | $0, 0, 0, e^{12}, e^{13}, e^{14}, a_3e^{15} + e^{24}, e^{25} + e^{34} + e^{16}, e^{26} + e^{35} + e^{17}$                                  | 2469     |
| 9642:183  | $0, 0, 0, e^{12}, e^{13}, e^{24}, e^{25} + e^{34}, e^{14}a_2 + e^{26} + e^{35}, e^{36} + e^{27} + e^{15}$                                  | 2469     |
| 9642:184a | $0, 0, 0, -a_1e^{12}, e^{13}, e^{14}, a_1e^{15} + e^{23}, e^{35} + e^{16} + e^{24}, e^{27} + e^{45} + e^{36}$                              | 2469     |
| 9642:184b | $0, 0, 0, -a_1e^{12}, -e^{13}, -e^{14}, a_1e^{15} + e^{23}, e^{16} + e^{35} + e^{24}, e^{27} + e^{36} + e^{45}$                            | 2469     |
| 9642:185  | $0, 0, 0, -e^{12}, -e^{13}, -e^{14}, e^{23} + e^{15}, e^{16} + e^{25} + e^{34}, e^{36} + e^{45} + e^{27}$                                  | 2469     |
| 9642:186  | $0, 0, 0, -e^{12}, -e^{13}, -e^{14}, e^{24} + e^{15}, e^{16} + e^{25} + e^{34}, e^{36} + e^{45} + e^{27}$                                  | 2469     |
| 9642:187a | $0, 0, 0, e^{12}, e^{13}, 2e^{14}, e^{25} + e^{34}, e^{24} + e^{35} + e^{16}, e^{36} + e^{17} + e^{45}$                                    | 2469     |
| 9642:187b | $0, 0, 0, -e^{12}, e^{13}, 2e^{14}, -e^{25} + e^{34}, e^{16} + e^{24} + e^{35}, e^{45} + e^{17} + e^{36}$                                  | 2469     |
| 9642:190  | $0, 0, 0, (-1 + a_3)e^{12}, e^{13}a_3, e^{14}a_3 + e^{23}, -(-1 + a_3)e^{15}, e^{34} + e^{25} + e^{16}, e^{27} + e^{45} + e^{36}$          | 2469     |
| 9642:192  | $0, 0, 0, -e^{12}, e^{13}, e^{14}, e^{15} + e^{24}, e^{26} + e^{17} + e^{35}, e^{45} + e^{27} + e^{36}$                                    | 2469     |
| 9642:194  | $0, 0, 0, e^{12}a_1, (1 + a_1)e^{13}, e^{14} + e^{23}, e^{15}a_4 + e^{24}, e^{25} + e^{34} + e^{16}, e^{26} + e^{35} + e^{17}$             | 2469     |
| 9642:197  | $0, 0, 0, (-1 + a_3)e^{12}, e^{13}a_3, e^{23} + e^{14}a_3, -(-1 + a_3)e^{15} + e^{24}, e^{25} + e^{16} + e^{34}, e^{45} + e^{27} + e^{36}$ | 2469     |
| 9642:198a | $0, 0, 0, e^{12}, e^{13}, e^{25} + e^{34}, e^{24} + e^{35}, e^{36} + e^{27} + e^{14}a_1, e^{37} + e^{26} + e^{15}$                         | 2469     |
| 9642:198b | $0, 0, 0, -e^{12}, e^{13}, -e^{25} + e^{34}, e^{24} + e^{35}, e^{36} - e^{27} + e^{14}a_1, e^{15} + e^{37} + e^{26}$                       | 2469     |
| 9642:199a | $0, 0, 0, e^{12}, e^{13}, e^{25} + e^{34}, e^{35} + a_4e^{24}, e^{37} + e^{14} + a_4e^{26}, e^{36} + e^{27} + e^{15}$                      | 2469     |

Table 2 – Continued to next page

Table 2 – Continued from previous page

| Name        | $\mathfrak{g}$                                                                                                          | UCS Dim. |
|-------------|-------------------------------------------------------------------------------------------------------------------------|----------|
| 9642:199b   | $0, 0, 0, e^{12}, e^{13}, e^{25} + e^{34}, e^{35} + a_4 e^{24}, e^{37} - e^{14} + a_4 e^{26}, e^{36} + e^{27} + e^{15}$ | 2469     |
| 9642:200    | $0, 0, 0, -e^{12}, e^{13}, e^{14} + a_4 e^{23}, e^{15} + e^{24}, e^{26} + e^{17} + e^{35}, e^{45} + e^{27} + e^{36}$    | 2469     |
| Type: 33111 |                                                                                                                         |          |
| 96321:1     | $0, 0, 0, e^{12}, e^{13}, e^{23}, e^{14}, e^{17}, e^{18}$                                                               | 35679    |
| 96321:2     | $0, 0, 0, e^{12}, e^{13}, e^{23}, e^{14}, e^{17}, e^{18} + e^{35}$                                                      | 24679    |
| 96321:3a    | $0, 0, 0, e^{12}, e^{13}, e^{23}, e^{24}, e^{27}, e^{28} + e^{35}$                                                      | 24679    |
| 96321:3b    | $0, 0, 0, -e^{12}, e^{13}, e^{23}, e^{24}, e^{27}, e^{28} + e^{35}$                                                     | 24679    |
| 96321:4     | $0, 0, 0, e^{12}, e^{13}, e^{23}, e^{24}, e^{27}, e^{28} + e^{15}$                                                      | 24679    |
| 96321:5     | $0, 0, 0, e^{12}, e^{13}, e^{23}, e^{14}, e^{17}, e^{18} + e^{24}$                                                      | 35679    |
| 96321:6     | $0, 0, 0, -e^{12}, e^{13}, e^{23}, e^{14}, e^{17}, e^{47} + e^{28}$                                                     | 35679    |
| 96321:7     | $0, 0, 0, e^{12}, e^{13}, e^{23}, e^{14}, e^{17}, e^{26} + e^{35} + e^{18}$                                             | 14679    |
| 96321:8a    | $0, 0, 0, e^{12}, e^{13}, e^{23}, e^{14}, e^{17}, e^{18} + e^{35} + e^{24}$                                             | 24679    |
| 96321:8b    | $0, 0, 0, -e^{12}, e^{13}, e^{23}, e^{14}, e^{17}, e^{18} + e^{35} + e^{24}$                                            | 24679    |
| 96321:9     | $0, 0, 0, e^{12}, e^{13}, e^{23}, e^{14}, e^{17}, e^{25} + e^{18} + e^{34}$                                             | 24679    |
| 96321:10a   | $0, 0, 0, e^{12}, e^{13}, e^{23}, e^{24}, e^{27}, e^{35} + e^{28} + e^{14}$                                             | 24679    |
| 96321:10b   | $0, 0, 0, -e^{12}, e^{13}, e^{23}, e^{24}, e^{27}, e^{35} + e^{28} + e^{14}$                                            | 24679    |
| 96321:11a   | $0, 0, 0, -e^{12}, e^{13}, e^{23}, e^{14}, e^{17}, e^{28} + e^{47} + e^{35}$                                            | 24679    |
| 96321:11b   | $0, 0, 0, -e^{12}, -e^{13}, e^{23}, e^{14}, e^{17}, e^{28} + e^{47} + e^{35}$                                           | 24679    |
| 96321:12    | $0, 0, 0, e^{12}, e^{13}, e^{23}, e^{24}, e^{27}, e^{18} + e^{35} + e^{47}$                                             | 24679    |
| 96321:13    | $0, 0, 0, e^{12}, e^{13}, e^{23}, e^{14}, e^{17} + e^{24}, e^{18} + e^{27}$                                             | 35679    |
| 96321:14    | $0, 0, 0, -e^{12}, e^{13}, e^{23}, e^{14}, e^{17}, e^{15} + e^{28} + e^{47}$                                            | 24679    |
| 96321:15    | $0, 0, 0, -e^{12}, e^{13}, e^{23}, e^{14}, e^{24} + e^{17}, e^{28} + e^{47}$                                            | 35679    |
| 96321:16    | $0, 0, 0, -e^{12}, e^{13}, e^{23}, e^{14}, e^{17}, e^{47} + e^{28} + e^{15} + e^{36}$                                   | 14679    |
| 96321:17    | $0, 0, 0, e^{12}, e^{13}, e^{23}, e^{14}, e^{17} + e^{24}, e^{35} + e^{18} + e^{27}$                                    | 24679    |
| 96321:18a   | $0, 0, 0, e^{12}, e^{13}, e^{23}, e^{24}, e^{14} + e^{27}, e^{35} + e^{28} + e^{17}$                                    | 24679    |
| 96321:18b   | $0, 0, 0, -e^{12}, e^{13}, e^{23}, e^{24}, e^{14} + e^{27}, e^{17} + e^{35} + e^{28}$                                   | 24679    |
| 96321:19a   | $0, 0, 0, -e^{12}, e^{13}, e^{23}, e^{14}, e^{17} + e^{24}, e^{28} + e^{35} + e^{47}$                                   | 24679    |
| 96321:19b   | $0, 0, 0, -e^{12}, -e^{13}, e^{23}, e^{14}, e^{17} + e^{24}, e^{35} + e^{47} + e^{28}$                                  | 24679    |
| 96321:20    | $0, 0, 0, e^{12}, e^{13}, e^{23}, e^{24}, e^{14} + e^{27}, e^{35} + e^{47} + e^{18}$                                    | 24679    |
| 96321:21    | $0, 0, 0, -e^{12}, e^{13}, e^{23}, e^{14}, e^{24} + e^{17}, e^{15} + e^{28} + e^{47}$                                   | 24679    |
| 96321:22    | $0, 0, 0, -e^{12}, e^{13}, e^{23}, e^{14}, e^{17} + e^{24}, e^{28} + e^{15} + e^{36} + e^{47}$                          | 14679    |
| 96321:23    | $0, 0, 0, e^{12}, e^{13}, e^{23}, e^{24}, e^{27} + e^{15}, e^{18} + e^{47}$                                             | 23579    |
| 96321:25    | $0, 0, 0, e^{12}, e^{13}, e^{23}, e^{24}, e^{15} + e^{27}, e^{18} + e^{35} + e^{47}$                                    | 23579    |
| 96321:26a   | $0, 0, 0, e^{12}, e^{13}, e^{23}, e^{24}, e^{27} + e^{15}, e^{36} + e^{47} + e^{18}$                                    | 13579    |
| 96321:26b   | $0, 0, 0, e^{12}, e^{13}, -e^{23}, e^{24}, e^{15} + e^{27}, e^{47} + e^{36} + e^{18}$                                   | 13579    |
| 96321:28    | $0, 0, 0, e^{12}, e^{13}, e^{23}, e^{24}, e^{15} + e^{27}, e^{26} + e^{47} + e^{18}$                                    | 13579    |
| 96321:30    | $0, 0, 0, e^{12}, e^{13}, e^{23}, 2e^{14}, e^{17} + e^{25} + e^{34}, e^{37} + e^{45} + e^{18}$                          | 23579    |
| 96321:31    | $0, 0, 0, e^{12}, e^{13}, e^{23}, e^{24}, e^{15} + e^{27}, e^{35} + e^{47} + e^{18} + e^{26}$                           | 13579    |
| 96321:32    | $0, 0, 0, e^{12}, e^{13}, e^{23}, 2e^{14}, e^{25} + e^{17} + e^{34}, e^{37} + e^{26} + e^{45} + e^{18}$                 | 13579    |
| Type: 3123  |                                                                                                                         |          |
| 9653:1      | $0, 0, 0, e^{12}, e^{14}, e^{24}, e^{15}, e^{26}, e^{25} + e^{16}$                                                      | 4679     |
| 9653:2      | $0, 0, 0, e^{12}, e^{14}, e^{24}, e^{15}, e^{26} + e^{13}, e^{16} + e^{25}$                                             | 3679     |
| 9653:3      | $0, 0, 0, e^{12}, e^{14}, e^{24}, e^{15} + e^{23}, e^{13} + e^{26}, e^{25} + e^{16}$                                    | 3679     |
| 9653:4      | $0, 0, 0, e^{12}, e^{14}, e^{24} + e^{13}, e^{15}, e^{26} + e^{34}, e^{16} + e^{25}$                                    | 3579     |
| 9653:5      | $0, 0, 0, e^{12}, e^{14}, e^{24} + e^{13}, e^{15} + e^{23}, e^{26} + e^{34}, e^{16} + e^{25}$                           | 3579     |
| Type: 3231  |                                                                                                                         |          |
| 9641:1      | $0, 0, 0, e^{12}, e^{13}, e^{14}, e^{15}, e^{35}, e^{16}$                                                               | 3579     |
| 9641:2      | $0, 0, 0, e^{12}, e^{13}, e^{24}, e^{15}, e^{35}, e^{26}$                                                               | 3579     |
| 9641:3      | $0, 0, 0, e^{12}, e^{13}, e^{14}, e^{24}, e^{35}, e^{16}$                                                               | 3579     |
| 9641:4      | $0, 0, 0, e^{12}, e^{13}, e^{24}, e^{14}, e^{35}, e^{26}$                                                               | 3579     |
| 9641:5      | $0, 0, 0, e^{12}, e^{13}, e^{14}, e^{35}, e^{15} + e^{23}, e^{16}$                                                      | 3579     |
| 9641:6      | $0, 0, 0, e^{12}, e^{13}, e^{24}, e^{35}, e^{15} + e^{23}, e^{26}$                                                      | 3579     |
| 9641:7      | $0, 0, 0, e^{12}, e^{13}, e^{14}, e^{35}, e^{25} + e^{34}, e^{16}$                                                      | 3579     |
| 9641:8      | $0, 0, 0, e^{12}, e^{13}, e^{24}, e^{35}, e^{25} + e^{34}, e^{26}$                                                      | 3579     |
| 9641:9      | $0, 0, 0, e^{12}, e^{13}, e^{14}, e^{24}, e^{15}, e^{16}$                                                               | 3579     |
| 9641:10     | $0, 0, 0, e^{12}, e^{13}, e^{24}, e^{14}, e^{15}, e^{26}$                                                               | 3579     |
| 9641:11     | $0, 0, 0, e^{12}, e^{13}, e^{14}, e^{15}, e^{35}, e^{16} + e^{23}$                                                      | 3579     |
| 9641:12     | $0, 0, 0, e^{12}, e^{13}, e^{24}, e^{14} + e^{23}, e^{35}, e^{26}$                                                      | 3579     |

Table 2 – Continued to next page



Table 2 – Continued from previous page

| Name     | $\mathfrak{g}$                                                                         | UCS Dim. |
|----------|----------------------------------------------------------------------------------------|----------|
| 9641:13a | $0, 0, 0, e^{12}, e^{13}, e^{14}, e^{15}, e^{24} + e^{35}, e^{16}$                     | 3579     |
| 9641:13b | $0, 0, 0, -e^{12}, e^{13}, e^{14}, e^{15}, e^{35} + e^{24}, e^{16}$                    | 3579     |
| 9641:14  | $0, 0, 0, e^{12}, e^{13}, e^{14}, e^{15}, e^{25} + e^{34}, e^{16}$                     | 3579     |
| 9641:15  | $0, 0, 0, e^{12}, e^{13}, e^{24}, e^{15}, e^{35} + e^{14}, e^{26}$                     | 3579     |
| 9641:16  | $0, 0, 0, e^{12}, e^{13}, e^{24}, e^{15}, e^{34} + e^{25}, e^{26}$                     | 3579     |
| 9641:17  | $0, 0, 0, e^{12}, e^{13}, e^{14}, e^{35}, e^{15} + e^{24}, e^{16}$                     | 3579     |
| 9641:18  | $0, 0, 0, e^{12}, e^{13}, e^{14}, e^{24}, e^{15} + e^{23}, e^{16}$                     | 3579     |
| 9641:19  | $0, 0, 0, e^{12}, e^{13}, e^{24}, e^{14}, e^{23} + e^{15}, e^{26}$                     | 3579     |
| 9641:20  | $0, 0, 0, e^{12}, e^{13}, e^{14}, e^{24}, e^{35}, e^{23} + e^{16}$                     | 3579     |
| 9641:21  | $0, 0, 0, e^{12}, e^{13}, e^{24}, e^{14} + e^{23}, e^{15}, e^{26}$                     | 3579     |
| 9641:22  | $0, 0, 0, e^{12}, e^{13}, e^{14}, e^{24}, e^{25} + e^{34}, e^{16}$                     | 3579     |
| 9641:23  | $0, 0, 0, e^{12}, e^{13}, e^{24}, e^{14}, e^{25} + e^{34}, e^{26}$                     | 3579     |
| 9641:24  | $0, 0, 0, e^{12}, e^{13}, e^{14}, e^{24}, e^{15}, e^{35} + e^{16}$                     | 3579     |
| 9641:25  | $0, 0, 0, e^{12}, e^{13}, e^{24}, e^{14}, e^{15}, e^{35} + e^{26}$                     | 3579     |
| 9641:26  | $0, 0, 0, e^{12}, e^{13}, e^{24}, e^{14}, e^{35}, e^{15} + e^{26}$                     | 3579     |
| 9641:27  | $0, 0, 0, e^{12}, e^{13}, e^{14}, e^{15}, e^{35}, e^{24} + e^{16}$                     | 3579     |
| 9641:28  | $0, 0, 0, e^{12}, e^{13}, e^{24}, e^{15}, e^{35}, e^{14} + e^{26}$                     | 3579     |
| 9641:29a | $0, 0, 0, e^{12}, e^{13}, e^{14}, e^{15} + e^{23}, e^{35} + e^{24}, e^{16}$            | 3579     |
| 9641:29b | $0, 0, 0, -e^{12}, e^{13}, e^{14}, e^{15} + e^{23}, e^{35} + e^{24}, e^{16}$           | 3579     |
| 9641:30  | $0, 0, 0, e^{12}, e^{13}, e^{14}, e^{15} + e^{23}, e^{25} + e^{34}, e^{16}$            | 3579     |
| 9641:31  | $0, 0, 0, e^{12}, e^{13}, e^{24}, e^{15} + e^{23}, e^{14} + e^{35}, e^{26}$            | 3579     |
| 9641:32  | $0, 0, 0, e^{12}, e^{13}, e^{24}, e^{23} + e^{15}, e^{25} + e^{34}, e^{26}$            | 3579     |
| 9641:33  | $0, 0, 0, e^{12}, e^{13}, e^{14}, e^{35}, e^{25} + e^{34}, e^{23} + e^{16}$            | 3579     |
| 9641:34  | $0, 0, 0, e^{12}, e^{13}, e^{23} + e^{14}, e^{15}, e^{35}, e^{16} + e^{25}$            | 3579     |
| 9641:35a | $0, 0, 0, e^{12}, e^{13}, e^{14}, e^{25} + e^{34}, e^{24} + e^{35}, e^{16}$            | 3579     |
| 9641:35b | $0, 0, 0, -e^{12}, e^{13}, e^{14}, -e^{25} + e^{34}, e^{24} + e^{35}, e^{16}$          | 3579     |
| 9641:36  | $0, 0, 0, e^{12}, e^{13}, e^{24}, e^{35} + e^{14}, e^{34} + e^{25}, e^{26}$            | 3579     |
| 9641:37  | $0, 0, 0, e^{12}, e^{13}, e^{14}, e^{15}, e^{25} + e^{34}, e^{16} + e^{35}$            | 3579     |
| 9641:38  | $0, 0, 0, e^{12}, e^{13}, e^{24}, e^{15}, e^{34} + e^{25}, e^{35} + e^{26}$            | 3579     |
| 9641:39  | $0, 0, 0, e^{12}, e^{13}, e^{24}, e^{35}, e^{25} + e^{34}, e^{15} + e^{26}$            | 3579     |
| 9641:40  | $0, 0, 0, -e^{12}, e^{13}, e^{23} + e^{14}, e^{15}, e^{35}, e^{16} + e^{34}$           | 3579     |
| 9641:41  | $0, 0, 0, e^{12}, e^{13}, e^{14}, e^{24}, e^{15}, e^{16} + e^{23}$                     | 3579     |
| 9641:42a | $0, 0, 0, e^{12}, e^{13}, e^{14}, e^{15}, e^{24} + e^{35}, e^{16} + e^{23}$            | 3579     |
| 9641:42b | $0, 0, 0, -e^{12}, e^{13}, e^{14}, e^{15}, e^{35} + e^{24}, e^{23} + e^{16}$           | 3579     |
| 9641:43  | $0, 0, 0, e^{12}, e^{13}, e^{14}, e^{15}, e^{34} + e^{25}, e^{16} + e^{23}$            | 3579     |
| 9641:44a | $0, 0, 0, e^{12}, e^{13}, e^{14}, e^{35}, e^{24} + e^{15}, e^{16} + e^{23}$            | 3579     |
| 9641:44b | $0, 0, 0, e^{12}, -e^{13}, e^{14}, e^{35}, e^{15} + e^{24}, e^{23} + e^{16}$           | 3579     |
| 9641:45  | $0, 0, 0, e^{12}, e^{13}, e^{24}, e^{14} + e^{23}, e^{34} + e^{25}, e^{26}$            | 3579     |
| 9641:46a | $0, 0, 0, e^{12}, e^{13}, e^{14}, e^{24}, e^{15} + e^{23}, e^{16} + e^{35}$            | 3579     |
| 9641:46b | $0, 0, 0, -e^{12}, e^{13}, e^{14}, e^{24}, e^{15} + e^{23}, e^{35} + e^{16}$           | 3579     |
| 9641:47a | $0, 0, 0, e^{12}, e^{13}, e^{24}, e^{14}, e^{15} + e^{23}, e^{35} + e^{26}$            | 3579     |
| 9641:47b | $0, 0, 0, -e^{12}, e^{13}, e^{24}, e^{14}, e^{23} + e^{15}, e^{35} + e^{26}$           | 3579     |
| 9641:48  | $0, 0, 0, e^{12}, e^{13}, e^{24}, e^{14} + e^{23}, e^{15}, e^{26} + e^{35}$            | 3579     |
| 9641:49  | $0, 0, 0, e^{12}, e^{13}, e^{24}, e^{14} + e^{23}, e^{35}, e^{26} + e^{15}$            | 3579     |
| 9641:50  | $0, 0, 0, e^{12}, a_1 e^{13}, e^{14}, e^{35}, e^{23} + e^{15}, e^{16} + e^{24}$        | 3579     |
| 9641:51  | $0, 0, 0, e^{12}, e^{13}, e^{24}, e^{35}, e^{15} + e^{23}, e^{14} + e^{26}$            | 3579     |
| 9641:52  | $0, 0, 0, e^{12}, e^{13}, e^{14}, e^{15} + e^{24}, e^{25} + e^{34}, e^{16}$            | 3579     |
| 9641:53  | $0, 0, 0, e^{12}, e^{13}, e^{23} + e^{14}, e^{24}, e^{35}, e^{16} + e^{25}$            | 3579     |
| 9641:54  | $0, 0, 0, e^{12}, e^{13}, e^{14}, e^{15}, e^{35}, e^{34} + e^{25} + e^{16}$            | 3579     |
| 9641:55  | $0, 0, 0, e^{12}, e^{13}, e^{14}, e^{24}, e^{25} + e^{34}, e^{16} + e^{35}$            | 3579     |
| 9641:56  | $0, 0, 0, e^{12}, e^{13}, e^{24}, e^{14}, e^{25} + e^{34}, e^{26} + e^{35}$            | 3579     |
| 9641:57  | $0, 0, 0, e^{12}, e^{13}, e^{14}, e^{35}, e^{25} + e^{34}, e^{24} + e^{16}$            | 3579     |
| 9641:58  | $0, 0, 0, e^{12}, e^{13}, e^{24}, e^{35}, e^{25} + e^{34}, e^{14} + e^{26}$            | 3579     |
| 9641:59  | $0, 0, 0, -e^{12}, e^{13}, e^{14} + e^{23}, e^{24}, e^{35}, e^{16} + e^{34}$           | 3579     |
| 9641:60a | $0, 0, 0, e^{12}, e^{13}, e^{14}, e^{15} + e^{23}, e^{34} + e^{25}, e^{35} + e^{16}$   | 3579     |
| 9641:60b | $0, 0, 0, -e^{12}, -e^{13}, e^{14}, e^{15} + e^{23}, e^{25} + e^{34}, e^{35} + e^{16}$ | 3579     |
| 9641:61a | $0, 0, 0, e^{12}, e^{13}, e^{24}, e^{15} + e^{23}, e^{34} + e^{25}, e^{35} + e^{26}$   | 3579     |
| 9641:61b | $0, 0, 0, -e^{12}, -e^{13}, e^{24}, e^{15} + e^{23}, e^{25} + e^{34}, e^{26} + e^{35}$ | 3579     |

Table 2 – Continued to next page

Table 2 – Continued from previous page

| Name        | $\mathfrak{g}$                                                                                                   | UCS Dim. |
|-------------|------------------------------------------------------------------------------------------------------------------|----------|
| 9641:62     | $0, 0, 0, e^{12}, e^{13}, e^{14}, e^{24}, e^{34} + e^{25}, e^{23} + e^{16}$                                      | 3579     |
| 9641:63     | $0, 0, 0, e^{12}, e^{13}, e^{23} + e^{14}, e^{24}, e^{15}, e^{16} + e^{25}$                                      | 3579     |
| 9641:64     | $0, 0, 0, e^{12}, e^{13}, e^{24}, e^{14}, e^{25} + e^{34}, e^{26} + e^{15}$                                      | 3579     |
| 9641:65     | $0, 0, 0, e^{12}, e^{13}, e^{14}, e^{15}, e^{25} + e^{34}, e^{16} + e^{24}$                                      | 3579     |
| 9641:66     | $0, 0, 0, e^{12}, e^{13}, e^{24}, e^{15}, e^{25} + e^{34}, e^{14} + e^{26}$                                      | 3579     |
| 9641:67     | $0, 0, 0, -e^{12}, e^{13}, e^{14} + e^{23}, e^{24}, e^{15}, e^{34} + e^{16}$                                     | 3579     |
| 9641:68     | $0, 0, 0, e^{12}, e^{13}, e^{14}, e^{24}, e^{35}, e^{34} + e^{25} + e^{16}$                                      | 3579     |
| 9641:69a    | $0, 0, 0, e^{12}, e^{13}, e^{14}, e^{25} + e^{34}, e^{35} + e^{24}, e^{16} + e^{23}$                             | 3579     |
| 9641:69b    | $0, 0, 0, -e^{12}, e^{13}, e^{14}, e^{34} - e^{25}, e^{35} + e^{24}, e^{23} + e^{16}$                            | 3579     |
| 9641:70     | $0, 0, 0, e^{12}, e^{13}, e^{14}, e^{35}, e^{23} + e^{15}, e^{16} + e^{25} + e^{34}$                             | 3579     |
| 9641:71     | $0, 0, 0, e^{12}, e^{13}, e^{24}, e^{14} + e^{23}, e^{25} + e^{34}, e^{26} + e^{35}$                             | 3579     |
| 9641:72a    | $0, 0, 0, e^{12}, e^{13}, e^{23} + e^{14}, e^{15}, e^{35} + e^{24}, e^{16} + e^{25}$                             | 3579     |
| 9641:72b    | $0, 0, 0, -e^{12}, e^{13}, e^{14} + e^{23}, e^{15}, e^{35} + e^{24}, e^{25} + e^{16}$                            | 3579     |
| 9641:73     | $0, 0, 0, e^{12}, e^{13}, e^{23} + e^{14}, e^{35}, e^{24} + e^{15}, e^{16} + e^{25}$                             | 3579     |
| 9641:74     | $0, 0, 0, e^{12}, e^{13}, e^{14}, e^{15} + e^{24}, e^{34} + e^{25}, e^{35} + e^{16}$                             | 3579     |
| 9641:75     | $0, 0, 0, e^{12}, e^{13}, e^{24}, e^{35} + e^{14}, e^{25} + e^{34}, e^{15} + e^{26}$                             | 3579     |
| 9641:76     | $0, 0, 0, e^{12}(-1 + a_2), a_2 e^{13}, e^{14} + e^{23}, e^{15}, e^{35}, e^{25} + e^{16} + e^{34}$               | 3579     |
| 9641:77a    | $0, 0, 0, -e^{12}, e^{13}, e^{23} + e^{14}, e^{15}, e^{35} + e^{24}, e^{16} + e^{34}$                            | 3579     |
| 9641:77b    | $0, 0, 0, -e^{12}, -e^{13}, e^{14} + e^{23}, e^{15}, e^{24} + e^{35}, e^{16} + e^{34}$                           | 3579     |
| 9641:78     | $0, 0, 0, -e^{12}, e^{13}, e^{14} + e^{23}, e^{35}, e^{15} + e^{24}, e^{16} + e^{34}$                            | 3579     |
| 9641:79     | $0, 0, 0, e^{12}, e^{13}, e^{14}, e^{24}, e^{15}, e^{16} + e^{25} + e^{34}$                                      | 3579     |
| 9641:80a    | $0, 0, 0, e^{12}, e^{13}, e^{14}, e^{15} + e^{24}, e^{34} + e^{25}, e^{23} + e^{16}$                             | 3579     |
| 9641:80b    | $0, 0, 0, -e^{12}, -e^{13}, e^{14}, e^{15} + e^{24}, e^{25} + e^{34}, e^{16} + e^{23}$                           | 3579     |
| 9641:81     | $0, 0, 0, e^{12}, e^{13}, e^{24}, e^{14} + e^{23}, e^{25} + e^{34}, e^{26} + e^{15}$                             | 3579     |
| 9641:82     | $0, 0, 0, e^{12} a_2, e^{13} a_2, e^{14}, e^{23} + e^{15}, e^{25} + e^{34}, e^{24} + e^{16}$                     | 3579     |
| 9641:83     | $0, 0, 0, e^{12}, e^{13}, e^{24}, e^{15} + e^{23}, e^{25} + e^{34}, e^{26} + e^{14}$                             | 3579     |
| 9641:84a    | $0, 0, 0, e^{12}, e^{13}, e^{14}, e^{15}, e^{35} + e^{24}, e^{34} + e^{25} + e^{16}$                             | 3579     |
| 9641:84b    | $0, 0, 0, e^{12}, e^{13}, e^{14}, e^{15}, e^{35} - e^{24}, e^{16} + e^{25} + e^{34}$                             | 3579     |
| 9641:85a    | $0, 0, 0, e^{12}, e^{13}, e^{14}, e^{15}, e^{34} + e^{25}, e^{35} + e^{16} + e^{24}$                             | 3579     |
| 9641:85b    | $0, 0, 0, -e^{12}, e^{13}, e^{14}, e^{15}, -e^{25} + e^{34}, e^{16} + e^{24} + e^{35}$                           | 3579     |
| 9641:86     | $0, 0, 0, e^{12}, e^{13}, e^{24}, e^{15}, e^{25} + e^{34}, e^{14} + e^{26} + e^{35}$                             | 3579     |
| 9641:87     | $0, 0, 0, e^{12}, e^{13}, e^{14}, e^{35}, e^{24} + e^{15}, e^{16} + e^{25} + e^{34}$                             | 3579     |
| 9641:88     | $0, 0, 0, (-1 + a_2) e^{12}, e^{13} a_2, e^{14} + e^{23}, e^{24}, e^{35}, e^{25} + e^{16} + e^{34}$              | 3579     |
| 9641:89     | $0, 0, 0, e^{12}, e^{13}, e^{14}, e^{24}, e^{15} + e^{23}, e^{25} + e^{16} + e^{34}$                             | 3579     |
| 9641:90     | $0, 0, 0, (-1 + a_2) e^{12}, a_2 e^{13}, e^{23} + e^{14}, e^{24}, e^{15}, e^{16} + e^{25} + e^{34}$              | 3579     |
| 9641:91     | $0, 0, 0, e^{12}, e^{13}, e^{14}, e^{15} + e^{23}, e^{35} + a_2 e^{24}, e^{16} + e^{25} + e^{34}$                | 3579     |
| 9641:92a(*) | $0, 0, 0, e^{12}, a_1 e^{13}, e^{14}, e^{23} + e^{15}, \frac{1}{a_1} e^{25} + e^{34}, e^{35} + e^{24} + e^{16}$  | 3579     |
| 9641:92b(*) | $0, 0, 0, -e^{12}, a_1 e^{13}, e^{14}, e^{15} + e^{23}, \frac{1}{a_1} e^{25} + e^{34}, e^{16} + e^{35} + e^{24}$ | 3579     |
| 9641:93a    | $0, 0, 0, e^{12}, e^{13}, e^{24}, e^{23} + e^{15}, e^{25} + e^{34}, e^{35} + e^{14} + e^{26}$                    | 3579     |
| 9641:93b    | $0, 0, 0, -e^{12}, -e^{13}, e^{24}, e^{15} + e^{23}, e^{34} + e^{25}, e^{14} + e^{26} + e^{35}$                  | 3579     |
| 9641:94a    | $0, 0, 0, e^{12} a_1, e^{13}(1 + a_1), e^{23} + e^{14}, e^{15}, e^{35} + e^{24}, e^{16} + e^{25} + e^{34}$       | 3579     |
| 9641:94b    | $0, 0, 0, e^{12} a_1, e^{13}(1 + a_1), e^{23} + e^{14}, e^{15}, e^{35} - e^{24}, e^{16} + e^{25} + e^{34}$       | 3579     |
| 9641:95     | $0, 0, 0, (-1 + a_2) e^{12}, a_2 e^{13}, e^{23} + e^{14}, e^{35}, e^{15} + e^{24}, e^{16} + e^{25} + e^{34}$     | 3579     |
| 9641:96a    | $0, 0, 0, e^{12}, e^{13}, e^{14}, e^{24}, e^{35}, e^{27} + e^{16}$                                               | 2579     |
| 9641:96b    | $0, 0, 0, e^{12}, e^{13}, -e^{14}, e^{24}, e^{35}, e^{27} + e^{16}$                                              | 2579     |
| 9641:97     | $0, 0, 0, e^{12}, e^{13}, e^{14}, e^{24}, e^{35}, e^{17} + e^{26}$                                               | 2579     |
| 9641:98a    | $0, 0, 0, e^{12}, e^{13}, e^{14}, e^{24}, e^{15}, e^{27} + e^{16}$                                               | 2579     |
| 9641:98b    | $0, 0, 0, e^{12}, e^{13}, -e^{14}, e^{24}, e^{15}, e^{16} + e^{27}$                                              | 2579     |
| 9641:99     | $0, 0, 0, e^{12}, e^{13}, e^{14}, e^{24}, e^{15}, e^{17} + e^{26}$                                               | 2579     |
| 9641:100    | $0, 0, 0, e^{12}, e^{13}, e^{24}, e^{23} + e^{14}, e^{35}, e^{27} + e^{16}$                                      | 2579     |
| 9641:101a   | $0, 0, 0, e^{12}, e^{13}, e^{14}, e^{24}, e^{15} + e^{23}, e^{16} + e^{27}$                                      | 2579     |
| 9641:101b   | $0, 0, 0, e^{12}, e^{13}, -e^{14}, e^{24}, e^{23} + e^{15}, e^{16} + e^{27}$                                     | 2579     |
| 9641:102    | $0, 0, 0, e^{12}, e^{13}, e^{14}, e^{24}, e^{15} + e^{23}, e^{17} + e^{26}$                                      | 2579     |
| 9641:103    | $0, 0, 0, e^{12}, e^{13}, e^{24}, e^{14} + e^{23}, e^{15}, e^{27} + e^{16}$                                      | 2579     |
| 9641:104a   | $0, 0, 0, e^{12}, e^{13}, e^{14}, e^{24}, e^{15}, e^{35} + e^{27} + e^{16}$                                      | 2579     |
| 9641:104b   | $0, 0, 0, e^{12}, e^{13}, -e^{14}, e^{24}, e^{15}, e^{27} + e^{35} + e^{16}$                                     | 2579     |
| 9641:105    | $0, 0, 0, e^{12}, e^{13}, e^{14}, e^{24}, e^{15}, e^{17} + e^{35} + e^{26}$                                      | 2579     |

Table 2 – Continued to next page

Table 2 – Continued from previous page

| Name      | $\mathfrak{g}$                                                                                | UCS Dim. |
|-----------|-----------------------------------------------------------------------------------------------|----------|
| 9641:106a | $0, 0, 0, e^{12}, e^{13}, e^{14}, e^{24}, e^{25} + e^{34}, e^{27} + e^{16}$                   | 2579     |
| 9641:106b | $0, 0, 0, e^{12}, e^{13}, -e^{14}, e^{24}, e^{34} + e^{25}, e^{27} + e^{16}$                  | 2579     |
| 9641:107  | $0, 0, 0, e^{12}, e^{13}, e^{14}, e^{24}, e^{25} + e^{34}, e^{17} + e^{26}$                   | 2579     |
| 9641:108a | $0, 0, 0, e^{12}, e^{13}, e^{14}, e^{24}, e^{15} + e^{23}, e^{27} + e^{16} + e^{35}$          | 2579     |
| 9641:108b | $0, 0, 0, e^{12}, e^{13}, -e^{14}, e^{24}, e^{15} + e^{23}, e^{16} + e^{27} + e^{35}$         | 2579     |
| 9641:108c | $0, 0, 0, -e^{12}, e^{13}, e^{14}, e^{24}, e^{15} + e^{23}, e^{27} + e^{16} + e^{35}$         | 2579     |
| 9641:108d | $0, 0, 0, -e^{12}, e^{13}, -e^{14}, e^{24}, e^{23} + e^{15}, e^{35} + e^{27} + e^{16}$        | 2579     |
| 9641:109  | $0, 0, 0, e^{12}, e^{13}, e^{14}, e^{24}, e^{23} + e^{15}, e^{35} + e^{17} + e^{26}$          | 2579     |
| 9641:110  | $0, 0, 0, e^{12}, e^{13}, e^{24}, e^{14} + e^{23}, e^{15}, e^{27} + e^{35} + e^{16}$          | 2579     |
| 9641:111  | $0, 0, 0, e^{12}, e^{13}, e^{24}, e^{23} + e^{14}, e^{25} + e^{34}, e^{27} + e^{16}$          | 2579     |
| 9641:112a | $0, 0, 0, e^{12}, e^{13}, e^{14}, e^{24}, e^{25} + e^{34}, e^{35} + e^{27} + e^{16}$          | 2579     |
| 9641:112b | $0, 0, 0, e^{12}, e^{13}, -e^{14}, e^{24}, e^{25} + e^{34}, e^{16} + e^{27} + e^{35}$         | 2579     |
| 9641:113  | $0, 0, 0, e^{12}, e^{13}, e^{14}, e^{24}, e^{25} + e^{34}, e^{17} + e^{26} + e^{35}$          | 2579     |
| 9641:114a | $0, 0, 0, -e^{12}, e^{13}, e^{24}, e^{14} + e^{23}, e^{35}, e^{26} + e^{34} + e^{17}$         | 2579     |
| 9641:114b | $0, 0, 0, -e^{12}, e^{13}, e^{24}, -e^{14} + e^{23}, e^{35}, e^{26} + e^{34} + e^{17}$        | 2579     |
| 9641:115a | $0, 0, 0, -e^{12}, e^{13}, e^{24}, e^{14} + e^{23}, e^{15}, e^{17} + e^{26} + e^{34}$         | 2579     |
| 9641:115b | $0, 0, 0, -e^{12}, e^{13}, e^{24}, -e^{14} + e^{23}, e^{15}, e^{17} + e^{34} + e^{26}$        | 2579     |
| 9641:116  | $0, 0, 0, e^{12}, e^{13}, e^{24}, e^{23} + e^{14}, e^{25} + e^{34}, e^{35} + e^{27} + e^{16}$ | 2579     |
| 9641:138  | $0, 0, 0, e^{12}, e^{13}, e^{24}, e^{15}, e^{14}, e^{17} + e^{26}$                            | 2469     |
| 9641:139  | $0, 0, 0, e^{12}, e^{13}, e^{14}, e^{35}, e^{24}, e^{37} + e^{16}$                            | 2469     |
| 9641:140  | $0, 0, 0, e^{12}, e^{13}, e^{24}, e^{35}, e^{14}, e^{37} + e^{26}$                            | 2469     |
| 9641:141  | $0, 0, 0, e^{12}, e^{13}, e^{24}, e^{15}, e^{14} + e^{23}, e^{26} + e^{17}$                   | 2469     |
| 9641:142  | $0, 0, 0, e^{12}, e^{13}, e^{24}, e^{35}, e^{23} + e^{14}, e^{26} + e^{37}$                   | 2469     |
| 9641:143  | $0, 0, 0, e^{12}, e^{13}, e^{24}, e^{15}, e^{35} + e^{14}, e^{17} + e^{26}$                   | 2469     |
| 9641:144  | $0, 0, 0, e^{12}, e^{13}, e^{24}, e^{15}, e^{25} + e^{34}, e^{17} + e^{26}$                   | 2469     |
| 9641:145  | $0, 0, 0, e^{12}, e^{13}, e^{24}, e^{35}, e^{34} + e^{25}, e^{26} + e^{37}$                   | 2469     |
| 9641:146  | $0, 0, 0, e^{12}, e^{13}, e^{24}, e^{25} + e^{34}, e^{14}, e^{36} + e^{27}$                   | 2469     |
| 9641:147  | $0, 0, 0, e^{12}, e^{13}, e^{14}, e^{15} + e^{24}, e^{35}, e^{17} + e^{26}$                   | 2469     |
| 9641:148  | $0, 0, 0, e^{12}, e^{13}, e^{24}, e^{34} + e^{25}, e^{15}, e^{27} + e^{36}$                   | 2469     |
| 9641:149  | $0, 0, 0, e^{12}, e^{13}, e^{24}, e^{34} + e^{25}, e^{35}, e^{27} + e^{36}$                   | 2469     |
| 9641:150  | $0, 0, 0, e^{12}, e^{13}, e^{24}, e^{15}, e^{14}, e^{35} + e^{26} + e^{17}$                   | 2469     |
| 9641:151  | $0, 0, 0, e^{12}, e^{13}, e^{24}, e^{35}, e^{14}, e^{37} + e^{15} + e^{26}$                   | 2469     |
| 9641:152  | $0, 0, 0, -e^{12}, e^{13}, e^{14}, e^{15}, e^{24}, e^{27} + e^{45} + e^{36}$                  | 2469     |
| 9641:153  | $0, 0, 0, e^{12}, e^{13}, e^{24}, e^{25} + e^{34}, e^{14} + e^{23}, e^{36} + e^{27}$          | 2469     |
| 9641:154  | $0, 0, 0, e^{12}, e^{13}, e^{24}, e^{25} + e^{34}, e^{15} + e^{23}, e^{36} + e^{27}$          | 2469     |
| 9641:155  | $0, 0, 0, e^{12}, e^{13}, e^{14}, e^{15} + e^{24}, e^{25} + e^{34}, e^{17} + e^{26}$          | 2469     |
| 9641:156  | $0, 0, 0, e^{12}, e^{13}, e^{24}, e^{25} + e^{34}, e^{35} + e^{14}, e^{36} + e^{27}$          | 2469     |
| 9641:157  | $0, 0, 0, e^{12}, e^{13}, e^{14} + e^{23}, e^{15} + e^{24}, e^{35}, e^{17} + e^{26}$          | 2469     |
| 9641:158a | $0, 0, 0, e^{12}, e^{13}, e^{34} + e^{25}, e^{35} + e^{24}, e^{14}, e^{26} + e^{37}$          | 2469     |
| 9641:158b | $0, 0, 0, -e^{12}, e^{13}, -e^{25} + e^{34}, e^{35} + e^{24}, e^{14}, e^{26} + e^{37}$        | 2469     |
| 9641:159a | $0, 0, 0, e^{12}, e^{13}, e^{35} + e^{24}, e^{34} + e^{25}, e^{14}, e^{26} + e^{37}$          | 2469     |
| 9641:159b | $0, 0, 0, e^{12}, e^{13}, e^{35} - e^{24}, e^{34} + e^{25}, e^{14}, e^{26} + e^{37}$          | 2469     |
| 9641:160  | $0, 0, 0, a_1 e^{12}, e^{13}, e^{24}, e^{15}, e^{14} + e^{23}, e^{17} + e^{35} + e^{26}$      | 2469     |
| 9641:161  | $0, 0, 0, e^{12}, e^{13}, e^{24}, e^{35}, e^{14} + e^{23}, e^{37} + e^{26} + e^{15}$          | 2469     |
| 9641:162  | $0, 0, 0, e^{12}, e^{13}, e^{14}, e^{35}, e^{25} + e^{34}, e^{37} + e^{16} + e^{24}$          | 2469     |
| 9641:163  | $0, 0, 0, e^{12}, e^{13}, e^{24}, e^{35}, e^{25} + e^{34}, e^{26} + e^{37} + e^{14}$          | 2469     |
| 9641:164  | $0, 0, 0, -e^{12}, e^{13}, e^{24}, e^{15} + e^{23}, e^{14}, e^{17} + e^{34} + e^{26}$         | 2469     |
| 9641:165  | $0, 0, 0, e^{12}, e^{13}, e^{23} + e^{14}, e^{35}, e^{24}, e^{37} + e^{16} + e^{25}$          | 2469     |
| 9641:166a | $0, 0, 0, -e^{12}, e^{13}, e^{14}, e^{15}, e^{35} + e^{24}, e^{27} + e^{36} + e^{45}$         | 2469     |
| 9641:166b | $0, 0, 0, -e^{12}, -e^{13}, -e^{14}, e^{15}, e^{35} + e^{24}, e^{27} + e^{36} + e^{45}$       | 2469     |
| 9641:167  | $0, 0, 0, -e^{12}, -e^{13}, -e^{14}, e^{15}, e^{25} + e^{34}, e^{36} + e^{27} + e^{45}$       | 2469     |
| 9641:168  | $0, 0, 0, e^{12}, e^{13}, e^{24}, e^{34} + e^{25}, e^{14}, e^{36} + e^{27} + e^{15}$          | 2469     |
| 9641:169  | $0, 0, 0, e^{12}, e^{13}, e^{24}, e^{34} + e^{25}, e^{15}, e^{27} + e^{36} + e^{14}$          | 2469     |
| 9641:170  | $0, 0, 0, e^{12}, e^{13}, e^{24}, e^{34} + e^{25}, e^{35}, e^{36} + e^{27} + e^{14}$          | 2469     |
| 9641:171  | $0, 0, 0, e^{12}, e^{13}, e^{24}, e^{25} + e^{34}, e^{35}, e^{15} + e^{27} + e^{36}$          | 2469     |
| 9641:172  | $0, 0, 0, -e^{12}, e^{13}, e^{14}, e^{23} + e^{15}, e^{24}, e^{27} + e^{36} + e^{45}$         | 2469     |
| 9641:173  | $0, 0, 0, -e^{12}, e^{13}, e^{14} + e^{23}, e^{15}, e^{24}, e^{27} + e^{36} + e^{45}$         | 2469     |
| 9641:175  | $0, 0, 0, e^{12}, e^{13}, 2e^{14}, e^{25} + e^{34}, e^{24}, e^{17} + e^{45} + e^{36}$         | 2469     |

Table 2 – Continued to next page

Table 2 – Continued from previous page

| Name      | $\mathfrak{g}$                                                                                              | UCS Dim. |
|-----------|-------------------------------------------------------------------------------------------------------------|----------|
| 9641:176  | $0, 0, 0, -e^{12}, e^{13}, e^{14}, e^{15} + e^{24}, e^{35}, e^{27} + e^{36} + e^{45}$                       | 2469     |
| 9641:178  | $0, 0, 0, e^{12}, e^{13}, 2e^{14}, e^{25} + e^{34}, e^{15}, e^{17} + e^{45} + e^{36}$                       | 2469     |
| 9641:180  | $0, 0, 0, e^{12}, e^{13}, 2e^{14}, e^{25} + e^{34}, e^{35}, e^{17} + e^{45} + e^{36}$                       | 2469     |
| 9641:181  | $0, 0, 0, e^{12}, e^{13}, e^{14} + e^{23}, e^{15} + e^{24}, e^{34} + e^{25}, e^{17} + e^{26}$               | 2469     |
| 9641:182a | $0, 0, 0, e^{12}, e^{13}, e^{34} + e^{25}, e^{35} + e^{24}, e^{14} + e^{23}, e^{26} + e^{27}$               | 2469     |
| 9641:182b | $0, 0, 0, -e^{12}, e^{13}, e^{34} - e^{25}, e^{35} + e^{24}, e^{14} + e^{23}, e^{26} + e^{37}$              | 2469     |
| 9641:183a | $0, 0, 0, e^{12}, e^{13}, e^{24} + e^{35}, e^{25} + e^{34}, e^{14} + e^{23}, e^{37} + e^{26}$               | 2469     |
| 9641:183b | $0, 0, 0, e^{12}, e^{13}, -e^{24} + e^{35}, e^{25} + e^{34}, e^{14} + e^{23}, e^{26} + e^{37}$              | 2469     |
| 9641:184  | $0, 0, 0, -e^{12}, e^{13}, e^{24}, e^{15} + e^{23}, e^{14} + e^{35}, e^{26} + e^{34} + e^{17}$              | 2469     |
| 9641:185  | $0, 0, 0, e^{12}, e^{13}, e^{24}, e^{25} + e^{34}, e^{23} + e^{14}, e^{15} + e^{27} + e^{36}$               | 2469     |
| 9641:186  | $0, 0, 0, e^{12}, e^{13}, e^{24}, e^{25} + e^{34}, e^{23} + e^{15}, e^{36} + e^{14} + e^{27}$               | 2469     |
| 9641:187  | $0, 0, 0, e^{12}, e^{13}, e^{14}, e^{15} + e^{24}, e^{25} + e^{34}, e^{17} + e^{26} + e^{35}$               | 2469     |
| 9641:188  | $0, 0, 0, e^{12}, e^{13}, e^{24}, e^{25} + e^{34}, e^{35} + e^{14}, e^{36} + e^{15} + e^{27}$               | 2469     |
| 9641:189a | $0, 0, 0, -e^{12}, e^{13}, e^{14}, e^{15} + e^{23}, e^{24} + e^{35}, e^{45} + e^{36} + e^{27}$              | 2469     |
| 9641:189b | $0, 0, 0, -e^{12}, -e^{13}, -e^{14}, e^{23} + e^{15}, e^{35} + e^{24}, e^{27} + e^{36} + e^{45}$            | 2469     |
| 9641:190  | $0, 0, 0, -e^{12}, -e^{13}, -e^{14}, e^{15} + e^{23}, e^{34} + e^{25}, e^{27} + e^{36} + e^{45}$            | 2469     |
| 9641:193  | $0, 0, 0, e^{12}, e^{13}, 2e^{14}, e^{25} + e^{34}, e^{15} + e^{23}, e^{17} + e^{36} + e^{45}$              | 2469     |
| 9641:194  | $0, 0, 0, -e^{12}, -e^{13}, -e^{14}, e^{24} + e^{15}, e^{34} + e^{25}, e^{27} + e^{36} + e^{45}$            | 2469     |
| 9641:195  | $0, 0, 0, e^{12}, e^{13}, 2e^{14}, e^{25} + e^{34}, e^{15} + e^{24}, e^{17} + e^{36} + e^{45}$              | 2469     |
| 9641:197a | $0, 0, 0, e^{12}, e^{13}, 2e^{14}, e^{25} + e^{34}, e^{35} + e^{24}, e^{36} + e^{45} + e^{17}$              | 2469     |
| 9641:197b | $0, 0, 0, -e^{12}, e^{13}, 2e^{14}, -e^{25} + e^{34}, e^{35} + e^{24}, e^{17} + e^{36} + e^{45}$            | 2469     |
| 9641:198a | $0, 0, 0, e^{12}, e^{13}, e^{25} + e^{34}, e^{35} + e^{24}, e^{14}, e^{37} + e^{15} + e^{26}$               | 2469     |
| 9641:198b | $0, 0, 0, -e^{12}, e^{13}, -e^{25} + e^{34}, e^{24} + e^{35}, e^{14}, e^{15} + e^{37} + e^{26}$             | 2469     |
| 9641:199a | $0, 0, 0, e^{12}, e^{13}, e^{25} + e^{34}, e^{35} + e^{24}, e^{14}, e^{36} + e^{15} + e^{27}$               | 2469     |
| 9641:199b | $0, 0, 0, e^{12}, e^{13}, e^{25} + e^{34}, e^{35} - e^{24}, e^{14}, e^{15} + e^{27} + e^{36}$               | 2469     |
| 9641:200  | $0, 0, 0, e^{12}, e^{13}, e^{23} + 2e^{14}, e^{25} + e^{34}, e^{24}, e^{36} + e^{45} + e^{17}$              | 2469     |
| 9641:201  | $0, 0, 0, -e^{12}, e^{13}, e^{14} + e^{23}, e^{24} + e^{15}, e^{35}, e^{36} + e^{27} + e^{45}$              | 2469     |
| 9641:202  | $0, 0, 0, e^{12}, e^{13}, e^{23} + 2e^{14}, e^{25} + e^{34}, e^{15}, e^{17} + e^{36} + e^{45}$              | 2469     |
| 9641:203  | $0, 0, 0, e^{12}, e^{13}, e^{23} + 2e^{14}, e^{25} + e^{34}, e^{35}, e^{17} + e^{36} + e^{45}$              | 2469     |
| 9641:204  | $0, 0, 0, -e^{12}, -e^{13}, e^{24} + 2e^{15}, e^{34} + e^{25}, e^{14}, e^{26} + e^{45} + e^{17}$            | 2469     |
| 9641:205  | $0, 0, 0, e^{12}, e^{13}, e^{35} + 2e^{14}, e^{25} + e^{34}, e^{24}, e^{17} + e^{36} + e^{45}$              | 2469     |
| 9641:206  | $0, 0, 0, e^{12}, e^{13}, a_2, e^{23} + e^{14}, e^{15} + e^{24}, e^{25} + e^{34}, e^{17} + e^{26} + e^{35}$ | 2469     |
| 9641:207a | $0, 0, 0, e^{12}, e^{13}, e^{25} + e^{34}, e^{35} + e^{24}, e^{23} + e^{14}, e^{15} + e^{26} + e^{37}$      | 2469     |
| 9641:207b | $0, 0, 0, -e^{12}, e^{13}, -e^{25} + e^{34}, e^{24} + e^{35}, e^{14} + e^{23}, e^{37} + e^{26} + e^{15}$    | 2469     |
| 9641:208a | $0, 0, 0, e^{12}, e^{13}, e^{25} + e^{34}, e^{35} + e^{24}, e^{23} + e^{14}, e^{15} + e^{27} + e^{36}$      | 2469     |
| 9641:208b | $0, 0, 0, e^{12}, e^{13}, e^{25} + e^{34}, e^{35} - e^{24}, e^{23} + e^{14}, e^{36} + e^{15} + e^{27}$      | 2469     |
| 9641:209  | $0, 0, 0, -e^{12}, -e^{13}, -e^{14} + e^{23}, e^{15} + e^{24}, e^{34} + e^{25}, e^{27} + e^{36} + e^{45}$   | 2469     |
| 9641:210  | $0, 0, 0, e^{12}, e^{13}, e^{23} + 2e^{14}, e^{25} + e^{34}, e^{15} + e^{24}, e^{17} + e^{36} + e^{45}$     | 2469     |
| 9641:211a | $0, 0, 0, e^{12}, e^{13}, e^{23} + 2e^{14}, e^{25} + e^{34}, e^{35} + e^{24}, e^{17} + e^{36} + e^{45}$     | 2469     |
| 9641:211b | $0, 0, 0, -e^{12}, e^{13}, e^{23} + 2e^{14}, -e^{25} + e^{34}, e^{35} + e^{24}, e^{36} + e^{45} + e^{17}$   | 2469     |
| 9641:212  | $0, 0, 0, -e^{12}, -e^{13}, 2e^{15} + e^{24}, e^{34} + e^{25}, e^{14} + e^{23}, e^{17} + e^{26} + e^{45}$   | 2469     |
| 9641:213  | $0, 0, 0, -e^{12}, -e^{13}, 2e^{15} + e^{24}, e^{34} + e^{25}, e^{14} + e^{35}, e^{17} + e^{26} + e^{45}$   | 2469     |
| 9641:214  | $0, 0, 0, e^{12}, e^{13}, -e^{15} + e^{24}, e^{14} + e^{35}, e^{34} + e^{25}, e^{26} + e^{37} + e^{45}$     | 2469     |
| 9641:215a | $0, 0, 0, e^{12}, e^{13}, e^{14}, e^{24}, e^{35}, e^{27} + e^{38} + e^{16}$                                 | 1469     |
| 9641:215b | $0, 0, 0, e^{12}, e^{13}, -e^{14}, e^{24}, e^{35}, e^{38} + e^{27} + e^{16}$                                | 1469     |
| 9641:216  | $0, 0, 0, e^{12}, e^{13}, e^{14}, e^{24}, e^{35}, e^{17} + e^{26} + e^{38}$                                 | 1469     |
| 9641:217  | $0, 0, 0, e^{12}, e^{13}, e^{24}, e^{14} + e^{23}, e^{35}, e^{27} + e^{16} + e^{38}$                        | 1469     |
| 9641:218  | $0, 0, 0, e^{12}, e^{13}, e^{14}, e^{24}, e^{25} + e^{34}, e^{37} + e^{16} + e^{28}$                        | 1469     |
| 9641:219a | $0, 0, 0, e^{12}, e^{13}, e^{14}, e^{15}, e^{35} + e^{24}, e^{18} + e^{26} + e^{37}$                        | 1469     |
| 9641:219b | $0, 0, 0, -e^{12}, e^{13}, e^{14}, e^{15}, e^{35} + e^{24}, e^{26} + e^{37} + e^{18}$                       | 1469     |
| 9641:220  | $0, 0, 0, e^{12}, e^{13}, e^{14}, e^{15}, e^{34} + e^{25}, e^{18} + e^{27} + e^{36}$                        | 1469     |
| 9641:221a | $0, 0, 0, e^{12}, e^{13}, e^{24}, e^{15}, e^{35} + e^{14}, e^{37} + e^{18} + e^{26}$                        | 1469     |
| 9641:221b | $0, 0, 0, e^{12}, e^{13}, e^{24}, e^{15}, -e^{14} + e^{35}, e^{37} + e^{26} + e^{18}$                       | 1469     |
| 9641:222a | $0, 0, 0, e^{12}, e^{13}, e^{24}, e^{15}, e^{25} + e^{34}, e^{28} + e^{17} + e^{36}$                        | 1469     |
| 9641:222b | $0, 0, 0, e^{12}, e^{13}, e^{24}, -e^{15}, e^{25} + e^{34}, e^{36} + e^{28} + e^{17}$                       | 1469     |
| 9641:223a | $0, 0, 0, e^{12}, e^{13}, e^{14}, e^{15} + e^{23}, e^{35} + e^{24}, e^{18} + e^{26} + e^{37}$               | 1469     |
| 9641:223b | $0, 0, 0, -e^{12}, e^{13}, e^{14}, e^{23} + e^{15}, e^{35} + e^{24}, e^{37} + e^{18} + e^{26}$              | 1469     |
| 9641:224  | $0, 0, 0, e^{12}, e^{13}, e^{14}, e^{15} + e^{23}, e^{25} + e^{34}, e^{27} + e^{18} + e^{36}$               | 1469     |

Table 2 – Continued to next page

Table 2 – Continued from previous page

| Name       | $\mathfrak{g}$                                                                                                                            | UCS Dim. |
|------------|-------------------------------------------------------------------------------------------------------------------------------------------|----------|
| 9641:225a  | $0, 0, 0, e^{12}, e^{13}, e^{24}, e^{15} + e^{23}, e^{35} + e^{14}, e^{18} + e^{26} + e^{37}$                                             | 1469     |
| 9641:225b  | $0, 0, 0, e^{12}, e^{13}, e^{24}, e^{15} + e^{23}, e^{35} - e^{14}, e^{37} + e^{18} + e^{26}$                                             | 1469     |
| 9641:226   | $0, 0, 0, e^{12}, e^{13}, e^{14}, e^{24} + e^{15}, e^{25} + e^{34}, e^{36} + e^{27} + e^{18}$                                             | 1469     |
| 9641:227a  | $0, 0, 0, e^{12}, e^{13}, e^{14}, e^{25} + e^{34}, e^{35} + e^{24}, e^{38} + e^{27} + e^{16}$                                             | 1469     |
| 9641:227b  | $0, 0, 0, -e^{12}, e^{13}, e^{14}, -e^{25} + e^{34}, e^{24} + e^{35}, e^{16} + e^{38} + e^{27}$                                           | 1469     |
| 9641:228a  | $0, 0, 0, e^{12}, e^{13}, e^{14}, e^{25} + e^{34}, e^{35} + e^{24}, e^{37} + e^{16} + e^{28}$                                             | 1469     |
| 9641:228b  | $0, 0, 0, e^{12}, e^{13}, e^{14}, e^{25} + e^{34}, e^{35} - e^{24}, e^{16} + e^{28} + e^{37}$                                             | 1469     |
| 9641:228c  | $0, 0, 0, e^{12}, e^{13}, -e^{14}, e^{25} + e^{34}, e^{35} + e^{24}, e^{37} + e^{16} + e^{28}$                                            | 1469     |
| 9641:228d  | $0, 0, 0, e^{12}, e^{13}, -e^{14}, e^{25} + e^{34}, e^{35} - e^{24}, e^{16} + e^{28} + e^{37}$                                            | 1469     |
| 9641:229   | $0, 0, 0, e^{12}, e^{13}, e^{24}, e^{35} + e^{14}, e^{25} + e^{34}, e^{38} + e^{27} + e^{16}$                                             | 1469     |
| 9641:230   | $0, 0, 0, e^{12}, e^{13}, 2e^{14}, e^{24}, e^{25} + e^{34}, e^{36} + e^{45} + e^{27} + e^{18}$                                            | 1469     |
| 9641:231   | $0, 0, 0, e^{12}a_2, e^{13}a_2, (1 + a_2)e^{14}, -(-1 + a_2)e^{15}, e^{25} + e^{34}, e^{36} + e^{45} + e^{27} + e^{18}$                   | 1469     |
| 9641:233   | $0, 0, 0, e^{12}, e^{13}, e^{14} + e^{23}, e^{15} + e^{24}, e^{25} + e^{34}, e^{36} + e^{18} + e^{27}$                                    | 1469     |
| 9641:234   | $0, 0, 0, e^{12}, e^{13}, e^{15} + e^{24}, e^{14} + e^{35}, e^{25} + e^{34}, e^{16} + e^{38} + e^{27}$                                    | 1469     |
| 9641:235   | $0, 0, 0, e^{12}, e^{13}, e^{15} + e^{24}, e^{14} + e^{35}, e^{25} + e^{34}, e^{37} + e^{18} + e^{26}$                                    | 1469     |
| 9641:236   | $0, 0, 0, e^{12}, e^{13}, e^{24}, e^{23} + 2e^{14}, e^{34} + e^{25}, e^{18} + e^{26} + e^{37} + e^{45}$                                   | 1469     |
| 9641:237   | $0, 0, 0, (-1 + a_3)e^{12}, (-1 + a_3)e^{13}, e^{14}a_3, -e^{15}(-2 + a_3) + e^{23}, e^{34} + e^{25}, e^{27} + e^{36} + e^{45} + e^{18}$  | 1469     |
| 9641:238   | $0, 0, 0, e^{12}a_1, e^{13}a_1, (1 + a_1)e^{14}, -(-1 + a_1)e^{15} + e^{24}, e^{34} + e^{25}, e^{27} + e^{36} + e^{45} + e^{18}$          | 1469     |
| 9641:239   | $0, 0, 0, e^{12}, e^{13}, e^{24}, 2e^{14} + e^{35}, e^{34} + e^{25}, e^{26} + e^{37} + e^{45} + e^{18}$                                   | 1469     |
| 9641:240   | $0, 0, 0, e^{12}a_1, e^{13}a_1, e^{14}(1 + a_1) + e^{23}, -(-1 + a_1)e^{15} + e^{24}, e^{34} + e^{25}, e^{18} + e^{27} + e^{36} + e^{45}$ | 1469     |
| 9641:241   | $0, 0, 0, e^{12}a_2, e^{13}a_2, -(-1 + a_2)e^{15} + e^{24}, (1 + a_2)e^{14} + e^{35}, e^{34} + e^{25}, e^{18} + e^{26} + e^{37} + e^{45}$ | 1469     |
| Type: 3321 |                                                                                                                                           |          |
| 9631:1     | $0, 0, 0, e^{12}, e^{13}, e^{23}, e^{14}, e^{24}, e^{17}$                                                                                 | 4679     |
| 9631:2     | $0, 0, 0, e^{12}, e^{13}, e^{23}, e^{14}, e^{35}, e^{17}$                                                                                 | 3579     |
| 9631:3     | $0, 0, 0, e^{12}, e^{13}, e^{23}, e^{24}, e^{35}, e^{27}$                                                                                 | 3579     |
| 9631:4     | $0, 0, 0, e^{12}, e^{13}, e^{23}, e^{14}, e^{15}, e^{17}$                                                                                 | 3579     |
| 9631:5     | $0, 0, 0, e^{12}, e^{13}, e^{23}, e^{24}, e^{15}, e^{27}$                                                                                 | 3579     |
| 9631:6a    | $0, 0, 0, e^{12}, e^{13}, e^{23}, e^{14}, e^{35} + e^{24}, e^{17}$                                                                        | 3579     |
| 9631:6b    | $0, 0, 0, -e^{12}, e^{13}, e^{23}, e^{14}, e^{35} + e^{24}, e^{17}$                                                                       | 3579     |
| 9631:7     | $0, 0, 0, e^{12}, e^{13}, e^{23}, e^{14}, e^{25} + e^{34}, e^{17}$                                                                        | 3579     |
| 9631:8     | $0, 0, 0, e^{12}, e^{13}, e^{23}, e^{24}, e^{35} + e^{14}, e^{27}$                                                                        | 3579     |
| 9631:9     | $0, 0, 0, e^{12}, e^{13}, e^{23}, e^{24}, e^{34} + e^{25}, e^{27}$                                                                        | 3579     |
| 9631:10    | $0, 0, 0, e^{12}, e^{13}, e^{23}, e^{14}, e^{15}, e^{35} + e^{17}$                                                                        | 3579     |
| 9631:11    | $0, 0, 0, e^{12}, e^{13}, e^{23}, e^{24}, e^{15}, e^{27} + e^{35}$                                                                        | 3579     |
| 9631:12    | $0, 0, 0, e^{12}, e^{13}, e^{23}, e^{24}, e^{35}, e^{27} + e^{15}$                                                                        | 3579     |
| 9631:13    | $0, 0, 0, e^{12}, e^{13}, e^{23}, e^{14}, e^{15} + e^{36}, e^{17}$                                                                        | 2579     |
| 9631:14    | $0, 0, 0, e^{12}, e^{13}, e^{23}, e^{14}, e^{26} + e^{35}, e^{17}$                                                                        | 2579     |
| 9631:15    | $0, 0, 0, e^{12}, e^{13}, e^{23}, e^{14}, e^{35}, e^{17} + e^{36}$                                                                        | 2579     |
| 9631:16    | $0, 0, 0, e^{12}, e^{13}, e^{23}, e^{24}, e^{35}, e^{27} + e^{36}$                                                                        | 2579     |
| 9631:17    | $0, 0, 0, e^{12}, e^{13}, e^{23}, e^{14}, e^{24} + e^{15}, e^{17}$                                                                        | 3579     |
| 9631:18a   | $0, 0, 0, e^{12}, e^{13}, e^{23}, e^{14}, e^{26} + e^{15}, e^{17}$                                                                        | 2579     |
| 9631:18b   | $0, 0, 0, e^{12}, -e^{13}, e^{23}, e^{14}, e^{26} + e^{15}, e^{17}$                                                                       | 2579     |
| 9631:19    | $0, 0, 0, e^{12}, e^{13}, e^{23}, e^{14}, e^{16} + e^{25}, e^{17}$                                                                        | 2579     |
| 9631:20    | $0, 0, 0, e^{12}, e^{13}, e^{23}, e^{14}, e^{24}, e^{17} + e^{35}$                                                                        | 3579     |
| 9631:21    | $0, 0, 0, e^{12}, e^{13}, e^{23}, e^{24}, e^{14}, e^{27} + e^{35}$                                                                        | 3579     |
| 9631:22    | $0, 0, 0, e^{12}, e^{13}, e^{23}, e^{14}, e^{35}, e^{24} + e^{17}$                                                                        | 3579     |
| 9631:23    | $0, 0, 0, e^{12}, e^{13}, e^{23}, e^{24}, e^{35}, e^{14} + e^{27}$                                                                        | 3579     |
| 9631:24    | $0, 0, 0, e^{12}, e^{13}, e^{23}, e^{14}, e^{15}, e^{36} + e^{17}$                                                                        | 2579     |
| 9631:25    | $0, 0, 0, e^{12}, e^{13}, e^{23}, e^{24}, e^{15}, e^{27} + e^{36}$                                                                        | 2579     |
| 9631:26    | $0, 0, 0, e^{12}, e^{13}, e^{23}, e^{14}, e^{35}, e^{17} + e^{26}$                                                                        | 2579     |
| 9631:27    | $0, 0, 0, e^{12}, e^{13}, e^{23}, e^{14}, e^{25} + e^{34}, e^{17} + e^{35}$                                                               | 3579     |
| 9631:28    | $0, 0, 0, e^{12}, e^{13}, e^{23}, e^{24}, e^{34} + e^{25}, e^{35} + e^{27}$                                                               | 3579     |
| 9631:29    | $0, 0, 0, e^{12}, e^{13}, e^{23}, e^{14}, e^{36} + e^{15}, e^{35} + e^{17}$                                                               | 2579     |
| 9631:30    | $0, 0, 0, e^{12}, e^{13}, e^{23}, e^{24}, e^{36} + e^{15}, e^{27} + e^{35}$                                                               | 2579     |
| 9631:31    | $0, 0, 0, e^{12}, e^{13}, e^{23}, e^{24}, e^{14}, e^{27} + e^{15}$                                                                        | 3579     |
| 9631:32    | $0, 0, 0, e^{12}, e^{13}, e^{23}, e^{14}, e^{15}, e^{24} + e^{17}$                                                                        | 3579     |
| 9631:33    | $0, 0, 0, e^{12}, e^{13}, e^{23}, e^{24}, e^{15}, e^{27} + e^{14}$                                                                        | 3579     |
| 9631:34    | $0, 0, 0, e^{12}, e^{13}, e^{23}, e^{14}, e^{15}, e^{17} + e^{26}$                                                                        | 2579     |

Table 2 – Continued to next page

Table 2 – Continued from previous page

| Name     | $\mathfrak{g}$                                                                                    | UCS Dim. |
|----------|---------------------------------------------------------------------------------------------------|----------|
| 9631:35  | $0, 0, 0, e^{12}, e^{13}, e^{23}, e^{14}, e^{15} + e^{24}, e^{35} + e^{17}$                       | 3579     |
| 9631:36  | $0, 0, 0, e^{12}, e^{13}, e^{23}, e^{24}, e^{14} + e^{35}, e^{15} + e^{27}$                       | 3579     |
| 9631:37  | $0, 0, 0, e^{12}, e^{13}, e^{23}, e^{24}, e^{25} + e^{34}, e^{15} + e^{27}$                       | 3579     |
| 9631:38  | $0, 0, 0, e^{12}, e^{13}, e^{23}, e^{14}, e^{15} + e^{24} + e^{36}, e^{17}$                       | 2579     |
| 9631:39  | $0, 0, 0, e^{12}(-1 + a_2), a_2 e^{13}, e^{23}, e^{14}, e^{16} + e^{34} + e^{25}, e^{17}$         | 2579     |
| 9631:40a | $0, 0, 0, e^{12}, e^{13}, e^{23}, e^{14}, e^{26} + e^{15}, e^{35} + e^{17}$                       | 2579     |
| 9631:40b | $0, 0, 0, e^{12}, -e^{13}, e^{23}, e^{14}, e^{15} + e^{26}, e^{35} + e^{17}$                      | 2579     |
| 9631:41  | $0, 0, 0, e^{12}, e^{13}, e^{23}, e^{14}, e^{25} + e^{16}, e^{35} + e^{17}$                       | 2579     |
| 9631:42a | $0, 0, 0, e^{12}, e^{13}, e^{23}, e^{24}, e^{26} + e^{15}, e^{27} + e^{35}$                       | 2579     |
| 9631:42b | $0, 0, 0, e^{12}, -e^{13}, e^{23}, e^{24}, e^{15} + e^{26}, e^{27} + e^{35}$                      | 2579     |
| 9631:43  | $0, 0, 0, e^{12}, e^{13}, e^{23}, e^{24}, e^{16} + e^{25}, e^{27} + e^{35}$                       | 2579     |
| 9631:44  | $0, 0, 0, e^{12}, e^{13}, e^{23}, e^{24}, e^{35} + e^{26}, e^{27} + e^{15}$                       | 2579     |
| 9631:45  | $0, 0, 0, e^{12}, e^{13}, e^{23}, e^{14}, e^{35}, e^{17} + e^{25} + e^{34}$                       | 3579     |
| 9631:46  | $0, 0, 0, e^{12}, e^{13}, e^{23}, e^{24}, e^{35}, e^{15} + e^{27} + e^{36}$                       | 2579     |
| 9631:47a | $0, 0, 0, e^{12}, e^{13}, e^{23}, e^{14}, e^{35} + e^{24}, e^{17} + e^{36}$                       | 2579     |
| 9631:47b | $0, 0, 0, -e^{12}, e^{13}, e^{23}, e^{14}, e^{35} + e^{24}, e^{17} + e^{36}$                      | 2579     |
| 9631:48  | $0, 0, 0, e^{12}, e^{13}, e^{23}, e^{14}, e^{25} + e^{34}, e^{17} + e^{36}$                       | 2579     |
| 9631:49  | $0, 0, 0, e^{12}, e^{13}, e^{23}, e^{24}, e^{35} + e^{14}, e^{27} + e^{36}$                       | 2579     |
| 9631:50  | $0, 0, 0, e^{12}, e^{13}, e^{23}, e^{24}, e^{25} + e^{34}, e^{36} + e^{27}$                       | 2579     |
| 9631:51  | $0, 0, 0, e^{12}, e^{13}, e^{23}, e^{24}, e^{25} + e^{16}, e^{27} + e^{15}$                       | 2579     |
| 9631:52a | $0, 0, 0, e^{12}, e^{13}, e^{23}, e^{14}, e^{15}, e^{17} + e^{35} + e^{24}$                       | 3579     |
| 9631:52b | $0, 0, 0, -e^{12}, e^{13}, e^{23}, e^{14}, e^{15}, e^{17} + e^{24} + e^{35}$                      | 3579     |
| 9631:53  | $0, 0, 0, e^{12}, e^{13}, e^{23}, e^{14}, e^{15}, e^{17} + e^{25} + e^{34}$                       | 3579     |
| 9631:54  | $0, 0, 0, e^{12}, e^{13}, e^{23}, e^{24}, e^{15}, e^{35} + e^{14} + e^{27}$                       | 3579     |
| 9631:55  | $0, 0, 0, e^{12}, e^{13}, e^{23}, e^{14}, e^{25} + e^{34}, e^{24} + e^{17}$                       | 3579     |
| 9631:56  | $0, 0, 0, e^{12}, e^{13}, e^{23}, e^{24}, e^{34} + e^{25}, e^{27} + e^{14}$                       | 2579     |
| 9631:57  | $0, 0, 0, e^{12}, e^{13}, e^{23}, e^{14}, e^{15}, e^{17} + e^{26} + e^{35}$                       | 2579     |
| 9631:58  | $0, 0, 0, e^{12}, e^{13}, e^{23}, e^{14}, e^{15} + e^{24}, e^{17} + e^{36}$                       | 2579     |
| 9631:59a | $0, 0, 0, e^{12}, e^{13}, e^{23}, e^{14}, e^{35} + e^{24}, e^{17} + e^{26}$                       | 2579     |
| 9631:59b | $0, 0, 0, -e^{12}, e^{13}, e^{23}, e^{14}, e^{35} + e^{24}, e^{17} + e^{26}$                      | 2579     |
| 9631:60  | $0, 0, 0, e^{12}, e^{13}, e^{23}, e^{14}, e^{25} + e^{34}, e^{26} + e^{17}$                       | 2579     |
| 9631:61  | $0, 0, 0, e^{12}, e^{13}, e^{23}, e^{14}, e^{15} + e^{36}, e^{24} + e^{17}$                       | 2579     |
| 9631:62  | $0, 0, 0, e^{12}, e^{13}, e^{23}, e^{14}, e^{26} + e^{35}, e^{17} + e^{24}$                       | 2579     |
| 9631:63  | $0, 0, 0, e^{12}, e^{13}, e^{23}, e^{14}, e^{35}, e^{17} + e^{24} + e^{36}$                       | 2579     |
| 9631:64a | $0, 0, 0, e^{12}, e^{13}, e^{23}, e^{24}, e^{35}, e^{27} + e^{14} + e^{36}$                       | 2579     |
| 9631:64b | $0, 0, 0, -e^{12}, e^{13}, e^{23}, e^{24}, e^{35}, e^{27} + e^{36} + e^{14}$                      | 2579     |
| 9631:65  | $0, 0, 0, -e^{12}, e^{13}, e^{23}, e^{24}, e^{35}, e^{34} + e^{27} + e^{16}$                      | 2579     |
| 9631:66  | $0, 0, 0, e^{12}, e^{13}, e^{23}, e^{14}, e^{15} + e^{36}, e^{26} + e^{17} + e^{35}$              | 2579     |
| 9631:67  | $0, 0, 0, e^{12}, e^{13}, e^{23}, e^{14}, e^{36} + e^{24} + e^{15}, e^{17} + e^{35}$              | 2579     |
| 9631:68  | $0, 0, 0, (-1 + a_2)e^{12}, e^{13}a_2, e^{23}, e^{14}, e^{16} + e^{25} + e^{34}, e^{17} + e^{35}$ | 2579     |
| 9631:69  | $0, 0, 0, e^{12}a_1, (1 + a_1)e^{13}, e^{23}, e^{24}, e^{16} + e^{25} + e^{34}, e^{35} + e^{27}$  | 2579     |
| 9631:70  | $0, 0, 0, e^{12}, e^{13}, e^{23}, e^{14}, e^{15} + e^{24}, e^{17} + e^{26}$                       | 2579     |
| 9631:71a | $0, 0, 0, e^{12}, e^{13}, e^{23}, e^{14}, e^{15} + e^{26}, e^{17} + e^{24}$                       | 2579     |
| 9631:71b | $0, 0, 0, e^{12}, -e^{13}, e^{23}, e^{14}, e^{26} + e^{15}, e^{17} + e^{24}$                      | 2579     |
| 9631:72  | $0, 0, 0, e^{12}, e^{13}, e^{23}, e^{14}, e^{16} + e^{25}, e^{17} + e^{24}$                       | 2579     |
| 9631:73  | $0, 0, 0, e^{12}, e^{13}, e^{23}, e^{14}, e^{24}, e^{25} + e^{34} + e^{17}$                       | 3579     |
| 9631:74  | $0, 0, 0, e^{12}, e^{13}, e^{23}, e^{14}, e^{24}, e^{17} + e^{26} + e^{35}$                       | 2579     |
| 9631:75  | $0, 0, 0, e^{12}, e^{13}, e^{23}, e^{14}, e^{15}, e^{17} + e^{36} + e^{24}$                       | 2579     |
| 9631:76a | $0, 0, 0, e^{12}, e^{13}, e^{23}, e^{24}, e^{15}, e^{14} + e^{36} + e^{27}$                       | 2579     |
| 9631:76b | $0, 0, 0, -e^{12}, e^{13}, e^{23}, e^{24}, e^{15}, e^{27} + e^{14} + e^{36}$                      | 2579     |
| 9631:77  | $0, 0, 0, -e^{12}, e^{13}, e^{23}, e^{24}, e^{15}, e^{27} + e^{16} + e^{34}$                      | 2579     |
| 9631:78  | $0, 0, 0, e^{12}, e^{13}, e^{23}, e^{14}, e^{25} + e^{16}, e^{26} + e^{35} + e^{17}$              | 2579     |
| 9631:79  | $0, 0, 0, e^{12}, e^{13}, e^{23}, e^{24}, e^{14} + e^{26} + e^{35}, e^{15} + e^{27}$              | 2579     |
| 9631:80  | $0, 0, 0, e^{12}a_1, e^{13}(1 + a_1), e^{23}, e^{24}, e^{16} + e^{25} + e^{34}, e^{15} + e^{27}$  | 2579     |
| 9631:81a | $0, 0, 0, e^{12}, e^{13}, e^{23}, e^{14}, e^{35} + e^{24}, e^{17} + e^{25} + e^{34}$              | 3579     |
| 9631:81b | $0, 0, 0, e^{12}, e^{13}, e^{23}, e^{14}, -e^{24} + e^{35}, e^{25} + e^{17} + e^{34}$             | 3579     |
| 9631:82a | $0, 0, 0, e^{12}, e^{13}, e^{23}, e^{14}, e^{25} + e^{34}, e^{17} + e^{35} + e^{24}$              | 3579     |
| 9631:82b | $0, 0, 0, -e^{12}, e^{13}, e^{23}, e^{14}, e^{34} - e^{25}, e^{35} + e^{24} + e^{17}$             | 3579     |

Table 2 – Continued to next page

Table 2 – Continued from previous page

| Name      | $\mathfrak{g}$                                                                                                 | UCS Dim. |
|-----------|----------------------------------------------------------------------------------------------------------------|----------|
| 9631:83   | $0, 0, 0, e^{12}, e^{13}, e^{23}, e^{24}, e^{25} + e^{34}, e^{35} + e^{14} + e^{27}$                           | 3579     |
| 9631:84   | $0, 0, 0, e^{12}, e^{13}, e^{23}, e^{14}, e^{34} + e^{25}, e^{17} + e^{35} + e^{26}$                           | 2579     |
| 9631:85   | $0, 0, 0, e^{12}, e^{13}, e^{23}, e^{24}, e^{35} + e^{14}, e^{15} + e^{27} + e^{36}$                           | 2579     |
| 9631:86   | $0, 0, 0, e^{12}, e^{13}, e^{23}, e^{24}, e^{25} + e^{34}, e^{15} + e^{36} + e^{27}$                           | 2579     |
| 9631:87a  | $0, 0, 0, e^{12}, e^{13}, e^{23}, e^{14}, e^{15} + e^{36}, e^{17} + e^{35} + e^{24}$                           | 2579     |
| 9631:87b  | $0, 0, 0, -e^{12}, e^{13}, e^{23}, e^{14}, e^{36} + e^{15}, e^{35} + e^{24} + e^{17}$                          | 2579     |
| 9631:88   | $0, 0, 0, e^{12}, e^{13}, e^{23}, e^{14}, e^{36} + e^{15}, e^{25} + e^{34} + e^{17}$                           | 2579     |
| 9631:89   | $0, 0, 0, e^{12}, e^{13}, e^{23}, e^{14}, e^{26} + e^{35}, e^{17} + e^{34} + e^{25}$                           | 2579     |
| 9631:90   | $0, 0, 0, e^{12}, e^{13}, e^{23}, e^{24}, e^{15} + e^{36}, e^{14} + e^{27} + e^{35}$                           | 2579     |
| 9631:91   | $0, 0, 0, e^{12}, e^{13}, e^{23}, e^{14}, e^{15} + e^{24}, e^{17} + e^{25} + e^{34}$                           | 3579     |
| 9631:92   | $0, 0, 0, a_1 e^{12}, e^{13}, e^{23}, e^{14}, e^{24} + e^{15}, e^{35} + e^{17} + e^{26}$                       | 2579     |
| 9631:93a  | $0, 0, 0, e^{12}, e^{13}, e^{23}, e^{14}, e^{26} + e^{15}, e^{17} + e^{35} + e^{24}$                           | 2579     |
| 9631:93b  | $0, 0, 0, e^{12}, -e^{13}, e^{23}, e^{14}, e^{26} + e^{15}, e^{35} + e^{24} + e^{17}$                          | 2579     |
| 9631:93c  | $0, 0, 0, -e^{12}, e^{13}, e^{23}, e^{14}, e^{15} + e^{26}, e^{17} + e^{35} + e^{24}$                          | 2579     |
| 9631:93d  | $0, 0, 0, -e^{12}, -e^{13}, e^{23}, e^{14}, e^{15} + e^{26}, e^{17} + e^{24} + e^{35}$                         | 2579     |
| 9631:94a  | $0, 0, 0, e^{12}, e^{13}, e^{23}, e^{14}, e^{26} + e^{15}, e^{17} + e^{25} + e^{34}$                           | 2579     |
| 9631:94b  | $0, 0, 0, -e^{12}, -e^{13}, e^{23}, e^{14}, e^{26} + e^{15}, e^{25} + e^{34} + e^{17}$                         | 2579     |
| 9631:95a  | $0, 0, 0, e^{12}, e^{13}, e^{23}, e^{14}, e^{25} + e^{16}, e^{24} + e^{17} + e^{35}$                           | 2579     |
| 9631:95b  | $0, 0, 0, -e^{12}, e^{13}, e^{23}, e^{14}, e^{16} + e^{25}, e^{17} + e^{35} + e^{24}$                          | 2579     |
| 9631:96a  | $0, 0, 0, e^{12}, e^{13}, e^{23}, e^{24}, e^{26} + e^{15}, e^{35} + e^{27} + e^{14}$                           | 2579     |
| 9631:96b  | $0, 0, 0, e^{12}, -e^{13}, e^{23}, e^{24}, e^{15} + e^{26}, e^{14} + e^{35} + e^{27}$                          | 2579     |
| 9631:97   | $0, 0, 0, e^{12}, e^{13}, e^{23}, e^{24}, e^{16} + e^{25}, e^{35} + e^{14} + e^{27}$                           | 2579     |
| 9631:98   | $0, 0, 0, (-1 + a_2) e^{12}, a_2 e^{13}, e^{23}, e^{14}, e^{34} + e^{25} + e^{16}, e^{17} + e^{24}$            | 2579     |
| 9631:99   | $0, 0, 0, e^{12}, e^{13}, e^{23}, e^{14}, e^{34} + e^{25}, e^{36} + e^{17} + e^{24}$                           | 2579     |
| 9631:100  | $0, 0, 0, -e^{12}, e^{13}, e^{23}, e^{24}, e^{35} + e^{14}, e^{34} + e^{27} + e^{16}$                          | 2579     |
| 9631:101a | $0, 0, 0, e^{12}, e^{13}, e^{23}, e^{24}, e^{25} + e^{34}, e^{14} + e^{27} + e^{36}$                           | 2579     |
| 9631:101b | $0, 0, 0, -e^{12}, -e^{13}, e^{23}, e^{24}, e^{25} + e^{34}, e^{14} + e^{36} + e^{27}$                         | 2579     |
| 9631:102  | $0, 0, 0, e^{12} a_1, e^{13}, e^{23}, e^{14}, e^{15} + e^{24} + e^{36}, e^{17} + e^{26} + e^{35}$              | 2579     |
| 9631:103  | $0, 0, 0, e^{12}(-1 + a_2), a_2 e^{13}, e^{23}, e^{14}, e^{16} + e^{25} + e^{34}, e^{35} + e^{17} + e^{26}$    | 2579     |
| 9631:104a | $0, 0, 0, e^{12} a_1, e^{13}, e^{23}, e^{14}, e^{16} + e^{34} + e^{25}(1 + a_1), e^{17} + e^{35} + e^{24}$     | 2579     |
| 9631:104b | $0, 0, 0, -e^{12} a_1, -e^{13}, e^{23}, e^{14}, (-1 + a_1) e^{25} + e^{34} + e^{16}, e^{24} + e^{35} + e^{17}$ | 2579     |
| 9631:105  | $0, 0, 0, e^{12}, e^{13}, e^{23}, e^{14}, e^{15} + e^{36} + e^{24}, e^{17} + e^{25} + e^{34}$                  | 2579     |
| 9631:106  | $0, 0, 0, e^{12}(-1 + a_2), e^{13} a_2, e^{23}, e^{24}, e^{34} + e^{25} + e^{16}, e^{35} + e^{27} + e^{14}$    | 2579     |
| 9631:107a | $0, 0, 0, e^{12}, e^{13}, e^{23}, e^{14}, e^{24}, e^{17} + e^{28}$                                             | 3679     |
| 9631:107b | $0, 0, 0, e^{12}, e^{13}, e^{23}, -e^{14}, e^{24}, e^{28} + e^{17}$                                            | 3679     |
| 9631:108  | $0, 0, 0, e^{12}, e^{13}, e^{23}, e^{14}, e^{24}, e^{27} + e^{18}$                                             | 3679     |
| 9631:109a | $0, 0, 0, e^{12}, e^{13}, e^{23}, e^{14}, e^{24}, e^{35} + e^{17} + e^{28}$                                    | 2579     |
| 9631:109b | $0, 0, 0, e^{12}, e^{13}, e^{23}, -e^{14}, e^{24}, e^{17} + e^{35} + e^{28}$                                   | 2579     |
| 9631:110  | $0, 0, 0, e^{12}, e^{13}, e^{23}, e^{14}, e^{24}, e^{35} + e^{27} + e^{18}$                                    | 2579     |
| 9631:132  | $0, 0, 0, e^{12}, e^{13}, e^{23}, e^{24}, e^{15}, e^{27} + e^{18}$                                             | 2469     |
| 9631:133  | $0, 0, 0, e^{12}, e^{13}, e^{23}, e^{24}, e^{35}, e^{38} + e^{27}$                                             | 2469     |
| 9631:134  | $0, 0, 0, e^{12}, e^{13}, e^{23}, e^{14}, e^{15} + e^{24}, e^{18} + e^{27}$                                    | 2469     |
| 9631:135  | $0, 0, 0, e^{12}, e^{13}, e^{23}, e^{24}, e^{25} + e^{34}, e^{37} + e^{28}$                                    | 2469     |
| 9631:136  | $0, 0, 0, e^{12}, e^{13}, e^{23}, e^{14}, e^{35}, e^{17} + e^{38} + e^{24}$                                    | 2469     |
| 9631:137  | $0, 0, 0, e^{12}, e^{13}, e^{23}, e^{24}, e^{35}, e^{14} + e^{38} + e^{27}$                                    | 2469     |
| 9631:138  | $0, 0, 0, e^{12}, e^{13}, e^{23}, e^{24}, e^{15}, e^{36} + e^{18} + e^{27}$                                    | 1469     |
| 9631:139  | $0, 0, 0, -e^{12}, e^{13}, e^{23}, e^{14}, e^{15}, e^{37} + e^{45} + e^{28}$                                   | 2469     |
| 9631:140a | $0, 0, 0, e^{12}, e^{13}, e^{23}, e^{25} + e^{34}, e^{24} + e^{35}, e^{38} + e^{27}$                           | 2469     |
| 9631:140b | $0, 0, 0, -e^{12}, e^{13}, e^{23}, e^{34} - e^{25}, e^{35} + e^{24}, e^{38} + e^{27}$                          | 2469     |
| 9631:141  | $0, 0, 0, e^{12}, e^{13}, e^{23}, e^{24}, e^{34} + e^{25}, e^{28} + e^{37} + e^{14}$                           | 2469     |
| 9631:142  | $0, 0, 0, e^{12}, e^{13}, e^{23}, e^{14}, e^{15} + e^{24}, e^{18} + e^{27} + e^{35}$                           | 2469     |
| 9631:143  | $0, 0, 0, e^{12}, e^{13}, e^{23}, e^{24}, e^{25} + e^{34}, e^{37} + e^{15} + e^{28}$                           | 2469     |
| 9631:144  | $0, 0, 0, e^{12}, e^{13}, e^{23}, e^{14}, e^{15} + e^{24}, e^{27} + e^{18} + e^{36}$                           | 1469     |
| 9631:145  | $0, 0, 0, -e^{12}, e^{13}, e^{23}, e^{14}, e^{15} + e^{24}, e^{28} + e^{37} + e^{45}$                          | 2469     |
| 9631:147  | $0, 0, 0, e^{12}, e^{13}, e^{23}, 2e^{14}, e^{25} + e^{34}, e^{18} + e^{45} + e^{37}$                          | 2469     |
| 9631:148a | $0, 0, 0, e^{12}, e^{13}, e^{23}, e^{34} + e^{25}, e^{35} + e^{24}, e^{38} + e^{27} + e^{14}$                  | 2469     |
| 9631:148b | $0, 0, 0, -e^{12}, e^{13}, e^{23}, e^{34} - e^{25}, e^{35} + e^{24}, e^{14} + e^{38} + e^{27}$                 | 2469     |
| 9631:149a | $0, 0, 0, e^{12}, e^{13}, e^{23}, e^{25} + e^{34}, e^{24} + e^{35}, e^{28} + e^{14} + e^{37}$                  | 2469     |

Table 2 – Continued to next page

Table 2 – Continued from previous page

| Name      | $\mathfrak{g}$                                                                                                                   | UCS Dim. |
|-----------|----------------------------------------------------------------------------------------------------------------------------------|----------|
| 9631:149b | $0, 0, 0, e^{12}, e^{13}, e^{23}, e^{25} + e^{34}, -e^{24} + e^{35}, e^{37} + e^{14} + e^{28}$                                   | 2469     |
| 9631:150  | $0, 0, 0, -e^{12}, -e^{13}, e^{23}, e^{24} + 2e^{15}, e^{25} + e^{34}, e^{27} + e^{18} + e^{45}$                                 | 2469     |
| 9631:151  | $0, 0, 0, -e^{12}, e^{13}, e^{23}, e^{24} + e^{15}, e^{35} + e^{14}, e^{38} + e^{27} + e^{45}$                                   | 2469     |
| 9631:152  | $0, 0, 0, e^{12}, e^{13}, e^{23}, 2e^{14}, e^{25} + e^{34}, e^{18} + e^{45} + e^{37} + e^{26}$                                   | 1469     |
| 9631:154  | $0, 0, 0, -e^{12}, -e^{13}, e^{23}, e^{24} + 2e^{15}, e^{25} + e^{34}, e^{36} + e^{45} + e^{27} + e^{18}$                        | 1469     |
| 9631:155  | $0, 0, 0, e^{12}, -e^{13}, e^{23}, e^{34} - 2e^{16} + e^{25}, e^{14}, e^{45} + e^{17}$                                           | 2369     |
| 9631:156  | $0, 0, 0, e^{12}, -e^{13}, e^{23}, -2e^{16} + e^{34} + e^{25}, e^{24}, e^{17} + e^{45}$                                          | 2369     |
| 9631:157  | $0, 0, 0, -2e^{12}, -e^{13}, e^{23}, e^{16} + e^{25} + e^{34}, e^{14}, e^{56} + e^{37}$                                          | 2369     |
| 9631:158  | $0, 0, 0, e^{12}, -e^{13}, e^{23}, -2e^{16} + e^{34} + e^{25}, e^{24} + e^{15}, e^{17} + e^{45}$                                 | 2369     |
| 9631:159a | $0, 0, 0, e^{12}, -e^{13}, e^{23}, -2e^{16} + e^{25} + e^{34}, e^{35} + e^{24}, e^{45} + e^{17}$                                 | 2369     |
| 9631:159b | $0, 0, 0, -e^{12}, -e^{13}, e^{23}, e^{34} - e^{25} + 2e^{16}, e^{35} + e^{24}, e^{45} + e^{17}$                                 | 2369     |
| 9631:160  | $0, 0, 0, -e^{12}, -2e^{13}, -e^{23}, e^{16} + e^{25} + e^{34}, e^{24} + e^{15}, e^{46} + e^{27}$                                | 2369     |
| 9631:161  | $0, 0, 0, -e^{12}, -2e^{13}, -e^{23}, e^{16} + e^{25} + e^{34}, e^{35} + e^{14}, e^{46} + e^{27}$                                | 2369     |
| 9631:162a | $0, 0, 0, -e^{12}, e^{13}, -e^{23}, e^{16} - 2e^{25} + e^{34}, e^{35} + e^{24}, e^{46} + e^{27}$                                 | 2369     |
| 9631:162b | $0, 0, 0, -e^{12}, -e^{13}, -e^{23}, e^{16} + 2e^{25} + e^{34}, e^{35} + e^{24}, e^{27} + e^{46}$                                | 2369     |
| 9631:163  | $0, 0, 0, -e^{12}, -2e^{13}, -e^{23}, e^{16} + e^{25} + e^{34}, e^{14}, e^{46} + e^{15} + e^{27}$                                | 2369     |
| 9631:164  | $0, 0, 0, e^{12}, -e^{13}, e^{23}, -2e^{16} + e^{34} + e^{25}, e^{14}, e^{17} + e^{26} + e^{45}$                                 | 2369     |
| 9631:165  | $0, 0, 0, e^{12}, -e^{13}, e^{23}, e^{34} + e^{25} - 2e^{16}, e^{14}, e^{36} + e^{45} + e^{17}$                                  | 2369     |
| 9631:166  | $0, 0, 0, -2e^{12}, -e^{13}, e^{23}, e^{16} + e^{25} + e^{34}, e^{14}, e^{37} + e^{24} + e^{56}$                                 | 2369     |
| 9631:167  | $0, 0, 0, -e^{12}, -2e^{13}, -e^{23}, e^{16} + e^{25} + e^{34}, e^{14}, e^{35} + e^{46} + e^{27}$                                | 2369     |
| 9631:168  | $0, 0, 0, e^{12}, -e^{13}, e^{23}, -2e^{16} + e^{34} + e^{25}, e^{15} + e^{24} + e^{36}, e^{17} + e^{45}$                        | 2369     |
| 9631:169  | $0, 0, 0, e^{12}, -e^{13}, e^{23}, -2e^{16} + e^{34} + e^{25}, e^{15} + e^{24}, e^{17} + e^{26} + e^{45}$                        | 2369     |
| 9631:170  | $0, 0, 0, -2e^{12}, -e^{13}, e^{23}, e^{16} + e^{25} + e^{34}, e^{15} + e^{24}, e^{37} + e^{14} + e^{56}$                        | 2369     |
| 9631:171  | $0, 0, 0, e^{12}, -e^{13}, e^{23}, -2e^{16} + e^{34} + e^{25}, e^{15} + e^{24}, e^{17} + e^{36} + e^{45}$                        | 2369     |
| 9631:172  | $0, 0, 0, -e^{12}, -2e^{13}, -e^{23}, e^{16} + e^{25} + e^{34}, e^{24} + e^{15}, e^{35} + e^{46} + e^{27}$                       | 2369     |
| 9631:173a | $0, 0, 0, -e^{12}, e^{13}, -e^{23}, e^{16} - 2e^{25} + e^{34}, e^{35} + e^{24}, e^{46} + e^{15} + e^{27}$                        | 2369     |
| 9631:173b | $0, 0, 0, -e^{12}, -e^{13}, -e^{23}, e^{16} + 2e^{25} + e^{34}, e^{35} + e^{24}, e^{15} + e^{27} + e^{46}$                       | 2369     |
| 9631:174a | $0, 0, 0, e^{12}, -e^{13}, e^{23}, -2e^{16} + e^{25} + e^{34}, e^{35} + e^{24}, e^{17} + e^{26} + e^{45}$                        | 2369     |
| 9631:174b | $0, 0, 0, -e^{12}, -e^{13}, e^{23}, e^{34} - e^{25} + 2e^{16}, e^{35} + e^{24}, e^{45} + e^{17} + e^{26}$                        | 2369     |
| 9631:175  | $0, 0, 0, -e^{12}, -2e^{13}, -e^{23}, e^{16} + e^{25} + e^{34}, e^{35} + e^{14} + e^{26}, e^{46} + e^{15} + e^{27}$              | 2369     |
| 9631:176  | $0, 0, 0, e^{12}, e^{13}, e^{23}, e^{24} + e^{15}, e^{26} + e^{14}, e^{17} + e^{28}$                                             | 1369     |
| 9631:177  | $0, 0, 0, -e^{12}, e^{13}, e^{23}, e^{35} + e^{14}, e^{16} + e^{34}, e^{18} + e^{37}$                                            | 1369     |
| 9631:178  | $0, 0, 0, e^{12}, e^{13}, e^{23}, e^{14}, e^{25} + e^{16}, e^{37} + e^{45} + e^{18}$                                             | 1369     |
| 9631:179a | $0, 0, 0, -e^{12}, e^{13}, e^{23}, e^{14}, e^{15} + e^{26}, e^{37} + e^{45} + e^{28}$                                            | 1369     |
| 9631:179b | $0, 0, 0, -e^{12}, -e^{13}, e^{23}, -e^{14}, e^{26} + e^{15}, e^{28} + e^{45} + e^{37}$                                          | 1369     |
| 9631:181  | $0, 0, 0, -e^{12}, e^{13}, e^{23}, e^{35} + e^{14}, e^{16} + e^{34}, e^{24} + e^{37} + e^{18}$                                   | 1369     |
| 9631:182  | $0, 0, 0, e^{12}, e^{13}, e^{23}, e^{15} + e^{24}, e^{14} + e^{26}, e^{28} + e^{35} + e^{17}$                                    | 1369     |
| 9631:183  | $0, 0, 0, e^{12}, e^{13}, e^{23}, e^{25} + e^{34}, e^{24} + e^{36}, e^{38} + e^{15} + e^{27}$                                    | 1369     |
| 9631:184  | $0, 0, 0, e^{12}, -e^{13}, e^{23}, e^{24} - 2e^{16} + e^{34} + e^{25}, e^{18} + e^{27} + e^{45}$                                 | 1369     |
| 9631:185  | $0, 0, 0, e^{12}, (-1 + a_3)e^{13}, e^{23}, e^{14}a_3, e^{25} + e^{34} + e^{16}(-2 + a_3), e^{37} + e^{18} + e^{45}$             | 1369     |
| 9631:186a | $0, 0, 0, -2e^{12}, -e^{13}, e^{23}, e^{14}, e^{16} + e^{25} + e^{34}, e^{56} + e^{17} + e^{38}$                                 | 1369     |
| 9631:186b | $0, 0, 0, -2e^{12}, -e^{13}, e^{23}, -e^{14}, e^{16} + e^{25} + e^{34}, e^{17} + e^{38} + e^{56}$                                | 1369     |
| 9631:187  | $0, 0, 0, -e^{12}, -e^{13}, e^{23}, e^{15} + e^{24}, e^{16} + e^{34}, e^{27} + e^{18} + e^{45}$                                  | 1369     |
| 9631:188a | $0, 0, 0, e^{12}, e^{13}, e^{23}, e^{24} - e^{15}, e^{36} + e^{14}, e^{38} + e^{27} + e^{45}$                                    | 1369     |
| 9631:188b | $0, 0, 0, -e^{12}, e^{13}, e^{23}, e^{15} + e^{24}, e^{14} + e^{36}, e^{38} + e^{27} + e^{45}$                                   | 1369     |
| 9631:189a | $0, 0, 0, e^{12}, e^{13}, e^{23}, e^{25} + e^{34}, e^{36} + 2e^{14}, e^{17} + e^{45} + e^{38}$                                   | 1369     |
| 9631:189b | $0, 0, 0, e^{12}, e^{13}, -e^{23}, e^{25} + e^{34}, e^{36} + 2e^{14}, e^{38} + e^{45} + e^{17}$                                  | 1369     |
| 9631:190  | $0, 0, 0, e^{12}, e^{13}, -e^{23}, e^{14} + e^{35}, e^{24} + e^{36}, e^{56} + e^{18} + e^{27}$                                   | 1369     |
| 9631:191a | $0, 0, 0, e^{12}, e^{13}, -e^{23}, e^{24} + e^{35}, e^{36} + e^{14}, e^{18} + e^{56} + e^{27}$                                   | 1369     |
| 9631:191b | $0, 0, 0, e^{12}, e^{13}, -e^{23}, e^{35} + e^{24}, e^{36} - e^{14}, e^{56} + e^{27} + e^{18}$                                   | 1369     |
| 9631:191c | $0, 0, 0, -e^{12}, e^{13}, -e^{23}, e^{35} + e^{24}, e^{36} + e^{14}, e^{56} + e^{27} + e^{18}$                                  | 1369     |
| 9631:192a | $0, 0, 0, e^{12}, e^{13}, e^{23}, e^{25} + e^{34}, e^{36} + e^{14}, e^{37} + e^{18} + e^{56}$                                    | 1369     |
| 9631:192b | $0, 0, 0, e^{12}, e^{13}, e^{23}, e^{25} + e^{34}, e^{36} - e^{14}, e^{18} + e^{56} + e^{37}$                                    | 1369     |
| 9631:194  | $0, 0, 0, e^{12}, e^{13}, e^{23}, e^{14}, e^{25} + e^{16}, e^{18} + e^{45} + e^{37} + e^{26}$                                    | 1369     |
| 9631:195  | $0, 0, 0, -e^{12}a_1, -e^{13}, e^{23}, e^{24} + e^{15}(1 + a_1), (-1 + a_1)e^{16} + e^{25} + e^{34}, e^{27} + e^{18} + e^{45}$   | 1369     |
| 9631:196  | $0, 0, 0, e^{12}, e^{13}, e^{23}, e^{24} + e^{15}, e^{26} + e^{35} + e^{14}, e^{37} + e^{18} + e^{46}$                           | 1369     |
| 9631:197a | $0, 0, 0, -e^{12}, e^{13}, (1 + a_4)e^{23}, e^{35} + (2 + a_4)e^{24}, a_4e^{25} + e^{16} + e^{34}, e^{37} + e^{46} + e^{28}$     | 1369     |
| 9631:197b | $0, 0, 0, -e^{12}, -e^{13}, -e^{23}(-1 + a_4), e^{35} - (-2 + a_4)e^{24}, a_4e^{25} + e^{16} + e^{34}, e^{37} + e^{46} + e^{28}$ | 1369     |

Table 2 – Continued to next page



Table 2 – Continued from previous page

| Name      | $\mathfrak{g}$                                                                                                                          | UCS Dim. |
|-----------|-----------------------------------------------------------------------------------------------------------------------------------------|----------|
| 9631:198a | $0, 0, 0, -2e^{12}, -e^{13}, e^{23}, e^{14}, e^{16} + e^{25} + e^{34}, e^{56} + e^{17} + e^{38} + e^{24}$                               | 1369     |
| 9631:198b | $0, 0, 0, -2e^{12}, -e^{13}, e^{23}, -e^{14}, e^{16} + e^{25} + e^{34}, e^{56} + e^{17} + e^{38} + e^{24}$                              | 1369     |
| 9631:199  | $0, 0, 0, -e^{12}, -2e^{13}, -e^{23}, e^{14}, e^{16} + e^{25} + e^{34}, e^{35} + e^{46} + e^{28} + e^{17}$                              | 1369     |
| 9631:200  | $0, 0, 0, e^{12}, (1 + a_4)e^{13}, e^{23}, (2 + a_4)e^{14}, e^{16}a_4 + e^{25} + e^{34}, e^{37} + e^{26} + e^{18} + e^{45}$             | 1369     |
| 9631:201  | $0, 0, 0, -e^{12}, -e^{13}, e^{23}, e^{15} + e^{24}, e^{16} + e^{34}, e^{27} + e^{18} + e^{36} + e^{45}$                                | 1369     |
| 9631:202a | $0, 0, 0, e^{12}, e^{13}, e^{23}, e^{25} + e^{34}, e^{36} + 2e^{14}, e^{38} + e^{45} + e^{26} + e^{17}$                                 | 1369     |
| 9631:202b | $0, 0, 0, e^{12}, e^{13}, -e^{23}, e^{25} + e^{34}, e^{36} + 2e^{14}, e^{26} + e^{17} + e^{45} + e^{38}$                                | 1369     |
| 9631:203a | $0, 0, 0, e^{12}, e^{13}, e^{23}, e^{25} + e^{34}, e^{36} + e^{14}, e^{18} + e^{56} + e^{24} + e^{37}$                                  | 1369     |
| 9631:203b | $0, 0, 0, e^{12}, e^{13}, e^{23}, e^{25} + e^{34}, e^{36} - e^{14}, e^{24} + e^{37} + e^{18} + e^{56}$                                  | 1369     |
| 9631:204  | $0, 0, 0, -e^{12}, e^{13}, a_3e^{23}, e^{15} + e^{24} + e^{36}, e^{14} + e^{26} + e^{35}, e^{38} + e^{45} + e^{27}$                     | 1369     |
| 9631:205  | $0, 0, 0, -(1 + a_4)e^{12}, -e^{13}, e^{23}, (2 + a_4)e^{15} + e^{24}, a_4e^{16} + e^{25} + e^{34}, e^{18} + e^{27} + e^{45} + e^{36}$  | 1369     |
| 9631:206a | $0, 0, 0, -e^{12}(1 + 2a_3), -e^{13}, e^{23}, a_3e^{24} + e^{35}, e^{16} + e^{34} + (1 + a_3)e^{25}, e^{27} + e^{14} + e^{38} + e^{56}$ | 1369     |
| 9631:206b | $0, 0, 0, -e^{12}(1 + 2a_3), -e^{13}, e^{23}, a_3e^{35} - e^{24}, e^{34} + e^{16} + (1 + a_3)e^{25}, e^{38} + e^{56} + e^{27} + e^{14}$ | 1369     |
| Type: 333 |                                                                                                                                         |          |
| 963:1     | $0, 0, 0, e^{12}, e^{13}, e^{23}, e^{14}, e^{24}, e^{15}$                                                                               | 469      |
| 963:2     | $0, 0, 0, e^{12}, e^{13}, e^{23}, e^{14}, e^{24}, e^{35}$                                                                               | 469      |
| 963:3     | $0, 0, 0, e^{12}, e^{13}, e^{23}, e^{14}, e^{24}, e^{25} + e^{34}$                                                                      | 469      |
| 963:4a    | $0, 0, 0, e^{12}, e^{13}, e^{23}, e^{14}, e^{15}, e^{35} + e^{24}$                                                                      | 469      |
| 963:4b    | $0, 0, 0, -e^{12}, e^{13}, e^{23}, e^{14}, e^{15}, e^{35} + e^{24}$                                                                     | 469      |
| 963:5     | $0, 0, 0, e^{12}, e^{13}, e^{23}, e^{14}, e^{15}, e^{25} + e^{34}$                                                                      | 469      |
| 963:6     | $0, 0, 0, e^{12}, e^{13}, e^{23}, e^{24}, e^{15}, e^{35} + e^{14}$                                                                      | 469      |
| 963:7     | $0, 0, 0, e^{12}, e^{13}, e^{23}, e^{24}, e^{15}, e^{25} + e^{34}$                                                                      | 469      |
| 963:8     | $0, 0, 0, e^{12}, e^{13}, e^{23}, e^{24}, e^{35}, e^{34} + e^{25}$                                                                      | 469      |
| 963:9     | $0, 0, 0, e^{12}, e^{13}, e^{23}, e^{14}, e^{24} + e^{15}, e^{25} + e^{34}$                                                             | 469      |
| 963:10a   | $0, 0, 0, e^{12}, e^{13}, e^{23}, e^{14}, e^{34} + e^{25}, e^{35} + e^{24}$                                                             | 469      |
| 963:10b   | $0, 0, 0, -e^{12}, e^{13}, e^{23}, e^{14}, -e^{25} + e^{34}, e^{24} + e^{35}$                                                           | 469      |
| 963:11    | $0, 0, 0, e^{12}, e^{13}, e^{23}, e^{24}, e^{14} + e^{35}, e^{25} + e^{34}$                                                             | 469      |
| 963:12    | $0, 0, 0, e^{12}, e^{13}, e^{23}, e^{24} + e^{15}, e^{35} + e^{14}, e^{25} + e^{34}$                                                    | 469      |
| 963:13    | $0, 0, 0, e^{12}, e^{13}, e^{23}, e^{14}, e^{15}, e^{26}$                                                                               | 369      |
| 963:14    | $0, 0, 0, e^{12}, e^{13}, e^{23}, e^{24}, e^{15}, e^{36}$                                                                               | 369      |
| 963:15a   | $0, 0, 0, e^{12}, e^{13}, e^{23}, e^{14}, e^{24}, e^{15} + e^{26}$                                                                      | 369      |
| 963:15b   | $0, 0, 0, e^{12}, -e^{13}, e^{23}, e^{14}, e^{24}, e^{15} + e^{26}$                                                                     | 369      |
| 963:16    | $0, 0, 0, e^{12}, e^{13}, e^{23}, e^{14}, e^{24}, e^{25} + e^{16}$                                                                      | 369      |
| 963:17    | $0, 0, 0, e^{12}, e^{13}, e^{23}, e^{14}, e^{24}, e^{36} + e^{15}$                                                                      | 369      |
| 963:18    | $0, 0, 0, e^{12}, e^{13}, e^{23}, e^{24}, e^{15}, e^{26} + e^{14}$                                                                      | 369      |
| 963:19    | $0, 0, 0, -e^{12}, e^{13}, e^{23}, e^{14}, e^{15}, e^{34} + e^{16}$                                                                     | 369      |
| 963:20    | $0, 0, 0, e^{12}, e^{13}, e^{23}, e^{14}, e^{15}, e^{36} + e^{24}$                                                                      | 369      |
| 963:21a   | $0, 0, 0, e^{12}, e^{13}, e^{23}, e^{24}, e^{15}, e^{14} + e^{36}$                                                                      | 369      |
| 963:21b   | $0, 0, 0, -e^{12}, e^{13}, e^{23}, e^{24}, e^{15}, e^{14} + e^{36}$                                                                     | 369      |
| 963:22    | $0, 0, 0, -e^{12}, e^{13}, e^{23}, e^{24}, e^{15}, e^{16} + e^{34}$                                                                     | 369      |
| 963:23    | $0, 0, 0, e^{12}, e^{13}, e^{23}, e^{24}, e^{35}, e^{26} + e^{14}$                                                                      | 369      |
| 963:24    | $0, 0, 0, -e^{12}, e^{13}, e^{23}, e^{14}, e^{35}, e^{16} + e^{34}$                                                                     | 369      |
| 963:25    | $0, 0, 0, e^{12}, e^{13}, e^{23}, e^{14}, e^{35}, e^{36} + e^{24}$                                                                      | 369      |
| 963:26a   | $0, 0, 0, e^{12}, e^{13}, e^{23}, e^{24}, e^{35}, e^{14} + e^{36}$                                                                      | 369      |
| 963:26b   | $0, 0, 0, -e^{12}, e^{13}, e^{23}, e^{24}, e^{35}, e^{36} + e^{14}$                                                                     | 369      |
| 963:27    | $0, 0, 0, -e^{12}, e^{13}, e^{23}, e^{24}, e^{35}, e^{16} + e^{34}$                                                                     | 369      |
| 963:28    | $0, 0, 0, (-1 + a_2)e^{12}, e^{13}, a_2e^{23}, e^{14}, e^{24}, e^{25} + e^{34} + e^{16}$                                                | 369      |
| 963:29    | $0, 0, 0, (-1 + a_2)e^{12}, e^{13}, a_2e^{23}, e^{14}, e^{15}, e^{16} + e^{25} + e^{34}$                                                | 369      |
| 963:30    | $0, 0, 0, e^{12}, e^{13}, e^{23}, e^{24}, e^{15}, e^{14} + e^{35} + e^{26}$                                                             | 369      |
| 963:31    | $0, 0, 0, e^{12}, a_1e^{13}, (1 + a_1), e^{23}, e^{24}, e^{15}, e^{16} + e^{25} + e^{34}$                                               | 369      |
| 963:32    | $0, 0, 0, e^{12}, (-1 + a_2), a_2e^{13}, e^{23}, e^{24}, e^{35}, e^{16} + e^{25} + e^{34}$                                              | 369      |
| 963:33    | $0, 0, 0, -e^{12}, e^{13}, e^{23}, e^{14}, e^{24} + e^{15}, e^{16} + e^{34}$                                                            | 369      |
| 963:34a   | $0, 0, 0, -e^{12}, e^{13}, e^{23}, e^{14}, e^{35} + e^{24}, e^{34} + e^{16}$                                                            | 369      |
| 963:34b   | $0, 0, 0, -e^{12}, -e^{13}, e^{23}, e^{14}, e^{35} + e^{24}, e^{16} + e^{34}$                                                           | 369      |
| 963:35    | $0, 0, 0, e^{12}, e^{13}, e^{23}, e^{14}, e^{25} + e^{34}, e^{24} + e^{36}$                                                             | 369      |
| 963:36    | $0, 0, 0, e^{12}, e^{13}, e^{23}, e^{14}, e^{24} + e^{15}, e^{25} + e^{16}$                                                             | 369      |
| 963:37    | $0, 0, 0, e^{12}, a_1e^{13}, e^{23}, e^{14}, e^{24} + e^{15}, e^{26} + e^{35}$                                                          | 369      |
| 963:38a   | $0, 0, 0, e^{12}, e^{13}, e^{23}, e^{14}, e^{35} + e^{24}, e^{26} + e^{15}$                                                             | 369      |

Table 2 – Continued to next page

Table 2 – Continued from previous page

| Name    | $\mathfrak{g}$                                                                                      | UCS Dim. |
|---------|-----------------------------------------------------------------------------------------------------|----------|
| 963:38b | $0, 0, 0, e^{12}, -e^{13}, e^{23}, e^{14}, e^{35} + e^{24}, e^{15} + e^{26}$                        | 369      |
| 963:38c | $0, 0, 0, -e^{12}, e^{13}, e^{23}, e^{14}, e^{24} + e^{35}, e^{15} + e^{26}$                        | 369      |
| 963:38d | $0, 0, 0, -e^{12}, -e^{13}, e^{23}, e^{14}, e^{35} + e^{24}, e^{26} + e^{15}$                       | 369      |
| 963:39a | $0, 0, 0, e^{12}, e^{13}, e^{23}, e^{14}, e^{34} + e^{25}, e^{15} + e^{26}$                         | 369      |
| 963:39b | $0, 0, 0, -e^{12}, -e^{13}, e^{23}, e^{14}, e^{34} + e^{25}, e^{26} + e^{15}$                       | 369      |
| 963:40a | $0, 0, 0, e^{12}, e^{13}, e^{23}, e^{14}, e^{35} + e^{24}, e^{16} + e^{25}$                         | 369      |
| 963:40b | $0, 0, 0, -e^{12}, e^{13}, e^{23}, e^{14}, e^{24} + e^{35}, e^{16} + e^{25}$                        | 369      |
| 963:41a | $0, 0, 0, e^{12}, e^{13}, e^{23}, e^{24}, e^{14} + e^{35}, e^{15} + e^{26}$                         | 369      |
| 963:41b | $0, 0, 0, e^{12}, -e^{13}, e^{23}, e^{24}, e^{35} + e^{14}, e^{15} + e^{26}$                        | 369      |
| 963:42  | $0, 0, 0, e^{12}, e^{13}, e^{23}, e^{24}, e^{35} + e^{14}, e^{25} + e^{16}$                         | 369      |
| 963:43a | $0, 0, 0, e^{12}, e^{13}, e^{23}, e^{24}, e^{34} + e^{25}, e^{26} + e^{15}$                         | 369      |
| 963:43b | $0, 0, 0, -e^{12}, -e^{13}, e^{23}, e^{24}, e^{25} + e^{34}, e^{26} + e^{15}$                       | 369      |
| 963:44a | $0, 0, 0, e^{12}, e^{13}, e^{23}, e^{14}, e^{35} + e^{24}, e^{15} + e^{36}$                         | 369      |
| 963:44b | $0, 0, 0, -e^{12}, e^{13}, e^{23}, e^{14}, e^{35} + e^{24}, e^{36} + e^{15}$                        | 369      |
| 963:45  | $0, 0, 0, e^{12}, e^{13}, e^{23}, e^{14}, e^{25} + e^{34}, e^{36} + e^{15}$                         | 369      |
| 963:46  | $0, 0, 0, e^{12}, e^{13}, e^{23}, e^{14}, e^{34} + e^{25}, e^{26} + e^{35}$                         | 369      |
| 963:47  | $0, 0, 0, e^{12}, e^{13}, e^{23}, e^{24}, e^{14} + e^{35}, e^{15} + e^{36}$                         | 369      |
| 963:48  | $0, 0, 0, e^{12}, e^{13}, e^{23}, e^{24}, e^{25} + e^{34}, e^{15} + e^{36}$                         | 369      |
| 963:49  | $0, 0, 0, e^{12}, e^{13}, e^{23}, e^{24}, e^{25} + e^{34}, e^{35} + e^{26}$                         | 369      |
| 963:50  | $0, 0, 0, e^{12}, e^{13}, e^{23}, e^{15} + e^{24}, e^{14} + e^{35}, e^{26}$                         | 369      |
| 963:51  | $0, 0, 0, e^{12}, e^{13}, e^{23}, e^{24} + e^{15}, e^{34} + e^{25}, e^{26}$                         | 369      |
| 963:52  | $0, 0, 0, e^{12}, e^{13}, e^{23}, e^{15} + e^{24}, e^{25} + e^{34}, e^{36}$                         | 369      |
| 963:53a | $0, 0, 0, e^{12}, e^{13}, e^{23}, e^{34} + e^{25}, e^{35} + e^{24}, e^{26}$                         | 369      |
| 963:53b | $0, 0, 0, -e^{12}, e^{13}, e^{23}, e^{34} - e^{25}, e^{35} + e^{24}, e^{26}$                        | 369      |
| 963:54  | $0, 0, 0, e^{12}(-1 + a_2), a_2 e^{13}, e^{23}, e^{14}, e^{15} + e^{24}, e^{34} + e^{16} + e^{25}$  | 369      |
| 963:55a | $0, 0, 0, e^{12} a_1, (1 + a_1) e^{13}, e^{23}, e^{14}, e^{35} + e^{24}, e^{16} + e^{34} + e^{25}$  | 369      |
| 963:55b | $0, 0, 0, e^{12} a_1, (1 + a_1) e^{13}, e^{23}, e^{14}, e^{35} - e^{24}, e^{16} + e^{34} + e^{25}$  | 369      |
| 963:56  | $0, 0, 0, e^{12}, e^{13}, e^{23}, e^{14}, e^{34} + e^{25}, e^{24} + e^{36} + e^{15}$                | 369      |
| 963:57  | $0, 0, 0, e^{12} a_1, e^{13}(1 + a_1), e^{23}, e^{24}, e^{35} + e^{14}, e^{25} + e^{34} + e^{16}$   | 369      |
| 963:58  | $0, 0, 0, e^{12}, e^{13}, e^{23}, e^{24}, e^{25} + e^{34}, e^{14} + e^{26} + e^{35}$                | 369      |
| 963:59a | $0, 0, 0, e^{12} a_1, e^{13}(1 + a_1), e^{23}, e^{14}, e^{26} + e^{15}, e^{34} + e^{25} + e^{16}$   | 369      |
| 963:59b | $0, 0, 0, e^{12} a_1, e^{13}(1 + a_1), e^{23}, e^{14}, e^{26} - e^{15}, e^{16} + e^{34} + e^{25}$   | 369      |
| 963:60  | $0, 0, 0, e^{12}, e^{13}, e^{23}, e^{14}, e^{25} + e^{16}, e^{24} + e^{36} + e^{15}$                | 369      |
| 963:61  | $0, 0, 0, e^{12}(-1 + a_2), e^{13} a_2, e^{23}, e^{14}, e^{36} + e^{15}, e^{25} + e^{34} + e^{16}$  | 369      |
| 963:62  | $0, 0, 0, a_1 e^{12}, e^{13}, e^{23}, e^{14}, e^{26} + e^{35}, e^{15} + e^{24} + e^{36}$            | 369      |
| 963:63  | $0, 0, 0, (-1 + a_2) e^{12}, e^{13} a_2, e^{23}, e^{14}, e^{35} + e^{26}, e^{16} + e^{34} + e^{25}$ | 369      |
| 963:64  | $0, 0, 0, e^{12}, e^{13}, e^{23}, e^{24} + e^{15}, e^{34} + e^{25}, e^{26} + e^{14}$                | 369      |
| 963:65  | $0, 0, 0, -e^{12}, e^{13}, e^{23}, e^{15} + e^{24}, e^{14} + e^{35}, e^{16} + e^{34}$               | 369      |
| 963:66a | $0, 0, 0, e^{12}, e^{13}, e^{23}, e^{15} + e^{24}, e^{34} + e^{25}, e^{14} + e^{36}$                | 369      |
| 963:66b | $0, 0, 0, -e^{12}, -e^{13}, e^{23}, e^{15} + e^{24}, e^{34} + e^{25}, e^{36} + e^{14}$              | 369      |
| 963:67a | $0, 0, 0, e^{12}, e^{13}, e^{23}, e^{34} + e^{25}, e^{35} + e^{24}, e^{14} + e^{26}$                | 369      |
| 963:67b | $0, 0, 0, -e^{12}, e^{13}, e^{23}, -e^{25} + e^{34}, e^{24} + e^{35}, e^{14} + e^{26}$              | 369      |
| 963:68  | $0, 0, 0, e^{12} a_2, e^{13} a_2, e^{23}, e^{35} + e^{14}, e^{34} + e^{25}, e^{24} + e^{36}$        | 369      |
| 963:69a | $0, 0, 0, e^{12}, e^{13}, e^{23}, e^{34} + e^{25}, e^{35} + e^{24}, e^{36} + e^{14}$                | 369      |
| 963:69b | $0, 0, 0, e^{12}, -e^{13}, e^{23}, e^{34} - e^{25}, e^{35} + e^{24}, e^{36} + e^{14}$               | 369      |
| 963:69c | $0, 0, 0, -e^{12}, e^{13}, e^{23}, -e^{25} + e^{34}, e^{35} + e^{24}, e^{36} + e^{14}$              | 369      |
| 963:69d | $0, 0, 0, -e^{12}, -e^{13}, e^{23}, e^{25} + e^{34}, e^{24} + e^{35}, e^{36} + e^{14}$              | 369      |
| 963:70  | $0, 0, 0, e^{12}, e^{13}, e^{23}, e^{15} + e^{24}, e^{14} + e^{26}, e^{16} + e^{25}$                | 369      |
| 963:71a | $0, 0, 0, e^{12}, e^{13}, e^{23}, e^{15} + e^{24}, e^{14} + e^{36}, e^{16} + e^{25}$                | 369      |
| 963:71b | $0, 0, 0, -e^{12}, e^{13}, e^{23}, e^{15} + e^{24}, e^{14} + e^{36}, e^{16} + e^{25}$               | 369      |
| 963:72a | $0, 0, 0, e^{12}, e^{13}, e^{23}, e^{24} + a_1 e^{15}, e^{36} + e^{14}, e^{26} + e^{35}$            | 369      |
| 963:72b | $0, 0, 0, -e^{12}, e^{13}, e^{23}, e^{24} + a_1 e^{15}, e^{36} + e^{14}, e^{26} + e^{35}$           | 369      |
| 963:73  | $0, 0, 0, -e^{12}, e^{13}, e^{23}, a_2 e^{15} + e^{24}, e^{16} + e^{34}, e^{26} + e^{35}$           | 369      |
| 963:74a | $0, 0, 0, e^{12}, e^{13}, e^{23}, e^{24} + e^{35}, e^{36} + a_1 e^{14}, e^{26} + e^{15}$            | 369      |
| 963:74b | $0, 0, 0, e^{12}, -e^{13}, e^{23}, e^{35} + e^{24}, e^{36} + a_1 e^{14}, e^{26} + e^{15}$           | 369      |
| 963:75a | $0, 0, 0, e^{12}, e^{13}, e^{23}, e^{25} + e^{34}, e^{14} + e^{36}, e^{15} + e^{26}$                | 369      |
| 963:75b | $0, 0, 0, e^{12}, e^{13}, e^{23}, e^{34} + e^{25}, e^{36} - e^{14}, e^{26} + e^{15}$                | 369      |
| 963:75c | $0, 0, 0, -e^{12}, -e^{13}, e^{23}, e^{25} + e^{34}, -e^{14} + e^{36}, e^{26} + e^{15}$             | 369      |

Table 2 – Continued to next page

Table 2 – Continued from previous page

| Name         | $\mathfrak{g}$                                                                                                                       | UCS Dim. |
|--------------|--------------------------------------------------------------------------------------------------------------------------------------|----------|
| 963:76       | $0, 0, 0, (-1 + a_2)e^{12}, a_2e^{13}, e^{23}, e^{14}, e^{16} + e^{34} + e^{25}, e^{36} + e^{24} + e^{15}$                           | 369      |
| 963:77       | $0, 0, 0, (-1 + a_2)e^{12}, e^{13}a_2, e^{23}, e^{24} + e^{15}, e^{35} + e^{14}, e^{34} + e^{25} + e^{16}$                           | 369      |
| 963:78       | $0, 0, 0, e^{12}a_1, e^{13}a_1, e^{23}, e^{15} + e^{24}, e^{34} + e^{25}, e^{35} + e^{14} + e^{26}$                                  | 369      |
| 963:79       | $0, 0, 0, (-1 + a_2)e^{12}, e^{13}a_2, e^{23}, e^{15} + e^{24}, e^{14} + e^{26}, e^{25} + e^{16} + e^{34}$                           | 369      |
| 963:80a      | $0, 0, 0, (-1 + a_2)e^{12}, e^{13}a_2, e^{23}, e^{24} + e^{15}, e^{36} + e^{14}, e^{25} + e^{34} + e^{16}$                           | 369      |
| 963:80b      | $0, 0, 0, (-1 + a_2)e^{12}, e^{13}a_2, e^{23}, e^{15} + e^{24}, -e^{14} + e^{36}, e^{16} + e^{25} + e^{34}$                          | 369      |
| 963:81       | $0, 0, 0, -e^{12}, e^{13}, e^{23}, e^{24} + a_2e^{15}, e^{34} + e^{16}, e^{35} + e^{14} + e^{26}$                                    | 369      |
| 963:82       | $0, 0, 0, -e^{12}, a_2e^{13}, e^{23}, e^{14} + e^{35}, e^{16} + e^{34}, e^{15} + e^{24} + e^{36}$                                    | 369      |
| 963:83       | $0, 0, 0, e^{12}(-1 + a_2), e^{13}a_2, e^{23}, e^{35} + e^{14}a_3, e^{24} + e^{36}, e^{25} + e^{34} + e^{16}$                        | 369      |
| 963:84a      | $0, 0, 0, e^{12}a_1, (1 + a_1)e^{13}, e^{23}, e^{35} + e^{24}, e^{14} + e^{36}, e^{16} + e^{34} + e^{25}$                            | 369      |
| 963:84b      | $0, 0, 0, e^{12}a_1, (1 + a_1)e^{13}, e^{23}, e^{35} - e^{24}, e^{36} + e^{14}, e^{34} + e^{25} + e^{16}$                            | 369      |
| 963:84c      | $0, 0, 0, e^{12}a_1, (1 + a_1)e^{13}, e^{23}, e^{35} - e^{24}, e^{36} - e^{14}, e^{34} + e^{25} + e^{16}$                            | 369      |
| 963:85       | $0, 0, 0, e^{12}(-1 + a_2), a_2e^{13}, e^{23}, e^{24} + e^{15}a_3, e^{25} + e^{34} + e^{16}, e^{26} + e^{35} + e^{14}$               | 369      |
| 963:86       | $0, 0, 0, e^{12}a_1, e^{13}a_1, e^{23}, e^{25} + e^{34}, a_3e^{14} + e^{26} + e^{35}, e^{24} + e^{36} + e^{15}$                      | 369      |
| 963:87       | $0, 0, 0, a_1e^{12}, e^{13}a_2, e^{23}, -(a_1 - a_2)e^{16} + e^{34} + e^{25}, e^{35} + e^{26} + a_4e^{14}, e^{24} + e^{36} + e^{15}$ | 369      |
| Type: 411111 |                                                                                                                                      |          |
| 954321:1     | $0, 0, 0, 0, e^{12}, e^{15}, e^{16}, e^{17}, e^{18}$                                                                                 | 345679   |
| 954321:2     | $0, 0, 0, 0, e^{12}, e^{15}, e^{16}, e^{17}, e^{18} + e^{34}$                                                                        | 145679   |
| 954321:3     | $0, 0, 0, 0, e^{12}, e^{15}, e^{16}, e^{17}, e^{18} + e^{23}$                                                                        | 245679   |
| 954321:4     | $0, 0, 0, 0, e^{12}, e^{15}, e^{16}, e^{17}, e^{18} + e^{25}$                                                                        | 345679   |
| 954321:5     | $0, 0, 0, 0, -e^{12}, e^{15}, e^{16}, e^{17} + e^{23}, e^{35} + e^{18}$                                                              | 235679   |
| 954321:6     | $0, 0, 0, 0, e^{12}, e^{15}, e^{16}, e^{17}, e^{18} + e^{34} + e^{25}$                                                               | 145679   |
| 954321:7     | $0, 0, 0, 0, -e^{12}, e^{15}, e^{16} + e^{23}, e^{17} + e^{35}, e^{18} + e^{36}$                                                     | 234679   |
| 954321:8     | $0, 0, 0, 0, -e^{12}, e^{15}, e^{16}, e^{23} + e^{17}, e^{35} + e^{24} + e^{18}$                                                     | 135679   |
| 954321:9     | $0, 0, 0, 0, e^{12}, e^{15}, e^{16}, e^{25} + e^{17}, e^{18} + e^{26}$                                                               | 345679   |
| 954321:11    | $0, 0, 0, 0, -e^{12}, e^{15}, e^{16}, e^{17}, e^{56} + e^{27} + e^{18}$                                                              | 345679   |
| 954321:12    | $0, 0, 0, 0, e^{12}, e^{15}, e^{16}, e^{25} + e^{17}, e^{26} + e^{34} + e^{18}$                                                      | 145679   |
| 954321:13    | $0, 0, 0, 0, -e^{12}, e^{15}, e^{16} + e^{23}, e^{17} + e^{35}, e^{18} + e^{36} + e^{24}$                                            | 134679   |
| 954321:16    | $0, 0, 0, 0, -e^{12}, e^{15}, e^{16}, e^{17}, e^{56} + e^{27} + e^{18} + e^{34}$                                                     | 145679   |
| 954321:18    | $0, 0, 0, 0, -e^{12}, e^{15}, e^{23} + e^{16}, e^{17} + e^{35}, e^{18} + e^{25} + e^{36}$                                            | 234679   |
| 954321:19    | $0, 0, 0, 0, e^{12}, e^{15}, e^{25} + e^{16}, e^{26} + e^{17}, e^{18} + e^{56}$                                                      | 345679   |
| 954321:20    | $0, 0, 0, 0, e^{12}, e^{15}, e^{16} + e^{25}, e^{17} + e^{26}, e^{18} + e^{27}$                                                      | 345679   |
| 954321:22    | $0, 0, 0, 0, -e^{12}, e^{15}, e^{23} + e^{16}, e^{35} + e^{17} + e^{24}, e^{45} + e^{36} + e^{18}$                                   | 124679   |
| 954321:24    | $0, 0, 0, 0, e^{12}, e^{15}, e^{25} + e^{16}, e^{26} + e^{17}, e^{34} + e^{18} + e^{56}$                                             | 145679   |
| 954321:25    | $0, 0, 0, 0, e^{12}, e^{15}, e^{16} + e^{25}, e^{17} + e^{26}, e^{18} + e^{34} + e^{27}$                                             | 145679   |
| 954321:30    | $0, 0, 0, 0, e^{12}, e^{15}, e^{25} + e^{16}, e^{26} + e^{17}, e^{18} + e^{56} + e^{23}$                                             | 245679   |
| 954321:31    | $0, 0, 0, 0, -e^{12}, e^{15} + e^{23}, e^{35} + e^{16}, e^{36} + e^{17}, e^{37} + e^{18}$                                            | 234579   |
| 954321:34    | $0, 0, 0, 0, (-1 + a_3)e^{12}, e^{15}, e^{25} + e^{16}a_3, e^{17} + e^{26}, e^{18} + e^{27} + e^{56}$                                | 345679   |
| 954321:37    | $0, 0, 0, 0, -e^{12}, e^{15} + e^{23}, e^{35} + e^{16}, e^{17} + e^{36}, e^{18} + e^{37} + e^{24}$                                   | 134579   |
| 954321:38    | $0, 0, 0, 0, a_1e^{12}, e^{15}, -(-1 + a_1)e^{16} + e^{25}, e^{26} + e^{17}, e^{18} + e^{56} + e^{34} + e^{27}$                      | 145679   |
| 954321:40    | $0, 0, 0, 0, -e^{12}, e^{15} + e^{23}, e^{16} + e^{35}, e^{17} + e^{36}, e^{25} + e^{37} + e^{18}$                                   | 234579   |
| 954321:42    | $0, 0, 0, 0, -e^{12}, e^{15} + e^{23}, e^{16} + e^{35}, e^{24} + e^{17} + e^{36}, e^{37} + e^{45} + e^{18}$                          | 124579   |
| 954321:48    | $0, 0, 0, 0, -e^{12}, e^{15} + e^{23}, e^{16} + e^{24} + e^{35}, e^{17} + e^{45} + e^{36}, e^{37} + e^{18} + e^{46}$                 | 123579   |
| 954321:51    | $0, 0, 0, 0, -e^{12}, e^{15} + e^{23}, e^{35} + e^{16}, e^{17} + e^{36} + e^{25}, e^{18} + e^{37} + e^{26}$                          | 234579   |
| 954321:52    | $0, 0, 0, 0, -e^{12}, e^{15} + e^{23}, e^{35} + e^{16} + e^{24}, e^{17} + e^{45} + e^{36}, e^{18} + e^{37} + e^{46} + e^{25}$        | 123579   |
| Type: 41112  |                                                                                                                                      |          |
| 95432:1      | $0, 0, 0, 0, -e^{12}, e^{15}, e^{16}, e^{17}, e^{27} + e^{56}$                                                                       | 45679    |
| 95432:2      | $0, 0, 0, 0, -e^{12}, e^{15}, e^{16}, e^{17}, e^{27} + e^{34} + e^{56}$                                                              | 25679    |
| 95432:3      | $0, 0, 0, 0, -e^{12}, e^{15}, e^{16}, e^{34} + e^{17}, e^{56} + e^{27}$                                                              | 25679    |
| 95432:4      | $0, 0, 0, 0, -e^{12}, e^{15}, e^{16}, e^{17}, e^{13} + e^{27} + e^{56}$                                                              | 35679    |
| 95432:5      | $0, 0, 0, 0, -e^{12}, e^{15}, e^{16}, e^{23} + e^{17}, e^{56} + e^{27}$                                                              | 35679    |
| 95432:6      | $0, 0, 0, 0, -e^{12}, e^{15}, e^{16}, e^{17} + e^{23}, e^{56} + e^{27} + e^{34}$                                                     | 25679    |
| 95432:7      | $0, 0, 0, 0, -e^{12}, e^{15}, e^{16}, e^{17} + e^{34}, e^{27} + e^{13} + e^{56}$                                                     | 25679    |
| 95432:8      | $0, 0, 0, 0, -e^{12}, e^{15}, e^{16}, e^{17} + e^{25}, e^{56} + e^{27}$                                                              | 45679    |
| 95432:9      | $0, 0, 0, 0, -e^{12}, e^{15}, e^{23} + e^{16}, e^{17} + e^{35}, e^{27} + e^{56}$                                                     | 34679    |
| 95432:10a    | $0, 0, 0, 0, -e^{12}, e^{15}, e^{16}, e^{17} + e^{23}, e^{56} + e^{27} + e^{13}$                                                     | 35679    |
| 95432:10b    | $0, 0, 0, 0, -e^{12}, e^{15}, e^{16}, e^{23} - e^{17}, e^{13} + e^{27} + e^{56}$                                                     | 35679    |
| 95432:11     | $0, 0, 0, 0, -e^{12}, e^{15}, e^{16}, e^{23} + e^{17}, e^{14} + e^{56} + e^{27}$                                                     | 25679    |

Table 2 – Continued to next page

Table 2 – Continued from previous page

| Name        | $\mathfrak{g}$                                                                                      | UCS Dim. |
|-------------|-----------------------------------------------------------------------------------------------------|----------|
| 95432:12    | $0, 0, 0, 0, -e^{12}, e^{15}, e^{16}, e^{17} + e^{25}, e^{27} + e^{34} + e^{56}$                    | 25679    |
| 95432:13    | $0, 0, 0, 0, -e^{12}, e^{15}, e^{16}, e^{34} + e^{17} + e^{25}, e^{56} + e^{27}$                    | 25679    |
| 95432:14    | $0, 0, 0, 0, -e^{12}, e^{15}, e^{23} + e^{16}, e^{35} + e^{17}, e^{56} + e^{27} + e^{34}$           | 24679    |
| 95432:15    | $0, 0, 0, 0, -e^{12}, e^{15}, e^{16}, e^{17} + e^{25}, e^{56} + e^{27} + e^{13}$                    | 35679    |
| 95432:16    | $0, 0, 0, 0, -e^{12}, e^{15}, e^{23} + e^{16}, e^{35} + e^{17}, e^{56} + e^{27} + e^{13}$           | 34679    |
| 95432:17    | $0, 0, 0, 0, -e^{12}, e^{15}, e^{23} + e^{16}, e^{17} + e^{35}, e^{14} + e^{56} + e^{27}$           | 24679    |
| 95432:18    | $0, 0, 0, 0, -e^{12}, e^{15}, e^{23} + e^{16}, e^{17} + e^{24} + e^{35}, e^{27} + e^{56}$           | 24679    |
| 95432:19    | $0, 0, 0, 0, -e^{12}, e^{15}, e^{25} + e^{16}, e^{17} + e^{26}, e^{27} + e^{56}$                    | 45679    |
| 95432:20    | $0, 0, 0, 0, -e^{12}, e^{15}, e^{16}, e^{17} + e^{25} + e^{34}, e^{27} + e^{13} + e^{56}$           | 25679    |
| 95432:21a   | $0, 0, 0, 0, -e^{12}, e^{15}, e^{23} + e^{16}, e^{35} + e^{24} + e^{17}, e^{27} + e^{34} + e^{56}$  | 24679    |
| 95432:21b   | $0, 0, 0, 0, -e^{12}, -e^{15}, e^{16} + e^{23}, e^{17} + e^{35} + e^{24}, e^{27} + e^{34} + e^{56}$ | 24679    |
| 95432:22    | $0, 0, 0, 0, -e^{12}, e^{15}, e^{16} + e^{25}, e^{17} + e^{26}, e^{56} + e^{27} + e^{34}$           | 25679    |
| 95432:23    | $0, 0, 0, 0, -e^{12}, e^{15}, e^{16} + e^{25}, e^{17} + e^{26} + e^{34}, e^{27} + e^{56}$           | 25679    |
| 95432:24a   | $0, 0, 0, 0, e^{12}, e^{15}, e^{23} - e^{16}, e^{24} - e^{17} + e^{35}, e^{14} + e^{56} + e^{27}$   | 24679    |
| 95432:24b   | $0, 0, 0, 0, -e^{12}, e^{15}, e^{16} + e^{23}, e^{17} + e^{35} + e^{24}, e^{27} + e^{56} + e^{14}$  | 24679    |
| 95432:25    | $0, 0, 0, 0, -e^{12}, e^{15}, e^{23} + e^{16}, e^{35} + e^{24} + e^{17}, e^{56} + e^{13} + e^{27}$  | 24679    |
| 95432:26    | $0, 0, 0, 0, -e^{12}, e^{15}, e^{16} + e^{25}, e^{17} + e^{26}, e^{27} + e^{13} + e^{56}$           | 35679    |
| 95432:28    | $0, 0, 0, 0, -e^{12}, e^{15}, e^{16} + e^{25}, e^{17} + e^{26} + e^{34}, e^{56} + e^{13} + e^{27}$  | 25679    |
| Type: 41211 |                                                                                                     |          |
| 95421:1     | $0, 0, 0, 0, e^{12}, e^{15}, e^{25}, e^{16}, e^{18}$                                                | 45679    |
| 95421:2     | $0, 0, 0, 0, e^{12}, e^{15}, e^{25} + e^{34}, e^{16}, e^{18}$                                       | 25679    |
| 95421:3     | $0, 0, 0, 0, e^{12}, e^{15}, e^{25} + e^{13}, e^{16}, e^{18}$                                       | 35679    |
| 95421:4     | $0, 0, 0, 0, e^{12}, e^{15}, e^{25}, e^{16}, e^{34} + e^{18}$                                       | 25679    |
| 95421:5     | $0, 0, 0, 0, e^{12}, e^{15}, e^{25}, e^{16}, e^{23} + e^{18}$                                       | 35679    |
| 95421:6     | $0, 0, 0, 0, e^{12}, e^{15}, e^{13} + e^{25}, e^{16}, e^{18} + e^{34}$                              | 25679    |
| 95421:7     | $0, 0, 0, 0, e^{12}, e^{15}, e^{25} + e^{34}, e^{16}, e^{23} + e^{18}$                              | 25679    |
| 95421:8a    | $0, 0, 0, 0, e^{12}, e^{15}, e^{13} + e^{25}, e^{16}, e^{18} + e^{23}$                              | 35679    |
| 95421:8b    | $0, 0, 0, 0, e^{12}, -e^{15}, e^{13} + e^{25}, e^{16}, e^{18} + e^{23}$                             | 35679    |
| 95421:9     | $0, 0, 0, 0, e^{12}, e^{15}, e^{25} + e^{13}, e^{16}, e^{18} + e^{24}$                              | 25679    |
| 95421:10    | $0, 0, 0, 0, e^{12}, e^{15}, e^{25}, e^{16}, e^{18} + e^{27}$                                       | 35679    |
| 95421:11    | $0, 0, 0, 0, -e^{12}, e^{15}, e^{25}, e^{16}, e^{56} + e^{28}$                                      | 45679    |
| 95421:12    | $0, 0, 0, 0, -e^{12}, e^{15}, e^{25} + e^{34}, e^{16}, e^{28} + e^{56}$                             | 25679    |
| 95421:13    | $0, 0, 0, 0, -e^{12}, e^{15}, e^{25}, e^{16} + e^{23}, e^{18} + e^{35}$                             | 34679    |
| 95421:14    | $0, 0, 0, 0, -e^{12}, e^{15}, e^{25} + e^{34}, e^{16} + e^{23}, e^{18} + e^{35}$                    | 24679    |
| 95421:15    | $0, 0, 0, 0, e^{12}, e^{15}, e^{25}, e^{16}, e^{18} + e^{27} + e^{34}$                              | 15679    |
| 95421:16    | $0, 0, 0, 0, -e^{12}, e^{15}, e^{13} + e^{25}, e^{16}, e^{56} + e^{28}$                             | 35679    |
| 95421:17    | $0, 0, 0, 0, -e^{12}, e^{15}, e^{25}, e^{16}, e^{28} + e^{56} + e^{34}$                             | 25679    |
| 95421:18    | $0, 0, 0, 0, -e^{12}, e^{15}, e^{25} + e^{13}, e^{16} + e^{23}, e^{18} + e^{35}$                    | 34679    |
| 95421:19    | $0, 0, 0, 0, -e^{12}, e^{15}, e^{13} + e^{25}, e^{16} + e^{24}, e^{45} + e^{18}$                    | 24679    |
| 95421:20    | $0, 0, 0, 0, -e^{12}, e^{15}, e^{25}, e^{23} + e^{16}, e^{28} + e^{56}$                             | 34679    |
| 95421:21    | $0, 0, 0, 0, -e^{12}, e^{15}, e^{25} + e^{34}, e^{23} + e^{16}, e^{56} + e^{28}$                    | 24679    |
| 95421:22    | $0, 0, 0, 0, -e^{12}, e^{15}, e^{25}, e^{16}, e^{28} + e^{13} + e^{56}$                             | 35679    |
| 95421:23    | $0, 0, 0, 0, -e^{12}, e^{15}, e^{13} + e^{25}, e^{16}, e^{34} + e^{56} + e^{28}$                    | 25679    |
| 95421:24    | $0, 0, 0, 0, -e^{12}, e^{15}, e^{25} + e^{34}, e^{16}, e^{56} + e^{13} + e^{28}$                    | 25679    |
| 95421:25    | $0, 0, 0, 0, -e^{12}, e^{15}, e^{25}, e^{23} + e^{16}, e^{18} + e^{35} + e^{24}$                    | 24679    |
| 95421:26a   | $0, 0, 0, 0, -e^{12}, e^{15}, e^{25} + e^{34}, e^{16} + e^{23}, e^{18} + e^{35} + e^{24}$           | 24679    |
| 95421:26b   | $0, 0, 0, 0, -e^{12}, e^{15}, -e^{25} + e^{34}, e^{23} + e^{16}, e^{18} + e^{24} + e^{35}$          | 24679    |
| 95421:27    | $0, 0, 0, 0, -e^{12}, e^{15}, e^{13} + e^{25}, e^{23} + e^{16}, e^{28} + e^{56}$                    | 34679    |
| 95421:28    | $0, 0, 0, 0, e^{12}, e^{15}, e^{13} + e^{25}, e^{16} + e^{23}, e^{18} + e^{27}$                     | 24679    |
| 95421:29    | $0, 0, 0, 0, -e^{12}, e^{15}, e^{25}, e^{16} + e^{23}, e^{56} + e^{28} + e^{34}$                    | 24679    |
| 95421:30    | $0, 0, 0, 0, -e^{12}, e^{15}, e^{13} + e^{25}, e^{16} + e^{24}, e^{28} + e^{56}$                    | 24679    |
| 95421:31    | $0, 0, 0, 0, -e^{12}, e^{15}, e^{13} + e^{25}, e^{16}, e^{56} + e^{14} + e^{28}$                    | 25679    |
| 95421:32a   | $0, 0, 0, 0, -e^{12}, e^{15}, e^{13} + e^{25}, e^{16} + e^{24}, e^{18} + e^{45} + e^{23}$           | 24679    |
| 95421:32b   | $0, 0, 0, 0, -e^{12}, -e^{15}, e^{25} + e^{13}, e^{16} + e^{24}, e^{18} + e^{45} + e^{23}$          | 24679    |
| 95421:33    | $0, 0, 0, 0, -e^{12}, e^{15}, e^{13} + e^{25}, e^{23} + e^{16}, e^{18} + e^{24} + e^{35}$           | 24679    |
| 95421:34    | $0, 0, 0, 0, -e^{12}, e^{15}, e^{25}, e^{23} + e^{16}, e^{13} + e^{28} + e^{56}$                    | 34679    |
| 95421:35    | $0, 0, 0, 0, -e^{12}, e^{15}, e^{25}, e^{23} + e^{16}, e^{14} + e^{56} + e^{28}$                    | 24679    |
| 95421:36    | $0, 0, 0, 0, e^{12}, e^{15}, e^{25} + e^{13}, e^{16}, e^{18} + e^{27} + e^{35}$                     | 24679    |

Table 2 – Continued to next page

Table 2 – Continued from previous page

| Name       | $\mathfrak{g}$                                                                                                                       | UCS Dim. |
|------------|--------------------------------------------------------------------------------------------------------------------------------------|----------|
| 95421:37   | $0, 0, 0, 0, -e^{12}, e^{15}, e^{25} + a_2 e^{13}, e^{16} + e^{24}, e^{34} + e^{56} + e^{28}$                                        | 24679    |
| 95421:38a  | $0, 0, 0, 0, e^{12}, e^{15}, e^{34} + e^{25}, e^{23} - e^{16}, e^{28} + e^{56} + e^{14}$                                             | 24679    |
| 95421:38b  | $0, 0, 0, 0, -e^{12}, e^{15}, e^{34} + e^{25}, e^{23} + e^{16}, e^{14} + e^{28} + e^{56}$                                            | 24679    |
| 95421:39   | $0, 0, 0, 0, -e^{12}, e^{15}, e^{13} + e^{25}, e^{23} + e^{16}, e^{34} + e^{56} + e^{28}$                                            | 24679    |
| 95421:40   | $0, 0, 0, 0, -e^{12}, e^{15}, e^{25} + e^{34}, e^{23} + e^{16}, e^{13} + e^{28} + e^{56}$                                            | 24679    |
| 95421:41   | $0, 0, 0, 0, e^{12}, e^{15}, e^{13} + e^{25}, e^{16} + e^{23}, e^{18} + e^{34} + e^{27}$                                             | 14679    |
| 95421:42   | $0, 0, 0, 0, -e^{12}, e^{15}, e^{25}, e^{16} + e^{23}, e^{27} + e^{18} + e^{35}$                                                     | 24679    |
| 95421:43   | $0, 0, 0, 0, -e^{12}, e^{15}, e^{13} + e^{25}, e^{23} + e^{16}, e^{28} + e^{14} + e^{56}$                                            | 24679    |
| 95421:44   | $0, 0, 0, 0, -e^{12}, e^{15}, e^{13} + e^{25}, e^{24} + e^{16}, e^{56} + e^{14} + e^{28}$                                            | 24679    |
| 95421:45   | $0, 0, 0, 0, e^{12}(-1 + a_2), e^{15}, a_2 e^{13} + e^{25}, e^{16} + e^{23}, e^{27} + e^{35} + e^{18}$                               | 24679    |
| 95421:46   | $0, 0, 0, 0, e^{12}, e^{25} + e^{13}, e^{15}, e^{26} + e^{35}, e^{28} + e^{36}$                                                      | 34579    |
| 95421:47   | $0, 0, 0, 0, e^{12}, e^{13} + e^{25}, e^{34} + e^{15}, e^{26} + e^{35}, e^{28} + e^{36}$                                             | 24579    |
| 95421:48   | $0, 0, 0, 0, -e^{12}, e^{15} + e^{23}, e^{25} + e^{14}, e^{35} + e^{16}, e^{36} + e^{18}$                                            | 24579    |
| 95421:49a  | $0, 0, 0, 0, -e^{12}, e^{15} + e^{23}, e^{13} + e^{25}, e^{35} + e^{16}, e^{18} + e^{36}$                                            | 34579    |
| 95421:49b  | $0, 0, 0, 0, -e^{12}, e^{15} + e^{23}, -e^{13} + e^{25}, e^{16} + e^{35}, e^{18} + e^{36}$                                           | 34579    |
| 95421:52   | $0, 0, 0, 0, e^{12}, e^{13} + e^{25}, e^{15}, e^{26} + e^{35}, e^{36} + e^{14} + e^{28}$                                             | 24579    |
| 95421:53   | $0, 0, 0, 0, e^{12}, e^{25} + e^{13}, e^{15} + e^{34}, e^{26} + e^{35}, e^{28} + e^{14} + e^{36}$                                    | 24579    |
| 95421:59a  | $0, 0, 0, 0, -e^{12}, e^{15} + e^{23}, e^{25} + e^{14}, e^{35} + e^{16}, e^{36} + e^{18} + e^{24}$                                   | 24579    |
| 95421:59b  | $0, 0, 0, 0, -e^{12}, e^{15} + e^{23}, e^{25} - e^{14}, e^{16} + e^{35}, e^{24} + e^{18} + e^{36}$                                   | 24579    |
| 95421:60a  | $0, 0, 0, 0, -e^{12}, e^{15} + e^{23}, e^{13} + e^{25}, e^{35} + e^{16}, e^{36} + e^{18} + e^{24}$                                   | 24579    |
| 95421:60b  | $0, 0, 0, 0, -e^{12}, e^{15} + e^{23}, -e^{13} + e^{25}, e^{35} + e^{16}, e^{18} + e^{36} + e^{24}$                                  | 24579    |
| 95421:67   | $0, 0, 0, 0, e^{12}, e^{13} + e^{25}, e^{15}, e^{26} + e^{35}, e^{36} + e^{17} + e^{28}$                                             | 24579    |
| 95421:68   | $0, 0, 0, 0, e^{12}, e^{25} + e^{13}, 2e^{15}, e^{26} + e^{35}, e^{37} + e^{18} + e^{56}$                                            | 24579    |
| 95421:72   | $0, 0, 0, 0, e^{12}, e^{13} + e^{25}, e^{15}, e^{26} + e^{35} + e^{14}, e^{28} + e^{45} + e^{36}$                                    | 23579    |
| 95421:73a  | $0, 0, 0, 0, e^{12}, e^{13} + e^{25}, e^{34} + e^{15}, e^{26} + e^{35} + e^{14}, e^{36} + e^{28} + e^{45}$                           | 23579    |
| 95421:73b  | $0, 0, 0, 0, e^{12}, e^{13} + e^{25}, e^{34} - e^{15}, e^{26} + e^{35} + e^{14}, e^{28} + e^{45} + e^{36}$                           | 23579    |
| 95421:74   | $0, 0, 0, 0, e^{12}, e^{13} + e^{25}, e^{34} + 2e^{15}, e^{26} + e^{35}, e^{37} + e^{18} + e^{56}$                                   | 13579    |
| 95421:79   | $0, 0, 0, 0, -e^{12}, e^{15} + e^{23}, e^{25} + e^{14}, e^{16} + e^{24} + e^{35}, e^{18} + e^{45} + e^{36}$                          | 23579    |
| 95421:82a  | $0, 0, 0, 0, -e^{12}, e^{15} + e^{23}, e^{13} + e^{25}, e^{35} + e^{16} + e^{24}, e^{45} + e^{36} + e^{18}$                          | 23579    |
| 95421:82b  | $0, 0, 0, 0, -e^{12}, e^{15} + e^{23}, -e^{13} + e^{25}, e^{35} + e^{16} + e^{24}, e^{45} + e^{36} + e^{18}$                         | 23579    |
| 95421:85a  | $0, 0, 0, 0, -e^{12}, e^{15} + e^{23}, e^{13} + 2e^{25}, e^{16} + e^{35}, e^{28} + e^{37} + e^{56}$                                  | 24579    |
| 95421:85b  | $0, 0, 0, 0, -e^{12}, -e^{15} + e^{23}, e^{13} + 2e^{25}, e^{16} + e^{35}, e^{28} + e^{37} + e^{56}$                                 | 24579    |
| 95421:86   | $0, 0, 0, 0, e^{12}, e^{25} + e^{13}, 2e^{15}, e^{14} + e^{26} + e^{35}, e^{37} + e^{18} + e^{56}$                                   | 13579    |
| 95421:87a  | $0, 0, 0, 0, e^{12}, e^{25} + e^{13}, 2e^{15} + e^{34}, e^{14} + e^{26} + e^{35}, e^{56} + e^{37} + e^{18}$                          | 13579    |
| 95421:87b  | $0, 0, 0, 0, e^{12}, e^{25} + e^{13}, 2e^{15} + e^{34}, -e^{14} + e^{26} + e^{35}, e^{56} + e^{37} + e^{18}$                         | 13579    |
| 95421:88   | $0, 0, 0, 0, e^{12}, e^{25} + e^{13}, 2e^{15}, e^{26} + e^{35}, e^{24} + e^{37} + e^{18} + e^{56}$                                   | 14579    |
| 95421:91   | $0, 0, 0, 0, -e^{12}, e^{15} + e^{23}, e^{25} + e^{14}, e^{16} + e^{24} + e^{35}, e^{18} + e^{27} + e^{36}$                          | 13579    |
| 95421:92   | $0, 0, 0, 0, e^{12}, e^{25} + e^{13}, 2e^{15} + e^{34}, e^{26} + e^{35}, e^{24} + e^{37} + e^{18} + e^{56}$                          | 13579    |
| 95421:93a  | $0, 0, 0, 0, e^{12}, e^{25} + e^{13}, 2e^{15} + e^{23}, e^{14} + e^{26} + e^{35}, e^{37} + e^{18} + e^{56}$                          | 13579    |
| 95421:93b  | $0, 0, 0, 0, e^{12}, -e^{25} + e^{13}, 2e^{15} + e^{23}, e^{14} + e^{26} + e^{35}, e^{56} + e^{37} + e^{18}$                         | 13579    |
| 95421:94a  | $0, 0, 0, 0, -e^{12}, e^{15} + e^{23}, e^{13} + 2e^{25}, e^{16} + e^{35}, e^{28} + e^{14} + e^{37} + e^{56}$                         | 14579    |
| 95421:94b  | $0, 0, 0, 0, -e^{12}, -e^{15} + e^{23}, e^{13} + 2e^{25}, e^{35} + e^{16}, e^{37} + e^{56} + e^{28} + e^{14}$                        | 14579    |
| 95421:95   | $0, 0, 0, 0, -e^{12}, e^{15} + e^{23}, e^{25} - e^{14}, e^{35} + e^{16}, e^{18} + e^{27} + e^{45} + e^{36}$                          | 13579    |
| 95421:96   | $0, 0, 0, 0, e^{12}, e^{25} + e^{13}, e^{15}, e^{14} + e^{26} + e^{35}, e^{45} + e^{28} + e^{17} + e^{36}$                           | 13579    |
| 95421:97   | $0, 0, 0, 0, e^{12}, e^{25} + e^{13}, 2e^{15}, e^{14} + e^{26} + e^{35}, e^{24} + e^{37} + e^{18} + e^{56}$                          | 13579    |
| 95421:98a  | $0, 0, 0, 0, e^{12}, e^{25} + e^{13}, 2e^{15} + e^{34}, e^{14} + e^{26} + e^{35}, e^{24} + e^{37} + e^{18} + e^{56}$                 | 13579    |
| 95421:98b  | $0, 0, 0, 0, e^{12}, e^{25} + e^{13}, 2e^{15} + e^{34}, -e^{14} + e^{26} + e^{35}, e^{24} + e^{37} + e^{18} + e^{56}$                | 13579    |
| 95421:99   | $0, 0, 0, 0, -e^{12}a_4, e^{15} + e^{23}, e^{25} - (-1 + a_4)e^{14}, e^{24} + e^{35} + e^{16}a_4, e^{18} + e^{27} + e^{45} + e^{36}$ | 13579    |
| 95421:100a | $0, 0, 0, 0, -e^{12}, e^{15} + e^{23}, e^{13} + 2e^{25}, e^{35} + e^{16} + e^{24}, e^{37} + e^{56} + e^{28} + e^{14}$                | 13579    |
| 95421:100b | $0, 0, 0, 0, -e^{12}, -e^{15} + e^{23}, e^{13} + 2e^{25}, e^{35} + e^{16} + e^{24}, e^{37} + e^{56} + e^{28} + e^{14}$               | 13579    |
| 95421:101  | $0, 0, 0, 0, e^{12}, e^{15}, e^{25}, e^{17} + e^{26}, e^{56} + e^{18}$                                                               | 34679    |
| 95421:102a | $0, 0, 0, 0, -e^{12}, e^{15}, e^{25}, e^{16} + e^{27}, e^{56} + e^{28}$                                                              | 34679    |
| 95421:102b | $0, 0, 0, 0, -e^{12}, -e^{15}, e^{25}, e^{27} + e^{16}, e^{56} + e^{28}$                                                             | 34679    |
| 95421:103  | $0, 0, 0, 0, e^{12}, e^{15}, e^{25}, e^{17} + e^{26}, e^{18} + e^{34} + e^{56}$                                                      | 14679    |
| 95421:104a | $0, 0, 0, 0, -e^{12}, e^{15}, e^{25}, e^{27} + e^{16}, e^{28} + e^{56} + e^{34}$                                                     | 14679    |
| 95421:104b | $0, 0, 0, 0, -e^{12}, -e^{15}, e^{25}, e^{27} + e^{16}, e^{56} + e^{28} + e^{34}$                                                    | 14679    |
| 95421:105a | $0, 0, 0, 0, -e^{12}, e^{15}, e^{25}, e^{27} + e^{16}, e^{28} + e^{13} + e^{56}$                                                     | 24679    |
| 95421:105b | $0, 0, 0, 0, -e^{12}, -e^{15}, e^{25}, e^{27} + e^{16}, e^{13} + e^{28} + e^{56}$                                                    | 24679    |

Table 2 – Continued to next page

Table 2 – Continued from previous page

| Name        | $\mathfrak{g}$                                                                                                                            | UCS Dim. |
|-------------|-------------------------------------------------------------------------------------------------------------------------------------------|----------|
| 95421:106   | $0, 0, 0, 0, e^{12}, e^{15}, e^{25}, e^{26} + e^{17}, e^{18} + e^{56} + e^{23}$                                                           | 24679    |
| 95421:107   | $0, 0, 0, 0, -e^{12}, e^{15}, e^{25}, e^{17} + e^{26}, e^{57} + e^{28} + e^{16}$                                                          | 34679    |
| 95421:108   | $0, 0, 0, 0, e^{12}, e^{15}, e^{13} + e^{25}, e^{26} + e^{17}, e^{18} + e^{56}$                                                           | 23579    |
| 95421:109   | $0, 0, 0, 0, -e^{12}, e^{15}, e^{25}, e^{17} + e^{26}, e^{57} + e^{34} + e^{28} + e^{16}$                                                 | 14679    |
| 95421:110   | $0, 0, 0, 0, e^{12}, e^{15}, e^{13} + e^{25}, e^{26} + e^{17}, e^{18} + e^{56} + e^{34}$                                                  | 13579    |
| 95421:112   | $0, 0, 0, 0, e^{12}, e^{15}, e^{25} + e^{13}, e^{17} + e^{26}, e^{24} + e^{18} + e^{56}$                                                  | 13579    |
| 95421:113   | $0, 0, 0, 0, e^{12}, e^{15}, e^{13} + e^{25}, e^{26} + e^{17}, e^{18} + e^{56} + e^{23}$                                                  | 23579    |
| 95421:114   | $0, 0, 0, 0, -e^{12}, e^{15}, e^{13} + e^{25}, e^{17} + e^{26}, e^{57} + e^{36} + e^{28}$                                                 | 23579    |
| 95421:116a  | $0, 0, 0, 0, e^{12}, -e^{13} + e^{25}, e^{15} + e^{23}, e^{26} + e^{35} - 2e^{17}, e^{56} + e^{18}$                                       | 23579    |
| 95421:116b  | $0, 0, 0, 0, e^{12}, e^{25} - e^{13}, e^{23} - e^{15}, -2e^{17} + e^{26} + e^{35}, e^{18} + e^{56}$                                       | 23579    |
| 95421:119a  | $0, 0, 0, 0, e^{12}, e^{15} + e^{23}, e^{25} + e^{13}, e^{16} + e^{27}, e^{36} + e^{18} + e^{57}$                                         | 23579    |
| 95421:119b  | $0, 0, 0, 0, e^{12}, -e^{15} - e^{23}, -e^{13} + e^{25}, e^{27} + e^{16}, e^{36} + e^{57} + e^{18}$                                       | 23579    |
| 95421:120a  | $0, 0, 0, 0, e^{12}, e^{25} + e^{13}, e^{15} + e^{23}, e^{16} + e^{27}, e^{57} + e^{36} + e^{18}$                                         | 23579    |
| 95421:120b  | $0, 0, 0, 0, e^{12}, e^{25} - e^{13}, e^{15} + e^{23}, e^{16} + e^{27}, e^{36} + e^{18} + e^{57}$                                         | 23579    |
| 95421:121a  | $0, 0, 0, 0, e^{12}, e^{25} - e^{13}, e^{23} + e^{15}, -2e^{17} + e^{26} + e^{35}, e^{18} + e^{56} + e^{34}$                              | 13579    |
| 95421:121b  | $0, 0, 0, 0, e^{12}, -e^{13} + e^{25}, -e^{15} + e^{23}, e^{26} + e^{35} - 2e^{17}, e^{56} + e^{18} + e^{34}$                             | 13579    |
| 95421:122a  | $0, 0, 0, 0, e^{12}, 2e^{15}, e^{25} + e^{13}, e^{16} + e^{27} + e^{35}, e^{57} + e^{36} + e^{18}$                                        | 23579    |
| 95421:122b  | $0, 0, 0, 0, e^{12}, 2e^{15}, e^{25} + e^{13}, -e^{16} + e^{27} + e^{35}, e^{36} + e^{18} + e^{57}$                                       | 23579    |
| 95421:123a  | $0, 0, 0, 0, -e^{12}, e^{15}, -e^{13} + e^{25}, e^{35} + e^{27} + e^{16}, e^{37} + e^{28} + e^{56}$                                       | 23579    |
| 95421:123b  | $0, 0, 0, 0, -e^{12}, -e^{15}, -e^{13} + e^{25}, e^{35} + e^{27} + e^{16}, e^{56} + e^{37} + e^{28}$                                      | 23579    |
| 95421:124   | $0, 0, 0, 0, -e^{12}, e^{15}, e^{13} + e^{25}, e^{17} + e^{26}, e^{57} + e^{36} + e^{28} + e^{14}$                                        | 13579    |
| 95421:125a  | $0, 0, 0, 0, -e^{12}, e^{15} - e^{23}, e^{25} - 2e^{13}, e^{27} + e^{16} + e^{35}, e^{56} + e^{28} + e^{14}$                              | 13579    |
| 95421:125b  | $0, 0, 0, 0, -e^{12}, -e^{15} - e^{23}, e^{25} - 2e^{13}, e^{27} + e^{16} + e^{35}, e^{28} + e^{14} + e^{56}$                             | 13579    |
| 95421:126a  | $0, 0, 0, 0, e^{12}, e^{23}a_4 + e^{15}(2 + a_4), (1 + a_4)e^{13} + e^{25}, e^{16} + e^{27} + e^{35}, e^{36} + e^{18} + e^{57}$           | 23579    |
| 95421:126b  | $0, 0, 0, 0, e^{12}, -e^{15}(-2 + a_4) + e^{23}a_4, -(1 + a_4)e^{13} + e^{25}, -e^{16} + e^{27} + e^{35}, e^{57} + e^{36} + e^{18}$       | 23579    |
| 95421:127a  | $0, 0, 0, 0, -e^{12}, e^{15} + e^{23}, e^{13} + e^{25}, e^{27} + e^{16}, e^{37} + e^{56} + e^{28} + e^{14}$                               | 13579    |
| 95421:127b  | $0, 0, 0, 0, -e^{12}, -e^{15} + e^{23}, e^{13} + e^{25}, e^{27} + e^{16}, e^{28} + e^{14} + e^{37} + e^{56}$                              | 13579    |
| 95421:128a  | $0, 0, 0, 0, -e^{12}, e^{13} + e^{25}, e^{15} + e^{23}, e^{27} + e^{16}, e^{28} + e^{14} + e^{37} + e^{56}$                               | 13579    |
| 95421:128b  | $0, 0, 0, 0, -e^{12}, -e^{25} - e^{13}, -e^{15} + e^{23}, e^{27} + e^{16}, e^{28} + e^{37} + e^{14} + e^{56}$                             | 13579    |
| 95421:129a  | $0, 0, 0, 0, -e^{12}, e^{15}, -e^{13} + e^{25}, e^{35} + e^{27} + e^{16}, e^{56} + e^{37} + e^{14} + e^{28}$                              | 13579    |
| 95421:129b  | $0, 0, 0, 0, -e^{12}, -e^{15}, -e^{13} + e^{25}, e^{35} + e^{27} + e^{16}, e^{37} + e^{14} + e^{28} + e^{56}$                             | 13579    |
| 95421:130a  | $0, 0, 0, 0, e^{12}, 2e^{15}, e^{25} + e^{13}, e^{16} + e^{27} + e^{35}, e^{24} + e^{36} + e^{18} + e^{57}$                               | 13579    |
| 95421:130b  | $0, 0, 0, 0, e^{12}, 2e^{15}, e^{25} + e^{13}, -e^{16} + e^{27} + e^{35}, e^{24} + e^{36} + e^{18} + e^{57}$                              | 13579    |
| 95421:131   | $0, 0, 0, 0, e^{12}, e^{15} + e^{23}, e^{14} + e^{25}, e^{17} + e^{26} + e^{34}, e^{56} + e^{37} + e^{18}$                                | 12479    |
| 95421:132a  | $0, 0, 0, 0, -e^{12}, e^{23}(1 + a_2) + e^{15}, e^{25}(2 + a_2) + e^{13}a_2, e^{27} + e^{16} + e^{35}, e^{28} + e^{14} + e^{37} + e^{56}$ | 13579    |
| 95421:132b  | $0, 0, 0, 0, -e^{12}, e^{23}(1 + a_2) - e^{15}, e^{25}(2 + a_2) + e^{13}a_2, e^{35} + e^{27} + e^{16}, e^{37} + e^{56} + e^{28} + e^{14}$ | 13579    |
| 95421:133   | $0, 0, 0, 0, -e^{12}, e^{15} - e^{23}, e^{25} + e^{14}, e^{34} + e^{17} + e^{26}, e^{57} + e^{46} + e^{28} + e^{13}$                      | 12479    |
| Type: 42111 |                                                                                                                                           |          |
| 95321:1     | $0, 0, 0, 0, e^{12}, e^{34}, e^{15}, e^{17}, e^{18}$                                                                                      | 25679    |
| 95321:2     | $0, 0, 0, 0, e^{12}, e^{13}, e^{15}, e^{17}, e^{18}$                                                                                      | 35679    |
| 95321:3     | $0, 0, 0, 0, e^{12}, e^{13}, e^{25}, e^{27}, e^{28}$                                                                                      | 35679    |
| 95321:4     | $0, 0, 0, 0, e^{12}, e^{34}, e^{15}, e^{17}, e^{36} + e^{18}$                                                                             | 13679    |
| 95321:5     | $0, 0, 0, 0, e^{12}, e^{13}, e^{15}, e^{17}, e^{34} + e^{18}$                                                                             | 25679    |
| 95321:6     | $0, 0, 0, 0, e^{12}, e^{13}, e^{25}, e^{27}, e^{28} + e^{34}$                                                                             | 25679    |
| 95321:7     | $0, 0, 0, 0, e^{12}, e^{13} + e^{24}, e^{15}, e^{17}, e^{18}$                                                                             | 25679    |
| 95321:8     | $0, 0, 0, 0, e^{12}, e^{34}, e^{15}, e^{17}, e^{18} + e^{23}$                                                                             | 25679    |
| 95321:9     | $0, 0, 0, 0, e^{12}, e^{13}, e^{15}, e^{17}, e^{36} + e^{18}$                                                                             | 24679    |
| 95321:10a   | $0, 0, 0, 0, e^{12}, e^{13}, e^{25}, e^{27}, e^{36} + e^{28}$                                                                             | 24679    |
| 95321:10b   | $0, 0, 0, 0, -e^{12}, e^{13}, e^{25}, e^{27}, e^{28} + e^{36}$                                                                            | 24679    |
| 95321:11    | $0, 0, 0, 0, e^{12}, -e^{13}, e^{15}, e^{34} + e^{17}, e^{18} + e^{46}$                                                                   | 13679    |
| 95321:12    | $0, 0, 0, 0, e^{12}, e^{13}, e^{15}, e^{17}, e^{23} + e^{18}$                                                                             | 35679    |
| 95321:13    | $0, 0, 0, 0, e^{12}, e^{13}, e^{15}, e^{17}, e^{18} + e^{24}$                                                                             | 25679    |
| 95321:14    | $0, 0, 0, 0, e^{12}, e^{13}, e^{25}, e^{27}, e^{28} + e^{14}$                                                                             | 25679    |
| 95321:15    | $0, 0, 0, 0, e^{12}, e^{24} + e^{13}, e^{15}, e^{17}, e^{18} + e^{34}$                                                                    | 25679    |
| 95321:16    | $0, 0, 0, 0, e^{12}, e^{34}, e^{15}, e^{17}, e^{18} + e^{25}$                                                                             | 25679    |
| 95321:17    | $0, 0, 0, 0, e^{12}, e^{13}, e^{25}, e^{27}, e^{16} + e^{28}$                                                                             | 24679    |
| 95321:18    | $0, 0, 0, 0, e^{12}, e^{34}, e^{15}, e^{17}, e^{23} + e^{46} + e^{18}$                                                                    | 13679    |
| 95321:19    | $0, 0, 0, 0, -e^{12}, e^{34}, e^{15}, e^{17}, e^{28} + e^{57}$                                                                            | 25679    |

Table 2 – Continued to next page

Table 2 – Continued from previous page

| Name      | $\mathfrak{g}$                                                                            | UCS Dim. |
|-----------|-------------------------------------------------------------------------------------------|----------|
| 95321:20  | $0, 0, 0, 0, -e^{12}, e^{34}, e^{15}, e^{17} + e^{23}, e^{18} + e^{35}$                   | 24679    |
| 95321:21a | $0, 0, 0, 0, e^{12}, e^{14} + e^{23}, e^{15}, e^{17} + e^{34}, e^{36} + e^{18}$           | 13679    |
| 95321:21b | $0, 0, 0, 0, -e^{12}, e^{23} + e^{14}, e^{15}, e^{34} + e^{17}, e^{36} + e^{18}$          | 13679    |
| 95321:22  | $0, 0, 0, 0, e^{12}, e^{24} + e^{13}, e^{15}, e^{17}, e^{18} + e^{23}$                    | 25679    |
| 95321:23  | $0, 0, 0, 0, e^{12}, e^{13}, e^{15}, e^{17}, e^{25} + e^{18}$                             | 35679    |
| 95321:24  | $0, 0, 0, 0, e^{12}, e^{13}, e^{25}, e^{27}, e^{28} + e^{15}$                             | 35679    |
| 95321:25  | $0, 0, 0, 0, e^{12}, e^{13}, e^{15}, e^{17}, e^{18} + e^{36} + e^{24}$                    | 14679    |
| 95321:26a | $0, 0, 0, 0, e^{12}, e^{13}, e^{25}, e^{27}, e^{28} + e^{14} + e^{36}$                    | 14679    |
| 95321:26b | $0, 0, 0, 0, -e^{12}, e^{13}, e^{25}, e^{27}, e^{36} + e^{28} + e^{14}$                   | 14679    |
| 95321:27  | $0, 0, 0, 0, e^{12}, e^{13}, e^{25}, e^{27}, e^{16} + e^{34} + e^{28}$                    | 14679    |
| 95321:28  | $0, 0, 0, 0, -e^{12}, e^{13}, e^{15}, e^{17}, e^{28} + e^{57}$                            | 35679    |
| 95321:29  | $0, 0, 0, 0, e^{12}, e^{13}, e^{25}, e^{27}, e^{18} + e^{57}$                             | 35679    |
| 95321:30  | $0, 0, 0, 0, -e^{12}, e^{13}, e^{15}, e^{17} + e^{23}, e^{18} + e^{35}$                   | 34679    |
| 95321:31  | $0, 0, 0, 0, e^{12}, e^{13}, e^{15}, e^{17} + e^{23}, e^{18} + e^{26}$                    | 24679    |
| 95321:32  | $0, 0, 0, 0, -e^{12}, e^{13}, e^{15}, e^{24} + e^{17}, e^{18} + e^{45}$                   | 24679    |
| 95321:33  | $0, 0, 0, 0, e^{12}, e^{13}, e^{25}, e^{14} + e^{27}, e^{45} + e^{28}$                    | 24679    |
| 95321:34  | $0, 0, 0, 0, e^{12}, e^{34}, e^{15}, e^{17}, e^{25} + e^{18} + e^{36}$                    | 13679    |
| 95321:35  | $0, 0, 0, 0, e^{12}, -e^{13}, e^{15}, e^{17} + e^{34}, e^{18} + e^{23} + e^{46}$          | 13679    |
| 95321:36  | $0, 0, 0, 0, -e^{12}, e^{34}, e^{15}, e^{23} + e^{17}, e^{57} + e^{28}$                   | 24679    |
| 95321:37  | $0, 0, 0, 0, -e^{12}, e^{34}, e^{15}, e^{17} + e^{23}, e^{18} + e^{46} + e^{35}$          | 13679    |
| 95321:38  | $0, 0, 0, 0, -e^{12}, e^{34}, e^{15}, e^{17}, e^{57} + e^{28} + e^{36}$                   | 13679    |
| 95321:39  | $0, 0, 0, 0, e^{12}, e^{13}, e^{15}, e^{17}, e^{25} + e^{18} + e^{34}$                    | 25679    |
| 95321:40  | $0, 0, 0, 0, e^{12}, e^{13}, e^{25}, e^{27}, e^{34} + e^{28} + e^{15}$                    | 25679    |
| 95321:41  | $0, 0, 0, 0, e^{12}, e^{24} + e^{13}, e^{15}, e^{17}, e^{25} + e^{18}$                    | 25679    |
| 95321:42  | $0, 0, 0, 0, -e^{12}, e^{13}, e^{15}, e^{17}, e^{28} + e^{57} + e^{34}$                   | 25679    |
| 95321:43  | $0, 0, 0, 0, e^{12}, e^{13}, e^{25}, e^{27}, e^{57} + e^{18} + e^{34}$                    | 25679    |
| 95321:44  | $0, 0, 0, 0, -e^{12}, e^{24} + e^{13}, e^{15}, e^{17}, e^{57} + e^{28}$                   | 25679    |
| 95321:45  | $0, 0, 0, 0, -e^{12}, e^{34}, e^{15}, e^{17}, e^{57} + e^{28} + e^{13}$                   | 25679    |
| 95321:46a | $0, 0, 0, 0, e^{12}, e^{13}, e^{15}, e^{17}, e^{36} + e^{25} + e^{18}$                    | 24679    |
| 95321:46b | $0, 0, 0, 0, -e^{12}, e^{13}, e^{15}, e^{17}, e^{36} + e^{25} + e^{18}$                   | 24679    |
| 95321:47  | $0, 0, 0, 0, e^{12}, e^{13}, e^{15}, e^{17}, e^{18} + e^{35} + e^{26}$                    | 24679    |
| 95321:48a | $0, 0, 0, 0, e^{12}, e^{13}, e^{25}, e^{27}, e^{15} + e^{28} + e^{36}$                    | 24679    |
| 95321:48b | $0, 0, 0, 0, -e^{12}, e^{13}, e^{25}, e^{27}, e^{28} + e^{15} + e^{36}$                   | 24679    |
| 95321:49  | $0, 0, 0, 0, -e^{12}, e^{13} + e^{24}, e^{15}, e^{17} + e^{23}, e^{18} + e^{35}$          | 24679    |
| 95321:50  | $0, 0, 0, 0, -e^{12}, e^{34}, e^{15}, e^{17} + e^{23}, e^{18} + e^{24} + e^{35}$          | 24679    |
| 95321:51  | $0, 0, 0, 0, e^{12}, e^{13}, e^{15}, e^{23} + e^{17}, e^{26} + e^{18} + e^{34}$           | 14679    |
| 95321:52  | $0, 0, 0, 0, e^{12}, e^{34}, e^{15}, e^{17} + e^{25}, e^{27} + e^{18}$                    | 25679    |
| 95321:53  | $0, 0, 0, 0, -e^{12}, e^{13}, e^{15}, e^{17} + e^{23}, e^{57} + e^{28}$                   | 34679    |
| 95321:54  | $0, 0, 0, 0, -e^{12}, e^{13}, e^{15}, e^{24} + e^{17}, e^{28} + e^{57}$                   | 24679    |
| 95321:55  | $0, 0, 0, 0, e^{12}, e^{13}, e^{25}, e^{27} + e^{14}, e^{18} + e^{57}$                    | 24679    |
| 95321:56a | $0, 0, 0, 0, -e^{12}, e^{13}, e^{15}, e^{17}, e^{28} + e^{36} + e^{57}$                   | 24679    |
| 95321:56b | $0, 0, 0, 0, -e^{12}, -e^{13}, e^{15}, e^{17}, e^{57} + e^{28} + e^{36}$                  | 24679    |
| 95321:57  | $0, 0, 0, 0, e^{12}, e^{13}, e^{25}, e^{27}, e^{36} + e^{18} + e^{57}$                    | 24679    |
| 95321:58a | $0, 0, 0, 0, e^{12}, e^{24} - e^{13}, e^{15}, e^{17} + e^{34}, e^{18} + e^{46} + e^{23}$  | 13679    |
| 95321:58b | $0, 0, 0, 0, -e^{12}, e^{24} - e^{13}, e^{15}, e^{17} + e^{34}, e^{18} + e^{23} + e^{46}$ | 13679    |
| 95321:59  | $0, 0, 0, 0, e^{12}, e^{13} + e^{24}, e^{15}, e^{17} + e^{23}, e^{18} + e^{26}$           | 13679    |
| 95321:60  | $0, 0, 0, 0, e^{12}, -e^{13}, e^{15}, e^{34} + e^{17}, e^{25} + e^{18} + e^{46}$          | 13679    |
| 95321:61  | $0, 0, 0, 0, -e^{12}, e^{34}, e^{15}, e^{17} + e^{25}, e^{28} + e^{57}$                   | 25679    |
| 95321:62  | $0, 0, 0, 0, -e^{12}, e^{13}, e^{15}, e^{17} + e^{24}, e^{45} + e^{36} + e^{18}$          | 13679    |
| 95321:63a | $0, 0, 0, 0, e^{12}, e^{13}, e^{25}, e^{27} + e^{14}, e^{28} + e^{45} + e^{36}$           | 13679    |
| 95321:63b | $0, 0, 0, 0, e^{12}, -e^{13}, e^{25}, e^{14} + e^{27}, e^{36} + e^{45} + e^{28}$          | 13679    |
| 95321:64  | $0, 0, 0, 0, e^{12}, -e^{13}, e^{25}, e^{27} + e^{34}, e^{57} + e^{18} + e^{46}$          | 13679    |
| 95321:65  | $0, 0, 0, 0, -e^{12}, e^{34}, e^{15}, e^{23} + e^{17}, e^{57} + e^{28} + e^{36}$          | 13679    |
| 95321:66a | $0, 0, 0, 0, -e^{12}, e^{34}, e^{15}, e^{17} + e^{23}, e^{28} + e^{57} + e^{46}$          | 13679    |
| 95321:66b | $0, 0, 0, 0, -e^{12}, e^{34}, e^{15}, -e^{23} + e^{17}, e^{28} + e^{46} + e^{57}$         | 13679    |
| 95321:67  | $0, 0, 0, 0, e^{12}, e^{24} + e^{13}, e^{15}, e^{17}, e^{25} + e^{18} + e^{34}$           | 25679    |
| 95321:68  | $0, 0, 0, 0, e^{12}, e^{13}, e^{25}, e^{27}, e^{18} + e^{23} + e^{57}$                    | 35679    |
| 95321:69  | $0, 0, 0, 0, -e^{12}, e^{13}, e^{15}, e^{17}, e^{14} + e^{28} + e^{57}$                   | 25679    |

Table 2 – Continued to next page

Table 2 – Continued from previous page

| Name       | $\mathfrak{g}$                                                                                         | UCS Dim. |
|------------|--------------------------------------------------------------------------------------------------------|----------|
| 95321:70   | $0, 0, 0, 0, e^{12}, e^{13}, e^{25}, e^{27}, e^{18} + e^{57} + e^{24}$                                 | 25679    |
| 95321:71   | $0, 0, 0, 0, -e^{12}, e^{24} + e^{13}, e^{15}, e^{17}, e^{28} + e^{34} + e^{57}$                       | 25679    |
| 95321:72   | $0, 0, 0, 0, -e^{12}, e^{13}, e^{15}, e^{17} + e^{24}, e^{45} + e^{18} + e^{23}$                       | 24679    |
| 95321:73   | $0, 0, 0, 0, -e^{12}, e^{13}, e^{15}, e^{23} + e^{17}, e^{35} + e^{24} + e^{18}$                       | 24679    |
| 95321:74   | $0, 0, 0, 0, e^{12}, e^{13}, e^{15}, e^{25} + e^{17}, e^{27} + e^{18}$                                 | 35679    |
| 95321:75   | $0, 0, 0, 0, e^{12}, e^{13}, e^{25}, e^{15} + e^{27}, e^{28} + e^{17}$                                 | 35679    |
| 95321:76   | $0, 0, 0, 0, e^{12}(-1 + a_2), a_2 e^{13}, e^{15}, e^{17} + e^{23}, e^{18} + e^{26} + e^{35}$          | 24679    |
| 95321:77   | $0, 0, 0, 0, -e^{12}, e^{13}, e^{15}, e^{17}, e^{16} + e^{57} + e^{28}$                                | 24679    |
| 95321:78   | $0, 0, 0, 0, -e^{12}, e^{13}, e^{15}, e^{17} + e^{24}, e^{57} + e^{28} + e^{34}$                       | 24679    |
| 95321:79   | $0, 0, 0, 0, e^{12}, e^{13}, e^{25}, e^{14} + e^{27}, e^{18} + e^{34} + e^{57}$                        | 24679    |
| 95321:80   | $0, 0, 0, 0, -e^{12}, e^{24} + e^{13}, e^{15}, e^{23} + e^{17}, e^{57} + e^{28}$                       | 24679    |
| 95321:81   | $0, 0, 0, 0, -e^{12}, e^{34}, e^{15}, e^{17} + e^{23}, e^{28} + e^{57} + e^{14}$                       | 24679    |
| 95321:82   | $0, 0, 0, 0, -e^{12}, e^{13}, e^{15}, e^{17} + e^{23}, e^{57} + e^{28} + e^{34}$                       | 24679    |
| 95321:83   | $0, 0, 0, 0, -e^{12}, e^{34}, e^{15}, e^{17} + e^{23}, e^{28} + e^{13} + e^{57}$                       | 24679    |
| 95321:84   | $0, 0, 0, 0, e^{12}, e^{24} + e^{13}, e^{15}, e^{17}, e^{35} + e^{26} + e^{18}$                        | 13679    |
| 95321:85   | $0, 0, 0, 0, e^{12}, e^{24} + e^{13}, e^{15}, e^{17} + e^{23}, e^{18} + e^{26} + e^{34}$               | 13679    |
| 95321:86   | $0, 0, 0, 0, -e^{12}, e^{13}, e^{15}, e^{17} + e^{25}, e^{28} + e^{57}$                                | 35679    |
| 95321:87   | $0, 0, 0, 0, e^{12}, e^{13}, e^{25}, e^{15} + e^{27}, e^{18} + e^{57}$                                 | 35679    |
| 95321:88   | $0, 0, 0, 0, -e^{12}, e^{34}, e^{15}, e^{17}, e^{57} + e^{13} + e^{46} + e^{28}$                       | 13679    |
| 95321:89   | $0, 0, 0, 0, e^{12}, e^{13}, e^{25}, e^{27} + e^{14}, e^{16} + e^{28} + e^{45}$                        | 13679    |
| 95321:90a  | $0, 0, 0, 0, e^{12}, e^{14} + e^{23}, e^{15}, e^{34} + e^{17}, e^{36} + e^{18} + e^{25}$               | 13679    |
| 95321:90b  | $0, 0, 0, 0, -e^{12}, e^{14} + e^{23}, e^{15}, e^{17} + e^{34}, e^{36} + e^{25} + e^{18}$              | 13679    |
| 95321:91a  | $0, 0, 0, 0, -e^{12}, e^{13}, e^{15}, e^{23} + e^{17}, e^{36} + e^{28} + e^{57}$                       | 24679    |
| 95321:91b  | $0, 0, 0, 0, -e^{12}, -e^{13}, e^{15}, e^{23} + e^{17}, e^{57} + e^{28} + e^{36}$                      | 24679    |
| 95321:92   | $0, 0, 0, 0, e^{12}, e^{34}, e^{15}, e^{17} + e^{25}, e^{18} + e^{27} + e^{36}$                        | 13679    |
| 95321:93a  | $0, 0, 0, 0, -e^{12}, e^{13}, e^{15}, e^{17} + e^{24}, e^{28} + e^{57} + e^{36}$                       | 13679    |
| 95321:93b  | $0, 0, 0, 0, -e^{12}, -e^{13}, e^{15}, e^{24} + e^{17}, e^{57} + e^{36} + e^{28}$                      | 13679    |
| 95321:94   | $0, 0, 0, 0, e^{12}, e^{13}, e^{25}, e^{27} + e^{14}, e^{36} + e^{18} + e^{57}$                        | 13679    |
| 95321:95a  | $0, 0, 0, 0, -e^{12}, e^{24} + e^{13}, e^{15}, e^{17} + e^{34}, e^{57} + e^{28} + e^{36}$              | 13679    |
| 95321:95b  | $0, 0, 0, 0, -e^{12}, e^{24} - e^{13}, e^{15}, e^{17} + e^{34}, e^{36} + e^{28} + e^{57}$              | 13679    |
| 95321:96   | $0, 0, 0, 0, -e^{12}, e^{34}, e^{15}, e^{17} + e^{25}, e^{28} + e^{36} + e^{57}$                       | 13679    |
| 95321:97   | $0, 0, 0, 0, -e^{12}, e^{14} + e^{23}, e^{15}, e^{17}, e^{57} + e^{28} + e^{13}$                       | 25679    |
| 95321:98   | $0, 0, 0, 0, e^{12}, e^{13}, e^{15}, e^{17} + e^{25}, e^{18} + e^{34} + e^{27}$                        | 25679    |
| 95321:99   | $0, 0, 0, 0, e^{12}, e^{13}, e^{25}, e^{27} + e^{15}, e^{34} + e^{17} + e^{28}$                        | 25679    |
| 95321:100  | $0, 0, 0, 0, e^{12}, e^{13} + e^{24}, e^{15}, e^{17} + e^{25}, e^{27} + e^{18}$                        | 25679    |
| 95321:101  | $0, 0, 0, 0, e^{12}, e^{13}, e^{25}, e^{14} + e^{27}, e^{57} + e^{18} + e^{23}$                        | 24679    |
| 95321:102  | $0, 0, 0, 0, -e^{12}, e^{13}, e^{15}, e^{23} + e^{17}, e^{14} + e^{28} + e^{57}$                       | 24679    |
| 95321:103  | $0, 0, 0, 0, -e^{12}, e^{13}, e^{15}, e^{24} + e^{17}, e^{14} + e^{57} + e^{28}$                       | 24679    |
| 95321:104  | $0, 0, 0, 0, e^{12}, e^{13}, e^{25}, e^{27} + e^{14}, e^{18} + e^{57} + e^{24}$                        | 24679    |
| 95321:105a | $0, 0, 0, 0, -e^{12}, e^{13}, e^{15}, e^{17}, e^{28} + e^{14} + e^{57} + e^{36}$                       | 14679    |
| 95321:105b | $0, 0, 0, 0, -e^{12}, -e^{13}, e^{15}, e^{17}, e^{57} + e^{36} + e^{14} + e^{28}$                      | 14679    |
| 95321:106  | $0, 0, 0, 0, -e^{12}, e^{13}, e^{15}, e^{17}, e^{28} + e^{57} + e^{34} + e^{16}$                       | 14679    |
| 95321:107  | $0, 0, 0, 0, e^{12}, e^{13}, e^{25}, e^{27}, e^{36} + e^{57} + e^{18} + e^{24}$                        | 14679    |
| 95321:108  | $0, 0, 0, 0, -e^{12}, e^{13} + e^{24}, e^{15}, e^{17} + e^{23}, e^{28} + e^{57} + e^{34}$              | 24679    |
| 95321:109  | $0, 0, 0, 0, -e^{12}, e^{13}, e^{15}, e^{17} + e^{25}, e^{28} + e^{34} + e^{57}$                       | 25679    |
| 95321:110  | $0, 0, 0, 0, e^{12}, e^{13}, e^{25}, e^{27} + e^{15}, e^{18} + e^{57} + e^{34}$                        | 25679    |
| 95321:111  | $0, 0, 0, 0, -e^{12}, e^{24} + e^{13}, e^{15}, e^{17} + e^{25}, e^{28} + e^{57}$                       | 25679    |
| 95321:112  | $0, 0, 0, 0, -e^{12}, e^{34}, e^{15}, e^{17} + e^{25}, e^{57} + e^{28} + e^{13}$                       | 25679    |
| 95321:113a | $0, 0, 0, 0, -e^{12}, e^{13}, e^{15}, e^{23} + e^{17}, e^{57} + e^{16} + e^{28}$                       | 24679    |
| 95321:113b | $0, 0, 0, 0, -e^{12}, -e^{13}, e^{15}, e^{17} + e^{23}, e^{28} + e^{57} + e^{16}$                      | 24679    |
| 95321:114  | $0, 0, 0, 0, e^{12}, e^{13}, e^{15}, e^{17} + e^{25}, e^{27} + e^{36} + e^{18}$                        | 24679    |
| 95321:115a | $0, 0, 0, 0, e^{12}, e^{13}, e^{25}, e^{15} + e^{27}, e^{28} + e^{17} + e^{36}$                        | 24679    |
| 95321:115b | $0, 0, 0, 0, -e^{12}, e^{13}, e^{25}, e^{15} + e^{27}, e^{17} + e^{28} + e^{36}$                       | 24679    |
| 95321:116  | $0, 0, 0, 0, e^{12}(-1 + a_2), e^{24} + a_2 e^{13}, e^{15}, e^{17} + e^{23}, e^{18} + e^{26} + e^{35}$ | 13679    |
| 95321:117  | $0, 0, 0, 0, e^{12}, -e^{13}, e^{25}, e^{34} + e^{27}, e^{46} + e^{23} + e^{57} + e^{18}$              | 13679    |
| 95321:118a | $0, 0, 0, 0, -e^{12}, e^{34}, e^{15}, e^{17} + e^{23}, e^{28} + e^{57} + e^{46} + e^{13}$              | 13679    |
| 95321:118b | $0, 0, 0, 0, -e^{12}, e^{34}, e^{15}, e^{17} - e^{23}, e^{28} + e^{46} + e^{13} + e^{57}$              | 13679    |
| 95321:119  | $0, 0, 0, 0, -e^{12}, e^{34}, e^{15}, e^{17} + e^{23}, e^{57} + e^{36} + e^{28} + e^{14}$              | 13679    |

Table 2 – Continued to next page



Table 2 – Continued from previous page

| Name       | $\mathfrak{g}$                                                                                               | UCS Dim. |
|------------|--------------------------------------------------------------------------------------------------------------|----------|
| 95321:120  | $0, 0, 0, 0, -e^{12}, e^{34}, e^{23} + e^{15}, e^{35} + e^{17}, e^{37} + e^{18}$                             | 24579    |
| 95321:121  | $0, 0, 0, 0, -e^{12}, e^{13}, e^{15}, e^{17} + e^{24}, e^{16} + e^{28} + e^{57}$                             | 13679    |
| 95321:122a | $0, 0, 0, 0, -e^{12}, e^{13}, e^{15}, e^{17} + e^{25}, e^{57} + e^{36} + e^{28}$                             | 24679    |
| 95321:122b | $0, 0, 0, 0, -e^{12}, -e^{13}, e^{15}, e^{17} + e^{25}, e^{57} + e^{36} + e^{28}$                            | 24679    |
| 95321:123  | $0, 0, 0, 0, e^{12}, e^{13}, e^{25}, e^{27} + e^{15}, e^{36} + e^{18} + e^{57}$                              | 24679    |
| 95321:124  | $0, 0, 0, 0, e^{12}, -e^{13}, e^{15}, e^{17} + e^{25} + e^{34}, e^{27} + e^{18} + e^{46}$                    | 13679    |
| 95321:125  | $0, 0, 0, 0, e^{12}, -e^{13}, e^{25}, e^{34} + e^{27} + e^{15}, e^{18} + e^{57} + e^{46}$                    | 13679    |
| 95321:126  | $0, 0, 0, 0, e^{12}, e^{24} + e^{13}, e^{15}, e^{17} + e^{25}, e^{18} + e^{27} + e^{34}$                     | 25679    |
| 95321:127  | $0, 0, 0, 0, -e^{12}, e^{13} + e^{24}, e^{15}, e^{17} + e^{23}, e^{28} + e^{14} + e^{57}$                    | 24679    |
| 95321:128  | $0, 0, 0, 0, e^{12}, e^{13}, e^{25}, e^{15} + e^{27}, e^{18} + e^{23} + e^{57}$                              | 35679    |
| 95321:129  | $0, 0, 0, 0, -e^{12}, e^{13}, e^{15}, e^{17} + e^{25}, e^{28} + e^{57} + e^{14}$                             | 25679    |
| 95321:130  | $0, 0, 0, 0, e^{12}, e^{13}, e^{25}, e^{15} + e^{27}, e^{57} + e^{18} + e^{24}$                              | 25679    |
| 95321:131a | $0, 0, 0, 0, -e^{12}, e^{13} + e^{24}, e^{15}, e^{17} + e^{25}, e^{28} + e^{57} + e^{34}$                    | 25679    |
| 95321:131b | $0, 0, 0, 0, -e^{12}, e^{24} - e^{13}, e^{15}, e^{17} + e^{25}, e^{28} + e^{34} + e^{57}$                    | 25679    |
| 95321:132a | $0, 0, 0, 0, -e^{12}, e^{13}, e^{15}, e^{23} + e^{17}, e^{14} + e^{57} + e^{28} + e^{36}$                    | 14679    |
| 95321:132b | $0, 0, 0, 0, -e^{12}, -e^{13}, e^{15}, e^{17} + e^{23}, e^{28} + e^{36} + e^{14} + e^{57}$                   | 14679    |
| 95321:133a | $0, 0, 0, 0, -e^{12}, e^{13}, e^{15}, e^{17} + e^{23}, e^{57} + e^{34} + e^{28} + e^{16}$                    | 14679    |
| 95321:133b | $0, 0, 0, 0, -e^{12}, -e^{13}, e^{15}, e^{23} + e^{17}, e^{57} + e^{16} + e^{28} + e^{34}$                   | 14679    |
| 95321:134  | $0, 0, 0, 0, -e^{12}, e^{13}, e^{15} + e^{24}, e^{17} + e^{45}, e^{18} + e^{47}$                             | 24579    |
| 95321:135  | $0, 0, 0, 0, e^{12}, e^{13}, e^{14} + e^{25}, e^{45} + e^{27}, e^{47} + e^{28}$                              | 24579    |
| 95321:136  | $0, 0, 0, 0, -e^{12}, e^{13}, e^{15} + e^{23}, e^{17} + e^{35}, e^{37} + e^{18}$                             | 34579    |
| 95321:137a | $0, 0, 0, 0, -e^{12}, e^{13}, e^{15}, e^{17} + e^{24}, e^{28} + e^{14} + e^{57} + e^{36}$                    | 13679    |
| 95321:137b | $0, 0, 0, 0, -e^{12}, -e^{13}, e^{15}, e^{24} + e^{17}, e^{57} + e^{36} + e^{14} + e^{28}$                   | 13679    |
| 95321:138  | $0, 0, 0, 0, -e^{12}, e^{13}, e^{15}, e^{17} + e^{24}, e^{28} + e^{57} + e^{34} + e^{16}$                    | 13679    |
| 95321:139  | $0, 0, 0, 0, e^{12}, e^{13}, e^{25}, e^{14} + e^{27}, e^{36} + e^{57} + e^{18} + e^{24}$                     | 13679    |
| 95321:140  | $0, 0, 0, 0, -e^{12}, e^{13}, e^{15}, e^{17} + e^{25}, e^{57} + e^{28} + e^{16}$                             | 24679    |
| 95321:141a | $0, 0, 0, 0, -e^{12}, e^{24} + e^{13}, e^{15}, e^{17} + e^{34}, e^{36} + e^{14} + e^{28} + e^{57}$           | 13679    |
| 95321:141b | $0, 0, 0, 0, -e^{12}, e^{24} - e^{13}, e^{15}, e^{17} + e^{34}, e^{28} + e^{36} + e^{14} + e^{57}$           | 13679    |
| 95321:143  | $0, 0, 0, 0, -e^{12}, e^{34}, e^{15}, e^{17} + e^{25}, e^{57} + e^{28} + e^{46} + e^{13}$                    | 13679    |
| 95321:144  | $0, 0, 0, 0, -e^{12}, e^{34}, e^{15} + e^{23}, e^{17} + e^{35}, e^{18} + e^{46} + e^{37}$                    | 13579    |
| 95321:145a | $0, 0, 0, 0, e^{12}, e^{14} + e^{23}, e^{15}, e^{25} + e^{34} + e^{17}, e^{18} + e^{36} + e^{27}$            | 13679    |
| 95321:145b | $0, 0, 0, 0, -e^{12}, e^{14} + e^{23}, e^{15}, e^{17} + e^{25} + e^{34}, e^{36} + e^{18} + e^{27}$           | 13679    |
| 95321:146a | $0, 0, 0, 0, -e^{12}, e^{13} + e^{24}, e^{15}, e^{17} + e^{34} + e^{25}, e^{28} + e^{57} + e^{36}$           | 13679    |
| 95321:146b | $0, 0, 0, 0, -e^{12}, -e^{13} + e^{24}, e^{15}, e^{17} + e^{25} + e^{34}, e^{28} + e^{57} + e^{36}$          | 13679    |
| 95321:147  | $0, 0, 0, 0, -e^{12}, e^{14} + e^{23}, e^{15}, e^{25} + e^{17}, e^{13} + e^{57} + e^{28}$                    | 25679    |
| 95321:148  | $0, 0, 0, 0, -e^{12}, e^{24} + e^{13}, e^{15} + e^{23}, e^{17} + e^{35}, e^{18} + e^{37}$                    | 24579    |
| 95321:149  | $0, 0, 0, 0, -e^{12}, e^{34}, e^{23} + e^{15}, e^{35} + e^{17}, e^{24} + e^{37} + e^{18}$                    | 24579    |
| 95321:152a | $0, 0, 0, 0, -e^{12}, e^{13}, e^{15}, e^{17} + e^{25}, e^{57} + e^{28} + e^{36} + e^{14}$                    | 14679    |
| 95321:152b | $0, 0, 0, 0, -e^{12}, -e^{13}, e^{15}, e^{17} + e^{25}, e^{28} + e^{14} + e^{57} + e^{36}$                   | 14679    |
| 95321:153  | $0, 0, 0, 0, -e^{12}, e^{13}, e^{15}, e^{17} + e^{25}, e^{57} + e^{16} + e^{28} + e^{34}$                    | 14679    |
| 95321:154  | $0, 0, 0, 0, e^{12}, e^{13}, e^{25}, e^{27} + e^{15}, e^{24} + e^{36} + e^{18} + e^{57}$                     | 14679    |
| 95321:156  | $0, 0, 0, 0, -e^{12}, e^{13}, e^{24} + e^{15}, e^{45} + e^{17}, e^{47} + e^{36} + e^{18}$                    | 13579    |
| 95321:157a | $0, 0, 0, 0, e^{12}, e^{13}, e^{25} + e^{14}, e^{27} + e^{45}, e^{28} + e^{36} + e^{47}$                     | 13579    |
| 95321:157b | $0, 0, 0, 0, e^{12}, -e^{13}, e^{25} + e^{14}, e^{27} + e^{45}, e^{47} + e^{28} + e^{36}$                    | 13579    |
| 95321:158  | $0, 0, 0, 0, e^{12}, -e^{13}, e^{25}, e^{15} + e^{34} + e^{27}, e^{57} + e^{46} + e^{18} + e^{23}$           | 13679    |
| 95321:162  | $0, 0, 0, 0, e^{12}, e^{13}, e^{25}, e^{27} + e^{16}, e^{57} + e^{18}$                                       | 23579    |
| 95321:163  | $0, 0, 0, 0, -e^{12}, e^{13}, e^{15} + e^{24}, e^{17} + e^{45}, e^{18} + e^{23} + e^{47}$                    | 24579    |
| 95321:164  | $0, 0, 0, 0, -e^{12}, e^{13}, e^{15} + e^{23}, e^{17} + e^{35}, e^{37} + e^{24} + e^{18}$                    | 24579    |
| 95321:172  | $0, 0, 0, 0, -e^{12}, e^{34}, e^{15} + e^{23}, e^{35} + e^{17}, e^{37} + e^{18} + e^{25}$                    | 24579    |
| 95321:173  | $0, 0, 0, 0, e^{12}, e^{13}, e^{25} + e^{14}, e^{27} + e^{45}, e^{16} + e^{28} + e^{47}$                     | 13579    |
| 95321:179a | $0, 0, 0, 0, -e^{12}, e^{13} + e^{24}, e^{15}, e^{17} + e^{34} + e^{25}, e^{28} + e^{57} + e^{36} + e^{14}$  | 13679    |
| 95321:179b | $0, 0, 0, 0, -e^{12}, -e^{13} + e^{24}, e^{15}, e^{17} + e^{25} + e^{34}, e^{28} + e^{14} + e^{57} + e^{36}$ | 13679    |
| 95321:180  | $0, 0, 0, 0, -e^{12}, e^{34}, e^{15} + e^{23}, e^{24} + e^{17} + e^{35}, e^{37} + e^{45} + e^{18}$           | 23579    |
| 95321:183  | $0, 0, 0, 0, e^{12}, e^{13}, e^{25}, e^{16} + e^{27}, e^{57} + e^{18} + e^{34}$                              | 13579    |
| 95321:184  | $0, 0, 0, 0, e^{12}, e^{13}, e^{25}, e^{27} + e^{16}, e^{57} + e^{36} + e^{18}$                              | 23579    |
| 95321:188  | $0, 0, 0, 0, -e^{12}, e^{13}, e^{15} + e^{24}, e^{17} + e^{45}, e^{18} + e^{47} + e^{25}$                    | 24579    |
| 95321:189  | $0, 0, 0, 0, e^{12}, e^{13}, e^{14} + e^{25}, e^{27} + e^{45}, e^{28} + e^{15} + e^{47}$                     | 24579    |
| 95321:191  | $0, 0, 0, 0, -e^{12}, e^{13}, e^{15} + e^{23}, e^{17} + e^{35}, e^{18} + e^{37} + e^{25}$                    | 34579    |

Table 2 – Continued to next page

Table 2 – Continued from previous page

| Name       | $\mathfrak{g}$                                                                                                                     | UCS Dim. |
|------------|------------------------------------------------------------------------------------------------------------------------------------|----------|
| 95321:194  | $0, 0, 0, 0, e^{12}, -e^{13}, e^{25}, e^{34} + e^{27} + e^{16}, e^{46} + e^{57} + e^{18}$                                          | 12579    |
| 95321:196  | $0, 0, 0, 0, e^{12}, -e^{13}, e^{23} + e^{15}, -2e^{17} + e^{26} + e^{35}, e^{18} + e^{56}$                                        | 23579    |
| 95321:198  | $0, 0, 0, 0, -e^{12}, e^{13}, e^{15} + e^{24}, e^{17} + e^{45} + e^{23}, e^{18} + e^{47} + e^{35}$                                 | 23579    |
| 95321:201  | $0, 0, 0, 0, -e^{12}, e^{13}, e^{15} + e^{24}, e^{17} + e^{23} + e^{45}, e^{18} + e^{26} + e^{47}$                                 | 13579    |
| 95321:204  | $0, 0, 0, 0, -e^{12}, e^{34}, e^{15} + e^{23}, e^{17} + e^{35}, e^{25} + e^{37} + e^{18} + e^{46}$                                 | 13579    |
| 95321:205  | $0, 0, 0, 0, -e^{12}, e^{13}, e^{15} + e^{23}, e^{17} + e^{24} + e^{35}, e^{18} + e^{45} + e^{37}$                                 | 23579    |
| 95321:210  | $0, 0, 0, 0, e^{12}, e^{13}, e^{25}, e^{16} + e^{27}, e^{24} + e^{18} + e^{57}$                                                    | 13579    |
| 95321:211  | $0, 0, 0, 0, e^{12}, e^{13}, e^{25}, e^{27} + e^{16}, e^{23} + e^{57} + e^{18}$                                                    | 23579    |
| 95321:214  | $0, 0, 0, 0, -e^{12}, e^{13} + e^{24}, e^{15} + e^{23}, e^{17} + e^{35}, e^{18} + e^{37} + e^{25}$                                 | 24579    |
| 95321:216  | $0, 0, 0, 0, e^{12}, e^{13}, e^{15} + e^{23}, e^{17} + e^{26}, e^{37} + e^{18} + e^{56}$                                           | 23579    |
| 95321:219  | $0, 0, 0, 0, e^{12}, -e^{13}, e^{15} + e^{23}, -2e^{17} + e^{35} + e^{26}, e^{18} + e^{34} + e^{56}$                               | 13579    |
| 95321:220  | $0, 0, 0, 0, e^{12}, e^{13}, 2e^{15}, e^{26} + e^{35} + e^{17}, e^{18} + e^{56} + e^{37}$                                          | 23579    |
| 95321:225a | $0, 0, 0, 0, -e^{12}, e^{13}, e^{15} + e^{24}, e^{45} + e^{17}, e^{36} + e^{47} + e^{18} + e^{25}$                                 | 13579    |
| 95321:225b | $0, 0, 0, 0, -e^{12}, -e^{13}, e^{15} + e^{24}, e^{17} + e^{45}, e^{25} + e^{47} + e^{18} + e^{36}$                                | 13579    |
| 95321:226  | $0, 0, 0, 0, -e^{12}, -e^{13}, e^{24} + e^{15}, e^{45} + e^{17}, e^{35} + e^{47} + e^{18} + e^{26}$                                | 13579    |
| 95321:227a | $0, 0, 0, 0, e^{12}, e^{13}, e^{14} + e^{25}, e^{45} + e^{27}, e^{47} + e^{28} + e^{15} + e^{36}$                                  | 13579    |
| 95321:227b | $0, 0, 0, 0, e^{12}, -e^{13}, e^{25} + e^{14}, e^{45} + e^{27}, e^{28} + e^{47} + e^{36} + e^{15}$                                 | 13579    |
| 95321:229  | $0, 0, 0, 0, -e^{12}, -2e^{13}, e^{15} - e^{23}, e^{17} + e^{26} + e^{35}, e^{28} + e^{57}$                                        | 23579    |
| 95321:234  | $0, 0, 0, 0, e^{12}, e^{13}, e^{25}, e^{27} + e^{16}, e^{18} + e^{57} + e^{24} + e^{36}$                                           | 13579    |
| 95321:235  | $0, 0, 0, 0, e^{12}, -e^{13}, e^{15} + e^{23}, e^{26} + e^{35} - 2e^{17}, e^{24} + e^{18} + e^{56}$                                | 13579    |
| 95321:236  | $0, 0, 0, 0, e^{12}, -e^{13}, e^{25}, e^{16} + e^{34} + e^{27}, e^{57} + e^{46} + e^{18} + e^{23}$                                 | 12579    |
| 95321:237  | $0, 0, 0, 0, -e^{12}, -2e^{13}, e^{15} - e^{23}, e^{17} + e^{26} + e^{35}, e^{28} + e^{57} + e^{34}$                               | 13579    |
| 95321:240  | $0, 0, 0, 0, e^{12}(-1 + a_2), a_2e^{13}, e^{24} + e^{15}, -e^{17}(-1 + a_2) + e^{23} + e^{45}, e^{35} + e^{47} + e^{18} + e^{26}$ | 13579    |
| 95321:243  | $0, 0, 0, 0, e^{12}, (-1 + a_3)e^{13}, e^{15} + a_3 + e^{23}, (-2 + a_3)e^{17} + e^{35} + e^{26}, e^{18} + e^{56} + e^{37}$        | 23579    |
| 95321:244a | $0, 0, 0, 0, -e^{12}, -2e^{13}, e^{15} - e^{23}, e^{35} + e^{17} + e^{26}, e^{57} + e^{36} + e^{28}$                               | 23579    |
| 95321:244b | $0, 0, 0, 0, -e^{12}, -2e^{13}, -e^{15} - e^{23}, e^{17} + e^{26} + e^{35}, e^{28} + e^{57} + e^{36}$                              | 23579    |
| 95321:245  | $0, 0, 0, 0, e^{12}, e^{13}, e^{23} + e^{15}, e^{26} + e^{17}, e^{24} + e^{56} + e^{37} + e^{18}$                                  | 13579    |
| 95321:246  | $0, 0, 0, 0, e^{12}, e^{13}, 2e^{15}, e^{35} + e^{26} + e^{17}, e^{24} + e^{56} + e^{37} + e^{18}$                                 | 13579    |
| 95321:247  | $0, 0, 0, 0, -e^{12}, -2e^{13}, e^{15} - e^{23}, e^{35} + e^{17} + e^{26}, e^{57} + e^{28} + e^{14}$                               | 13579    |
| 95321:248  | $0, 0, 0, 0, -e^{12}, -2e^{13}, e^{15} - e^{23}, e^{17} + e^{26} + e^{35}, e^{28} + e^{16} + e^{57}$                               | 23579    |
| 95321:250a | $0, 0, 0, 0, -e^{12}, -2e^{13}, e^{15} - e^{23}, e^{26} + e^{17} + e^{35}, e^{14} + e^{57} + e^{28} + e^{36}$                      | 13579    |
| 95321:250b | $0, 0, 0, 0, -e^{12}, -2e^{13}, -e^{15} - e^{23}, e^{17} + e^{35} + e^{26}, e^{28} + e^{57} + e^{36} + e^{14}$                     | 13579    |
| 95321:251  | $0, 0, 0, 0, -e^{12}, -2e^{13}, e^{15} - e^{23}, e^{26} + e^{17} + e^{35}, e^{16} + e^{57} + e^{34} + e^{28}$                      | 13579    |
| 95321:252  | $0, 0, 0, 0, e^{12}, e^{13}a_2, e^{23} + (1 + a_2)e^{15}, e^{26} + e^{35} + (-1 + a_2)e^{17}, e^{18} + e^{37} + e^{56} + e^{24}$   | 13579    |
| 95321:254  | $0, 0, 0, 0, e^{12}, e^{14} + e^{23}, e^{25} - e^{13}, -2e^{16} + e^{27} + e^{35}, e^{57} + e^{18}$                                | 12479    |
| 95321:258  | $0, 0, 0, 0, e^{12}, e^{14} + e^{23}, e^{25} - e^{13}, -2e^{16} + e^{27} + e^{35}, e^{18} + e^{34} + e^{57}$                       | 12479    |
| 95321:259  | $0, 0, 0, 0, e^{12}, e^{14} + e^{23}, e^{25} - e^{13}, -2e^{16} + e^{27} + e^{35}, e^{57} + e^{24} + e^{18}$                       | 12479    |
| Type: 4122 |                                                                                                                                    |          |
| 9542:1     | $0, 0, 0, 0, e^{12}, e^{15}, e^{25}, e^{16}, e^{27}$                                                                               | 4679     |
| 9542:2     | $0, 0, 0, 0, e^{12}, e^{15}, e^{25}, e^{16}, e^{27} + e^{34}$                                                                      | 2679     |
| 9542:3     | $0, 0, 0, 0, e^{12}, e^{15}, e^{25}, e^{16}, e^{13} + e^{27}$                                                                      | 3679     |
| 9542:4     | $0, 0, 0, 0, e^{12}, e^{15}, e^{25}, e^{23} + e^{16}, e^{27} + e^{34}$                                                             | 2679     |
| 9542:5     | $0, 0, 0, 0, e^{12}, e^{15}, e^{25}, e^{16}, e^{26} + e^{17}$                                                                      | 4679     |
| 9542:6     | $0, 0, 0, 0, e^{12}, e^{15}, e^{25}, e^{16} + e^{23}, e^{27} + e^{13}$                                                             | 3679     |
| 9542:7     | $0, 0, 0, 0, e^{12}, e^{15}, e^{25}, e^{23} + e^{16}, e^{27} + e^{14}$                                                             | 2679     |
| 9542:8     | $0, 0, 0, 0, e^{12}, e^{15}, e^{25}, e^{16}, e^{34} + e^{26} + e^{17}$                                                             | 2679     |
| 9542:9     | $0, 0, 0, 0, e^{12}, e^{15}, e^{25}, e^{34} + e^{16}, e^{26} + e^{17}$                                                             | 2679     |
| 9542:10    | $0, 0, 0, 0, e^{12}, e^{15}, e^{25}, e^{16} + e^{23}, e^{17} + e^{26}$                                                             | 3679     |
| 9542:11    | $0, 0, 0, 0, e^{12}, e^{15}, e^{25} + e^{13}, e^{16}, e^{27} + e^{35}$                                                             | 3579     |
| 9542:12    | $0, 0, 0, 0, e^{12}, e^{15}, e^{25}, e^{23} + e^{16}, e^{34} + e^{26} + e^{17}$                                                    | 2679     |
| 9542:13a   | $0, 0, 0, 0, e^{12}, e^{15}, e^{25}, e^{26} + e^{17}, e^{27} + e^{16}$                                                             | 4679     |
| 9542:13b   | $0, 0, 0, 0, e^{12}, -e^{15}, e^{25}, -e^{17} + e^{26}, e^{27} + e^{16}$                                                           | 4679     |
| 9542:14    | $0, 0, 0, 0, e^{12}, e^{15}, e^{25} + e^{13}, e^{16}, e^{17} + e^{26}$                                                             | 3579     |
| 9542:15    | $0, 0, 0, 0, e^{12}, e^{15}, e^{13} + e^{25}, e^{16} + e^{34}, e^{35} + e^{27}$                                                    | 2579     |
| 9542:16a   | $0, 0, 0, 0, e^{12}, e^{15}, e^{25}, e^{27} + e^{16}, e^{26} + e^{34} + e^{17}$                                                    | 2679     |
| 9542:16b   | $0, 0, 0, 0, e^{12}, e^{15}, e^{25}, -e^{16} + e^{27}, e^{17} + e^{26} + e^{34}$                                                   | 2679     |
| 9542:17a   | $0, 0, 0, 0, e^{12}, e^{15}, e^{25}, e^{17} + e^{26}, e^{16} + e^{34} + e^{27}$                                                    | 2679     |
| 9542:17b   | $0, 0, 0, 0, e^{12}, -e^{15}, e^{25}, -e^{17} + e^{26}, e^{27} + e^{16} + e^{34}$                                                  | 2679     |

Table 2 – Continued to next page

Table 2 – Continued from previous page

| Name       | $\mathfrak{g}$                                                                                                           | UCS Dim. |
|------------|--------------------------------------------------------------------------------------------------------------------------|----------|
| 9542:18    | $0, 0, 0, 0, e^{12}, e^{15}, e^{13} + e^{25}, e^{16} + e^{23}, e^{27} + e^{35}$                                          | 3579     |
| 9542:19    | $0, 0, 0, 0, e^{12}, e^{15}, e^{13} + e^{25}, e^{16}, e^{14} + e^{27} + e^{35}$                                          | 2579     |
| 9542:20    | $0, 0, 0, 0, e^{12}, e^{15}, e^{25} + e^{13}, e^{16} + e^{24}, e^{27} + e^{35}$                                          | 2579     |
| 9542:21    | $0, 0, 0, 0, e^{12}, e^{15}, e^{25} + e^{13}, e^{16}, e^{34} + e^{26} + e^{17}$                                          | 2579     |
| 9542:22    | $0, 0, 0, 0, e^{12}, e^{15}, e^{13} + e^{25}, e^{34} + e^{16}, e^{26} + e^{17}$                                          | 2579     |
| 9542:23    | $0, 0, 0, 0, e^{12}, e^{15}, e^{25} + e^{13}, e^{16} + e^{23}, e^{17} + e^{26}$                                          | 3579     |
| 9542:24    | $0, 0, 0, 0, e^{12}, e^{15}, e^{25} + e^{13}, e^{16} + e^{24}, e^{17} + e^{26}$                                          | 2579     |
| 9542:25    | $0, 0, 0, 0, e^{12}, e^{15}, e^{25} + e^{13}, e^{34} + e^{16}, e^{35} + e^{27} + e^{14}$                                 | 2579     |
| 9542:26    | $0, 0, 0, 0, e^{12}, e^{13} + e^{25}, e^{15}, e^{26} + e^{35}, e^{27} + e^{16}$                                          | 3579     |
| 9542:27    | $0, 0, 0, 0, e^{12}, e^{15}, e^{25} + e^{13}, e^{16} + e^{24}, e^{14} + e^{27} + e^{35}$                                 | 2579     |
| 9542:28    | $0, 0, 0, 0, e^{12}, e^{15}, e^{13} + e^{25}, e^{16} + e^{24}, e^{17} + e^{34} + e^{26}$                                 | 2579     |
| 9542:29    | $0, 0, 0, 0, e^{12}, e^{15}, e^{13} + e^{25}, e^{16} + e^{23}, e^{27} + e^{35} + e^{14}$                                 | 2579     |
| 9542:30    | $0, 0, 0, 0, e^{12}, e^{15}, e^{25} + e^{13}, e^{16} + e^{23}, e^{17} + e^{26} + e^{34}$                                 | 2579     |
| 9542:31    | $0, 0, 0, 0, e^{12}, e^{25} + e^{13}, e^{15}, e^{26} + e^{35}, e^{16} + e^{34} + e^{27}$                                 | 2579     |
| 9542:32a   | $0, 0, 0, 0, -e^{12}, e^{15} + e^{23}, e^{13} + e^{25}, e^{35} + e^{16}, e^{17} + e^{26}$                                | 3579     |
| 9542:32b   | $0, 0, 0, 0, -e^{12}, e^{15} + e^{23}, -e^{13} + e^{25}, e^{16} + e^{35}, e^{17} + e^{26}$                               | 2579     |
| 9542:33    | $0, 0, 0, 0, e^{12}, e^{13} + e^{25}, e^{15}, e^{26} + e^{35} + e^{14}, e^{27} + e^{16}$                                 | 2579     |
| 9542:34    | $0, 0, 0, 0, -e^{12}, e^{15} + e^{23}, -e^{14} + e^{25}, e^{16} + e^{35}, e^{27} + e^{45}$                               | 2479     |
| 9542:35a   | $0, 0, 0, 0, e^{12}, e^{23} + e^{15}, e^{13} + e^{25}, e^{17} + e^{26}, e^{27} + e^{16}$                                 | 3579     |
| 9542:35b   | $0, 0, 0, 0, e^{12}, -e^{15} + e^{23}, e^{13} + e^{25}, -e^{17} + e^{26}, e^{27} + e^{16}$                               | 3579     |
| 9542:36a   | $0, 0, 0, 0, -e^{12}, e^{15} + e^{23}, e^{13} + e^{25}, e^{35} + e^{16}, e^{26} + e^{34} + e^{17}$                       | 2579     |
| 9542:36b   | $0, 0, 0, 0, -e^{12}, e^{15} + e^{23}, e^{25} - e^{13}, e^{16} + e^{35}, e^{17} + e^{26} + e^{34}$                       | 2579     |
| 9542:37    | $0, 0, 0, 0, e^{12}, e^{13} + e^{25}, e^{15}, e^{35} + e^{14} + e^{26}, e^{27} + e^{16} + e^{34}$                        | 2579     |
| 9542:38a   | $0, 0, 0, 0, e^{12}, e^{15}, e^{25} + e^{13}, e^{17} + e^{26}, e^{27} + e^{16} + e^{35}$                                 | 3579     |
| 9542:38b   | $0, 0, 0, 0, e^{12}, -e^{15}, e^{13} + e^{25}, e^{26} - e^{17}, e^{16} + e^{27} + e^{35}$                                | 3579     |
| 9542:39    | $0, 0, 0, 0, -e^{12}, e^{15} + e^{23}, e^{14} + e^{25}, e^{16} + e^{35}, e^{17} + e^{26}$                                | 2479     |
| 9542:40a   | $0, 0, 0, 0, e^{12}, e^{13} + e^{25}, e^{23} + e^{15}, e^{35} + e^{14} + e^{26}, e^{27} + e^{16}$                        | 2579     |
| 9542:40b   | $0, 0, 0, 0, -e^{12}, e^{25} - e^{13}, e^{15} + e^{23}, e^{14} + e^{26} + e^{35}, e^{16} + e^{27}$                       | 2579     |
| 9542:41a   | $0, 0, 0, 0, e^{12}, e^{23} + e^{15}, e^{13} + e^{25}, e^{27} + e^{16}, e^{17} + e^{26} + e^{34}$                        | 2579     |
| 9542:41b   | $0, 0, 0, 0, e^{12}, e^{15} + e^{23}, -e^{13} + e^{25}, e^{27} - e^{16}, e^{17} + e^{26} + e^{34}$                       | 2579     |
| 9542:42a   | $0, 0, 0, 0, e^{12}, e^{13} + e^{25}, e^{23} + e^{15}, e^{27} + e^{16}, e^{17} + e^{26} + e^{34}$                        | 2579     |
| 9542:42b   | $0, 0, 0, 0, e^{12}, e^{13} + e^{25}, -e^{15} + e^{23}, e^{27} - e^{16}, e^{17} + e^{26} + e^{34}$                       | 2579     |
| 9542:43    | $0, 0, 0, 0, -e^{12}, e^{23} + e^{15}, e^{25} - e^{14}, e^{16} + e^{35}, e^{27} + e^{45} + e^{13}$                       | 2479     |
| 9542:44a   | $0, 0, 0, 0, e^{12}, e^{15}, e^{25} + e^{13}, e^{17} + e^{26} + e^{34}, e^{27} + e^{16} + e^{35}$                        | 2579     |
| 9542:44b   | $0, 0, 0, 0, e^{12}, -e^{15}, e^{13} + e^{25}, -e^{17} + e^{34} + e^{26}, e^{27} + e^{35} + e^{16}$                      | 2579     |
| 9542:45    | $0, 0, 0, 0, -e^{12}, e^{15} + e^{23}, a_3 e^{14} + e^{25}, e^{16} + e^{35}, e^{17} + e^{26} + e^{34}$                   | 2479     |
| 9542:46a   | $0, 0, 0, 0, -e^{12}, e^{15} + e^{23}, e^{25} + e^{13}, e^{16} + e^{24} + e^{35}, e^{17} + e^{26} + e^{34}$              | 2579     |
| 9542:46b   | $0, 0, 0, 0, -e^{12}, e^{15} + e^{23}, -e^{13} + e^{25}, e^{24} + e^{35} + e^{16}, e^{26} + e^{34} + e^{17}$             | 2579     |
| 9542:47a   | $0, 0, 0, 0, e^{12} a_1, e^{13}(1 + a_1) + e^{25}, e^{15} + e^{23}, e^{27} + e^{16}, e^{17} + e^{26} + e^{35}$           | 3579     |
| 9542:47b   | $0, 0, 0, 0, e^{12} a_1, e^{13}(1 + a_1) + e^{25}, -e^{15} + e^{23}, -e^{16} + e^{27}, e^{17} + e^{26} + e^{35}$         | 3579     |
| 9542:48    | $0, 0, 0, 0, e^{12}, e^{13} + e^{25}, e^{24} + e^{15}, e^{35} + e^{14} + e^{26}, e^{27} + e^{16}$                        | 2479     |
| 9542:49a   | $0, 0, 0, 0, e^{12} a_1, e^{15} + e^{23}, e^{25} + e^{13}(1 + a_1), e^{17} + e^{26} + e^{34}, e^{27} + e^{16} + e^{35}$  | 2579     |
| 9542:49b   | $0, 0, 0, 0, e^{12} a_1, e^{23} - e^{15}, e^{25} + e^{13}(1 + a_1), -e^{17} + e^{26} + e^{34}, e^{16} + e^{27} + e^{35}$ | 2579     |
| 9542:50    | $0, 0, 0, 0, -e^{12}, e^{15} + e^{23}, e^{25} - e^{14}, e^{35} + e^{16} + e^{24}, e^{27} + e^{45} + e^{13}$              | 2479     |
| 9542:51    | $0, 0, 0, 0, -e^{12}, e^{15} + e^{23}, e^{14} a_3 + e^{25}, e^{16} + e^{35} + e^{24}, e^{17} + e^{26} + e^{34}$          | 2479     |
| Type: 4221 |                                                                                                                          |          |
| 9531:1     | $0, 0, 0, 0, e^{12}, e^{34}, e^{15}, e^{25}, e^{17}$                                                                     | 3679     |
| 9531:2     | $0, 0, 0, 0, e^{12}, e^{13}, e^{15}, e^{25}, e^{17}$                                                                     | 4679     |
| 9531:3     | $0, 0, 0, 0, e^{12}, e^{13}, e^{25}, e^{15}, e^{27}$                                                                     | 4679     |
| 9531:4     | $0, 0, 0, 0, e^{12}, e^{13}, e^{15}, e^{34} + e^{25}, e^{17}$                                                            | 3679     |
| 9531:5     | $0, 0, 0, 0, e^{12}, e^{13}, e^{25}, e^{15} + e^{34}, e^{27}$                                                            | 3679     |
| 9531:6     | $0, 0, 0, 0, e^{12}, e^{34}, e^{15}, e^{13} + e^{25}, e^{17}$                                                            | 3679     |
| 9531:7     | $0, 0, 0, 0, e^{12}, e^{13}, e^{15}, e^{36}, e^{17}$                                                                     | 3579     |
| 9531:8     | $0, 0, 0, 0, e^{12}, e^{13}, e^{25}, e^{36}, e^{27}$                                                                     | 3579     |
| 9531:9     | $0, 0, 0, 0, e^{12}, e^{13}, e^{25}, e^{15} + e^{23}, e^{27}$                                                            | 4679     |
| 9531:10    | $0, 0, 0, 0, e^{12}, e^{13}, e^{15}, e^{25}, e^{17} + e^{34}$                                                            | 3679     |
| 9531:11    | $0, 0, 0, 0, e^{12}, e^{13}, e^{25}, e^{15}, e^{34} + e^{27}$                                                            | 3679     |
| 9531:12    | $0, 0, 0, 0, e^{12}, e^{13} + e^{24}, e^{15}, e^{25}, e^{17}$                                                            | 3679     |

Table 2 – Continued to next page

Table 2 – Continued from previous page

| Name     | $\mathfrak{g}$                                                                   | UCS Dim. |
|----------|----------------------------------------------------------------------------------|----------|
| 9531:13  | $0, 0, 0, 0, e^{12}, e^{34}, e^{15}, e^{25}, e^{17} + e^{23}$                    | 3679     |
| 9531:14  | $0, 0, 0, 0, e^{12}, e^{13}, e^{15}, e^{14} + e^{25}, e^{17}$                    | 3679     |
| 9531:15  | $0, 0, 0, 0, e^{12}, e^{13}, e^{25}, e^{24} + e^{15}, e^{27}$                    | 3679     |
| 9531:16  | $0, 0, 0, 0, e^{12}, e^{13} + e^{24}, e^{15}, e^{25} + e^{34}, e^{17}$           | 3679     |
| 9531:17  | $0, 0, 0, 0, e^{12}, e^{13}, e^{15}, e^{16}, e^{17}$                             | 3579     |
| 9531:18  | $0, 0, 0, 0, e^{12}, e^{13}, e^{25}, e^{16}, e^{27}$                             | 3579     |
| 9531:19  | $0, 0, 0, 0, e^{12}, e^{13}, e^{15}, e^{25}, e^{17} + e^{23}$                    | 4679     |
| 9531:20  | $0, 0, 0, 0, e^{12}, e^{13}, e^{15}, e^{25}, e^{17} + e^{24}$                    | 3679     |
| 9531:21  | $0, 0, 0, 0, e^{12}, e^{13}, e^{25}, e^{15}, e^{27} + e^{14}$                    | 3679     |
| 9531:22  | $0, 0, 0, 0, e^{12}, e^{34}, e^{15}, e^{36}, e^{17}$                             | 2479     |
| 9531:23a | $0, 0, 0, 0, e^{12}, e^{24} + e^{13}, e^{15}, e^{25}, e^{34} + e^{17}$           | 3679     |
| 9531:23b | $0, 0, 0, 0, -e^{12}, e^{13} + e^{24}, e^{15}, e^{25}, e^{17} + e^{34}$          | 3679     |
| 9531:24  | $0, 0, 0, 0, e^{12}, e^{13}, e^{25}, e^{15} + e^{23}, e^{27} + e^{34}$           | 3679     |
| 9531:25  | $0, 0, 0, 0, e^{12}, e^{13}, e^{15}, e^{25} + e^{34}, e^{17} + e^{23}$           | 3679     |
| 9531:26  | $0, 0, 0, 0, e^{12}, e^{13}, e^{15}, e^{14} + e^{25}, e^{17} + e^{34}$           | 3679     |
| 9531:27  | $0, 0, 0, 0, e^{12}, e^{13}, e^{25}, e^{15} + e^{24}, e^{34} + e^{27}$           | 3679     |
| 9531:28  | $0, 0, 0, 0, e^{12}, e^{13}, e^{15}, e^{34} + e^{25}, e^{24} + e^{17}$           | 3679     |
| 9531:29  | $0, 0, 0, 0, e^{12}, e^{13}, e^{25}, e^{15} + e^{34}, e^{14} + e^{27}$           | 3679     |
| 9531:30  | $0, 0, 0, 0, e^{12}, e^{14} + e^{23}, e^{15}, e^{13} + e^{25}, e^{17}$           | 3679     |
| 9531:31  | $0, 0, 0, 0, e^{12}, e^{34}, e^{15}, e^{13} + e^{25}, e^{23} + e^{17}$           | 3679     |
| 9531:32  | $0, 0, 0, 0, e^{12}, e^{34}, e^{15}, e^{25} + e^{13}, e^{17} + e^{24}$           | 3679     |
| 9531:33  | $0, 0, 0, 0, e^{12}, e^{13}, e^{15}, e^{36}, e^{17} + e^{34}$                    | 2579     |
| 9531:34  | $0, 0, 0, 0, e^{12}, e^{13}, e^{25}, e^{36}, e^{34} + e^{27}$                    | 2579     |
| 9531:35  | $0, 0, 0, 0, e^{12}, e^{13}, e^{15}, e^{36} + e^{14}, e^{17}$                    | 2579     |
| 9531:36  | $0, 0, 0, 0, e^{12}, e^{13}, e^{15}, e^{34} + e^{16}, e^{17}$                    | 2579     |
| 9531:37  | $0, 0, 0, 0, e^{12}, e^{13}, e^{15}, e^{24} + e^{36}, e^{17}$                    | 2579     |
| 9531:38  | $0, 0, 0, 0, e^{12}, e^{13}, e^{25}, e^{36} + e^{14}, e^{27}$                    | 2579     |
| 9531:39  | $0, 0, 0, 0, e^{12}, e^{13}, e^{25}, e^{34} + e^{16}, e^{27}$                    | 2579     |
| 9531:40  | $0, 0, 0, 0, e^{12}, e^{13}, e^{25}, e^{36} + e^{24}, e^{27}$                    | 2579     |
| 9531:41  | $0, 0, 0, 0, e^{12}, e^{24} + e^{13}, e^{15}, e^{25}, e^{17} + e^{23}$           | 3679     |
| 9531:42  | $0, 0, 0, 0, e^{12}, e^{13}, e^{15}, e^{16} + e^{23}, e^{17}$                    | 3579     |
| 9531:43  | $0, 0, 0, 0, e^{12}, e^{13}, e^{25}, e^{23} + e^{16}, e^{27}$                    | 3579     |
| 9531:44  | $0, 0, 0, 0, e^{12}, e^{13}, e^{15}, e^{36}, e^{17} + e^{23}$                    | 3579     |
| 9531:45  | $0, 0, 0, 0, e^{12}, e^{13}, e^{15}, e^{16}, e^{17} + e^{34}$                    | 2579     |
| 9531:46  | $0, 0, 0, 0, e^{12}, e^{13}, e^{25}, e^{16}, e^{34} + e^{27}$                    | 2579     |
| 9531:47  | $0, 0, 0, 0, e^{12}, e^{13}, e^{15}, e^{36}, e^{24} + e^{17}$                    | 2579     |
| 9531:48  | $0, 0, 0, 0, e^{12}, e^{13}, e^{25}, e^{36}, e^{27} + e^{14}$                    | 2579     |
| 9531:49  | $0, 0, 0, 0, e^{12}, e^{13}, e^{15}, e^{16} + e^{24}, e^{17}$                    | 2579     |
| 9531:50  | $0, 0, 0, 0, e^{12}, e^{13}, e^{25}, e^{16} + e^{24}, e^{27}$                    | 2579     |
| 9531:51  | $0, 0, 0, 0, e^{12}, e^{13}, e^{25}, e^{15} + e^{23}, e^{27} + e^{14}$           | 3679     |
| 9531:52  | $0, 0, 0, 0, e^{12}, e^{13}, e^{15}, e^{14} + e^{25}, e^{17} + e^{23}$           | 3679     |
| 9531:53  | $0, 0, 0, 0, e^{12}, e^{13}, e^{15}, e^{14} + e^{25}, e^{24} + e^{17}$           | 3679     |
| 9531:54  | $0, 0, 0, 0, e^{12}, e^{13}, e^{25}, e^{24} + e^{15}, e^{27} + e^{14}$           | 3679     |
| 9531:55a | $0, 0, 0, 0, e^{12}, e^{14} + e^{23}, e^{15}, e^{13} + e^{25}, e^{17} + e^{34}$  | 3679     |
| 9531:55b | $0, 0, 0, 0, -e^{12}, e^{14} + e^{23}, e^{15}, e^{13} + e^{25}, e^{34} + e^{17}$ | 3679     |
| 9531:56  | $0, 0, 0, 0, e^{12}, e^{24} + e^{13}, e^{15}, e^{25} + e^{34}, e^{17} + e^{23}$  | 3679     |
| 9531:57  | $0, 0, 0, 0, e^{12}, e^{34}, e^{15}, e^{13} + e^{46}, e^{17}$                    | 2479     |
| 9531:58  | $0, 0, 0, 0, e^{12}, e^{34}, e^{15}, e^{23} + e^{46}, e^{17}$                    | 2479     |
| 9531:59a | $0, 0, 0, 0, e^{12}, e^{13}, e^{15}, e^{25} + e^{36}, e^{17}$                    | 3579     |
| 9531:59b | $0, 0, 0, 0, -e^{12}, e^{13}, e^{15}, e^{36} + e^{25}, e^{17}$                   | 3579     |
| 9531:60  | $0, 0, 0, 0, e^{12}, e^{13}, e^{15}, e^{26} + e^{35}, e^{17}$                    | 3579     |
| 9531:61  | $0, 0, 0, 0, e^{12}, e^{13}, e^{25}, e^{36} + e^{15}, e^{27}$                    | 3579     |
| 9531:62  | $0, 0, 0, 0, e^{12}, e^{13}, e^{25}, e^{26} + e^{35}, e^{27}$                    | 3579     |
| 9531:63  | $0, 0, 0, 0, e^{12}, e^{13}, e^{15}, e^{16}, e^{36} + e^{17}$                    | 3579     |
| 9531:64  | $0, 0, 0, 0, e^{12}, e^{13}, e^{25}, e^{16}, e^{27} + e^{36}$                    | 3579     |
| 9531:65  | $0, 0, 0, 0, e^{12}, e^{13}, e^{25}, e^{36}, e^{27} + e^{16}$                    | 3579     |
| 9531:66  | $0, 0, 0, 0, e^{12}, e^{13}, e^{15}, e^{36} + e^{14}, e^{34} + e^{17}$           | 2579     |
| 9531:67  | $0, 0, 0, 0, e^{12}, e^{13}, e^{15}, e^{36} + e^{24}, e^{17} + e^{34}$           | 2579     |

Table 2 – Continued to next page

Table 2 – Continued from previous page

| Name      | $\mathfrak{g}$                                                                  | UCS Dim. |
|-----------|---------------------------------------------------------------------------------|----------|
| 9531:68   | $0, 0, 0, 0, e^{12}, e^{13}, e^{25}, e^{14} + e^{36}, e^{27} + e^{34}$          | 2579     |
| 9531:69   | $0, 0, 0, 0, e^{12}, e^{13}, e^{25}, e^{36} + e^{24}, e^{27} + e^{34}$          | 2579     |
| 9531:70   | $0, 0, 0, 0, e^{12}, e^{34}, e^{15}, e^{36}, e^{46} + e^{17}$                   | 2479     |
| 9531:71   | $0, 0, 0, 0, e^{12}, e^{13}, e^{15}, e^{16} + e^{34}, e^{17} + e^{36}$          | 2579     |
| 9531:72   | $0, 0, 0, 0, e^{12}, e^{13}, e^{25}, e^{16} + e^{34}, e^{27} + e^{36}$          | 2579     |
| 9531:73   | $0, 0, 0, 0, e^{12}, e^{13}, e^{15}, e^{16}, e^{23} + e^{17}$                   | 3579     |
| 9531:74   | $0, 0, 0, 0, e^{12}, e^{13}, e^{15}, e^{16}, e^{24} + e^{17}$                   | 2579     |
| 9531:75   | $0, 0, 0, 0, e^{12}, e^{13}, e^{25}, e^{16}, e^{14} + e^{27}$                   | 2579     |
| 9531:76   | $0, 0, 0, 0, e^{12}, e^{34}, e^{15}, e^{36}, e^{17} + e^{23}$                   | 2479     |
| 9531:77   | $0, 0, 0, 0, e^{12}, e^{34}, e^{15}, e^{36}, e^{17} + e^{24}$                   | 2479     |
| 9531:78   | $0, 0, 0, 0, e^{12}, e^{14} + e^{23}, e^{15}, e^{25} + e^{13}, e^{17} + e^{24}$ | 3679     |
| 9531:79   | $0, 0, 0, 0, e^{12}, e^{13}, e^{15}, e^{25} + e^{16}, e^{17}$                   | 3579     |
| 9531:80   | $0, 0, 0, 0, e^{12}, e^{13}, e^{15}, e^{24} + e^{16}, e^{34} + e^{17}$          | 2579     |
| 9531:81   | $0, 0, 0, 0, e^{12}, e^{13}, e^{25}, e^{24} + e^{16}, e^{27} + e^{34}$          | 2579     |
| 9531:82   | $0, 0, 0, 0, e^{12}, e^{13}, e^{15}, e^{36} + e^{14}, e^{24} + e^{17}$          | 2579     |
| 9531:83   | $0, 0, 0, 0, e^{12}, e^{13}, e^{15}, e^{34} + e^{16}, e^{17} + e^{24}$          | 2579     |
| 9531:84   | $0, 0, 0, 0, e^{12}, e^{13}, e^{25}, e^{34} + e^{16}, e^{14} + e^{27}$          | 2579     |
| 9531:85   | $0, 0, 0, 0, e^{12}, e^{13}, e^{25}, e^{36} + e^{24}, e^{27} + e^{14}$          | 2579     |
| 9531:86   | $0, 0, 0, 0, e^{12}, e^{13}, e^{15}, e^{25}, e^{17} + e^{36}$                   | 3579     |
| 9531:87   | $0, 0, 0, 0, e^{12}, e^{13}, e^{25}, e^{15}, e^{36} + e^{27}$                   | 3579     |
| 9531:88   | $0, 0, 0, 0, e^{12}, e^{13}, e^{15}, e^{36}, e^{25} + e^{17}$                   | 3579     |
| 9531:89   | $0, 0, 0, 0, e^{12}, e^{13}, e^{25}, e^{36}, e^{15} + e^{27}$                   | 3579     |
| 9531:90   | $0, 0, 0, 0, e^{12}, e^{13}, e^{15}, e^{16} + e^{23}, e^{34} + e^{17}$          | 2579     |
| 9531:91   | $0, 0, 0, 0, e^{12}, e^{13}, e^{25}, e^{23} + e^{16}, e^{34} + e^{27}$          | 2579     |
| 9531:92   | $0, 0, 0, 0, e^{12}, e^{13}, e^{15}, e^{36} + e^{14}, e^{17} + e^{23}$          | 2579     |
| 9531:93   | $0, 0, 0, 0, e^{12}, e^{13}, e^{15}, e^{16} + e^{34}, e^{17} + e^{23}$          | 2579     |
| 9531:94   | $0, 0, 0, 0, e^{12}, e^{13}, e^{15}, e^{24} + e^{36}, e^{17} + e^{23}$          | 2579     |
| 9531:95   | $0, 0, 0, 0, e^{12}, e^{34}, e^{15}, e^{36} + e^{25}, e^{17}$                   | 2479     |
| 9531:96a  | $0, 0, 0, 0, e^{12}, e^{13}, e^{15}, e^{16} + e^{23}, e^{17} + e^{36}$          | 3579     |
| 9531:96b  | $0, 0, 0, 0, -e^{12}, e^{13}, e^{15}, e^{23} + e^{16}, e^{36} + e^{17}$         | 3579     |
| 9531:97a  | $0, 0, 0, 0, e^{12}, e^{13}, e^{25}, e^{16} + e^{23}, e^{36} + e^{27}$          | 3579     |
| 9531:97b  | $0, 0, 0, 0, -e^{12}, e^{13}, e^{25}, e^{23} + e^{16}, e^{27} + e^{36}$         | 3579     |
| 9531:98a  | $0, 0, 0, 0, e^{12}, e^{13}, e^{15}, e^{36} + e^{25}, e^{34} + e^{17}$          | 2579     |
| 9531:98b  | $0, 0, 0, 0, -e^{12}, e^{13}, e^{15}, e^{25} + e^{36}, e^{17} + e^{34}$         | 2579     |
| 9531:99   | $0, 0, 0, 0, e^{12}, e^{13}, e^{15}, e^{26} + e^{35}, e^{17} + e^{34}$          | 2579     |
| 9531:100  | $0, 0, 0, 0, e^{12}, e^{13}, e^{25}, e^{15} + e^{36}, e^{34} + e^{27}$          | 2579     |
| 9531:101  | $0, 0, 0, 0, e^{12}, e^{13}, e^{25}, e^{35} + e^{26}, e^{27} + e^{34}$          | 2579     |
| 9531:102a | $0, 0, 0, 0, e^{12}, e^{13}, e^{15}, e^{25} + e^{14} + e^{36}, e^{17}$          | 2579     |
| 9531:102b | $0, 0, 0, 0, -e^{12}, e^{13}, e^{15}, e^{36} + e^{25} + e^{14}, e^{17}$         | 2579     |
| 9531:103  | $0, 0, 0, 0, e^{12}, e^{13}, e^{15}, e^{26} + e^{35} + e^{14}, e^{17}$          | 2579     |
| 9531:104  | $0, 0, 0, 0, e^{12}, e^{13}, e^{15}, e^{25} + e^{16} + e^{34}, e^{17}$          | 2579     |
| 9531:105  | $0, 0, 0, 0, e^{12}, e^{13}, e^{25}, e^{15} + e^{24} + e^{36}, e^{27}$          | 2579     |
| 9531:106  | $0, 0, 0, 0, e^{12}, e^{13}, e^{25}, e^{35} + e^{14} + e^{26}, e^{27}$          | 2579     |
| 9531:107  | $0, 0, 0, 0, e^{12}, e^{13}, e^{25}, e^{36}, e^{27} + e^{34} + e^{16}$          | 2579     |
| 9531:108  | $0, 0, 0, 0, e^{12}, e^{13}, e^{15}, e^{16} + e^{24}, e^{36} + e^{17}$          | 2579     |
| 9531:109  | $0, 0, 0, 0, e^{12}, e^{13}, e^{25}, e^{16} + e^{24}, e^{27} + e^{36}$          | 2579     |
| 9531:110  | $0, 0, 0, 0, e^{12}, e^{13}, e^{25}, e^{14} + e^{36}, e^{16} + e^{27}$          | 2579     |
| 9531:111  | $0, 0, 0, 0, e^{12}, e^{13}, e^{25}, e^{24} + e^{36}, e^{27} + e^{16}$          | 2579     |
| 9531:112  | $0, 0, 0, 0, e^{12}, e^{34}, e^{15}, e^{46} + e^{13}, e^{36} + e^{17}$          | 2479     |
| 9531:113  | $0, 0, 0, 0, e^{12}, e^{34}, e^{15}, e^{23} + e^{46}, e^{36} + e^{17}$          | 2479     |
| 9531:114  | $0, 0, 0, 0, e^{12}, e^{13}, e^{15}, e^{25} + e^{34}, e^{36} + e^{17}$          | 2579     |
| 9531:115  | $0, 0, 0, 0, e^{12}, e^{13}, e^{25}, e^{15} + e^{34}, e^{27} + e^{36}$          | 2579     |
| 9531:116  | $0, 0, 0, 0, e^{12}, e^{13}, e^{23} + e^{15}, e^{36}, e^{17} + e^{26}$          | 3579     |
| 9531:117  | $0, 0, 0, 0, e^{12}, e^{13}, e^{15}, e^{26} + e^{35}, e^{17} + e^{36}$          | 3579     |
| 9531:118  | $0, 0, 0, 0, e^{12}, e^{13}, e^{25}, e^{35} + e^{26}, e^{27} + e^{36}$          | 3579     |
| 9531:119  | $0, 0, 0, 0, e^{12}, e^{34}, e^{13} + e^{25}, e^{15}, e^{27} + e^{35}$          | 3579     |
| 9531:120  | $0, 0, 0, 0, -e^{12}, e^{13}, e^{15} + e^{23}, e^{36}, e^{17} + e^{35}$         | 3579     |
| 9531:121  | $0, 0, 0, 0, e^{12}, -e^{13}, e^{34} + e^{15}, e^{36}, e^{46} + e^{17}$         | 2479     |

Table 2 – Continued to next page

Table 2 – Continued from previous page

| Name      | $\mathfrak{g}$                                                                   | UCS Dim. |
|-----------|----------------------------------------------------------------------------------|----------|
| 9531:122  | $0, 0, 0, 0, e^{12}, e^{13}, e^{25}, e^{16} + e^{24}, e^{14} + e^{27}$           | 2579     |
| 9531:123  | $0, 0, 0, 0, e^{12}, e^{13}, e^{25}, e^{15}, e^{27} + e^{16}$                    | 3579     |
| 9531:124  | $0, 0, 0, 0, e^{12}, e^{13}, e^{15}, e^{16}, e^{25} + e^{17}$                    | 3579     |
| 9531:125  | $0, 0, 0, 0, e^{12}, e^{13}, e^{25}, e^{16}, e^{15} + e^{27}$                    | 3579     |
| 9531:126  | $0, 0, 0, 0, e^{12}, e^{13}, e^{15}, e^{16} + e^{23}, e^{17} + e^{24}$           | 2579     |
| 9531:127  | $0, 0, 0, 0, e^{12}, e^{13}, e^{25}, e^{16} + e^{23}, e^{27} + e^{14}$           | 2579     |
| 9531:128  | $0, 0, 0, 0, e^{12}, e^{13}, e^{15}, e^{16} + e^{24}, e^{17} + e^{23}$           | 2579     |
| 9531:129  | $0, 0, 0, 0, e^{12}, e^{34}, e^{15}, e^{13} + e^{46}, e^{17} + e^{23}$           | 2479     |
| 9531:130  | $0, 0, 0, 0, e^{12}, e^{34}, e^{15}, e^{36} + e^{14}, e^{23} + e^{17}$           | 2479     |
| 9531:131  | $0, 0, 0, 0, e^{12}, e^{34}, e^{15}, e^{24} + e^{36}, e^{23} + e^{17}$           | 2479     |
| 9531:132  | $0, 0, 0, 0, e^{12}, e^{34}, e^{15}, e^{25}, e^{36} + e^{17}$                    | 2479     |
| 9531:133  | $0, 0, 0, 0, e^{12}, e^{34}, e^{15}, e^{36}, e^{17} + e^{25}$                    | 2479     |
| 9531:134a | $0, 0, 0, 0, e^{12}, e^{13}, e^{15}, e^{36} + e^{25}, e^{23} + e^{17}$           | 3579     |
| 9531:134b | $0, 0, 0, 0, -e^{12}, e^{13}, e^{15}, e^{25} + e^{36}, e^{17} + e^{23}$          | 3579     |
| 9531:135  | $0, 0, 0, 0, e^{12}, e^{13}, e^{15}, e^{26} + e^{35}, e^{17} + e^{23}$           | 3579     |
| 9531:136  | $0, 0, 0, 0, e^{12}, e^{13}, e^{15}, e^{25} + e^{16}, e^{34} + e^{17}$           | 2579     |
| 9531:137a | $0, 0, 0, 0, e^{12}, e^{13}, e^{15}, e^{36} + e^{25}, e^{24} + e^{17}$           | 2579     |
| 9531:137b | $0, 0, 0, 0, -e^{12}, e^{13}, e^{15}, e^{36} + e^{25}, e^{24} + e^{17}$          | 2579     |
| 9531:138  | $0, 0, 0, 0, e^{12}, e^{13}, e^{15}, e^{26} + e^{35}, e^{24} + e^{17}$           | 2579     |
| 9531:139  | $0, 0, 0, 0, e^{12}, e^{13}, e^{25}, e^{15} + e^{36}, e^{27} + e^{14}$           | 2579     |
| 9531:140  | $0, 0, 0, 0, e^{12}, e^{13}, e^{25}, e^{26} + e^{35}, e^{14} + e^{27}$           | 2579     |
| 9531:141  | $0, 0, 0, 0, e^{12}, e^{13}, e^{15}, e^{16}, e^{17} + e^{24} + e^{36}$           | 2579     |
| 9531:142  | $0, 0, 0, 0, e^{12}, e^{13}, e^{25}, e^{16}, e^{36} + e^{14} + e^{27}$           | 2579     |
| 9531:143  | $0, 0, 0, 0, e^{12}, e^{34}, e^{15}, e^{36}, e^{17} + e^{23} + e^{46}$           | 2479     |
| 9531:144  | $0, 0, 0, 0, e^{12}, e^{13}, e^{25}, e^{15} + e^{23}, e^{27} + e^{36}$           | 3579     |
| 9531:145  | $0, 0, 0, 0, e^{12}, e^{13}, e^{15}, e^{14} + e^{25}, e^{36} + e^{17}$           | 2579     |
| 9531:146  | $0, 0, 0, 0, e^{12}, e^{13}, e^{25}, e^{15} + e^{24}, e^{27} + e^{36}$           | 2579     |
| 9531:147  | $0, 0, 0, 0, e^{12}, e^{13}, e^{25}, e^{15} + e^{34}, e^{16} + e^{27}$           | 2579     |
| 9531:148  | $0, 0, 0, 0, e^{12}, e^{13}, e^{15}, e^{36}, e^{17} + e^{25} + e^{34}$           | 2579     |
| 9531:149  | $0, 0, 0, 0, e^{12}, e^{13}, e^{25}, e^{36}, e^{15} + e^{34} + e^{27}$           | 2579     |
| 9531:150  | $0, 0, 0, 0, e^{12}, e^{13}, e^{15}, e^{36} + e^{14}, e^{17} + e^{25}$           | 2579     |
| 9531:151  | $0, 0, 0, 0, e^{12}, e^{13}, e^{15}, e^{34} + e^{16}, e^{25} + e^{17}$           | 2579     |
| 9531:152  | $0, 0, 0, 0, e^{12}, e^{13}, e^{15}, e^{24} + e^{36}, e^{25} + e^{17}$           | 2579     |
| 9531:153  | $0, 0, 0, 0, e^{12}, e^{13}, e^{25}, e^{36} + e^{14}, e^{27} + e^{15}$           | 2579     |
| 9531:154  | $0, 0, 0, 0, e^{12}, e^{13}, e^{25}, e^{16} + e^{34}, e^{15} + e^{27}$           | 2579     |
| 9531:155  | $0, 0, 0, 0, e^{12}, e^{13}, e^{25}, e^{24} + e^{36}, e^{15} + e^{27}$           | 2579     |
| 9531:156  | $0, 0, 0, 0, e^{12}, e^{34}, e^{15}, e^{13} + e^{25} + e^{46}, e^{17}$           | 2479     |
| 9531:157  | $0, 0, 0, 0, e^{12}, e^{13}, e^{15} + e^{23}, e^{16}, e^{17} + e^{26}$           | 3579     |
| 9531:158  | $0, 0, 0, 0, e^{12}, e^{13}, e^{15}, e^{25} + e^{16}, e^{36} + e^{17}$           | 3579     |
| 9531:159  | $0, 0, 0, 0, e^{12}, e^{13}, e^{25}, e^{36} + e^{15}, e^{27} + e^{16}$           | 3579     |
| 9531:160  | $0, 0, 0, 0, e^{12}, e^{13}, e^{25}, e^{26} + e^{35}, e^{27} + e^{16}$           | 3579     |
| 9531:161a | $0, 0, 0, 0, e^{12}, e^{13}, e^{15}, e^{14} + e^{36} + e^{25}, e^{17} + e^{34}$  | 2579     |
| 9531:161b | $0, 0, 0, 0, -e^{12}, e^{13}, e^{15}, e^{25} + e^{14} + e^{36}, e^{17} + e^{34}$ | 2579     |
| 9531:162  | $0, 0, 0, 0, e^{12}, e^{13}, e^{15}, e^{35} + e^{26} + e^{14}, e^{34} + e^{17}$  | 2579     |
| 9531:163  | $0, 0, 0, 0, e^{12}, e^{13}, e^{25}, e^{24} + e^{36} + e^{15}, e^{34} + e^{27}$  | 2579     |
| 9531:164  | $0, 0, 0, 0, e^{12}, e^{13}, e^{25}, e^{14} + e^{26} + e^{35}, e^{34} + e^{27}$  | 2579     |
| 9531:165  | $0, 0, 0, 0, e^{12}, e^{13}, e^{15}, e^{16} + e^{34}, e^{17} + e^{36} + e^{24}$  | 2579     |
| 9531:166a | $0, 0, 0, 0, e^{12}, e^{13}, e^{25}, e^{14} + e^{36}, e^{16} + e^{34} + e^{27}$  | 2579     |
| 9531:166b | $0, 0, 0, 0, e^{12}, e^{13}, e^{25}, e^{36} - e^{14}, e^{34} + e^{27} + e^{16}$  | 2579     |
| 9531:167a | $0, 0, 0, 0, e^{12}, e^{13}, e^{25}, e^{34} + e^{16}, e^{27} + e^{36} + e^{14}$  | 2579     |
| 9531:167b | $0, 0, 0, 0, e^{12}, e^{13}, e^{25}, -e^{16} + e^{34}, e^{36} + e^{14} + e^{27}$ | 2579     |
| 9531:168  | $0, 0, 0, 0, e^{12}, e^{13}, e^{25}, e^{24} + e^{36}, e^{34} + e^{27} + e^{16}$  | 2579     |
| 9531:169  | $0, 0, 0, 0, e^{12}, e^{34}, e^{15}, e^{36} + e^{25}, e^{17} + e^{46}$           | 2479     |
| 9531:170  | $0, 0, 0, 0, -e^{12}, e^{13}, e^{15} + e^{23}, e^{25}, e^{17} + e^{35}$          | 4579     |
| 9531:171  | $0, 0, 0, 0, e^{12}, e^{13}, e^{14} + e^{25}, e^{15}, e^{45} + e^{27}$           | 3579     |
| 9531:172  | $0, 0, 0, 0, -e^{12}, e^{13}, e^{24} + e^{15}, e^{25}, e^{45} + e^{17}$          | 3579     |
| 9531:173  | $0, 0, 0, 0, -e^{12}, e^{13}, e^{15} + e^{23}, e^{16}, e^{17} + e^{35}$          | 3579     |
| 9531:174  | $0, 0, 0, 0, e^{12}, e^{13}, e^{15}, e^{36}, e^{17} + e^{26} + e^{35}$           | 3579     |

Table 2 – Continued to next page

Table 2 – Continued from previous page

| Name      | $\mathfrak{g}$                                                                   | UCS Dim. |
|-----------|----------------------------------------------------------------------------------|----------|
| 9531:175  | $0, 0, 0, 0, e^{12}, -e^{13}, e^{15} + e^{34}, e^{16}, e^{17} + e^{46}$          | 2479     |
| 9531:176  | $0, 0, 0, 0, -e^{12}, e^{34}, e^{23} + e^{15}, e^{36}, e^{35} + e^{17}$          | 2479     |
| 9531:177  | $0, 0, 0, 0, -e^{12}, e^{34}, e^{15} + e^{23}, e^{46}, e^{17} + e^{35}$          | 2479     |
| 9531:178  | $0, 0, 0, 0, e^{12}, e^{13}, e^{14} + e^{25}, e^{15} + e^{34}, e^{27} + e^{45}$  | 3579     |
| 9531:179  | $0, 0, 0, 0, -e^{12}, e^{13}, e^{15} + e^{24}, e^{34} + e^{25}, e^{45} + e^{17}$ | 3579     |
| 9531:180  | $0, 0, 0, 0, -e^{12}, e^{34}, e^{23} + e^{15}, e^{14} + e^{25}, e^{35} + e^{17}$ | 3579     |
| 9531:181  | $0, 0, 0, 0, e^{12}, e^{13}, e^{15} + e^{23}, e^{36}, e^{26} + e^{34} + e^{17}$  | 2579     |
| 9531:182  | $0, 0, 0, 0, e^{12}, e^{13}, e^{23} + e^{15}, e^{36} + e^{14}, e^{17} + e^{26}$  | 2579     |
| 9531:183  | $0, 0, 0, 0, e^{12}, e^{13}, e^{15} + e^{23}, e^{16} + e^{34}, e^{17} + e^{26}$  | 2579     |
| 9531:184  | $0, 0, 0, 0, e^{12}, e^{13}, e^{15} + e^{23}, e^{24} + e^{36}, e^{17} + e^{26}$  | 2579     |
| 9531:185  | $0, 0, 0, 0, e^{12}, e^{13}, e^{15}, e^{26} + e^{35} + e^{14}, e^{36} + e^{17}$  | 2579     |
| 9531:186  | $0, 0, 0, 0, e^{12}, e^{13}, e^{15}, e^{34} + e^{16} + e^{25}, e^{36} + e^{17}$  | 2579     |
| 9531:187  | $0, 0, 0, 0, e^{12}, e^{13}, e^{25}, e^{26} + e^{35} + e^{14}, e^{27} + e^{36}$  | 2579     |
| 9531:188  | $0, 0, 0, 0, -e^{12}, e^{13}, e^{15} + e^{23}, e^{34} + e^{25}, e^{17} + e^{35}$ | 3579     |
| 9531:189a | $0, 0, 0, 0, -e^{12}, e^{34}, e^{15} + e^{23}, e^{13} + e^{25}, e^{35} + e^{17}$ | 3579     |
| 9531:189b | $0, 0, 0, 0, -e^{12}, e^{34}, e^{23} - e^{15}, e^{25} + e^{13}, e^{17} + e^{35}$ | 3579     |
| 9531:190  | $0, 0, 0, 0, -e^{12}, e^{13}, e^{15} + e^{23}, e^{14} + e^{36}, e^{17} + e^{35}$ | 2579     |
| 9531:191  | $0, 0, 0, 0, -e^{12}, e^{13}, e^{15} + e^{23}, e^{16} + e^{34}, e^{17} + e^{35}$ | 2579     |
| 9531:192  | $0, 0, 0, 0, -e^{12}, e^{13}, e^{15} + e^{23}, e^{24} + e^{36}, e^{35} + e^{17}$ | 2579     |
| 9531:193  | $0, 0, 0, 0, e^{12}, -e^{13}, e^{15} + e^{34}, e^{14} + e^{36}, e^{46} + e^{17}$ | 2479     |
| 9531:194  | $0, 0, 0, 0, e^{12}, -e^{13}, e^{15} + e^{34}, e^{24} + e^{36}, e^{17} + e^{46}$ | 2479     |
| 9531:195a | $0, 0, 0, 0, e^{12}, e^{13}, e^{15}, e^{25} + e^{16}, e^{17} + e^{23}$           | 3579     |
| 9531:195b | $0, 0, 0, 0, e^{12}, -e^{13}, e^{15}, e^{25} + e^{16}, e^{23} + e^{17}$          | 3579     |
| 9531:196  | $0, 0, 0, 0, e^{12}, e^{13}, e^{15}, e^{16} + e^{25}, e^{24} + e^{17}$           | 2579     |
| 9531:197  | $0, 0, 0, 0, e^{12}, e^{13}, e^{25}, e^{15} + e^{23}, e^{27} + e^{16}$           | 3579     |
| 9531:198  | $0, 0, 0, 0, e^{12}, e^{13}, e^{15}, e^{23} + e^{16}, e^{25} + e^{17}$           | 3579     |
| 9531:199  | $0, 0, 0, 0, e^{12}, e^{13}, e^{25}, e^{16} + e^{23}, e^{15} + e^{27}$           | 3579     |
| 9531:200  | $0, 0, 0, 0, e^{12}, e^{13}, e^{15}, e^{25}, e^{17} + e^{24} + e^{36}$           | 2579     |
| 9531:201  | $0, 0, 0, 0, e^{12}, e^{13}, e^{25}, e^{15}, e^{36} + e^{27} + e^{14}$           | 2579     |
| 9531:202  | $0, 0, 0, 0, e^{12}, e^{13}, e^{25}, e^{15}, e^{16} + e^{34} + e^{27}$           | 2579     |
| 9531:203  | $0, 0, 0, 0, e^{12}, e^{13}, e^{25}, e^{24} + e^{15}, e^{27} + e^{16}$           | 2579     |
| 9531:204  | $0, 0, 0, 0, e^{12}, e^{13}, e^{15}, e^{16}, e^{25} + e^{34} + e^{17}$           | 2579     |
| 9531:205  | $0, 0, 0, 0, e^{12}, e^{13}, e^{25}, e^{16}, e^{27} + e^{34} + e^{15}$           | 2579     |
| 9531:206  | $0, 0, 0, 0, e^{12}, e^{13}, e^{15}, e^{16} + e^{24}, e^{17} + e^{25}$           | 2579     |
| 9531:207  | $0, 0, 0, 0, e^{12}, e^{13}, e^{25}, e^{16} + e^{24}, e^{15} + e^{27}$           | 2579     |
| 9531:208  | $0, 0, 0, 0, e^{12}, e^{34}, e^{15}, e^{36} + e^{25}, e^{17} + e^{23}$           | 2479     |
| 9531:209a | $0, 0, 0, 0, e^{12}, e^{34}, e^{15}, e^{36} + e^{25}, e^{17} + e^{24}$           | 2479     |
| 9531:209b | $0, 0, 0, 0, e^{12}, e^{34}, -e^{15}, e^{25} + e^{36}, e^{17} + e^{24}$          | 2479     |
| 9531:210  | $0, 0, 0, 0, e^{12}, e^{34}, e^{15}, e^{13} + e^{25}, e^{36} + e^{17}$           | 2479     |
| 9531:211  | $0, 0, 0, 0, e^{12}, e^{34}, e^{15}, e^{13} + e^{25}, e^{46} + e^{17}$           | 2479     |
| 9531:212  | $0, 0, 0, 0, e^{12}, e^{34}, e^{15}, e^{13} + e^{46}, e^{25} + e^{17}$           | 2479     |
| 9531:213a | $0, 0, 0, 0, e^{12}, e^{34}, e^{15}, e^{46} + e^{23}, e^{17} + e^{25}$           | 2479     |
| 9531:213b | $0, 0, 0, 0, e^{12}, e^{34}, -e^{15}, e^{46} + e^{23}, e^{17} + e^{25}$          | 2479     |
| 9531:214a | $0, 0, 0, 0, e^{12}, e^{13}, e^{15}, e^{14} + e^{36} + e^{25}, e^{17} + e^{24}$  | 2579     |
| 9531:214b | $0, 0, 0, 0, -e^{12}, e^{13}, e^{15}, e^{25} + e^{14} + e^{36}, e^{17} + e^{24}$ | 2579     |
| 9531:215  | $0, 0, 0, 0, e^{12}, e^{13}, e^{15}, e^{35} + e^{26} + e^{14}, e^{24} + e^{17}$  | 2579     |
| 9531:216  | $0, 0, 0, 0, e^{12}, e^{13}, e^{15}, e^{25} + e^{34} + e^{16}, e^{24} + e^{17}$  | 2579     |
| 9531:217  | $0, 0, 0, 0, e^{12}, e^{13}, e^{25}, e^{36} + e^{15} + e^{24}, e^{27} + e^{14}$  | 2579     |
| 9531:218  | $0, 0, 0, 0, e^{12}, e^{13}, e^{25}, e^{16} + e^{24}, e^{14} + e^{27} + e^{36}$  | 2579     |
| 9531:219  | $0, 0, 0, 0, -e^{12}, e^{14} + e^{23}, e^{15}, e^{16} + e^{35}, e^{17}$          | 2479     |
| 9531:220  | $0, 0, 0, 0, e^{12}, e^{13} + e^{24}, e^{15}, e^{35} + e^{26}, e^{17}$           | 2479     |
| 9531:221  | $0, 0, 0, 0, e^{12}, e^{13}, e^{23} + e^{15}, e^{25}, e^{17} + e^{26}$           | 3579     |
| 9531:222a | $0, 0, 0, 0, e^{12}, e^{13}, e^{15}, e^{16}, e^{25} + e^{17} + e^{36}$           | 3579     |
| 9531:222b | $0, 0, 0, 0, -e^{12}, e^{13}, e^{15}, e^{16}, e^{17} + e^{36} + e^{25}$          | 3579     |
| 9531:223  | $0, 0, 0, 0, e^{12}, e^{13}, e^{15}, e^{16}, e^{17} + e^{26} + e^{35}$           | 3579     |
| 9531:224  | $0, 0, 0, 0, e^{12}, e^{13}, e^{25}, e^{16}, e^{36} + e^{27} + e^{15}$           | 3579     |
| 9531:225  | $0, 0, 0, 0, e^{12}, e^{13}, e^{15}, e^{35} + e^{26}, e^{25} + e^{17}$           | 3579     |
| 9531:226  | $0, 0, 0, 0, e^{12}, e^{13}, e^{25}, e^{26} + e^{35}, e^{27} + e^{15}$           | 3579     |

Table 2 – Continued to next page

Table 2 – Continued from previous page

| Name      | $\mathfrak{g}$                                                                           | UCS Dim. |
|-----------|------------------------------------------------------------------------------------------|----------|
| 9531:227a | $0, 0, 0, 0, e^{12}, e^{13}, e^{15}, e^{14} + e^{36} + e^{25}, e^{23} + e^{17}$          | 2579     |
| 9531:227b | $0, 0, 0, 0, -e^{12}, e^{13}, e^{15}, e^{25} + e^{36} + e^{14}, e^{17} + e^{23}$         | 2579     |
| 9531:228  | $0, 0, 0, 0, e^{12}, e^{13}, e^{15}, e^{14} + e^{26} + e^{35}, e^{17} + e^{23}$          | 2579     |
| 9531:229a | $0, 0, 0, 0, e^{12}, e^{13}, e^{15}, e^{16} + e^{34} + e^{25}, e^{17} + e^{23}$          | 2579     |
| 9531:229b | $0, 0, 0, 0, e^{12}, -e^{13}, e^{15}, e^{16} + e^{25} + e^{34}, e^{23} + e^{17}$         | 2579     |
| 9531:230a | $0, 0, 0, 0, e^{12}, e^{13}, e^{15}, e^{16} + e^{23}, e^{24} + e^{36} + e^{17}$          | 2579     |
| 9531:230b | $0, 0, 0, 0, -e^{12}, e^{13}, e^{15}, e^{23} + e^{16}, e^{24} + e^{17} + e^{36}$         | 2579     |
| 9531:231a | $0, 0, 0, 0, e^{12}, e^{13}, e^{25}, e^{16} + e^{23}, e^{27} + e^{36} + e^{14}$          | 2579     |
| 9531:231b | $0, 0, 0, 0, -e^{12}, e^{13}, e^{25}, e^{16} + e^{23}, e^{27} + e^{36} + e^{14}$         | 2579     |
| 9531:232  | $0, 0, 0, 0, e^{12}, e^{13}, e^{15}, e^{25} + e^{34}, e^{17} + e^{24} + e^{36}$          | 2579     |
| 9531:233  | $0, 0, 0, 0, e^{12}, e^{13}, e^{25}, e^{15} + e^{34}, e^{27} + e^{14} + e^{36}$          | 2579     |
| 9531:234  | $0, 0, 0, 0, e^{12}, e^{13}, e^{15}, e^{14} + e^{36}, e^{17} + e^{34} + e^{25}$          | 2579     |
| 9531:235  | $0, 0, 0, 0, e^{12}, e^{13}, e^{15}, e^{24} + e^{36}, e^{17} + e^{25} + e^{34}$          | 2579     |
| 9531:236  | $0, 0, 0, 0, e^{12}, e^{13}, e^{25}, e^{36} + e^{14}, e^{34} + e^{27} + e^{15}$          | 2579     |
| 9531:237  | $0, 0, 0, 0, e^{12}, e^{13}, e^{25}, e^{36} + e^{24}, e^{27} + e^{34} + e^{15}$          | 2579     |
| 9531:238  | $0, 0, 0, 0, e^{12}, e^{34}, e^{15}, e^{13} + e^{46}, e^{36} + e^{24} + e^{17}$          | 2479     |
| 9531:239a | $0, 0, 0, 0, e^{12}, e^{34}, e^{15}, e^{46} + e^{23}, e^{17} + e^{36} + e^{24}$          | 2479     |
| 9531:239b | $0, 0, 0, 0, e^{12}, e^{34}, e^{15}, -e^{23} + e^{46}, e^{17} + e^{24} + e^{36}$         | 2479     |
| 9531:240  | $0, 0, 0, 0, e^{12}, e^{34}, e^{15}, e^{36}, e^{17} + e^{25} + e^{46}$                   | 2479     |
| 9531:241  | $0, 0, 0, 0, e^{12}, -e^{13}, e^{15} + e^{34}, e^{25}, e^{46} + e^{17}$                  | 2479     |
| 9531:242  | $0, 0, 0, 0, -e^{12}, e^{13}, e^{15} + e^{24}, e^{36}, e^{17} + e^{45}$                  | 2479     |
| 9531:243  | $0, 0, 0, 0, e^{12}, e^{13}, e^{25} + e^{14}, e^{36}, e^{27} + e^{45}$                   | 2479     |
| 9531:244  | $0, 0, 0, 0, e^{12}, e^{13}, e^{14} + e^{25}, e^{15} + e^{23}, e^{27} + e^{45}$          | 3579     |
| 9531:245  | $0, 0, 0, 0, e^{12}, e^{23} + e^{14}, e^{25} + e^{13}, e^{15}, e^{35} + e^{27}$          | 3579     |
| 9531:246  | $0, 0, 0, 0, e^{12}, e^{34}, e^{13} + e^{25}, e^{15}, e^{27} + e^{35} + e^{14}$          | 3579     |
| 9531:247  | $0, 0, 0, 0, e^{12}, e^{13}, e^{15} + e^{23}, e^{16}, e^{26} + e^{34} + e^{17}$          | 2579     |
| 9531:248  | $0, 0, 0, 0, e^{12}, e^{13}, e^{15} + e^{23}, e^{16} + e^{24}, e^{17} + e^{26}$          | 2579     |
| 9531:249  | $0, 0, 0, 0, e^{12}, e^{13}, e^{15}, e^{35} + e^{26}, e^{17} + e^{24} + e^{36}$          | 2579     |
| 9531:250  | $0, 0, 0, 0, e^{12}, e^{13}, e^{25}, e^{36} + e^{15}, e^{34} + e^{27} + e^{16}$          | 2579     |
| 9531:251  | $0, 0, 0, 0, e^{12}, e^{13}, e^{25}, e^{26} + e^{35}, e^{14} + e^{27} + e^{36}$          | 2579     |
| 9531:252  | $0, 0, 0, 0, e^{12}, e^{13}, e^{25}, e^{26} + e^{35}, e^{27} + e^{16} + e^{34}$          | 2579     |
| 9531:253  | $0, 0, 0, 0, e^{12}, e^{13}, e^{25}, e^{15} + e^{24} + e^{36}, e^{27} + e^{16}$          | 2579     |
| 9531:254  | $0, 0, 0, 0, e^{12}, e^{13}, e^{25}, e^{35} + e^{26} + e^{14}, e^{27} + e^{16}$          | 2579     |
| 9531:255  | $0, 0, 0, 0, e^{12}, e^{34}, e^{15}, e^{13} + e^{25} + e^{46}, e^{36} + e^{17}$          | 2479     |
| 9531:256  | $0, 0, 0, 0, -e^{12}, e^{13}, e^{15} + e^{23}, e^{14} + e^{25}, e^{35} + e^{17}$         | 3579     |
| 9531:257a | $0, 0, 0, 0, -e^{12}, e^{13}, e^{15} + e^{24}, e^{14} + e^{25}, e^{17} + e^{45}$         | 3579     |
| 9531:257b | $0, 0, 0, 0, -e^{12}, e^{13}, e^{24} - e^{15}, e^{25} + e^{14}, e^{45} + e^{17}$         | 3579     |
| 9531:258a | $0, 0, 0, 0, e^{12}, e^{13}, e^{14} + e^{25}, e^{24} + e^{15}, e^{45} + e^{27}$          | 3579     |
| 9531:258b | $0, 0, 0, 0, -e^{12}, e^{13}, e^{25} - e^{14}, e^{24} + e^{15}, e^{27} + e^{45}$         | 3579     |
| 9531:259  | $0, 0, 0, 0, e^{12}, e^{13}, e^{15} + e^{23}, e^{25} + e^{34}, e^{17} + e^{26}$          | 2579     |
| 9531:260  | $0, 0, 0, 0, -e^{12}, e^{13}, e^{15} + e^{23}, e^{36}, e^{17} + e^{35} + e^{24}$         | 2579     |
| 9531:261  | $0, 0, 0, 0, -e^{12}, e^{13}, e^{15} + e^{23}, e^{24} + e^{16}, e^{35} + e^{17}$         | 2579     |
| 9531:262  | $0, 0, 0, 0, e^{12}, e^{13}, e^{15}, e^{36} + e^{14}, e^{17} + e^{35} + e^{26}$          | 2579     |
| 9531:263a | $0, 0, 0, 0, e^{12}, e^{13}, e^{15}, e^{16} + e^{34}, e^{17} + e^{25} + e^{36}$          | 2579     |
| 9531:263b | $0, 0, 0, 0, -e^{12}, e^{13}, e^{15}, e^{16} + e^{34}, e^{17} + e^{36} + e^{25}$         | 2579     |
| 9531:264  | $0, 0, 0, 0, e^{12}, e^{13}, e^{15}, e^{16} + e^{34}, e^{17} + e^{26} + e^{35}$          | 2579     |
| 9531:265  | $0, 0, 0, 0, e^{12}, e^{13}, e^{15}, e^{24} + e^{36}, e^{35} + e^{17} + e^{26}$          | 2579     |
| 9531:266  | $0, 0, 0, 0, e^{12}, e^{13}, e^{25}, e^{16} + e^{34}, e^{15} + e^{27} + e^{36}$          | 2579     |
| 9531:267  | $0, 0, 0, 0, e^{12}, -e^{13}, e^{15} + e^{34}, e^{16} + e^{23}, e^{17} + e^{46}$         | 2479     |
| 9531:268  | $0, 0, 0, 0, e^{12}, -e^{13}, e^{15} + e^{34}, e^{36}, e^{17} + e^{23} + e^{46}$         | 2479     |
| 9531:269a | $0, 0, 0, 0, e^{12}, -e^{13}, e^{15} + e^{34}, e^{24} + e^{16}, e^{46} + e^{17}$         | 2479     |
| 9531:269b | $0, 0, 0, 0, -e^{12}, -e^{13}, e^{34} + e^{15}, e^{16} + e^{24}, e^{17} + e^{46}$        | 2479     |
| 9531:270  | $0, 0, 0, 0, -e^{12}, e^{34}, e^{15} + e^{23}, e^{46} + e^{13}, e^{17} + e^{35}$         | 2479     |
| 9531:271  | $0, 0, 0, 0, -e^{12}, e^{34}, e^{15} + e^{23}, e^{14} + e^{36}, e^{17} + e^{35}$         | 2479     |
| 9531:272  | $0, 0, 0, 0, e^{12}, e^{34}, e^{25} + e^{13}, e^{36} + e^{14}, e^{35} + e^{27}$          | 2479     |
| 9531:273  | $0, 0, 0, 0, e^{12}, e^{14} + e^{23}, e^{13} + e^{25}, e^{34} + e^{15}, e^{27} + e^{35}$ | 3579     |
| 9531:274a | $0, 0, 0, 0, e^{12}, e^{13}, e^{23} + e^{15}, e^{36} + e^{25}, e^{17} + e^{26}$          | 3579     |
| 9531:274b | $0, 0, 0, 0, -e^{12}, e^{13}, e^{15} + e^{23}, e^{36} + e^{25}, e^{17} + e^{26}$         | 3579     |

Table 2 – Continued to next page



Table 2 – Continued from previous page

| Name      | $\mathfrak{g}$                                                                                | UCS Dim. |
|-----------|-----------------------------------------------------------------------------------------------|----------|
| 9531:275  | $0, 0, 0, 0, e^{12}, e^{13}, e^{15} + e^{23}, e^{14} + e^{36}, e^{17} + e^{34} + e^{26}$      | 2579     |
| 9531:276a | $0, 0, 0, 0, e^{12}, e^{13}, e^{15} + e^{23}, e^{24} + e^{36}, e^{26} + e^{34} + e^{17}$      | 2579     |
| 9531:276b | $0, 0, 0, 0, e^{12}, e^{13}, e^{15} + e^{23}, e^{36} - e^{24}, e^{26} + e^{34} + e^{17}$      | 2579     |
| 9531:277  | $0, 0, 0, 0, e^{12}(-1 + a_2), a_2 e^{13}, e^{15} + e^{23}, e^{36}, e^{17} + e^{26} + e^{35}$ | 3579     |
| 9531:278a | $0, 0, 0, 0, -e^{12}, e^{13}, e^{15} + e^{23}, e^{25} + e^{36}, e^{17} + e^{35}$              | 3579     |
| 9531:278b | $0, 0, 0, 0, -e^{12}, -e^{13}, e^{15} + e^{23}, e^{25} + e^{36}, e^{17} + e^{35}$             | 3579     |
| 9531:279  | $0, 0, 0, 0, -e^{12}, e^{34}, e^{15} + e^{23}, e^{36}, e^{17} + e^{46} + e^{35}$              | 2479     |
| 9531:280a | $0, 0, 0, 0, e^{12}, -e^{13}, e^{15} + e^{34}, e^{36} + e^{25}, e^{46} + e^{17}$              | 2479     |
| 9531:280b | $0, 0, 0, 0, -e^{12}, -e^{13}, e^{34} + e^{15}, e^{36} + e^{25}, e^{17} + e^{46}$             | 2479     |
| 9531:281  | $0, 0, 0, 0, -e^{12}, -e^{13}, e^{34} + e^{15}, e^{35} + e^{26}, e^{46} + e^{17}$             | 2479     |
| 9531:282  | $0, 0, 0, 0, e^{12}, e^{34}, e^{15}, e^{25}, e^{46} + e^{23} + e^{17}$                        | 2479     |
| 9531:283  | $0, 0, 0, 0, e^{12}, e^{13}, e^{15}, e^{14} + e^{25}, e^{24} + e^{36} + e^{17}$               | 2579     |
| 9531:284a | $0, 0, 0, 0, e^{12}, e^{13}, e^{25}, e^{24} + e^{15}, e^{36} + e^{27} + e^{14}$               | 2579     |
| 9531:284b | $0, 0, 0, 0, -e^{12}, e^{13}, e^{25}, e^{15} + e^{24}, e^{14} + e^{27} + e^{36}$              | 2579     |
| 9531:285  | $0, 0, 0, 0, a_1 e^{12}, e^{13}, e^{25}, e^{24} + e^{15}, e^{16} + e^{27} + e^{34}$           | 2579     |
| 9531:286  | $0, 0, 0, 0, e^{12}, e^{13}, e^{15}, e^{16} + e^{24}, e^{17} + e^{25} + e^{34}$               | 2579     |
| 9531:287a | $0, 0, 0, 0, e^{12}, e^{13}, e^{25}, e^{16} + e^{24}, e^{34} + e^{27} + e^{15}$               | 2579     |
| 9531:287b | $0, 0, 0, 0, -e^{12}, e^{13}, e^{25}, e^{16} + e^{24}, e^{15} + e^{34} + e^{27}$              | 2579     |
| 9531:288  | $0, 0, 0, 0, e^{12}, e^{13}, e^{15}, e^{25}, e^{35} + e^{17} + e^{26}$                        | 3579     |
| 9531:289  | $0, 0, 0, 0, e^{12}, e^{13}, e^{25}, e^{15} + e^{23}, e^{27} + e^{36} + e^{14}$               | 2579     |
| 9531:290  | $0, 0, 0, 0, e^{12}, e^{13}, e^{25}, e^{15} + e^{23}, e^{27} + e^{34} + e^{16}$               | 2579     |
| 9531:291  | $0, 0, 0, 0, e^{12}, e^{13}, a_1, e^{15}, e^{16} + e^{23}, e^{17} + e^{25} + e^{34}$          | 2579     |
| 9531:292  | $0, 0, 0, 0, e^{12}, e^{13}, e^{25}, e^{23} + e^{16}, e^{34} + e^{27} + e^{15}$               | 2579     |
| 9531:293a | $0, 0, 0, 0, e^{12}, e^{34}, e^{15}, e^{13} + e^{46} + e^{25}, e^{17} + e^{23}$               | 2479     |
| 9531:293b | $0, 0, 0, 0, e^{12}, e^{34}, -e^{15}, e^{13} + e^{46} + e^{25}, e^{23} + e^{17}$              | 2479     |
| 9531:294  | $0, 0, 0, 0, e^{12}, e^{34}, e^{15}, e^{36} + e^{25} + e^{14}, e^{17} + e^{23}$               | 2479     |
| 9531:295  | $0, 0, 0, 0, -e^{12}, e^{13}, e^{24} + e^{15}, e^{16}, e^{17} + e^{45}$                       | 2479     |
| 9531:296  | $0, 0, 0, 0, e^{12}, e^{13}, e^{25} + e^{14}, e^{16}, e^{27} + e^{45}$                        | 2479     |
| 9531:297  | $0, 0, 0, 0, -e^{12}, e^{13}, e^{15} + e^{24}, e^{25}, e^{17} + e^{23} + e^{45}$              | 3579     |
| 9531:298  | $0, 0, 0, 0, e^{12}, e^{13}, e^{15}, e^{16} + e^{25}, e^{24} + e^{36} + e^{17}$               | 2579     |
| 9531:299a | $0, 0, 0, 0, -e^{12}, e^{14} + e^{23}, e^{15}, e^{35} + e^{16}, e^{17} + e^{34}$              | 2479     |
| 9531:299b | $0, 0, 0, 0, -e^{12}, e^{23} - e^{14}, e^{15}, e^{16} + e^{35}, e^{34} + e^{17}$              | 2479     |
| 9531:300a | $0, 0, 0, 0, e^{12}, e^{24} + e^{13}, e^{15}, e^{26} + e^{35}, e^{17} + e^{34}$               | 2479     |
| 9531:300b | $0, 0, 0, 0, e^{12}, e^{24} + e^{13}, -e^{15}, e^{35} + e^{26}, e^{34} + e^{17}$              | 2479     |
| 9531:301  | $0, 0, 0, 0, e^{12}, e^{24} + e^{13}, e^{15}, e^{26} + e^{35} + e^{14}, e^{17}$               | 2479     |
| 9531:302  | $0, 0, 0, 0, -e^{12}, e^{24} + e^{13}, e^{15}, e^{16} + e^{45} + e^{23}, e^{17}$              | 2479     |
| 9531:303  | $0, 0, 0, 0, e^{12}, e^{34}, e^{15}, e^{36} + e^{25}, e^{17} + e^{23} + e^{46}$               | 2479     |
| 9531:304  | $0, 0, 0, 0, -e^{12}, e^{13}, e^{23} + e^{15}, e^{25}, e^{35} + e^{24} + e^{17}$              | 3579     |
| 9531:305a | $0, 0, 0, 0, e^{12}, a_1 e^{13}, e^{15}, e^{23} + e^{16}, e^{36} + e^{17} + e^{25}$           | 3579     |
| 9531:305b | $0, 0, 0, 0, -e^{12}, a_1 e^{13}, e^{15}, e^{23} + e^{16}, e^{17} + e^{36} + e^{25}$          | 3579     |
| 9531:306  | $0, 0, 0, 0, e^{12}, e^{13}, e^{15}, e^{16} + e^{23}, e^{17} + e^{26} + e^{35}$               | 3579     |
| 9531:307a | $0, 0, 0, 0, e^{12}, e^{13}, e^{25}, e^{23} + e^{16}, e^{27} + e^{15} + e^{36}$               | 3579     |
| 9531:307b | $0, 0, 0, 0, -e^{12}, e^{13}, e^{25}, e^{16} + e^{23}, e^{15} + e^{27} + e^{36}$              | 3579     |
| 9531:308  | $0, 0, 0, 0, e^{12}, e^{13}, e^{23} + e^{15}, e^{25}, e^{17} + e^{26} + e^{34}$               | 2579     |
| 9531:309  | $0, 0, 0, 0, e^{12}, e^{13}, e^{15} + e^{23}, e^{25} + e^{14}, e^{26} + e^{17}$               | 2579     |
| 9531:310  | $0, 0, 0, 0, -e^{12}, e^{13}, e^{15} + e^{23}, e^{16}, e^{17} + e^{24} + e^{35}$              | 2579     |
| 9531:311a | $0, 0, 0, 0, e^{12}, e^{13}, e^{15}, e^{16} + e^{24}, e^{17} + e^{25} + e^{36}$               | 2579     |
| 9531:311b | $0, 0, 0, 0, -e^{12}, e^{13}, e^{15}, e^{24} + e^{16}, e^{25} + e^{36} + e^{17}$              | 2579     |
| 9531:312  | $0, 0, 0, 0, e^{12}, e^{13}, e^{15}, e^{24} + e^{16}, e^{35} + e^{17} + e^{26}$               | 2579     |
| 9531:313  | $0, 0, 0, 0, e^{12}, e^{13}, e^{25}, e^{16} + e^{24}, e^{27} + e^{36} + e^{15}$               | 2579     |
| 9531:314  | $0, 0, 0, 0, e^{12}, e^{13}, e^{15}, e^{26} + e^{35}, e^{34} + e^{17} + e^{25}$               | 2579     |
| 9531:315  | $0, 0, 0, 0, e^{12}, e^{13}, e^{25}, e^{26} + e^{35}, e^{15} + e^{34} + e^{27}$               | 2579     |
| 9531:316  | $0, 0, 0, 0, e^{12}, e^{13}, e^{15}, e^{35} + e^{26} + e^{14}, e^{25} + e^{17}$               | 2579     |
| 9531:317  | $0, 0, 0, 0, e^{12}, e^{13}, e^{25}, e^{26} + e^{35} + e^{14}, e^{27} + e^{15}$               | 2579     |
| 9531:318  | $0, 0, 0, 0, e^{12}, -e^{13}, e^{15} + e^{34}, e^{16}, e^{17} + e^{46} + e^{23}$              | 2479     |
| 9531:319  | $0, 0, 0, 0, e^{12}, e^{34}, e^{15}, e^{46} + e^{13}, e^{17} + e^{36} + e^{25}$               | 2479     |
| 9531:320a | $0, 0, 0, 0, e^{12}, e^{34}, e^{15}, e^{46} + e^{23}, e^{36} + e^{17} + e^{25}$               | 2479     |
| 9531:320b | $0, 0, 0, 0, e^{12}, e^{34}, -e^{15}, e^{46} + e^{23}, e^{25} + e^{36} + e^{17}$              | 2479     |

Table 2 – Continued to next page

Table 2 – Continued from previous page

| Name      | $\mathfrak{g}$                                                                                          | UCS Dim. |
|-----------|---------------------------------------------------------------------------------------------------------|----------|
| 9531:321  | $0, 0, 0, 0, e^{12}, e^{13}, e^{15}, e^{25} + e^{34}, e^{35} + e^{17} + e^{26}$                         | 2579     |
| 9531:322  | $0, 0, 0, 0, e^{12}, -e^{13}, e^{15} + e^{34}, e^{14} + e^{25}, e^{46} + e^{17}$                        | 2479     |
| 9531:323  | $0, 0, 0, 0, e^{12}, e^{34}, e^{25} + e^{13}, e^{36}, e^{27} + e^{35} + e^{14}$                         | 2479     |
| 9531:324  | $0, 0, 0, 0, e^{12}, e^{34}, e^{13} + e^{25}, e^{46}, e^{35} + e^{27} + e^{14}$                         | 2479     |
| 9531:325a | $0, 0, 0, 0, -e^{12}, e^{13}, e^{24} + e^{15}, e^{25} + e^{34}, e^{45} + e^{17} + e^{23}$               | 3579     |
| 9531:325b | $0, 0, 0, 0, -e^{12}, e^{13}, e^{24} + e^{15}, e^{34} - e^{25}, e^{17} + e^{45} + e^{23}$               | 3579     |
| 9531:326  | $0, 0, 0, 0, -e^{12}, e^{24} + e^{13}, e^{15} + e^{23}, e^{14} + e^{25}, e^{17} + e^{35}$               | 3579     |
| 9531:327  | $0, 0, 0, 0, -e^{12}, e^{34}, e^{15} + e^{23}, e^{14} + e^{25}, e^{17} + e^{35} + e^{24}$               | 3579     |
| 9531:328  | $0, 0, 0, 0, e^{12}, e^{13}, e^{23} + e^{15}, e^{16} + e^{25}, e^{17} + e^{26}$                         | 3579     |
| 9531:329  | $0, 0, 0, 0, e^{12}, e^{13}, e^{15} + e^{23}, e^{16} + e^{24}, e^{17} + e^{34} + e^{26}$                | 2579     |
| 9531:330  | $0, 0, 0, 0, e^{12}, e^{13}, e^{15}, e^{26} + e^{35} + e^{14}, e^{17} + e^{36} + e^{24}$                | 2579     |
| 9531:331  | $0, 0, 0, 0, e^{12}, e^{13}, e^{15}, e^{25} + e^{16} + e^{34}, e^{17} + e^{24} + e^{36}$                | 2579     |
| 9531:332  | $0, 0, 0, 0, e^{12}, a_1, e^{13}, e^{25}, e^{24} + e^{36} + e^{15}, e^{34} + e^{27} + e^{16}$           | 2579     |
| 9531:333  | $0, 0, 0, 0, e^{12}, e^{13}, e^{25}, e^{26} + e^{35} + e^{14}, e^{34} + e^{27} + e^{16}$                | 2579     |
| 9531:334a | $0, 0, 0, 0, -e^{12}, e^{13}, e^{15} + e^{24}, e^{36} + e^{14}, e^{17} + e^{45}$                        | 2479     |
| 9531:334b | $0, 0, 0, 0, -e^{12}, -e^{13}, e^{15} + e^{24}, e^{36} + e^{14}, e^{45} + e^{17}$                       | 2479     |
| 9531:335  | $0, 0, 0, 0, -e^{12}, a_2, e^{13}, e^{24} + e^{15}, e^{16} + e^{34}, e^{45} + e^{17}$                   | 2479     |
| 9531:336a | $0, 0, 0, 0, e^{12}, e^{13}, e^{14} + e^{25}, e^{34} + e^{16}, e^{27} + e^{45}$                         | 2479     |
| 9531:336b | $0, 0, 0, 0, e^{12}, -e^{13}, e^{14} + e^{25}, e^{16} + e^{34}, e^{45} + e^{27}$                        | 2479     |
| 9531:337  | $0, 0, 0, 0, e^{12}, e^{13}, e^{14} + e^{25}, e^{24} + e^{36}, e^{27} + e^{45}$                         | 2479     |
| 9531:338a | $0, 0, 0, 0, -e^{12}, e^{13}, e^{15} + e^{23}, e^{25} + e^{34}, e^{24} + e^{17} + e^{35}$               | 3579     |
| 9531:338b | $0, 0, 0, 0, -e^{12}, e^{13}, e^{15} + e^{23}, -e^{25} + e^{34}, e^{17} + e^{35} + e^{24}$              | 3579     |
| 9531:339a | $0, 0, 0, 0, -e^{12}, e^{34}, e^{15} + e^{23}, e^{13} + e^{25}, e^{17} + e^{24} + e^{35}$               | 3579     |
| 9531:339b | $0, 0, 0, 0, -e^{12}, e^{34}, e^{23} - e^{15}, e^{13} + e^{25}, e^{35} + e^{24} + e^{17}$               | 3579     |
| 9531:340  | $0, 0, 0, 0, e^{12}, a_1, e^{13}(1 + a_1), e^{15} + e^{23}, e^{16}, e^{26} + e^{35} + e^{17}$           | 3579     |
| 9531:341  | $0, 0, 0, 0, -e^{12}, e^{13}, e^{15} + e^{23}, e^{25} + e^{16}, e^{35} + e^{17}$                        | 3579     |
| 9531:342a | $0, 0, 0, 0, e^{12}, e^{13}, e^{15}, e^{25} + e^{36}, e^{35} + e^{26} + e^{17}$                         | 3579     |
| 9531:342b | $0, 0, 0, 0, e^{12}, e^{13}, e^{15}, e^{36} - e^{25}, e^{26} + e^{35} + e^{17}$                         | 3579     |
| 9531:343a | $0, 0, 0, 0, e^{12}, e^{13}, e^{15}, e^{26} + e^{35}, e^{17} + e^{36} + e^{25}$                         | 3579     |
| 9531:343b | $0, 0, 0, 0, -e^{12}, e^{13}, e^{15}, e^{35} - e^{26}, e^{36} + e^{17} + e^{25}$                        | 3579     |
| 9531:344  | $0, 0, 0, 0, e^{12}, e^{13}, e^{25}, e^{35} + e^{26}, e^{27} + e^{36} + e^{15}$                         | 3579     |
| 9531:345  | $0, 0, 0, 0, -e^{12}, e^{13}, e^{15} + e^{23}, e^{36} + e^{14}, e^{17} + e^{35} + e^{24}$               | 2579     |
| 9531:346  | $0, 0, 0, 0, -e^{12}, e^{13}, e^{15} + e^{23}, e^{16} + e^{34}, e^{17} + e^{35} + e^{24}$               | 2579     |
| 9531:347  | $0, 0, 0, 0, e^{12}, e^{14} + e^{23}, e^{15} + e^{34}, e^{25}, e^{17} + e^{36}$                         | 2479     |
| 9531:348  | $0, 0, 0, 0, e^{12}, -e^{13}, e^{15} + e^{34}, e^{16} + e^{25}, e^{46} + e^{17}$                        | 2479     |
| 9531:349  | $0, 0, 0, 0, e^{12}, -e^{13}, e^{15} + e^{34}, e^{14} + e^{36}, e^{23} + e^{17} + e^{46}$               | 2479     |
| 9531:350a | $0, 0, 0, 0, e^{12}, -e^{13}, e^{15} + e^{34}, e^{36} + e^{24}, e^{17} + e^{46} + e^{23}$               | 2479     |
| 9531:350b | $0, 0, 0, 0, e^{12}, -e^{13}, e^{15} + e^{34}, -e^{24} + e^{36}, e^{17} + e^{23} + e^{46}$              | 2479     |
| 9531:351  | $0, 0, 0, 0, e^{12}, -e^{13}, e^{15} + e^{34}, e^{36}, e^{46} + e^{17} + e^{25}$                        | 2479     |
| 9531:352  | $0, 0, 0, 0, e^{12}, e^{34}, e^{13} + e^{25}, e^{36} + e^{15}, e^{27} + e^{35}$                         | 2479     |
| 9531:353  | $0, 0, 0, 0, e^{12}, e^{34}, e^{13} + e^{25}, e^{15} + e^{46}, e^{27} + e^{35}$                         | 2479     |
| 9531:354a | $0, 0, 0, 0, e^{12}, e^{13}, e^{15} + e^{23}, e^{36} + e^{25}, e^{17} + e^{26} + e^{34}$                | 2579     |
| 9531:354b | $0, 0, 0, 0, -e^{12}, e^{13}, e^{23} + e^{15}, e^{25} + e^{36}, e^{34} + e^{26} + e^{17}$               | 2579     |
| 9531:355a | $0, 0, 0, 0, e^{12}, e^{13}, e^{15} + e^{23}, e^{36} + e^{25} + e^{14}, e^{26} + e^{17}$                | 2579     |
| 9531:355b | $0, 0, 0, 0, -e^{12}, e^{13}, e^{23} + e^{15}, e^{36} + e^{25} + e^{14}, e^{17} + e^{26}$               | 2579     |
| 9531:356  | $0, 0, 0, 0, e^{12}, e^{13}, e^{15} + e^{23}, e^{16} + e^{25} + e^{34}, e^{17} + e^{26}$                | 2579     |
| 9531:357  | $0, 0, 0, 0, e^{12}, a_1, (1 + a_1)e^{13}, e^{23} + e^{15}, e^{36} + e^{14}, e^{35} + e^{26} + e^{17}$  | 2579     |
| 9531:358  | $0, 0, 0, 0, (-1 + a_2)e^{12}, a_2, e^{13}, e^{15} + e^{23}, e^{34} + e^{16}, e^{26} + e^{35} + e^{17}$ | 2579     |
| 9531:359  | $0, 0, 0, 0, e^{12}, a_1, e^{13}(1 + a_1), e^{15} + e^{23}, e^{24} + e^{36}, e^{17} + e^{35} + e^{26}$  | 2579     |
| 9531:360a | $0, 0, 0, 0, -e^{12}, e^{13}, e^{15} + e^{23}, e^{25} + e^{36} + e^{14}, e^{17} + e^{35}$               | 2579     |
| 9531:360b | $0, 0, 0, 0, -e^{12}, -e^{13}, e^{15} + e^{23}, e^{25} + e^{14} + e^{36}, e^{17} + e^{35}$              | 2579     |
| 9531:361  | $0, 0, 0, 0, -e^{12}, e^{13}, e^{23} + e^{15}, e^{16} + e^{25} + e^{34}, e^{35} + e^{17}$               | 2579     |
| 9531:362  | $0, 0, 0, 0, -e^{12}, e^{34}, e^{15} + e^{23}, e^{36} + e^{14}, e^{17} + e^{46} + e^{35}$               | 2479     |
| 9531:363  | $0, 0, 0, 0, e^{12}, e^{34}, e^{13} + e^{25}, e^{14} + e^{36}, e^{27} + e^{46} + e^{35}$                | 2479     |
| 9531:364a | $0, 0, 0, 0, e^{12}, -e^{13}, e^{34} + e^{15}, e^{36} + e^{25} + e^{14}, e^{46} + e^{17}$               | 2479     |
| 9531:364b | $0, 0, 0, 0, -e^{12}, -e^{13}, e^{15} + e^{34}, e^{36} + e^{14} + e^{25}, e^{46} + e^{17}$              | 2479     |
| 9531:365a | $0, 0, 0, 0, -e^{12}, -e^{13}, e^{15} + e^{34}, e^{26} + e^{35} + e^{14}, e^{17} + e^{46}$              | 2479     |
| 9531:365b | $0, 0, 0, 0, -e^{12}, -e^{13}, -e^{15} + e^{34}, e^{35} + e^{14} + e^{26}, e^{46} + e^{17}$             | 2479     |

Table 2 – Continued to next page

Table 2 – Continued from previous page

| Name      | $\mathfrak{g}$                                                                                        | UCS Dim. |
|-----------|-------------------------------------------------------------------------------------------------------|----------|
| 9531:366  | $0, 0, 0, 0, -e^{12}, e^{14} + e^{23}, e^{34} + e^{15}, e^{35} + e^{16}, e^{17} + e^{36}$             | 2479     |
| 9531:367  | $0, 0, 0, 0, -e^{12}, e^{24} - e^{13}, e^{15} + e^{34}, e^{35} + e^{26}, e^{46} + e^{17}$             | 2479     |
| 9531:368  | $0, 0, 0, 0, e^{12}, e^{34}, e^{15}, e^{13} + e^{25}, e^{46} + e^{17} + e^{23}$                       | 2479     |
| 9531:369  | $0, 0, 0, 0, e^{12}, e^{34}, e^{15}, e^{13} + e^{25}, e^{24} + e^{17} + e^{36}$                       | 2479     |
| 9531:370  | $0, 0, 0, 0, e^{12}, e^{24} + e^{13}, e^{15}, e^{26} + e^{35}, e^{17} + e^{23}$                       | 2479     |
| 9531:371  | $0, 0, 0, 0, -e^{12}, e^{14} + e^{23}, e^{15}, e^{16} + e^{35}, e^{17} + e^{24}$                      | 2479     |
| 9531:372  | $0, 0, 0, 0, e^{12}, e^{13}, e^{15}, e^{14} + e^{25}, e^{17} + e^{35} + e^{26}$                       | 2579     |
| 9531:373  | $0, 0, 0, 0, e^{12}, -e^{13}, e^{34} + e^{15}, e^{25}, e^{17} + e^{46} + e^{23}$                      | 2479     |
| 9531:374  | $0, 0, 0, 0, -e^{12}, e^{13}, e^{15} + e^{24}, e^{16} + e^{23}, e^{17} + e^{45}$                      | 2479     |
| 9531:375  | $0, 0, 0, 0, e^{12}, e^{13}, e^{14} + e^{25}, e^{16} + e^{23}, e^{27} + e^{45}$                       | 2479     |
| 9531:376  | $0, 0, 0, 0, -e^{12}, e^{13}, e^{24} + e^{15}, e^{36}, e^{23} + e^{45} + e^{17}$                      | 2479     |
| 9531:377  | $0, 0, 0, 0, e^{12}, e^{13}, e^{25} + e^{14}, e^{24} + e^{16}, e^{45} + e^{27}$                       | 2479     |
| 9531:378  | $0, 0, 0, 0, -e^{12}, e^{13}, e^{15} + e^{23}, e^{25} + e^{14}, e^{17} + e^{35} + e^{24}$             | 3579     |
| 9531:379a | $0, 0, 0, 0, -e^{12}, e^{13}, e^{15} + e^{24}, e^{25} + e^{14}, e^{45} + e^{17} + e^{23}$             | 3579     |
| 9531:379b | $0, 0, 0, 0, -e^{12}, e^{13}, e^{24} - e^{15}, e^{14} + e^{25}, e^{23} + e^{45} + e^{17}$             | 3579     |
| 9531:380  | $0, 0, 0, 0, e^{12}, e^{13}, e^{15}, e^{25} + e^{16}, e^{26} + e^{35} + e^{17}$                       | 3579     |
| 9531:381  | $0, 0, 0, 0, e^{12}, e^{13}, e^{15} + e^{23}, e^{14} + e^{25}, e^{26} + e^{34} + e^{17}$              | 2579     |
| 9531:382  | $0, 0, 0, 0, e^{12}, e^{13}, e^{15}, e^{14} + e^{26} + e^{35}, e^{17} + e^{25} + e^{34}$              | 2579     |
| 9531:383a | $0, 0, 0, 0, e^{12}, e^{13}, e^{25}, e^{14} + e^{35} + e^{26}, e^{15} + e^{34} + e^{27}$              | 2579     |
| 9531:383b | $0, 0, 0, 0, e^{12}, e^{13}, e^{25}, e^{26} + e^{35} - e^{14}, e^{34} + e^{27} + e^{15}$              | 2579     |
| 9531:384a | $0, 0, 0, 0, e^{12}, e^{24} + e^{13}, e^{15}, e^{26} + e^{35} + e^{14}, e^{17} + e^{34}$              | 2479     |
| 9531:384b | $0, 0, 0, 0, e^{12}, e^{24} + e^{13}, -e^{15}, e^{14} + e^{26} + e^{35}, e^{17} + e^{34}$             | 2479     |
| 9531:385a | $0, 0, 0, 0, -e^{12}, e^{24} + e^{13}, e^{15}, e^{23} + e^{45} + e^{16}, e^{17} + e^{34}$             | 2479     |
| 9531:385b | $0, 0, 0, 0, -e^{12}, -e^{13} + e^{24}, e^{15}, e^{45} + e^{23} + e^{16}, e^{17} + e^{34}$            | 2479     |
| 9531:386  | $0, 0, 0, 0, e^{12}, e^{34}, e^{15}, e^{14} + e^{36} + e^{25}, e^{46} + e^{23} + e^{17}$              | 2479     |
| 9531:387  | $0, 0, 0, 0, (-1 + a_2)e^{12}, a_2e^{13}, e^{15} + e^{23}, e^{25}, e^{17} + e^{26} + e^{35}$          | 3579     |
| 9531:388a | $0, 0, 0, 0, e^{12}, -e^{13}, e^{34} + e^{15}, e^{24} + e^{16}, e^{46} + e^{17} + e^{23}$             | 2479     |
| 9531:388b | $0, 0, 0, 0, -e^{12}, -e^{13}, e^{34} + e^{15}, e^{16} + e^{24}, e^{17} + e^{46} + e^{23}$            | 2479     |
| 9531:389  | $0, 0, 0, 0, e^{12}, -e^{13}, e^{15} + e^{34}, e^{16}, e^{46} + e^{17} + e^{25}$                      | 2479     |
| 9531:390  | $0, 0, 0, 0, -e^{12}, e^{34}, e^{15} + e^{23}, e^{13} + e^{46}, e^{17} + e^{35} + e^{24}$             | 2479     |
| 9531:391  | $0, 0, 0, 0, -e^{12}, e^{34}, e^{15} + e^{23}, e^{36} + e^{14}, e^{24} + e^{35} + e^{17}$             | 2479     |
| 9531:392  | $0, 0, 0, 0, -e^{12}, e^{13}, e^{15} + e^{24}, e^{16}, e^{36} + e^{45} + e^{17}$                      | 2479     |
| 9531:393  | $0, 0, 0, 0, e^{12}, e^{13}, e^{25} + e^{14}, e^{16}, e^{27} + e^{36} + e^{45}$                       | 2479     |
| 9531:394  | $0, 0, 0, 0, e^{12}, e^{13}, e^{25} + e^{14}, e^{36}, e^{27} + e^{16} + e^{45}$                       | 2479     |
| 9531:395  | $0, 0, 0, 0, e^{12}, e^{34}, e^{13} + e^{25}, e^{15}, e^{35} + e^{46} + e^{27}$                       | 2479     |
| 9531:396  | $0, 0, 0, 0, e^{12}, e^{13}, e^{25} + e^{14}, e^{15} + e^{36}, e^{45} + e^{27}$                       | 2479     |
| 9531:397a | $0, 0, 0, 0, -e^{12}, e^{13}, e^{15} + e^{24}, e^{36} + e^{25}, e^{45} + e^{17}$                      | 2479     |
| 9531:397b | $0, 0, 0, 0, -e^{12}, -e^{13}, e^{15} + e^{24}, e^{25} + e^{36}, e^{17} + e^{45}$                     | 2479     |
| 9531:398  | $0, 0, 0, 0, -e^{12}, -e^{13}, e^{15} + e^{24}, e^{26} + e^{35}, e^{45} + e^{17}$                     | 2479     |
| 9531:399  | $0, 0, 0, 0, e^{12}, e^{13}, e^{25} + e^{14}, e^{26} + e^{35}, e^{27} + e^{45}$                       | 2479     |
| 9531:400  | $0, 0, 0, 0, e^{12}, e^{13}, e^{23} + e^{15}, e^{16} + e^{25}, e^{17} + e^{26} + e^{34}$              | 2579     |
| 9531:401  | $0, 0, 0, 0, e^{12}a_1, (1 + a_1)e^{13}, e^{15} + e^{23}, e^{16} + e^{24}, e^{26} + e^{17} + e^{35}$  | 2579     |
| 9531:402a | $0, 0, 0, 0, -e^{12}, e^{13}, e^{23} + e^{15}, e^{25} + e^{36}, e^{35} + e^{24} + e^{17}$             | 2579     |
| 9531:402b | $0, 0, 0, 0, -e^{12}, -e^{13}, e^{15} + e^{23}, e^{36} + e^{25}, e^{24} + e^{35} + e^{17}$            | 2579     |
| 9531:403a | $0, 0, 0, 0, e^{12}, e^{13}, e^{15}, e^{35} + e^{14} + e^{26}, e^{17} + e^{36} + e^{25}$              | 2579     |
| 9531:403b | $0, 0, 0, 0, -e^{12}, e^{13}, e^{15}, e^{14} - e^{26} + e^{35}, e^{17} + e^{36} + e^{25}$             | 2579     |
| 9531:404a | $0, 0, 0, 0, e^{12}, e^{13}, e^{15}, e^{25} + e^{14} + e^{36}, e^{17} + e^{26} + e^{35}$              | 2579     |
| 9531:404b | $0, 0, 0, 0, e^{12}, e^{13}, e^{15}, e^{36} + e^{14} - e^{25}, e^{35} + e^{17} + e^{26}$              | 2579     |
| 9531:405  | $0, 0, 0, 0, e^{12}, e^{13}, e^{15}, e^{25} + e^{16} + e^{34}, e^{26} + e^{17} + e^{35}$              | 2579     |
| 9531:406  | $0, 0, 0, 0, e^{12}, e^{13}, e^{25}, e^{26} + e^{35} + e^{14}, e^{15} + e^{27} + e^{36}$              | 2579     |
| 9531:407  | $0, 0, 0, 0, e^{12}, e^{14} + e^{23}, e^{15} + e^{34}, e^{13} + e^{25}, e^{17} + e^{36}$              | 2479     |
| 9531:408a | $0, 0, 0, 0, e^{12}, -e^{13}, e^{34} + e^{15}, e^{36} + e^{25}, e^{17} + e^{23} + e^{46}$             | 2479     |
| 9531:408b | $0, 0, 0, 0, -e^{12}, -e^{13}, e^{15} + e^{34}, e^{36} + e^{25}, e^{46} + e^{23} + e^{17}$            | 2479     |
| 9531:409  | $0, 0, 0, 0, -e^{12}, -e^{13}, e^{34} + e^{15}, e^{35} + e^{26}, e^{46} + e^{23} + e^{17}$            | 2479     |
| 9531:410  | $0, 0, 0, 0, (-1 + a_2)e^{12}, e^{13}a_2, e^{23} + e^{15}, e^{25} + e^{34}, e^{35} + e^{17} + e^{26}$ | 2579     |
| 9531:411  | $0, 0, 0, 0, e^{12}, -e^{13}, e^{15} + e^{34}, e^{14} + e^{36}, e^{46} + e^{17} + e^{25}$             | 2479     |
| 9531:412  | $0, 0, 0, 0, e^{12}, -e^{13}, e^{15} + e^{34}, e^{24} + e^{36}, e^{17} + e^{46} + e^{25}$             | 2479     |
| 9531:413a | $0, 0, 0, 0, -e^{12}, e^{34}, e^{15} + e^{23}, e^{13} + e^{25} + e^{46}, e^{35} + e^{17}$             | 2479     |

Table 2 – Continued to next page

Table 2 – Continued from previous page

| Name      | $\mathfrak{g}$                                                                                         | UCS Dim. |
|-----------|--------------------------------------------------------------------------------------------------------|----------|
| 9531:413b | $0, 0, 0, 0, -e^{12}, e^{34}, -e^{15} + e^{23}, e^{13} + e^{46} + e^{25}, e^{35} + e^{17}$             | 2479     |
| 9531:414  | $0, 0, 0, 0, -e^{12}, e^{34}, e^{15} + e^{23}, e^{14} + e^{36} + e^{25}, e^{17} + e^{35}$              | 2479     |
| 9531:415a | $0, 0, 0, 0, e^{12}, e^{13}, e^{15} + e^{23}, e^{36} + e^{25} + e^{14}, e^{34} + e^{17} + e^{26}$      | 2579     |
| 9531:415b | $0, 0, 0, 0, -e^{12}, e^{13}, e^{23} + e^{15}, e^{36} + e^{14} + e^{25}, e^{17} + e^{26} + e^{34}$     | 2579     |
| 9531:416  | $0, 0, 0, 0, -e^{12}, a_2 e^{13}, e^{24} + e^{15}, e^{16} + e^{34}, e^{17} + e^{36} + e^{45}$          | 2479     |
| 9531:417a | $0, 0, 0, 0, e^{12}, e^{13}, e^{25} + e^{14}, e^{16} + e^{34}, e^{27} + e^{45} + e^{36}$               | 2479     |
| 9531:417b | $0, 0, 0, 0, e^{12}, -e^{13}, e^{14} + e^{25}, e^{16} + e^{34}, e^{36} + e^{45} + e^{27}$              | 2479     |
| 9531:418a | $0, 0, 0, 0, e^{12} a_1, e^{13}(1 + a_1), e^{15} + e^{23}, e^{36} + e^{25}, e^{17} + e^{35} + e^{26}$  | 3579     |
| 9531:418b | $0, 0, 0, 0, e^{12} a_1, e^{13}(1 + a_1), e^{15} + e^{23}, -e^{25} + e^{36}, e^{17} + e^{26} + e^{35}$ | 3579     |
| 9531:419  | $0, 0, 0, 0, e^{12}, e^{34}, e^{13} + e^{25}, e^{15} + e^{36}, e^{46} + e^{27} + e^{35}$               | 2479     |
| 9531:420a | $0, 0, 0, 0, e^{12}, e^{23} + e^{14}, e^{15} + e^{34}, e^{26} + e^{45} + e^{13}, e^{17} + e^{36}$      | 2479     |
| 9531:420b | $0, 0, 0, 0, e^{12}, e^{23} + e^{14}, -e^{15} + e^{34}, e^{13} + e^{45} + e^{26}, e^{36} + e^{17}$     | 2479     |
| 9531:421  | $0, 0, 0, 0, -e^{12}, e^{14} + e^{23}, e^{15} + e^{34}, e^{16} + e^{24} + e^{35}, e^{17} + e^{36}$     | 2479     |
| 9531:422  | $0, 0, 0, 0, -e^{12}, e^{13}, e^{24} + e^{15}, e^{16}, e^{45} + e^{17} + e^{23}$                       | 2479     |
| 9531:423  | $0, 0, 0, 0, e^{12}, e^{13} + e^{24}, e^{15}, e^{14} + e^{26} + e^{35}, e^{23} + e^{17}$               | 2479     |
| 9531:424  | $0, 0, 0, 0, -e^{12}, e^{14} + e^{23}, e^{15}, e^{16} + e^{35}, e^{17} + e^{25}$                       | 2479     |
| 9531:425  | $0, 0, 0, 0, e^{12}, e^{13} + e^{24}, e^{15}, e^{26} + e^{35}, e^{17} + e^{25}$                        | 2479     |
| 9531:426  | $0, 0, 0, 0, e^{12}, e^{23} + e^{14}, e^{13} + e^{25}, e^{15}, e^{27} + e^{16}$                        | 2479     |
| 9531:427  | $0, 0, 0, 0, e^{12}, -e^{13}, e^{15} + e^{34}, e^{14} + e^{25}, e^{46} + e^{23} + e^{17}$              | 2479     |
| 9531:428  | $0, 0, 0, 0, -e^{12}, e^{13}, e^{15} + e^{24}, e^{16} + e^{25}, e^{17} + e^{45}$                       | 2479     |
| 9531:429a | $0, 0, 0, 0, -e^{12}, e^{13}, e^{24} + e^{15}, e^{36} + e^{14}, e^{23} + e^{45} + e^{17}$              | 2479     |
| 9531:429b | $0, 0, 0, 0, -e^{12}, -e^{13}, e^{24} + e^{15}, e^{36} + e^{14}, e^{45} + e^{17} + e^{23}$             | 2479     |
| 9531:430  | $0, 0, 0, 0, -e^{12}, a_2 e^{13}, e^{24} + e^{15}, e^{16} + e^{34}, e^{17} + e^{45} + e^{23}$          | 2479     |
| 9531:431  | $0, 0, 0, 0, e^{12}, e^{13}, e^{25} + e^{14}, e^{15}, e^{45} + e^{36} + e^{27}$                        | 2479     |
| 9531:432  | $0, 0, 0, 0, -e^{12}, e^{13}, e^{24} + e^{15}, e^{25}, e^{36} + e^{17} + e^{45}$                       | 2479     |
| 9531:433  | $0, 0, 0, 0, -e^{12}, e^{13}, e^{15} + e^{23}, e^{16} + e^{25}, e^{35} + e^{24} + e^{17}$              | 2579     |
| 9531:434  | $0, 0, 0, 0, e^{12}, e^{24} - e^{13}, e^{15} + e^{34}, e^{25}, e^{46} + e^{17} + e^{23}$               | 2479     |
| 9531:435a | $0, 0, 0, 0, e^{12}, -e^{13}, e^{15} + e^{34}, e^{16} + e^{25}, e^{17} + e^{46} + e^{23}$              | 2479     |
| 9531:435b | $0, 0, 0, 0, e^{12}, -e^{13}, e^{34} - e^{15}, e^{25} + e^{16}, e^{46} + e^{17} + e^{23}$              | 2479     |
| 9531:436  | $0, 0, 0, 0, e^{12}(-1 + a_2), a_2 e^{13}, e^{15} + e^{23}, e^{25} + e^{14}, e^{26} + e^{17} + e^{35}$ | 2579     |
| 9531:437  | $0, 0, 0, 0, e^{12}, e^{14} + e^{23}, e^{13} + e^{25}, e^{15} + e^{34}, e^{27} + e^{16}$               | 2479     |
| 9531:438  | $0, 0, 0, 0, e^{12}, -e^{13}, a_2 e^{15} + e^{34}, e^{16} + e^{23}, e^{25} + e^{17} + e^{46}$          | 2479     |
| 9531:439a | $0, 0, 0, 0, e^{12}, -e^{13}, e^{15} + e^{34}, e^{16} + e^{24}, e^{17} + e^{25} + e^{46}$              | 2479     |
| 9531:439b | $0, 0, 0, 0, -e^{12}, -e^{13}, e^{34} + e^{15}, e^{24} + e^{16}, e^{46} + e^{25} + e^{17}$             | 2479     |
| 9531:440a | $0, 0, 0, 0, e^{12}, e^{34}, e^{13} + e^{25}, e^{36} + e^{15}, e^{35} + e^{14} + e^{27}$               | 2479     |
| 9531:440b | $0, 0, 0, 0, e^{12}, e^{34}, e^{13} + e^{25}, -e^{15} + e^{36}, e^{14} + e^{27} + e^{35}$              | 2479     |
| 9531:441  | $0, 0, 0, 0, e^{12}, e^{34}, e^{25} + e^{13}, e^{15} + e^{46}, e^{27} + e^{35} + e^{14}$               | 2479     |
| 9531:442a | $0, 0, 0, 0, -e^{12}, e^{13}, e^{24} + e^{15}, e^{23} + e^{16}, e^{36} + e^{45} + e^{17}$              | 2479     |
| 9531:442b | $0, 0, 0, 0, -e^{12}, e^{13}, e^{24} - e^{15}, e^{16} + e^{23}, e^{36} + e^{17} + e^{45}$              | 2479     |
| 9531:443a | $0, 0, 0, 0, e^{12}, e^{13}, e^{25} + e^{14}, e^{23} + e^{16}, e^{27} + e^{45} + e^{36}$               | 2479     |
| 9531:443b | $0, 0, 0, 0, -e^{12}, e^{13}, -e^{14} + e^{25}, e^{16} + e^{23}, e^{45} + e^{36} + e^{27}$             | 2479     |
| 9531:444  | $0, 0, 0, 0, e^{12}, e^{13}, e^{25} + e^{14}, e^{16} + e^{24}, e^{27} + e^{45} + e^{36}$               | 2479     |
| 9531:445  | $0, 0, 0, 0, e^{12}, e^{13}, e^{14} + e^{25}, e^{24} + e^{36}, e^{45} + e^{27} + e^{16}$               | 2479     |
| 9531:446a | $0, 0, 0, 0, -e^{12}, e^{34}, e^{23} + e^{15}, e^{25} + e^{13}, e^{17} + e^{46} + e^{35}$              | 2479     |
| 9531:446b | $0, 0, 0, 0, -e^{12}, e^{34}, -e^{15} + e^{23}, e^{25} + e^{13}, e^{46} + e^{17} + e^{35}$             | 2479     |
| 9531:447  | $0, 0, 0, 0, -e^{12}, e^{34}, e^{23} + e^{15}, e^{25} + e^{14}, e^{46} + e^{35} + e^{17}$              | 2479     |
| 9531:448a | $0, 0, 0, 0, -e^{12}, e^{13}, e^{24} + e^{15}, e^{36} + e^{25} + e^{14}, e^{17} + e^{45}$              | 2479     |
| 9531:448b | $0, 0, 0, 0, -e^{12}, e^{13}, -e^{15} + e^{24}, e^{14} + e^{36} + e^{25}, e^{45} + e^{17}$             | 2479     |
| 9531:448c | $0, 0, 0, 0, -e^{12}, -e^{13}, e^{15} + e^{24}, e^{14} + e^{36} + e^{25}, e^{17} + e^{45}$             | 2479     |
| 9531:448d | $0, 0, 0, 0, -e^{12}, -e^{13}, e^{24} - e^{15}, e^{25} + e^{36} + e^{14}, e^{45} + e^{17}$             | 2479     |
| 9531:449  | $0, 0, 0, 0, -e^{12}, -e^{13}, e^{24} + e^{15}, e^{26} + e^{35} + e^{14}, e^{17} + e^{45}$             | 2479     |
| 9531:450  | $0, 0, 0, 0, -e^{12}, a_2 e^{13}, e^{15} + e^{24}, e^{16} + e^{25} + e^{34}, e^{45} + e^{17}$          | 2479     |
| 9531:451a | $0, 0, 0, 0, e^{12}, e^{13}, e^{14} + e^{25}, e^{24} + e^{36} + e^{15}, e^{45} + e^{27}$               | 2479     |
| 9531:451b | $0, 0, 0, 0, -e^{12}, e^{13}, -e^{14} + e^{25}, e^{15} + e^{36} + e^{24}, e^{27} + e^{45}$             | 2479     |
| 9531:452  | $0, 0, 0, 0, e^{12}(-1 + a_2), a_2 e^{13}, e^{15} + e^{23}, e^{16} + e^{25}, e^{17} + e^{26} + e^{35}$ | 3579     |
| 9531:453a | $0, 0, 0, 0, -e^{12}, e^{13}, e^{15} + e^{23}, e^{36} + e^{25} + e^{14}, e^{24} + e^{35} + e^{17}$     | 2579     |
| 9531:453b | $0, 0, 0, 0, -e^{12}, -e^{13}, e^{23} + e^{15}, e^{36} + e^{25} + e^{14}, e^{17} + e^{35} + e^{24}$    | 2579     |
| 9531:454a | $0, 0, 0, 0, -e^{12}, e^{13}, e^{15} + e^{23}, e^{16} + e^{25} + e^{34}, e^{17} + e^{24} + e^{35}$     | 2579     |

Table 2 – Continued to next page

Table 2 – Continued from previous page

| Name      | $\mathfrak{g}$                                                                                                | UCS Dim. |
|-----------|---------------------------------------------------------------------------------------------------------------|----------|
| 9531:454b | $0, 0, 0, 0, -e^{12}, e^{13}, e^{15} + e^{23}, e^{16} + e^{34} - e^{25}, e^{17} + e^{35} + e^{24}$            | 2579     |
| 9531:455  | $0, 0, 0, 0, -e^{12}, e^{24} + e^{13}, e^{15} + e^{23}, e^{16} + e^{45}, e^{35} + e^{17}$                     | 2479     |
| 9531:456  | $0, 0, 0, 0, e^{12}, e^{13}, e^{25} + e^{14}, e^{15} + e^{34}, e^{27} + e^{36} + e^{45}$                      | 2479     |
| 9531:457  | $0, 0, 0, 0, -e^{12}, e^{13}, e^{24} + e^{15}, e^{34} + e^{25}, e^{36} + e^{45} + e^{17}$                     | 2479     |
| 9531:458a | $0, 0, 0, 0, e^{12}, -e^{13}, e^{34} + e^{15}, e^{36} + e^{25} + e^{14}, e^{46} + e^{17} + e^{23}$            | 2479     |
| 9531:458b | $0, 0, 0, 0, -e^{12}, -e^{13}, e^{34} + e^{15}, e^{25} + e^{14} + e^{36}, e^{23} + e^{17} + e^{46}$           | 2479     |
| 9531:459a | $0, 0, 0, 0, -e^{12}, -e^{13}, e^{15} + e^{34}, e^{14} + e^{35} + e^{26}, e^{17} + e^{46} + e^{23}$           | 2479     |
| 9531:459b | $0, 0, 0, 0, -e^{12}, -e^{13}, -e^{15} + e^{34}, e^{14} + e^{26} + e^{35}, e^{46} + e^{23} + e^{17}$          | 2479     |
| 9531:460  | $0, 0, 0, 0, -e^{12}, -e^{13}, e^{15} + e^{34}, e^{35} + e^{26}, e^{17} + e^{46} + e^{25}$                    | 2479     |
| 9531:461  | $0, 0, 0, 0, -e^{12}, e^{24} + e^{13}, e^{15} + e^{23}, e^{45} + e^{16}, e^{26} + e^{17}$                     | 2479     |
| 9531:462  | $0, 0, 0, 0, -e^{12}, -e^{13}, e^{24} + e^{15}, e^{35} + e^{26}, e^{36} + e^{45} + e^{17}$                    | 2479     |
| 9531:463  | $0, 0, 0, 0, e^{12}, e^{13}, e^{14} + e^{25}, e^{35} + e^{26}, e^{36} + e^{45} + e^{27}$                      | 2479     |
| 9531:464a | $0, 0, 0, 0, e^{12}a_1, e^{13}(1 + a_1), e^{15} + e^{23}, e^{25} + e^{36} + e^{14}, e^{17} + e^{26} + e^{35}$ | 2579     |
| 9531:464b | $0, 0, 0, 0, e^{12}a_1, e^{13}(1 + a_1), e^{23} + e^{15}, e^{36} + e^{14} - e^{25}, e^{35} + e^{17} + e^{26}$ | 2579     |
| 9531:465  | $0, 0, 0, 0, e^{12}a_1, e^{13}(1 + a_1), e^{15} + e^{23}, e^{16} + e^{25} + e^{34}, e^{17} + e^{26} + e^{35}$ | 2579     |
| 9531:466  | $0, 0, 0, 0, -e^{12}, e^{34}, e^{15} + e^{23}, e^{36} + e^{25} + e^{14}, e^{35} + e^{17} + e^{46}$            | 2479     |
| 9531:467  | $0, 0, 0, 0, -e^{12}, e^{14} + e^{23}, e^{15} + e^{34}, e^{35} + e^{16}, e^{36} + e^{24} + e^{17}$            | 2479     |
| 9531:468  | $0, 0, 0, 0, -e^{12}, e^{24} - e^{13}, e^{34} + e^{15}, e^{26} + e^{35}, e^{46} + e^{17} + e^{23}$            | 2479     |
| 9531:469  | $0, 0, 0, 0, e^{12}, e^{13} + e^{24}, e^{15}, e^{25}, e^{26} + e^{17} + e^{35}$                               | 2479     |
| 9531:470  | $0, 0, 0, 0, e^{12}, e^{13}, e^{25} + e^{14}, e^{15}, e^{27} + e^{16} + e^{45}$                               | 2479     |
| 9531:471a | $0, 0, 0, 0, -e^{12}, e^{14} + e^{23}, e^{15}, e^{16} + e^{35}, e^{17} + e^{34} + e^{25}$                     | 2479     |
| 9531:471b | $0, 0, 0, 0, -e^{12}, -e^{14} + e^{23}, e^{15}, e^{35} + e^{16}, e^{25} + e^{34} + e^{17}$                    | 2479     |
| 9531:472a | $0, 0, 0, 0, e^{12}, e^{13} + e^{24}, e^{15}, e^{35} + e^{26}, e^{17} + e^{34} + e^{25}$                      | 2479     |
| 9531:472b | $0, 0, 0, 0, e^{12}, e^{24} + e^{13}, -e^{15}, e^{26} + e^{35}, e^{17} + e^{25} + e^{34}$                     | 2479     |
| 9531:473  | $0, 0, 0, 0, e^{12}, e^{13} + e^{24}, e^{15}, e^{14} + e^{26} + e^{35}, e^{17} + e^{25}$                      | 2479     |
| 9531:474  | $0, 0, 0, 0, -e^{12}, e^{13}a_2 + e^{24}, e^{15}, e^{45} + e^{16} + e^{23}, e^{25} + e^{17}$                  | 2479     |
| 9531:475a | $0, 0, 0, 0, e^{12}, e^{23} + e^{14}, e^{25} + e^{13}, e^{15}, e^{27} + e^{16} + e^{34}$                      | 2479     |
| 9531:475b | $0, 0, 0, 0, -e^{12}, e^{14} + e^{23}, e^{13} + e^{25}, e^{15}, e^{34} + e^{27} + e^{16}$                     | 2479     |
| 9531:476  | $0, 0, 0, 0, e^{12}, e^{23} + e^{14}, e^{13} + e^{25}, e^{24} + e^{15}, e^{27} + e^{16}$                      | 2479     |
| 9531:477  | $0, 0, 0, 0, e^{12}, e^{13} + e^{24}, e^{15}, e^{34} + e^{25}, e^{17} + e^{35} + e^{26}$                      | 2479     |
| 9531:478a | $0, 0, 0, 0, -e^{12}, e^{13}, e^{15} + e^{24}, e^{36} + e^{25}, e^{45} + e^{17} + e^{23}$                     | 2479     |
| 9531:478b | $0, 0, 0, 0, -e^{12}, -e^{13}, e^{15} + e^{24}, e^{25} + e^{36}, e^{17} + e^{23} + e^{45}$                    | 2479     |
| 9531:479  | $0, 0, 0, 0, -e^{12}, -e^{13}, e^{24} + e^{15}, e^{26} + e^{35}, e^{17} + e^{45} + e^{23}$                    | 2479     |
| 9531:480  | $0, 0, 0, 0, e^{12}, e^{13}, e^{25} + e^{14}, e^{15} + e^{23}, e^{27} + e^{36} + e^{45}$                      | 2479     |
| 9531:481a | $0, 0, 0, 0, -e^{12}, e^{13}, e^{24} + e^{15}, e^{25} + e^{14}, e^{36} + e^{45} + e^{17}$                     | 2479     |
| 9531:481b | $0, 0, 0, 0, -e^{12}, e^{13}, e^{24} - e^{15}, e^{25} + e^{14}, e^{36} + e^{17} + e^{45}$                     | 2479     |
| 9531:482a | $0, 0, 0, 0, e^{12}, e^{13}, e^{25} + e^{14}, e^{15} + e^{24}, e^{27} + e^{45} + e^{36}$                      | 2479     |
| 9531:482b | $0, 0, 0, 0, -e^{12}, e^{13}, -e^{14} + e^{25}, e^{15} + e^{24}, e^{36} + e^{27} + e^{45}$                    | 2479     |
| 9531:483  | $0, 0, 0, 0, e^{12}, e^{13}, e^{25} + e^{14}, e^{34} + e^{15}, e^{45} + e^{27} + e^{16}$                      | 2479     |
| 9531:484  | $0, 0, 0, 0, e^{12}, e^{23} + e^{14}, e^{15} + e^{34}, e^{13} + e^{25}, e^{24} + e^{36} + e^{17}$             | 2479     |
| 9531:485a | $0, 0, 0, 0, e^{12}, e^{34}, e^{13} + e^{25}, e^{15} + e^{23} + e^{46}, e^{14} + e^{27} + e^{35}$             | 2479     |
| 9531:485b | $0, 0, 0, 0, -e^{12}, e^{34}, e^{25} - e^{13}, e^{46} + e^{15} + e^{23}, e^{14} + e^{27} + e^{35}$            | 2479     |
| 9531:486a | $0, 0, 0, 0, e^{12}, e^{34}, e^{13} + e^{25}, e^{36} + e^{15} + e^{24}, e^{35} + e^{27} + e^{14}$             | 2479     |
| 9531:486b | $0, 0, 0, 0, e^{12}, e^{34}, e^{13} + e^{25}, e^{24} + e^{36} - e^{15}, e^{35} + e^{14} + e^{27}$             | 2479     |
| 9531:487  | $0, 0, 0, 0, -e^{12}, e^{13}, e^{15} + e^{24}, e^{16} + e^{25}, e^{36} + e^{45} + e^{17}$                     | 2479     |
| 9531:488  | $0, 0, 0, 0, e^{12}, e^{13}, e^{25} + e^{14}, e^{15} + e^{36}, e^{27} + e^{16} + e^{45}$                      | 2479     |
| 9531:489  | $0, 0, 0, 0, e^{12}, e^{13}, e^{25} + e^{14}, e^{35} + e^{26}, e^{45} + e^{27} + e^{16}$                      | 2479     |
| 9531:490  | $0, 0, 0, 0, -e^{12}, -e^{14} + e^{23}, e^{15}, e^{16} + e^{35}, e^{17} + e^{26} + e^{45}$                    | 2479     |
| 9531:491a | $0, 0, 0, 0, -e^{12}, -e^{13}, e^{34} + e^{15}, e^{26} + e^{35} + e^{14}, e^{25} + e^{17} + e^{46}$           | 2479     |
| 9531:491b | $0, 0, 0, 0, -e^{12}, -e^{13}, -e^{15} + e^{34}, e^{14} + e^{26} + e^{35}, e^{17} + e^{25} + e^{46}$          | 2479     |
| 9531:492a | $0, 0, 0, 0, -e^{12}, e^{24} + e^{13}, e^{23} + e^{15}, e^{45} + e^{16}, e^{34} + e^{26} + e^{17}$            | 2479     |
| 9531:492b | $0, 0, 0, 0, -e^{12}, e^{24} + e^{13}, e^{23} - e^{15}, e^{16} + e^{45}, e^{17} + e^{26} + e^{34}$            | 2479     |
| 9531:493  | $0, 0, 0, 0, -e^{12}, -e^{13}, e^{24} + e^{15}, e^{26} + e^{35} + e^{14}, e^{36} + e^{17} + e^{45}$           | 2479     |
| 9531:494  | $0, 0, 0, 0, -e^{12}, e^{13}a_2, e^{15} + e^{24}, e^{34} + e^{16} + e^{25}, e^{36} + e^{45} + e^{17}$         | 2479     |
| 9531:495a | $0, 0, 0, 0, -e^{12}, e^{24} - e^{13}, e^{34} + e^{15}, e^{26} + e^{35} + e^{14}, e^{46} + e^{17} + e^{23}$   | 2479     |
| 9531:495b | $0, 0, 0, 0, -e^{12}, e^{24} - e^{13}, -e^{15} + e^{34}, e^{14} + e^{26} + e^{35}, e^{17} + e^{23} + e^{46}$  | 2479     |
| 9531:496  | $0, 0, 0, 0, -e^{12}, e^{23} + e^{14}, e^{34} + e^{15}, e^{35} + e^{16}, e^{25} + e^{36} + e^{17}$            | 2479     |
| 9531:497  | $0, 0, 0, 0, -e^{12}, e^{24} - e^{13}, e^{15} + e^{34}, e^{26} + e^{35}, e^{17} + e^{25} + e^{46}$            | 2479     |

Table 2 – Continued to next page

Table 2 – Continued from previous page

| Name      | $\mathfrak{g}$                                                                                                         | UCS Dim. |
|-----------|------------------------------------------------------------------------------------------------------------------------|----------|
| 9531:498  | $0, 0, 0, 0, e^{12}, e^{14} + e^{23}, e^{15}, e^{13} + e^{25}, e^{45} + e^{17} + e^{26}$                               | 2479     |
| 9531:499a | $0, 0, 0, 0, -e^{12}, e^{13}, e^{24} + e^{15}, e^{25} + e^{16}, e^{45} + e^{17} + e^{23}$                              | 2479     |
| 9531:499b | $0, 0, 0, 0, -e^{12}, -e^{13}, e^{24} + e^{15}, e^{16} + e^{25}, e^{17} + e^{45} + e^{23}$                             | 2479     |
| 9531:500  | $0, 0, 0, 0, e^{12}, e^{13}, e^{25} + e^{14}, e^{15} + e^{23}, e^{27} + e^{16} + e^{45}$                               | 2479     |
| 9531:501a | $0, 0, 0, 0, e^{12}, e^{13}, e^{25} + e^{14}, e^{15} + e^{24}, e^{45} + e^{27} + e^{16}$                               | 2479     |
| 9531:501b | $0, 0, 0, 0, -e^{12}, e^{13}, e^{25} - e^{14}, e^{24} + e^{15}, e^{27} + e^{16} + e^{45}$                              | 2479     |
| 9531:502a | $0, 0, 0, 0, e^{12}, e^{13} + e^{24}, e^{15}, e^{35} + e^{14} + e^{26}, e^{17} + e^{34} + e^{25}$                      | 2479     |
| 9531:502b | $0, 0, 0, 0, e^{12}, e^{24} + e^{13}, -e^{15}, e^{26} + e^{35} + e^{14}, e^{17} + e^{25} + e^{34}$                     | 2479     |
| 9531:503a | $0, 0, 0, 0, -e^{12}, e^{13} + e^{24}, e^{15}, a_2 e^{23} + e^{16} + e^{45}, e^{17} + e^{34} + e^{25}$                 | 2479     |
| 9531:503b | $0, 0, 0, 0, -e^{12}, e^{24} - e^{13}, e^{15}, a_2 e^{23} + e^{16} + e^{45}, e^{17} + e^{34} + e^{25}$                 | 2479     |
| 9531:504  | $0, 0, 0, 0, a_1 e^{12}, e^{13} + e^{24}, e^{15} + e^{23}, e^{25} + e^{14}, e^{17} + e^{26} + e^{34}$                  | 2479     |
| 9531:505  | $0, 0, 0, 0, e^{12} a_1, e^{14} + e^{23}, (1 + a_1) e^{13} + e^{25}, e^{15}, e^{27} + e^{35} + e^{16}$                 | 2479     |
| 9531:506a | $0, 0, 0, 0, -e^{12}, e^{13}, e^{24} + e^{15}, e^{25} + e^{36} + e^{14}, e^{23} + e^{45} + e^{17}$                     | 2479     |
| 9531:506b | $0, 0, 0, 0, -e^{12}, e^{13}, e^{24} - e^{15}, e^{36} + e^{25} + e^{14}, e^{45} + e^{17} + e^{23}$                     | 2479     |
| 9531:506c | $0, 0, 0, 0, -e^{12}, -e^{13}, e^{24} + e^{15}, e^{36} + e^{25} + e^{14}, e^{17} + e^{45} + e^{23}$                    | 2479     |
| 9531:506d | $0, 0, 0, 0, -e^{12}, -e^{13}, -e^{15} + e^{24}, e^{14} + e^{36} + e^{25}, e^{17} + e^{23} + e^{45}$                   | 2479     |
| 9531:507  | $0, 0, 0, 0, -e^{12}, -e^{13}, e^{24} + e^{15}, e^{26} + e^{35} + e^{14}, e^{17} + e^{23} + e^{45}$                    | 2479     |
| 9531:508a | $0, 0, 0, 0, -e^{12}, a_2 e^{13}, e^{15} + e^{24}, e^{34} + e^{16} + e^{25}, e^{45} + e^{23} + e^{17}$                 | 2479     |
| 9531:508b | $0, 0, 0, 0, -e^{12}, a_2 e^{13}, e^{15} + e^{24}, e^{16} + e^{34} - e^{25}, e^{17} + e^{23} + e^{45}$                 | 2479     |
| 9531:509  | $0, 0, 0, 0, e^{12} a_1, e^{14} + e^{23}, e^{25} + e^{13}(1 + a_1), e^{15} + e^{34}, e^{16} + e^{27} + e^{35}$         | 2479     |
| 9531:510a | $0, 0, 0, 0, e^{12}, e^{13}, e^{25} + e^{14}, e^{15} + e^{24} + e^{36}, e^{27} + e^{16} + e^{45}$                      | 2479     |
| 9531:510b | $0, 0, 0, 0, -e^{12}, e^{13}, e^{25} - e^{14}, e^{24} + e^{36} + e^{15}, e^{27} + e^{16} + e^{45}$                     | 2479     |
| 9531:511  | $0, 0, 0, 0, -e^{12}, e^{24} - e^{13}, e^{15}, e^{16} + e^{23} + e^{45}, e^{17} + e^{26} + e^{35}$                     | 2479     |
| 9531:512  | $0, 0, 0, 0, -e^{12} a_1, -(-1 + a_1) e^{13} + e^{24}, e^{23} + e^{15}, e^{45} + e^{16} a_1, e^{35} + e^{26} + e^{17}$ | 2479     |
| 9531:513a | $0, 0, 0, 0, e^{12}, e^{14} + e^{23}, e^{34} + e^{15}, e^{45} + e^{13} + e^{26}, e^{36} + e^{17} + e^{25}$             | 2479     |
| 9531:513b | $0, 0, 0, 0, e^{12}, e^{14} + e^{23}, e^{34} - e^{15}, e^{45} + e^{13} + e^{26}, e^{17} + e^{36} + e^{25}$             | 2479     |
| 9531:514  | $0, 0, 0, 0, -e^{12}, e^{14} + e^{23}, e^{34} + a_3 e^{15}, e^{16} + e^{35} + e^{24}, e^{17} + e^{25} + e^{36}$        | 2479     |
| 9531:515  | $0, 0, 0, 0, (-1 + a_2) e^{12}, e^{24} + e^{13} a_2, e^{15} + e^{23}, e^{25} + e^{14}, e^{17} + e^{26} + e^{35}$       | 2479     |
| 9531:516a | $0, 0, 0, 0, e^{12}, e^{34}, e^{15}, e^{25}, e^{17} + e^{28}$                                                          | 2679     |
| 9531:516b | $0, 0, 0, 0, e^{12}, e^{34}, -e^{15}, e^{25}, e^{28} + e^{17}$                                                         | 2679     |
| 9531:517  | $0, 0, 0, 0, e^{12}, e^{34}, e^{15}, e^{25}, e^{27} + e^{18}$                                                          | 2679     |
| 9531:518a | $0, 0, 0, 0, e^{12}, e^{13}, e^{15}, e^{25}, e^{17} + e^{28}$                                                          | 3679     |
| 9531:518b | $0, 0, 0, 0, e^{12}, e^{13}, -e^{15}, e^{25}, e^{28} + e^{17}$                                                         | 3679     |
| 9531:519  | $0, 0, 0, 0, e^{12}, e^{13}, e^{15}, e^{25}, e^{27} + e^{18}$                                                          | 3679     |
| 9531:520a | $0, 0, 0, 0, e^{12}, e^{13}, e^{15}, e^{25}, e^{17} + e^{34} + e^{28}$                                                 | 2679     |
| 9531:520b | $0, 0, 0, 0, e^{12}, e^{13}, -e^{15}, e^{25}, e^{17} + e^{28} + e^{34}$                                                | 2679     |
| 9531:521  | $0, 0, 0, 0, e^{12}, e^{13}, e^{15}, e^{25}, e^{27} + e^{18} + e^{34}$                                                 | 2679     |
| 9531:522a | $0, 0, 0, 0, e^{12}, e^{13} + e^{24}, e^{15}, e^{25}, e^{17} + e^{28}$                                                 | 2679     |
| 9531:522b | $0, 0, 0, 0, e^{12}, e^{13} + e^{24}, -e^{15}, e^{25}, e^{17} + e^{28}$                                                | 2679     |
| 9531:523  | $0, 0, 0, 0, e^{12}, e^{24} + e^{13}, e^{15}, e^{25}, e^{27} + e^{18}$                                                 | 2679     |
| 9531:524a | $0, 0, 0, 0, e^{12}, e^{13} + e^{24}, e^{15}, e^{25}, e^{17} + e^{28} + e^{34}$                                        | 2679     |
| 9531:524b | $0, 0, 0, 0, e^{12}, e^{13} + e^{24}, -e^{15}, e^{25}, e^{28} + e^{34} + e^{17}$                                       | 2679     |
| 9531:524c | $0, 0, 0, 0, -e^{12}, e^{24} + e^{13}, e^{15}, e^{25}, e^{28} + e^{17} + e^{34}$                                       | 2679     |
| 9531:525  | $0, 0, 0, 0, e^{12}, e^{24} + e^{13}, e^{15}, e^{25}, e^{18} + e^{34} + e^{27}$                                        | 2679     |
| 9531:526  | $0, 0, 0, 0, e^{12}, e^{34}, e^{15}, e^{13} + e^{25}, e^{18} + e^{27}$                                                 | 2579     |
| 9531:527  | $0, 0, 0, 0, e^{12}, e^{13}, e^{25}, e^{15} + e^{23}, e^{28} + e^{17}$                                                 | 3579     |
| 9531:528  | $0, 0, 0, 0, e^{12}, e^{13}, e^{15}, e^{25} + e^{14}, e^{18} + e^{27}$                                                 | 2579     |
| 9531:529  | $0, 0, 0, 0, e^{12}, e^{13}, e^{25}, e^{15} + e^{24}, e^{28} + e^{17}$                                                 | 2579     |
| 9531:530a | $0, 0, 0, 0, e^{12}, e^{34}, e^{23} + e^{15}, e^{25} + e^{13}, e^{28} + e^{17}$                                        | 2579     |
| 9531:530b | $0, 0, 0, 0, e^{12}, e^{34}, -e^{15} + e^{23}, e^{13} + e^{25}, e^{17} + e^{28}$                                       | 2579     |
| 9531:531a | $0, 0, 0, 0, e^{12}, e^{34}, e^{13} + e^{25}, e^{15} + e^{23}, e^{28} + e^{17}$                                        | 2579     |
| 9531:531b | $0, 0, 0, 0, e^{12}, e^{34}, e^{25} - e^{13}, e^{15} + e^{23}, e^{28} + e^{17}$                                        | 2579     |
| 9531:532a | $0, 0, 0, 0, e^{12}, e^{13}, e^{15}, e^{25}, e^{28} + e^{36} + e^{17}$                                                 | 2579     |
| 9531:532b | $0, 0, 0, 0, e^{12}, e^{13}, -e^{15}, e^{25}, e^{36} + e^{28} + e^{17}$                                                | 2579     |
| 9531:533  | $0, 0, 0, 0, e^{12}, e^{13}, e^{15}, e^{25}, e^{18} + e^{36} + e^{27}$                                                 | 2579     |
| 9531:534  | $0, 0, 0, 0, e^{12}, e^{13}, e^{15}, e^{25} + e^{14}, e^{18} + e^{27} + e^{34}$                                        | 2579     |
| 9531:535  | $0, 0, 0, 0, e^{12}, e^{13}, e^{25}, e^{15} + e^{24}, e^{28} + e^{17} + e^{34}$                                        | 2579     |
| 9531:536  | $0, 0, 0, 0, e^{12}, e^{14} + e^{23}, e^{15}, e^{13} + e^{25}, e^{18} + e^{27}$                                        | 2579     |

Table 2 – Continued to next page

Table 2 – Continued from previous page

| Name      | $\mathfrak{g}$                                                                                        | UCS Dim. |
|-----------|-------------------------------------------------------------------------------------------------------|----------|
| 9531:537  | $0, 0, 0, 0, e^{12}, e^{13}, e^{25}, e^{15} + e^{23}, e^{34} + e^{17} + e^{28}$                       | 2579     |
| 9531:538a | $0, 0, 0, 0, e^{12}, e^{13}, e^{15} + e^{24}, e^{14} + e^{25}, e^{28} + e^{17}$                       | 2579     |
| 9531:538b | $0, 0, 0, 0, e^{12}, e^{13}, -e^{15} + e^{24}, e^{14} + e^{25}, e^{28} + e^{17}$                      | 2579     |
| 9531:539a | $0, 0, 0, 0, e^{12}, e^{13}, e^{14} + e^{25}, e^{15} + e^{24}, e^{17} + e^{28}$                       | 2579     |
| 9531:539b | $0, 0, 0, 0, e^{12}, e^{13}, e^{25} - e^{14}, e^{24} + e^{15}, e^{28} + e^{17}$                       | 2579     |
| 9531:540a | $0, 0, 0, 0, e^{12}, e^{34}, e^{15}, e^{25} + e^{13}, e^{17} + e^{28} + e^{35}$                       | 2579     |
| 9531:540b | $0, 0, 0, 0, e^{12}, e^{34}, -e^{15}, e^{25} + e^{13}, e^{28} + e^{17} + e^{35}$                      | 2579     |
| 9531:541a | $0, 0, 0, 0, e^{12}, e^{34}, e^{15}, e^{25}, e^{17} + e^{28} + e^{36}$                                | 1479     |
| 9531:541b | $0, 0, 0, 0, e^{12}, e^{34}, -e^{15}, e^{25}, e^{36} + e^{28} + e^{17}$                               | 1479     |
| 9531:542  | $0, 0, 0, 0, e^{12}, e^{34}, e^{15}, e^{25}, e^{36} + e^{27} + e^{18}$                                | 1479     |
| 9531:543  | $0, 0, 0, 0, e^{12}, e^{14} + e^{23}, e^{15}, e^{13} + e^{25}, e^{27} + e^{18} + e^{34}$              | 2579     |
| 9531:544a | $0, 0, 0, 0, -e^{12}, e^{13}, e^{25}, e^{15} + e^{23}, e^{18} + e^{27} + e^{35}$                      | 3579     |
| 9531:544b | $0, 0, 0, 0, -e^{12}, e^{13}, e^{25}, e^{23} - e^{15}, e^{35} + e^{27} + e^{18}$                      | 3579     |
| 9531:545a | $0, 0, 0, 0, e^{12}, e^{13}, e^{15}, e^{25} + e^{14}, e^{28} + e^{45} + e^{17}$                       | 2579     |
| 9531:545b | $0, 0, 0, 0, e^{12}, e^{13}, -e^{15}, e^{25} + e^{14}, e^{17} + e^{28} + e^{45}$                      | 2579     |
| 9531:546a | $0, 0, 0, 0, -e^{12}, e^{13}, e^{25}, e^{15} + e^{24}, e^{45} + e^{18} + e^{27}$                      | 2579     |
| 9531:546b | $0, 0, 0, 0, -e^{12}, e^{13}, e^{25}, e^{24} - e^{15}, e^{45} + e^{27} + e^{18}$                      | 2579     |
| 9531:547  | $0, 0, 0, 0, e^{12}, e^{13}, e^{25}, e^{15} + e^{23}, e^{36} + e^{17} + e^{28}$                       | 2579     |
| 9531:548  | $0, 0, 0, 0, e^{12}, e^{34}, e^{13} + e^{25}, e^{15} + e^{24}, e^{28} + e^{17}$                       | 2479     |
| 9531:549a | $0, 0, 0, 0, e^{12}, e^{13}, e^{15} + e^{24}, e^{14} + e^{25}, e^{28} + e^{17} + e^{34}$              | 2579     |
| 9531:549b | $0, 0, 0, 0, e^{12}, e^{13}, -e^{15} + e^{24}, e^{14} + e^{25}, e^{17} + e^{34} + e^{28}$             | 2579     |
| 9531:550a | $0, 0, 0, 0, e^{12}, e^{13}, e^{24} + e^{15}, e^{25} + e^{14}, e^{18} + e^{34} + e^{27}$              | 2579     |
| 9531:550b | $0, 0, 0, 0, e^{12}, e^{13}, e^{24} + e^{15}, e^{25} - e^{14}, e^{18} + e^{27} + e^{34}$              | 2579     |
| 9531:551a | $0, 0, 0, 0, (-1 + a_2)e^{12}, e^{34}, e^{15} + e^{23}, e^{25} + e^{13}a_2, e^{28} + e^{17} + e^{35}$ | 2579     |
| 9531:551b | $0, 0, 0, 0, (-1 + a_2)e^{12}, e^{34}, e^{23} - e^{15}, e^{25} + e^{13}a_2, e^{35} + e^{28} + e^{17}$ | 2579     |
| 9531:552  | $0, 0, 0, 0, e^{12}, e^{13}, e^{15} + e^{23}, e^{14} + e^{25}, e^{27} + e^{18}$                       | 2479     |
| 9531:553  | $0, 0, 0, 0, e^{12}, -e^{13}, e^{15}, e^{34} + e^{25}, e^{46} + e^{18} + e^{27}$                      | 1479     |
| 9531:554a | $0, 0, 0, 0, e^{12}, -e^{13}, e^{25}, e^{15} + e^{34}, e^{18} + e^{46} + e^{27}$                      | 1479     |
| 9531:554b | $0, 0, 0, 0, e^{12}, -e^{13}, e^{25}, -e^{15} + e^{34}, e^{27} + e^{18} + e^{46}$                     | 1479     |
| 9531:555  | $0, 0, 0, 0, e^{12}, e^{34}, e^{15}, e^{25} + e^{13}, e^{36} + e^{18} + e^{27}$                       | 1479     |
| 9531:556a | $0, 0, 0, 0, e^{12}, e^{34}, e^{15}, e^{13} + e^{25}, e^{18} + e^{46} + e^{27}$                       | 1479     |
| 9531:556b | $0, 0, 0, 0, e^{12}, e^{34}, e^{15}, -e^{13} + e^{25}, e^{27} + e^{18} + e^{46}$                      | 1479     |
| 9531:557a | $0, 0, 0, 0, e^{12}, e^{14} + e^{23}, e^{15}, e^{13} + e^{25}, e^{28} + e^{35} + e^{17}$              | 2579     |
| 9531:557b | $0, 0, 0, 0, e^{12}, e^{14} + e^{23}, -e^{15}, e^{25} + e^{13}, e^{28} + e^{17} + e^{35}$             | 2579     |
| 9531:558a | $0, 0, 0, 0, e^{12}a_1, e^{13}, e^{15} + e^{24}, e^{25} + (1 + a_1)e^{14}, e^{17} + e^{28} + e^{45}$  | 2579     |
| 9531:558b | $0, 0, 0, 0, e^{12}a_1, e^{13}, e^{24} - e^{15}, e^{25} + (1 + a_1)e^{14}, e^{17} + e^{28} + e^{45}$  | 2579     |
| 9531:559  | $0, 0, 0, 0, e^{12}, e^{13}, e^{15}, e^{14} + e^{25}, e^{18} + e^{27} + e^{36}$                       | 1479     |
| 9531:560  | $0, 0, 0, 0, e^{12}, e^{13}, e^{25}, e^{24} + e^{15}, e^{36} + e^{17} + e^{28}$                       | 1479     |
| 9531:561  | $0, 0, 0, 0, e^{12}, e^{14} + e^{23}, e^{13} + e^{25}, e^{15} + e^{24}, e^{28} + e^{17}$              | 2479     |
| 9531:562  | $0, 0, 0, 0, e^{12}a_1, e^{13}, e^{15} + e^{23}, e^{14} + e^{25}, e^{18} + e^{34} + e^{27}$           | 2479     |
| 9531:563a | $0, 0, 0, 0, e^{12}, e^{24} + e^{13}, e^{15}, e^{25} + e^{34}, e^{28} + e^{36} + e^{17}$              | 1479     |
| 9531:563b | $0, 0, 0, 0, e^{12}, e^{24} + e^{13}, -e^{15}, e^{34} + e^{25}, e^{17} + e^{28} + e^{36}$             | 1479     |
| 9531:564  | $0, 0, 0, 0, e^{12}, e^{14} + e^{23}, e^{15}, e^{25} + e^{34}, e^{36} + e^{18} + e^{27}$              | 1479     |
| 9531:565  | $0, 0, 0, 0, e^{12}, -e^{13}, e^{15} + e^{23}, e^{34} + e^{25}, e^{18} + e^{27} + e^{46}$             | 1479     |
| 9531:566  | $0, 0, 0, 0, e^{12}, -e^{13}, e^{15} + e^{24}, e^{34} + e^{25}, e^{46} + e^{18} + e^{27}$             | 1479     |
| 9531:567a | $0, 0, 0, 0, e^{12}, e^{34}, e^{15} + e^{23}, e^{13} + e^{25}, e^{28} + e^{36} + e^{17}$              | 1479     |
| 9531:567b | $0, 0, 0, 0, e^{12}, e^{34}, e^{23} - e^{15}, e^{25} + e^{13}, e^{17} + e^{28} + e^{36}$              | 1479     |
| 9531:568a | $0, 0, 0, 0, e^{12}, e^{34}, e^{15} + e^{23}, e^{25} + e^{13}, e^{36} + e^{18} + e^{27}$              | 1479     |
| 9531:568b | $0, 0, 0, 0, e^{12}, e^{34}, e^{23} + e^{15}, e^{25} - e^{13}, e^{27} + e^{36} + e^{18}$              | 1479     |
| 9531:569a | $0, 0, 0, 0, e^{12}, e^{34}, e^{15} + e^{23}, e^{13} + e^{25}, e^{17} + e^{28} + e^{46}$              | 1479     |
| 9531:569b | $0, 0, 0, 0, e^{12}, e^{34}, -e^{15} + e^{23}, e^{13} + e^{25}, e^{28} + e^{46} + e^{17}$             | 1479     |
| 9531:570a | $0, 0, 0, 0, e^{12}, e^{34}, e^{15} + e^{23}, e^{25} + e^{13}, e^{18} + e^{27} + e^{46}$              | 1479     |
| 9531:570b | $0, 0, 0, 0, e^{12}, e^{34}, -e^{23} + e^{15}, e^{25} + e^{13}, e^{46} + e^{27} + e^{18}$             | 1479     |
| 9531:570c | $0, 0, 0, 0, e^{12}, e^{34}, e^{15} - e^{23}, -e^{13} + e^{25}, e^{18} + e^{46} + e^{27}$             | 1479     |
| 9531:571a | $0, 0, 0, 0, e^{12}, e^{34}, e^{23} + e^{15}, e^{25} + e^{14}, e^{18} + e^{27} + e^{36}$              | 1479     |
| 9531:571b | $0, 0, 0, 0, e^{12}, e^{34}, e^{15} + e^{23}, -e^{14} + e^{25}, e^{36} + e^{18} + e^{27}$             | 1479     |
| 9531:572  | $0, 0, 0, 0, e^{12}a_1, e^{24} + e^{13}, e^{23} + e^{15}, e^{25} + e^{14}, e^{34} + e^{27} + e^{18}$  | 2479     |
| 9531:573  | $0, 0, 0, 0, e^{12}, e^{13}, e^{15} + e^{23}, e^{25} + e^{14}, e^{18} + e^{27} + e^{36}$              | 1479     |

Table 2 – Continued to next page

Table 2 – Continued from previous page

| Name      | $\mathfrak{g}$                                                                                                  | UCS Dim. |
|-----------|-----------------------------------------------------------------------------------------------------------------|----------|
| 9531:574a | $0, 0, 0, 0, e^{12}, e^{13}, e^{15} + e^{24}, e^{25} + e^{14}, e^{28} + e^{17} + e^{36}$                        | 1479     |
| 9531:574b | $0, 0, 0, 0, e^{12}, e^{13}, -e^{15} + e^{24}, e^{25} + e^{14}, e^{36} + e^{17} + e^{28}$                       | 1479     |
| 9531:575a | $0, 0, 0, 0, e^{12}, e^{13}, e^{24} + e^{15}, e^{14} + e^{25}, e^{36} + e^{27} + e^{18}$                        | 1479     |
| 9531:575b | $0, 0, 0, 0, e^{12}, e^{13}, e^{15} + e^{24}, e^{25} - e^{14}, e^{18} + e^{27} + e^{36}$                        | 1479     |
| 9531:576a | $0, 0, 0, 0, e^{12}, e^{34}, e^{15}, e^{25} + e^{13}, e^{28} + e^{17} + e^{35} + e^{46}$                        | 1479     |
| 9531:576b | $0, 0, 0, 0, e^{12}, e^{34}, -e^{15}, e^{13} + e^{25}, e^{17} + e^{28} + e^{46} + e^{35}$                       | 1479     |
| 9531:577  | $0, 0, 0, 0, e^{12}, e^{14} - e^{23}, e^{13} + e^{25}, e^{34} + e^{15}, e^{17} + e^{28} + e^{46}$               | 1479     |
| 9531:578a | $0, 0, 0, 0, e^{12}, e^{13}, e^{15}, e^{25} + e^{14}, e^{28} + e^{17} + e^{36} + e^{45}$                        | 1479     |
| 9531:578b | $0, 0, 0, 0, e^{12}, e^{13}, -e^{15}, e^{25} + e^{14}, e^{17} + e^{28} + e^{45} + e^{36}$                       | 1479     |
| 9531:579a | $0, 0, 0, 0, -e^{12}, e^{13}, e^{25}, e^{24} + e^{15}, e^{18} + e^{45} + e^{36} + e^{27}$                       | 1479     |
| 9531:579b | $0, 0, 0, 0, -e^{12}, e^{13}, e^{25}, e^{24} - e^{15}, e^{18} + e^{27} + e^{36} + e^{45}$                       | 1479     |
| 9531:580a | $0, 0, 0, 0, e^{12}a_1, e^{34}, e^{15} + e^{23}, (1 + a_1)e^{13} + e^{25}, e^{28} + e^{17} + e^{35} + e^{46}$   | 1479     |
| 9531:580b | $0, 0, 0, 0, e^{12}a_1, e^{34}, e^{23} - e^{15}, (1 + a_1)e^{13} + e^{25}, e^{46} + e^{35} + e^{28} + e^{17}$   | 1479     |
| 9531:581a | $0, 0, 0, 0, (-1 + a_2)e^{12}, e^{13}, e^{15} + e^{24}, e^{25} + e^{14}a_2, e^{45} + e^{36} + e^{17} + e^{28}$  | 1479     |
| 9531:581b | $0, 0, 0, 0, (-1 + a_2)e^{12}, e^{13}, -e^{15} + e^{24}, e^{25} + e^{14}a_2, e^{17} + e^{28} + e^{45} + e^{36}$ | 1479     |
| 9531:649  | $0, 0, 0, 0, e^{12}, e^{13}, e^{25}, e^{16}, e^{27} + e^{18}$                                                   | 2469     |
| 9531:650  | $0, 0, 0, 0, e^{12}, e^{13}, e^{25}, e^{36}, e^{27} + e^{38}$                                                   | 2469     |
| 9531:651  | $0, 0, 0, 0, e^{12}, e^{13}, e^{25}, e^{16}, e^{18} + e^{27} + e^{34}$                                          | 1469     |
| 9531:652  | $0, 0, 0, 0, e^{12}, e^{13}, e^{25}, e^{36}, e^{14} + e^{38} + e^{27}$                                          | 1469     |
| 9531:653  | $0, 0, 0, 0, e^{12}, e^{13}, e^{15}, e^{16} + e^{25}, e^{27} + e^{18}$                                          | 2469     |
| 9531:654  | $0, 0, 0, 0, e^{12}, e^{13}, e^{25}, e^{35} + e^{26}, e^{37} + e^{28}$                                          | 2469     |
| 9531:655  | $0, 0, 0, 0, e^{12}, e^{13}, e^{15}, e^{36}, e^{25} + e^{38} + e^{17}$                                          | 2469     |
| 9531:656  | $0, 0, 0, 0, e^{12}, e^{13}, e^{25}, e^{36}, e^{38} + e^{27} + e^{15}$                                          | 2469     |
| 9531:657  | $0, 0, 0, 0, -e^{12}, e^{13}, e^{15}, e^{16}, e^{56} + e^{28} + e^{37}$                                         | 2469     |
| 9531:658  | $0, 0, 0, 0, e^{12}, e^{13}, e^{15}, e^{16} + e^{25}, e^{18} + e^{34} + e^{27}$                                 | 1469     |
| 9531:659  | $0, 0, 0, 0, e^{12}, e^{13}, e^{25}, e^{26} + e^{35}, e^{37} + e^{14} + e^{28}$                                 | 1469     |
| 9531:660  | $0, 0, 0, 0, e^{12}, e^{13}, e^{14} + e^{25}, e^{16} + e^{24}, e^{18} + e^{27}$                                 | 1369     |
| 9531:661  | $0, 0, 0, 0, e^{12}, e^{13}, e^{34} + e^{25}, e^{24} + e^{36}, e^{38} + e^{27}$                                 | 1369     |
| 9531:662  | $0, 0, 0, 0, e^{12}, e^{13}, e^{15} + e^{23}, e^{25} + e^{16}, e^{18} + e^{27}$                                 | 2469     |
| 9531:663a | $0, 0, 0, 0, e^{12}, e^{13}, e^{26} + e^{35}, e^{36} + e^{25}, e^{38} + e^{27}$                                 | 2469     |
| 9531:663b | $0, 0, 0, 0, -e^{12}, e^{13}, e^{35} - e^{26}, e^{36} + e^{25}, e^{38} + e^{27}$                                | 2469     |
| 9531:664  | $0, 0, 0, 0, -e^{12}, e^{13}, e^{25}, e^{16} + e^{23}, e^{27} + e^{18} + e^{35}$                                | 2469     |
| 9531:665  | $0, 0, 0, 0, -e^{12}, e^{13}, e^{15}, e^{16}, e^{28} + e^{14} + e^{37} + e^{56}$                                | 1469     |
| 9531:666  | $0, 0, 0, 0, -e^{12}, e^{13}, e^{25}, e^{24} + e^{16}, e^{18} + e^{45} + e^{27}$                                | 1369     |
| 9531:667  | $0, 0, 0, 0, e^{12}, e^{13}, e^{25} + e^{14}, e^{16}, e^{45} + e^{18} + e^{27}$                                 | 1369     |
| 9531:668  | $0, 0, 0, 0, -e^{12}, e^{13}, e^{15} + e^{24}, e^{36}, e^{17} + e^{38} + e^{45}$                                | 1369     |
| 9531:669  | $0, 0, 0, 0, e^{12}, e^{13}, e^{25} + e^{14}, e^{36}, e^{45} + e^{38} + e^{27}$                                 | 1369     |
| 9531:670  | $0, 0, 0, 0, e^{12}, e^{13}, e^{25}, e^{35} + e^{26}, e^{37} + e^{15} + e^{28}$                                 | 2469     |
| 9531:671  | $0, 0, 0, 0, e^{12}, e^{13}, e^{15}, e^{16} + e^{25}, e^{27} + e^{18} + e^{36}$                                 | 2469     |
| 9531:672  | $0, 0, 0, 0, e^{12}, e^{13}, e^{25}, e^{35} + e^{26}, e^{37} + e^{28} + e^{16}$                                 | 2469     |
| 9531:673  | $0, 0, 0, 0, -e^{12}, e^{13}, e^{15}, e^{16} + e^{23}, e^{28} + e^{37} + e^{56}$                                | 2469     |
| 9531:674  | $0, 0, 0, 0, e^{12}, e^{13}, e^{15} + e^{24}, e^{25} + e^{16}, e^{18} + e^{27}$                                 | 1369     |
| 9531:675  | $0, 0, 0, 0, e^{12}, e^{13}, e^{25} + e^{34}, e^{35} + e^{26}, e^{37} + e^{28}$                                 | 1369     |
| 9531:676  | $0, 0, 0, 0, -e^{12}, e^{13}, e^{15}, e^{16} + e^{25}, e^{28} + e^{37} + e^{56}$                                | 2469     |
| 9531:678  | $0, 0, 0, 0, e^{12}, e^{13}, 2e^{15}, e^{26} + e^{35}, e^{18} + e^{37} + e^{56}$                                | 2469     |
| 9531:679  | $0, 0, 0, 0, e^{12}, e^{13}, e^{25} + e^{14}, e^{16} + e^{24}, e^{27} + e^{18} + e^{34}$                        | 1369     |
| 9531:680  | $0, 0, 0, 0, e^{12}, e^{13}, e^{25} + e^{34}, e^{24} + e^{36}, e^{27} + e^{14} + e^{38}$                        | 1369     |
| 9531:681  | $0, 0, 0, 0, -e^{12}, e^{13}, e^{15}, e^{24} + e^{16}, e^{28} + e^{56} + e^{37}$                                | 1369     |
| 9531:682  | $0, 0, 0, 0, e^{12}, e^{13}, e^{15} + e^{23}, e^{16} + e^{25}, e^{27} + e^{18} + e^{34}$                        | 1469     |
| 9531:683  | $0, 0, 0, 0, e^{12}a_1, e^{13}, e^{25} + e^{14}(1 + a_1), e^{16} + e^{24}, e^{18} + e^{27} + e^{45}$            | 1369     |
| 9531:684a | $0, 0, 0, 0, e^{12}, e^{13}, e^{35} + e^{26}, e^{36} + e^{25}, e^{27} + e^{38} + e^{14}$                        | 1469     |
| 9531:684b | $0, 0, 0, 0, -e^{12}, e^{13}, e^{35} - e^{26}, e^{25} + e^{36}, e^{38} + e^{27} + e^{14}$                       | 1469     |
| 9531:685  | $0, 0, 0, 0, -e^{12}, e^{13}, e^{15}, e^{16} + e^{23}, e^{28} + e^{37} + e^{56} + e^{14}$                       | 1469     |
| 9531:686  | $0, 0, 0, 0, e^{12}, e^{13}, e^{34} + e^{15}, e^{36} + e^{14}, e^{38} + e^{17} + e^{25}$                        | 1369     |
| 9531:687  | $0, 0, 0, 0, e^{12}, e^{13}, e^{25} + e^{34}, e^{24} + e^{36}, e^{38} + e^{15} + e^{27}$                        | 1369     |
| 9531:688  | $0, 0, 0, 0, e^{12}, e^{13}, e^{15} + e^{24}, e^{25} + e^{16}, e^{18} + e^{27} + e^{34}$                        | 1369     |
| 9531:689  | $0, 0, 0, 0, e^{12}, e^{13}, e^{25} + e^{34}, e^{26} + e^{35}, e^{28} + e^{37} + e^{14}$                        | 1369     |
| 9531:690  | $0, 0, 0, 0, a_1e^{12}, e^{13}, e^{23} + e^{15}, e^{16} + e^{25}, e^{36} + e^{27} + e^{18}$                     | 2469     |

Table 2 – Continued to next page



Table 2 – Continued from previous page

| Name      | $\mathfrak{g}$                                                                                                   | UCS Dim. |
|-----------|------------------------------------------------------------------------------------------------------------------|----------|
| 9531:691  | $0, 0, 0, 0, -e^{12}, e^{13}, e^{15}, e^{16} + e^{25}, e^{56} + e^{28} + e^{14} + e^{37}$                        | 1469     |
| 9531:692  | $0, 0, 0, 0, e^{12}, e^{13}, 2e^{15}, e^{35} + e^{26}, e^{56} + e^{24} + e^{37} + e^{18}$                        | 1469     |
| 9531:694  | $0, 0, 0, 0, -e^{12}, e^{13}, e^{15} + e^{24}, e^{16} + e^{34}, e^{56} + e^{28} + e^{37}$                        | 1369     |
| 9531:695a | $0, 0, 0, 0, -e^{12}, e^{13}, e^{15} + e^{34}, e^{16} + e^{24}, e^{28} + e^{37} + e^{56}$                        | 1369     |
| 9531:695b | $0, 0, 0, 0, -e^{12}, e^{13}, e^{15} + e^{34}, e^{16} - e^{24}, e^{28} + e^{37} + e^{56}$                        | 1369     |
| 9531:696  | $0, 0, 0, 0, e^{12}, e^{13}, e^{25}, e^{35} + e^{14} + e^{26}, e^{37} + e^{45} + e^{28}$                         | 1369     |
| 9531:697  | $0, 0, 0, 0, e^{12}, -e^{13}, e^{15}, e^{25} + e^{34} + e^{16}, e^{27} + e^{18} + e^{46}$                        | 1369     |
| 9531:698  | $0, 0, 0, 0, e^{12}, e^{13}, e^{25} + e^{14}, e^{26} + e^{35}, e^{28} + e^{37} + e^{46}$                         | 1369     |
| 9531:699a | $0, 0, 0, 0, e^{12}, e^{13}, e^{26} + e^{35}, e^{25} + e^{36}, e^{15} + e^{27} + e^{38}$                         | 2469     |
| 9531:699b | $0, 0, 0, 0, -e^{12}, e^{13}, -e^{26} + e^{35}, e^{36} + e^{25}, e^{27} + e^{15} + e^{38}$                       | 2469     |
| 9531:700a | $0, 0, 0, 0, e^{12}, e^{13}, e^{26} + e^{35}, e^{25} + e^{36}, e^{15} + e^{28} + e^{37}$                         | 2469     |
| 9531:700b | $0, 0, 0, 0, e^{12}, e^{13}, e^{35} + e^{26}, e^{36} - e^{25}, e^{37} + e^{15} + e^{28}$                         | 2469     |
| 9531:701  | $0, 0, 0, 0, -e^{12}, e^{13}, e^{15} + e^{23}, e^{16} + e^{25}, e^{28} + e^{37} + e^{56}$                        | 2469     |
| 9531:702  | $0, 0, 0, 0, e^{12}, e^{13}, e^{23} + 2e^{15}, e^{35} + e^{26}, e^{56} + e^{37} + e^{18}$                        | 2469     |
| 9531:703  | $0, 0, 0, 0, -e^{12}, -e^{13}, 2e^{16} + e^{25}, e^{26} + e^{35}, e^{18} + e^{27} + e^{56}$                      | 2469     |
| 9531:704  | $0, 0, 0, 0, -e^{12}, e^{13}, e^{25} + e^{16}, e^{36} + e^{15}, e^{27} + e^{56} + e^{38}$                        | 2469     |
| 9531:705  | $0, 0, 0, 0, -e^{12}, e^{13}, e^{15}, e^{16} + e^{24}, e^{56} + e^{28} + e^{37} + e^{14}$                        | 1369     |
| 9531:706  | $0, 0, 0, 0, -e^{12}, e^{13}, e^{25}, e^{24} + e^{16}, e^{36} + e^{45} + e^{27} + e^{18}$                        | 1369     |
| 9531:707  | $0, 0, 0, 0, e^{12}, e^{13}, e^{15}, e^{36} + e^{14}, e^{38} + e^{46} + e^{25} + e^{17}$                         | 1369     |
| 9531:708  | $0, 0, 0, 0, e^{12}, e^{13}, e^{25}, e^{36} + e^{14}, e^{26} + e^{27} + e^{46} + e^{15}$                         | 1369     |
| 9531:709  | $0, 0, 0, 0, e^{12}, e^{13}, e^{25} + e^{34}, e^{26} + e^{35}, e^{28} + e^{15} + e^{37}$                         | 1369     |
| 9531:710  | $0, 0, 0, 0, e^{12}, e^{13}, e^{24} + e^{15}, e^{25} + e^{16}, e^{36} + e^{27} + e^{18}$                         | 1369     |
| 9531:711  | $0, 0, 0, 0, e^{12}, e^{13}, e^{34} + e^{25}, e^{26} + e^{35}, e^{28} + e^{37} + e^{16}$                         | 1369     |
| 9531:712  | $0, 0, 0, 0, -e^{12}, e^{13}, e^{23} + e^{15}, e^{24} + e^{16}, e^{37} + e^{28} + e^{56}$                        | 1369     |
| 9531:714  | $0, 0, 0, 0, e^{12}, e^{13}, 2e^{15}, e^{35} + e^{26} + e^{14}, e^{56} + e^{37} + e^{18}$                        | 1369     |
| 9531:715  | $0, 0, 0, 0, -e^{12}, e^{13}, e^{15} + e^{34}, e^{16} + e^{25}, e^{37} + e^{28} + e^{56}$                        | 1369     |
| 9531:716  | $0, 0, 0, 0, e^{12}, e^{13}, e^{34} + 2e^{15}, e^{26} + e^{35}, e^{18} + e^{37} + e^{56}$                        | 1369     |
| 9531:717  | $0, 0, 0, 0, e^{12}, e^{13}, e^{34} + e^{25}, e^{14} + e^{26} + e^{35}, e^{28} + e^{37} + e^{45}$                | 1369     |
| 9531:718  | $0, 0, 0, 0, a_1 e^{12}, -e^{13}, e^{15} + e^{24}, e^{16} + e^{25} + e^{34}, e^{46} + e^{18} + e^{27}$           | 1369     |
| 9531:719  | $0, 0, 0, 0, (-1 + a_2) e^{12}, e^{13}, a_2 e^{14} + e^{25}, e^{16} + e^{24}, e^{27} + e^{36} + e^{45} + e^{18}$ | 1369     |
| 9531:720  | $0, 0, 0, 0, -e^{12}, e^{13}, e^{24} + e^{15}, e^{16} + e^{34}, e^{37} + e^{14} + e^{28} + e^{56}$               | 1369     |
| 9531:721a | $0, 0, 0, 0, -e^{12}, e^{13}, e^{15} + e^{34}, e^{16} + e^{24}, e^{28} + e^{14} + e^{37} + e^{56}$               | 1369     |
| 9531:721b | $0, 0, 0, 0, -e^{12}, e^{13}, e^{34} + e^{15}, -e^{24} + e^{16}, e^{37} + e^{14} + e^{28} + e^{56}$              | 1369     |
| 9531:722  | $0, 0, 0, 0, -e^{12}, e^{13}, e^{15} + e^{23}, e^{16} + e^{25}, e^{28} + e^{37} + e^{14} + e^{56}$               | 1469     |
| 9531:723  | $0, 0, 0, 0, e^{12}, e^{13}, e^{23} + 2e^{15}, e^{35} + e^{26}, e^{24} + e^{56} + e^{37} + e^{18}$               | 1469     |
| 9531:724  | $0, 0, 0, 0, e^{12}, -e^{13}, e^{23} + e^{15}, e^{16} + e^{25} + e^{34}, e^{46} + e^{27} + e^{18}$               | 1369     |
| 9531:725  | $0, 0, 0, 0, -e^{12}, e^{13}, e^{16} + e^{25}, e^{15} + e^{36}, e^{27} + e^{38} + e^{14} + e^{56}$               | 1469     |
| 9531:726  | $0, 0, 0, 0, -e^{12}, -e^{13}, e^{25} + 2e^{16}, e^{26} + e^{35}, e^{18} + e^{56} + e^{34} + e^{27}$             | 1469     |
| 9531:727  | $0, 0, 0, 0, -e^{12}, e^{13}, e^{24} + e^{15}, e^{34} + e^{25} + e^{16}, e^{56} + e^{28} + e^{37}$               | 1369     |
| 9531:728a | $0, 0, 0, 0, e^{12}, e^{13}, e^{34} + 2e^{15}, e^{35} + e^{14} + e^{26}, e^{37} + e^{56} + e^{18}$               | 1369     |
| 9531:728b | $0, 0, 0, 0, e^{12}, e^{13}, e^{34} + 2e^{15}, e^{35} - e^{14} + e^{26}, e^{37} + e^{56} + e^{18}$               | 1369     |
| 9531:729a | $0, 0, 0, 0, e^{12}, e^{13}, e^{25} + e^{36}, e^{14} + e^{26} + e^{35}, e^{28} + e^{45} + e^{37}$                | 1369     |
| 9531:729b | $0, 0, 0, 0, e^{12}, -e^{13}, e^{36} + e^{25}, e^{35} + e^{14} - e^{26}, e^{28} + e^{37} + e^{45}$               | 1369     |
| 9531:730a | $0, 0, 0, 0, e^{12}, e^{13}, e^{26} + e^{35}, e^{25} + e^{14} + e^{36}, e^{28} + e^{45} + e^{37}$                | 1369     |
| 9531:730b | $0, 0, 0, 0, e^{12}, e^{13}, e^{35} + e^{26}, e^{36} - e^{25} + e^{14}, e^{45} + e^{37} + e^{28}$                | 1369     |
| 9531:731  | $0, 0, 0, 0, -e^{12}, e^{13}, e^{15} + e^{23}, e^{16} + e^{24}, e^{14} + e^{56} + e^{28} + e^{37}$               | 1369     |
| 9531:732  | $0, 0, 0, 0, e^{12}, e^{13}, 2e^{15}, e^{14} + e^{26} + e^{35}, e^{37} + e^{24} + e^{56} + e^{18}$               | 1369     |
| 9531:733  | $0, 0, 0, 0, e^{12}, e^{13}, e^{25}, e^{35} + e^{14} + e^{26}, e^{28} + e^{37} + e^{45} + e^{16}$                | 1369     |
| 9531:735  | $0, 0, 0, 0, e^{12}, e^{13}, e^{25} + e^{14}, e^{35} + e^{26}, e^{46} + e^{37} + e^{28} + e^{15}$                | 1369     |
| 9531:736  | $0, 0, 0, 0, -e^{12}, e^{13}, e^{15} + e^{34}, e^{16} + e^{25}, e^{14} + e^{56} + e^{28} + e^{37}$               | 1369     |
| 9531:737  | $0, 0, 0, 0, e^{12}, e^{13}, 2e^{15} + e^{34}, e^{26} + e^{35}, e^{37} + e^{24} + e^{56} + e^{18}$               | 1369     |
| 9531:738  | $0, 0, 0, 0, e^{12}, e^{13}, 2e^{15} + e^{23}, e^{35} + e^{14} + e^{26}, e^{18} + e^{37} + e^{56}$               | 1369     |
| 9531:739  | $0, 0, 0, 0, -e^{12}, -e^{13}, 2e^{16} + e^{25}, e^{14} + e^{26} + e^{35}, e^{18} + e^{27} + e^{56}$             | 1369     |
| 9531:740  | $0, 0, 0, 0, -e^{12}, e^{13}, e^{15} + e^{24}, e^{34} + e^{16} + e^{25}, e^{14} + e^{28} + e^{37} + e^{56}$      | 1369     |
| 9531:741a | $0, 0, 0, 0, e^{12}, e^{13}, 2e^{15} + e^{34}, e^{14} + e^{26} + e^{35}, e^{37} + e^{24} + e^{56} + e^{18}$      | 1369     |
| 9531:741b | $0, 0, 0, 0, e^{12}, e^{13}, e^{34} + 2e^{15}, e^{35} - e^{14} + e^{26}, e^{18} + e^{37} + e^{56} + e^{24}$      | 1369     |
| 9531:742  | $0, 0, 0, 0, e^{12}, e^{13}, e^{25} + e^{34}, e^{14} + e^{26} + e^{35}, e^{37} + e^{16} + e^{45} + e^{28}$       | 1369     |
| 9531:743  | $0, 0, 0, 0, -e^{12}, e^{13}, e^{34} + e^{16} + e^{25}, e^{15} + e^{36} + e^{24}, e^{38} + e^{27} + e^{56}$      | 1369     |

Table 2 – Continued to next page

Table 2 – Continued from previous page

| Name         | $\mathfrak{g}$                                                                                                                                               | UCS Dim. |
|--------------|--------------------------------------------------------------------------------------------------------------------------------------------------------------|----------|
| 9531:744     | $0, 0, 0, 0, e^{12}, e^{13}, e^{23} + 2e^{15}, e^{35} + e^{14} + e^{26}, e^{24} + e^{37} + e^{18} + e^{56}$                                                  | 1369     |
| 9531:745     | $0, 0, 0, 0, -e^{12}, -e^{13}, 2e^{16} + e^{25}, e^{14} + e^{26} + e^{35}, e^{27} + e^{56} + e^{18} + e^{34}$                                                | 1369     |
| 9531:746a    | $0, 0, 0, 0, e^{12}, e^{13}, e^{36} + e^{25}, e^{35} + e^{14} + e^{26}, e^{38} + e^{46} + e^{15} + e^{27}$                                                   | 1369     |
| 9531:746b    | $0, 0, 0, 0, e^{12}, e^{13}, e^{36} - e^{25}, e^{35} + e^{14} + e^{26}, e^{38} + e^{46} + e^{15} + e^{27}$                                                   | 1369     |
| 9531:747a    | $0, 0, 0, 0, e^{12}, e^{13}, e^{35} + e^{26}, e^{36} + e^{14} + e^{25}, e^{38} + e^{46} + e^{15} + e^{27}$                                                   | 1369     |
| 9531:747b    | $0, 0, 0, 0, -e^{12}, e^{13}, e^{35} - e^{26}, e^{36} + e^{25} + e^{14}, e^{27} + e^{38} + e^{46} + e^{15}$                                                  | 1369     |
| 9531:748     | $0, 0, 0, 0, -e^{12}, e^{13}, e^{25} + e^{34} + e^{16}, e^{24} + e^{36} + e^{15}, e^{38} + e^{56} + e^{27} + e^{14}$                                         | 1369     |
| 9531:749     | $0, 0, 0, 0, e^{12}, e^{34}, e^{15}, e^{36}, e^{38} + e^{17}$                                                                                                | 1359     |
| 9531:750     | $0, 0, 0, 0, e^{12}, e^{34}, e^{15}, e^{36}, e^{17} + e^{24} + e^{38}$                                                                                       | 1359     |
| 9531:751     | $0, 0, 0, 0, e^{12}, e^{34}, e^{15}, e^{36}, e^{38} + e^{17} + e^{25}$                                                                                       | 1359     |
| 9531:752     | $0, 0, 0, 0, -e^{12}, e^{14} + e^{23}, e^{15}, e^{35} + e^{16}, e^{18} + e^{37}$                                                                             | 1359     |
| 9531:753     | $0, 0, 0, 0, -e^{12}, e^{34}, e^{15} + e^{23}, e^{46}, e^{35} + e^{48} + e^{17}$                                                                             | 1359     |
| 9531:754     | $0, 0, 0, 0, e^{12}, e^{34}, e^{15}, e^{36}, e^{17} + e^{46} + e^{25} + e^{38}$                                                                              | 1359     |
| 9531:755     | $0, 0, 0, 0, -e^{12}, e^{14} + e^{23}, e^{34} + e^{15}, e^{35} + e^{16}, e^{18} + e^{37}$                                                                    | 1359     |
| 9531:756     | $0, 0, 0, 0, -e^{12}, e^{14} + e^{23}, e^{15}, e^{16} + e^{35}, e^{24} + e^{37} + e^{18}$                                                                    | 1359     |
| 9531:757     | $0, 0, 0, 0, -e^{12}, e^{14} + e^{23}, e^{15}, e^{35} + e^{16}, e^{25} + e^{37} + e^{18}$                                                                    | 1359     |
| 9531:759a    | $0, 0, 0, 0, e^{23} + e^{14}, e^{24} + e^{13}, e^{16} + e^{25}, e^{15} + e^{26}, e^{28} + e^{17}$                                                            | 1359     |
| 9531:759b    | $0, 0, 0, 0, -e^{14} + e^{23}, e^{24} + e^{13}, -e^{16} + e^{25}, e^{15} + e^{26}, e^{28} + e^{17}$                                                          | 1359     |
| 9531:760     | $0, 0, 0, 0, -e^{12}, e^{14} + e^{23}, e^{34} + e^{15}, e^{35} + e^{16}, e^{18} + e^{24} + e^{37}$                                                           | 1359     |
| 9531:761     | $0, 0, 0, 0, -e^{12}, e^{24} + e^{13}, e^{15}, e^{16} + e^{23} + e^{45}, e^{18} + e^{35} + e^{47}$                                                           | 1359     |
| 9531:762     | $0, 0, 0, 0, -e^{12}, e^{14} + e^{23}, e^{15} + e^{34}, e^{16} + e^{35}, e^{25} + e^{37} + e^{18}$                                                           | 1359     |
| 9531:763     | $0, 0, 0, 0, -e^{12}, e^{14} + e^{23}, e^{15}, e^{24} + e^{35} + e^{16}, e^{18} + e^{37} + e^{26}$                                                           | 1359     |
| 9531:764     | $0, 0, 0, 0, -e^{12}, e^{24} + e^{13}, e^{15} + e^{23}, e^{16} + e^{45}, e^{36} + e^{18} + e^{47}$                                                           | 1359     |
| 9531:770     | $0, 0, 0, 0, -e^{12}, -e^{14} + e^{23}, e^{15}, e^{16} + e^{35}, e^{45} + e^{37} + e^{18} + e^{26}$                                                          | 1359     |
| 9531:771     | $0, 0, 0, 0, -e^{12}, e^{13} + e^{24}, e^{15} + e^{34}, e^{45} + e^{23} + e^{16}, e^{47} + e^{18} + e^{35}$                                                  | 1359     |
| 9531:772a    | $0, 0, 0, 0, e^{14} + e^{23}, e^{13} + e^{24}, e^{25} + e^{34}, e^{16} + e^{26} + e^{15}, e^{17} + e^{34} + e^{28}$                                          | 1359     |
| 9531:772b    | $0, 0, 0, 0, -e^{14} + e^{23}, e^{13} + e^{24}, -e^{16} + e^{25}, e^{26} + e^{15}, e^{28} + e^{34} + e^{17}$                                                 | 1359     |
| 9531:773     | $0, 0, 0, 0, -e^{12}, e^{23} + e^{14}, e^{34} + e^{15}, e^{35} + e^{24} + e^{16}, e^{26} + e^{37} + e^{18}$                                                  | 1359     |
| 9531:778     | $0, 0, 0, 0, -e^{12}a_1, -(1 + a_1)e^{13} + e^{24}, e^{15}, e^{16}a_1 + e^{23} + e^{45}, e^{18} + e^{26} + e^{35} + e^{47}$                                  | 1359     |
| 9531:780a    | $0, 0, 0, 0, -e^{12}, e^{24} + e^{13}, e^{15} + e^{23}, e^{16} + e^{45}, e^{36} + e^{25} + e^{18} + e^{47}$                                                  | 1359     |
| 9531:780b    | $0, 0, 0, 0, -e^{12}, e^{24} - e^{13}, e^{15} + e^{23}, e^{45} + e^{16}, e^{47} + e^{36} + e^{25} + e^{18}$                                                  | 1359     |
| 9531:782     | $0, 0, 0, 0, -e^{12}, e^{23} - e^{14}, e^{34} + e^{15}, e^{35} + e^{16}, e^{26} + e^{37} + e^{45} + e^{18}$                                                  | 1359     |
| 9531:784a    | $0, 0, 0, 0, e^{14} + e^{23}, e^{13} + e^{24}, e^{26} + e^{15}, e^{34} + e^{25} + e^{16}, e^{35} + e^{18} + e^{27}$                                          | 1359     |
| 9531:784b    | $0, 0, 0, 0, e^{14} + e^{23}, e^{13} - e^{24}, e^{26} + e^{15}, e^{34} + e^{25} - e^{16}, e^{35} + e^{18} + e^{27}$                                          | 1359     |
| 9531:785a    | $0, 0, 0, 0, e^{13} + e^{24}, e^{14} + e^{23}, e^{26} + e^{15}, e^{34} + e^{25} + e^{16}, e^{35} + e^{17} + e^{28}$                                          | 1359     |
| 9531:785b    | $0, 0, 0, 0, e^{24} + e^{13}, e^{23} - e^{14}, -e^{15} + e^{26}, e^{16} + e^{25} + e^{34}, e^{35} + e^{28} + e^{17}$                                         | 1359     |
| 9531:789     | $0, 0, 0, 0, (-1 + a_2)e^{12}, e^{13}a_2 + e^{24}, e^{15} + e^{34}, e^{23} + e^{45} - (-1 + a_2)e^{16}, e^{18} + e^{26} + e^{35} + e^{47}$                   | 1359     |
| 9531:792a    | $0, 0, 0, 0, e^{23} + e^{14}, e^{24} + e^{13}, e^{16} + e^{25}, e^{15} + e^{26}, e^{28} + e^{17} + e^{35} + e^{46}$                                          | 1359     |
| 9531:792b    | $0, 0, 0, 0, -e^{14} - e^{23}, -e^{13} + e^{24}, -e^{16} + e^{25}, e^{15} + e^{26}, e^{17} + e^{46} + e^{35} + e^{28}$                                       | 1359     |
| 9531:795a(*) | $0, 0, 0, 0, (-1 + a_5)e^{23} + a_5e^{14}, e^{13} + a_5e^{24}, \frac{1}{a_5-1}e^{15} + e^{26}, e^{34} + e^{25} + e^{16}, e^{45} + e^{36} + e^{17} + e^{28}$  | 1359     |
| 9531:795b(*) | $0, 0, 0, 0, (-1 + a_5)e^{23} + a_5e^{14}, -e^{13} + a_5e^{24}, \frac{1}{1-a_5}e^{15} + e^{26}, e^{34} + e^{25} + e^{16}, e^{45} + e^{36} + e^{17} + e^{28}$ | 1359     |
| Type: 4311   |                                                                                                                                                              |          |
| 9521:1       | $0, 0, 0, 0, e^{12}, e^{13}, e^{34}, e^{15}, e^{18}$                                                                                                         | 3679     |
| 9521:2       | $0, 0, 0, 0, e^{12}, e^{13}, e^{34}, e^{25}, e^{28}$                                                                                                         | 3679     |
| 9521:3       | $0, 0, 0, 0, e^{12}, e^{13}, e^{23}, e^{15}, e^{18}$                                                                                                         | 4679     |
| 9521:4       | $0, 0, 0, 0, e^{12}, e^{13}, e^{14}, e^{15}, e^{18}$                                                                                                         | 3679     |
| 9521:5       | $0, 0, 0, 0, e^{12}, e^{13}, e^{14}, e^{25}, e^{28}$                                                                                                         | 3679     |
| 9521:6       | $0, 0, 0, 0, e^{12}, e^{13}, e^{24}, e^{15}, e^{18}$                                                                                                         | 3679     |
| 9521:7       | $0, 0, 0, 0, e^{12}, e^{34}, e^{24} + e^{13}, e^{15}, e^{18}$                                                                                                | 3679     |
| 9521:8       | $0, 0, 0, 0, e^{12}, e^{13}, e^{23}, e^{15}, e^{18} + e^{34}$                                                                                                | 3679     |
| 9521:9       | $0, 0, 0, 0, e^{12}, e^{13}, e^{14} + e^{23}, e^{15}, e^{18}$                                                                                                | 3679     |
| 9521:10      | $0, 0, 0, 0, e^{12}, e^{13}, e^{14} + e^{23}, e^{25}, e^{28}$                                                                                                | 3679     |
| 9521:11      | $0, 0, 0, 0, e^{12}, e^{13}, e^{34}, e^{15}, e^{23} + e^{18}$                                                                                                | 3679     |
| 9521:12      | $0, 0, 0, 0, e^{12}, e^{13}, e^{14}, e^{15}, e^{18} + e^{34}$                                                                                                | 3679     |
| 9521:13      | $0, 0, 0, 0, e^{12}, e^{13}, e^{14}, e^{25}, e^{34} + e^{28}$                                                                                                | 3679     |
| 9521:14      | $0, 0, 0, 0, e^{12}, e^{13}, e^{24}, e^{15}, e^{18} + e^{34}$                                                                                                | 3679     |
| 9521:15      | $0, 0, 0, 0, e^{12}, e^{13}, e^{34}, e^{15}, e^{18} + e^{24}$                                                                                                | 3679     |

Table 2 – Continued to next page

Table 2 – Continued from previous page

| Name     | $\mathfrak{g}$                                                                    | UCS Dim. |
|----------|-----------------------------------------------------------------------------------|----------|
| 9521:16  | $0, 0, 0, 0, e^{12}, e^{13}, e^{34}, e^{25}, e^{28} + e^{14}$                     | 3679     |
| 9521:17  | $0, 0, 0, 0, e^{12}, e^{13}, e^{23}, e^{15}, e^{18} + e^{24}$                     | 3679     |
| 9521:18  | $0, 0, 0, 0, e^{12}, e^{13}, e^{14}, e^{15}, e^{23} + e^{18}$                     | 3679     |
| 9521:19  | $0, 0, 0, 0, e^{12}, e^{13}, e^{24}, e^{15}, e^{23} + e^{18}$                     | 3679     |
| 9521:20a | $0, 0, 0, 0, e^{12}, e^{13}, e^{14} + e^{23}, e^{15}, e^{34} + e^{18}$            | 3679     |
| 9521:20b | $0, 0, 0, 0, -e^{12}, e^{13}, e^{14} + e^{23}, e^{15}, e^{18} + e^{34}$           | 3679     |
| 9521:21a | $0, 0, 0, 0, e^{12}, e^{13}, e^{14} + e^{23}, e^{25}, e^{28} + e^{34}$            | 3679     |
| 9521:21b | $0, 0, 0, 0, -e^{12}, e^{13}, e^{23} + e^{14}, e^{25}, e^{28} + e^{34}$           | 3679     |
| 9521:22a | $0, 0, 0, 0, e^{12}, e^{14} + e^{23}, e^{24} + e^{13}, e^{15}, e^{18}$            | 3679     |
| 9521:22b | $0, 0, 0, 0, e^{12}, -e^{14} + e^{23}, e^{13} + e^{24}, e^{15}, e^{18}$           | 3679     |
| 9521:23  | $0, 0, 0, 0, e^{12}, e^{34}, e^{24} + e^{13}, e^{15}, e^{23} + e^{18}$            | 3679     |
| 9521:24  | $0, 0, 0, 0, e^{12}, e^{13}, e^{34}, e^{15}, e^{25} + e^{18}$                     | 3679     |
| 9521:25  | $0, 0, 0, 0, e^{12}, e^{13}, e^{34}, e^{25}, e^{28} + e^{15}$                     | 3679     |
| 9521:26  | $0, 0, 0, 0, e^{12}, e^{13}, e^{14} + e^{23}, e^{15}, e^{24} + e^{18}$            | 3679     |
| 9521:27a | $0, 0, 0, 0, e^{12}, e^{23} + e^{14}, e^{24} + e^{13}, e^{15}, e^{18} + e^{34}$   | 3679     |
| 9521:27b | $0, 0, 0, 0, e^{12}, e^{23} - e^{14}, e^{24} + e^{13}, e^{15}, e^{18} + e^{34}$   | 3679     |
| 9521:27c | $0, 0, 0, 0, -e^{12}, -e^{14} + e^{23}, e^{24} + e^{13}, e^{15}, e^{18} + e^{34}$ | 3679     |
| 9521:28  | $0, 0, 0, 0, e^{12}, e^{13}, e^{23}, e^{15}, e^{18} + e^{25}$                     | 4679     |
| 9521:29  | $0, 0, 0, 0, e^{12}, e^{13}, e^{14}, e^{15}, e^{25} + e^{18}$                     | 3679     |
| 9521:30  | $0, 0, 0, 0, e^{12}, e^{13}, e^{14}, e^{25}, e^{15} + e^{28}$                     | 3679     |
| 9521:31  | $0, 0, 0, 0, e^{12}, e^{13}, e^{24}, e^{15}, e^{25} + e^{18}$                     | 3679     |
| 9521:32  | $0, 0, 0, 0, e^{12}, e^{34}, e^{13} + e^{24}, e^{15}, e^{18} + e^{25}$            | 3679     |
| 9521:33  | $0, 0, 0, 0, e^{12}, e^{13}, e^{34}, e^{15}, e^{36} + e^{18}$                     | 2579     |
| 9521:34  | $0, 0, 0, 0, e^{12}, e^{13}, e^{34}, e^{25}, e^{28} + e^{36}$                     | 2579     |
| 9521:35  | $0, 0, 0, 0, e^{12}, e^{13}, e^{23}, e^{15}, e^{25} + e^{18} + e^{34}$            | 3679     |
| 9521:36  | $0, 0, 0, 0, e^{12}, e^{13}, e^{14} + e^{23}, e^{15}, e^{18} + e^{25}$            | 3679     |
| 9521:37  | $0, 0, 0, 0, e^{12}, e^{13}, e^{14} + e^{23}, e^{25}, e^{15} + e^{28}$            | 3679     |
| 9521:38  | $0, 0, 0, 0, e^{12}, e^{13}, e^{14}, e^{15}, e^{25} + e^{18} + e^{34}$            | 3679     |
| 9521:39  | $0, 0, 0, 0, e^{12}, e^{13}, e^{14}, e^{25}, e^{28} + e^{34} + e^{15}$            | 3679     |
| 9521:40  | $0, 0, 0, 0, e^{12}, e^{13}, e^{24}, e^{15}, e^{25} + e^{18} + e^{34}$            | 3679     |
| 9521:41  | $0, 0, 0, 0, e^{12}, e^{13}, e^{23}, e^{15}, e^{18} + e^{36}$                     | 3579     |
| 9521:42  | $0, 0, 0, 0, e^{12}, e^{13}, e^{23}, e^{25}, e^{28} + e^{36}$                     | 3579     |
| 9521:43  | $0, 0, 0, 0, e^{12}, e^{13}, e^{14}, e^{15}, e^{36} + e^{18}$                     | 2579     |
| 9521:44  | $0, 0, 0, 0, e^{12}, e^{13}, e^{14}, e^{25}, e^{28} + e^{36}$                     | 2579     |
| 9521:45  | $0, 0, 0, 0, e^{12}, e^{13}, e^{24}, e^{15}, e^{18} + e^{36}$                     | 2579     |
| 9521:46  | $0, 0, 0, 0, e^{12}, e^{13}, e^{24}, e^{25}, e^{36} + e^{28}$                     | 2579     |
| 9521:47  | $0, 0, 0, 0, e^{12}, e^{13}, e^{34}, e^{25}, e^{16} + e^{28}$                     | 2579     |
| 9521:48  | $0, 0, 0, 0, -e^{12}, e^{13}, e^{34}, e^{15} + e^{24}, e^{45} + e^{18}$           | 3579     |
| 9521:49  | $0, 0, 0, 0, e^{12}, e^{13}, e^{34}, e^{25} + e^{14}, e^{28} + e^{45}$            | 3579     |
| 9521:50  | $0, 0, 0, 0, -e^{12}, e^{13}, e^{34}, e^{23} + e^{15}, e^{35} + e^{18}$           | 3579     |
| 9521:51  | $0, 0, 0, 0, e^{12}, e^{13}, e^{23}, e^{25}, e^{16} + e^{28}$                     | 3579     |
| 9521:52  | $0, 0, 0, 0, e^{12}, e^{13}, e^{14}, e^{25}, e^{28} + e^{16}$                     | 2579     |
| 9521:53  | $0, 0, 0, 0, e^{12}, e^{13}, e^{24}, e^{25}, e^{16} + e^{28}$                     | 2579     |
| 9521:54a | $0, 0, 0, 0, e^{12}, e^{13}, e^{23} + e^{14}, e^{15}, e^{34} + e^{25} + e^{18}$   | 3679     |
| 9521:54b | $0, 0, 0, 0, -e^{12}, e^{13}, e^{23} + e^{14}, e^{15}, e^{25} + e^{18} + e^{34}$  | 3679     |
| 9521:55a | $0, 0, 0, 0, e^{12}, e^{13}, e^{14} + e^{23}, e^{25}, e^{28} + e^{15} + e^{34}$   | 3679     |
| 9521:55b | $0, 0, 0, 0, -e^{12}, e^{13}, e^{14} + e^{23}, e^{25}, e^{34} + e^{28} + e^{15}$  | 3679     |
| 9521:56a | $0, 0, 0, 0, e^{12}, e^{14} + e^{23}, e^{13} + e^{24}, e^{15}, e^{18} + e^{25}$   | 3679     |
| 9521:56b | $0, 0, 0, 0, e^{12}, e^{23} - e^{14}, e^{24} + e^{13}, e^{15}, e^{25} + e^{18}$   | 3679     |
| 9521:57  | $0, 0, 0, 0, e^{12}, e^{34}, e^{13}, e^{15}, e^{36} + e^{18}$                     | 2479     |
| 9521:58  | $0, 0, 0, 0, e^{12}, e^{34}, e^{13}, e^{25}, e^{28} + e^{36}$                     | 2479     |
| 9521:59  | $0, 0, 0, 0, e^{12}, e^{34}, e^{13}, e^{15}, e^{46} + e^{18}$                     | 2479     |
| 9521:60  | $0, 0, 0, 0, e^{12}, e^{34}, e^{13}, e^{25}, e^{28} + e^{46}$                     | 2479     |
| 9521:61  | $0, 0, 0, 0, e^{12}, e^{13}, e^{14} + e^{23}, e^{15}, e^{36} + e^{18}$            | 2579     |
| 9521:62  | $0, 0, 0, 0, e^{12}, e^{13}, e^{14} + e^{23}, e^{25}, e^{36} + e^{28}$            | 2579     |
| 9521:63  | $0, 0, 0, 0, e^{12}, e^{13}, e^{34}, e^{15}, e^{18} + e^{24} + e^{36}$            | 2579     |
| 9521:64  | $0, 0, 0, 0, e^{12}, e^{13}, e^{34}, e^{25}, e^{36} + e^{14} + e^{28}$            | 2579     |
| 9521:65  | $0, 0, 0, 0, -e^{12}, e^{13}, e^{23}, e^{15} + e^{24}, e^{45} + e^{18}$           | 3579     |

Table 2 – Continued to next page

Table 2 – Continued from previous page

| Name      | $\mathfrak{g}$                                                                                | UCS Dim. |
|-----------|-----------------------------------------------------------------------------------------------|----------|
| 9521:66   | $0, 0, 0, 0, -e^{12}, e^{13}, e^{14}, e^{15} + e^{23}, e^{18} + e^{35}$                       | 3579     |
| 9521:67   | $0, 0, 0, 0, -e^{12}, e^{13}, e^{24}, e^{15} + e^{23}, e^{18} + e^{35}$                       | 3579     |
| 9521:68   | $0, 0, 0, 0, e^{12}, e^{13}, e^{34}, e^{23} + e^{15}, e^{26} + e^{18}$                        | 2579     |
| 9521:69   | $0, 0, 0, 0, -e^{12}, e^{34}, e^{13} + e^{24}, e^{15} + e^{23}, e^{18} + e^{35}$              | 3579     |
| 9521:70a  | $0, 0, 0, 0, e^{12}, e^{14} + e^{23}, e^{13} + e^{24}, e^{15}, e^{18} + e^{34} + e^{25}$      | 3679     |
| 9521:70b  | $0, 0, 0, 0, e^{12}, e^{23} - e^{14}, e^{24} + e^{13}, e^{15}, e^{25} + e^{18} + e^{34}$      | 3679     |
| 9521:70c  | $0, 0, 0, 0, -e^{12}, -e^{14} + e^{23}, e^{24} + e^{13}, e^{15}, e^{25} + e^{18} + e^{34}$    | 3679     |
| 9521:71   | $0, 0, 0, 0, e^{12}, e^{13}, e^{14} + e^{23}, e^{25}, e^{28} + e^{16}$                        | 2579     |
| 9521:72   | $0, 0, 0, 0, e^{12}, e^{13}, e^{14}, e^{15}, e^{24} + e^{36} + e^{18}$                        | 2579     |
| 9521:73   | $0, 0, 0, 0, e^{12}, e^{13}, e^{14}, e^{25}, e^{16} + e^{28} + e^{34}$                        | 2579     |
| 9521:74   | $0, 0, 0, 0, e^{12}, e^{13}, e^{24}, e^{25}, e^{28} + e^{36} + e^{14}$                        | 2579     |
| 9521:75   | $0, 0, 0, 0, e^{12}, e^{13}, e^{24}, e^{25}, e^{16} + e^{34} + e^{28}$                        | 2579     |
| 9521:76   | $0, 0, 0, 0, e^{12}, e^{13}, e^{23}, e^{15}, e^{18} + e^{36} + e^{24}$                        | 2579     |
| 9521:77   | $0, 0, 0, 0, e^{12}, e^{13}, e^{23}, e^{25}, e^{28} + e^{36} + e^{14}$                        | 2579     |
| 9521:78   | $0, 0, 0, 0, e^{12}, e^{13}, e^{23}, e^{25}, e^{16} + e^{28} + e^{34}$                        | 2579     |
| 9521:79   | $0, 0, 0, 0, e^{12}, e^{34}, e^{13} + e^{24}, e^{15}, e^{36} + e^{18}$                        | 2479     |
| 9521:80   | $0, 0, 0, 0, e^{12}, e^{34}, e^{14} + e^{23}, e^{15}, e^{18} + e^{36}$                        | 2479     |
| 9521:81   | $0, 0, 0, 0, e^{12}, e^{13}, e^{14}, e^{23} + e^{15}, e^{18} + e^{26}$                        | 2579     |
| 9521:82   | $0, 0, 0, 0, e^{12}, e^{13}, e^{24}, e^{15} + e^{23}, e^{18} + e^{26}$                        | 2579     |
| 9521:83a  | $0, 0, 0, 0, e^{12}, e^{13}, e^{34}, e^{15}, e^{25} + e^{18} + e^{36}$                        | 2579     |
| 9521:83b  | $0, 0, 0, 0, -e^{12}, e^{13}, e^{34}, e^{15}, e^{36} + e^{25} + e^{18}$                       | 2579     |
| 9521:84   | $0, 0, 0, 0, e^{12}, e^{13}, e^{34}, e^{15}, e^{35} + e^{18} + e^{26}$                        | 2579     |
| 9521:85   | $0, 0, 0, 0, e^{12}, e^{13}, e^{34}, e^{25}, e^{36} + e^{15} + e^{28}$                        | 2579     |
| 9521:86   | $0, 0, 0, 0, e^{12}, -e^{13}, e^{23}, e^{15} + e^{34}, e^{18} + e^{46}$                       | 2479     |
| 9521:87   | $0, 0, 0, 0, e^{12}, -e^{13}, e^{14}, e^{15} + e^{34}, e^{18} + e^{46}$                       | 2479     |
| 9521:88   | $0, 0, 0, 0, e^{12}, -e^{13}, e^{24}, e^{15} + e^{34}, e^{18} + e^{46}$                       | 2479     |
| 9521:89   | $0, 0, 0, 0, -e^{12}, e^{13}, e^{23} + e^{14}, e^{24} + e^{15}, e^{45} + e^{18}$              | 3579     |
| 9521:90   | $0, 0, 0, 0, -e^{12}, e^{13}, e^{34}, e^{15} + e^{24}, e^{18} + e^{45} + e^{23}$              | 3579     |
| 9521:91   | $0, 0, 0, 0, -e^{12}, e^{13}, e^{34}, e^{15} + e^{23}, e^{18} + e^{35} + e^{24}$              | 3579     |
| 9521:92   | $0, 0, 0, 0, e^{12}, e^{34}, e^{13}, e^{15}, e^{18} + e^{23} + e^{46}$                        | 2479     |
| 9521:93   | $0, 0, 0, 0, e^{12}, e^{34}, e^{13}, e^{15}, e^{18} + e^{24} + e^{36}$                        | 2479     |
| 9521:94   | $0, 0, 0, 0, e^{12}, e^{34}, e^{13}, e^{25}, e^{28} + e^{36} + e^{14}$                        | 2479     |
| 9521:95   | $0, 0, 0, 0, e^{12}, e^{13}, e^{23} + e^{14}, e^{15}, e^{24} + e^{36} + e^{18}$               | 2579     |
| 9521:96a  | $0, 0, 0, 0, e^{12}, e^{13}, e^{14} + e^{23}, e^{25}, e^{28} + e^{34} + e^{16}$               | 2579     |
| 9521:96b  | $0, 0, 0, 0, -e^{12}, e^{13}, e^{14} + e^{23}, e^{25}, e^{16} + e^{34} + e^{28}$              | 2579     |
| 9521:97a  | $0, 0, 0, 0, e^{12}, e^{13}, e^{23}, e^{15}, e^{18} + e^{36} + e^{25}$                        | 3579     |
| 9521:97b  | $0, 0, 0, 0, -e^{12}, e^{13}, e^{23}, e^{15}, e^{25} + e^{18} + e^{36}$                       | 3579     |
| 9521:98   | $0, 0, 0, 0, e^{12}, e^{13}, e^{23}, e^{15}, e^{18} + e^{26} + e^{35}$                        | 3579     |
| 9521:99   | $0, 0, 0, 0, e^{12}, e^{13}, e^{23}, e^{25}, e^{28} + e^{36} + e^{15}$                        | 3579     |
| 9521:100a | $0, 0, 0, 0, e^{12}, e^{13}, e^{14}, e^{15}, e^{36} + e^{25} + e^{18}$                        | 2579     |
| 9521:100b | $0, 0, 0, 0, -e^{12}, e^{13}, e^{14}, e^{15}, e^{36} + e^{25} + e^{18}$                       | 2579     |
| 9521:101  | $0, 0, 0, 0, e^{12}, e^{13}, e^{14}, e^{15}, e^{18} + e^{35} + e^{26}$                        | 2579     |
| 9521:102  | $0, 0, 0, 0, e^{12}, e^{13}, e^{14}, e^{25}, e^{15} + e^{28} + e^{36}$                        | 2579     |
| 9521:103a | $0, 0, 0, 0, e^{12}, e^{13}, e^{24}, e^{15}, e^{36} + e^{25} + e^{18}$                        | 2579     |
| 9521:103b | $0, 0, 0, 0, -e^{12}, e^{13}, e^{24}, e^{15}, e^{18} + e^{25} + e^{36}$                       | 2579     |
| 9521:104  | $0, 0, 0, 0, e^{12}, e^{13}, e^{24}, e^{15}, e^{18} + e^{35} + e^{26}$                        | 2579     |
| 9521:105  | $0, 0, 0, 0, e^{12}, e^{13}, e^{24}, e^{25}, e^{28} + e^{36} + e^{15}$                        | 2579     |
| 9521:106  | $0, 0, 0, 0, e^{12}, e^{13}, e^{23}, e^{15}, e^{18} + e^{27} + e^{36}$                        | 2579     |
| 9521:107  | $0, 0, 0, 0, -e^{12}, e^{13}, e^{14}, e^{15} + e^{23}, e^{18} + e^{35} + e^{24}$              | 3579     |
| 9521:108  | $0, 0, 0, 0, e^{12}, e^{13}, e^{34}, e^{15}, e^{47} + e^{36} + e^{18}$                        | 1479     |
| 9521:109  | $0, 0, 0, 0, e^{12}, e^{13}, e^{34}, e^{25}, e^{28} + e^{36} + e^{47}$                        | 1479     |
| 9521:110  | $0, 0, 0, 0, e^{12}, e^{13}, e^{14}, e^{23} + e^{15}, e^{34} + e^{26} + e^{18}$               | 2579     |
| 9521:111  | $0, 0, 0, 0, e^{12}, e^{13}, e^{24}, e^{15} + e^{23}, e^{26} + e^{34} + e^{18}$               | 2579     |
| 9521:112  | $0, 0, 0, 0, e^{12}, -e^{13}, e^{23} + e^{14}, e^{15} + e^{34}, e^{18} + e^{46}$              | 2479     |
| 9521:113  | $0, 0, 0, 0, e^{12}, e^{14} + e^{23}, e^{13}, e^{15} + e^{34}, e^{36} + e^{18}$               | 2479     |
| 9521:114  | $0, 0, 0, 0, e^{12}, -e^{23} + e^{14}, e^{13}, e^{25} + e^{34}, e^{46} + e^{28}$              | 2479     |
| 9521:115  | $0, 0, 0, 0, e^{12}, a_1, e^{13}(1 + a_1), e^{34}, e^{15} + e^{23}, e^{18} + e^{26} + e^{35}$ | 2579     |
| 9521:116  | $0, 0, 0, 0, e^{12}, e^{34}, e^{24} + e^{13}, e^{15}, e^{46} + e^{18} + e^{23}$               | 2479     |

Table 2 – Continued to next page

Table 2 – Continued from previous page

| Name      | $\mathfrak{g}$                                                                                       | UCS Dim. |
|-----------|------------------------------------------------------------------------------------------------------|----------|
| 9521:117  | $0, 0, 0, 0, e^{12}, e^{34}, e^{13}, e^{15}, e^{36} + e^{18} + e^{25}$                               | 2479     |
| 9521:118  | $0, 0, 0, 0, e^{12}, e^{34}, e^{13}, e^{25}, e^{28} + e^{36} + e^{15}$                               | 2479     |
| 9521:119  | $0, 0, 0, 0, e^{12}, e^{34}, e^{13}, e^{15}, e^{46} + e^{25} + e^{18}$                               | 2479     |
| 9521:120  | $0, 0, 0, 0, e^{12}, e^{34}, e^{13}, e^{25}, e^{15} + e^{28} + e^{46}$                               | 2479     |
| 9521:121  | $0, 0, 0, 0, e^{12}, e^{13}, e^{34}, e^{25}, e^{28} + e^{37} + e^{16}$                               | 1479     |
| 9521:122a | $0, 0, 0, 0, e^{12}, e^{13}, e^{34}, e^{25}, e^{28} + e^{47} + e^{16}$                               | 1479     |
| 9521:122b | $0, 0, 0, 0, e^{12}, -e^{13}, e^{34}, e^{25}, e^{16} + e^{28} + e^{47}$                              | 1479     |
| 9521:123  | $0, 0, 0, 0, e^{12}, -e^{13}, e^{34}, e^{25}, e^{46} + e^{17} + e^{28}$                              | 1479     |
| 9521:124a | $0, 0, 0, 0, e^{12}, e^{13}, e^{14}, e^{15}, e^{18} + e^{47} + e^{36}$                               | 1479     |
| 9521:124b | $0, 0, 0, 0, e^{12}, -e^{13}, e^{14}, e^{15}, e^{47} + e^{36} + e^{18}$                              | 1479     |
| 9521:125  | $0, 0, 0, 0, e^{12}, e^{13}, e^{14}, e^{15}, e^{18} + e^{46} + e^{37}$                               | 1479     |
| 9521:126a | $0, 0, 0, 0, e^{12}, e^{13}, e^{14}, e^{25}, e^{28} + e^{36} + e^{47}$                               | 1479     |
| 9521:126b | $0, 0, 0, 0, e^{12}, -e^{13}, e^{14}, e^{25}, e^{28} + e^{47} + e^{36}$                              | 1479     |
| 9521:127  | $0, 0, 0, 0, e^{12}, e^{13}, e^{14}, e^{25}, e^{46} + e^{28} + e^{37}$                               | 1479     |
| 9521:128  | $0, 0, 0, 0, e^{12}, e^{13}, e^{24}, e^{15}, e^{18} + e^{47} + e^{36}$                               | 1479     |
| 9521:129a | $0, 0, 0, 0, e^{12}, e^{13}, e^{23} + e^{14}, e^{15}, e^{36} + e^{25} + e^{18}$                      | 2579     |
| 9521:129b | $0, 0, 0, 0, -e^{12}, e^{13}, e^{14} + e^{23}, e^{15}, e^{36} + e^{25} + e^{18}$                     | 2579     |
| 9521:130  | $0, 0, 0, 0, e^{12}, e^{13}, e^{14} + e^{23}, e^{15}, e^{18} + e^{35} + e^{26}$                      | 2579     |
| 9521:131  | $0, 0, 0, 0, e^{12}, e^{13}, e^{23} + e^{14}, e^{25}, e^{15} + e^{28} + e^{36}$                      | 2579     |
| 9521:132  | $0, 0, 0, 0, e^{12}, -e^{13}, e^{14}, e^{15} + e^{34}, e^{18} + e^{23} + e^{46}$                     | 2479     |
| 9521:133  | $0, 0, 0, 0, e^{12}, -e^{13}, e^{24}, e^{15} + e^{34}, e^{23} + e^{46} + e^{18}$                     | 2479     |
| 9521:134  | $0, 0, 0, 0, (-1 + a_2)e^{12}, a_2e^{13}, e^{14}, e^{15} + e^{23}, e^{18} + e^{26} + e^{35}$         | 2579     |
| 9521:135  | $0, 0, 0, 0, (-1 + a_2)e^{12}, e^{13}a_2, e^{24}, e^{15} + e^{23}, e^{18} + e^{26} + e^{35}$         | 2579     |
| 9521:136  | $0, 0, 0, 0, e^{12}, e^{14} + e^{23}, e^{34}, e^{13} + e^{25}, e^{16} + e^{28}$                      | 2479     |
| 9521:137  | $0, 0, 0, 0, -e^{12}, e^{34}, e^{13}, e^{15} + e^{23}, e^{18} + e^{35} + e^{46}$                     | 2479     |
| 9521:138  | $0, 0, 0, 0, -e^{12}, e^{34}, e^{13}, e^{15} + e^{24}, e^{45} + e^{36} + e^{18}$                     | 2479     |
| 9521:139  | $0, 0, 0, 0, e^{12}, e^{34}, e^{13}, e^{14} + e^{25}, e^{28} + e^{36} + e^{45}$                      | 2479     |
| 9521:140  | $0, 0, 0, 0, e^{12}, -e^{13}, e^{23}, e^{15} + e^{34}, e^{37} + e^{18} + e^{46}$                     | 1479     |
| 9521:141  | $0, 0, 0, 0, e^{12}, e^{13}a_1, (1 + a_1)e^{14}, e^{34} + e^{15}, e^{18} + e^{37} + e^{46}$          | 1479     |
| 9521:142a | $0, 0, 0, 0, e^{12}, e^{14} + e^{23}, e^{13} + e^{24}, e^{15} + e^{34}, e^{18} + e^{36}$             | 2479     |
| 9521:142b | $0, 0, 0, 0, e^{12}, e^{23} + e^{14}, e^{24} - e^{13}, e^{15} + e^{34}, e^{36} + e^{18}$             | 2479     |
| 9521:143  | $0, 0, 0, 0, -e^{12}, e^{13}, e^{34}, e^{15} + e^{24}, e^{36} + e^{45} + e^{18}$                     | 2479     |
| 9521:144  | $0, 0, 0, 0, e^{12}, e^{13}, e^{34}, e^{25} + e^{14}, e^{28} + e^{36} + e^{45}$                      | 2479     |
| 9521:145  | $0, 0, 0, 0, e^{12}, e^{13}, e^{14}, e^{25}, e^{36} + e^{17} + e^{28}$                               | 1479     |
| 9521:146  | $0, 0, 0, 0, e^{12}, e^{13}, e^{24}, e^{15}, e^{27} + e^{36} + e^{18}$                               | 1479     |
| 9521:147  | $0, 0, 0, 0, e^{12}, e^{34}, e^{24} + e^{13}, e^{15}, e^{36} + e^{25} + e^{18}$                      | 2479     |
| 9521:148  | $0, 0, 0, 0, e^{12}, e^{34}, e^{14} + e^{23}, e^{15}, e^{18} + e^{36} + e^{25}$                      | 2479     |
| 9521:149  | $0, 0, 0, 0, e^{12}, e^{14} + e^{23}, e^{13}, e^{15} + e^{24}, e^{26} + e^{18}$                      | 2479     |
| 9521:150  | $0, 0, 0, 0, e^{12}, e^{34}, e^{24} + e^{13}, e^{15}, e^{18} + e^{26} + e^{37}$                      | 1479     |
| 9521:151  | $0, 0, 0, 0, e^{12}, -e^{13}, e^{23}, e^{34} + e^{15}, e^{46} + e^{25} + e^{18}$                     | 2479     |
| 9521:152  | $0, 0, 0, 0, e^{12}, -e^{13}, e^{14}, e^{34} + e^{15}, e^{25} + e^{18} + e^{46}$                     | 2479     |
| 9521:153  | $0, 0, 0, 0, e^{12}, -e^{13}, e^{24}, e^{15} + e^{34}, e^{46} + e^{18} + e^{25}$                     | 2479     |
| 9521:154  | $0, 0, 0, 0, e^{12}, e^{24} + e^{13}, e^{34}, e^{15}, e^{18} + e^{26} + e^{35}$                      | 2479     |
| 9521:155  | $0, 0, 0, 0, e^{12}, -e^{13}, e^{23}, e^{15} + e^{34}, e^{18} + e^{46} + e^{27}$                     | 1479     |
| 9521:156  | $0, 0, 0, 0, e^{12}, e^{13}, e^{34}, e^{23} + e^{15}, e^{37} + e^{18} + e^{26}$                      | 1479     |
| 9521:157  | $0, 0, 0, 0, e^{12}, e^{13}, e^{14} + e^{23}, e^{15}, e^{37} + e^{18} + e^{46}$                      | 1479     |
| 9521:158  | $0, 0, 0, 0, e^{12}, e^{13}, e^{23} + e^{14}, e^{25}, e^{28} + e^{37} + e^{46}$                      | 1479     |
| 9521:159  | $0, 0, 0, 0, e^{12}, e^{13}, e^{34}, e^{15} + e^{23}, e^{18} + e^{26} + e^{47}$                      | 1479     |
| 9521:160  | $0, 0, 0, 0, e^{12}, e^{13}, e^{24}, e^{25} + e^{34}, e^{37} + e^{16} + e^{28}$                      | 1479     |
| 9521:161  | $0, 0, 0, 0, -e^{12}, e^{13}, e^{23}, e^{15} + e^{24}, e^{36} + e^{45} + e^{18}$                     | 2479     |
| 9521:162  | $0, 0, 0, 0, e^{12}, e^{13}, e^{23}, e^{25} + e^{14}, e^{28} + e^{36} + e^{45}$                      | 2479     |
| 9521:163  | $0, 0, 0, 0, -e^{12}, e^{13}, e^{14}, e^{24} + e^{15}, e^{36} + e^{45} + e^{18}$                     | 2479     |
| 9521:164  | $0, 0, 0, 0, e^{12}, e^{13}, e^{24}, e^{14} + e^{25}, e^{36} + e^{45} + e^{28}$                      | 2479     |
| 9521:165  | $0, 0, 0, 0, e^{12}, e^{13}, e^{34}, e^{25} + e^{14}, e^{16} + e^{45} + e^{28}$                      | 2479     |
| 9521:166  | $0, 0, 0, 0, e^{12}, e^{23} + e^{14}, e^{13}, e^{15} + e^{34}, e^{18} + e^{36} + e^{24}$             | 2479     |
| 9521:167  | $0, 0, 0, 0, -e^{12}, e^{34}, e^{24} + e^{13}, e^{23} + e^{15}, e^{46} + e^{35} + e^{18}$            | 2479     |
| 9521:168  | $0, 0, 0, 0, e^{12}, e^{13}a_1, e^{14}(1 + a_1) + e^{23}, e^{15} + e^{34}, e^{37} + e^{46} + e^{18}$ | 1479     |
| 9521:169a | $0, 0, 0, 0, e^{12}, e^{13}, e^{14} - e^{23}, e^{25} + e^{34}, e^{47} + e^{28} + e^{36}$             | 1479     |

Table 2 – Continued to next page

Table 2 – Continued from previous page

| Name      | $\mathfrak{g}$                                                                                                 | UCS Dim. |
|-----------|----------------------------------------------------------------------------------------------------------------|----------|
| 9521:169b | $0, 0, 0, 0, e^{12}, -e^{13}, e^{14} - e^{23}, e^{34} + e^{25}, e^{47} + e^{28} + e^{36}$                      | 1479     |
| 9521:170  | $0, 0, 0, 0, -e^{12}, e^{14} + e^{23}, e^{13}, e^{25}, e^{28} + e^{35} + e^{16}$                               | 2479     |
| 9521:171  | $0, 0, 0, 0, e^{12}, e^{14} + e^{23}, e^{13}, e^{15}, e^{26} + e^{45} + e^{18}$                                | 2479     |
| 9521:172  | $0, 0, 0, 0, e^{12}, e^{13}, e^{23}, e^{25} + e^{14}, e^{16} + e^{28} + e^{45}$                                | 2479     |
| 9521:173  | $0, 0, 0, 0, e^{12}, e^{13}, e^{24}, e^{25} + e^{14}, e^{28} + e^{16} + e^{45}$                                | 2479     |
| 9521:174  | $0, 0, 0, 0, e^{12}, e^{13}, e^{14}, e^{23} + e^{15}, e^{47} + e^{18} + e^{26}$                                | 1479     |
| 9521:175  | $0, 0, 0, 0, e^{12}, e^{13}, e^{24}, e^{15} + e^{23}, e^{18} + e^{47} + e^{26}$                                | 1479     |
| 9521:176a | $0, 0, 0, 0, e^{12}, e^{13}, e^{34}, e^{15}, e^{25} + e^{18} + e^{47} + e^{36}$                                | 1479     |
| 9521:176b | $0, 0, 0, 0, -e^{12}, e^{13}, e^{34}, e^{15}, e^{36} + e^{25} + e^{18} + e^{47}$                               | 1479     |
| 9521:177  | $0, 0, 0, 0, e^{12}, e^{13}, e^{34}, e^{15}, e^{35} + e^{47} + e^{18} + e^{26}$                                | 1479     |
| 9521:178  | $0, 0, 0, 0, e^{12}, e^{13}, e^{34}, e^{25}, e^{47} + e^{36} + e^{15} + e^{28}$                                | 1479     |
| 9521:179a | $0, 0, 0, 0, e^{12}, e^{14} + e^{23}, e^{13}, e^{24} + e^{15}, e^{18} + e^{26} + e^{34}$                       | 2479     |
| 9521:179b | $0, 0, 0, 0, -e^{12}, e^{23} + e^{14}, e^{13}, e^{24} + e^{15}, e^{18} + e^{26} + e^{34}$                      | 2479     |
| 9521:180  | $0, 0, 0, 0, e^{12}, -e^{13}, e^{14} + e^{23}, e^{34} + e^{15}, e^{46} + e^{18} + e^{25}$                      | 2479     |
| 9521:181  | $0, 0, 0, 0, -e^{12}, e^{13}, e^{23} + e^{14}, e^{24} + e^{15}, e^{36} + e^{45} + e^{18}$                      | 2479     |
| 9521:182  | $0, 0, 0, 0, e^{12}, e^{14} + e^{23}, e^{13}, e^{34} + e^{15}, e^{36} + e^{25} + e^{18}$                       | 2479     |
| 9521:183  | $0, 0, 0, 0, e^{12}, -e^{23} + e^{14}, e^{13}, e^{25} + e^{34}, e^{15} + e^{28} + e^{46}$                      | 2479     |
| 9521:184  | $0, 0, 0, 0, e^{12}, e^{13}, e^{14} - e^{23}, e^{25} + e^{34}, e^{28} + e^{16} + e^{47}$                       | 1479     |
| 9521:185a | $0, 0, 0, 0, e^{12}, e^{34}, e^{14} + e^{23}, e^{13} + e^{25}, e^{17} + e^{28} + e^{36}$                       | 1479     |
| 9521:185b | $0, 0, 0, 0, e^{12}, e^{34}, -e^{14} + e^{23}, e^{13} + e^{25}, e^{28} + e^{36} + e^{17}$                      | 1479     |
| 9521:186a | $0, 0, 0, 0, e^{12}, e^{23} + e^{14}, e^{24} + e^{13}, e^{15}, e^{18} + e^{36} + e^{47}$                       | 1479     |
| 9521:186b | $0, 0, 0, 0, e^{12}, e^{14} - e^{23}, e^{24} + e^{13}, e^{15}, e^{36} + e^{18} + e^{47}$                       | 1479     |
| 9521:187a | $0, 0, 0, 0, e^{12}, e^{14} + e^{23}, e^{13} + e^{24}, e^{15}, e^{18} + e^{46} + e^{37}$                       | 1479     |
| 9521:187b | $0, 0, 0, 0, e^{12}, -e^{14} + e^{23}, e^{24} + e^{13}, e^{15}, e^{37} + e^{18} + e^{46}$                      | 1479     |
| 9521:188  | $0, 0, 0, 0, e^{12}, e^{34}, e^{14} + e^{23}, e^{13} + e^{25}, e^{28} + e^{46} + e^{17}$                       | 1479     |
| 9521:189  | $0, 0, 0, 0, (-1 + a_2)e^{12}, e^{14} + e^{23}, e^{34}, a_2e^{13} + e^{25}, e^{16} + e^{28} + e^{35}$          | 2479     |
| 9521:190a | $0, 0, 0, 0, e^{12}, e^{14}a_1 + e^{23}, (-1 + a_1)e^{13} + e^{24}, e^{34} + e^{15}, e^{18} + e^{47} + e^{36}$ | 1479     |
| 9521:190b | $0, 0, 0, 0, e^{12}, e^{14}a_1 - e^{23}, (-1 + a_1)e^{13} + e^{24}, e^{15} + e^{34}, e^{18} + e^{47} + e^{36}$ | 1479     |
| 9521:191a | $0, 0, 0, 0, e^{12}, e^{13}, e^{14}, e^{15}, e^{18} + e^{47} + e^{25} + e^{36}$                                | 1479     |
| 9521:191b | $0, 0, 0, 0, e^{12}, -e^{13}, e^{14}, e^{15}, e^{47} + e^{36} + e^{25} + e^{18}$                               | 1479     |
| 9521:191c | $0, 0, 0, 0, -e^{12}, e^{13}, e^{14}, e^{15}, e^{36} + e^{25} + e^{18} + e^{47}$                               | 1479     |
| 9521:192  | $0, 0, 0, 0, e^{12}, e^{13}, e^{14}, e^{15}, e^{18} + e^{47} + e^{35} + e^{26}$                                | 1479     |
| 9521:193  | $0, 0, 0, 0, e^{12}, e^{13}, e^{14}, e^{15}, e^{25} + e^{18} + e^{37} + e^{46}$                                | 1479     |
| 9521:194a | $0, 0, 0, 0, e^{12}, e^{13}, e^{14}, e^{25}, e^{36} + e^{47} + e^{28} + e^{15}$                                | 1479     |
| 9521:194b | $0, 0, 0, 0, e^{12}, -e^{13}, e^{14}, e^{25}, e^{15} + e^{47} + e^{28} + e^{36}$                               | 1479     |
| 9521:195  | $0, 0, 0, 0, e^{12}, e^{13}, e^{14}, e^{25}, e^{37} + e^{46} + e^{15} + e^{28}$                                | 1479     |
| 9521:196a | $0, 0, 0, 0, e^{12}, e^{13}, e^{24}, e^{15}, e^{25} + e^{47} + e^{18} + e^{36}$                                | 1479     |
| 9521:196b | $0, 0, 0, 0, -e^{12}, e^{13}, e^{24}, e^{15}, e^{18} + e^{36} + e^{47} + e^{25}$                               | 1479     |
| 9521:197  | $0, 0, 0, 0, e^{12}, e^{13}, e^{24}, e^{15}, e^{18} + e^{26} + e^{35} + e^{47}$                                | 1479     |
| 9521:198a | $0, 0, 0, 0, e^{12}, e^{13} + e^{24}, e^{14} + e^{23}, e^{15}, e^{18} + e^{26} + e^{35}$                       | 2479     |
| 9521:198b | $0, 0, 0, 0, -e^{12}, e^{24} - e^{13}, e^{14} + e^{23}, e^{15}, e^{26} + e^{35} + e^{18}$                      | 2479     |
| 9521:199  | $0, 0, 0, 0, e^{12}a_1, e^{23} + (1 + a_1)e^{14}, e^{13}, e^{15} + e^{24}, e^{18} + e^{45} + e^{26}$           | 2479     |
| 9521:200  | $0, 0, 0, 0, e^{12}, e^{13}, e^{14} + e^{23}, e^{15} + e^{24}, e^{36} + e^{18} + e^{27}$                       | 1479     |
| 9521:201  | $0, 0, 0, 0, e^{12}, e^{34}, e^{24} + e^{13}, e^{15}, e^{35} + e^{46} + e^{27} + e^{18}$                       | 1479     |
| 9521:202  | $0, 0, 0, 0, e^{12}, -e^{13}, e^{23}, e^{34} + e^{15}, e^{18} + e^{37} + e^{46} + e^{25}$                      | 1479     |
| 9521:203  | $0, 0, 0, 0, e^{12}a_1, (1 + a_1)e^{13}, e^{34}, e^{15} + e^{23}, e^{18} + e^{26} + e^{35} + e^{47}$           | 1479     |
| 9521:204  | $0, 0, 0, 0, e^{12}, e^{13}a_1, (1 + a_1)e^{14}, e^{15} + e^{34}, e^{37} + e^{46} + e^{25} + e^{18}$           | 1479     |
| 9521:205  | $0, 0, 0, 0, e^{12}, e^{13}, e^{34}, e^{14} + e^{25}, e^{28} + e^{37} + e^{45} + e^{16}$                       | 1479     |
| 9521:206a | $0, 0, 0, 0, e^{12}, e^{14} + e^{23}, e^{24} + e^{13}, e^{15} + e^{34}, e^{36} + e^{25} + e^{18}$              | 2479     |
| 9521:206b | $0, 0, 0, 0, e^{12}, e^{14} + e^{23}, -e^{13} + e^{24}, e^{15} + e^{34}, e^{18} + e^{25} + e^{36}$             | 2479     |
| 9521:207  | $0, 0, 0, 0, e^{12}, e^{13}, e^{14} + e^{23}, e^{15}, e^{18} + e^{46} + e^{25} + e^{37}$                       | 1479     |
| 9521:208  | $0, 0, 0, 0, e^{12}, e^{13}, e^{23} + e^{14}, e^{15}, e^{18} + e^{27} + e^{36} + e^{45}$                       | 1479     |
| 9521:209a | $0, 0, 0, 0, e^{12}, e^{13}, e^{14} + e^{23}, e^{25}, e^{46} + e^{28} + e^{15} + e^{37}$                       | 1479     |
| 9521:209b | $0, 0, 0, 0, -e^{12}, e^{13}, e^{14} + e^{23}, e^{25}, e^{15} + e^{46} + e^{28} + e^{37}$                      | 1479     |
| 9521:210  | $0, 0, 0, 0, e^{12}, e^{13}, e^{23}, e^{25} + e^{14}, e^{37} + e^{16} + e^{28} + e^{45}$                       | 1479     |
| 9521:211  | $0, 0, 0, 0, e^{12}(-1 + a_2), a_2e^{13}, e^{14}, e^{15} + e^{23}, e^{26} + e^{47} + e^{18} + e^{35}$          | 1479     |
| 9521:212  | $0, 0, 0, 0, (-1 + a_2)e^{12}, e^{13}a_2, e^{24}, e^{23} + e^{15}, e^{35} + e^{47} + e^{26} + e^{18}$          | 1479     |
| 9521:213  | $0, 0, 0, 0, e^{12}, (-1 + a_2)e^{13}, e^{14}a_2 + e^{23}, e^{34} + e^{15}, e^{18} + e^{37} + e^{46} + e^{25}$ | 1479     |

Table 2 – Continued to next page

Table 2 – Continued from previous page

| Name      | $\mathfrak{g}$                                                                                                          | UCS Dim. |
|-----------|-------------------------------------------------------------------------------------------------------------------------|----------|
| 9521:214a | $0, 0, 0, 0, e^{12}, e^{13}, -e^{23} + e^{14}, e^{25} + e^{34}, e^{47} + e^{36} + e^{15} + e^{28}$                      | 1479     |
| 9521:214b | $0, 0, 0, 0, e^{12}, -e^{13}, e^{14} - e^{23}, e^{34} + e^{25}, e^{28} + e^{47} + e^{36} + e^{15}$                      | 1479     |
| 9521:215  | $0, 0, 0, 0, e^{12}, a_1, e^{34}, e^{14} + e^{23}, e^{25} + (1 + a_1)e^{13}, e^{28} + e^{46} + e^{35} + e^{17}$         | 1479     |
| 9521:216a | $0, 0, 0, 0, e^{12}, e^{14} + e^{23}, e^{13} + e^{24}, e^{15}, e^{18} + e^{47} + e^{25} + e^{36}$                       | 1479     |
| 9521:216b | $0, 0, 0, 0, e^{12}, e^{14} - e^{23}, e^{24} + e^{13}, e^{15}, e^{18} + e^{47} + e^{36} + e^{25}$                       | 1479     |
| 9521:217a | $0, 0, 0, 0, e^{12}, e^{23} + e^{14}, e^{24} + e^{13}, e^{15}, e^{18} + e^{37} + e^{46} + e^{25}$                       | 1479     |
| 9521:217b | $0, 0, 0, 0, e^{12}, -e^{14} + e^{23}, e^{24} + e^{13}, e^{15}, e^{46} + e^{25} + e^{37} + e^{18}$                      | 1479     |
| 9521:217c | $0, 0, 0, 0, -e^{12}, e^{23} + e^{14}, e^{24} + e^{13}, e^{15}, e^{46} + e^{25} + e^{37} + e^{18}$                      | 1479     |
| 9521:218  | $0, 0, 0, 0, e^{12}(-1 + a_2), e^{13}, a_2e^{14} + e^{23}, e^{24} + e^{15}, e^{36} + e^{27} + e^{18} + e^{45}$          | 1479     |
| 9521:219a | $0, 0, 0, 0, e^{12}, e^{14}a_1 + e^{23}, (-1 + a_1)e^{13} + e^{24}, e^{15} + e^{34}, e^{36} + e^{25} + e^{18} + e^{47}$ | 1479     |
| 9521:219b | $0, 0, 0, 0, e^{12}, e^{14}a_1 - e^{23}, (-1 + a_1)e^{13} + e^{24}, e^{15} + e^{34}, e^{47} + e^{36} + e^{25} + e^{18}$ | 1479     |
| 9521:249  | $0, 0, 0, 0, e^{12}, -e^{13}, e^{23}, -2e^{17} + e^{26} + e^{35}, e^{18} + e^{56}$                                      | 2369     |
| 9521:250  | $0, 0, 0, 0, e^{12}, -e^{13}, e^{23}, -2e^{17} + e^{35} + e^{26}, e^{18} + e^{56} + e^{24}$                             | 1369     |
| 9521:251  | $0, 0, 0, 0, -e^{12}, -2e^{13}, -e^{23}, e^{17} + e^{26} + e^{35}, e^{16} + e^{28} + e^{57}$                            | 2369     |
| 9521:252  | $0, 0, 0, 0, -2e^{12}, -e^{13}, e^{23}, e^{17} + e^{35} + e^{26}, e^{14} + e^{25} + e^{38} + e^{67}$                    | 1369     |
| 9521:254  | $0, 0, 0, 0, e^{12}, -e^{13}, e^{23} + e^{14}, -2e^{17} + e^{26} + e^{35}, e^{56} + e^{18}$                             | 1259     |
| 9521:258  | $0, 0, 0, 0, e^{12}, -e^{13}, e^{23} + e^{14}, e^{35} - 2e^{17} + e^{26}, e^{56} + e^{24} + e^{18}$                     | 1259     |
| Type: 324 |                                                                                                                         |          |
| 964:1     | $0, 0, 0, 0, e^{12}, e^{13}, e^{14}, e^{24}, e^{15}, e^{35}$                                                            | 469      |
| 964:2     | $0, 0, 0, 0, e^{12}, e^{13}, e^{14}, e^{24}, e^{35}, e^{15} + e^{23}$                                                   | 469      |
| 964:3     | $0, 0, 0, 0, e^{12}, e^{13}, e^{14}, e^{24}, e^{15}, e^{25} + e^{34}$                                                   | 469      |
| 964:4     | $0, 0, 0, 0, e^{12}, e^{13}, e^{14}, e^{24}, e^{35}, e^{25} + e^{34}$                                                   | 469      |
| 964:5     | $0, 0, 0, 0, e^{12}, e^{13}, e^{14}, e^{24}, e^{15} + e^{23}, e^{25} + e^{34}$                                          | 469      |
| 964:6     | $0, 0, 0, 0, e^{12}, e^{13}, e^{24}, e^{23} + e^{14}, e^{15}, e^{25} + e^{34}$                                          | 469      |
| 964:7     | $0, 0, 0, 0, e^{12}, e^{13}, e^{24}, e^{14} + e^{23}, e^{35}, e^{34} + e^{25}$                                          | 469      |
| 964:8a    | $0, 0, 0, 0, e^{12}, e^{13}, e^{14}, e^{15}, e^{25} + e^{34}, e^{35} + e^{24}$                                          | 469      |
| 964:8b    | $0, 0, 0, -e^{12}, e^{13}, e^{14}, e^{15}, e^{34} - e^{25}, e^{35} + e^{24}$                                            | 469      |
| 964:9     | $0, 0, 0, 0, e^{12}, e^{13}, e^{24}, e^{15}, e^{35} + e^{14}, e^{25} + e^{34}$                                          | 469      |
| 964:10a   | $0, 0, 0, 0, e^{12}, e^{13}, e^{14}, e^{15} + e^{23}, e^{25} + e^{34}, e^{24} + e^{35}$                                 | 469      |
| 964:10b   | $0, 0, 0, -e^{12}, e^{13}, e^{14}, e^{15} + e^{23}, -e^{25} + e^{34}, e^{24} + e^{35}$                                  | 469      |
| 964:11    | $0, 0, 0, 0, e^{12}, e^{13}, e^{24}, e^{15} + e^{23}, e^{35} + e^{14}, e^{34} + e^{25}$                                 | 469      |
| Type: 423 |                                                                                                                         |          |
| 953:1     | $0, 0, 0, 0, e^{12}, e^{13}, e^{15}, e^{25}, e^{16}$                                                                    | 469      |
| 953:2     | $0, 0, 0, 0, e^{12}, e^{13}, e^{15}, e^{25}, e^{36}$                                                                    | 469      |
| 953:3     | $0, 0, 0, 0, e^{12}, e^{13}, e^{15}, e^{25}, e^{23} + e^{16}$                                                           | 469      |
| 953:4     | $0, 0, 0, 0, e^{12}, e^{13}, e^{25}, e^{15} + e^{23}, e^{16}$                                                           | 469      |
| 953:5     | $0, 0, 0, 0, e^{12}, e^{13}, e^{25}, e^{15} + e^{23}, e^{36}$                                                           | 469      |
| 953:6     | $0, 0, 0, 0, e^{12}, e^{13}, e^{15}, e^{25}, e^{16} + e^{24}$                                                           | 369      |
| 953:7     | $0, 0, 0, 0, e^{12}, e^{13}, e^{15}, e^{25}, e^{14} + e^{36}$                                                           | 369      |
| 953:8     | $0, 0, 0, 0, e^{12}, e^{13}, e^{15}, e^{25}, e^{16} + e^{34}$                                                           | 369      |
| 953:9     | $0, 0, 0, 0, e^{12}, e^{13}, e^{15}, e^{25}, e^{24} + e^{36}$                                                           | 369      |
| 953:10    | $0, 0, 0, 0, e^{12}, e^{13}, e^{15}, e^{25} + e^{14}, e^{16}$                                                           | 369      |
| 953:11    | $0, 0, 0, 0, e^{12}, e^{13}, e^{25}, e^{15} + e^{24}, e^{16}$                                                           | 369      |
| 953:12    | $0, 0, 0, 0, e^{12}, e^{13}, e^{15}, e^{25} + e^{14}, e^{36}$                                                           | 369      |
| 953:13    | $0, 0, 0, 0, e^{12}, e^{13}, e^{25}, e^{15} + e^{24}, e^{36}$                                                           | 369      |
| 953:14    | $0, 0, 0, 0, e^{12}, e^{13}, e^{15}, e^{25} + e^{34}, e^{16}$                                                           | 369      |
| 953:15    | $0, 0, 0, 0, e^{12}, e^{13}, e^{25}, e^{15} + e^{34}, e^{16}$                                                           | 369      |
| 953:16    | $0, 0, 0, 0, e^{12}, e^{13}, e^{15}, e^{34} + e^{25}, e^{36}$                                                           | 369      |
| 953:17    | $0, 0, 0, 0, e^{12}, e^{13}, e^{25}, e^{15} + e^{34}, e^{36}$                                                           | 369      |
| 953:18    | $0, 0, 0, 0, e^{12}, e^{13}, e^{15}, e^{25}, e^{26} + e^{35}$                                                           | 469      |
| 953:19a   | $0, 0, 0, 0, e^{12}, e^{13}, e^{15}, e^{16}, e^{36} + e^{25}$                                                           | 469      |
| 953:19b   | $0, 0, 0, 0, -e^{12}, e^{13}, e^{15}, e^{16}, e^{25} + e^{36}$                                                          | 469      |
| 953:20    | $0, 0, 0, 0, e^{12}, e^{13}, e^{15}, e^{16}, e^{26} + e^{35}$                                                           | 469      |
| 953:21    | $0, 0, 0, 0, e^{12}, e^{13}, e^{25}, e^{16}, e^{36} + e^{15}$                                                           | 469      |
| 953:22    | $0, 0, 0, 0, e^{12}, e^{13}, e^{25}, e^{16}, e^{35} + e^{26}$                                                           | 469      |
| 953:23    | $0, 0, 0, 0, e^{12}, e^{13}, e^{25}, e^{36}, e^{26} + e^{35}$                                                           | 469      |
| 953:24    | $0, 0, 0, 0, e^{12}, e^{13}, e^{15}, e^{25} + e^{14}, e^{16} + e^{24}$                                                  | 369      |
| 953:25a   | $0, 0, 0, 0, e^{12}, e^{13}, e^{15}, e^{14} + e^{25}, e^{16} + e^{34}$                                                  | 369      |

Table 2 – Continued to next page

Table 2 – Continued from previous page

| Name    | $\mathfrak{g}$                                                            | UCS Dim. |
|---------|---------------------------------------------------------------------------|----------|
| 953:25b | $0, 0, 0, 0, -e^{12}, e^{13}, e^{15}, e^{25} + e^{14}, e^{34} + e^{16}$   | 369      |
| 953:26  | $0, 0, 0, 0, e^{12}, e^{13}, e^{15}, e^{25} + e^{14}, e^{24} + e^{36}$    | 369      |
| 953:27a | $0, 0, 0, 0, e^{12}, e^{13}, e^{25}, e^{24} + e^{15}, e^{36} + e^{14}$    | 369      |
| 953:27b | $0, 0, 0, 0, -e^{12}, e^{13}, e^{25}, e^{24} + e^{15}, e^{36} + e^{14}$   | 369      |
| 953:28  | $0, 0, 0, 0, e^{12}a_1, e^{13}, e^{25}, e^{15} + e^{24}, e^{34} + e^{16}$ | 369      |
| 953:29  | $0, 0, 0, 0, e^{12}, e^{13}, e^{15}, e^{25} + e^{34}, e^{16} + e^{24}$    | 369      |
| 953:30a | $0, 0, 0, 0, e^{12}, e^{13}, e^{25}, e^{15} + e^{34}, e^{16} + e^{24}$    | 369      |
| 953:30b | $0, 0, 0, 0, -e^{12}, e^{13}, e^{25}, e^{34} + e^{15}, e^{16} + e^{24}$   | 369      |
| 953:31  | $0, 0, 0, 0, e^{12}, e^{13}, e^{15}, e^{34} + e^{25}, e^{14} + e^{36}$    | 369      |
| 953:32  | $0, 0, 0, 0, e^{12}, e^{13}, e^{15}, e^{25} + e^{34}, e^{24} + e^{36}$    | 369      |
| 953:33  | $0, 0, 0, 0, e^{12}, e^{13}, e^{25}, e^{34} + e^{15}, e^{36} + e^{14}$    | 369      |
| 953:34  | $0, 0, 0, 0, e^{12}, e^{13}, e^{25}, e^{15} + e^{34}, e^{24} + e^{36}$    | 369      |
| 953:35a | $0, 0, 0, 0, e^{12}, e^{13}, e^{24} + e^{15}, e^{25} + e^{14}, e^{16}$    | 369      |
| 953:35b | $0, 0, 0, 0, e^{12}, e^{13}, -e^{15} + e^{24}, e^{25} + e^{14}, e^{16}$   | 369      |
| 953:36a | $0, 0, 0, 0, e^{12}, e^{13}, e^{15} + e^{24}, e^{14} + e^{25}, e^{36}$    | 369      |
| 953:36b | $0, 0, 0, 0, e^{12}, e^{13}, -e^{15} + e^{24}, e^{25} + e^{14}, e^{36}$   | 369      |
| 953:37  | $0, 0, 0, 0, e^{12}, e^{13}, e^{14} + e^{25}, e^{15} + e^{34}, e^{16}$    | 369      |
| 953:38  | $0, 0, 0, 0, e^{12}, e^{13}, e^{24} + e^{15}, e^{25} + e^{34}, e^{16}$    | 369      |
| 953:39  | $0, 0, 0, 0, e^{12}, e^{13}, e^{25} + e^{14}, e^{34} + e^{15}, e^{36}$    | 369      |
| 953:40  | $0, 0, 0, 0, e^{12}, e^{13}, e^{15} + e^{24}, e^{34} + e^{25}, e^{36}$    | 369      |
| 953:41  | $0, 0, 0, 0, e^{12}, e^{13}, e^{25}, e^{15} + e^{23}, e^{16} + e^{24}$    | 369      |
| 953:42  | $0, 0, 0, 0, e^{12}, e^{13}, e^{25}, e^{15} + e^{23}, e^{36} + e^{14}$    | 369      |
| 953:43  | $0, 0, 0, 0, e^{12}, e^{13}, e^{25}, e^{15} + e^{23}, e^{16} + e^{34}$    | 369      |
| 953:44  | $0, 0, 0, 0, e^{12}, e^{13}, e^{25}, e^{15} + e^{23}, e^{24} + e^{36}$    | 369      |
| 953:45  | $0, 0, 0, 0, e^{12}, e^{13}, e^{15}, e^{25} + e^{14}, e^{23} + e^{16}$    | 369      |
| 953:46  | $0, 0, 0, 0, e^{12}, e^{13}, e^{25}, e^{24} + e^{15}, e^{23} + e^{16}$    | 369      |
| 953:47  | $0, 0, 0, 0, e^{12}, e^{13}, e^{15}, e^{25} + e^{34}, e^{16} + e^{23}$    | 369      |
| 953:48  | $0, 0, 0, 0, e^{12}, e^{13}, e^{25}, e^{15} + e^{34}, e^{23} + e^{16}$    | 369      |
| 953:49  | $0, 0, 0, 0, e^{12}, e^{13}, e^{23} + e^{15}, e^{25} + e^{14}, e^{16}$    | 369      |
| 953:50  | $0, 0, 0, 0, e^{12}, e^{13}, e^{15} + e^{23}, e^{25} + e^{14}, e^{36}$    | 369      |
| 953:51  | $0, 0, 0, 0, e^{12}, e^{13}, e^{15} + e^{23}, e^{25} + e^{34}, e^{16}$    | 369      |
| 953:52  | $0, 0, 0, 0, e^{12}, e^{13}, e^{15} + e^{23}, e^{34} + e^{25}, e^{36}$    | 369      |
| 953:53  | $0, 0, 0, 0, e^{12}, e^{13}, e^{25}, e^{15} + e^{23}, e^{35} + e^{26}$    | 469      |
| 953:54a | $0, 0, 0, 0, e^{12}, e^{13}, e^{15}, e^{16} + e^{23}, e^{36} + e^{25}$    | 469      |
| 953:54b | $0, 0, 0, 0, -e^{12}, e^{13}, e^{15}, e^{23} + e^{16}, e^{36} + e^{25}$   | 469      |
| 953:55  | $0, 0, 0, 0, e^{12}, e^{13}, e^{15}, e^{23} + e^{16}, e^{26} + e^{35}$    | 469      |
| 953:56  | $0, 0, 0, 0, e^{12}, e^{13}, e^{25}, e^{16} + e^{23}, e^{15} + e^{36}$    | 469      |
| 953:57  | $0, 0, 0, 0, e^{12}, e^{13}, e^{25}, e^{23} + e^{16}, e^{35} + e^{26}$    | 469      |
| 953:58  | $0, 0, 0, 0, e^{12}, e^{13}, e^{15}, e^{25}, e^{35} + e^{14} + e^{26}$    | 369      |
| 953:59  | $0, 0, 0, 0, e^{12}, e^{13}, e^{15}, e^{25} + e^{14}, e^{26} + e^{35}$    | 369      |
| 953:60  | $0, 0, 0, 0, e^{12}, e^{13}, e^{25}, e^{15} + e^{24}, e^{26} + e^{35}$    | 369      |
| 953:61  | $0, 0, 0, 0, e^{12}, e^{13}, e^{15}, e^{25} + e^{34}, e^{26} + e^{35}$    | 369      |
| 953:62  | $0, 0, 0, 0, e^{12}, e^{13}, e^{25}, e^{15} + e^{34}, e^{35} + e^{26}$    | 369      |
| 953:63a | $0, 0, 0, 0, e^{12}, e^{13}, e^{15}, e^{16}, e^{36} + e^{25} + e^{14}$    | 369      |
| 953:63b | $0, 0, 0, 0, -e^{12}, e^{13}, e^{15}, e^{16}, e^{14} + e^{36} + e^{25}$   | 369      |
| 953:64  | $0, 0, 0, 0, e^{12}, e^{13}, e^{15}, e^{16}, e^{26} + e^{35} + e^{14}$    | 369      |
| 953:65  | $0, 0, 0, 0, e^{12}, e^{13}, e^{25}, e^{16}, e^{36} + e^{15} + e^{24}$    | 369      |
| 953:66  | $0, 0, 0, 0, e^{12}, e^{13}, e^{25}, e^{16}, e^{35} + e^{26} + e^{14}$    | 369      |
| 953:67  | $0, 0, 0, 0, e^{12}, e^{13}, e^{25}, e^{36}, e^{26} + e^{35} + e^{14}$    | 369      |
| 953:68a | $0, 0, 0, 0, e^{12}, e^{13}, e^{15}, e^{16} + e^{24}, e^{36} + e^{25}$    | 369      |
| 953:68b | $0, 0, 0, 0, -e^{12}, e^{13}, e^{15}, e^{16} + e^{24}, e^{25} + e^{36}$   | 369      |
| 953:69  | $0, 0, 0, 0, e^{12}, e^{13}, e^{15}, e^{16} + e^{24}, e^{26} + e^{35}$    | 369      |
| 953:70  | $0, 0, 0, 0, e^{12}, e^{13}, e^{25}, e^{24} + e^{16}, e^{36} + e^{15}$    | 369      |
| 953:71  | $0, 0, 0, 0, e^{12}, e^{13}, e^{25}, e^{24} + e^{16}, e^{35} + e^{26}$    | 369      |
| 953:72  | $0, 0, 0, 0, e^{12}, e^{13}, e^{15}, e^{36} + e^{14}, e^{25} + e^{16}$    | 369      |
| 953:73  | $0, 0, 0, 0, e^{12}, e^{13}, e^{15}, e^{36} + e^{24}, e^{16} + e^{25}$    | 369      |
| 953:74a | $0, 0, 0, 0, e^{12}, e^{13}, e^{15}, e^{16} + e^{34}, e^{25} + e^{36}$    | 369      |
| 953:74b | $0, 0, 0, 0, -e^{12}, e^{13}, e^{15}, e^{16} + e^{34}, e^{36} + e^{25}$   | 369      |

Table 2 – Continued to next page



Table 2 – Continued from previous page

| Name     | $\mathfrak{g}$                                                                       | UCS Dim. |
|----------|--------------------------------------------------------------------------------------|----------|
| 953:75   | $0, 0, 0, 0, e^{12}, e^{13}, e^{15}, e^{14} + e^{36}, e^{26} + e^{35}$               | 369      |
| 953:76   | $0, 0, 0, 0, e^{12}, e^{13}, e^{15}, e^{16} + e^{34}, e^{35} + e^{26}$               | 369      |
| 953:77   | $0, 0, 0, 0, e^{12}, e^{13}, e^{15}, e^{24} + e^{36}, e^{26} + e^{35}$               | 369      |
| 953:78   | $0, 0, 0, 0, e^{12}, e^{13}, e^{25}, e^{16} + e^{34}, e^{15} + e^{36}$               | 369      |
| 953:79   | $0, 0, 0, 0, e^{12}, e^{13}, e^{25}, e^{14} + e^{36}, e^{26} + e^{35}$               | 369      |
| 953:80   | $0, 0, 0, 0, e^{12}, e^{13}, e^{25}, e^{16} + e^{34}, e^{35} + e^{26}$               | 369      |
| 953:81   | $0, 0, 0, 0, e^{12}, e^{13}, e^{25}, e^{24} + e^{36}, e^{26} + e^{35}$               | 369      |
| 953:82   | $0, 0, 0, 0, e^{12}, e^{13}, e^{15}, e^{16} + e^{25}, e^{26} + e^{35}$               | 469      |
| 953:83a  | $0, 0, 0, 0, e^{12}, e^{13}, e^{15}, e^{26} + e^{35}, e^{36} + e^{25}$               | 469      |
| 953:83b  | $0, 0, 0, 0, -e^{12}, e^{13}, e^{15}, e^{35} - e^{26}, e^{36} + e^{25}$              | 469      |
| 953:84   | $0, 0, 0, 0, e^{12}, e^{13}, e^{25}, e^{36} + e^{15}, e^{26} + e^{35}$               | 469      |
| 953:85a  | $0, 0, 0, 0, e^{12}, e^{13}, e^{24} + a_1 e^{15}, e^{25} + e^{14}, e^{16} + e^{34}$  | 369      |
| 953:85b  | $0, 0, 0, 0, -e^{12}, e^{13}, e^{24} + a_1 e^{15}, e^{14} + e^{25}, e^{16} + e^{34}$ | 369      |
| 953:86a  | $0, 0, 0, 0, e^{12}, e^{13}, e^{25} + e^{14}, e^{34} + e^{15}, e^{24} + e^{16}$      | 369      |
| 953:86b  | $0, 0, 0, 0, -e^{12}, e^{13}, e^{14} + e^{25}, e^{15} + e^{34}, e^{24} + e^{16}$     | 369      |
| 953:87   | $0, 0, 0, 0, e^{12}, e^{13}, e^{25} + e^{14}, e^{34} + e^{15}, e^{24} + e^{36}$      | 369      |
| 953:88a  | $0, 0, 0, 0, e^{12}, e^{13}, e^{15} + e^{24}, e^{34} + e^{25}, e^{36} + e^{14}$      | 369      |
| 953:88b  | $0, 0, 0, 0, -e^{12}, e^{13}, e^{15} + e^{24}, e^{34} + e^{25}, e^{14} + e^{36}$     | 369      |
| 953:89   | $0, 0, 0, 0, e^{12}, e^{13}, e^{15} + e^{23}, e^{25} + e^{14}, e^{16} + e^{24}$      | 369      |
| 953:90a  | $0, 0, 0, 0, e^{12}, e^{13}, e^{15} + e^{23}, e^{14} + e^{25}, e^{16} + e^{34}$      | 369      |
| 953:90b  | $0, 0, 0, 0, -e^{12}, e^{13}, e^{15} + e^{23}, e^{25} + e^{14}, e^{16} + e^{34}$     | 369      |
| 953:91   | $0, 0, 0, 0, e^{12}, e^{13}, e^{15} + e^{23}, e^{14} + e^{25}, e^{24} + e^{36}$      | 369      |
| 953:92   | $0, 0, 0, 0, e^{12}, e^{13}, e^{23} + e^{15}, e^{25} + e^{34}, e^{24} + e^{16}$      | 369      |
| 953:93   | $0, 0, 0, 0, e^{12}, e^{13}, e^{15} + e^{23}, e^{25} + e^{34}, e^{36} + e^{14}$      | 369      |
| 953:94   | $0, 0, 0, 0, e^{12}, e^{13}, e^{15} + e^{23}, e^{25} + e^{34}, e^{24} + e^{36}$      | 369      |
| 953:95a  | $0, 0, 0, 0, e^{12}, e^{13}, e^{24} + e^{15}, e^{25} + e^{14}, e^{16} + e^{23}$      | 369      |
| 953:95b  | $0, 0, 0, 0, e^{12}, e^{13}, -e^{15} + e^{24}, e^{25} + e^{14}, e^{16} + e^{23}$     | 369      |
| 953:96   | $0, 0, 0, 0, e^{12}, e^{13}, e^{14} + e^{25}, e^{15} + e^{34}, e^{16} + e^{23}$      | 369      |
| 953:97   | $0, 0, 0, 0, e^{12}, e^{13}, e^{15} + e^{24}, e^{25} + e^{34}, e^{23} + e^{16}$      | 369      |
| 953:98   | $0, 0, 0, 0, e^{12}, e^{13}, e^{25}, e^{24} + e^{15}, e^{35} + e^{26} + e^{14}$      | 369      |
| 953:99   | $0, 0, 0, 0, e^{12}, e^{13}, e^{15}, e^{25} + e^{34}, e^{26} + e^{35} + e^{14}$      | 369      |
| 953:100a | $0, 0, 0, 0, e^{12}, e^{13}, e^{25}, e^{15} + e^{34}, e^{14} + e^{26} + e^{35}$      | 369      |
| 953:100b | $0, 0, 0, 0, e^{12}, e^{13}, e^{25}, -e^{15} + e^{34}, e^{14} + e^{26} + e^{35}$     | 369      |
| 953:101a | $0, 0, 0, 0, e^{12}, e^{13}, e^{24} + e^{15}, e^{25} + e^{14}, e^{35} + e^{26}$      | 369      |
| 953:101b | $0, 0, 0, 0, e^{12}, e^{13}, e^{24} - e^{15}, e^{25} + e^{14}, e^{26} + e^{35}$      | 369      |
| 953:102  | $0, 0, 0, 0, e^{12}, e^{13}, e^{25} + e^{14}, e^{34} + e^{15}, e^{26} + e^{35}$      | 369      |
| 953:103  | $0, 0, 0, 0, e^{12}, e^{13}, e^{15} + e^{24}, e^{25} + e^{34}, e^{26} + e^{35}$      | 369      |
| 953:104a | $0, 0, 0, 0, e^{12}, e^{13}, e^{15}, e^{16} + e^{24}, e^{14} + e^{25} + e^{36}$      | 369      |
| 953:104b | $0, 0, 0, 0, -e^{12}, e^{13}, e^{15}, e^{24} + e^{16}, e^{36} + e^{14} + e^{25}$     | 369      |
| 953:105a | $0, 0, 0, 0, e^{12}, e^{13}, e^{15}, e^{24} + e^{16}, e^{26} + e^{35} + e^{14}$      | 369      |
| 953:105b | $0, 0, 0, 0, e^{12}, e^{13}, e^{15}, -e^{16} + e^{24}, e^{14} + e^{26} + e^{35}$     | 369      |
| 953:106a | $0, 0, 0, 0, e^{12}, e^{13}, e^{25}, e^{16} + e^{24}, e^{14} + e^{26} + e^{35}$      | 369      |
| 953:106b | $0, 0, 0, 0, e^{12}, e^{13}, e^{25}, -e^{16} + e^{24}, e^{14} + e^{35} + e^{26}$     | 369      |
| 953:107a | $0, 0, 0, 0, e^{12}, e^{13}, e^{15}, e^{36} + e^{14}, e^{25} + e^{34} + e^{16}$      | 369      |
| 953:107b | $0, 0, 0, 0, e^{12}, e^{13}, e^{15}, -e^{14} + e^{36}, e^{25} + e^{16} + e^{34}$     | 369      |
| 953:108a | $0, 0, 0, 0, e^{12}, e^{13}, e^{15}, e^{16} + e^{34}, e^{36} + e^{25} + e^{14}$      | 369      |
| 953:108b | $0, 0, 0, 0, e^{12}, e^{13}, e^{15}, -e^{16} + e^{34}, e^{25} + e^{36} + e^{14}$     | 369      |
| 953:108c | $0, 0, 0, 0, -e^{12}, e^{13}, e^{15}, e^{16} + e^{34}, e^{14} + e^{36} + e^{25}$     | 369      |
| 953:108d | $0, 0, 0, 0, -e^{12}, e^{13}, e^{15}, -e^{16} + e^{34}, e^{25} + e^{14} + e^{36}$    | 369      |
| 953:109  | $0, 0, 0, 0, e^{12}, e^{13}, e^{15}, e^{16} + e^{34}, e^{14} + e^{35} + e^{26}$      | 369      |
| 953:110  | $0, 0, 0, 0, e^{12}, e^{13}, e^{15}, e^{24} + e^{36}, e^{26} + e^{35} + e^{14}$      | 369      |
| 953:111  | $0, 0, 0, 0, e^{12}, e^{13}, e^{15}, e^{36} + e^{24}, e^{34} + e^{16} + e^{25}$      | 369      |
| 953:112  | $0, 0, 0, 0, a_1 e^{12}, e^{13}, e^{25}, e^{16} + e^{34}, e^{15} + e^{36} + e^{24}$  | 369      |
| 953:113  | $0, 0, 0, 0, e^{12}, e^{13}, e^{25}, e^{16} + e^{34}, e^{14} + e^{26} + e^{35}$      | 369      |
| 953:114  | $0, 0, 0, 0, e^{12}, e^{13}, e^{25}, e^{24} + e^{36}, e^{35} + e^{14} + e^{26}$      | 369      |
| 953:115  | $0, 0, 0, 0, e^{12}, e^{13}, e^{25} + e^{14}, e^{16} + e^{24}, e^{15} + e^{36}$      | 369      |
| 953:116  | $0, 0, 0, 0, e^{12}, e^{13}, e^{25} + e^{14}, e^{16} + e^{24}, e^{26} + e^{35}$      | 369      |
| 953:117a | $0, 0, 0, 0, e^{12}, e^{13}, e^{15} + e^{24}, e^{14} + e^{36}, e^{16} + e^{25}$      | 369      |

Table 2 – Continued to next page

Table 2 – Continued from previous page

| Name     | $\mathfrak{g}$                                                                                | UCS Dim. |
|----------|-----------------------------------------------------------------------------------------------|----------|
| 953:117b | $0, 0, 0, 0, -e^{12}, e^{13}, e^{15} + e^{24}, e^{36} + e^{14}, e^{25} + e^{16}$              | 369      |
| 953:118a | $0, 0, 0, 0, e^{12}, e^{13}, e^{15}a_1 + e^{24}, e^{16} + e^{34}, e^{25} + e^{36}$            | 369      |
| 953:118b | $0, 0, 0, 0, -e^{12}, e^{13}, e^{15}a_1 + e^{24}, e^{34} + e^{16}, e^{36} + e^{25}$           | 369      |
| 953:119a | $0, 0, 0, 0, e^{12}, e^{13}, e^{15} + e^{24}, e^{14} + e^{36}, e^{26} + e^{35}$               | 369      |
| 953:119b | $0, 0, 0, 0, e^{12}, e^{13}, -e^{15} + e^{24}, e^{14} + e^{36}, e^{26} + e^{35}$              | 369      |
| 953:120  | $0, 0, 0, 0, e^{12}, e^{13}, e^{24} + e^{15}a_2, e^{16} + e^{34}, e^{35} + e^{26}$            | 369      |
| 953:121  | $0, 0, 0, 0, e^{12}, e^{13}, e^{25} + e^{14}, e^{36} + e^{24}, e^{26} + e^{35}$               | 369      |
| 953:122a | $0, 0, 0, 0, e^{12}, e^{13}, a_1e^{15} + e^{34}, e^{16} + e^{24}, e^{36} + e^{25}$            | 369      |
| 953:122b | $0, 0, 0, 0, -e^{12}, e^{13}, a_1e^{15} + e^{34}, e^{24} + e^{16}, e^{25} + e^{36}$           | 369      |
| 953:123a | $0, 0, 0, 0, e^{12}, e^{13}, e^{34} + e^{15}, e^{24} + e^{16}, e^{26} + e^{35}$               | 369      |
| 953:123b | $0, 0, 0, 0, e^{12}, e^{13}, -e^{15} + e^{34}, e^{16} + e^{24}, e^{26} + e^{35}$              | 369      |
| 953:124a | $0, 0, 0, 0, e^{12}, e^{13}, e^{25} + e^{34}, e^{16} + e^{24}, e^{15} + e^{36}$               | 369      |
| 953:124b | $0, 0, 0, 0, e^{12}, e^{13}, e^{34} + e^{25}, -e^{16} + e^{24}, e^{36} + e^{15}$              | 369      |
| 953:125  | $0, 0, 0, 0, e^{12}, e^{13}, e^{34} + e^{25}, e^{24} + e^{16}, e^{35} + e^{26}$               | 369      |
| 953:126  | $0, 0, 0, 0, e^{12}, e^{13}, e^{25} + e^{34}, e^{24} + e^{36}, e^{26} + e^{35}$               | 369      |
| 953:127  | $0, 0, 0, 0, e^{12}, e^{13}, e^{25}, e^{23} + e^{15}, e^{26} + e^{35} + e^{14}$               | 369      |
| 953:128  | $0, 0, 0, 0, e^{12}, e^{13}, e^{15} + e^{23}, e^{14} + e^{25}, e^{26} + e^{35}$               | 369      |
| 953:129  | $0, 0, 0, 0, e^{12}, e^{13}, e^{15} + e^{23}, e^{34} + e^{25}, e^{35} + e^{26}$               | 369      |
| 953:130a | $0, 0, 0, 0, e^{12}, e^{13}, e^{15}, e^{16} + e^{23}, e^{36} + e^{25} + e^{14}$               | 369      |
| 953:130b | $0, 0, 0, 0, -e^{12}, e^{13}, e^{15}, e^{23} + e^{16}, e^{36} + e^{25} + e^{14}$              | 369      |
| 953:131  | $0, 0, 0, 0, e^{12}, e^{13}, e^{15}, e^{23} + e^{16}, e^{14} + e^{26} + e^{35}$               | 369      |
| 953:132  | $0, 0, 0, 0, e^{12}, e^{13}, e^{25}, e^{16} + e^{23}, e^{15} + e^{24} + e^{36}$               | 369      |
| 953:133  | $0, 0, 0, 0, e^{12}, e^{13}, e^{25}, e^{23} + e^{16}, e^{14} + e^{26} + e^{35}$               | 369      |
| 953:134a | $0, 0, 0, 0, e^{12}, e^{13}, e^{23} + e^{15}, e^{24} + e^{16}, e^{36} + e^{25}$               | 369      |
| 953:134b | $0, 0, 0, 0, -e^{12}, e^{13}, e^{15} + e^{23}, e^{24} + e^{16}, e^{36} + e^{25}$              | 369      |
| 953:135  | $0, 0, 0, 0, e^{12}, e^{13}, e^{15} + e^{23}, e^{16} + e^{24}, e^{26} + e^{35}$               | 369      |
| 953:136  | $0, 0, 0, 0, e^{12}, e^{13}, e^{15} + e^{23}, e^{36} + e^{14}, e^{16} + e^{25}$               | 369      |
| 953:137  | $0, 0, 0, 0, e^{12}, e^{13}, e^{15} + e^{23}, e^{24} + e^{36}, e^{16} + e^{25}$               | 369      |
| 953:138a | $0, 0, 0, 0, e^{12}, e^{13}, e^{15} + e^{23}, e^{16} + e^{34}, e^{25} + e^{36}$               | 369      |
| 953:138b | $0, 0, 0, 0, -e^{12}, e^{13}, e^{15} + e^{23}, e^{16} + e^{34}, e^{25} + e^{36}$              | 369      |
| 953:139  | $0, 0, 0, 0, e^{12}, e^{13}, e^{23} + e^{15}, e^{36} + e^{14}, e^{35} + e^{26}$               | 369      |
| 953:140  | $0, 0, 0, 0, e^{12}, e^{13}, e^{15} + e^{23}, e^{34} + e^{16}, e^{35} + e^{26}$               | 369      |
| 953:141  | $0, 0, 0, 0, e^{12}, e^{13}, e^{15} + e^{23}, e^{36} + e^{24}, e^{26} + e^{35}$               | 369      |
| 953:142  | $0, 0, 0, 0, e^{12}, e^{13}, e^{15} + e^{23}, e^{25} + e^{16}, e^{26} + e^{35}$               | 469      |
| 953:143a | $0, 0, 0, 0, e^{12}, e^{13}, e^{23} + e^{15}, e^{35} + e^{26}, e^{36} + e^{25}$               | 469      |
| 953:143b | $0, 0, 0, 0, -e^{12}, e^{13}, e^{23} + e^{15}, -e^{26} + e^{35}, e^{36} + e^{25}$             | 469      |
| 953:144  | $0, 0, 0, 0, e^{12}, e^{13}, e^{15}, e^{16} + e^{25}, e^{26} + e^{35} + e^{14}$               | 369      |
| 953:145a | $0, 0, 0, 0, e^{12}, e^{13}, e^{15}, e^{36} + e^{25}, e^{35} + e^{14} + e^{26}$               | 369      |
| 953:145b | $0, 0, 0, 0, e^{12}, e^{13}, e^{15}, e^{36} - e^{25}, e^{35} + e^{14} + e^{26}$               | 369      |
| 953:146a | $0, 0, 0, 0, e^{12}, e^{13}, e^{15}, e^{35} + e^{26}, e^{36} + e^{25} + e^{14}$               | 369      |
| 953:146b | $0, 0, 0, 0, -e^{12}, e^{13}, e^{15}, -e^{26} + e^{35}, e^{14} + e^{36} + e^{25}$             | 369      |
| 953:147  | $0, 0, 0, 0, e^{12}, e^{13}, e^{15}, e^{26} + e^{35}, e^{25} + e^{16} + e^{34}$               | 369      |
| 953:148  | $0, 0, 0, 0, e^{12}, e^{13}, e^{25}, e^{36} + e^{15}, e^{35} + e^{14} + e^{26}$               | 369      |
| 953:149  | $0, 0, 0, 0, e^{12}, e^{13}, e^{25}, e^{26} + e^{35}, e^{15} + e^{24} + e^{36}$               | 369      |
| 953:150  | $0, 0, 0, 0, e^{12}, e^{13}, e^{15} + e^{24}, e^{16} + e^{25}, e^{26} + e^{35}$               | 369      |
| 953:151  | $0, 0, 0, 0, e^{12}, e^{13}, e^{25} + e^{14}, e^{15} + e^{36}, e^{26} + e^{35}$               | 369      |
| 953:152a | $0, 0, 0, 0, e^{12}, e^{13}, e^{24} + e^{15}, e^{35} + e^{26}, e^{36} + e^{25}$               | 369      |
| 953:152b | $0, 0, 0, 0, -e^{12}, e^{13}, e^{15} + e^{24}, -e^{26} + e^{35}, e^{36} + e^{25}$             | 369      |
| 953:153  | $0, 0, 0, 0, e^{12}, e^{13}, e^{15} + e^{34}, e^{16} + e^{25}, e^{26} + e^{35}$               | 369      |
| 953:154a | $0, 0, 0, 0, e^{12}, e^{13}, e^{34} + e^{15}, e^{35} + e^{26}, e^{36} + e^{25}$               | 369      |
| 953:154b | $0, 0, 0, 0, -e^{12}, e^{13}, e^{34} + e^{15}, -e^{26} + e^{35}, e^{36} + e^{25}$             | 369      |
| 953:155  | $0, 0, 0, 0, e^{12}, e^{13}, e^{25} + e^{34}, e^{15} + e^{36}, e^{26} + e^{35}$               | 369      |
| 953:156  | $0, 0, 0, 0, e^{12}, e^{13}, e^{16} + e^{25}, e^{15} + e^{36}, e^{26} + e^{35}$               | 469      |
| 953:157  | $0, 0, 0, 0, e^{12}, e^{13}, e^{15} + e^{24}, e^{34} + e^{25}, e^{35} + e^{14} + e^{26}$      | 369      |
| 953:158a | $0, 0, 0, 0, a_1e^{12}, e^{13}, e^{24} + e^{15}, e^{36} + e^{14}, e^{16} + e^{25} + e^{34}$   | 369      |
| 953:158b | $0, 0, 0, 0, a_1e^{12}, e^{13}, e^{15} + e^{24}, e^{36} - e^{14}, e^{34} + e^{25} + e^{16}$   | 369      |
| 953:159a | $0, 0, 0, 0, e^{12}, e^{13}, e^{15} + e^{24}, a_1e^{16} + e^{34}, e^{25} + e^{36} + e^{14}$   | 369      |
| 953:159b | $0, 0, 0, 0, e^{12}, e^{13}, -e^{15} + e^{24}, -a_1e^{16} + e^{34}, e^{36} + e^{25} + e^{14}$ | 369      |

Table 2 – Continued to next page

Table 2 – Continued from previous page

| Name     | $\mathfrak{g}$                                                                                        | UCS Dim. |
|----------|-------------------------------------------------------------------------------------------------------|----------|
| 953:159c | $0, 0, 0, 0, -e^{12}, e^{13}, e^{15} + e^{24}, a_1 e^{16} + e^{34}, e^{14} + e^{25} + e^{36}$         | 369      |
| 953:159d | $0, 0, 0, 0, -e^{12}, e^{13}, e^{24} - e^{15}, -a_1 e^{16} + e^{34}, e^{36} + e^{25} + e^{14}$        | 369      |
| 953:160  | $0, 0, 0, 0, e^{12}, e^{13}, e^{24} + e^{15} a_2, e^{16} + e^{34}, e^{14} + e^{26} + e^{35}$          | 369      |
| 953:161a | $0, 0, 0, 0, e^{12}, e^{13}, e^{34} + e^{15} a_1, e^{16} + e^{24}, e^{25} + e^{14} + e^{36}$          | 369      |
| 953:161b | $0, 0, 0, 0, -e^{12}, e^{13}, e^{34} + e^{15} a_1, e^{24} + e^{16}, e^{36} + e^{14} + e^{25}$         | 369      |
| 953:162a | $0, 0, 0, 0, e^{12}, e^{13}, e^{34} + e^{15}, e^{16} + e^{24}, e^{35} + e^{14} + e^{26}$              | 369      |
| 953:162b | $0, 0, 0, 0, e^{12}, e^{13}, e^{15} + e^{34}, -e^{16} + e^{24}, e^{26} + e^{35} + e^{14}$             | 369      |
| 953:162c | $0, 0, 0, 0, e^{12}, e^{13}, -e^{15} + e^{34}, -e^{16} + e^{24}, e^{14} + e^{26} + e^{35}$            | 369      |
| 953:163a | $0, 0, 0, 0, e^{12}, e^{13}, e^{25} + e^{34}, e^{24} + e^{16}, e^{35} + e^{14} + e^{26}$              | 369      |
| 953:163b | $0, 0, 0, 0, e^{12}, e^{13}, e^{25} + e^{34}, -e^{16} + e^{24}, e^{14} + e^{26} + e^{35}$             | 369      |
| 953:164  | $0, 0, 0, 0, e^{12}, e^{13}, e^{25} + e^{34}, e^{36} + e^{24}, e^{26} + e^{35} + e^{14}$              | 369      |
| 953:165  | $0, 0, 0, 0, e^{12}, e^{13}, e^{15} + e^{23}, e^{34} + e^{25}, e^{35} + e^{14} + e^{26}$              | 369      |
| 953:166a | $0, 0, 0, 0, e^{12}, e^{13}, e^{23} + e^{15}, e^{24} + e^{16}, e^{36} + e^{14} + e^{25}$              | 369      |
| 953:166b | $0, 0, 0, 0, -e^{12}, e^{13}, e^{15} + e^{23}, e^{24} + e^{16}, e^{36} + e^{25} + e^{14}$             | 369      |
| 953:167a | $0, 0, 0, 0, e^{12}, e^{13}, e^{15} + e^{23}, e^{16} + e^{24}, e^{35} + e^{14} + e^{26}$              | 369      |
| 953:167b | $0, 0, 0, 0, e^{12}, e^{13}, e^{15} + e^{23}, -e^{16} + e^{24}, e^{26} + e^{35} + e^{14}$             | 369      |
| 953:168a | $0, 0, 0, 0, e^{12}, e^{13}, e^{15} + e^{23}, e^{36} + e^{14}, e^{34} + e^{25} + e^{16}$              | 369      |
| 953:168b | $0, 0, 0, 0, e^{12}, e^{13}, e^{15} + e^{23}, -e^{14} + e^{36}, e^{16} + e^{34} + e^{25}$             | 369      |
| 953:169a | $0, 0, 0, 0, e^{12}, e^{13}, e^{23} + e^{15}, e^{16} + e^{34}, e^{36} + e^{14} + e^{25}$              | 369      |
| 953:169b | $0, 0, 0, 0, e^{12}, e^{13}, e^{15} + e^{23}, e^{34} - e^{16}, e^{36} + e^{25} + e^{14}$              | 369      |
| 953:169c | $0, 0, 0, 0, -e^{12}, e^{13}, e^{15} + e^{23}, e^{16} + e^{34}, e^{25} + e^{14} + e^{36}$             | 369      |
| 953:169d | $0, 0, 0, 0, -e^{12}, e^{13}, e^{23} + e^{15}, -e^{16} + e^{34}, e^{36} + e^{25} + e^{14}$            | 369      |
| 953:170  | $0, 0, 0, 0, e^{12}, e^{13}, e^{15} + e^{23}, e^{16} + e^{34}, e^{26} + e^{35} + e^{14}$              | 369      |
| 953:171  | $0, 0, 0, 0, e^{12}, e^{13}, e^{15} + e^{23}, e^{24} + e^{36}, e^{14} + e^{26} + e^{35}$              | 369      |
| 953:172  | $0, 0, 0, 0, e^{12}, e^{13}, e^{23} + e^{15}, e^{24} + e^{36}, e^{16} + e^{25} + e^{34}$              | 369      |
| 953:173  | $0, 0, 0, 0, e^{12}, e^{13}, e^{15}, e^{25} + e^{34} + e^{16}, e^{26} + e^{35} + e^{14}$              | 369      |
| 953:174  | $0, 0, 0, 0, e^{12}, e^{13}, e^{25}, e^{14} + e^{26} + e^{35}, e^{15} + e^{36} + e^{24}$              | 369      |
| 953:175  | $0, 0, 0, 0, e^{12}, e^{13}, e^{15} + e^{24}, e^{16} + e^{25}, e^{14} + e^{26} + e^{35}$              | 369      |
| 953:176a | $0, 0, 0, 0, e^{12}, e^{13}, e^{24} + e^{15}, e^{25} + e^{36}, e^{35} + e^{26} + e^{14}$              | 369      |
| 953:176b | $0, 0, 0, 0, e^{12}, e^{13}, e^{24} + e^{15}, e^{36} - e^{25}, e^{26} + e^{35} + e^{14}$              | 369      |
| 953:177a | $0, 0, 0, 0, e^{12}, e^{13}, e^{25} + e^{14}, e^{26} + e^{35}, e^{36} + e^{24} + e^{15}$              | 369      |
| 953:177b | $0, 0, 0, 0, e^{12}, e^{13}, -e^{14} + e^{25}, e^{26} + e^{35}, e^{15} + e^{24} + e^{36}$             | 369      |
| 953:178a | $0, 0, 0, 0, e^{12}, e^{13}, e^{24} + e^{15}, e^{35} + e^{26}, e^{25} + e^{36} + e^{14}$              | 369      |
| 953:178b | $0, 0, 0, 0, e^{12}, e^{13}, e^{24} - e^{15}, e^{26} + e^{35}, e^{36} + e^{25} + e^{14}$              | 369      |
| 953:178c | $0, 0, 0, 0, -e^{12}, e^{13}, e^{15} + e^{24}, -e^{26} + e^{35}, e^{25} + e^{36} + e^{14}$            | 369      |
| 953:178d | $0, 0, 0, 0, -e^{12}, e^{13}, -e^{15} + e^{24}, -e^{26} + e^{35}, e^{25} + e^{14} + e^{36}$           | 369      |
| 953:179  | $0, 0, 0, 0, e^{12}, e^{13}, e^{15} a_2 + e^{24}, e^{35} + e^{26}, e^{16} + e^{34} + e^{25}$          | 369      |
| 953:180a | $0, 0, 0, 0, e^{12}, e^{13}, e^{34} + e^{15}, e^{16} + e^{25}, e^{26} + e^{35} + e^{14}$              | 369      |
| 953:180b | $0, 0, 0, 0, e^{12}, e^{13}, -e^{15} + e^{34}, e^{16} + e^{25}, e^{14} + e^{26} + e^{35}$             | 369      |
| 953:181a | $0, 0, 0, 0, e^{12}, e^{13}, e^{15} + e^{34}, e^{25} + e^{36}, e^{14} + e^{35} + e^{26}$              | 369      |
| 953:181b | $0, 0, 0, 0, e^{12}, e^{13}, e^{34} + e^{15}, e^{36} - e^{25}, e^{26} + e^{35} + e^{14}$              | 369      |
| 953:181c | $0, 0, 0, 0, e^{12}, e^{13}, -e^{15} + e^{34}, e^{36} + e^{25}, e^{14} + e^{26} + e^{35}$             | 369      |
| 953:181d | $0, 0, 0, 0, e^{12}, e^{13}, -e^{15} + e^{34}, e^{36} - e^{25}, e^{14} + e^{26} + e^{35}$             | 369      |
| 953:182a | $0, 0, 0, 0, e^{12}, e^{13}, e^{34} + e^{15}, e^{35} + e^{26}, e^{25} + e^{36} + e^{14}$              | 369      |
| 953:182b | $0, 0, 0, 0, -e^{12}, e^{13}, e^{15} + e^{34}, -e^{26} + e^{35}, e^{25} + e^{14} + e^{36}$            | 369      |
| 953:183  | $0, 0, 0, 0, e^{12}, e^{13}, e^{34} + e^{25}, e^{36} + e^{15} a_2, e^{26} + e^{35} + e^{14}$          | 369      |
| 953:184  | $0, 0, 0, 0, e^{12}, e^{13}, e^{34} + e^{25}, e^{35} + e^{26}, e^{24} + e^{36} + e^{15}$              | 369      |
| 953:185  | $0, 0, 0, 0, e^{12}, e^{13}, e^{15} + e^{23}, e^{25} + e^{16}, e^{26} + e^{35} + e^{14}$              | 369      |
| 953:186a | $0, 0, 0, 0, e^{12}, e^{13}, e^{15} + e^{23}, e^{36} + e^{25}, e^{14} + e^{26} + e^{35}$              | 369      |
| 953:186b | $0, 0, 0, 0, e^{12}, e^{13}, e^{15} + e^{23}, e^{36} - e^{25}, e^{14} + e^{26} + e^{35}$              | 369      |
| 953:187a | $0, 0, 0, 0, e^{12}, e^{13}, e^{15} + e^{23}, e^{35} + e^{26}, e^{14} + e^{25} + e^{36}$              | 369      |
| 953:187b | $0, 0, 0, 0, -e^{12}, e^{13}, e^{15} + e^{23}, -e^{26} + e^{35}, e^{25} + e^{14} + e^{36}$            | 369      |
| 953:188  | $0, 0, 0, 0, e^{12}, e^{13}, e^{23} + e^{15}, e^{26} + e^{35}, e^{16} + e^{34} + e^{25}$              | 369      |
| 953:189  | $0, 0, 0, 0, e^{12}, e^{13}, e^{16} + e^{25}, e^{15} + e^{36}, e^{14} + e^{26} + e^{35}$              | 369      |
| 953:190  | $0, 0, 0, 0, e^{12}, e^{13}, e^{25} + e^{16}, e^{35} + e^{26}, e^{24} + e^{36} + e^{15}$              | 369      |
| 953:191  | $0, 0, 0, 0, e^{12}, e^{13}, e^{15} a_2 + e^{24}, e^{25} + e^{34} + e^{16}, e^{26} + e^{35} + e^{14}$ | 369      |
| 953:192  | $0, 0, 0, 0, e^{12}, e^{13}, e^{25} + e^{34}, e^{26} + e^{35} + a_2 e^{14}, e^{15} + e^{24} + e^{36}$ | 369      |
| 953:193  | $0, 0, 0, 0, e^{12}, e^{13}, e^{15} + e^{23}, e^{25} + e^{34} + e^{16}, e^{26} + e^{35} + e^{14}$     | 369      |

Table 2 – Continued to next page

Table 2 – Continued from previous page

| Name     | $\mathfrak{g}$                                                                                                     | UCS Dim. |
|----------|--------------------------------------------------------------------------------------------------------------------|----------|
| 953:194  | $0, 0, 0, 0, e^{12}, e^{13}, e^{25} + a_2 e^{16}, e^{26} + e^{35} + e^{14}, e^{36} + e^{24} + e^{15}$              | 369      |
| 953:195  | $0, 0, 0, 0, e^{12}, e^{13}, e^{35} + e^{26}, a_2 e^{16} + e^{34} + e^{25}, e^{24} + e^{36} + e^{15}$              | 369      |
| 953:196  | $0, 0, 0, 0, e^{12}, e^{13}, e^{34} + e^{25} + a_2 e^{16}, a_3 e^{14} + e^{26} + e^{35}, e^{15} + e^{36} + e^{24}$ | 369      |
| 953:197  | $0, 0, 0, 0, e^{12}, e^{34}, e^{15}, e^{25}, e^{36}$                                                               | 359      |
| 953:198  | $0, 0, 0, 0, e^{12}, e^{34}, e^{15}, e^{13} + e^{25}, e^{36}$                                                      | 359      |
| 953:199  | $0, 0, 0, 0, e^{12}, e^{34}, e^{15}, e^{25}, e^{46} + e^{13}$                                                      | 359      |
| 953:200  | $0, 0, 0, 0, e^{12}, e^{34}, e^{15}, e^{25} + e^{13}, e^{46}$                                                      | 359      |
| 953:201  | $0, 0, 0, 0, e^{12}, e^{34}, e^{15}, e^{36}, e^{46} + e^{25}$                                                      | 359      |
| 953:202  | $0, 0, 0, 0, -e^{12}, e^{14} + e^{23}, e^{15}, e^{25}, e^{16} + e^{35}$                                            | 359      |
| 953:203a | $0, 0, 0, 0, e^{12}, e^{34}, e^{23} + e^{15}, e^{13} + e^{25}, e^{36}$                                             | 359      |
| 953:203b | $0, 0, 0, 0, e^{12}, e^{34}, -e^{15} + e^{23}, e^{13} + e^{25}, e^{36}$                                            | 359      |
| 953:204  | $0, 0, 0, 0, e^{12}, e^{34}, e^{15}, e^{13} + e^{25}, e^{36} + e^{14}$                                             | 359      |
| 953:205  | $0, 0, 0, 0, e^{12}, e^{34}, e^{15}, e^{13} + e^{25}, e^{46} + e^{23}$                                             | 359      |
| 953:206  | $0, 0, 0, 0, e^{12}, e^{34}, e^{15}, e^{25} + e^{13}, e^{36} + e^{24}$                                             | 359      |
| 953:207a | $0, 0, 0, 0, e^{12}, e^{34}, e^{15} + e^{23}, e^{25} + e^{13}, e^{46}$                                             | 359      |
| 953:207b | $0, 0, 0, 0, e^{12}, e^{34}, -e^{15} + e^{23}, e^{13} + e^{25}, e^{46}$                                            | 359      |
| 953:208  | $0, 0, 0, 0, e^{12}, e^{34}, e^{23} + e^{15}, e^{25} + e^{14}, e^{36}$                                             | 359      |
| 953:209  | $0, 0, 0, 0, e^{12}, e^{34}, e^{15}, e^{36}, e^{13} + e^{46} + e^{25}$                                             | 359      |
| 953:210  | $0, 0, 0, 0, e^{12}, e^{34}, e^{13} + e^{25}, e^{36}, e^{46} + e^{15}$                                             | 359      |
| 953:211  | $0, 0, 0, 0, e^{12}, e^{34}, e^{15}, e^{23} + e^{46}, e^{25} + e^{36}$                                             | 359      |
| 953:212  | $0, 0, 0, 0, -e^{12}, e^{23} + e^{14}, e^{15}, e^{25} + e^{13}, e^{16} + e^{35}$                                   | 359      |
| 953:213  | $0, 0, 0, 0, e^{12}, e^{24} + e^{13}, e^{15}, e^{25}, e^{14} + e^{26} + e^{35}$                                    | 359      |
| 953:214  | $0, 0, 0, 0, e^{12}, e^{14} + e^{23}, e^{15}, e^{13} + e^{25}, e^{26} + e^{45}$                                    | 359      |
| 953:215  | $0, 0, 0, 0, -e^{12}, e^{14} + e^{23}, e^{15}, e^{34} + e^{25}, e^{35} + e^{16}$                                   | 359      |
| 953:216  | $0, 0, 0, 0, e^{12}, e^{13} + e^{24}, e^{15}, e^{34} + e^{25}, e^{26} + e^{35}$                                    | 359      |
| 953:217  | $0, 0, 0, 0, -e^{12}, e^{23} - e^{14}, e^{15}, e^{35} + e^{16}, e^{45} + e^{26}$                                   | 359      |
| 953:218a | $0, 0, 0, 0, e^{12}, e^{34}, e^{15} + e^{23}, e^{13} + e^{25}, e^{36} + e^{14}$                                    | 359      |
| 953:218b | $0, 0, 0, 0, e^{12}, e^{34}, -e^{15} + e^{23}, e^{13} + e^{25}, e^{14} + e^{36}$                                   | 359      |
| 953:219  | $0, 0, 0, 0, e^{12}, e^{34}, e^{23} + e^{15}, e^{25} + e^{14}, e^{46} + e^{13}$                                    | 359      |
| 953:220a | $0, 0, 0, 0, e^{12}, e^{34}, e^{25} + e^{13}, e^{36}, e^{15} + e^{46} + e^{23}$                                    | 359      |
| 953:220b | $0, 0, 0, 0, e^{12}, e^{34}, e^{25} - e^{13}, e^{36}, e^{15} + e^{23} + e^{46}$                                    | 359      |
| 953:221  | $0, 0, 0, 0, e^{12}, e^{34}, e^{15} + e^{23}, e^{13} + e^{46}, e^{25} + e^{36}$                                    | 359      |
| 953:222  | $0, 0, 0, 0, e^{12}, e^{34}, e^{15}, e^{46} + e^{23}, e^{25} + e^{36} + e^{14}$                                    | 359      |
| 953:223a | $0, 0, 0, 0, e^{12}, e^{34}, e^{23} + e^{15}, e^{36} + e^{14}, e^{46} + e^{25}$                                    | 359      |
| 953:223b | $0, 0, 0, 0, e^{12}, e^{34}, -e^{15} + e^{23}, e^{36} + e^{14}, e^{25} + e^{46}$                                   | 359      |
| 953:224  | $0, 0, 0, 0, -e^{12}, e^{14} + e^{23}, e^{15}, e^{13} + e^{25}, e^{35} + e^{16} + e^{24}$                          | 359      |
| 953:225  | $0, 0, 0, 0, -e^{12}, e^{14} + e^{23}, e^{25} + e^{13}, e^{15} + e^{24}, e^{16} + e^{35}$                          | 359      |
| 953:226  | $0, 0, 0, 0, -e^{12}, e^{23} + e^{14}, e^{25} + e^{13}, e^{34} + e^{15}, e^{35} + e^{16}$                          | 359      |
| 953:227  | $0, 0, 0, 0, e^{12}, e^{24} + e^{13}, e^{15}, e^{25} + e^{34}, e^{35} + e^{14} + e^{26}$                           | 359      |
| 953:228a | $0, 0, 0, 0, -e^{12}, e^{24} + e^{13}, e^{15}, e^{34} + e^{25}, e^{16} + e^{45} + e^{23}$                          | 359      |
| 953:228b | $0, 0, 0, 0, -e^{12}, e^{24} + e^{13}, e^{15}, -e^{25} + e^{34}, e^{45} + e^{16} + e^{23}$                         | 359      |
| 953:229  | $0, 0, 0, 0, e^{12}, e^{14} + e^{23}, e^{13} + e^{25}, e^{34} + e^{15}, e^{45} + e^{26}$                           | 359      |
| 953:230  | $0, 0, 0, 0, -e^{12}, -e^{14} + e^{23}, e^{15}, e^{35} + e^{16}, e^{26} + e^{13} + e^{45}$                         | 359      |
| 953:231  | $0, 0, 0, 0, -e^{12}, -e^{13} + e^{24}, e^{15}, e^{35} + e^{26}, e^{16} + e^{23} + e^{45}$                         | 359      |
| 953:232  | $0, 0, 0, 0, -e^{12}, e^{23} - e^{14}, e^{25} + e^{13}, e^{16} + e^{35}, e^{26} + e^{45}$                          | 359      |
| 953:233  | $0, 0, 0, 0, -e^{12}, -e^{14} + e^{23}, e^{15} + e^{34}, e^{16} + e^{35}, e^{26} + e^{45}$                         | 359      |
| 953:234a | $0, 0, 0, 0, e^{12}, e^{34}, e^{23} + e^{15}, e^{13} + e^{46}, e^{36} + e^{14} + e^{25}$                           | 359      |
| 953:234b | $0, 0, 0, 0, e^{12}, e^{34}, e^{15} + e^{23}, -e^{13} + e^{46}, e^{36} + e^{25} + e^{14}$                          | 359      |
| 953:235a | $0, 0, 0, 0, e^{12}, e^{34}, e^{15} + e^{23}, e^{36} + e^{14}, e^{46} + e^{13} + e^{25}$                           | 359      |
| 953:235b | $0, 0, 0, 0, e^{12}, e^{34}, e^{15} + e^{23}, -e^{14} + e^{36}, e^{13} + e^{46} + e^{25}$                          | 359      |
| 953:235c | $0, 0, 0, 0, e^{12}, e^{34}, -e^{15} + e^{23}, e^{36} - e^{14}, e^{25} + e^{46} + e^{13}$                          | 359      |
| 953:236  | $0, 0, 0, 0, -e^{12}, e^{14} + e^{23}, e^{13} + e^{25}, e^{15} + e^{34}, e^{16} + e^{24} + e^{35}$                 | 359      |
| 953:237  | $0, 0, 0, 0, -e^{12}, -e^{13} + e^{24}, e^{15}, e^{23} + e^{16} + e^{45}, e^{14} + e^{26} + e^{35}$                | 359      |
| 953:238  | $0, 0, 0, 0, -e^{12}, -e^{13} + e^{24}, e^{15} + e^{23}, e^{45} + e^{16}, e^{35} + e^{14} + e^{26}$                | 359      |
| 953:239a | $0, 0, 0, 0, -e^{12}, -e^{14} + e^{23}, e^{34} + e^{15}, e^{35} + e^{16}, e^{45} + e^{13} + e^{26}$                | 359      |
| 953:239b | $0, 0, 0, 0, -e^{12}, -e^{14} + e^{23}, -e^{15} + e^{34}, e^{16} + e^{35}, e^{13} + e^{26} + e^{45}$               | 359      |
| 953:240  | $0, 0, 0, 0, -e^{12}, -e^{13} + e^{24}, e^{15} + e^{34}, e^{26} + e^{35}, e^{23} + e^{16} + e^{45}$                | 359      |
| 953:241a | $0, 0, 0, 0, e^{23} + e^{14}, e^{24} + e^{13}, e^{16} + e^{25}, e^{26} + e^{15}, e^{46} + e^{35}$                  | 359      |

Table 2 – Continued to next page

Table 2 – Continued from previous page

| Name      | $\mathfrak{g}$                                                                                                       | UCS Dim. |
|-----------|----------------------------------------------------------------------------------------------------------------------|----------|
| 953:241b  | $0, 0, 0, 0, -e^{14} - e^{23}, -e^{13} + e^{24}, e^{25} - e^{16}, e^{26} + e^{15}, e^{46} + e^{35}$                  | 359      |
| 953:242a  | $0, 0, 0, 0, -e^{12}, -e^{13} + e^{24}, e^{15} + e^{34}, e^{23} + e^{16} + e^{45}, e^{14} + e^{26} + e^{35}$         | 359      |
| 953:242b  | $0, 0, 0, 0, -e^{12}, -e^{13} + e^{24}, e^{34} - e^{15}, e^{45} + e^{23} + e^{16}, e^{35} + e^{14} + e^{26}$         | 359      |
| 953:243a  | $0, 0, 0, 0, e^{23} + e^{14}, e^{24} + e^{13}, e^{25} + e^{16}, e^{26} + e^{15}, e^{46} + e^{35} + e^{12}$           | 359      |
| 953:243b  | $0, 0, 0, 0, -e^{14} - e^{23}, -e^{13} + e^{24}, e^{25} - e^{16}, e^{26} + e^{15}, e^{12} + e^{46} + e^{35}$         | 359      |
| 953:244a  | $0, 0, 0, 0, e^{23} + e^{14}, e^{24} + e^{13}, e^{26} + e^{15}, e^{46} + e^{35}, e^{36} + e^{45} + e^{12}$           | 359      |
| 953:244b  | $0, 0, 0, 0, e^{23} - e^{14}, e^{24} + e^{13}, e^{26} + e^{15}, e^{46} - e^{35}, e^{36} + e^{45} + e^{12}$           | 359      |
| 953:245a  | $0, 0, 0, 0, e^{23} + e^{14}, e^{24} + e^{13}, e^{26} + e^{15}, e^{16} + e^{34} + e^{25}, e^{46} + e^{35} + e^{12}$  | 359      |
| 953:245b  | $0, 0, 0, 0, e^{14} - e^{23}, e^{13} + e^{24}, -e^{15} + e^{26}, e^{16} + e^{34} + e^{25}, e^{12} + e^{46} + e^{35}$ | 359      |
| Type: 432 |                                                                                                                      |          |
| 952:1     | $0, 0, 0, 0, e^{12}, e^{13}, e^{23}, e^{15}, e^{25}$                                                                 | 579      |
| 952:2     | $0, 0, 0, 0, e^{12}, e^{13}, e^{34}, e^{15}, e^{25}$                                                                 | 479      |
| 952:3     | $0, 0, 0, 0, e^{12}, e^{13}, e^{14}, e^{15}, e^{25}$                                                                 | 479      |
| 952:4     | $0, 0, 0, 0, e^{12}, e^{13}, e^{24}, e^{15}, e^{25}$                                                                 | 479      |
| 952:5     | $0, 0, 0, 0, e^{12}, e^{13}, e^{34}, e^{24} + e^{13}, e^{15}, e^{25}$                                                | 479      |
| 952:6     | $0, 0, 0, 0, e^{12}, e^{13}, e^{23}, e^{15}, e^{25} + e^{34}$                                                        | 479      |
| 952:7     | $0, 0, 0, 0, e^{12}, e^{13}, e^{14} + e^{23}, e^{15}, e^{25}$                                                        | 479      |
| 952:8     | $0, 0, 0, 0, e^{12}, e^{13}, e^{34}, e^{25}, e^{15} + e^{23}$                                                        | 479      |
| 952:9     | $0, 0, 0, 0, e^{12}, e^{13}, e^{14}, e^{15}, e^{34} + e^{25}$                                                        | 479      |
| 952:10    | $0, 0, 0, 0, e^{12}, e^{13}, e^{14}, e^{25}, e^{15} + e^{34}$                                                        | 479      |
| 952:11    | $0, 0, 0, 0, e^{12}, e^{13}, e^{24}, e^{15}, e^{25} + e^{34}$                                                        | 479      |
| 952:12    | $0, 0, 0, 0, e^{12}, e^{13}, e^{34}, e^{15}, e^{25} + e^{14}$                                                        | 479      |
| 952:13    | $0, 0, 0, 0, e^{12}, e^{13}, e^{34}, e^{25}, e^{24} + e^{15}$                                                        | 479      |
| 952:14    | $0, 0, 0, 0, e^{12}, e^{13}, e^{23}, e^{15}, e^{14} + e^{25}$                                                        | 479      |
| 952:15    | $0, 0, 0, 0, e^{12}, e^{13}, e^{14}, e^{25}, e^{15} + e^{23}$                                                        | 479      |
| 952:16    | $0, 0, 0, 0, e^{12}, e^{13}, e^{24}, e^{25}, e^{15} + e^{23}$                                                        | 479      |
| 952:17    | $0, 0, 0, 0, e^{12}, e^{13}, e^{23} + e^{14}, e^{15}, e^{34} + e^{25}$                                               | 479      |
| 952:18    | $0, 0, 0, 0, e^{12}, e^{13}, e^{23} + e^{14}, e^{25}, e^{15} + e^{34}$                                               | 479      |
| 952:19a   | $0, 0, 0, 0, e^{12}, e^{14} + e^{23}, e^{24} + e^{13}, e^{15}, e^{25}$                                               | 479      |
| 952:19b   | $0, 0, 0, 0, e^{12}, -e^{14} + e^{23}, e^{13} + e^{24}, e^{15}, e^{25}$                                              | 479      |
| 952:20    | $0, 0, 0, 0, e^{12}, e^{34}, e^{23} + e^{14}, e^{15}, e^{25} + e^{13}$                                               | 479      |
| 952:21    | $0, 0, 0, 0, e^{12}, e^{13}, e^{23}, e^{14} + e^{25}, e^{15} + e^{34}$                                               | 479      |
| 952:22    | $0, 0, 0, 0, e^{12}, e^{13}, e^{14}, e^{15} + e^{23}, e^{25} + e^{34}$                                               | 479      |
| 952:23    | $0, 0, 0, 0, e^{12}, e^{13}, e^{24}, e^{15} + e^{23}, e^{34} + e^{25}$                                               | 479      |
| 952:24    | $0, 0, 0, 0, e^{12}, e^{13}, e^{14} + e^{23}, e^{25}, e^{15} + e^{24}$                                               | 479      |
| 952:25    | $0, 0, 0, 0, e^{12}, e^{13}, e^{34}, e^{15} + e^{23}, e^{25} + e^{14}$                                               | 479      |
| 952:26a   | $0, 0, 0, 0, e^{12}, e^{13}, e^{34}, e^{15} + e^{24}, e^{14} + e^{25}$                                               | 479      |
| 952:26b   | $0, 0, 0, 0, e^{12}, e^{13}, e^{34}, -e^{15} + e^{24}, e^{25} + e^{14}$                                              | 479      |
| 952:27a   | $0, 0, 0, 0, e^{12}, e^{14} + e^{23}, e^{13} + e^{24}, e^{15}, e^{34} + e^{25}$                                      | 479      |
| 952:27b   | $0, 0, 0, 0, e^{12}, e^{23} - e^{14}, e^{24} + e^{13}, e^{15}, e^{25} + e^{34}$                                      | 479      |
| 952:28a   | $0, 0, 0, 0, e^{12}, e^{13}, e^{23}, e^{24} + e^{15}, e^{25} + e^{14}$                                               | 479      |
| 952:28b   | $0, 0, 0, 0, e^{12}, e^{13}, e^{23}, -e^{15} + e^{24}, e^{25} + e^{14}$                                              | 479      |
| 952:29    | $0, 0, 0, 0, e^{12}, e^{13}, e^{24}, e^{23} + e^{15}, e^{25} + e^{14}$                                               | 479      |
| 952:30    | $0, 0, 0, 0, e^{12}, e^{13}, e^{23} + e^{14}, e^{15} + e^{24}, e^{25} + e^{34}$                                      | 479      |
| 952:31    | $0, 0, 0, 0, e^{12}, e^{34}, e^{24} + e^{13}, e^{15} + e^{23}, e^{14} + e^{25}$                                      | 479      |
| 952:32    | $0, 0, 0, 0, e^{12}, e^{13}, e^{23}, e^{15}, e^{16}$                                                                 | 469      |
| 952:33    | $0, 0, 0, 0, e^{12}, e^{13}, e^{23}, e^{25}, e^{16}$                                                                 | 469      |
| 952:34    | $0, 0, 0, 0, e^{12}, e^{13}, e^{23}, e^{25}, e^{36}$                                                                 | 469      |
| 952:35    | $0, 0, 0, 0, e^{12}, e^{13}, e^{14}, e^{15}, e^{16}$                                                                 | 369      |
| 952:36    | $0, 0, 0, 0, e^{12}, e^{13}, e^{14}, e^{25}, e^{16}$                                                                 | 369      |
| 952:37    | $0, 0, 0, 0, e^{12}, e^{13}, e^{24}, e^{15}, e^{16}$                                                                 | 369      |
| 952:38    | $0, 0, 0, 0, e^{12}, e^{13}, e^{24}, e^{25}, e^{16}$                                                                 | 369      |
| 952:39    | $0, 0, 0, 0, e^{12}, e^{13}, e^{14}, e^{25}, e^{36}$                                                                 | 369      |
| 952:40    | $0, 0, 0, 0, e^{12}, e^{13}, e^{24}, e^{15}, e^{36}$                                                                 | 369      |
| 952:41    | $0, 0, 0, 0, e^{12}, e^{13}, e^{24}, e^{25}, e^{36}$                                                                 | 369      |
| 952:42    | $0, 0, 0, 0, e^{12}, e^{13}, e^{23} + e^{14}, e^{15}, e^{16}$                                                        | 369      |
| 952:43    | $0, 0, 0, 0, e^{12}, e^{13}, e^{14} + e^{23}, e^{25}, e^{16}$                                                        | 369      |
| 952:44    | $0, 0, 0, 0, e^{12}, e^{13}, e^{14} + e^{23}, e^{25}, e^{36}$                                                        | 369      |

Table 2 – Continued to next page

Table 2 – Continued from previous page

| Name    | $\mathfrak{g}$                                                         | UCS Dim. |
|---------|------------------------------------------------------------------------|----------|
| 952:45  | $0, 0, 0, 0, e^{12}, e^{13}, e^{14}, e^{15}, e^{16} + e^{24}$          | 369      |
| 952:46  | $0, 0, 0, 0, e^{12}, e^{13}, e^{14}, e^{25}, e^{16} + e^{24}$          | 369      |
| 952:47  | $0, 0, 0, 0, e^{12}, e^{13}, e^{14}, e^{15}, e^{16} + e^{34}$          | 369      |
| 952:48  | $0, 0, 0, 0, e^{12}, e^{13}, e^{14}, e^{15}, e^{36} + e^{24}$          | 369      |
| 952:49  | $0, 0, 0, 0, e^{12}, e^{13}, e^{14}, e^{25}, e^{34} + e^{16}$          | 369      |
| 952:50  | $0, 0, 0, 0, e^{12}, e^{13}, e^{14}, e^{25}, e^{24} + e^{36}$          | 369      |
| 952:51  | $0, 0, 0, 0, e^{12}, e^{13}, e^{24}, e^{15}, e^{36} + e^{14}$          | 369      |
| 952:52  | $0, 0, 0, 0, e^{12}, e^{13}, e^{24}, e^{15}, e^{34} + e^{16}$          | 369      |
| 952:53  | $0, 0, 0, 0, e^{12}, e^{13}, e^{24}, e^{25}, e^{14} + e^{36}$          | 369      |
| 952:54  | $0, 0, 0, 0, e^{12}, e^{13}, e^{24}, e^{25}, e^{16} + e^{34}$          | 369      |
| 952:55  | $0, 0, 0, 0, e^{12}, e^{13}, e^{34}, e^{15}, e^{16} + e^{24}$          | 369      |
| 952:56  | $0, 0, 0, 0, e^{12}, e^{13}, e^{34}, e^{25}, e^{16} + e^{24}$          | 369      |
| 952:57  | $0, 0, 0, 0, e^{12}, e^{13}, e^{34}, e^{15}, e^{14} + e^{36}$          | 369      |
| 952:58  | $0, 0, 0, 0, e^{12}, e^{13}, e^{34}, e^{15}, e^{24} + e^{36}$          | 369      |
| 952:59  | $0, 0, 0, 0, e^{12}, e^{13}, e^{34}, e^{25}, e^{36} + e^{14}$          | 369      |
| 952:60  | $0, 0, 0, 0, e^{12}, e^{13}, e^{34}, e^{25}, e^{24} + e^{36}$          | 369      |
| 952:61  | $0, 0, 0, 0, e^{12}, e^{13}, e^{23}, e^{15}, e^{16} + e^{24}$          | 369      |
| 952:62  | $0, 0, 0, 0, e^{12}, e^{13}, e^{23}, e^{25}, e^{16} + e^{24}$          | 369      |
| 952:63  | $0, 0, 0, 0, e^{12}, e^{13}, e^{23}, e^{15}, e^{14} + e^{36}$          | 369      |
| 952:64  | $0, 0, 0, 0, e^{12}, e^{13}, e^{23}, e^{15}, e^{16} + e^{34}$          | 369      |
| 952:65  | $0, 0, 0, 0, e^{12}, e^{13}, e^{23}, e^{15}, e^{24} + e^{36}$          | 369      |
| 952:66  | $0, 0, 0, 0, e^{12}, e^{13}, e^{23}, e^{25}, e^{36} + e^{14}$          | 369      |
| 952:67  | $0, 0, 0, 0, e^{12}, e^{13}, e^{23}, e^{25}, e^{34} + e^{16}$          | 369      |
| 952:68  | $0, 0, 0, 0, e^{12}, e^{13}, e^{23}, e^{25}, e^{36} + e^{24}$          | 369      |
| 952:69  | $0, 0, 0, 0, e^{12}, e^{13}, e^{14}, e^{15}, e^{23} + e^{16}$          | 369      |
| 952:70  | $0, 0, 0, 0, e^{12}, e^{13}, e^{14}, e^{25}, e^{16} + e^{23}$          | 369      |
| 952:71  | $0, 0, 0, 0, e^{12}, e^{13}, e^{24}, e^{15}, e^{16} + e^{23}$          | 369      |
| 952:72  | $0, 0, 0, 0, e^{12}, e^{13}, e^{24}, e^{25}, e^{23} + e^{16}$          | 369      |
| 952:73  | $0, 0, 0, 0, e^{12}, e^{13}, e^{24}, e^{23} + e^{15}, e^{16}$          | 369      |
| 952:74  | $0, 0, 0, 0, e^{12}, e^{13}, e^{24}, e^{23} + e^{15}, e^{36}$          | 369      |
| 952:75  | $0, 0, 0, 0, e^{12}, e^{13}, e^{23}, e^{15}, e^{25} + e^{16}$          | 469      |
| 952:76a | $0, 0, 0, 0, e^{12}, e^{13}, e^{23}, e^{15}, e^{25} + e^{36}$          | 469      |
| 952:76b | $0, 0, 0, 0, -e^{12}, e^{13}, e^{23}, e^{15}, e^{36} + e^{25}$         | 469      |
| 952:77  | $0, 0, 0, 0, e^{12}, e^{13}, e^{23}, e^{15}, e^{26} + e^{35}$          | 469      |
| 952:78  | $0, 0, 0, 0, e^{12}, e^{13}, e^{23}, e^{25}, e^{36} + e^{15}$          | 469      |
| 952:79  | $0, 0, 0, 0, e^{12}, e^{13}, e^{23}, e^{25}, e^{35} + e^{26}$          | 469      |
| 952:80  | $0, 0, 0, 0, e^{12}, e^{13}, e^{14}, e^{15}, e^{25} + e^{16}$          | 369      |
| 952:81  | $0, 0, 0, 0, e^{12}, e^{13}, e^{24}, e^{15}, e^{25} + e^{16}$          | 369      |
| 952:82a | $0, 0, 0, 0, e^{12}, e^{13}, e^{14}, e^{15}, e^{36} + e^{25}$          | 369      |
| 952:82b | $0, 0, 0, 0, -e^{12}, e^{13}, e^{14}, e^{15}, e^{25} + e^{36}$         | 369      |
| 952:83  | $0, 0, 0, 0, e^{12}, e^{13}, e^{14}, e^{15}, e^{26} + e^{35}$          | 369      |
| 952:84  | $0, 0, 0, 0, e^{12}, e^{13}, e^{14}, e^{25}, e^{15} + e^{36}$          | 369      |
| 952:85  | $0, 0, 0, 0, e^{12}, e^{13}, e^{14}, e^{25}, e^{35} + e^{26}$          | 369      |
| 952:86a | $0, 0, 0, 0, e^{12}, e^{13}, e^{24}, e^{15}, e^{25} + e^{36}$          | 369      |
| 952:86b | $0, 0, 0, 0, -e^{12}, e^{13}, e^{24}, e^{15}, e^{36} + e^{25}$         | 369      |
| 952:87  | $0, 0, 0, 0, e^{12}, e^{13}, e^{24}, e^{15}, e^{26} + e^{35}$          | 369      |
| 952:88  | $0, 0, 0, 0, e^{12}, e^{13}, e^{24}, e^{25}, e^{15} + e^{36}$          | 369      |
| 952:89  | $0, 0, 0, 0, e^{12}, e^{13}, e^{24}, e^{25}, e^{35} + e^{26}$          | 369      |
| 952:90  | $0, 0, 0, 0, e^{12}, e^{13}, e^{34}, e^{15}, e^{25} + e^{16}$          | 369      |
| 952:91a | $0, 0, 0, 0, e^{12}, e^{13}, e^{34}, e^{15}, e^{36} + e^{25}$          | 369      |
| 952:91b | $0, 0, 0, 0, -e^{12}, e^{13}, e^{34}, e^{15}, e^{36} + e^{25}$         | 369      |
| 952:92  | $0, 0, 0, 0, e^{12}, e^{13}, e^{34}, e^{15}, e^{26} + e^{35}$          | 369      |
| 952:93  | $0, 0, 0, 0, e^{12}, e^{13}, e^{34}, e^{25}, e^{15} + e^{36}$          | 369      |
| 952:94  | $0, 0, 0, 0, e^{12}, e^{13}, e^{34}, e^{25}, e^{35} + e^{26}$          | 369      |
| 952:95  | $0, 0, 0, 0, e^{12}, e^{13}, e^{14} + e^{23}, e^{15}, e^{24} + e^{16}$ | 369      |
| 952:96  | $0, 0, 0, 0, e^{12}, e^{13}, e^{14} + e^{23}, e^{25}, e^{16} + e^{24}$ | 369      |
| 952:97  | $0, 0, 0, 0, e^{12}, e^{13}, e^{23} + e^{14}, e^{15}, e^{16} + e^{34}$ | 369      |
| 952:98  | $0, 0, 0, 0, e^{12}, e^{13}, e^{23} + e^{14}, e^{15}, e^{36} + e^{24}$ | 369      |

Table 2 – Continued to next page

Table 2 – Continued from previous page

| Name     | $\mathfrak{g}$                                                             | UCS Dim. |
|----------|----------------------------------------------------------------------------|----------|
| 952:99   | $0, 0, 0, 0, e^{12}, e^{13}, e^{14} + e^{23}, e^{25}, e^{16} + e^{34}$     | 369      |
| 952:100  | $0, 0, 0, 0, e^{12}, e^{13}, e^{14} + e^{23}, e^{25}, e^{36} + e^{24}$     | 369      |
| 952:101  | $0, 0, 0, 0, a_1 e^{12}, e^{13}, e^{14}, e^{15} + e^{24}, e^{16} + e^{34}$ | 369      |
| 952:102a | $0, 0, 0, 0, e^{12}, e^{13}, e^{24}, e^{25} + e^{14}, e^{34} + e^{16}$     | 369      |
| 952:102b | $0, 0, 0, 0, -e^{12}, e^{13}, e^{24}, e^{25} + e^{14}, e^{34} + e^{16}$    | 369      |
| 952:103a | $0, 0, 0, 0, e^{12}, e^{13}, e^{14}, e^{15} + e^{34}, e^{16} + e^{24}$     | 369      |
| 952:103b | $0, 0, 0, 0, -e^{12}, e^{13}, e^{14}, e^{15} + e^{34}, e^{16} + e^{24}$    | 369      |
| 952:104  | $0, 0, 0, 0, e^{12}, e^{13}, e^{14}, e^{25} + e^{34}, e^{16} + e^{24}$     | 369      |
| 952:105  | $0, 0, 0, 0, e^{12}, e^{13}, e^{14}, e^{34} + e^{25}, e^{36} + e^{24}$     | 369      |
| 952:106  | $0, 0, 0, 0, e^{12}, e^{13}, e^{24}, e^{15} + e^{34}, e^{14} + e^{36}$     | 369      |
| 952:107  | $0, 0, 0, 0, e^{12}, e^{13}, e^{24}, e^{25} + e^{34}, e^{36} + e^{14}$     | 369      |
| 952:108  | $0, 0, 0, 0, e^{12}, e^{13}, e^{23}, e^{25} + e^{14}, e^{24} + e^{16}$     | 369      |
| 952:109a | $0, 0, 0, 0, e^{12}, e^{13}, e^{23}, e^{15} + e^{24}, e^{14} + e^{36}$     | 369      |
| 952:109b | $0, 0, 0, 0, -e^{12}, e^{13}, e^{23}, e^{24} + e^{15}, e^{36} + e^{14}$    | 369      |
| 952:110  | $0, 0, 0, 0, a_1 e^{12}, e^{13}, e^{23}, e^{15} + e^{24}, e^{16} + e^{34}$ | 369      |
| 952:111  | $0, 0, 0, 0, e^{12}, e^{13}, e^{23}, e^{25} + e^{14}, e^{24} + e^{36}$     | 369      |
| 952:112a | $0, 0, 0, 0, e^{12}, e^{13}, e^{23}, e^{34} + e^{15}, e^{24} + e^{16}$     | 369      |
| 952:112b | $0, 0, 0, 0, -e^{12}, e^{13}, e^{23}, e^{15} + e^{34}, e^{24} + e^{16}$    | 369      |
| 952:113  | $0, 0, 0, 0, e^{12}, e^{13}, e^{23}, e^{25} + e^{34}, e^{24} + e^{16}$     | 369      |
| 952:114  | $0, 0, 0, 0, e^{12}, e^{13}, e^{23}, e^{34} + e^{25}, e^{36} + e^{24}$     | 369      |
| 952:115  | $0, 0, 0, 0, e^{12}, e^{13}, e^{14}, e^{15} + e^{23}, e^{16} + e^{24}$     | 369      |
| 952:116  | $0, 0, 0, 0, e^{12}, e^{13}, e^{14}, e^{15} + e^{23}, e^{16} + e^{34}$     | 369      |
| 952:117  | $0, 0, 0, 0, e^{12}, e^{13}, e^{14}, e^{15} + e^{23}, e^{24} + e^{36}$     | 369      |
| 952:118  | $0, 0, 0, 0, e^{12}, e^{13}, e^{24}, e^{15} + e^{23}, e^{36} + e^{14}$     | 369      |
| 952:119  | $0, 0, 0, 0, e^{12}, e^{13}, e^{24}, e^{23} + e^{15}, e^{34} + e^{16}$     | 369      |
| 952:120  | $0, 0, 0, 0, e^{12}, e^{13}, e^{34}, e^{23} + e^{15}, e^{24} + e^{16}$     | 369      |
| 952:121  | $0, 0, 0, 0, e^{12}, e^{13}, e^{34}, e^{15} + e^{23}, e^{36} + e^{14}$     | 369      |
| 952:122  | $0, 0, 0, 0, e^{12}, e^{13}, e^{34}, e^{15} + e^{23}, e^{24} + e^{36}$     | 369      |
| 952:123  | $0, 0, 0, 0, e^{12}, e^{13}, e^{23} + e^{14}, e^{15}, e^{16} + e^{25}$     | 369      |
| 952:124a | $0, 0, 0, 0, e^{12}, e^{13}, e^{23} + e^{14}, e^{15}, e^{25} + e^{36}$     | 369      |
| 952:124b | $0, 0, 0, 0, -e^{12}, e^{13}, e^{14} + e^{23}, e^{15}, e^{36} + e^{25}$    | 369      |
| 952:125  | $0, 0, 0, 0, e^{12}, e^{13}, e^{14} + e^{23}, e^{15}, e^{35} + e^{26}$     | 369      |
| 952:126  | $0, 0, 0, 0, e^{12}, e^{13}, e^{23} + e^{14}, e^{25}, e^{36} + e^{15}$     | 369      |
| 952:127  | $0, 0, 0, 0, e^{12}, e^{13}, e^{14} + e^{23}, e^{25}, e^{26} + e^{35}$     | 369      |
| 952:128  | $0, 0, 0, 0, e^{12}, e^{13}, e^{14}, e^{15}, e^{34} + e^{16} + e^{25}$     | 369      |
| 952:129  | $0, 0, 0, 0, e^{12}, e^{13}, e^{14}, e^{25}, e^{15} + e^{36} + e^{24}$     | 369      |
| 952:130a | $0, 0, 0, 0, e^{12}, e^{13}, e^{24}, e^{15}, e^{14} + e^{36} + e^{25}$     | 369      |
| 952:130b | $0, 0, 0, 0, -e^{12}, e^{13}, e^{24}, e^{15}, e^{25} + e^{14} + e^{36}$    | 369      |
| 952:131  | $0, 0, 0, 0, e^{12}, e^{13}, e^{24}, e^{15}, e^{14} + e^{35} + e^{26}$     | 369      |
| 952:132  | $0, 0, 0, 0, e^{12}, e^{13}, e^{24}, e^{15}, e^{25} + e^{34} + e^{16}$     | 369      |
| 952:133  | $0, 0, 0, 0, e^{12}, e^{13}, e^{24}, e^{25}, e^{14} + e^{26} + e^{35}$     | 369      |
| 952:134a | $0, 0, 0, 0, e^{12}, e^{13}, e^{34}, e^{15}, e^{25} + e^{36} + e^{14}$     | 369      |
| 952:134b | $0, 0, 0, 0, -e^{12}, e^{13}, e^{34}, e^{15}, e^{14} + e^{36} + e^{25}$    | 369      |
| 952:135  | $0, 0, 0, 0, e^{12}, e^{13}, e^{34}, e^{15}, e^{14} + e^{26} + e^{35}$     | 369      |
| 952:136  | $0, 0, 0, 0, e^{12}, e^{13}, e^{34}, e^{25}, e^{24} + e^{36} + e^{15}$     | 369      |
| 952:137  | $0, 0, 0, 0, e^{12}, e^{13}, e^{34}, e^{25}, e^{26} + e^{35} + e^{14}$     | 369      |
| 952:138  | $0, 0, 0, 0, e^{12}, e^{13}, e^{14}, e^{15} + e^{24}, e^{16} + e^{25}$     | 369      |
| 952:139a | $0, 0, 0, 0, e^{12}, e^{13}, e^{14}, e^{15} + e^{24}, e^{25} + e^{36}$     | 369      |
| 952:139b | $0, 0, 0, 0, -e^{12}, e^{13}, e^{14}, e^{15} + e^{24}, e^{36} + e^{25}$    | 369      |
| 952:140  | $0, 0, 0, 0, e^{12}, e^{13}, e^{14}, e^{15} + e^{24}, e^{26} + e^{35}$     | 369      |
| 952:141  | $0, 0, 0, 0, e^{12}, e^{13}, e^{24}, e^{14} + e^{25}, e^{36} + e^{15}$     | 369      |
| 952:142  | $0, 0, 0, 0, e^{12}, e^{13}, e^{24}, e^{25} + e^{14}, e^{26} + e^{35}$     | 369      |
| 952:143  | $0, 0, 0, 0, e^{12}, e^{13}, e^{14}, e^{34} + e^{15}, e^{16} + e^{25}$     | 369      |
| 952:144  | $0, 0, 0, 0, e^{12}, e^{13}, e^{24}, e^{15} + e^{34}, e^{16} + e^{25}$     | 369      |
| 952:145a | $0, 0, 0, 0, e^{12}, e^{13}, e^{14}, e^{15} + e^{34}, e^{36} + e^{25}$     | 369      |
| 952:145b | $0, 0, 0, 0, -e^{12}, e^{13}, e^{14}, e^{34} + e^{15}, e^{36} + e^{25}$    | 369      |
| 952:146  | $0, 0, 0, 0, e^{12}, e^{13}, e^{14}, e^{34} + e^{15}, e^{35} + e^{26}$     | 369      |
| 952:147  | $0, 0, 0, 0, e^{12}, e^{13}, e^{14}, e^{25} + e^{34}, e^{36} + e^{15}$     | 369      |

Table 2 – Continued to next page

Table 2 – Continued from previous page

| Name     | $\mathfrak{g}$                                                                      | UCS Dim. |
|----------|-------------------------------------------------------------------------------------|----------|
| 952:148  | $0, 0, 0, 0, e^{12}, e^{13}, e^{14}, e^{34} + e^{25}, e^{35} + e^{26}$              | 369      |
| 952:149a | $0, 0, 0, 0, e^{12}, e^{13}, e^{24}, e^{15} + e^{34}, e^{25} + e^{36}$              | 369      |
| 952:149b | $0, 0, 0, 0, -e^{12}, e^{13}, e^{24}, e^{15} + e^{34}, e^{36} + e^{25}$             | 369      |
| 952:150  | $0, 0, 0, 0, e^{12}, e^{13}, e^{24}, e^{15} + e^{34}, e^{26} + e^{35}$              | 369      |
| 952:151  | $0, 0, 0, 0, e^{12}, e^{13}, e^{24}, e^{25} + e^{34}, e^{36} + e^{15}$              | 369      |
| 952:152  | $0, 0, 0, 0, e^{12}, e^{13}, e^{24}, e^{25} + e^{34}, e^{26} + e^{35}$              | 369      |
| 952:153  | $0, 0, 0, 0, e^{12}, e^{13}, e^{34}, e^{24} + e^{15}, e^{16} + e^{25}$              | 369      |
| 952:154  | $0, 0, 0, 0, e^{12}, e^{13}, e^{34}, e^{25} + e^{14}, e^{15} + e^{36}$              | 369      |
| 952:155a | $0, 0, 0, 0, e^{12}, e^{13}, e^{34}, e^{15} + e^{24}, e^{36} + e^{25}$              | 369      |
| 952:155b | $0, 0, 0, 0, -e^{12}, e^{13}, e^{34}, e^{15} + e^{24}, e^{25} + e^{36}$             | 369      |
| 952:156  | $0, 0, 0, 0, e^{12}, e^{13}, e^{34}, e^{25} + e^{14}, e^{35} + e^{26}$              | 369      |
| 952:157  | $0, 0, 0, 0, e^{12}, e^{13}, e^{34}, e^{24} + e^{15}, e^{26} + e^{35}$              | 369      |
| 952:158  | $0, 0, 0, 0, a_1 e^{12}, e^{13}, e^{14} + e^{23}, e^{15} + e^{24}, e^{34} + e^{16}$ | 369      |
| 952:159a | $0, 0, 0, 0, e^{12}, e^{13}, e^{14} + e^{23}, e^{15} + e^{34}, e^{16} + e^{24}$     | 369      |
| 952:159b | $0, 0, 0, 0, -e^{12}, e^{13}, e^{14} + e^{23}, e^{34} + e^{15}, e^{16} + e^{24}$    | 369      |
| 952:160  | $0, 0, 0, 0, e^{12}, e^{13}, e^{23} + e^{14}, e^{34} + e^{25}, e^{24} + e^{16}$     | 369      |
| 952:161  | $0, 0, 0, 0, e^{12}, e^{13}, e^{23} + e^{14}, e^{25} + e^{34}, e^{24} + e^{36}$     | 369      |
| 952:162a | $0, 0, 0, 0, e^{12}, e^{13}, e^{23}, e^{15}, e^{36} + e^{25} + e^{14}$              | 369      |
| 952:162b | $0, 0, 0, 0, -e^{12}, e^{13}, e^{23}, e^{15}, e^{26} + e^{35} + e^{14}$             | 369      |
| 952:163  | $0, 0, 0, 0, e^{12}, e^{13}, e^{23}, e^{15}, e^{26} + e^{35} + e^{14}$              | 369      |
| 952:164  | $0, 0, 0, 0, e^{12}, e^{13}, e^{23}, e^{15}, e^{16} + e^{25} + e^{34}$              | 369      |
| 952:165  | $0, 0, 0, 0, e^{12}, e^{13}, e^{23}, e^{25}, e^{36} + e^{15} + e^{24}$              | 369      |
| 952:166  | $0, 0, 0, 0, e^{12}, e^{13}, e^{23}, e^{25}, e^{14} + e^{35} + e^{26}$              | 369      |
| 952:167  | $0, 0, 0, 0, e^{12}, e^{13}, e^{23}, e^{24} + e^{15}, e^{25} + e^{16}$              | 369      |
| 952:168  | $0, 0, 0, 0, e^{12}, e^{13}, e^{23}, e^{25} + e^{14}, e^{36} + e^{15}$              | 369      |
| 952:169a | $0, 0, 0, 0, e^{12}, e^{13}, e^{23}, e^{15} + e^{24}, e^{36} + e^{25}$              | 369      |
| 952:169b | $0, 0, 0, 0, -e^{12}, e^{13}, e^{23}, e^{15} + e^{24}, e^{25} + e^{36}$             | 369      |
| 952:170  | $0, 0, 0, 0, e^{12}, e^{13}, e^{23}, e^{14} + e^{25}, e^{26} + e^{35}$              | 369      |
| 952:171  | $0, 0, 0, 0, e^{12}, e^{13}, e^{23}, e^{15} + e^{24}, e^{35} + e^{26}$              | 369      |
| 952:172  | $0, 0, 0, 0, e^{12}, e^{13}, e^{23}, e^{34} + e^{15}, e^{25} + e^{16}$              | 369      |
| 952:173a | $0, 0, 0, 0, e^{12}, e^{13}, e^{23}, e^{15} + e^{34}, e^{25} + e^{36}$              | 369      |
| 952:173b | $0, 0, 0, 0, -e^{12}, e^{13}, e^{23}, e^{34} + e^{15}, e^{36} + e^{25}$             | 369      |
| 952:174  | $0, 0, 0, 0, e^{12}, e^{13}, e^{23}, e^{15} + e^{34}, e^{26} + e^{35}$              | 369      |
| 952:175  | $0, 0, 0, 0, e^{12}, e^{13}, e^{23}, e^{25} + e^{34}, e^{15} + e^{36}$              | 369      |
| 952:176  | $0, 0, 0, 0, e^{12}, e^{13}, e^{23}, e^{34} + e^{25}, e^{35} + e^{26}$              | 369      |
| 952:177  | $0, 0, 0, 0, e^{12}, e^{13}, e^{14}, e^{15} + e^{23}, e^{25} + e^{16}$              | 369      |
| 952:178  | $0, 0, 0, 0, e^{12}, e^{13}, e^{24}, e^{15} + e^{23}, e^{25} + e^{16}$              | 369      |
| 952:179a | $0, 0, 0, 0, e^{12}, e^{13}, e^{14}, e^{15} + e^{23}, e^{36} + e^{25}$              | 369      |
| 952:179b | $0, 0, 0, 0, -e^{12}, e^{13}, e^{14}, e^{15} + e^{23}, e^{25} + e^{36}$             | 369      |
| 952:180  | $0, 0, 0, 0, e^{12}, e^{13}, e^{14}, e^{15} + e^{23}, e^{26} + e^{35}$              | 369      |
| 952:181a | $0, 0, 0, 0, e^{12}, e^{13}, e^{24}, e^{23} + e^{15}, e^{25} + e^{36}$              | 369      |
| 952:181b | $0, 0, 0, 0, -e^{12}, e^{13}, e^{24}, e^{23} + e^{15}, e^{36} + e^{25}$             | 369      |
| 952:182  | $0, 0, 0, 0, e^{12}, e^{13}, e^{24}, e^{15} + e^{23}, e^{26} + e^{35}$              | 369      |
| 952:183  | $0, 0, 0, 0, e^{12}, e^{13}, e^{34}, e^{23} + e^{15}, e^{16} + e^{25}$              | 369      |
| 952:184a | $0, 0, 0, 0, e^{12}, e^{13}, e^{34}, e^{15} + e^{23}, e^{25} + e^{36}$              | 369      |
| 952:184b | $0, 0, 0, 0, -e^{12}, e^{13}, e^{34}, e^{15} + e^{23}, e^{36} + e^{25}$             | 369      |
| 952:185  | $0, 0, 0, 0, e^{12}, e^{13}, e^{34}, e^{15} + e^{23}, e^{35} + e^{26}$              | 369      |
| 952:186  | $0, 0, 0, 0, e^{12}, e^{13}, e^{23}, e^{16} + e^{25}, e^{36} + e^{15}$              | 469      |
| 952:187  | $0, 0, 0, 0, e^{12}, e^{13}, e^{23}, e^{25} + e^{16}, e^{26} + e^{35}$              | 469      |
| 952:188a | $0, 0, 0, 0, e^{12}, e^{13}, e^{23}, e^{26} + e^{35}, e^{36} + e^{25}$              | 469      |
| 952:188b | $0, 0, 0, 0, -e^{12}, e^{13}, e^{23}, e^{35} - e^{26}, e^{36} + e^{25}$             | 469      |
| 952:189  | $0, 0, 0, 0, e^{12}, e^{13}, e^{14}, e^{16} + e^{25}, e^{15} + e^{36}$              | 369      |
| 952:190  | $0, 0, 0, 0, e^{12}, e^{13}, e^{14}, e^{16} + e^{25}, e^{35} + e^{26}$              | 369      |
| 952:191  | $0, 0, 0, 0, e^{12}, e^{13}, e^{24}, e^{25} + e^{16}, e^{15} + e^{36}$              | 369      |
| 952:192  | $0, 0, 0, 0, e^{12}, e^{13}, e^{24}, e^{16} + e^{25}, e^{26} + e^{35}$              | 369      |
| 952:193a | $0, 0, 0, 0, e^{12}, e^{13}, e^{14}, e^{26} + e^{35}, e^{36} + e^{25}$              | 369      |
| 952:193b | $0, 0, 0, 0, -e^{12}, e^{13}, e^{14}, e^{35} - e^{26}, e^{36} + e^{25}$             | 369      |
| 952:194  | $0, 0, 0, 0, e^{12}, e^{13}, e^{24}, e^{36} + e^{15}, e^{26} + e^{35}$              | 369      |

Table 2 – Continued to next page



Table 2 – Continued from previous page

| Name     | $\mathfrak{g}$                                                                     | UCS Dim. |
|----------|------------------------------------------------------------------------------------|----------|
| 952:195a | $0, 0, 0, 0, e^{12}, e^{13}, e^{24}, e^{26} + e^{35}, e^{36} + e^{25}$             | 369      |
| 952:195b | $0, 0, 0, 0, -e^{12}, e^{13}, e^{24}, e^{35} - e^{26}, e^{36} + e^{25}$            | 369      |
| 952:196  | $0, 0, 0, 0, e^{12}, e^{13}, e^{23} + e^{14}, e^{15}, e^{34} + e^{25} + e^{16}$    | 369      |
| 952:197  | $0, 0, 0, 0, e^{12}, e^{13}, e^{23} + e^{14}, e^{25}, e^{24} + e^{36} + e^{15}$    | 369      |
| 952:198  | $0, 0, 0, 0, e^{12}, e^{13}, e^{14} + e^{23}, e^{24} + e^{15}, e^{25} + e^{16}$    | 369      |
| 952:199a | $0, 0, 0, 0, e^{12}, e^{13}, e^{14} + e^{23}, e^{15} + e^{24}, e^{25} + e^{36}$    | 369      |
| 952:199b | $0, 0, 0, 0, -e^{12}, e^{13}, e^{23} + e^{14}, e^{24} + e^{15}, e^{36} + e^{25}$   | 369      |
| 952:200  | $0, 0, 0, 0, e^{12}, e^{13}, e^{23} + e^{14}, e^{15} + e^{24}, e^{26} + e^{35}$    | 369      |
| 952:201  | $0, 0, 0, 0, e^{12}, e^{13}, e^{14} + e^{23}, e^{34} + e^{15}, e^{25} + e^{16}$    | 369      |
| 952:202a | $0, 0, 0, 0, e^{12}, e^{13}, e^{23} + e^{14}, e^{34} + e^{15}, e^{25} + e^{36}$    | 369      |
| 952:202b | $0, 0, 0, 0, -e^{12}, e^{13}, e^{23} + e^{14}, e^{15} + e^{34}, e^{36} + e^{25}$   | 369      |
| 952:203  | $0, 0, 0, 0, e^{12}, e^{13}, e^{14} + e^{23}, e^{34} + e^{15}, e^{26} + e^{35}$    | 369      |
| 952:204  | $0, 0, 0, 0, e^{12}, e^{13}, e^{14} + e^{23}, e^{34} + e^{25}, e^{15} + e^{36}$    | 369      |
| 952:205  | $0, 0, 0, 0, e^{12}, e^{13}, e^{23} + e^{14}, e^{25} + e^{34}, e^{26} + e^{35}$    | 369      |
| 952:206  | $0, 0, 0, 0, e^{12}a_1, e^{13}, e^{14}, e^{15} + e^{24}, e^{34} + e^{25} + e^{16}$ | 369      |
| 952:207  | $0, 0, 0, 0, e^{12}, e^{13}, e^{14}, e^{25} + e^{34}, e^{24} + e^{36} + e^{15}$    | 369      |
| 952:208a | $0, 0, 0, 0, e^{12}, e^{13}, e^{24}, e^{34} + e^{15}, e^{36} + e^{25} + e^{14}$    | 369      |
| 952:208b | $0, 0, 0, 0, -e^{12}, e^{13}, e^{24}, e^{15} + e^{34}, e^{25} + e^{14} + e^{36}$   | 369      |
| 952:209a | $0, 0, 0, 0, e^{12}, e^{13}, e^{24}, e^{34} + e^{15}, e^{26} + e^{35} + e^{14}$    | 369      |
| 952:209b | $0, 0, 0, 0, e^{12}, e^{13}, e^{24}, -e^{15} + e^{34}, e^{14} + e^{26} + e^{35}$   | 369      |
| 952:210  | $0, 0, 0, 0, e^{12}, e^{13}, e^{24}, e^{34} + e^{25}, e^{14} + e^{35} + e^{26}$    | 369      |
| 952:211a | $0, 0, 0, 0, e^{12}, e^{13}, e^{34}, e^{25} + e^{14}, e^{24} + e^{36} + e^{15}$    | 369      |
| 952:211b | $0, 0, 0, 0, e^{12}, e^{13}, e^{34}, e^{25} - e^{14}, e^{36} + e^{15} + e^{24}$    | 369      |
| 952:212a | $0, 0, 0, 0, e^{12}, e^{13}, e^{34}, e^{15} + e^{24}, e^{14} + e^{36} + e^{25}$    | 369      |
| 952:212b | $0, 0, 0, 0, e^{12}, e^{13}, e^{34}, -e^{15} + e^{24}, e^{25} + e^{36} + e^{14}$   | 369      |
| 952:212c | $0, 0, 0, 0, -e^{12}, e^{13}, e^{34}, e^{15} + e^{24}, e^{14} + e^{36} + e^{25}$   | 369      |
| 952:212d | $0, 0, 0, 0, -e^{12}, e^{13}, e^{34}, -e^{15} + e^{24}, e^{25} + e^{14} + e^{36}$  | 369      |
| 952:213  | $0, 0, 0, 0, e^{12}, e^{13}, e^{34}, e^{24} + e^{15}, e^{35} + e^{26} + e^{14}$    | 369      |
| 952:214a | $0, 0, 0, 0, e^{12}, e^{13}, e^{23}, e^{25} + e^{14}, e^{24} + e^{36} + e^{15}$    | 369      |
| 952:214b | $0, 0, 0, 0, e^{12}, e^{13}, e^{23}, e^{25} - e^{14}, e^{15} + e^{24} + e^{36}$    | 369      |
| 952:215a | $0, 0, 0, 0, e^{12}, e^{13}, e^{23}, e^{24} + e^{15}, e^{36} + e^{25} + e^{14}$    | 369      |
| 952:215b | $0, 0, 0, 0, e^{12}, e^{13}, e^{23}, -e^{15} + e^{24}, e^{25} + e^{36} + e^{14}$   | 369      |
| 952:215c | $0, 0, 0, 0, -e^{12}, e^{13}, e^{23}, e^{15} + e^{24}, e^{14} + e^{36} + e^{25}$   | 369      |
| 952:215d | $0, 0, 0, 0, -e^{12}, e^{13}, e^{23}, -e^{15} + e^{24}, e^{36} + e^{25} + e^{14}$  | 369      |
| 952:216  | $0, 0, 0, 0, e^{12}, e^{13}, e^{23}, e^{24} + e^{15}, e^{35} + e^{26} + e^{14}$    | 369      |
| 952:217  | $0, 0, 0, 0, a_1e^{12}, e^{13}, e^{23}, e^{24} + e^{15}, e^{25} + e^{34} + e^{16}$ | 369      |
| 952:218a | $0, 0, 0, 0, e^{12}, e^{13}, e^{23}, e^{15} + e^{34}, e^{14} + e^{36} + e^{25}$    | 369      |
| 952:218b | $0, 0, 0, 0, -e^{12}, e^{13}, e^{23}, e^{15} + e^{34}, e^{25} + e^{36} + e^{14}$   | 369      |
| 952:219a | $0, 0, 0, 0, e^{12}, e^{13}, e^{23}, e^{15} + e^{34}, e^{14} + e^{26} + e^{35}$    | 369      |
| 952:219b | $0, 0, 0, 0, e^{12}, e^{13}, e^{23}, -e^{15} + e^{34}, e^{14} + e^{35} + e^{26}$   | 369      |
| 952:220  | $0, 0, 0, 0, e^{12}, e^{13}, e^{23}, e^{25} + e^{34}, e^{24} + e^{36} + e^{15}$    | 369      |
| 952:221  | $0, 0, 0, 0, e^{12}, e^{13}, e^{23}, e^{25} + e^{34}, e^{14} + e^{26} + e^{35}$    | 369      |
| 952:222  | $0, 0, 0, 0, e^{12}, e^{13}, e^{14}, e^{15} + e^{23}, e^{16} + e^{25} + e^{34}$    | 369      |
| 952:223a | $0, 0, 0, 0, e^{12}, e^{13}, e^{24}, e^{15} + e^{23}, e^{14} + e^{36} + e^{25}$    | 369      |
| 952:223b | $0, 0, 0, 0, -e^{12}, e^{13}, e^{24}, e^{15} + e^{23}, e^{25} + e^{14} + e^{36}$   | 369      |
| 952:224  | $0, 0, 0, 0, e^{12}, e^{13}, e^{24}, e^{23} + e^{15}, e^{35} + e^{26} + e^{14}$    | 369      |
| 952:225  | $0, 0, 0, 0, e^{12}, e^{13}, e^{24}, e^{15} + e^{23}, e^{25} + e^{34} + e^{16}$    | 369      |
| 952:226a | $0, 0, 0, 0, e^{12}, e^{13}, e^{34}, e^{15} + e^{23}, e^{36} + e^{25} + e^{14}$    | 369      |
| 952:226b | $0, 0, 0, 0, -e^{12}, e^{13}, e^{34}, e^{15} + e^{23}, e^{14} + e^{36} + e^{25}$   | 369      |
| 952:227  | $0, 0, 0, 0, e^{12}, e^{13}, e^{34}, e^{15} + e^{23}, e^{26} + e^{35} + e^{14}$    | 369      |
| 952:228  | $0, 0, 0, 0, e^{12}, e^{13}, e^{14} + e^{23}, e^{25} + e^{16}, e^{36} + e^{15}$    | 369      |
| 952:229  | $0, 0, 0, 0, e^{12}, e^{13}, e^{23} + e^{14}, e^{25} + e^{16}, e^{35} + e^{26}$    | 369      |
| 952:230a | $0, 0, 0, 0, e^{12}, e^{13}, e^{14} + e^{23}, e^{26} + e^{35}, e^{36} + e^{25}$    | 369      |
| 952:230b | $0, 0, 0, 0, -e^{12}, e^{13}, e^{23} + e^{14}, -e^{26} + e^{35}, e^{25} + e^{36}$  | 369      |
| 952:231  | $0, 0, 0, 0, e^{12}, e^{13}, e^{14}, e^{16} + e^{25}, e^{15} + e^{24} + e^{36}$    | 369      |
| 952:232  | $0, 0, 0, 0, e^{12}, e^{13}, e^{24}, e^{25} + e^{16}, e^{35} + e^{14} + e^{26}$    | 369      |
| 952:233  | $0, 0, 0, 0, e^{12}, e^{13}, e^{14}, e^{35} + e^{26}, e^{24} + e^{36} + e^{15}$    | 369      |
| 952:234  | $0, 0, 0, 0, e^{12}, e^{13}, e^{24}, e^{36} + e^{15}, e^{35} + e^{14} + e^{26}$    | 369      |

Table 2 – Continued to next page

Table 2 – Continued from previous page

| Name     | $\mathfrak{g}$                                                                                        | UCS Dim. |
|----------|-------------------------------------------------------------------------------------------------------|----------|
| 952:235  | $0, 0, 0, 0, e^{12}, e^{13}, e^{24}, e^{15} + e^{36}, e^{16} + e^{25} + e^{34}$                       | 369      |
| 952:236a | $0, 0, 0, 0, e^{12}, e^{13}, e^{24}, e^{36} + e^{25}, e^{14} + e^{26} + e^{35}$                       | 369      |
| 952:236b | $0, 0, 0, 0, e^{12}, e^{13}, e^{24}, -e^{25} + e^{36}, e^{14} + e^{35} + e^{26}$                      | 369      |
| 952:237a | $0, 0, 0, 0, e^{12}, e^{13}, e^{24}, e^{26} + e^{35}, e^{36} + e^{25} + e^{14}$                       | 369      |
| 952:237b | $0, 0, 0, 0, -e^{12}, e^{13}, e^{24}, -e^{26} + e^{35}, e^{25} + e^{36} + e^{14}$                     | 369      |
| 952:238  | $0, 0, 0, 0, e^{12}, e^{13}, e^{24}, e^{26} + e^{35}, e^{16} + e^{25} + e^{34}$                       | 369      |
| 952:239  | $0, 0, 0, 0, a_1 e^{12}, e^{13}, e^{14} + e^{23}, e^{15} + e^{24}, e^{16} + e^{34} + e^{25}$          | 369      |
| 952:240  | $0, 0, 0, 0, e^{12}, e^{13}, e^{14} + e^{23}, e^{25} + e^{34}, e^{24} + e^{36} + e^{15}$              | 369      |
| 952:241  | $0, 0, 0, 0, e^{12}, e^{13}, e^{23}, e^{25} + e^{16}, e^{36} + e^{15} + e^{24}$                       | 369      |
| 952:242  | $0, 0, 0, 0, e^{12}, e^{13}, e^{23}, e^{16} + e^{25}, e^{14} + e^{26} + e^{35}$                       | 369      |
| 952:243a | $0, 0, 0, 0, e^{12}, e^{13}, e^{23}, e^{36} + e^{25}, e^{14} + e^{26} + e^{35}$                       | 369      |
| 952:243b | $0, 0, 0, 0, e^{12}, e^{13}, e^{23}, -e^{25} + e^{36}, e^{35} + e^{26} + e^{14}$                      | 369      |
| 952:244a | $0, 0, 0, 0, e^{12}, e^{13}, e^{23}, e^{26} + e^{35}, e^{36} + e^{25} + e^{14}$                       | 369      |
| 952:244b | $0, 0, 0, 0, -e^{12}, e^{13}, e^{23}, -e^{26} + e^{35}, e^{25} + e^{36} + e^{14}$                     | 369      |
| 952:245  | $0, 0, 0, 0, e^{12}, e^{13}, e^{23}, e^{26} + e^{35}, e^{15} + e^{24} + e^{36}$                       | 369      |
| 952:246  | $0, 0, 0, 0, e^{12}, e^{13}, e^{14} + e^{23}, e^{16} + e^{25}, e^{15} + e^{24} + e^{36}$              | 369      |
| 952:247  | $0, 0, 0, 0, e^{12}, e^{13}, e^{23} + e^{14}, e^{35} + e^{26}, e^{24} + e^{36} + e^{15}$              | 369      |
| 952:248  | $0, 0, 0, 0, a_1 e^{12}, e^{13}, e^{14}, e^{34} + e^{25} + e^{16}, e^{36} + e^{15} + e^{24}$          | 369      |
| 952:249  | $0, 0, 0, 0, e^{12}, e^{13}, e^{24}, e^{16} + e^{25} + e^{34}, e^{26} + e^{35} + e^{14}$              | 369      |
| 952:250  | $0, 0, 0, 0, e^{12}, e^{13}, e^{23}, e^{35} + e^{14} + e^{26}, e^{36} + e^{15} + e^{24}$              | 369      |
| 952:251  | $0, 0, 0, 0, a_1 e^{12}, e^{13}, e^{23}, e^{16} + e^{25} + e^{34}, e^{24} + e^{36} + e^{15}$          | 369      |
| 952:252  | $0, 0, 0, 0, a_1 e^{12}, e^{13}, e^{14} + e^{23}, e^{25} + e^{16} + e^{34}, e^{15} + e^{24} + e^{36}$ | 369      |
| 952:253a | $0, 0, 0, 0, e^{12}, e^{13}, e^{23}, e^{15}, e^{27} + e^{16}$                                         | 369      |
| 952:253b | $0, 0, 0, 0, e^{12}, -e^{13}, e^{23}, e^{15}, e^{16} + e^{27}$                                        | 369      |
| 952:254  | $0, 0, 0, 0, e^{12}, e^{13}, e^{23}, e^{15}, e^{17} + e^{26}$                                         | 369      |
| 952:255  | $0, 0, 0, 0, e^{12}, e^{13}, e^{23}, e^{15}, e^{37} + e^{16}$                                         | 369      |
| 952:256  | $0, 0, 0, 0, e^{12}, e^{13}, e^{23}, e^{15}, e^{36} + e^{27}$                                         | 369      |
| 952:257  | $0, 0, 0, 0, e^{12}, e^{13}, e^{23}, e^{15}, e^{37} + e^{16} + e^{24}$                                | 269      |
| 952:258  | $0, 0, 0, 0, e^{12}, e^{13}, e^{23}, e^{15}, e^{14} + e^{27} + e^{36}$                                | 269      |
| 952:259a | $0, 0, 0, 0, e^{12}, e^{13}, e^{23}, e^{15}, e^{27} + e^{16} + e^{34}$                                | 269      |
| 952:259b | $0, 0, 0, 0, e^{12}, -e^{13}, e^{23}, e^{15}, e^{16} + e^{34} + e^{27}$                               | 269      |
| 952:260  | $0, 0, 0, 0, e^{12}, e^{13}, e^{23}, e^{15}, e^{34} + e^{17} + e^{26}$                                | 269      |
| 952:261a | $0, 0, 0, 0, e^{12}, e^{13}, e^{23}, e^{14} + e^{25}, e^{27} + e^{16}$                                | 269      |
| 952:261b | $0, 0, 0, 0, e^{12}, -e^{13}, e^{23}, e^{25} + e^{14}, e^{27} + e^{16}$                               | 269      |
| 952:262  | $0, 0, 0, 0, e^{12}, e^{13}, e^{23}, e^{25} + e^{14}, e^{26} + e^{17}$                                | 269      |
| 952:263  | $0, 0, 0, 0, e^{12}, e^{13}, e^{23}, e^{25} + e^{14}, e^{16} + e^{37}$                                | 269      |
| 952:264  | $0, 0, 0, 0, e^{12}, e^{13}, e^{23}, e^{15} + e^{24}, e^{16} + e^{37}$                                | 269      |
| 952:265a | $0, 0, 0, 0, e^{12}, e^{13}, e^{23}, e^{34} + e^{15}, e^{27} + e^{16}$                                | 269      |
| 952:265b | $0, 0, 0, 0, e^{12}, -e^{13}, e^{23}, e^{15} + e^{34}, e^{16} + e^{27}$                               | 269      |
| 952:266  | $0, 0, 0, 0, e^{12}, e^{13}, e^{23}, e^{15} + e^{34}, e^{17} + e^{26}$                                | 269      |
| 952:267  | $0, 0, 0, 0, e^{12}, e^{13}, e^{23}, e^{34} + e^{15}, e^{37} + e^{16}$                                | 269      |
| 952:268  | $0, 0, 0, 0, e^{12}, e^{13}, e^{23}, e^{15} + e^{34}, e^{27} + e^{36}$                                | 269      |
| 952:269  | $0, 0, 0, 0, e^{12}, e^{13}, e^{23}, e^{15}, e^{16} + e^{25} + e^{37}$                                | 369      |
| 952:270  | $0, 0, 0, 0, (-1 + a_2) e^{12}, e^{13} a_2, e^{23}, e^{15}, e^{17} + e^{26} + e^{35}$                 | 369      |
| 952:271  | $0, 0, 0, 0, e^{12}, e^{13}, e^{23}, e^{25} + e^{16}, e^{27} + e^{15}$                                | 369      |
| 952:272a | $0, 0, 0, 0, e^{12}, e^{13}, e^{23}, e^{25} + e^{16}, e^{37} + e^{15}$                                | 369      |
| 952:272b | $0, 0, 0, 0, -e^{12}, e^{13}, e^{23}, e^{16} + e^{25}, e^{37} + e^{15}$                               | 369      |
| 952:273  | $0, 0, 0, 0, -e^{12}, e^{13}, e^{23}, e^{16} + e^{25}, e^{17} + e^{35}$                               | 369      |
| 952:274  | $0, 0, 0, 0, -e^{12}, e^{13}, e^{23}, e^{15} + e^{36}, e^{17} + e^{35}$                               | 369      |
| 952:275  | $0, 0, 0, 0, e^{12}, a_1 e^{13}, e^{23}, e^{36} + e^{15}, e^{37} + e^{25}$                            | 369      |
| 952:276a | $0, 0, 0, 0, e^{12}, e^{13}, e^{23}, e^{36} + e^{25}, e^{37} + e^{15}$                                | 369      |
| 952:276b | $0, 0, 0, 0, e^{12}, -e^{13}, e^{23}, e^{36} + e^{25}, e^{15} + e^{37}$                               | 369      |
| 952:276c | $0, 0, 0, 0, -e^{12}, -e^{13}, e^{23}, e^{25} + e^{36}, e^{15} + e^{37}$                              | 369      |
| 952:277a | $0, 0, 0, 0, e^{12}, e^{13}, e^{23}, e^{26} + e^{35}, e^{15} + e^{37}$                                | 369      |
| 952:277b | $0, 0, 0, 0, -e^{12}, -e^{13}, e^{23}, e^{35} + e^{26}, e^{37} + e^{15}$                              | 369      |
| 952:278a | $0, 0, 0, 0, e^{12}, e^{13}, e^{23}, e^{25} + e^{14}, e^{24} + e^{37} + e^{16}$                       | 269      |
| 952:278b | $0, 0, 0, 0, -e^{12}, e^{13}, e^{23}, e^{25} + e^{14}, e^{37} + e^{16} + e^{24}$                      | 269      |
| 952:279a | $0, 0, 0, 0, a_1 e^{12}, e^{13}, e^{23}, e^{25} + e^{14}, e^{16} + e^{27} + e^{34}$                   | 269      |

Table 2 – Continued to next page

Table 2 – Continued from previous page

| Name     | $\mathfrak{g}$                                                                                           | UCS Dim. |
|----------|----------------------------------------------------------------------------------------------------------|----------|
| 952:279b | $0, 0, 0, 0, a_1 e^{12}, -e^{13}, e^{23}, e^{14} + e^{25}, e^{16} + e^{34} + e^{27}$                     | 269      |
| 952:280  | $0, 0, 0, 0, e^{12}, e^{13}, e^{23}, e^{25} + e^{14}, e^{34} + e^{26} + e^{17}$                          | 269      |
| 952:281a | $0, 0, 0, 0, e^{12}, e^{13}, e^{23}, e^{34} + e^{15}, e^{24} + e^{37} + e^{16}$                          | 269      |
| 952:281b | $0, 0, 0, 0, -e^{12}, e^{13}, e^{23}, e^{34} + e^{15}, e^{37} + e^{16} + e^{24}$                         | 269      |
| 952:282  | $0, 0, 0, 0, e^{12}, e^{13}, e^{23}, e^{15} + e^{34}, e^{14} + e^{27} + e^{36}$                          | 269      |
| 952:283  | $0, 0, 0, 0, e^{12}, e^{13}, e^{23}, e^{25} + e^{14}, e^{15} + e^{27} + e^{36}$                          | 269      |
| 952:284  | $0, 0, 0, 0, (-1 + a_2) e^{12}, a_2 e^{13}, e^{23}, e^{14} + e^{25}, e^{17} + e^{26} + e^{35}$           | 269      |
| 952:285  | $0, 0, 0, 0, e^{12}, e^{13}, e^{23}, e^{34} + e^{15}, e^{25} + e^{37} + e^{16}$                          | 269      |
| 952:286  | $0, 0, 0, 0, e^{12}(-1 + a_2), a_2 e^{13}, e^{23}, e^{15} + e^{34}, e^{26} + e^{17} + e^{35}$            | 269      |
| 952:287a | $0, 0, 0, 0, e^{12}, e^{13}, e^{23}, e^{25} + e^{16}, e^{15} + e^{24} + e^{37}$                          | 269      |
| 952:287b | $0, 0, 0, 0, -e^{12}, e^{13}, e^{23}, e^{25} + e^{16}, e^{24} + e^{37} + e^{15}$                         | 269      |
| 952:288  | $0, 0, 0, 0, e^{12}, e^{13}, e^{23}, e^{16} + e^{25}, e^{15} + e^{27} + e^{34}$                          | 269      |
| 952:289  | $0, 0, 0, 0, -e^{12}, e^{13}, e^{23}, e^{25} + e^{16}, e^{17} + e^{35} + e^{24}$                         | 269      |
| 952:290  | $0, 0, 0, 0, e^{12}, a_1 e^{13}, e^{23}, e^{15} + e^{36}, e^{14} + e^{37} + e^{25}$                      | 269      |
| 952:291  | $0, 0, 0, 0, -e^{12}, e^{13}, e^{23}, e^{36} + e^{15}, e^{35} + e^{17} + e^{24}$                         | 269      |
| 952:292a | $0, 0, 0, 0, e^{12}, e^{13}, e^{23}, e^{25} + e^{36}, e^{24} + e^{37} + e^{15}$                          | 269      |
| 952:292b | $0, 0, 0, 0, e^{12}, -e^{13}, e^{23}, e^{36} + e^{25}, e^{24} + e^{37} + e^{15}$                         | 269      |
| 952:292c | $0, 0, 0, 0, -e^{12}, e^{13}, e^{23}, e^{36} + e^{25}, e^{24} + e^{37} + e^{15}$                         | 269      |
| 952:292d | $0, 0, 0, 0, -e^{12}, -e^{13}, e^{23}, e^{25} + e^{36}, e^{37} + e^{15} + e^{24}$                        | 269      |
| 952:293a | $0, 0, 0, 0, e^{12}, e^{13}, e^{23}, e^{36} + e^{25}, e^{27} + e^{34} + e^{15}$                          | 269      |
| 952:293b | $0, 0, 0, 0, -e^{12}, e^{13}, e^{23}, e^{25} + e^{36}, e^{15} + e^{27} + e^{34}$                         | 269      |
| 952:294a | $0, 0, 0, 0, -e^{12}, e^{13}, e^{23}, e^{36} + e^{25}, e^{35} + e^{17} + e^{24}$                         | 269      |
| 952:294b | $0, 0, 0, 0, -e^{12}, -e^{13}, e^{23}, e^{36} + e^{25}, e^{35} + e^{24} + e^{17}$                        | 269      |
| 952:295  | $0, 0, 0, 0, e^{12}, e^{13}, e^{23}, e^{26} + e^{35}, e^{25} + e^{37} + e^{14}$                          | 269      |
| 952:296a | $0, 0, 0, 0, e^{12}, e^{13}, e^{23}, e^{26} + e^{35}, e^{15} + e^{37} + e^{24}$                          | 269      |
| 952:296b | $0, 0, 0, 0, -e^{12}, -e^{13}, e^{23}, e^{35} + e^{26}, e^{37} + e^{15} + e^{24}$                        | 269      |
| 952:297  | $0, 0, 0, 0, e^{12}, e^{13}, e^{23}, e^{35} + e^{26}, e^{15} + e^{34} + e^{27}$                          | 269      |
| 952:298  | $0, 0, 0, 0, a_1 e^{12}, e^{13}, e^{23}, e^{25} + e^{16}, e^{36} + e^{27} + e^{15}$                      | 369      |
| 952:299  | $0, 0, 0, 0, (-1 + a_2) e^{12}, a_2 e^{13}, e^{23}, e^{16} + e^{25}, e^{17} + e^{26} + e^{35}$           | 369      |
| 952:300a | $0, 0, 0, 0, e^{12}(-1 + a_2), a_2 e^{13}, e^{23}, e^{25} + e^{36}, e^{17} + e^{35} + e^{26}$            | 369      |
| 952:300b | $0, 0, 0, 0, e^{12}(-1 + a_2), a_2 e^{13}, e^{23}, e^{36} - e^{25}, e^{17} + e^{35} + e^{26}$            | 369      |
| 952:301  | $0, 0, 0, 0, e^{12}, e^{13}, e^{23}, e^{26} + e^{35}, e^{16} + e^{25} + e^{37}$                          | 369      |
| 952:302a | $0, 0, 0, 0, e^{12}, e^{13}, e^{23}, a_1 e^{15} + e^{24} + e^{36}, e^{25} + e^{37} + e^{14}$             | 269      |
| 952:302b | $0, 0, 0, 0, e^{12}, -e^{13}, e^{23}, a_1 e^{15} + e^{24} + e^{36}, e^{25} + e^{37} + e^{14}$            | 269      |
| 952:303a | $0, 0, 0, 0, e^{12}, e^{13}, e^{23}, e^{14} a_1 + e^{36} + e^{25}, e^{37} + e^{24} + e^{15}$             | 269      |
| 952:303b | $0, 0, 0, 0, e^{12}, -e^{13}, e^{23}, e^{14} a_1 + e^{36} + e^{25}, e^{15} + e^{24} + e^{37}$            | 269      |
| 952:303c | $0, 0, 0, 0, -e^{12}, -e^{13}, e^{23}, e^{14} a_1 + e^{25} + e^{36}, e^{15} + e^{24} + e^{37}$           | 269      |
| 952:304a | $0, 0, 0, 0, e^{12}, e^{13}, e^{23}, e^{26} + e^{35} + e^{14}, e^{24} + e^{37} + e^{15}$                 | 269      |
| 952:304b | $0, 0, 0, 0, -e^{12}, -e^{13}, e^{23}, e^{26} + e^{35} + e^{14}, e^{15} + e^{37} + e^{24}$               | 269      |
| 952:305a | $0, 0, 0, 0, e^{12}, a_1 e^{13}, e^{23}, e^{16} + e^{25} + e^{34}, e^{15} + e^{24} + e^{37}$             | 269      |
| 952:305b | $0, 0, 0, 0, -e^{12}, a_1 e^{13}, e^{23}, e^{16} + e^{34} + e^{25}, e^{15} + e^{24} + e^{37}$            | 269      |
| 952:306a | $0, 0, 0, 0, e^{12}, e^{13}, e^{23}, e^{26} + e^{35} + e^{14}, e^{34} + e^{27} + e^{15}$                 | 269      |
| 952:306b | $0, 0, 0, 0, e^{12}, e^{13}, e^{23}, e^{26} + e^{35} - e^{14}, e^{27} + e^{34} + e^{15}$                 | 269      |
| 952:307  | $0, 0, 0, 0, e^{12}, e^{13}, a_1 e^{23}, e^{15} + e^{24} + e^{36}, e^{16} + e^{25} + e^{37}$             | 269      |
| 952:308  | $0, 0, 0, 0, e^{12}, e^{13}, e^{23}, e^{35} + e^{26} + e^{14}, e^{25} + e^{37} + e^{16}$                 | 269      |
| 952:309a | $0, 0, 0, 0, (-1 + a_2) e^{12}, a_2 e^{13}, e^{23}, e^{36} + e^{25} + e^{14}, e^{26} + e^{35} + e^{17}$  | 269      |
| 952:309b | $0, 0, 0, 0, (-1 + a_2) e^{12}, a_2 e^{13}, e^{23}, -e^{25} + e^{36} + e^{14}, e^{17} + e^{26} + e^{35}$ | 269      |
| 952:310  | $0, 0, 0, 0, (-1 + a_2) e^{12}, e^{13} a_2, e^{23}, e^{24} + e^{36} + e^{15}, e^{35} + e^{26} + e^{17}$  | 269      |
| 952:311  | $0, 0, 0, 0, a_1 e^{12}, e^{13} a_2, e^{23}, e^{27} + e^{36} + e^{15}, e^{16} + e^{37} + e^{25}$         | 369      |
| 952:312  | $0, 0, 0, 0, e^{12} a_1, e^{13}(1 + a_1), e^{23}, e^{17} + e^{26} + e^{35}, e^{16} + e^{25} + e^{37}$    | 369      |
| 952:313  | $0, 0, 0, 0, e^{12}, e^{34}, e^{13}, e^{15}, e^{36}$                                                     | 359      |
| 952:314  | $0, 0, 0, 0, e^{12}, e^{34}, e^{13}, e^{25}, e^{36}$                                                     | 359      |
| 952:315  | $0, 0, 0, 0, e^{12}, e^{34}, e^{13}, e^{25}, e^{46}$                                                     | 359      |
| 952:316  | $0, 0, 0, 0, e^{12}, e^{34}, e^{13} + e^{24}, e^{15}, e^{36}$                                            | 359      |
| 952:317  | $0, 0, 0, 0, e^{12}, e^{34}, e^{14} + e^{23}, e^{15}, e^{36}$                                            | 359      |
| 952:318  | $0, 0, 0, 0, e^{12}, e^{34}, e^{13}, e^{15} + e^{23}, e^{36}$                                            | 359      |
| 952:319  | $0, 0, 0, 0, e^{12}, e^{34}, e^{13}, e^{15}, e^{46} + e^{23}$                                            | 359      |
| 952:320  | $0, 0, 0, 0, e^{12}, e^{34}, e^{13}, e^{15}, e^{24} + e^{36}$                                            | 359      |

Table 2 – Continued to next page

Table 2 – Continued from previous page

| Name     | $\mathfrak{g}$                                                                      | UCS Dim. |
|----------|-------------------------------------------------------------------------------------|----------|
| 952:321  | $0, 0, 0, 0, e^{12}, e^{34}, e^{13}, e^{25}, e^{14} + e^{36}$                       | 359      |
| 952:322  | $0, 0, 0, 0, e^{12}, e^{34}, e^{13}, e^{25}, e^{23} + e^{46}$                       | 359      |
| 952:323  | $0, 0, 0, 0, e^{12}, e^{34}, e^{13}, e^{25}, e^{24} + e^{36}$                       | 359      |
| 952:324  | $0, 0, 0, 0, e^{12}, e^{34}, e^{13}, e^{15}, e^{25} + e^{36}$                       | 359      |
| 952:325  | $0, 0, 0, 0, e^{12}, e^{34}, e^{13}, e^{25}, e^{36} + e^{15}$                       | 359      |
| 952:326  | $0, 0, 0, 0, e^{12}, e^{34}, e^{13}, e^{15}, e^{25} + e^{46}$                       | 359      |
| 952:327  | $0, 0, 0, 0, e^{12}, e^{34}, e^{13}, e^{25}, e^{15} + e^{46}$                       | 359      |
| 952:328  | $0, 0, 0, 0, e^{12}, e^{34}, e^{14} + e^{23}, e^{13} + e^{25}, e^{36}$              | 359      |
| 952:329  | $0, 0, 0, 0, e^{12}, e^{34}, e^{13} + e^{24}, e^{15}, e^{46} + e^{23}$              | 359      |
| 952:330  | $0, 0, 0, 0, e^{12}, e^{34}, e^{24} + e^{13}, e^{15}, e^{36} + e^{25}$              | 359      |
| 952:331  | $0, 0, 0, 0, e^{12}, e^{34}, e^{14} + e^{23}, e^{15}, e^{36} + e^{25}$              | 359      |
| 952:332  | $0, 0, 0, 0, -e^{12}, e^{14} + e^{23}, e^{13}, e^{15}, e^{35} + e^{16}$             | 359      |
| 952:333  | $0, 0, 0, 0, -e^{12}, e^{14} + e^{23}, e^{13}, e^{25}, e^{16} + e^{35}$             | 359      |
| 952:334  | $0, 0, 0, 0, e^{12}, e^{14} + e^{23}, e^{13}, e^{15}, e^{26} + e^{45}$              | 359      |
| 952:335  | $0, 0, 0, 0, e^{12}, e^{23} + e^{14}, e^{13}, e^{25}, e^{45} + e^{26}$              | 359      |
| 952:336  | $0, 0, 0, 0, -e^{12}, e^{23} + e^{14}, e^{34}, e^{15}, e^{16} + e^{35}$             | 359      |
| 952:337  | $0, 0, 0, 0, e^{12}, e^{24} + e^{13}, e^{34}, e^{15}, e^{26} + e^{35}$              | 359      |
| 952:338  | $0, 0, 0, 0, e^{12}, e^{34}, e^{13}, e^{15} + e^{23}, e^{36} + e^{14}$              | 359      |
| 952:339  | $0, 0, 0, 0, e^{12}, e^{34}, e^{13}, e^{23} + e^{15}, e^{24} + e^{36}$              | 359      |
| 952:340  | $0, 0, 0, 0, e^{12}, e^{34}, e^{13}, e^{14} + e^{25}, e^{23} + e^{46}$              | 359      |
| 952:341  | $0, 0, 0, 0, e^{12}, e^{34}, e^{13}, e^{24} + e^{15}, e^{23} + e^{46}$              | 359      |
| 952:342  | $0, 0, 0, 0, e^{12}, e^{34}, e^{13}, e^{15} + e^{23}, e^{36} + e^{25}$              | 359      |
| 952:343  | $0, 0, 0, 0, e^{12}, e^{34}, e^{13}, e^{15}, e^{14} + e^{36} + e^{25}$              | 359      |
| 952:344  | $0, 0, 0, 0, e^{12}, e^{34}, e^{13}, e^{25}, e^{15} + e^{46} + e^{23}$              | 359      |
| 952:345  | $0, 0, 0, 0, e^{12}, e^{34}, e^{13}, e^{25}, e^{15} + e^{24} + e^{36}$              | 359      |
| 952:346  | $0, 0, 0, 0, e^{12}, e^{34}, e^{13}, e^{15} + e^{23}, e^{25} + e^{46}$              | 359      |
| 952:347  | $0, 0, 0, 0, e^{12}, e^{34}, e^{13}, e^{14} + e^{25}, e^{15} + e^{36}$              | 359      |
| 952:348  | $0, 0, 0, 0, e^{12}, e^{34}, e^{13}, e^{24} + e^{15}, e^{36} + e^{25}$              | 359      |
| 952:349  | $0, 0, 0, 0, e^{12}, e^{34}, e^{13}, e^{25} + e^{14}, e^{46} + e^{15}$              | 359      |
| 952:350  | $0, 0, 0, 0, e^{12}, e^{34}, e^{13}, e^{15} + e^{24}, e^{25} + e^{46}$              | 359      |
| 952:351  | $0, 0, 0, 0, e^{12}, e^{34}, e^{13}, e^{36} + e^{15}, e^{46} + e^{25}$              | 359      |
| 952:352  | $0, 0, 0, 0, e^{12}, e^{34}, e^{13}, e^{25} + e^{36}, e^{15} + e^{46}$              | 359      |
| 952:353a | $0, 0, 0, 0, -e^{12}, e^{14} + e^{23}, e^{13} + e^{24}, e^{15}, e^{16} + e^{35}$    | 359      |
| 952:353b | $0, 0, 0, 0, -e^{12}, e^{23} - e^{14}, e^{24} + e^{13}, e^{15}, e^{35} + e^{16}$    | 359      |
| 952:354a | $0, 0, 0, 0, e^{12}, e^{24} + e^{13}, e^{14} + e^{23}, e^{15}, e^{26} + e^{35}$     | 359      |
| 952:354b | $0, 0, 0, 0, -e^{12}, e^{24} - e^{13}, e^{23} + e^{14}, e^{15}, e^{26} + e^{35}$    | 359      |
| 952:355  | $0, 0, 0, 0, e^{12}, e^{34}, e^{24} + e^{13}, e^{15} + e^{23}, e^{14} + e^{36}$     | 359      |
| 952:356  | $0, 0, 0, 0, e^{12}, e^{34}, e^{14} + e^{23}, e^{13} + e^{25}, e^{36} + e^{15}$     | 359      |
| 952:357  | $0, 0, 0, 0, e^{12}, e^{34}, e^{24} + e^{13}, e^{15}, e^{25} + e^{36} + e^{14}$     | 359      |
| 952:358  | $0, 0, 0, 0, e^{12}, e^{34}, e^{23} + e^{14}, e^{13} + e^{25}, e^{46} + e^{15}$     | 359      |
| 952:359  | $0, 0, 0, 0, -e^{12}, e^{14} + e^{23}, e^{13}, e^{15}, e^{16} + e^{24} + e^{35}$    | 359      |
| 952:360  | $0, 0, 0, 0, -e^{12}, e^{23} + e^{14}, e^{13}, e^{25}, e^{16} + e^{35} + e^{24}$    | 359      |
| 952:361  | $0, 0, 0, 0, -e^{12}, e^{14} + e^{23}, e^{13}, e^{15} + e^{24}, e^{35} + e^{16}$    | 359      |
| 952:362  | $0, 0, 0, 0, -e^{12}, e^{23} + e^{14}, e^{13}, e^{15} + e^{34}, e^{35} + e^{16}$    | 359      |
| 952:363  | $0, 0, 0, 0, -e^{12}, e^{14} + e^{23}, e^{13}, e^{34} + e^{25}, e^{35} + e^{16}$    | 359      |
| 952:364  | $0, 0, 0, 0, e^{12}, e^{14} + e^{23}, e^{13}, e^{15} + e^{24}, e^{26} + e^{45}$     | 359      |
| 952:365  | $0, 0, 0, 0, e^{12}, e^{14} + e^{23}, e^{13}, e^{15} + e^{34}, e^{45} + e^{26}$     | 359      |
| 952:366  | $0, 0, 0, 0, e^{12}, e^{14} + e^{23}, e^{13}, e^{34} + e^{25}, e^{26} + e^{45}$     | 359      |
| 952:367  | $0, 0, 0, 0, -e^{12}, e^{14} + e^{23}, e^{34}, e^{13} + e^{25}, e^{16} + e^{35}$    | 359      |
| 952:368  | $0, 0, 0, 0, e^{12}, e^{24} + e^{13}, e^{34}, e^{15}, e^{26} + e^{35} + e^{14}$     | 359      |
| 952:369  | $0, 0, 0, 0, -e^{12}, e^{13} + e^{24}, e^{34}, e^{15}, e^{23} + e^{16} + e^{45}$    | 359      |
| 952:370  | $0, 0, 0, 0, -e^{12}, e^{24} + e^{13}, e^{34}, e^{23} + e^{15}, e^{45} + e^{16}$    | 359      |
| 952:371a | $0, 0, 0, 0, e^{12}, e^{34}, e^{24} + e^{13}, e^{36} + e^{15}, e^{25} + e^{46}$     | 359      |
| 952:371b | $0, 0, 0, 0, e^{12}, e^{34}, -e^{13} + e^{24}, e^{36} + e^{15}, e^{46} + e^{25}$    | 359      |
| 952:372  | $0, 0, 0, 0, e^{12}, e^{34}, e^{23} + a_1 e^{14}, e^{15} + e^{36}, e^{46} + e^{25}$ | 359      |
| 952:373  | $0, 0, 0, 0, -e^{12}, e^{23} - e^{14}, e^{13}, e^{35} + e^{16}, e^{45} + e^{26}$    | 359      |
| 952:374  | $0, 0, 0, 0, -e^{12}, e^{23} - e^{14}, e^{34}, e^{16} + e^{35}, e^{26} + e^{45}$    | 359      |
| 952:375  | $0, 0, 0, 0, e^{12}, e^{34}, e^{13}, e^{15} + e^{23}, e^{25} + e^{36} + e^{14}$     | 359      |

Table 2 – Continued to next page

Table 2 – Continued from previous page

| Name     | $\mathfrak{g}$                                                                                         | UCS Dim. |
|----------|--------------------------------------------------------------------------------------------------------|----------|
| 952:376  | $0, 0, 0, 0, e^{12}, e^{34}, e^{13}, e^{14} + e^{25}, e^{15} + e^{23} + e^{46}$                        | 359      |
| 952:377a | $0, 0, 0, 0, e^{12}, e^{34}, e^{13}, e^{25} + e^{14}, e^{36} + e^{15} + e^{24}$                        | 359      |
| 952:377b | $0, 0, 0, 0, e^{12}, e^{34}, e^{13}, -e^{14} + e^{25}, e^{15} + e^{24} + e^{36}$                       | 359      |
| 952:378a | $0, 0, 0, 0, e^{12}, e^{34}, e^{13}, e^{24} + e^{15}, e^{36} + e^{14} + e^{25}$                        | 359      |
| 952:378b | $0, 0, 0, 0, e^{12}, e^{34}, e^{13}, e^{24} - e^{15}, e^{36} + e^{25} + e^{14}$                        | 359      |
| 952:379  | $0, 0, 0, 0, e^{12}, e^{34}, e^{13}, e^{36} + e^{25}, e^{46} + e^{15} + e^{23}$                        | 359      |
| 952:380  | $0, 0, 0, 0, e^{12}, e^{34}, e^{13}, e^{46} + e^{25}, e^{15} + e^{36} + e^{24}$                        | 359      |
| 952:381a | $0, 0, 0, 0, -e^{12}, e^{14} + e^{23}, e^{24} + e^{13}, e^{15} + e^{34}, e^{16} + e^{35}$              | 359      |
| 952:381b | $0, 0, 0, 0, -e^{12}, -e^{14} + e^{23}, e^{13} + e^{24}, e^{15} + e^{34}, e^{16} + e^{35}$             | 359      |
| 952:382a | $0, 0, 0, 0, e^{12}, e^{24} + e^{13}, e^{23} + e^{14}, e^{15} + e^{34}, e^{35} + e^{26}$               | 359      |
| 952:382b | $0, 0, 0, 0, -e^{12}, e^{24} - e^{13}, e^{23} + e^{14}, e^{34} + e^{15}, e^{26} + e^{35}$              | 359      |
| 952:383a | $0, 0, 0, 0, -e^{12}, -e^{14} + e^{23}, e^{13} + e^{24}, e^{16} + e^{35}, e^{26} + e^{45}$             | 359      |
| 952:383b | $0, 0, 0, 0, -e^{12}, -e^{14} + e^{23}, e^{24} - e^{13}, e^{35} + e^{16}, e^{26} + e^{45}$             | 359      |
| 952:384  | $0, 0, 0, 0, e^{12}, e^{34}, e^{14} + e^{23}, e^{13} + e^{25}, e^{36} + e^{15} + e^{24}$               | 359      |
| 952:385a | $0, 0, 0, 0, e^{14} + e^{23}, e^{13} + e^{24}, e^{12}, e^{16} + e^{25}, e^{26} + e^{15}$               | 359      |
| 952:385b | $0, 0, 0, 0, e^{23} - e^{14}, e^{24} + e^{13}, e^{12}, -e^{16} + e^{25}, e^{15} + e^{26}$              | 359      |
| 952:386a | $0, 0, 0, 0, e^{14} + e^{23}, e^{24} + e^{13}, e^{12}, e^{26} + e^{15}, e^{46} + e^{35}$               | 359      |
| 952:386b | $0, 0, 0, 0, -e^{23} - e^{14}, e^{24} - e^{13}, e^{12}, e^{15} + e^{26}, e^{35} + e^{46}$              | 359      |
| 952:387a | $0, 0, 0, 0, e^{14} + e^{23}, e^{24} + e^{13}, e^{12}, e^{36} + e^{45}, e^{35} + e^{46}$               | 359      |
| 952:387b | $0, 0, 0, 0, e^{14} - e^{23}, e^{13} + e^{24}, e^{12}, e^{45} - e^{36}, e^{46} + e^{35}$               | 359      |
| 952:388  | $0, 0, 0, 0, -e^{12}, e^{23} + e^{14}, e^{13}, e^{15} + e^{34}, e^{35} + e^{24} + e^{16}$              | 359      |
| 952:389a | $0, 0, 0, 0, -e^{12}, e^{14} + e^{23}, e^{13}, e^{25} + e^{34}, e^{16} + e^{24} + e^{35}$              | 359      |
| 952:389b | $0, 0, 0, 0, -e^{12}, e^{23} + e^{14}, e^{13}, -e^{25} + e^{34}, e^{16} + e^{35} + e^{24}$             | 359      |
| 952:390  | $0, 0, 0, 0, -e^{12}, e^{14} + e^{23}, e^{34}, e^{13} + e^{25}, e^{16} + e^{24} + e^{35}$              | 359      |
| 952:391  | $0, 0, 0, 0, e^{12}, e^{34}, e^{23} + e^{14}, a_1, e^{15} + e^{36}, e^{13} + e^{46} + e^{25}$          | 359      |
| 952:392  | $0, 0, 0, 0, -e^{12}, e^{23} - e^{14}, e^{13}, e^{26} + e^{45}, e^{16} + e^{35} + e^{24}$              | 359      |
| 952:393  | $0, 0, 0, 0, -e^{12}, e^{23} - e^{14}, e^{34}, e^{35} + e^{16}, e^{13} + e^{45} + e^{26}$              | 359      |
| 952:394  | $0, 0, 0, 0, e^{12}, e^{34}, e^{13}, e^{36} + e^{25} + e^{14}, e^{46} + e^{15} + e^{23}$               | 359      |
| 952:395a | $0, 0, 0, 0, e^{14} + e^{23}, e^{13} + e^{24}, e^{12} + e^{34}, e^{25} + e^{16}, e^{26} + e^{15}$      | 359      |
| 952:395b | $0, 0, 0, 0, -e^{14} + e^{23}, e^{24} + e^{13}, e^{12} + e^{34}, e^{25} - e^{16}, e^{26} + e^{15}$     | 359      |
| 952:395c | $0, 0, 0, 0, -e^{14} + e^{23}, e^{13} + e^{24}, e^{34} - e^{12}, e^{25} - e^{16}, e^{26} + e^{15}$     | 359      |
| 952:396a | $0, 0, 0, 0, e^{14} + e^{23}, e^{13} + e^{24}, e^{12} + e^{34}, e^{26} + e^{15}, e^{46} + e^{35}$      | 359      |
| 952:396b | $0, 0, 0, 0, e^{14} + e^{23}, e^{13} + e^{24}, -e^{12} + e^{34}, e^{15} + e^{26}, e^{46} + e^{35}$     | 359      |
| 952:396c | $0, 0, 0, 0, -e^{23} - e^{14}, e^{24} - e^{13}, e^{34} + e^{12}, e^{15} + e^{26}, e^{35} + e^{46}$     | 359      |
| 952:396d | $0, 0, 0, 0, -e^{14} - e^{23}, -e^{13} + e^{24}, -e^{12} + e^{34}, e^{26} + e^{15}, e^{46} + e^{35}$   | 359      |
| 952:397a | $0, 0, 0, 0, e^{23} + e^{14}, e^{24} + e^{13}, e^{12}, e^{26} + e^{15}, e^{34} + e^{25} + e^{16}$      | 359      |
| 952:397b | $0, 0, 0, 0, e^{14} + e^{23}, e^{24} - e^{13}, e^{12}, -e^{15} + e^{26}, e^{16} + e^{25} + e^{34}$     | 359      |
| 952:398a | $0, 0, 0, 0, e^{23} + e^{14}, e^{24} + e^{13}, e^{12}, e^{46} + e^{35}, e^{34} + e^{26} + e^{15}$      | 359      |
| 952:398b | $0, 0, 0, 0, -e^{14} - e^{23}, -e^{13} + e^{24}, e^{12}, e^{46} + e^{35}, e^{34} + e^{26} + e^{15}$    | 359      |
| 952:399  | $0, 0, 0, 0, e^{12}, e^{34}, e^{13}, a_1 + e^{24}, e^{14} + e^{25} + e^{36}, e^{15} + e^{46} + e^{23}$ | 359      |
| 952:400  | $0, 0, 0, 0, -e^{12}, -e^{13} + e^{24}, e^{34}, e^{45} + e^{23} + e^{16}, e^{14} + e^{26} + e^{35}$    | 359      |
| 952:401  | $0, 0, 0, 0, e^{12}, e^{13}, e^{24}, e^{15}, e^{27} + e^{16}$                                          | 259      |
| 952:402  | $0, 0, 0, 0, e^{12}, e^{13}, e^{14}, e^{15}, e^{17} + e^{36}$                                          | 259      |
| 952:403  | $0, 0, 0, 0, e^{12}, e^{13}, e^{14}, e^{25}, e^{36} + e^{17}$                                          | 259      |
| 952:404  | $0, 0, 0, 0, e^{12}, e^{13}, e^{24}, e^{15}, e^{27} + e^{36}$                                          | 259      |
| 952:405  | $0, 0, 0, 0, e^{12}, e^{13}, e^{24}, e^{25}, e^{36} + e^{27}$                                          | 259      |
| 952:406  | $0, 0, 0, 0, e^{12}, e^{13}, e^{34}, e^{15}, e^{37} + e^{16}$                                          | 259      |
| 952:407  | $0, 0, 0, 0, e^{12}, e^{13}, e^{34}, e^{25}, e^{37} + e^{16}$                                          | 259      |
| 952:408a | $0, 0, 0, 0, e^{12}, e^{13}, e^{14}, e^{15}, e^{36} + e^{47}$                                          | 259      |
| 952:408b | $0, 0, 0, 0, e^{12}, -e^{13}, e^{14}, e^{15}, e^{47} + e^{36}$                                         | 259      |
| 952:409  | $0, 0, 0, 0, e^{12}, e^{13}, e^{14}, e^{15}, e^{46} + e^{37}$                                          | 259      |
| 952:410a | $0, 0, 0, 0, e^{12}, e^{13}, e^{14}, e^{25}, e^{47} + e^{36}$                                          | 259      |
| 952:410b | $0, 0, 0, 0, e^{12}, -e^{13}, e^{14}, e^{25}, e^{47} + e^{36}$                                         | 259      |
| 952:411  | $0, 0, 0, 0, e^{12}, e^{13}, e^{14}, e^{25}, e^{37} + e^{46}$                                          | 259      |
| 952:412  | $0, 0, 0, 0, e^{12}, e^{13}, e^{24}, e^{15}, e^{36} + e^{47}$                                          | 259      |
| 952:413a | $0, 0, 0, 0, e^{12}, e^{13}, e^{34}, e^{15}, e^{16} + e^{47}$                                          | 259      |
| 952:413b | $0, 0, 0, 0, e^{12}, -e^{13}, e^{34}, e^{15}, e^{16} + e^{47}$                                         | 259      |
| 952:414  | $0, 0, 0, 0, e^{12}, -e^{13}, e^{34}, e^{15}, e^{46} + e^{17}$                                         | 259      |

Table 2 – Continued to next page

Table 2 – Continued from previous page

| Name     | $\mathfrak{g}$                                                          | UCS Dim. |
|----------|-------------------------------------------------------------------------|----------|
| 952:415a | $0, 0, 0, 0, e^{12}, e^{13}, e^{34}, e^{25}, e^{47} + e^{16}$           | 259      |
| 952:415b | $0, 0, 0, 0, e^{12}, -e^{13}, e^{34}, e^{25}, e^{47} + e^{16}$          | 259      |
| 952:416  | $0, 0, 0, 0, e^{12}, -e^{13}, e^{34}, e^{25}, e^{17} + e^{46}$          | 259      |
| 952:417  | $0, 0, 0, 0, e^{12}, e^{13}, e^{34}, e^{15}, e^{47} + e^{36}$           | 259      |
| 952:418  | $0, 0, 0, 0, e^{12}, e^{13}, e^{34}, e^{25}, e^{36} + e^{47}$           | 259      |
| 952:419  | $0, 0, 0, 0, e^{12}, e^{13}, e^{14} + e^{23}, e^{15}, e^{17} + e^{26}$  | 259      |
| 952:420  | $0, 0, 0, 0, e^{12}, e^{13}, e^{23} + e^{14}, e^{25}, e^{17} + e^{26}$  | 259      |
| 952:421  | $0, 0, 0, 0, e^{12}, e^{13}, e^{14} + e^{23}, e^{15}, e^{37} + e^{46}$  | 259      |
| 952:422  | $0, 0, 0, 0, e^{12}, e^{13}, e^{23} + e^{14}, e^{25}, e^{37} + e^{46}$  | 259      |
| 952:423  | $0, 0, 0, 0, e^{12}, e^{34}, e^{14} + e^{23}, e^{15}, e^{37} + e^{16}$  | 259      |
| 952:424  | $0, 0, 0, 0, e^{12}, e^{34}, e^{24} + e^{13}, e^{15}, e^{37} + e^{26}$  | 259      |
| 952:425  | $0, 0, 0, 0, e^{12}, e^{13}, e^{24}, e^{15} + e^{23}, e^{16} + e^{27}$  | 259      |
| 952:426  | $0, 0, 0, 0, e^{12}, e^{13}, e^{14}, e^{23} + e^{15}, e^{17} + e^{36}$  | 259      |
| 952:427  | $0, 0, 0, 0, e^{12}, e^{13}, e^{24}, e^{15} + e^{23}, e^{27} + e^{36}$  | 259      |
| 952:428  | $0, 0, 0, 0, e^{12}, e^{13}, e^{34}, e^{15} + e^{23}, e^{16} + e^{37}$  | 259      |
| 952:429  | $0, 0, 0, 0, e^{12}, e^{13}, e^{14}, e^{15}, e^{23} + e^{16} + e^{47}$  | 259      |
| 952:430  | $0, 0, 0, 0, e^{12}, e^{13}, e^{14}, e^{25}, e^{23} + e^{47} + e^{16}$  | 259      |
| 952:431  | $0, 0, 0, 0, e^{12}, e^{13}, e^{24}, e^{15}, e^{23} + e^{47} + e^{16}$  | 259      |
| 952:432  | $0, 0, 0, 0, e^{12}, e^{13}, e^{24}, e^{15}, e^{36} + e^{27} + e^{14}$  | 259      |
| 952:433  | $0, 0, 0, 0, e^{12}, e^{13}, e^{24}, e^{15}, e^{27} + e^{34} + e^{16}$  | 259      |
| 952:434  | $0, 0, 0, 0, e^{12}, e^{13}, e^{14}, e^{15} + e^{23}, e^{47} + e^{16}$  | 259      |
| 952:435  | $0, 0, 0, 0, e^{12}, e^{13}, e^{24}, e^{15} + e^{23}, e^{16} + e^{47}$  | 259      |
| 952:436a | $0, 0, 0, 0, e^{12}, e^{13}, e^{14}, e^{15} + e^{23}, e^{36} + e^{47}$  | 259      |
| 952:436b | $0, 0, 0, 0, e^{12}, -e^{13}, e^{14}, e^{15} + e^{23}, e^{36} + e^{47}$ | 259      |
| 952:437  | $0, 0, 0, 0, e^{12}, e^{13}, e^{14}, e^{23} + e^{15}, e^{46} + e^{37}$  | 259      |
| 952:438  | $0, 0, 0, 0, e^{12}, e^{13}, e^{24}, e^{15} + e^{23}, e^{47} + e^{36}$  | 259      |
| 952:439a | $0, 0, 0, 0, e^{12}, e^{13}, e^{34}, e^{15}, e^{23} + e^{47} + e^{16}$  | 259      |
| 952:439b | $0, 0, 0, 0, e^{12}, -e^{13}, e^{34}, e^{15}, e^{16} + e^{47} + e^{23}$ | 259      |
| 952:440  | $0, 0, 0, 0, e^{12}, e^{13}, e^{34}, e^{15}, e^{16} + e^{37} + e^{24}$  | 259      |
| 952:441  | $0, 0, 0, 0, e^{12}, -e^{13}, e^{34}, e^{15}, e^{46} + e^{17} + e^{23}$ | 259      |
| 952:442a | $0, 0, 0, 0, e^{12}, e^{13}, e^{34}, e^{25}, e^{23} + e^{47} + e^{16}$  | 259      |
| 952:442b | $0, 0, 0, 0, e^{12}, -e^{13}, e^{34}, e^{25}, e^{23} + e^{47} + e^{16}$ | 259      |
| 952:443  | $0, 0, 0, 0, e^{12}, e^{13}, e^{34}, e^{25}, e^{24} + e^{37} + e^{16}$  | 259      |
| 952:444  | $0, 0, 0, 0, e^{12}, -e^{13}, e^{34}, e^{25}, e^{46} + e^{23} + e^{17}$ | 259      |
| 952:445a | $0, 0, 0, 0, e^{12}, e^{13}, e^{34}, e^{15} + e^{23}, e^{16} + e^{47}$  | 259      |
| 952:445b | $0, 0, 0, 0, e^{12}, -e^{13}, e^{34}, e^{15} + e^{23}, e^{47} + e^{16}$ | 259      |
| 952:446  | $0, 0, 0, 0, e^{12}, -e^{13}, e^{34}, e^{15} + e^{23}, e^{17} + e^{46}$ | 259      |
| 952:447  | $0, 0, 0, 0, e^{12}, e^{13}, e^{34}, e^{23} + e^{15}, e^{47} + e^{36}$  | 259      |
| 952:448  | $0, 0, 0, 0, e^{12}, e^{13}, e^{24}, e^{34} + e^{15}, e^{27} + e^{16}$  | 259      |
| 952:449  | $0, 0, 0, 0, e^{12}, e^{13}, e^{14}, e^{15} + e^{34}, e^{17} + e^{36}$  | 259      |
| 952:450  | $0, 0, 0, 0, e^{12}, e^{13}, e^{14}, e^{34} + e^{25}, e^{17} + e^{36}$  | 259      |
| 952:451  | $0, 0, 0, 0, e^{12}, e^{13}, e^{24}, e^{15} + e^{34}, e^{27} + e^{36}$  | 259      |
| 952:452  | $0, 0, 0, 0, e^{12}, e^{13}, e^{24}, e^{25} + e^{34}, e^{36} + e^{27}$  | 259      |
| 952:453  | $0, 0, 0, 0, e^{12}, e^{13}, e^{34}, e^{25} + e^{14}, e^{16} + e^{37}$  | 259      |
| 952:454  | $0, 0, 0, 0, e^{12}, e^{13}, e^{34}, e^{15} + e^{24}, e^{16} + e^{37}$  | 259      |
| 952:455a | $0, 0, 0, 0, e^{12}, e^{13}, e^{14}, e^{15} + e^{34}, e^{47} + e^{36}$  | 259      |
| 952:455b | $0, 0, 0, 0, e^{12}, -e^{13}, e^{14}, e^{34} + e^{15}, e^{36} + e^{47}$ | 259      |
| 952:456  | $0, 0, 0, 0, e^{12}, e^{13}, e^{14}, e^{34} + e^{15}, e^{37} + e^{46}$  | 259      |
| 952:457a | $0, 0, 0, 0, e^{12}, e^{13}, e^{14}, e^{25} + e^{34}, e^{47} + e^{36}$  | 259      |
| 952:457b | $0, 0, 0, 0, e^{12}, -e^{13}, e^{14}, e^{25} + e^{34}, e^{36} + e^{47}$ | 259      |
| 952:458  | $0, 0, 0, 0, e^{12}, e^{13}, e^{14}, e^{25} + e^{34}, e^{46} + e^{37}$  | 259      |
| 952:459  | $0, 0, 0, 0, e^{12}, e^{13}, e^{24}, e^{15} + e^{34}, e^{47} + e^{36}$  | 259      |
| 952:460a | $0, 0, 0, 0, e^{12}, e^{13}, e^{34}, e^{25} + e^{14}, e^{47} + e^{16}$  | 259      |
| 952:460b | $0, 0, 0, 0, e^{12}, -e^{13}, e^{34}, e^{25} + e^{14}, e^{47} + e^{16}$ | 259      |
| 952:461a | $0, 0, 0, 0, e^{12}, e^{13}, e^{34}, e^{24} + e^{15}, e^{16} + e^{47}$  | 259      |
| 952:461b | $0, 0, 0, 0, e^{12}, -e^{13}, e^{34}, e^{15} + e^{24}, e^{16} + e^{47}$ | 259      |
| 952:462  | $0, 0, 0, 0, e^{12}, -e^{13}, e^{34}, e^{25} + e^{14}, e^{46} + e^{17}$ | 259      |
| 952:463  | $0, 0, 0, 0, e^{12}, -e^{13}, e^{34}, e^{24} + e^{15}, e^{46} + e^{17}$ | 259      |

Table 2 – Continued to next page

Table 2 – Continued from previous page

| Name     | $\mathfrak{g}$                                                           | UCS Dim. |
|----------|--------------------------------------------------------------------------|----------|
| 952:464  | $0, 0, 0, 0, e^{12}, e^{13}, e^{34}, e^{25} + e^{14}, e^{36} + e^{47}$   | 259      |
| 952:465  | $0, 0, 0, 0, e^{12}, e^{13}, e^{34}, e^{15} + e^{24}, e^{47} + e^{36}$   | 259      |
| 952:466a | $0, 0, 0, 0, e^{12}, e^{13}, e^{14}, e^{15}, e^{36} + e^{17} + e^{25}$   | 259      |
| 952:466b | $0, 0, 0, 0, -e^{12}, e^{13}, e^{14}, e^{15}, e^{17} + e^{25} + e^{36}$  | 259      |
| 952:467  | $0, 0, 0, 0, e^{12}, e^{13}, e^{14}, e^{15}, e^{17} + e^{26} + e^{35}$   | 259      |
| 952:468  | $0, 0, 0, 0, e^{12}, e^{13}, e^{14}, e^{25}, e^{17} + e^{35} + e^{26}$   | 259      |
| 952:469  | $0, 0, 0, 0, e^{12}, e^{13}, e^{24}, e^{25}, e^{36} + e^{27} + e^{15}$   | 259      |
| 952:470  | $0, 0, 0, 0, e^{12}, e^{13}, e^{34}, e^{15}, e^{25} + e^{37} + e^{16}$   | 259      |
| 952:471a | $0, 0, 0, 0, e^{12}, e^{13}, e^{14}, e^{15}, e^{36} + e^{47} + e^{25}$   | 259      |
| 952:471b | $0, 0, 0, 0, e^{12}, -e^{13}, e^{14}, e^{15}, e^{25} + e^{47} + e^{36}$  | 259      |
| 952:471c | $0, 0, 0, 0, -e^{12}, e^{13}, e^{14}, e^{15}, e^{47} + e^{36} + e^{25}$  | 259      |
| 952:472  | $0, 0, 0, 0, e^{12}, e^{13}, e^{14}, e^{15}, e^{26} + e^{35} + e^{47}$   | 259      |
| 952:473  | $0, 0, 0, 0, e^{12}, e^{13}, e^{14}, e^{15}, e^{37} + e^{46} + e^{25}$   | 259      |
| 952:474a | $0, 0, 0, 0, e^{12}, e^{13}, e^{14}, e^{25}, e^{47} + e^{36} + e^{15}$   | 259      |
| 952:474b | $0, 0, 0, 0, e^{12}, -e^{13}, e^{14}, e^{25}, e^{15} + e^{36} + e^{47}$  | 259      |
| 952:475  | $0, 0, 0, 0, e^{12}, e^{13}, e^{14}, e^{25}, e^{15} + e^{37} + e^{46}$   | 259      |
| 952:476  | $0, 0, 0, 0, e^{12}, e^{13}, e^{14}, e^{25}, e^{35} + e^{47} + e^{26}$   | 259      |
| 952:477  | $0, 0, 0, 0, -e^{12}, e^{13}, e^{24}, e^{15}, e^{45} + e^{36} + e^{17}$  | 259      |
| 952:478a | $0, 0, 0, 0, e^{12}, e^{13}, e^{24}, e^{15}, e^{25} + e^{47} + e^{36}$   | 259      |
| 952:478b | $0, 0, 0, 0, -e^{12}, e^{13}, e^{24}, e^{15}, e^{36} + e^{47} + e^{25}$  | 259      |
| 952:479  | $0, 0, 0, 0, e^{12}, e^{13}, e^{24}, e^{15}, e^{26} + e^{35} + e^{47}$   | 259      |
| 952:480a | $0, 0, 0, 0, e^{12}, e^{13}, e^{34}, e^{15}, e^{47} + e^{25} + e^{16}$   | 259      |
| 952:480b | $0, 0, 0, 0, e^{12}, -e^{13}, e^{34}, e^{15}, e^{47} + e^{25} + e^{16}$  | 259      |
| 952:481  | $0, 0, 0, 0, e^{12}, -e^{13}, e^{34}, e^{15}, e^{25} + e^{17} + e^{46}$  | 259      |
| 952:482a | $0, 0, 0, 0, e^{12}, e^{13}, e^{34}, e^{15}, e^{47} + e^{36} + e^{25}$   | 259      |
| 952:482b | $0, 0, 0, 0, -e^{12}, e^{13}, e^{34}, e^{15}, e^{36} + e^{47} + e^{25}$  | 259      |
| 952:483  | $0, 0, 0, 0, e^{12}, e^{13}, e^{34}, e^{15}, e^{26} + e^{35} + e^{47}$   | 259      |
| 952:484  | $0, 0, 0, 0, e^{12}, e^{13}, e^{34}, e^{25}, e^{15} + e^{36} + e^{47}$   | 259      |
| 952:485  | $0, 0, 0, 0, e^{12}, e^{13}, e^{34}, e^{25}, e^{35} + e^{47} + e^{26}$   | 259      |
| 952:486  | $0, 0, 0, 0, e^{12}, e^{13}, e^{24}, e^{25} + e^{16}, e^{27} + e^{15}$   | 259      |
| 952:487  | $0, 0, 0, 0, e^{12}, e^{13}, e^{14}, e^{15} + e^{36}, e^{25} + e^{17}$   | 259      |
| 952:488  | $0, 0, 0, 0, e^{12}, e^{13}, e^{14}, e^{26} + e^{35}, e^{17} + e^{25}$   | 259      |
| 952:489a | $0, 0, 0, 0, e^{12}, e^{13}, e^{24}, e^{36} + e^{25}, e^{15} + e^{27}$   | 259      |
| 952:489b | $0, 0, 0, 0, -e^{12}, e^{13}, e^{24}, e^{25} + e^{36}, e^{27} + e^{15}$  | 259      |
| 952:490  | $0, 0, 0, 0, e^{12}, e^{13}, e^{24}, e^{35} + e^{26}, e^{15} + e^{27}$   | 259      |
| 952:491  | $0, 0, 0, 0, e^{12}, e^{13}, e^{34}, e^{25} + e^{16}, e^{37} + e^{15}$   | 259      |
| 952:492  | $0, 0, 0, 0, e^{12}, e^{13}, e^{34}, e^{36} + e^{15}, e^{37} + e^{25}$   | 259      |
| 952:493a | $0, 0, 0, 0, e^{12}, e^{13}, e^{34}, e^{36} + e^{25}, e^{15} + e^{37}$   | 259      |
| 952:493b | $0, 0, 0, 0, -e^{12}, e^{13}, e^{34}, e^{25} + e^{36}, e^{15} + e^{37}$  | 259      |
| 952:494  | $0, 0, 0, 0, e^{12}, e^{13}, e^{34}, e^{26} + e^{35}, e^{15} + e^{37}$   | 259      |
| 952:495  | $0, 0, 0, 0, e^{12}, e^{13}, e^{34}, e^{35} + e^{26}, e^{25} + e^{37}$   | 259      |
| 952:496a | $0, 0, 0, 0, e^{12}, e^{13}, e^{14}, e^{36} + e^{15}, e^{47} + e^{25}$   | 259      |
| 952:496b | $0, 0, 0, 0, -e^{12}, e^{13}, e^{14}, e^{15} + e^{36}, e^{25} + e^{47}$  | 259      |
| 952:497  | $0, 0, 0, 0, e^{12}, e^{13}, e^{14}, e^{15} + e^{36}, e^{45} + e^{27}$   | 259      |
| 952:498a | $0, 0, 0, 0, e^{12}, e^{13}, e^{14}, e^{26} + e^{35}, e^{25} + e^{47}$   | 259      |
| 952:498b | $0, 0, 0, 0, -e^{12}, -e^{13}, e^{14}, e^{35} + e^{26}, e^{47} + e^{25}$ | 259      |
| 952:499  | $0, 0, 0, 0, e^{12}, e^{13}, e^{14}, e^{26} + e^{35}, e^{27} + e^{45}$   | 259      |
| 952:500  | $0, 0, 0, 0, -e^{12}, e^{13}, e^{24}, e^{15} + e^{36}, e^{45} + e^{17}$  | 259      |
| 952:501a | $0, 0, 0, 0, e^{12}, e^{13}, e^{24}, e^{36} + e^{15}, e^{47} + e^{25}$   | 259      |
| 952:501b | $0, 0, 0, 0, e^{12}, -e^{13}, e^{24}, e^{15} + e^{36}, e^{47} + e^{25}$  | 259      |
| 952:502a | $0, 0, 0, 0, e^{12}, e^{13}, e^{24}, e^{36} + e^{25}, e^{47} + e^{15}$   | 259      |
| 952:502b | $0, 0, 0, 0, e^{12}, -e^{13}, e^{24}, e^{36} + e^{25}, e^{47} + e^{15}$  | 259      |
| 952:502c | $0, 0, 0, 0, -e^{12}, -e^{13}, e^{24}, e^{25} + e^{36}, e^{15} + e^{47}$ | 259      |
| 952:503a | $0, 0, 0, 0, e^{12}, e^{13}, e^{24}, e^{26} + e^{35}, e^{47} + e^{15}$   | 259      |
| 952:503b | $0, 0, 0, 0, -e^{12}, -e^{13}, e^{24}, e^{26} + e^{35}, e^{15} + e^{47}$ | 259      |
| 952:504  | $0, 0, 0, 0, -e^{12}, -e^{13}, e^{24}, e^{26} + e^{35}, e^{17} + e^{45}$ | 259      |
| 952:505  | $0, 0, 0, 0, e^{12}, e^{13}, e^{34}, e^{25} + e^{16}, e^{47} + e^{15}$   | 259      |
| 952:506  | $0, 0, 0, 0, e^{12}, e^{13}, e^{34}, e^{15} + e^{36}, e^{47} + e^{25}$   | 259      |

Table 2 – Continued to next page

Table 2 – Continued from previous page

| Name     | $\mathfrak{g}$                                                                               | UCS Dim. |
|----------|----------------------------------------------------------------------------------------------|----------|
| 952:507a | $0, 0, 0, 0, e^{12}, e^{13}, e^{34}, e^{25} + e^{36}, e^{15} + e^{47}$                       | 259      |
| 952:507b | $0, 0, 0, 0, -e^{12}, e^{13}, e^{34}, e^{36} + e^{25}, e^{15} + e^{47}$                      | 259      |
| 952:508  | $0, 0, 0, 0, e^{12}, e^{13}, e^{34}, e^{35} + e^{26}, e^{47} + e^{15}$                       | 259      |
| 952:509  | $0, 0, 0, 0, e^{12}, e^{13}, e^{34}, e^{35} + e^{26}, e^{47} + e^{25}$                       | 259      |
| 952:510a | $0, 0, 0, 0, e^{12}, e^{14} + e^{23}, e^{13} + e^{24}, e^{15}, e^{16} + e^{27}$              | 259      |
| 952:510b | $0, 0, 0, 0, e^{12}, e^{23} - e^{14}, e^{24} + e^{13}, e^{15}, e^{27} + e^{16}$              | 259      |
| 952:511a | $0, 0, 0, 0, e^{12}, e^{14} + e^{23}, e^{13} + e^{24}, e^{15}, e^{36} + e^{47}$              | 259      |
| 952:511b | $0, 0, 0, 0, e^{12}, -e^{23} + e^{14}, e^{24} + e^{13}, e^{15}, e^{47} + e^{36}$             | 259      |
| 952:512a | $0, 0, 0, 0, e^{12}, e^{13} + e^{24}, e^{14} + e^{23}, e^{15}, e^{47} + e^{36}$              | 259      |
| 952:512b | $0, 0, 0, 0, e^{12}, e^{24} - e^{13}, e^{23} + e^{14}, e^{15}, e^{47} + e^{36}$              | 259      |
| 952:513  | $0, 0, 0, 0, e^{12}, e^{13}, e^{14} + e^{23}, e^{15}, e^{34} + e^{17} + e^{26}$              | 259      |
| 952:514  | $0, 0, 0, 0, e^{12}, e^{13}, e^{23} + e^{14}, e^{25}, e^{17} + e^{26} + e^{34}$              | 259      |
| 952:515  | $0, 0, 0, 0, e^{12}, e^{13}, e^{14} + e^{23}, e^{15} + e^{24}, e^{26} + e^{17}$              | 259      |
| 952:516  | $0, 0, 0, 0, e^{12}, e^{13}, e^{23} + e^{14}, e^{15} + e^{34}, e^{17} + e^{26}$              | 259      |
| 952:517  | $0, 0, 0, 0, e^{12}, e^{13}, e^{14} + e^{23}, e^{25} + e^{34}, e^{17} + e^{26}$              | 259      |
| 952:518  | $0, 0, 0, 0, e^{12}, e^{13}, e^{23} + e^{14}, e^{24} + e^{15}, e^{37} + e^{46}$              | 259      |
| 952:519  | $0, 0, 0, 0, e^{12}, e^{13}, e^{14} + e^{23}, e^{34} + e^{15}, e^{37} + e^{46}$              | 259      |
| 952:520  | $0, 0, 0, 0, e^{12}, e^{13}, e^{23} + e^{14}, e^{25} + e^{34}, e^{37} + e^{46}$              | 259      |
| 952:521  | $0, 0, 0, 0, e^{12}, e^{34}, e^{14} + e^{23}, e^{13} + e^{25}, e^{16} + e^{37}$              | 259      |
| 952:522  | $0, 0, 0, 0, e^{12}, e^{34}, e^{24} - e^{13}, e^{15}, e^{47} + e^{16} + e^{23}$              | 259      |
| 952:523  | $0, 0, 0, 0, e^{12}, e^{34}, e^{13} + e^{24}, e^{15}, e^{37} + e^{14} + e^{26}$              | 259      |
| 952:524  | $0, 0, 0, 0, e^{12}, e^{34}, e^{24} - e^{13}, e^{15} + e^{23}, e^{16} + e^{47}$              | 259      |
| 952:525  | $0, 0, 0, 0, (-1 + a_2)e^{12}, a_2e^{13}, e^{14} + e^{23}, e^{15}, e^{35} + e^{17} + e^{26}$ | 259      |
| 952:526  | $0, 0, 0, 0, (-1 + a_2)e^{12}, e^{13}a_2, e^{14} + e^{23}, e^{25}, e^{17} + e^{35} + e^{26}$ | 259      |
| 952:527a | $0, 0, 0, 0, e^{12}, e^{13}, e^{14} + e^{23}, e^{15}, e^{27} + e^{16} + e^{45}$              | 259      |
| 952:527b | $0, 0, 0, 0, e^{12}, -e^{13}, e^{23} + e^{14}, e^{15}, e^{45} + e^{27} + e^{16}$             | 259      |
| 952:528a | $0, 0, 0, 0, e^{12}, e^{13}, e^{14} + e^{23}, e^{25}, e^{16} + e^{45} + e^{27}$              | 259      |
| 952:528b | $0, 0, 0, 0, e^{12}, -e^{13}, e^{23} + e^{14}, e^{25}, e^{27} + e^{16} + e^{45}$             | 259      |
| 952:529  | $0, 0, 0, 0, e^{12}, e^{13}, e^{14} + e^{23}, e^{15}, e^{25} + e^{46} + e^{37}$              | 259      |
| 952:530  | $0, 0, 0, 0, e^{12}, e^{13}, e^{23} + e^{14}, e^{15}, e^{36} + e^{45} + e^{27}$              | 259      |
| 952:531a | $0, 0, 0, 0, e^{12}, e^{13}, e^{14} + e^{23}, e^{25}, e^{37} + e^{46} + e^{15}$              | 259      |
| 952:531b | $0, 0, 0, 0, -e^{12}, e^{13}, e^{23} + e^{14}, e^{25}, e^{15} + e^{37} + e^{46}$             | 259      |
| 952:532  | $0, 0, 0, 0, e^{12}, e^{13}, e^{14} + e^{23}, e^{25}, e^{45} + e^{36} + e^{27}$              | 259      |
| 952:533  | $0, 0, 0, 0, e^{12}, e^{34}, e^{23} + e^{14}, e^{15}, e^{37} + e^{16} + e^{25}$              | 259      |
| 952:534  | $0, 0, 0, 0, -e^{12}, e^{34}, e^{24} + e^{13}, e^{15}, e^{17} + e^{36} + e^{45}$             | 259      |
| 952:535  | $0, 0, 0, 0, e^{12}, e^{34}, e^{24} + e^{13}, e^{15}, e^{27} + e^{35} + e^{46}$              | 259      |
| 952:536  | $0, 0, 0, 0, -e^{12}, e^{13}, e^{23} + e^{14}, e^{25} + e^{16}, e^{35} + e^{17}$             | 259      |
| 952:537  | $0, 0, 0, 0, -e^{12}, e^{13}, e^{14} + e^{23}, e^{36} + e^{15}, e^{35} + e^{17}$             | 259      |
| 952:538a | $0, 0, 0, 0, -e^{12}, e^{13}, e^{14} + e^{23}, e^{36} + e^{25}, e^{35} + e^{17}$             | 259      |
| 952:538b | $0, 0, 0, 0, -e^{12}, -e^{13}, e^{14} + e^{23}, e^{36} + e^{25}, e^{17} + e^{35}$            | 259      |
| 952:539  | $0, 0, 0, 0, e^{12}, e^{13}, e^{14} + e^{23}, e^{25} + e^{16}, e^{45} + e^{27}$              | 259      |
| 952:540  | $0, 0, 0, 0, e^{12}, e^{13}, e^{23} + e^{14}, e^{36} + e^{15}, e^{45} + e^{27}$              | 259      |
| 952:541a | $0, 0, 0, 0, e^{12}, e^{13}, e^{14} + e^{23}, e^{25} + e^{36}, e^{45} + e^{27}$              | 259      |
| 952:541b | $0, 0, 0, 0, e^{12}, -e^{13}, e^{23} + e^{14}, e^{25} + e^{36}, e^{27} + e^{45}$             | 259      |
| 952:542  | $0, 0, 0, 0, e^{12}, e^{13}, e^{14} + e^{23}, e^{26} + e^{35}, e^{27} + e^{45}$              | 259      |
| 952:543  | $0, 0, 0, 0, -e^{12}, e^{34}, e^{14} + e^{23}, e^{15} + e^{36}, e^{35} + e^{17}$             | 259      |
| 952:544  | $0, 0, 0, 0, e^{12}, e^{34}, e^{24} + e^{13}, e^{15} + e^{36}, e^{27} + e^{35}$              | 259      |
| 952:545  | $0, 0, 0, 0, -e^{12}, e^{34}, e^{24} + e^{13}, e^{36} + e^{15}, e^{45} + e^{17}$             | 259      |
| 952:546  | $0, 0, 0, 0, e^{12}, e^{34}, e^{23} + e^{14}, e^{36} + e^{15}, e^{45} + e^{27}$              | 259      |
| 952:547  | $0, 0, 0, 0, e^{23} + e^{14}, -e^{12}, e^{13}, e^{15} + e^{36}, e^{35} + e^{47}$             | 259      |
| 952:548  | $0, 0, 0, 0, e^{14} + e^{23}, e^{12}, e^{13}, e^{46} + e^{25}, e^{35} + e^{47}$              | 259      |
| 952:549  | $0, 0, 0, 0, e^{14} + e^{23}, -e^{12}, e^{34}, e^{15} + e^{36}, e^{35} + e^{17}$             | 259      |
| 952:550  | $0, 0, 0, 0, e^{14} - e^{23}, e^{12}, e^{34}, e^{36} + e^{15}, e^{45} + e^{27}$              | 259      |
| 952:551  | $0, 0, 0, 0, e^{12}, e^{13}, e^{14}, e^{15} + e^{23}, e^{17} + e^{24} + e^{36}$              | 259      |
| 952:552  | $0, 0, 0, 0, e^{12}, e^{13}, e^{24}, e^{23} + e^{15}, e^{36} + e^{14} + e^{27}$              | 259      |
| 952:553a | $0, 0, 0, 0, e^{12}, e^{13}, e^{24}, e^{15} + e^{23}, e^{34} + e^{27} + e^{16}$              | 259      |
| 952:553b | $0, 0, 0, 0, -e^{12}, e^{13}, e^{24}, e^{15} + e^{23}, e^{16} + e^{34} + e^{27}$             | 259      |
| 952:554  | $0, 0, 0, 0, e^{12}, e^{13}, e^{34}, e^{23} + e^{15}, e^{16} + e^{37} + e^{24}$              | 259      |

Table 2 – Continued to next page



Table 2 – Continued from previous page

| Name     | $\mathfrak{g}$                                                                    | UCS Dim. |
|----------|-----------------------------------------------------------------------------------|----------|
| 952:555  | $0, 0, 0, 0, e^{12}, e^{13}, e^{14}, e^{15} + e^{34}, e^{16} + e^{47} + e^{23}$   | 259      |
| 952:556  | $0, 0, 0, 0, e^{12}, e^{13}, e^{14}, e^{25} + e^{34}, e^{16} + e^{23} + e^{47}$   | 259      |
| 952:557  | $0, 0, 0, 0, e^{12}, e^{13}, e^{24}, e^{15} + e^{34}, e^{23} + e^{16} + e^{47}$   | 259      |
| 952:558  | $0, 0, 0, 0, e^{12}, e^{13}, e^{24}, e^{34} + e^{15}, e^{27} + e^{36} + e^{14}$   | 259      |
| 952:559a | $0, 0, 0, 0, e^{12}, e^{13}, e^{34}, e^{14} + e^{25}, e^{23} + e^{47} + e^{16}$   | 259      |
| 952:559b | $0, 0, 0, 0, e^{12}, -e^{13}, e^{34}, e^{25} + e^{14}, e^{16} + e^{23} + e^{47}$  | 259      |
| 952:560  | $0, 0, 0, 0, e^{12}, e^{13}, e^{34}, e^{25} + e^{14}, e^{37} + e^{16} + e^{24}$   | 259      |
| 952:561  | $0, 0, 0, 0, e^{12}, -e^{13}, e^{34}, e^{25} + e^{14}, e^{17} + e^{46} + e^{23}$  | 259      |
| 952:562a | $0, 0, 0, 0, e^{12}, e^{13}, e^{34}, e^{15} + e^{24}, e^{16} + e^{23} + e^{47}$   | 259      |
| 952:562b | $0, 0, 0, 0, e^{12}, -e^{13}, e^{34}, e^{15} + e^{24}, e^{47} + e^{23} + e^{16}$  | 259      |
| 952:563  | $0, 0, 0, 0, e^{12}, -e^{13}, e^{34}, e^{24} + e^{15}, e^{23} + e^{46} + e^{17}$  | 259      |
| 952:564a | $0, 0, 0, 0, e^{12}, e^{13}, e^{14}, e^{15} + e^{23}, e^{36} + e^{25} + e^{17}$   | 259      |
| 952:564b | $0, 0, 0, 0, -e^{12}, e^{13}, e^{14}, e^{15} + e^{23}, e^{25} + e^{17} + e^{36}$  | 259      |
| 952:565  | $0, 0, 0, 0, e^{12}, e^{13}, e^{14}, e^{23} + e^{15}, e^{17} + e^{26} + e^{35}$   | 259      |
| 952:566  | $0, 0, 0, 0, e^{12}, e^{13}, e^{34}, e^{15} + e^{23}, e^{16} + e^{25} + e^{37}$   | 259      |
| 952:567a | $0, 0, 0, 0, e^{12}, e^{13}, e^{14}, e^{15} + e^{23}, e^{47} + e^{25} + e^{16}$   | 259      |
| 952:567b | $0, 0, 0, 0, -e^{12}, e^{13}, e^{14}, e^{23} + e^{15}, e^{47} + e^{25} + e^{16}$  | 259      |
| 952:568  | $0, 0, 0, 0, e^{12}, e^{13}, e^{14}, e^{23} + e^{15}, e^{45} + e^{27} + e^{16}$   | 259      |
| 952:569  | $0, 0, 0, 0, e^{12}, e^{13}, e^{24}, e^{15} + e^{23}, e^{47} + e^{25} + e^{16}$   | 259      |
| 952:570a | $0, 0, 0, 0, e^{12}, e^{13}, e^{14}, e^{15} + e^{23}, e^{36} + e^{47} + e^{25}$   | 259      |
| 952:570b | $0, 0, 0, 0, e^{12}, -e^{13}, e^{14}, e^{15} + e^{23}, e^{25} + e^{47} + e^{36}$  | 259      |
| 952:570c | $0, 0, 0, 0, -e^{12}, e^{13}, e^{14}, e^{15} + e^{23}, e^{47} + e^{36} + e^{25}$  | 259      |
| 952:570d | $0, 0, 0, 0, -e^{12}, -e^{13}, e^{14}, e^{15} + e^{23}, e^{36} + e^{47} + e^{25}$ | 259      |
| 952:571  | $0, 0, 0, 0, e^{12}, e^{13}, e^{14}, e^{15} + e^{23}, e^{35} + e^{47} + e^{26}$   | 259      |
| 952:572  | $0, 0, 0, 0, e^{12}, e^{13}, e^{14}, e^{15} + e^{23}, e^{46} + e^{25} + e^{37}$   | 259      |
| 952:573  | $0, 0, 0, 0, e^{12}, e^{13}, e^{14}, e^{23} + e^{15}, e^{27} + e^{36} + e^{45}$   | 259      |
| 952:574  | $0, 0, 0, 0, -e^{12}, e^{13}, e^{24}, e^{15} + e^{23}, e^{17} + e^{45} + e^{36}$  | 259      |
| 952:575a | $0, 0, 0, 0, e^{12}, e^{13}, e^{24}, e^{15} + e^{23}, e^{47} + e^{25} + e^{36}$   | 259      |
| 952:575b | $0, 0, 0, 0, -e^{12}, e^{13}, e^{24}, e^{23} + e^{15}, e^{47} + e^{36} + e^{25}$  | 259      |
| 952:576  | $0, 0, 0, 0, e^{12}, e^{13}, e^{24}, e^{15} + e^{23}, e^{26} + e^{35} + e^{47}$   | 259      |
| 952:577a | $0, 0, 0, 0, e^{12}, e^{13}, e^{34}, e^{15} + e^{23}, e^{47} + e^{16} + e^{25}$   | 259      |
| 952:577b | $0, 0, 0, 0, e^{12}, -e^{13}, e^{34}, e^{15} + e^{23}, e^{16} + e^{25} + e^{47}$  | 259      |
| 952:578  | $0, 0, 0, 0, e^{12}, -e^{13}, e^{34}, e^{15} + e^{23}, e^{17} + e^{25} + e^{46}$  | 259      |
| 952:579a | $0, 0, 0, 0, e^{12}, e^{13}, e^{34}, e^{23} + e^{15}, e^{47} + e^{25} + e^{36}$   | 259      |
| 952:579b | $0, 0, 0, 0, -e^{12}, e^{13}, e^{34}, e^{23} + e^{15}, e^{47} + e^{36} + e^{25}$  | 259      |
| 952:580  | $0, 0, 0, 0, e^{12}, e^{13}, e^{34}, e^{15} + e^{23}, e^{47} + e^{26} + e^{35}$   | 259      |
| 952:581a | $0, 0, 0, 0, e^{12}, e^{13}, e^{14}, e^{34} + e^{15}, e^{17} + e^{36} + e^{25}$   | 259      |
| 952:581b | $0, 0, 0, 0, -e^{12}, e^{13}, e^{14}, e^{15} + e^{34}, e^{17} + e^{25} + e^{36}$  | 259      |
| 952:582  | $0, 0, 0, 0, e^{12}, e^{13}, e^{14}, e^{15} + e^{34}, e^{17} + e^{26} + e^{35}$   | 259      |
| 952:583  | $0, 0, 0, 0, e^{12}, e^{13}, e^{14}, e^{34} + e^{25}, e^{35} + e^{26} + e^{17}$   | 259      |
| 952:584  | $0, 0, 0, 0, e^{12}, e^{13}, e^{24}, e^{25} + e^{34}, e^{36} + e^{27} + e^{15}$   | 259      |
| 952:585  | $0, 0, 0, 0, e^{12}, e^{13}, e^{34}, e^{15} + e^{24}, e^{37} + e^{25} + e^{16}$   | 259      |
| 952:586a | $0, 0, 0, 0, e^{12}, e^{13}, e^{14}, e^{15} + e^{34}, e^{36} + e^{47} + e^{25}$   | 259      |
| 952:586b | $0, 0, 0, 0, e^{12}, -e^{13}, e^{14}, e^{15} + e^{34}, e^{25} + e^{47} + e^{36}$  | 259      |
| 952:586c | $0, 0, 0, 0, -e^{12}, e^{13}, e^{14}, e^{15} + e^{34}, e^{47} + e^{36} + e^{25}$  | 259      |
| 952:587  | $0, 0, 0, 0, e^{12}, e^{13}, e^{14}, e^{15} + e^{34}, e^{26} + e^{35} + e^{47}$   | 259      |
| 952:588  | $0, 0, 0, 0, e^{12}, e^{13}, e^{14}, e^{15} + e^{34}, e^{37} + e^{46} + e^{25}$   | 259      |
| 952:589a | $0, 0, 0, 0, e^{12}, e^{13}, e^{14}, e^{25} + e^{34}, e^{15} + e^{47} + e^{36}$   | 259      |
| 952:589b | $0, 0, 0, 0, e^{12}, -e^{13}, e^{14}, e^{34} + e^{25}, e^{36} + e^{47} + e^{15}$  | 259      |
| 952:590  | $0, 0, 0, 0, e^{12}, e^{13}, e^{14}, e^{25} + e^{34}, e^{15} + e^{37} + e^{46}$   | 259      |
| 952:591  | $0, 0, 0, 0, e^{12}, e^{13}, e^{14}, e^{25} + e^{34}, e^{26} + e^{35} + e^{47}$   | 259      |
| 952:592  | $0, 0, 0, 0, -e^{12}, e^{13}, e^{24}, e^{34} + e^{15}, e^{36} + e^{17} + e^{45}$  | 259      |
| 952:593a | $0, 0, 0, 0, e^{12}, e^{13}, e^{24}, e^{34} + e^{15}, e^{47} + e^{36} + e^{25}$   | 259      |
| 952:593b | $0, 0, 0, 0, -e^{12}, e^{13}, e^{24}, e^{15} + e^{34}, e^{36} + e^{47} + e^{25}$  | 259      |
| 952:594  | $0, 0, 0, 0, e^{12}, e^{13}, e^{24}, e^{15} + e^{34}, e^{26} + e^{35} + e^{47}$   | 259      |
| 952:595a | $0, 0, 0, 0, e^{12}, e^{13}, e^{34}, e^{15} + e^{24}, e^{47} + e^{25} + e^{16}$   | 259      |
| 952:595b | $0, 0, 0, 0, e^{12}, -e^{13}, e^{34}, e^{24} + e^{15}, e^{47} + e^{25} + e^{16}$  | 259      |
| 952:596  | $0, 0, 0, 0, e^{12}, -e^{13}, e^{34}, e^{24} + e^{15}, e^{46} + e^{25} + e^{17}$  | 259      |

Table 2 – Continued to next page

Table 2 – Continued from previous page

| Name     | $\mathfrak{g}$                                                                    | UCS Dim. |
|----------|-----------------------------------------------------------------------------------|----------|
| 952:597  | $0, 0, 0, 0, e^{12}, e^{13}, e^{34}, e^{25} + e^{14}, e^{15} + e^{47} + e^{36}$   | 259      |
| 952:598  | $0, 0, 0, 0, e^{12}, e^{13}, e^{34}, e^{25} + e^{14}, e^{26} + e^{47} + e^{35}$   | 259      |
| 952:599a | $0, 0, 0, 0, e^{12}, e^{13}, e^{34}, e^{15} + e^{24}, e^{47} + e^{36} + e^{25}$   | 259      |
| 952:599b | $0, 0, 0, 0, -e^{12}, e^{13}, e^{34}, e^{15} + e^{24}, e^{36} + e^{47} + e^{25}$  | 259      |
| 952:600  | $0, 0, 0, 0, e^{12}, e^{13}, e^{34}, e^{15} + e^{24}, e^{35} + e^{47} + e^{26}$   | 259      |
| 952:601  | $0, 0, 0, 0, e^{12}, e^{13}, e^{14}, e^{25} + e^{16}, e^{15} + e^{23} + e^{47}$   | 259      |
| 952:602a | $0, 0, 0, 0, e^{12}, e^{13}, e^{24}, e^{25} + e^{16}, e^{47} + e^{15} + e^{23}$   | 259      |
| 952:602b | $0, 0, 0, 0, -e^{12}, e^{13}, e^{24}, e^{16} + e^{25}, e^{15} + e^{47} + e^{23}$  | 259      |
| 952:603  | $0, 0, 0, 0, e^{12}, e^{13}, e^{24}, e^{16} + e^{25}, e^{15} + e^{27} + e^{34}$   | 259      |
| 952:604  | $0, 0, 0, 0, -e^{12}, e^{13}, e^{24}, e^{25} + e^{16}, e^{17} + e^{23} + e^{45}$  | 259      |
| 952:605  | $0, 0, 0, 0, e^{12}, e^{13}, e^{14}, e^{15} + e^{36}, e^{17} + e^{34} + e^{25}$   | 259      |
| 952:606a | $0, 0, 0, 0, e^{12}, e^{13}, e^{14}, e^{36} + e^{25}, e^{23} + e^{47} + e^{15}$   | 259      |
| 952:606b | $0, 0, 0, 0, -e^{12}, e^{13}, e^{14}, e^{36} + e^{25}, e^{47} + e^{15} + e^{23}$  | 259      |
| 952:607  | $0, 0, 0, 0, e^{12}, e^{13}, e^{14}, e^{26} + e^{35}, e^{15} + e^{23} + e^{47}$   | 259      |
| 952:608  | $0, 0, 0, 0, e^{12}, e^{13}, e^{14}, e^{26} + e^{35}, e^{17} + e^{25} + e^{34}$   | 259      |
| 952:609  | $0, 0, 0, 0, -e^{12}, e^{13}, e^{24}, e^{15} + e^{36}, e^{17} + e^{23} + e^{45}$  | 259      |
| 952:610a | $0, 0, 0, 0, e^{12}, e^{13}, e^{24}, e^{36} + e^{25}, e^{23} + e^{47} + e^{15}$   | 259      |
| 952:610b | $0, 0, 0, 0, e^{12}, -e^{13}, e^{24}, e^{36} + e^{25}, e^{15} + e^{23} + e^{47}$  | 259      |
| 952:610c | $0, 0, 0, 0, -e^{12}, e^{13}, e^{24}, e^{36} + e^{25}, e^{47} + e^{15} + e^{23}$  | 259      |
| 952:610d | $0, 0, 0, 0, -e^{12}, -e^{13}, e^{24}, e^{36} + e^{25}, e^{15} + e^{47} + e^{23}$ | 259      |
| 952:611a | $0, 0, 0, 0, e^{12}, e^{13}, e^{24}, e^{25} + e^{36}, e^{15} + e^{27} + e^{34}$   | 259      |
| 952:611b | $0, 0, 0, 0, -e^{12}, e^{13}, e^{24}, e^{36} + e^{25}, e^{15} + e^{34} + e^{27}$  | 259      |
| 952:612a | $0, 0, 0, 0, -e^{12}, e^{13}, e^{24}, e^{25} + e^{36}, e^{23} + e^{45} + e^{17}$  | 259      |
| 952:612b | $0, 0, 0, 0, -e^{12}, -e^{13}, e^{24}, e^{36} + e^{25}, e^{45} + e^{17} + e^{23}$ | 259      |
| 952:613a | $0, 0, 0, 0, e^{12}, e^{13}, e^{24}, e^{26} + e^{35}, e^{15} + e^{23} + e^{47}$   | 259      |
| 952:613b | $0, 0, 0, 0, -e^{12}, -e^{13}, e^{24}, e^{26} + e^{35}, e^{15} + e^{23} + e^{47}$ | 259      |
| 952:614  | $0, 0, 0, 0, e^{12}, e^{13}, e^{24}, e^{35} + e^{26}, e^{34} + e^{27} + e^{15}$   | 259      |
| 952:615  | $0, 0, 0, 0, -e^{12}, -e^{13}, e^{24}, e^{26} + e^{35}, e^{45} + e^{23} + e^{17}$ | 259      |
| 952:616  | $0, 0, 0, 0, e^{12}, e^{13}, e^{34}, e^{16} + e^{25}, e^{15} + e^{47} + e^{23}$   | 259      |
| 952:617  | $0, 0, 0, 0, e^{12}, e^{13}, e^{34}, e^{16} + e^{25}, e^{15} + e^{24} + e^{37}$   | 259      |
| 952:618  | $0, 0, 0, 0, e^{12}, e^{13}, e^{34}, e^{36} + e^{15}, e^{37} + e^{25} + e^{14}$   | 259      |
| 952:619a | $0, 0, 0, 0, e^{12}, e^{13}, e^{34}, e^{25} + e^{36}, e^{15} + e^{23} + e^{47}$   | 259      |
| 952:619b | $0, 0, 0, 0, -e^{12}, e^{13}, e^{34}, e^{36} + e^{25}, e^{23} + e^{47} + e^{15}$  | 259      |
| 952:620a | $0, 0, 0, 0, e^{12}, e^{13}, e^{34}, e^{36} + e^{25}, e^{24} + e^{37} + e^{15}$   | 259      |
| 952:620b | $0, 0, 0, 0, -e^{12}, e^{13}, e^{34}, e^{25} + e^{36}, e^{37} + e^{15} + e^{24}$  | 259      |
| 952:621  | $0, 0, 0, 0, e^{12}, e^{13}, e^{34}, e^{26} + e^{35}, e^{47} + e^{23} + e^{15}$   | 259      |
| 952:622  | $0, 0, 0, 0, e^{12}, e^{13}, e^{34}, e^{26} + e^{35}, e^{14} + e^{25} + e^{37}$   | 259      |
| 952:623  | $0, 0, 0, 0, e^{12}, e^{13}, e^{34}, e^{35} + e^{26}, e^{24} + e^{37} + e^{15}$   | 259      |
| 952:624a | $0, 0, 0, 0, e^{12}, e^{13}, e^{34}, e^{36} + e^{25} + e^{14}, e^{37} + e^{15}$   | 259      |
| 952:624b | $0, 0, 0, 0, -e^{12}, e^{13}, e^{34}, e^{36} + e^{25} + e^{14}, e^{37} + e^{15}$  | 259      |
| 952:625  | $0, 0, 0, 0, e^{12}, e^{13}, e^{34}, e^{14} + e^{26} + e^{35}, e^{15} + e^{37}$   | 259      |
| 952:626  | $0, 0, 0, 0, e^{12}, e^{13}, e^{34}, e^{15} + e^{24} + e^{36}, e^{25} + e^{37}$   | 259      |
| 952:627  | $0, 0, 0, 0, e^{12}, e^{13}, e^{34}, e^{35} + e^{14} + e^{26}, e^{37} + e^{25}$   | 259      |
| 952:628a | $0, 0, 0, 0, e^{12}, e^{13}, e^{34}, e^{36} + e^{14} + e^{25}, e^{47} + e^{15}$   | 259      |
| 952:628b | $0, 0, 0, 0, -e^{12}, e^{13}, e^{34}, e^{36} + e^{25} + e^{14}, e^{47} + e^{15}$  | 259      |
| 952:629  | $0, 0, 0, 0, e^{12}, e^{13}, e^{34}, e^{14} + e^{26} + e^{35}, e^{15} + e^{47}$   | 259      |
| 952:630  | $0, 0, 0, 0, e^{12}, e^{13}, e^{34}, e^{15} + e^{36} + e^{24}, e^{25} + e^{47}$   | 259      |
| 952:631  | $0, 0, 0, 0, e^{12}, e^{13}, e^{34}, e^{14} + e^{26} + e^{35}, e^{47} + e^{25}$   | 259      |
| 952:632  | $0, 0, 0, 0, e^{12}, e^{13}, e^{14}, e^{16} + e^{25}, e^{17} + e^{35} + e^{26}$   | 259      |
| 952:633  | $0, 0, 0, 0, e^{12}, e^{13}, e^{24}, e^{25} + e^{16}, e^{36} + e^{27} + e^{15}$   | 259      |
| 952:634a | $0, 0, 0, 0, e^{12}, e^{13}, e^{14}, e^{36} + e^{25}, e^{17} + e^{35} + e^{26}$   | 259      |
| 952:634b | $0, 0, 0, 0, e^{12}, e^{13}, e^{14}, -e^{25} + e^{36}, e^{17} + e^{26} + e^{35}$  | 259      |
| 952:635a | $0, 0, 0, 0, e^{12}, e^{13}, e^{14}, e^{26} + e^{35}, e^{17} + e^{25} + e^{36}$   | 259      |
| 952:635b | $0, 0, 0, 0, -e^{12}, e^{13}, e^{14}, -e^{26} + e^{35}, e^{36} + e^{25} + e^{17}$ | 259      |
| 952:636  | $0, 0, 0, 0, e^{12}, e^{13}, e^{24}, e^{26} + e^{35}, e^{15} + e^{27} + e^{36}$   | 259      |
| 952:637a | $0, 0, 0, 0, e^{12}, e^{13}, e^{14}, e^{16} + e^{25}, e^{15} + e^{47} + e^{36}$   | 259      |
| 952:637b | $0, 0, 0, 0, e^{12}, -e^{13}, e^{14}, e^{16} + e^{25}, e^{47} + e^{15} + e^{36}$  | 259      |
| 952:638  | $0, 0, 0, 0, e^{12}, e^{13}, e^{14}, e^{25} + e^{16}, e^{15} + e^{46} + e^{37}$   | 259      |

Table 2 – Continued to next page

Table 2 – Continued from previous page

| Name     | $\mathfrak{g}$                                                                                         | UCS Dim. |
|----------|--------------------------------------------------------------------------------------------------------|----------|
| 952:639  | $0, 0, 0, 0, e^{12}, e^{13}, e^{14}, e^{16} + e^{25}, e^{35} + e^{47} + e^{26}$                        | 259      |
| 952:640  | $0, 0, 0, 0, e^{12}, e^{13}, e^{14}, e^{25} + e^{16}, e^{27} + e^{45} + e^{36}$                        | 259      |
| 952:641a | $0, 0, 0, 0, e^{12}, e^{13}, e^{24}, e^{16} + e^{25}, e^{15} + e^{47} + e^{36}$                        | 259      |
| 952:641b | $0, 0, 0, 0, -e^{12}, e^{13}, e^{24}, e^{16} + e^{25}, e^{15} + e^{36} + e^{47}$                       | 259      |
| 952:642  | $0, 0, 0, 0, -e^{12}, e^{13}, e^{24}, e^{25} + e^{16}, e^{36} + e^{45} + e^{17}$                       | 259      |
| 952:643a | $0, 0, 0, 0, e^{12}, e^{13}, e^{24}, e^{16} + e^{25}, e^{35} + e^{47} + e^{26}$                        | 259      |
| 952:643b | $0, 0, 0, 0, -e^{12}, -e^{13}, e^{24}, e^{16} + e^{25}, e^{26} + e^{47} + e^{35}$                      | 259      |
| 952:644a | $0, 0, 0, 0, e^{12}, e^{13}, e^{14}, e^{25} + e^{36}, e^{27} + e^{16} + e^{45}$                        | 259      |
| 952:644b | $0, 0, 0, 0, e^{12}, -e^{13}, e^{14}, e^{36} + e^{25}, e^{45} + e^{27} + e^{16}$                       | 259      |
| 952:645a | $0, 0, 0, 0, e^{12}, e^{13}, e^{14}, e^{35} + e^{26}, e^{47} + e^{16} + e^{25}$                        | 259      |
| 952:645b | $0, 0, 0, 0, -e^{12}, -e^{13}, e^{14}, e^{26} + e^{35}, e^{47} + e^{16} + e^{25}$                      | 259      |
| 952:646  | $0, 0, 0, 0, e^{12}, e^{13}, e^{14}, e^{26} + e^{35}, e^{27} + e^{16} + e^{45}$                        | 259      |
| 952:647a | $0, 0, 0, 0, e^{12}, e^{13}, e^{24}, e^{36} + e^{15}, e^{47} + e^{16} + e^{25}$                        | 259      |
| 952:647b | $0, 0, 0, 0, e^{12}, -e^{13}, e^{24}, e^{36} + e^{15}, e^{47} + e^{25} + e^{16}$                       | 259      |
| 952:648  | $0, 0, 0, 0, e^{12}, e^{13}, e^{24}, e^{26} + e^{35}, e^{25} + e^{47} + e^{16}$                        | 259      |
| 952:649a | $0, 0, 0, 0, e^{12}, e^{13}, e^{14}, e^{25} + e^{36}, e^{26} + e^{35} + e^{47}$                        | 259      |
| 952:649b | $0, 0, 0, 0, e^{12}, e^{13}, e^{14}, -e^{25} + e^{36}, e^{26} + e^{35} + e^{47}$                       | 259      |
| 952:650a | $0, 0, 0, 0, e^{12}, e^{13}, e^{14}, e^{35} + e^{26}, e^{47} + e^{36} + e^{25}$                        | 259      |
| 952:650b | $0, 0, 0, 0, e^{12}, -e^{13}, e^{14}, -e^{26} + e^{35}, e^{36} + e^{47} + e^{25}$                      | 259      |
| 952:650c | $0, 0, 0, 0, -e^{12}, -e^{13}, e^{14}, e^{26} + e^{35}, e^{25} + e^{47} + e^{36}$                      | 259      |
| 952:651  | $0, 0, 0, 0, e^{12}, e^{13}, e^{14}, e^{35} + e^{26}, e^{46} + e^{37} + e^{25}$                        | 259      |
| 952:652  | $0, 0, 0, 0, e^{12}, e^{13}, e^{24}, e^{15} + e^{36}, e^{26} + e^{47} + e^{35}$                        | 259      |
| 952:653a | $0, 0, 0, 0, e^{12}, e^{13}, e^{24}, e^{26} + e^{35}, e^{15} + e^{47} + e^{36}$                        | 259      |
| 952:653b | $0, 0, 0, 0, -e^{12}, -e^{13}, e^{24}, e^{35} + e^{26}, e^{15} + e^{47} + e^{36}$                      | 259      |
| 952:654  | $0, 0, 0, 0, -e^{12}, -e^{13}, e^{24}, e^{26} + e^{35}, e^{36} + e^{45} + e^{17}$                      | 259      |
| 952:655a | $0, 0, 0, 0, e^{12}, e^{13}, e^{24}, e^{25} + e^{36}, e^{26} + e^{35} + e^{47}$                        | 259      |
| 952:655b | $0, 0, 0, 0, e^{12}, e^{13}, e^{24}, e^{36} - e^{25}, e^{35} + e^{47} + e^{26}$                        | 259      |
| 952:656a | $0, 0, 0, 0, e^{12}, e^{13}, e^{24}, e^{35} + e^{26}, e^{47} + e^{36} + e^{25}$                        | 259      |
| 952:656b | $0, 0, 0, 0, -e^{12}, e^{13}, e^{24}, -e^{26} + e^{35}, e^{36} + e^{47} + e^{25}$                      | 259      |
| 952:657  | $0, 0, 0, 0, e^{12}, e^{34}, -e^{13}, e^{15} + e^{36}, e^{16} + e^{25} + e^{47}$                       | 259      |
| 952:658a | $0, 0, 0, 0, e^{12}, e^{34}, e^{13}, e^{15} + e^{36}, e^{17} + e^{25} + e^{46}$                        | 259      |
| 952:658b | $0, 0, 0, 0, e^{12}, e^{34}, -e^{13}, e^{15} + e^{36}, e^{17} + e^{46} + e^{25}$                       | 259      |
| 952:659  | $0, 0, 0, 0, e^{12}, e^{34}, e^{13}, e^{36} + e^{25}, e^{37} + e^{46} + e^{15}$                        | 259      |
| 952:660  | $0, 0, 0, 0, e^{12}, e^{34}, e^{13}, e^{36} + e^{25}, e^{27} + e^{35} + e^{46}$                        | 259      |
| 952:661a | $0, 0, 0, 0, e^{12}, e^{14} + e^{23}, e^{13} + e^{24}, e^{15}, e^{27} + e^{34} + e^{16}$               | 259      |
| 952:661b | $0, 0, 0, 0, e^{12}, -e^{14} + e^{23}, e^{24} + e^{13}, e^{15}, e^{16} + e^{34} + e^{27}$              | 259      |
| 952:662a | $0, 0, 0, 0, e^{12}, e^{23} + e^{14}, e^{24} + e^{13}, e^{34} + e^{15}, e^{27} + e^{16}$               | 259      |
| 952:662b | $0, 0, 0, 0, e^{12}, -e^{14} + e^{23}, e^{24} + e^{13}, e^{34} + e^{15}, e^{27} + e^{16}$              | 259      |
| 952:663a | $0, 0, 0, 0, e^{12}, e^{23} + e^{14}, e^{24} + e^{13}, e^{34} + e^{15}, e^{36} + e^{47}$               | 259      |
| 952:663b | $0, 0, 0, 0, e^{12}, e^{14} - e^{23}, e^{24} + e^{13}, e^{15} + e^{34}, e^{36} + e^{47}$               | 259      |
| 952:664a | $0, 0, 0, 0, e^{12}, e^{13} + e^{24}, e^{14} + e^{23}, e^{15} + e^{34}, e^{47} + e^{36}$               | 259      |
| 952:664b | $0, 0, 0, 0, e^{12}, e^{24} - e^{13}, e^{14} + e^{23}, e^{34} + e^{15}, e^{36} + e^{47}$               | 259      |
| 952:665a | $0, 0, 0, 0, (-1 + a_2)e^{12}, e^{14} + e^{23}, a_2e^{13} + e^{24}, e^{15}, e^{27} + e^{35} + e^{16}$  | 259      |
| 952:665b | $0, 0, 0, 0, (-1 + a_2)e^{12}, -e^{14} + e^{23}, a_2e^{13} + e^{24}, e^{15}, e^{16} + e^{35} + e^{27}$ | 259      |
| 952:666a | $0, 0, 0, 0, e^{12}, e^{23} + e^{14}, e^{24} + e^{13}, e^{15}, e^{36} + e^{47} + e^{25}$               | 259      |
| 952:666b | $0, 0, 0, 0, e^{12}, e^{14} - e^{23}, e^{24} + e^{13}, e^{15}, e^{36} + e^{25} + e^{47}$               | 259      |
| 952:667a | $0, 0, 0, 0, e^{12}, e^{23} + e^{14}, e^{24} + e^{13}, e^{15}, e^{46} + e^{25} + e^{37}$               | 259      |
| 952:667b | $0, 0, 0, 0, e^{12}, -e^{14} + e^{23}, e^{24} + e^{13}, e^{15}, e^{25} + e^{37} + e^{46}$              | 259      |
| 952:667c | $0, 0, 0, 0, -e^{12}, e^{14} + e^{23}, e^{13} + e^{24}, e^{15}, e^{37} + e^{46} + e^{25}$              | 259      |
| 952:668a | $0, 0, 0, 0, -e^{12}, e^{14} + e^{23}, e^{13} + e^{24}, e^{35} + e^{16}, e^{45} + e^{17}$              | 259      |
| 952:668b | $0, 0, 0, 0, -e^{12}, -e^{14} + e^{23}, e^{24} + e^{13}, e^{35} + e^{16}, e^{45} + e^{17}$             | 259      |
| 952:669a | $0, 0, 0, 0, e^{14} + e^{23}, -e^{12}, e^{24} + e^{13}, e^{15} + e^{36}, e^{17} + e^{25}$              | 259      |
| 952:669b | $0, 0, 0, 0, e^{14} + e^{23}, -e^{12}, e^{24} - e^{13}, e^{36} + e^{15}, e^{25} + e^{17}$              | 259      |
| 952:670a | $0, 0, 0, 0, e^{14} - e^{23}, e^{12}, e^{24} + e^{13}, e^{15} + e^{36}, e^{47} + e^{35}$               | 259      |
| 952:670b | $0, 0, 0, 0, e^{14} + e^{23}, -e^{12}, e^{13} + e^{24}, e^{15} + e^{36}, e^{35} + e^{47}$              | 259      |
| 952:671a | $0, 0, 0, 0, e^{23} + e^{14}, -e^{12}, e^{24} + e^{13}, e^{15} + e^{36}, e^{37} + e^{45}$              | 259      |
| 952:671b | $0, 0, 0, 0, e^{23} - e^{14}, -e^{12}, e^{24} + e^{13}, e^{36} + e^{15}, e^{37} + e^{45}$              | 259      |
| 952:672  | $0, 0, 0, 0, e^{12}, e^{13}, e^{14} + e^{23}, e^{15} + e^{24}, e^{26} + e^{34} + e^{17}$               | 259      |

Table 2 – Continued to next page

Table 2 – Continued from previous page

| Name     | $\mathfrak{g}$                                                                                        | UCS Dim. |
|----------|-------------------------------------------------------------------------------------------------------|----------|
| 952:673  | $0, 0, 0, 0, e^{12}, e^{34}, e^{14} + e^{23}, e^{25} + e^{13}, e^{16} + e^{24} + e^{37}$              | 259      |
| 952:674  | $0, 0, 0, 0, (-1 + a_2)e^{12}, e^{13}a_2, e^{23} + e^{14}, e^{24} + e^{15}, e^{35} + e^{26} + e^{17}$ | 259      |
| 952:675  | $0, 0, 0, 0, (-1 + a_2)e^{12}, a_2e^{13}, e^{23} + e^{14}, e^{34} + e^{15}, e^{17} + e^{26} + e^{35}$ | 259      |
| 952:676  | $0, 0, 0, 0, e^{12}(-1 + a_2), e^{13}a_2, e^{23} + e^{14}, e^{34} + e^{25}, e^{35} + e^{26} + e^{17}$ | 259      |
| 952:677a | $0, 0, 0, 0, e^{12}, e^{13}, e^{14} + e^{23}, e^{15} + e^{24}, e^{27} + e^{45} + e^{16}$              | 259      |
| 952:677b | $0, 0, 0, 0, e^{12}, -e^{13}, e^{14} + e^{23}, e^{15} + e^{24}, e^{45} + e^{16} + e^{27}$             | 259      |
| 952:678  | $0, 0, 0, 0, e^{12}, e^{13}, e^{14} + e^{23}, e^{15} + e^{24}, e^{46} + e^{25} + e^{37}$              | 259      |
| 952:679  | $0, 0, 0, 0, e^{12}, e^{13}, e^{14} + e^{23}, e^{24} + e^{15}, e^{45} + e^{36} + e^{27}$              | 259      |
| 952:680a | $0, 0, 0, 0, e^{12}, e^{13}, e^{23} + e^{14}, e^{34} + e^{15}, e^{16} + e^{27} + e^{45}$              | 259      |
| 952:680b | $0, 0, 0, 0, e^{12}, -e^{13}, e^{14} + e^{23}, e^{15} + e^{34}, e^{45} + e^{16} + e^{27}$             | 259      |
| 952:681a | $0, 0, 0, 0, e^{12}, e^{13}, e^{23} + e^{14}, e^{34} + e^{25}, e^{27} + e^{45} + e^{16}$              | 259      |
| 952:681b | $0, 0, 0, 0, e^{12}, -e^{13}, e^{14} + e^{23}, e^{25} + e^{34}, e^{27} + e^{16} + e^{45}$             | 259      |
| 952:682  | $0, 0, 0, 0, e^{12}, e^{13}, e^{14} + e^{23}, e^{15} + e^{34}, e^{37} + e^{46} + e^{25}$              | 259      |
| 952:683  | $0, 0, 0, 0, e^{12}, e^{13}, e^{14} + e^{23}, e^{15} + e^{34}, e^{36} + e^{27} + e^{45}$              | 259      |
| 952:684a | $0, 0, 0, 0, e^{12}, e^{13}, e^{23} + e^{14}, e^{34} + e^{25}, e^{46} + e^{37} + e^{15}$              | 259      |
| 952:684b | $0, 0, 0, 0, -e^{12}, e^{13}, e^{14} + e^{23}, e^{25} + e^{34}, e^{46} + e^{37} + e^{15}$             | 259      |
| 952:685  | $0, 0, 0, 0, e^{12}, e^{13}, e^{23} + e^{14}, e^{34} + e^{25}, e^{27} + e^{36} + e^{45}$              | 259      |
| 952:686  | $0, 0, 0, 0, e^{12}, e^{34}, e^{14} - e^{23}, e^{13} + e^{25}, e^{47} + e^{26} + e^{15}$              | 259      |
| 952:687  | $0, 0, 0, 0, -e^{12}, e^{34}, e^{23} + e^{14}, e^{13} + e^{25}, e^{35} + e^{46} + e^{17}$             | 259      |
| 952:688  | $0, 0, 0, 0, -e^{12}, e^{34}, e^{13} + e^{24}, e^{15} + e^{23}, e^{17} + e^{45} + e^{36}$             | 259      |
| 952:689  | $0, 0, 0, 0, -e^{12}, e^{13}, e^{23} + e^{14}, e^{16} + e^{25}, e^{17} + e^{35} + e^{24}$             | 259      |
| 952:690  | $0, 0, 0, 0, -e^{12}, e^{13}, e^{14} + e^{23}, e^{15} + e^{36}, e^{17} + e^{24} + e^{35}$             | 259      |
| 952:691a | $0, 0, 0, 0, -e^{12}, e^{13}, e^{23} + e^{14}, e^{36} + e^{25}, e^{35} + e^{24} + e^{17}$             | 259      |
| 952:691b | $0, 0, 0, 0, -e^{12}, -e^{13}, e^{14} + e^{23}, e^{25} + e^{36}, e^{24} + e^{17} + e^{35}$            | 259      |
| 952:692  | $0, 0, 0, 0, -e^{12}, e^{13}, e^{23} + e^{14}, e^{15} + e^{36} + e^{24}, e^{17} + e^{35}$             | 259      |
| 952:693  | $0, 0, 0, 0, -e^{12}, e^{13}, e^{14} + e^{23}, e^{25} + e^{16} + e^{34}, e^{17} + e^{35}$             | 259      |
| 952:694  | $0, 0, 0, 0, e^{12}, e^{13}, e^{14} + e^{23}, e^{15} + e^{24} + e^{36}, e^{27} + e^{45}$              | 259      |
| 952:695  | $0, 0, 0, 0, e^{12}, e^{13}, e^{14} + e^{23}, e^{25} + e^{34} + e^{16}, e^{27} + e^{45}$              | 259      |
| 952:696  | $0, 0, 0, 0, e^{12}, e^{34}, e^{13} + e^{24}, e^{15} + e^{36}, e^{14} + e^{27} + e^{35}$              | 259      |
| 952:697  | $0, 0, 0, 0, -e^{12}, e^{34}, e^{13} + e^{24}, e^{15} + e^{36}, e^{17} + e^{23} + e^{45}$             | 259      |
| 952:698  | $0, 0, 0, 0, e^{12}, e^{34}, e^{23} + e^{14}, e^{36} + e^{15}, e^{27} + e^{45} + e^{13}$              | 259      |
| 952:699  | $0, 0, 0, 0, -e^{12}, e^{34}, e^{14} + e^{23}, e^{15} + e^{36}, e^{24} + e^{17} + e^{35}$             | 259      |
| 952:700  | $0, 0, 0, 0, -e^{12}, e^{23} + e^{14}, e^{34}, e^{16} + e^{35}, e^{25} + e^{47} + e^{13}$             | 259      |
| 952:701  | $0, 0, 0, 0, -e^{12}, e^{14} + e^{23}, e^{34}, e^{35} + e^{16}, e^{37} + e^{15} + e^{24}$             | 259      |
| 952:702  | $0, 0, 0, 0, e^{14} + e^{23}, e^{12}, e^{13}, e^{46} + e^{25}, e^{15} + e^{34} + e^{27}$              | 259      |
| 952:703  | $0, 0, 0, 0, e^{14} - e^{23}, e^{12}, e^{34}, e^{15} + e^{36}, e^{45} + e^{27} + e^{13}$              | 259      |
| 952:704  | $0, 0, 0, 0, e^{14} + e^{23}, -e^{12}, e^{34}, e^{36} + e^{15}, e^{24} + e^{35} + e^{17}$             | 259      |
| 952:705  | $0, 0, 0, 0, e^{12}a_1, e^{13}(1 + a_1), e^{23} + e^{14}, e^{16} + e^{25}, e^{17} + e^{26} + e^{35}$  | 259      |
| 952:706a | $0, 0, 0, 0, e^{12}(-1 + a_2), a_2e^{13}, e^{23} + e^{14}, e^{25} + e^{36}, e^{35} + e^{26} + e^{17}$ | 259      |
| 952:706b | $0, 0, 0, 0, e^{12}(-1 + a_2), a_2e^{13}, e^{14} + e^{23}, e^{36} - e^{25}, e^{17} + e^{35} + e^{26}$ | 259      |
| 952:707a | $0, 0, 0, 0, e^{12}, e^{13}, e^{14} + e^{23}, e^{16} + e^{25}, e^{15} + e^{37} + e^{46}$              | 259      |
| 952:707b | $0, 0, 0, 0, -e^{12}, e^{13}, e^{23} + e^{14}, e^{25} + e^{16}, e^{46} + e^{37} + e^{15}$             | 259      |
| 952:708  | $0, 0, 0, 0, a_2e^{12}, e^{13}, a_2e^{14} + e^{23}, e^{25} + e^{16}, e^{45} + e^{36} + e^{27}$        | 259      |
| 952:709a | $0, 0, 0, 0, e^{12}, e^{13}, e^{14} + e^{23}, e^{36} + e^{25}, e^{45} + e^{16} + e^{27}$              | 259      |
| 952:709b | $0, 0, 0, 0, e^{12}, -e^{13}, e^{14} + e^{23}, e^{25} + e^{36}, e^{16} + e^{27} + e^{45}$             | 259      |
| 952:709c | $0, 0, 0, 0, -e^{12}, e^{13}, -e^{14} + e^{23}, e^{36} + e^{25}, e^{27} + e^{45} + e^{16}$            | 259      |
| 952:709d | $0, 0, 0, 0, -e^{12}, -e^{13}, e^{23} - e^{14}, e^{25} + e^{36}, e^{27} + e^{16} + e^{45}$            | 259      |
| 952:710a | $0, 0, 0, 0, e^{12}, e^{13}, e^{14} + e^{23}, e^{26} + e^{35}, e^{45} + e^{16} + e^{27}$              | 259      |
| 952:710b | $0, 0, 0, 0, -e^{12}, -e^{13}, e^{23} - e^{14}, e^{26} + e^{35}, e^{27} + e^{16} + e^{45}$            | 259      |
| 952:711  | $0, 0, 0, 0, e^{12}, e^{13}, e^{14} + e^{23}, e^{26} + e^{35}, e^{46} + e^{25} + e^{37}$              | 259      |
| 952:712  | $0, 0, 0, 0, e^{12}, e^{34}, e^{14} + e^{23}, e^{36} + e^{15}, e^{25} + e^{37} + e^{16}$              | 259      |
| 952:713  | $0, 0, 0, 0, e^{12}, e^{34}, e^{24} - e^{13}, e^{15} + e^{36}, e^{16} + e^{25} + e^{47}$              | 259      |
| 952:714a | $0, 0, 0, 0, -e^{12}, e^{23} - e^{14}, e^{13}, e^{35} + e^{16}, e^{45} + e^{17} + e^{26}$             | 259      |
| 952:714b | $0, 0, 0, 0, -e^{12}, e^{23} - e^{14}, -e^{13}, e^{16} + e^{35}, e^{17} + e^{26} + e^{45}$            | 259      |
| 952:715a | $0, 0, 0, 0, e^{12}, e^{23} + e^{14}, e^{13}, e^{35} - e^{16}, e^{47} + e^{36} + e^{15}$              | 259      |
| 952:715b | $0, 0, 0, 0, -e^{12}, e^{14} + e^{23}, e^{13}, e^{35} + e^{16}, e^{36} + e^{15} + e^{47}$             | 259      |
| 952:716  | $0, 0, 0, 0, -e^{12}, e^{14} + e^{23}, e^{13}, e^{16} + e^{35}, e^{25} + e^{36} + e^{47}$             | 259      |
| 952:717  | $0, 0, 0, 0, -e^{12}, e^{23} - e^{14}, e^{13}, e^{16} + e^{35}, e^{26} + e^{37} + e^{45}$             | 259      |

Table 2 – Continued to next page

Table 2 – Continued from previous page

| Name     | $\mathfrak{g}$                                                                                          | UCS Dim. |
|----------|---------------------------------------------------------------------------------------------------------|----------|
| 952:718  | $0, 0, 0, 0, e^{12}a_2, e^{23} + e^{14}a_2, e^{13}(1 + a_2), e^{45} + e^{26}, e^{16} + e^{27} + e^{35}$ | 259      |
| 952:719a | $0, 0, 0, 0, e^{12}, e^{14} + e^{23}, e^{13}, e^{26} + e^{45}, e^{15} + e^{36} + e^{47}$                | 259      |
| 952:719b | $0, 0, 0, 0, -e^{12}, e^{23} - e^{14}, -e^{13}, e^{26} + e^{45}, e^{15} + e^{47} + e^{36}$              | 259      |
| 952:720  | $0, 0, 0, 0, e^{12}, e^{14} + e^{23}, e^{13}, e^{45} + e^{26}, e^{47} + e^{36} + e^{25}$                | 259      |
| 952:721  | $0, 0, 0, 0, -e^{12}, e^{14} + e^{23}, e^{34}, e^{35} + e^{16}, e^{17} + e^{36} + e^{25}$               | 259      |
| 952:722  | $0, 0, 0, 0, e^{12}, e^{14} - e^{23}, e^{34}, e^{16} + e^{35}, e^{15} + e^{46} + e^{27}$                | 259      |
| 952:723  | $0, 0, 0, 0, -e^{12}, e^{23} - e^{14}, e^{34}, e^{16} + e^{35}, e^{26} + e^{37} + e^{45}$               | 259      |
| 952:724  | $0, 0, 0, 0, e^{12}, e^{13}, e^{14}, e^{16} + e^{25} + e^{34}, e^{47} + e^{15} + e^{23}$                | 259      |
| 952:725a | $0, 0, 0, 0, e^{12}, e^{13}, e^{24}, e^{25} + e^{14} + e^{36}, e^{15} + e^{23} + e^{47}$                | 259      |
| 952:725b | $0, 0, 0, 0, e^{12}, -e^{13}, e^{24}, e^{14} + e^{25} + e^{36}, e^{15} + e^{23} + e^{47}$               | 259      |
| 952:725c | $0, 0, 0, 0, -e^{12}, -e^{13}, e^{24}, e^{36} + e^{14} + e^{25}, e^{23} + e^{47} + e^{15}$              | 259      |
| 952:726a | $0, 0, 0, 0, e^{12}, e^{13}, e^{24}, e^{26} + e^{35} + e^{14}, e^{15} + e^{23} + e^{47}$                | 259      |
| 952:726b | $0, 0, 0, 0, -e^{12}, -e^{13}, e^{24}, e^{26} + e^{35} + e^{14}, e^{15} + e^{47} + e^{23}$              | 259      |
| 952:727a | $0, 0, 0, 0, e^{12}, e^{13}, e^{24}, e^{16} + e^{25} + e^{34}, e^{15} + e^{23} + e^{47}$                | 259      |
| 952:727b | $0, 0, 0, 0, -e^{12}, e^{13}, e^{24}, e^{25} + e^{16} + e^{34}, e^{15} + e^{23} + e^{47}$               | 259      |
| 952:728a | $0, 0, 0, 0, e^{12}, e^{13}, e^{24}, e^{35} + e^{26} + e^{14}, e^{34} + e^{27} + e^{15}$                | 259      |
| 952:728b | $0, 0, 0, 0, e^{12}, e^{13}, e^{24}, e^{26} + e^{35} - e^{14}, e^{34} + e^{27} + e^{15}$                | 259      |
| 952:729  | $0, 0, 0, 0, -e^{12}, -e^{13}, e^{24}, e^{14} + e^{26} + e^{35}, e^{17} + e^{23} + e^{45}$              | 259      |
| 952:730a | $0, 0, 0, 0, e^{12}, e^{13}, e^{34}, e^{36} + e^{25} + e^{14}, e^{47} + e^{15} + e^{23}$                | 259      |
| 952:730b | $0, 0, 0, 0, -e^{12}, e^{13}, e^{34}, e^{14} + e^{25} + e^{36}, e^{15} + e^{23} + e^{47}$               | 259      |
| 952:731  | $0, 0, 0, 0, e^{12}, e^{13}, e^{34}, e^{35} + e^{14} + e^{26}, e^{23} + e^{47} + e^{15}$                | 259      |
| 952:732a | $0, 0, 0, 0, e^{12}, e^{13}, e^{34}, e^{36} + e^{15} + e^{24}, e^{37} + e^{25} + e^{14}$                | 259      |
| 952:732b | $0, 0, 0, 0, e^{12}, e^{13}, e^{34}, -e^{15} + e^{36} + e^{24}, e^{14} + e^{37} + e^{25}$               | 259      |
| 952:733a | $0, 0, 0, 0, e^{12}, e^{13}, e^{34}, e^{25} + e^{36} + e^{14}, e^{15} + e^{37} + e^{24}$                | 259      |
| 952:733b | $0, 0, 0, 0, e^{12}, e^{13}, e^{34}, -e^{14} + e^{36} + e^{25}, e^{15} + e^{24} + e^{37}$               | 259      |
| 952:733c | $0, 0, 0, 0, -e^{12}, e^{13}, e^{34}, e^{36} + e^{25} + e^{14}, e^{37} + e^{15} + e^{24}$               | 259      |
| 952:733d | $0, 0, 0, 0, -e^{12}, e^{13}, e^{34}, -e^{14} + e^{25} + e^{36}, e^{15} + e^{24} + e^{37}$              | 259      |
| 952:734  | $0, 0, 0, 0, e^{12}, e^{13}, e^{34}, e^{35} + e^{14} + e^{26}, e^{24} + e^{37} + e^{15}$                | 259      |
| 952:735  | $0, 0, 0, 0, e^{12}, e^{13}, e^{14}, e^{15} + e^{24} + e^{36}, e^{26} + e^{17} + e^{35}$                | 259      |
| 952:736  | $0, 0, 0, 0, e^{12}, e^{13}, e^{24}, e^{26} + e^{35} + e^{14}, e^{15} + e^{27} + e^{36}$                | 259      |
| 952:737  | $0, 0, 0, 0, e^{12}, e^{13}, e^{24}, e^{25} + e^{16} + e^{34}, e^{27} + e^{15} + e^{36}$                | 259      |
| 952:738a | $0, 0, 0, 0, e^{12}, e^{13}, e^{14}, e^{24} + e^{36} + e^{15}, e^{47} + e^{25} + e^{16}$                | 259      |
| 952:738b | $0, 0, 0, 0, -e^{12}, e^{13}, e^{14}, e^{24} + e^{36} + e^{15}, e^{47} + e^{16} + e^{25}$               | 259      |
| 952:739  | $0, 0, 0, 0, e^{12}, e^{13}, e^{14}, e^{24} + e^{36} + e^{15}, e^{27} + e^{16} + e^{45}$                | 259      |
| 952:740  | $0, 0, 0, 0, e^{12}, e^{13}, e^{24}, e^{14} + e^{26} + e^{35}, e^{47} + e^{16} + e^{25}$                | 259      |
| 952:741  | $0, 0, 0, 0, e^{12}, e^{13}, e^{14}, e^{15} + e^{24} + e^{36}, e^{26} + e^{35} + e^{47}$                | 259      |
| 952:742  | $0, 0, 0, 0, e^{12}, e^{13}, e^{14}, e^{24} + e^{36} + e^{15}, e^{46} + e^{25} + e^{37}$                | 259      |
| 952:743a | $0, 0, 0, 0, e^{12}, e^{13}, e^{24}, e^{26} + e^{35} + e^{14}, e^{47} + e^{36} + e^{15}$                | 259      |
| 952:743b | $0, 0, 0, 0, -e^{12}, -e^{13}, e^{24}, e^{26} + e^{35} + e^{14}, e^{15} + e^{47} + e^{36}$              | 259      |
| 952:744a | $0, 0, 0, 0, e^{12}, e^{13}, e^{24}, e^{16} + e^{25} + e^{34}, e^{47} + e^{15} + e^{36}$                | 259      |
| 952:744b | $0, 0, 0, 0, -e^{12}, e^{13}, e^{24}, e^{34} + e^{25} + e^{16}, e^{36} + e^{47} + e^{15}$               | 259      |
| 952:745  | $0, 0, 0, 0, -e^{12}, -e^{13}, e^{24}, e^{35} + e^{14} + e^{26}, e^{17} + e^{45} + e^{36}$              | 259      |
| 952:746  | $0, 0, 0, 0, -e^{12}, e^{13}, e^{24}, e^{16} + e^{25} + e^{34}, e^{17} + e^{36} + e^{45}$               | 259      |
| 952:747a | $0, 0, 0, 0, e^{12}, e^{13}, e^{24}, e^{14} + e^{26} + e^{35}, e^{47} + e^{36} + e^{25}$                | 259      |
| 952:747b | $0, 0, 0, 0, -e^{12}, e^{13}, e^{24}, e^{35} + e^{14} - e^{26}, e^{47} + e^{36} + e^{25}$               | 259      |
| 952:748a | $0, 0, 0, 0, e^{12}, e^{13}, e^{24}, e^{36} + e^{25} + e^{14}, e^{47} + e^{26} + e^{35}$                | 259      |
| 952:748b | $0, 0, 0, 0, e^{12}, e^{13}, e^{24}, e^{36} - e^{25} + e^{14}, e^{26} + e^{47} + e^{35}$                | 259      |
| 952:749a | $0, 0, 0, 0, e^{12}, e^{13}, e^{24}, e^{16} + e^{25} + e^{34}, e^{26} + e^{35} + e^{47}$                | 259      |
| 952:749b | $0, 0, 0, 0, -e^{12}, -e^{13}, e^{24}, e^{16} + e^{25} + e^{34}, e^{35} + e^{47} + e^{26}$              | 259      |
| 952:750  | $0, 0, 0, 0, e^{12}, e^{34}, e^{13}, e^{15} + e^{23} + e^{46}, e^{36} + e^{25} + e^{17}$                | 259      |
| 952:751  | $0, 0, 0, 0, e^{12}, e^{34}, -e^{13}, e^{15} + e^{46} + e^{23}, e^{47} + e^{16} + e^{25}$               | 259      |
| 952:752  | $0, 0, 0, 0, e^{12}, e^{34}, -e^{13}, e^{15} + e^{24} + e^{36}, e^{16} + e^{25} + e^{47}$               | 259      |
| 952:753a | $0, 0, 0, 0, e^{12}, e^{34}, e^{13}, e^{15} + e^{24} + e^{36}, e^{17} + e^{25} + e^{46}$                | 259      |
| 952:753b | $0, 0, 0, 0, e^{12}, e^{34}, -e^{13}, e^{24} + e^{36} + e^{15}, e^{46} + e^{25} + e^{17}$               | 259      |
| 952:754a | $0, 0, 0, 0, e^{12}, e^{13}, e^{14}, e^{35} + e^{17} + e^{26}, e^{47} + e^{16} + e^{25}$                | 259      |
| 952:754b | $0, 0, 0, 0, -e^{12}, -e^{13}, e^{14}, e^{17} + e^{26} + e^{35}, e^{16} + e^{47} + e^{25}$              | 259      |
| 952:755a | $0, 0, 0, 0, e^{12}, e^{13}, e^{14}, e^{17} + e^{26} + e^{35}, e^{27} + e^{16} + e^{45}$                | 259      |
| 952:755b | $0, 0, 0, 0, e^{12}, e^{13}, e^{14}, e^{35} + e^{26} - e^{17}, e^{27} + e^{45} + e^{16}$                | 259      |

Table 2 – Continued to next page

Table 2 – Continued from previous page

| Name     | $\mathfrak{g}$                                                                                                             | UCS Dim. |
|----------|----------------------------------------------------------------------------------------------------------------------------|----------|
| 952:756  | $0, 0, 0, 0, e^{12}, a_1 e^{13}, e^{24}, e^{27} + e^{36} + e^{15}, e^{47} + e^{25} + e^{16}$                               | 259      |
| 952:757a | $0, 0, 0, 0, e^{12}, e^{13}, e^{14}, e^{17} + e^{26} + e^{35}, e^{25} + e^{47} + e^{36}$                                   | 259      |
| 952:757b | $0, 0, 0, 0, e^{12}, -e^{13}, e^{14}, e^{17} + e^{35} - e^{26}, e^{47} + e^{25} + e^{36}$                                  | 259      |
| 952:757c | $0, 0, 0, 0, -e^{12}, -e^{13}, e^{14}, e^{35} + e^{17} + e^{26}, e^{47} + e^{36} + e^{25}$                                 | 259      |
| 952:758a | $0, 0, 0, 0, e^{12}, e^{13}, e^{14}, e^{25} + e^{17} + e^{36}, e^{26} + e^{47} + e^{35}$                                   | 259      |
| 952:758b | $0, 0, 0, 0, e^{12}, e^{13}, e^{14}, e^{17} - e^{25} + e^{36}, e^{26} + e^{35} + e^{47}$                                   | 259      |
| 952:759  | $0, 0, 0, 0, e^{12}, e^{13}, e^{14}, e^{17} + e^{26} + e^{35}, e^{25} + e^{46} + e^{37}$                                   | 259      |
| 952:760  | $0, 0, 0, 0, e^{12}, e^{13}, e^{24}, e^{27} + e^{36} + e^{15}, e^{47} + e^{35} + e^{26}$                                   | 259      |
| 952:761  | $0, 0, 0, 0, e^{12}, e^{13}, e^{14}, e^{25} + e^{37} + e^{46}, e^{26} + e^{35} + e^{47}$                                   | 259      |
| 952:762  | $0, 0, 0, 0, -e^{12}, -e^{13}, e^{24}, e^{45} + e^{36} + e^{17}, e^{47} + e^{26} + e^{35}$                                 | 259      |
| 952:763a | $0, 0, 0, 0, e^{23} + e^{14}, e^{24} + e^{13}, e^{34} - e^{12}, e^{16} + e^{25}, e^{37} + e^{15}$                          | 259      |
| 952:763b | $0, 0, 0, 0, e^{14} + e^{23}, -e^{13} + e^{24}, -e^{12} + e^{34}, e^{16} + e^{25}, e^{15} + e^{37}$                        | 259      |
| 952:763c | $0, 0, 0, 0, -e^{14} + e^{23}, e^{24} + e^{13}, e^{34} - e^{12}, -e^{16} + e^{25}, e^{15} + e^{37}$                        | 259      |
| 952:763d | $0, 0, 0, 0, -e^{14} + e^{23}, e^{24} - e^{13}, -e^{12} + e^{34}, e^{25} - e^{16}, e^{37} + e^{15}$                        | 259      |
| 952:764a | $0, 0, 0, 0, e^{14} + e^{23}, e^{13} + e^{24}, e^{12} + e^{34}, e^{25} + e^{16}, e^{17} + e^{35}$                          | 259      |
| 952:764b | $0, 0, 0, 0, e^{14} + e^{23}, e^{24} + e^{13}, e^{34} - e^{12}, e^{16} + e^{25}, e^{17} + e^{35}$                          | 259      |
| 952:764c | $0, 0, 0, 0, e^{14} + e^{23}, e^{24} - e^{13}, e^{12} + e^{34}, e^{25} + e^{16}, e^{35} + e^{17}$                          | 259      |
| 952:765a | $0, 0, 0, 0, (-1 + a_2)e^{12}, e^{23} + e^{14}, e^{24} + a_2 e^{13}, e^{15} + e^{34}, e^{27} + e^{16} + e^{35}$            | 259      |
| 952:765b | $0, 0, 0, 0, (-1 + a_2)e^{12}, e^{23} - e^{14}, e^{24} + a_2 e^{13}, e^{15} + e^{34}, e^{35} + e^{27} + e^{16}$            | 259      |
| 952:766a | $0, 0, 0, 0, e^{12}, e^{23} + e^{14}, e^{24} + e^{13}, e^{15} + e^{34}, e^{25} + e^{47} + e^{36}$                          | 259      |
| 952:766b | $0, 0, 0, 0, e^{12}, e^{14} - e^{23}, e^{13} + e^{24}, e^{34} + e^{15}, e^{36} + e^{47} + e^{25}$                          | 259      |
| 952:767a | $0, 0, 0, 0, e^{12}, e^{23} + e^{14}, e^{24} + e^{13}, e^{15} + e^{34}, e^{37} + e^{46} + e^{25}$                          | 259      |
| 952:767b | $0, 0, 0, 0, e^{12}, -e^{14} + e^{23}, e^{13} + e^{24}, e^{34} + e^{15}, e^{37} + e^{46} + e^{25}$                         | 259      |
| 952:767c | $0, 0, 0, 0, -e^{12}, e^{23} + e^{14}, e^{24} + e^{13}, e^{15} + e^{34}, e^{25} + e^{37} + e^{46}$                         | 259      |
| 952:768a | $0, 0, 0, 0, e^{23} + e^{14}, -e^{12}, e^{24} + e^{13}, e^{36} + e^{15}, e^{17} + e^{25} + e^{34}$                         | 259      |
| 952:768b | $0, 0, 0, 0, e^{23} + e^{14}, -e^{12}, e^{24} - e^{13}, e^{15} + e^{36}, e^{17} + e^{25} + e^{34}$                         | 259      |
| 952:769a | $0, 0, 0, 0, (-1 + a_2)e^{12}, e^{14} a_2 + e^{23}, e^{24} + e^{13}, -(-1 + a_2)e^{16} + e^{35}, e^{26} + e^{45} + e^{17}$ | 259      |
| 952:769b | $0, 0, 0, 0, (-1 + a_2)e^{12}, e^{14} a_2 + e^{23}, e^{24} - e^{13}, -(-1 + a_2)e^{16} + e^{35}, e^{26} + e^{45} + e^{17}$ | 259      |
| 952:770a | $0, 0, 0, 0, e^{12}, -e^{23} + e^{14}, e^{24} + e^{13}, e^{35} + e^{16}, e^{47} + e^{36} + e^{15}$                         | 259      |
| 952:770b | $0, 0, 0, 0, e^{12}, e^{14} + e^{23}, e^{13} + e^{24}, e^{35} - e^{16}, e^{47} + e^{36} + e^{15}$                          | 259      |
| 952:770c | $0, 0, 0, 0, -e^{12}, e^{14} + e^{23}, e^{13} + e^{24}, e^{16} + e^{35}, e^{15} + e^{36} + e^{47}$                         | 259      |
| 952:770d | $0, 0, 0, 0, -e^{12}, -e^{23} + e^{14}, e^{24} + e^{13}, -e^{16} + e^{35}, e^{15} + e^{47} + e^{36}$                       | 259      |
| 952:771a | $0, 0, 0, 0, -e^{12}, e^{14} + e^{23}, e^{13} + e^{24}, e^{16} + e^{35}, e^{15} + e^{46} + e^{37}$                         | 259      |
| 952:771b | $0, 0, 0, 0, -e^{12}, -e^{14} + e^{23}, e^{13} + e^{24}, e^{35} + e^{16}, e^{15} + e^{37} + e^{46}$                        | 259      |
| 952:772a | $0, 0, 0, 0, e^{12}, -e^{23} + e^{14}, e^{24} + e^{13}, e^{35} + e^{16}, e^{47} + e^{36} + e^{25}$                         | 259      |
| 952:772b | $0, 0, 0, 0, -e^{12}, e^{14} + e^{23}, e^{13} + e^{24}, e^{16} + e^{35}, e^{25} + e^{47} + e^{36}$                         | 259      |
| 952:773a | $0, 0, 0, 0, -e^{12}, e^{23} + e^{14}, e^{24} + e^{13}, e^{35} + e^{16}, e^{46} + e^{25} + e^{37}$                         | 259      |
| 952:773b | $0, 0, 0, 0, -e^{12}, e^{14} + e^{23}, -e^{13} + e^{24}, e^{35} + e^{16}, e^{37} + e^{46} + e^{25}$                        | 259      |
| 952:773c | $0, 0, 0, 0, -e^{12}, -e^{14} + e^{23}, e^{13} + e^{24}, e^{16} + e^{35}, e^{46} + e^{25} + e^{37}$                        | 259      |
| 952:773d | $0, 0, 0, 0, -e^{12}, e^{23} - e^{14}, e^{24} - e^{13}, e^{16} + e^{35}, e^{37} + e^{46} + e^{25}$                         | 259      |
| 952:774a | $0, 0, 0, 0, e^{24} + e^{13}(1 + a_2), e^{14} + e^{23}, a_2 e^{12}, e^{26} + e^{15}, e^{25} + e^{16} + e^{37}$             | 259      |
| 952:774b | $0, 0, 0, 0, e^{24} + e^{13}(1 + a_2), e^{23} - e^{14}, a_2 e^{12}, e^{26} - e^{15}, e^{25} + e^{37} + e^{16}$             | 259      |
| 952:775a | $0, 0, 0, 0, e^{14} + e^{23}, e^{13} + e^{24}, e^{12}, e^{26} + e^{15}, e^{17} + e^{46} + e^{35}$                          | 259      |
| 952:775b | $0, 0, 0, 0, e^{14} + e^{23}, e^{13} + e^{24}, -e^{12}, e^{26} + e^{15}, e^{46} + e^{35} + e^{17}$                         | 259      |
| 952:775c | $0, 0, 0, 0, -e^{14} - e^{23}, e^{24} - e^{13}, e^{12}, e^{15} + e^{26}, e^{46} + e^{17} + e^{35}$                         | 259      |
| 952:775d | $0, 0, 0, 0, -e^{14} - e^{23}, e^{24} - e^{13}, -e^{12}, e^{26} + e^{15}, e^{46} + e^{35} + e^{17}$                        | 259      |
| 952:776a | $0, 0, 0, 0, e^{14} + e^{23}, e^{13} + e^{24}, e^{12}, e^{26} + e^{15}, e^{17} + e^{45} + e^{36}$                          | 259      |
| 952:776b | $0, 0, 0, 0, -e^{14} + e^{23}, e^{13} + e^{24}, e^{12}, e^{26} + e^{15}, e^{17} + e^{45} + e^{36}$                         | 259      |
| 952:777a | $0, 0, 0, 0, e^{14} + a_3 e^{23}, e^{13} + e^{24}, -(-1 + a_3)e^{12}, e^{46} + e^{35}, e^{37} + e^{26} + e^{15}$           | 259      |
| 952:777b | $0, 0, 0, 0, -e^{14} + a_3 e^{23}, e^{24} - e^{13}, -(1 + a_3)e^{12}, e^{35} + e^{46}, e^{15} + e^{37} + e^{26}$           | 259      |
| 952:778a | $0, 0, 0, 0, e^{14} + e^{23}, e^{13} + e^{24}, e^{12}, e^{46} + e^{35}, e^{17} + e^{45} + e^{36}$                          | 259      |
| 952:778b | $0, 0, 0, 0, e^{23} - e^{14}, e^{24} + e^{13}, e^{12}, -e^{35} + e^{46}, e^{36} + e^{45} + e^{17}$                         | 259      |
| 952:779a | $0, 0, 0, 0, e^{13} + e^{24}, e^{14} + e^{23}, e^{12}, e^{46} + e^{35}, e^{17} + e^{45} + e^{36}$                          | 259      |
| 952:779b | $0, 0, 0, 0, -e^{24} + e^{13}, e^{23} + e^{14}, e^{12}, -e^{35} + e^{46}, e^{36} + e^{45} + e^{17}$                        | 259      |
| 952:779c | $0, 0, 0, 0, e^{13} + e^{24}, e^{14} + e^{23}, -e^{12}, e^{46} + e^{35}, e^{17} + e^{45} + e^{36}$                         | 259      |
| 952:780a | $0, 0, 0, 0, -e^{12}, e^{13}, e^{23} + e^{14}, e^{34} + e^{25} + e^{16}, e^{35} + e^{24} + e^{17}$                         | 259      |
| 952:780b | $0, 0, 0, 0, -e^{12}, e^{13}, e^{14} + e^{23}, -e^{25} + e^{34} + e^{16}, e^{24} + e^{35} + e^{17}$                        | 259      |
| 952:781  | $0, 0, 0, 0, e^{12}, e^{34}, e^{13} + e^{24}, e^{15} + e^{23} + e^{46}, e^{14} + e^{27} + e^{35}$                          | 259      |

Table 2 – Continued to next page

Table 2 – Continued from previous page

| Name     | $\mathfrak{g}$                                                                                                                                 | UCS Dim. |
|----------|------------------------------------------------------------------------------------------------------------------------------------------------|----------|
| 952:782  | $0, 0, 0, 0, e^{24} + e^{13}, -e^{12}, e^{34}, e^{46} + e^{15} + e^{23}, e^{14} + e^{27} + e^{35}$                                             | 259      |
| 952:783  | $0, 0, 0, 0, e^{12}a_1, e^{13}(1 + a_1), e^{23} + e^{14}, e^{24} + e^{36} + e^{15}, e^{35} + e^{26} + e^{17}$                                  | 259      |
| 952:784a | $0, 0, 0, 0, e^{12}, e^{13}, e^{14} + e^{23}, e^{15} + e^{36} + e^{24}, e^{27} + e^{45} + e^{16}$                                              | 259      |
| 952:784b | $0, 0, 0, 0, e^{12}, -e^{13}, e^{14} + e^{23}, e^{15} + e^{24} + e^{36}, e^{45} + e^{16} + e^{27}$                                             | 259      |
| 952:785  | $0, 0, 0, 0, e^{12}, a_2e^{13}, a_2e^{14} + e^{23}, e^{15} + e^{24} + e^{36}, e^{46} + e^{25} + e^{37}$                                        | 259      |
| 952:786  | $0, 0, 0, 0, e^{12}, e^{34}, e^{24} + e^{13}, e^{36} + e^{25} + e^{14}, e^{26} + e^{37} + e^{15}$                                              | 259      |
| 952:787a | $0, 0, 0, 0, -e^{12}, e^{23} - e^{14}, e^{13}, e^{35} + e^{24} + e^{16}, e^{45} + e^{17} + e^{26}$                                             | 259      |
| 952:787b | $0, 0, 0, 0, -e^{12}, e^{23} - e^{14}, -e^{13}, e^{16} + e^{35} + e^{24}, e^{17} + e^{26} + e^{45}$                                            | 259      |
| 952:788a | $0, 0, 0, 0, e^{12}, e^{23} + e^{14}, e^{13}, e^{35} + e^{24} - e^{16}, e^{47} + e^{36} + e^{15}$                                              | 259      |
| 952:788b | $0, 0, 0, 0, -e^{12}, e^{14} + e^{23}, e^{13}, e^{24} + e^{35} + e^{16}, e^{47} + e^{36} + e^{15}$                                             | 259      |
| 952:789  | $0, 0, 0, 0, -e^{12}, e^{14} + e^{23}, e^{13}, e^{35} + e^{16} + e^{24}, e^{36} + e^{47} + e^{25}$                                             | 259      |
| 952:790  | $0, 0, 0, 0, -e^{12}, e^{23} - e^{14}, e^{13}, e^{16} + e^{35} + e^{24}, e^{26} + e^{37} + e^{45}$                                             | 259      |
| 952:791  | $0, 0, 0, 0, e^{12}, e^{24} + e^{13}, e^{34}, e^{14} + e^{26} + e^{35}, e^{15} + e^{36} + e^{27}$                                              | 259      |
| 952:792  | $0, 0, 0, 0, -e^{12}, e^{13} + e^{24}, e^{34}, e^{23} + e^{16} + e^{45}, e^{15} + e^{27} + e^{36}$                                             | 259      |
| 952:793  | $0, 0, 0, 0, -e^{12}, e^{24} - e^{13}, e^{34}, e^{35} + e^{14} + e^{26}, e^{37} + e^{45} + e^{16}$                                             | 259      |
| 952:794a | $0, 0, 0, 0, e^{12}, e^{13}a_1, e^{14} + e^{23}, e^{26} + e^{35} + (-1 + a_1)e^{17}, e^{27} + e^{16} + e^{45}$                                 | 259      |
| 952:794b | $0, 0, 0, 0, -e^{12}, e^{13}a_1, e^{23} - e^{14}, e^{26} + e^{35} + (1 + a_1)e^{17}, e^{16} + e^{27} + e^{45}$                                 | 259      |
| 952:795  | $0, 0, 0, 0, (-1 + a_2)e^{12}, e^{13}a_2, e^{14}a_2 + e^{23}, e^{26} + e^{35} + e^{17}, e^{25} + e^{37} + e^{46}$                              | 259      |
| 952:796a | $0, 0, 0, 0, e^{12}, e^{13}, e^{14} + e^{23}, e^{45} + e^{27} + e^{16}, e^{46} + e^{37} + e^{15}$                                              | 259      |
| 952:796b | $0, 0, 0, 0, e^{12}, e^{13}, e^{23} + e^{14}, e^{27} - e^{16} + e^{45}, e^{15} + e^{37} + e^{46}$                                              | 259      |
| 952:796c | $0, 0, 0, 0, -e^{12}, -e^{13}, -e^{14} + e^{23}, e^{27} + e^{45} - e^{16}, e^{37} + e^{46} + e^{15}$                                           | 259      |
| 952:797a | $0, 0, 0, 0, e^{12}, e^{13}, e^{14} + e^{23}, e^{27} + e^{45} + e^{16}, e^{37} + e^{46} + e^{25}$                                              | 259      |
| 952:797b | $0, 0, 0, 0, -e^{12}, -e^{13}, -e^{14} + e^{23}, e^{16} + e^{45} + e^{27}, e^{25} + e^{37} + e^{46}$                                           | 259      |
| 952:798  | $0, 0, 0, 0, e^{12}, e^{13}, e^{23} + e^{14}, e^{27} + e^{36} + e^{45}, e^{37} + e^{46} + e^{25}$                                              | 259      |
| 952:799a | $0, 0, 0, 0, e^{12}, e^{34}, -e^{13} + e^{24}, e^{15} + e^{26} + e^{37}, e^{16} + e^{47} + e^{25}$                                             | 259      |
| 952:799b | $0, 0, 0, 0, e^{12}, e^{34}, -e^{13} + e^{24}, e^{37} + e^{26} - e^{15}, e^{47} + e^{25} + e^{16}$                                             | 259      |
| 952:800  | $0, 0, 0, 0, -e^{12}, e^{34}, e^{13}a_2 + e^{24}, e^{15} + e^{37} + e^{26}, e^{45} + e^{17} + e^{36}$                                          | 259      |
| 952:801a | $0, 0, 0, 0, e^{12}, e^{34}, -e^{23} + e^{14}, e^{16} + e^{25} + e^{37}, e^{17} + e^{35} + e^{46}$                                             | 259      |
| 952:801b | $0, 0, 0, 0, -e^{12}, e^{34}, e^{14} + e^{23}, e^{16} + e^{25} + e^{37}, e^{17} + e^{35} + e^{46}$                                             | 259      |
| 952:802a | $0, 0, 0, 0, e^{24} + e^{13}(1 + a_2), e^{23} + e^{14}, e^{34} + e^{12}a_2, e^{15} + e^{26}, e^{37} + e^{16} + e^{25}$                         | 259      |
| 952:802b | $0, 0, 0, 0, -e^{24} + e^{13}(1 + a_2), e^{14} + e^{23}, e^{34} + e^{12}a_2, e^{26} - e^{15}, e^{25} + e^{37} + e^{16}$                        | 259      |
| 952:802c | $0, 0, 0, 0, -e^{24} + e^{13}(1 + a_2), -e^{14} + e^{23}, e^{34} + e^{12}a_2, e^{26} + e^{15}, e^{37} + e^{25} + e^{16}$                       | 259      |
| 952:803a | $0, 0, 0, 0, e^{14}a_1 + (-1 + a_1)e^{23}, e^{24} + (-1 + a_1)e^{13}, e^{34} + e^{12}, e^{15} + e^{26}, e^{17} + e^{35} + e^{46}$              | 259      |
| 952:803b | $0, 0, 0, 0, e^{14}a_1 - (-1 + a_1)e^{23}, e^{24} + (-1 + a_1)e^{13}, e^{12} + e^{34}, e^{26} - e^{15}, e^{17} + e^{46} + e^{35}$              | 259      |
| 952:803c | $0, 0, 0, 0, e^{14}a_1 + (-1 + a_1)e^{23}, e^{24} + (-1 + a_1)e^{13}, e^{34} - e^{12}, e^{15} + e^{26}, e^{17} + e^{35} + e^{46}$              | 259      |
| 952:803d | $0, 0, 0, 0, e^{14}a_1 - (-1 + a_1)e^{23}, e^{24} + (-1 + a_1)e^{13}, e^{34} - e^{12}, e^{26} - e^{15}, e^{46} + e^{35} + e^{17}$              | 259      |
| 952:804a | $0, 0, 0, 0, e^{23} + e^{14}, (1 + a_2)e^{13} + e^{24}, a_2e^{12}, e^{16} + e^{25} + e^{34}, e^{15} + e^{26} + e^{37}$                         | 259      |
| 952:804b | $0, 0, 0, 0, -e^{14} + e^{23}, (1 + a_2)e^{13} + e^{24}, a_2e^{12}, -e^{16} + e^{25} + e^{34}, e^{15} + e^{37} + e^{26}$                       | 259      |
| 952:805a | $0, 0, 0, 0, e^{23} + e^{14}, e^{24} + e^{13}, e^{12}, e^{15} + e^{26} + e^{34}, e^{35} + e^{46} + e^{17}$                                     | 259      |
| 952:805b | $0, 0, 0, 0, e^{23} + e^{14}, e^{24} + e^{13}, -e^{12}, e^{15} + e^{26} + e^{34}, e^{17} + e^{35} + e^{46}$                                    | 259      |
| 952:805c | $0, 0, 0, 0, -e^{23} - e^{14}, e^{24} - e^{13}, e^{12}, e^{26} + e^{34} + e^{15}, e^{17} + e^{46} + e^{35}$                                    | 259      |
| 952:805d | $0, 0, 0, 0, -e^{23} - e^{14}, e^{24} - e^{13}, -e^{12}, e^{34} + e^{26} + e^{15}, e^{46} + e^{35} + e^{17}$                                   | 259      |
| 952:806a | $0, 0, 0, 0, e^{23} + e^{14}, e^{24} + e^{13}, e^{12}, e^{15} + e^{26} + e^{34}, e^{36} + e^{45} + e^{17}$                                     | 259      |
| 952:806b | $0, 0, 0, 0, e^{23} - e^{14}, e^{24} + e^{13}, e^{12}, e^{15} + e^{26} + e^{34}, e^{17} + e^{36} + e^{45}$                                     | 259      |
| 952:807a | $0, 0, 0, 0, e^{12}a_1, e^{23}a_4 + (1 + a_1)e^{14}, e^{24} + (a_4 + a_1)e^{13}, e^{35} + e^{27} + e^{16}, e^{45} + e^{17} + e^{26}$           | 259      |
| 952:807b | $0, 0, 0, 0, e^{12}a_1, e^{23}a_4 + (1 + a_1)e^{14}, e^{24} - (a_4 - a_1)e^{13}, -e^{16} + e^{35} + e^{27}, e^{17} + e^{26} + e^{45}$          | 259      |
| 952:808a | $0, 0, 0, 0, e^{12}, (-1 + a_2)e^{23} + e^{14}a_2, e^{24} + e^{13}a_2, e^{27} + e^{16} + e^{35}, e^{15} + e^{36} + e^{47}$                     | 259      |
| 952:808b | $0, 0, 0, 0, e^{12}, -(1 + a_2)e^{23} + e^{14}a_2, e^{24} + e^{13}a_2, e^{35} + e^{27} - e^{16}, e^{36} + e^{47} + e^{15}$                     | 259      |
| 952:808c | $0, 0, 0, 0, -e^{12}, (1 + a_2)e^{23} + e^{14}a_2, e^{24} + e^{13}a_2, e^{35} + e^{27} + e^{16}, e^{36} + e^{47} + e^{15}$                     | 259      |
| 952:808d | $0, 0, 0, 0, -e^{12}, (-1 + a_2)e^{23} - e^{14}a_2, e^{24} - e^{13}a_2, e^{27} + e^{35} - e^{16}, e^{36} + e^{15} + e^{47}$                    | 259      |
| 952:809a | $0, 0, 0, 0, e^{12}a_1, e^{14} + e^{23}, e^{24} + (1 + a_1)e^{13}, e^{35} + e^{27} + e^{16}, e^{46} + e^{37} + e^{15}$                         | 259      |
| 952:809b | $0, 0, 0, 0, e^{12}a_1, -e^{14} + e^{23}, e^{24} + (1 + a_1)e^{13}, e^{35} + e^{27} + e^{16}, e^{46} + e^{37} + e^{15}$                        | 259      |
| 952:810a | $0, 0, 0, 0, e^{12}, a_2e^{14} + e^{23}, a_2e^{13} + e^{24}, e^{15} + e^{46} + e^{37}, e^{25} + e^{36} + e^{47}$                               | 259      |
| 952:810b | $0, 0, 0, 0, e^{12}, a_2e^{14} - e^{23}, a_2e^{13} + e^{24}, e^{15} + e^{46} - e^{37}, e^{25} + e^{36} + e^{47}$                               | 259      |
| 952:811a | $0, 0, 0, 0, e^{12}, e^{23} + e^{14}, e^{24} + a_3e^{13}, e^{47} + e^{15} + a_3e^{36}, e^{37} + e^{46} + e^{25}$                               | 259      |
| 952:811b | $0, 0, 0, 0, e^{12}, e^{23} - e^{14}, e^{24} - a_3e^{13}, e^{47} + e^{15} + a_3e^{36}, e^{37} + e^{46} + e^{25}$                               | 259      |
| 952:811c | $0, 0, 0, 0, -e^{12}, e^{23} - e^{14}, e^{24} - a_3e^{13}, e^{15} + e^{47} + a_3e^{36}, e^{25} + e^{37} + e^{46}$                              | 259      |
| 952:812a | $0, 0, 0, 0, e^{14} + e^{23}a_3, e^{13}(a_2 + a_3) - (-1 + a_2)e^{24}, a_2e^{12} + e^{34}, e^{37} + e^{26} + e^{15}, e^{47} + e^{25} + e^{16}$ | 259      |

Table 2 – Continued to next page

Table 2 – Continued from previous page

| Name      | $\mathfrak{g}$                                                                                                                                     | UCS Dim. |
|-----------|----------------------------------------------------------------------------------------------------------------------------------------------------|----------|
| 952:812b  | $0, 0, 0, 0, e^{14} + e^{23}a_3, (a_2 - a_3)e^{13} - (-1 + a_2)e^{24}, a_2e^{12} + e^{34}, -e^{15} + e^{26} + e^{37}, e^{16} + e^{47} + e^{25}$    | 259      |
| 952:812c  | $0, 0, 0, 0, -e^{14} + e^{23}a_3, e^{13}(a_2 + a_3) - (1 + a_2)e^{24}, a_2e^{12} + e^{34}, e^{26} + e^{15} + e^{37}, e^{47} + e^{16} + e^{25}$     | 259      |
| 952:812d  | $0, 0, 0, 0, -e^{14} - e^{23}a_3, -(a_2 - a_3)e^{13} + (-1 + a_2)e^{24}, -a_2e^{12} + e^{34}, -e^{15} + e^{37} + e^{26}, e^{16} + e^{25} + e^{47}$ | 259      |
| Type: 441 |                                                                                                                                                    |          |
| 951:1     | $0, 0, 0, 0, e^{12}, e^{13}, e^{23}, e^{34}, e^{15}$                                                                                               | 479      |
| 951:2     | $0, 0, 0, 0, e^{12}, e^{13}, e^{14}, e^{34}, e^{15}$                                                                                               | 479      |
| 951:3     | $0, 0, 0, 0, e^{12}, e^{13}, e^{14}, e^{34}, e^{25}$                                                                                               | 479      |
| 951:4     | $0, 0, 0, 0, e^{12}, e^{13}, e^{24}, e^{34}, e^{15}$                                                                                               | 479      |
| 951:5     | $0, 0, 0, 0, e^{12}, e^{13}, e^{23}, e^{14}, e^{15}$                                                                                               | 479      |
| 951:6     | $0, 0, 0, 0, e^{12}, e^{13}, e^{23}, e^{14}, e^{25}$                                                                                               | 479      |
| 951:7     | $0, 0, 0, 0, e^{12}, e^{13}, e^{34}, e^{23} + e^{14}, e^{15}$                                                                                      | 479      |
| 951:8     | $0, 0, 0, 0, e^{12}, e^{13}, e^{34}, e^{14} + e^{23}, e^{25}$                                                                                      | 479      |
| 951:9     | $0, 0, 0, 0, e^{12}, e^{13}, e^{23}, e^{14}, e^{34} + e^{15}$                                                                                      | 479      |
| 951:10    | $0, 0, 0, 0, e^{12}, e^{13}, e^{23}, e^{14}, e^{34} + e^{25}$                                                                                      | 479      |
| 951:11    | $0, 0, 0, 0, e^{12}, e^{13}, e^{23}, e^{34}, e^{14} + e^{25}$                                                                                      | 479      |
| 951:12    | $0, 0, 0, 0, e^{12}, e^{13}, e^{24}, e^{14} + e^{23}, e^{15}$                                                                                      | 479      |
| 951:13    | $0, 0, 0, 0, e^{12}, e^{13}, e^{14}, e^{34}, e^{15} + e^{23}$                                                                                      | 479      |
| 951:14    | $0, 0, 0, 0, e^{12}, e^{13}, e^{24}, e^{34}, e^{15} + e^{23}$                                                                                      | 479      |
| 951:15a   | $0, 0, 0, 0, e^{12}, e^{34}, e^{23} + e^{14}, e^{24} + e^{13}, e^{15}$                                                                             | 479      |
| 951:15b   | $0, 0, 0, 0, e^{12}, e^{34}, -e^{14} + e^{23}, e^{24} + e^{13}, e^{15}$                                                                            | 479      |
| 951:16    | $0, 0, 0, 0, e^{12}, e^{13}, e^{23}, e^{14}, e^{15} + e^{24}$                                                                                      | 479      |
| 951:17    | $0, 0, 0, 0, e^{12}, e^{13}, e^{24}, e^{14} + e^{23}, e^{15} + e^{34}$                                                                             | 479      |
| 951:18    | $0, 0, 0, 0, e^{12}, e^{13}, e^{34}, e^{23} + e^{14}, e^{24} + e^{15}$                                                                             | 479      |
| 951:19    | $0, 0, 0, 0, e^{12}, e^{13}, e^{14}, e^{24}, e^{25} + e^{16}$                                                                                      | 369      |
| 951:20    | $0, 0, 0, 0, e^{12}, e^{13}, e^{14}, e^{24}, e^{15} + e^{36}$                                                                                      | 369      |
| 951:21a   | $0, 0, 0, 0, e^{12}, e^{13}, e^{14}, e^{24}, e^{36} + e^{25}$                                                                                      | 369      |
| 951:21b   | $0, 0, 0, 0, -e^{12}, e^{13}, e^{14}, e^{24}, e^{25} + e^{36}$                                                                                     | 369      |
| 951:22    | $0, 0, 0, 0, e^{12}, e^{13}, e^{14}, e^{24}, e^{26} + e^{35}$                                                                                      | 369      |
| 951:23    | $0, 0, 0, 0, e^{12}, e^{13}, e^{24}, e^{34}, e^{16} + e^{25}$                                                                                      | 369      |
| 951:24a   | $0, 0, 0, 0, e^{12}, e^{13}, e^{24}, e^{34}, e^{36} + e^{25}$                                                                                      | 369      |
| 951:24b   | $0, 0, 0, 0, -e^{12}, e^{13}, e^{24}, e^{34}, e^{36} + e^{25}$                                                                                     | 369      |
| 951:25    | $0, 0, 0, 0, e^{12}, e^{13}, e^{24}, e^{34}, e^{35} + e^{26}$                                                                                      | 369      |
| 951:26    | $0, 0, 0, 0, e^{12}, e^{13}, e^{23}, e^{14}, e^{16} + e^{25}$                                                                                      | 369      |
| 951:27    | $0, 0, 0, 0, e^{12}, e^{13}, e^{23}, e^{24}, e^{16} + e^{25}$                                                                                      | 369      |
| 951:28a   | $0, 0, 0, 0, e^{12}, e^{13}, e^{23}, e^{14}, e^{25} + e^{36}$                                                                                      | 369      |
| 951:28b   | $0, 0, 0, 0, -e^{12}, e^{13}, e^{23}, e^{14}, e^{25} + e^{36}$                                                                                     | 369      |
| 951:29    | $0, 0, 0, 0, e^{12}, e^{13}, e^{23}, e^{14}, e^{35} + e^{26}$                                                                                      | 369      |
| 951:30    | $0, 0, 0, 0, e^{12}, e^{13}, e^{23}, e^{24}, e^{15} + e^{36}$                                                                                      | 369      |
| 951:31a   | $0, 0, 0, 0, e^{12}, e^{13}, e^{23}, e^{24}, e^{36} + e^{25}$                                                                                      | 369      |
| 951:31b   | $0, 0, 0, 0, -e^{12}, e^{13}, e^{23}, e^{24}, e^{25} + e^{36}$                                                                                     | 369      |
| 951:32    | $0, 0, 0, 0, e^{12}, e^{13}, e^{23}, e^{24}, e^{26} + e^{35}$                                                                                      | 369      |
| 951:33    | $0, 0, 0, 0, e^{12}, e^{13}, e^{24}, e^{14} + e^{23}, e^{16} + e^{25}$                                                                             | 369      |
| 951:34    | $0, 0, 0, 0, e^{12}, e^{13}, e^{24}, e^{23} + e^{14}, e^{36} + e^{15}$                                                                             | 369      |
| 951:35a   | $0, 0, 0, 0, e^{12}, e^{13}, e^{24}, e^{14} + e^{23}, e^{36} + e^{25}$                                                                             | 369      |
| 951:35b   | $0, 0, 0, 0, -e^{12}, e^{13}, e^{24}, e^{14} + e^{23}, e^{36} + e^{25}$                                                                            | 369      |
| 951:36    | $0, 0, 0, 0, e^{12}, e^{13}, e^{24}, e^{14} + e^{23}, e^{26} + e^{35}$                                                                             | 369      |
| 951:37    | $0, 0, 0, 0, e^{12}, e^{13}, e^{14}, e^{24}, e^{16} + e^{25} + e^{34}$                                                                             | 369      |
| 951:38a   | $0, 0, 0, 0, e^{12}, e^{13}, e^{24}, e^{34}, e^{36} + e^{25} + e^{14}$                                                                             | 369      |
| 951:38b   | $0, 0, 0, 0, -e^{12}, e^{13}, e^{24}, e^{34}, e^{14} + e^{25} + e^{36}$                                                                            | 369      |
| 951:39    | $0, 0, 0, 0, e^{12}, e^{13}, e^{24}, e^{34}, e^{35} + e^{14} + e^{26}$                                                                             | 369      |
| 951:40    | $0, 0, 0, 0, e^{12}, e^{13}, e^{23}, e^{14}, e^{15} + e^{24} + e^{36}$                                                                             | 369      |
| 951:41a   | $0, 0, 0, 0, e^{12}, e^{13}, e^{23}, e^{24}, e^{36} + e^{25} + e^{14}$                                                                             | 369      |
| 951:41b   | $0, 0, 0, 0, -e^{12}, e^{13}, e^{23}, e^{24}, e^{25} + e^{36} + e^{14}$                                                                            | 369      |
| 951:42    | $0, 0, 0, 0, e^{12}, e^{13}, e^{23}, e^{24}, e^{14} + e^{26} + e^{35}$                                                                             | 369      |
| 951:43    | $0, 0, 0, 0, e^{12}, e^{13}, e^{23}, e^{24}, e^{34} + e^{25} + e^{16}$                                                                             | 369      |
| 951:44    | $0, 0, 0, 0, e^{12}, e^{13}, e^{24}, e^{23} + e^{14}, e^{16} + e^{25} + e^{34}$                                                                    | 369      |
| 951:45    | $0, 0, 0, 0, e^{12}, e^{13}, e^{23}, e^{14}, e^{25} + e^{37} + e^{16}$                                                                             | 269      |
| 951:46    | $0, 0, 0, 0, (-1 + a_2)e^{12}, e^{13}a_2, e^{23}, e^{14}, e^{17} + e^{35} + e^{26}$                                                                | 269      |

Table 2 – Continued to next page



Table 2 – Continued from previous page

| Name    | $\mathfrak{g}$                                                                                | UCS Dim. |
|---------|-----------------------------------------------------------------------------------------------|----------|
| 951:47  | $0, 0, 0, 0, e^{12}, e^{34}, e^{13}, e^{23}, e^{15} + e^{36}$                                 | 359      |
| 951:48  | $0, 0, 0, 0, e^{12}, e^{34}, e^{13}, e^{23}, e^{46} + e^{15}$                                 | 359      |
| 951:49  | $0, 0, 0, 0, e^{12}, e^{34}, e^{13}, e^{24}, e^{36} + e^{15}$                                 | 359      |
| 951:50  | $0, 0, 0, 0, e^{12}, e^{34}, e^{13}, e^{24}, e^{36} + e^{25}$                                 | 359      |
| 951:51  | $0, 0, 0, 0, e^{12}, e^{34}, e^{13}, e^{14} + e^{23}, e^{36} + e^{15}$                        | 359      |
| 951:52  | $0, 0, 0, 0, e^{12}, e^{34}, e^{13}, e^{14} + e^{23}, e^{25} + e^{36}$                        | 359      |
| 951:53  | $0, 0, 0, 0, e^{12}, e^{34}, e^{13}, e^{23} + e^{14}, e^{46} + e^{25}$                        | 359      |
| 951:54  | $0, 0, 0, 0, -e^{12}, e^{14} + e^{23}, e^{13}, e^{24}, e^{16} + e^{35}$                       | 359      |
| 951:55  | $0, 0, 0, 0, -e^{12}, e^{14} + e^{23}, e^{13}, e^{34}, e^{16} + e^{35}$                       | 359      |
| 951:56  | $0, 0, 0, 0, e^{12}, e^{23} + e^{14}, e^{13}, e^{34}, e^{45} + e^{26}$                        | 359      |
| 951:57  | $0, 0, 0, 0, e^{12}, e^{34}, e^{13}, e^{23}, e^{36} + e^{25} + e^{14}$                        | 359      |
| 951:58  | $0, 0, 0, 0, e^{12}, e^{34}, e^{13}, e^{24}, e^{15} + e^{46} + e^{23}$                        | 359      |
| 951:59a | $0, 0, 0, 0, e^{12}, e^{34}, e^{23} + e^{14}, e^{24} + e^{13}, e^{15} + e^{36}$               | 359      |
| 951:59b | $0, 0, 0, 0, e^{12}, e^{34}, -e^{14} + e^{23}, e^{24} + e^{13}, e^{15} + e^{36}$              | 359      |
| 951:60a | $0, 0, 0, 0, -e^{12}, e^{14} + e^{23}, e^{34}, e^{13} + e^{24}, e^{16} + e^{35}$              | 359      |
| 951:60b | $0, 0, 0, 0, -e^{12}, -e^{14} + e^{23}, e^{34}, e^{24} + e^{13}, e^{35} + e^{16}$             | 359      |
| 951:61a | $0, 0, 0, 0, e^{14} + e^{23}, e^{13} + e^{24}, e^{12}, e^{34}, e^{26} + e^{15}$               | 359      |
| 951:61b | $0, 0, 0, 0, e^{23} - e^{14}, e^{24} + e^{13}, e^{12}, e^{34}, e^{15} + e^{26}$               | 359      |
| 951:62  | $0, 0, 0, 0, e^{12}, e^{34}, e^{13}, e^{14} + e^{23}, e^{15} + e^{24} + e^{36}$               | 359      |
| 951:63  | $0, 0, 0, 0, -e^{12}, e^{23} + e^{14}, e^{13}, e^{34}, e^{35} + e^{24} + e^{16}$              | 359      |
| 951:64a | $0, 0, 0, 0, e^{12}, e^{13}, e^{14}, e^{23}, e^{36} + e^{25} + e^{17}$                        | 259      |
| 951:64b | $0, 0, 0, 0, -e^{12}, e^{13}, e^{14}, e^{23}, e^{17} + e^{36} + e^{25}$                       | 259      |
| 951:65  | $0, 0, 0, 0, e^{12}, e^{13}, e^{14}, e^{23}, e^{26} + e^{35} + e^{17}$                        | 259      |
| 951:66  | $0, 0, 0, 0, e^{12}, e^{13}, e^{24}, e^{23}, e^{15} + e^{36} + e^{27}$                        | 259      |
| 951:67a | $0, 0, 0, 0, e^{12}, e^{13}, e^{14}, e^{23}, e^{25} + e^{16} + e^{47}$                        | 259      |
| 951:67b | $0, 0, 0, 0, -e^{12}, e^{13}, e^{14}, e^{23}, e^{47} + e^{25} + e^{16}$                       | 259      |
| 951:68  | $0, 0, 0, 0, e^{12}, e^{13}, e^{14}, e^{23}, e^{45} + e^{27} + e^{16}$                        | 259      |
| 951:69  | $0, 0, 0, 0, e^{12}, e^{13}, e^{24}, e^{23}, e^{25} + e^{47} + e^{16}$                        | 259      |
| 951:70a | $0, 0, 0, 0, e^{12}, e^{13}, e^{14}, e^{23}, e^{36} + e^{47} + e^{25}$                        | 259      |
| 951:70b | $0, 0, 0, 0, -e^{12}, -e^{13}, e^{14}, e^{23}, e^{25} + e^{47} + e^{36}$                      | 259      |
| 951:70c | $0, 0, 0, 0, -e^{12}, -e^{13}, e^{14}, e^{23}, e^{36} + e^{25} + e^{47}$                      | 259      |
| 951:71  | $0, 0, 0, 0, e^{12}, e^{13}, e^{14}, e^{23}, e^{35} + e^{47} + e^{26}$                        | 259      |
| 951:72  | $0, 0, 0, 0, e^{12}, e^{13}, e^{14}, e^{23}, e^{37} + e^{46} + e^{25}$                        | 259      |
| 951:73a | $0, 0, 0, 0, e^{12}, e^{13}, e^{24}, e^{23}, e^{47} + e^{36} + e^{15}$                        | 259      |
| 951:73b | $0, 0, 0, 0, -e^{12}, e^{13}, e^{24}, e^{23}, e^{15} + e^{36} + e^{47}$                       | 259      |
| 951:74  | $0, 0, 0, 0, -e^{12}, e^{13}, e^{24}, e^{23}, e^{45} + e^{17} + e^{36}$                       | 259      |
| 951:75a | $0, 0, 0, 0, e^{12}, e^{13}, e^{24}, e^{23}, e^{25} + e^{36} + e^{47}$                        | 259      |
| 951:75b | $0, 0, 0, 0, -e^{12}, e^{13}, e^{24}, e^{23}, e^{47} + e^{25} + e^{36}$                       | 259      |
| 951:76  | $0, 0, 0, 0, e^{12}, e^{13}, e^{24}, e^{23}, e^{35} + e^{47} + e^{26}$                        | 259      |
| 951:77  | $0, 0, 0, 0, e^{12}, e^{13}, e^{24}, e^{34}, e^{15} + e^{27} + e^{36}$                        | 259      |
| 951:78a | $0, 0, 0, 0, e^{12}, e^{13}, e^{24}, e^{34}, e^{36} + e^{47} + e^{15}$                        | 259      |
| 951:78b | $0, 0, 0, 0, -e^{12}, e^{13}, e^{24}, e^{34}, e^{15} + e^{47} + e^{36}$                       | 259      |
| 951:79  | $0, 0, 0, 0, -e^{12}, e^{13}, e^{24}, e^{34}, e^{17} + e^{45} + e^{36}$                       | 259      |
| 951:80  | $0, 0, 0, 0, e^{12}, e^{13}, e^{24}, e^{23} + e^{14}, e^{27} + e^{36} + e^{15}$               | 259      |
| 951:81a | $0, 0, 0, 0, e^{12}, e^{13}, e^{24}, e^{23} + e^{14}, e^{47} + e^{36} + e^{15}$               | 259      |
| 951:81b | $0, 0, 0, 0, -e^{12}, e^{13}, e^{24}, e^{14} + e^{23}, e^{36} + e^{15} + e^{47}$              | 259      |
| 951:82  | $0, 0, 0, 0, -e^{12}, e^{13}, e^{24}, e^{14} + e^{23}, e^{36} + e^{45} + e^{17}$              | 259      |
| 951:83  | $0, 0, 0, 0, e^{12}(-1 + a_2), a_2 e^{13}, e^{23} + e^{14}, e^{24}, e^{17} + e^{26} + e^{35}$ | 259      |
| 951:84a | $0, 0, 0, 0, e^{12}, e^{13}, e^{23} + e^{14}, e^{24}, e^{45} + e^{27} + e^{16}$               | 259      |
| 951:84b | $0, 0, 0, 0, e^{12}, -e^{13}, e^{14} + e^{23}, e^{24}, e^{16} + e^{45} + e^{27}$              | 259      |
| 951:85a | $0, 0, 0, 0, e^{12}, e^{13}, e^{23} + e^{14}, e^{24}, e^{15} + e^{37} + e^{46}$               | 259      |
| 951:85b | $0, 0, 0, 0, -e^{12}, e^{13}, e^{14} + e^{23}, e^{24}, e^{46} + e^{37} + e^{15}$              | 259      |
| 951:86  | $0, 0, 0, 0, e^{12}, e^{13}, e^{23} + e^{14}, e^{24}, e^{37} + e^{46} + e^{25}$               | 259      |
| 951:87  | $0, 0, 0, 0, e^{12}, e^{13}, e^{14} + e^{23}, e^{24}, e^{27} + e^{45} + e^{36}$               | 259      |
| 951:88  | $0, 0, 0, 0, e^{12}, e^{34}, e^{23} + e^{14}, e^{13}, e^{16} + e^{25} + e^{37}$               | 259      |
| 951:89  | $0, 0, 0, 0, e^{12}, e^{34}, e^{14} - e^{23}, e^{13}, e^{15} + e^{47} + e^{26}$               | 259      |
| 951:90a | $0, 0, 0, 0, e^{12}, e^{34}, e^{23} + e^{14}, e^{24} + e^{13}, e^{37} + e^{16} + e^{25}$      | 259      |
| 951:90b | $0, 0, 0, 0, e^{12}, e^{34}, e^{14} + e^{23}, -e^{13} + e^{24}, e^{25} + e^{37} + e^{16}$     | 259      |

Table 2 – Continued to next page

Table 2 – Continued from previous page

| Name        | $\mathfrak{g}$                                                                                                | UCS Dim. |
|-------------|---------------------------------------------------------------------------------------------------------------|----------|
| 951:91a     | $0, 0, 0, 0, (-1 + a_2)e^{12}, e^{23} + e^{14}, e^{24} + e^{13}a_2, e^{34}, e^{27} + e^{16} + e^{35}$         | 259      |
| 951:91b     | $0, 0, 0, 0, (-1 + a_2)e^{12}, -e^{14} + e^{23}, e^{24} + e^{13}a_2, e^{34}, e^{16} + e^{35} + e^{27}$        | 259      |
| 951:92a     | $0, 0, 0, 0, e^{12}, e^{14} + e^{23}, e^{13} + e^{24}, e^{34}, e^{47} + e^{36} + e^{15}$                      | 259      |
| 951:92b     | $0, 0, 0, 0, e^{12}, -e^{23} + e^{14}, e^{24} + e^{13}, e^{34}, e^{15} + e^{47} + e^{36}$                     | 259      |
| 951:92c     | $0, 0, 0, 0, -e^{12}, e^{14} + e^{23}, e^{13} + e^{24}, e^{34}, e^{15} + e^{36} + e^{47}$                     | 259      |
| 951:93a     | $0, 0, 0, 0, e^{12}, e^{23} + e^{14}, e^{24} + e^{13}, e^{34}, e^{37} + e^{46} + e^{15}$                      | 259      |
| 951:93b     | $0, 0, 0, 0, e^{12}, -e^{14} + e^{23}, e^{13} + e^{24}, e^{34}, e^{37} + e^{15} + e^{46}$                     | 259      |
| 951:94a     | $0, 0, 0, 0, e^{12}, e^{13}, e^{23}, e^{14}, e^{16} + e^{25} + e^{48} + e^{37}$                               | 159      |
| 951:94b     | $0, 0, 0, 0, -e^{12}, e^{13}, e^{23}, e^{14}, e^{16} + e^{25} + e^{37} + e^{48}$                              | 159      |
| 951:95      | $0, 0, 0, 0, (-1 + a_2)e^{12}, e^{13}a_2, e^{23}, e^{14}, e^{35} + e^{48} + e^{17} + e^{26}$                  | 159      |
| 951:96      | $0, 0, 0, 0, e^{12}, e^{13}, e^{23}, e^{14}, e^{27} + e^{15} + e^{38} + e^{46}$                               | 159      |
| 951:97      | $0, 0, 0, 0, e^{12}, e^{13}, e^{24}, e^{34}, e^{15} + e^{27} + e^{36} + e^{48}$                               | 159      |
| 951:98a     | $0, 0, 0, 0, e^{12}, e^{13}, e^{24}, e^{23} + e^{14}, e^{16} + e^{25} + e^{48} + e^{37}$                      | 159      |
| 951:98b     | $0, 0, 0, 0, -e^{12}, e^{13}, e^{24}, e^{14} + e^{23}, e^{37} + e^{48} + e^{25} + e^{16}$                     | 159      |
| 951:99      | $0, 0, 0, 0, e^{12}a_1, e^{13}, e^{24}, e^{14}(1 + a_1) + e^{23}, e^{36} + e^{45} + e^{28} + e^{17}$          | 159      |
| 951:100a    | $0, 0, 0, 0, e^{12}, e^{34}, e^{14}(1 + a_2) + e^{23}, e^{13}a_2 + e^{24}, e^{16} + e^{25} + e^{48} + e^{37}$ | 159      |
| 951:100b    | $0, 0, 0, 0, e^{12}, e^{34}, e^{14}(1 + a_2) - e^{23}, e^{13}a_2 + e^{24}, e^{48} + e^{25} + e^{37} + e^{16}$ | 159      |
| Type: 51111 |                                                                                                               |          |
| 94321:1     | $0, 0, 0, 0, 0, e^{12}, e^{16}, e^{17}, e^{18}$                                                               | 45679    |
| 94321:2     | $0, 0, 0, 0, 0, e^{12}, e^{16}, e^{17}, e^{18} + e^{34}$                                                      | 25679    |
| 94321:3     | $0, 0, 0, 0, 0, e^{12}, e^{16}, e^{17}, e^{18} + e^{23}$                                                      | 35679    |
| 94321:4     | $0, 0, 0, 0, 0, e^{12}, e^{16}, e^{17}, e^{18} + e^{23} + e^{45}$                                             | 15679    |
| 94321:5     | $0, 0, 0, 0, 0, e^{12}, e^{16}, e^{17}, e^{18} + e^{26}$                                                      | 45679    |
| 94321:6     | $0, 0, 0, 0, 0, -e^{12}, e^{16}, e^{17}, e^{28} + e^{67}$                                                     | 45679    |
| 94321:7     | $0, 0, 0, 0, 0, -e^{12}, e^{16}, e^{23} + e^{17}, e^{18} + e^{36}$                                            | 34679    |
| 94321:8     | $0, 0, 0, 0, 0, e^{12}, e^{16}, e^{17}, e^{18} + e^{26} + e^{34}$                                             | 25679    |
| 94321:9     | $0, 0, 0, 0, 0, -e^{12}, e^{16}, e^{17}, e^{67} + e^{28} + e^{34}$                                            | 25679    |
| 94321:10    | $0, 0, 0, 0, 0, -e^{12}, e^{16}, e^{23} + e^{17}, e^{36} + e^{45} + e^{18}$                                   | 14679    |
| 94321:11    | $0, 0, 0, 0, 0, -e^{12}, e^{16}, e^{17} + e^{23}, e^{67} + e^{28}$                                            | 34679    |
| 94321:12    | $0, 0, 0, 0, 0, -e^{12}, e^{16}, e^{17}, e^{28} + e^{13} + e^{67}$                                            | 35679    |
| 94321:13    | $0, 0, 0, 0, 0, -e^{12}, e^{16}, e^{17} + e^{23}, e^{24} + e^{36} + e^{18}$                                   | 24679    |
| 94321:14    | $0, 0, 0, 0, 0, e^{12}, e^{16}, e^{17} + e^{26}, e^{18} + e^{27}$                                             | 45679    |
| 94321:15    | $0, 0, 0, 0, 0, -e^{12}, e^{16}, e^{17} + e^{23}, e^{28} + e^{67} + e^{34}$                                   | 24679    |
| 94321:16    | $0, 0, 0, 0, 0, -e^{12}, e^{16}, e^{17} + e^{23}, e^{67} + e^{28} + e^{45}$                                   | 14679    |
| 94321:17    | $0, 0, 0, 0, 0, -e^{12}, e^{16}, e^{17} + e^{26}, e^{28} + e^{67}$                                            | 45679    |
| 94321:18    | $0, 0, 0, 0, 0, -e^{12}, e^{16}, e^{17}, e^{13} + e^{28} + e^{45} + e^{67}$                                   | 15679    |
| 94321:19    | $0, 0, 0, 0, 0, e^{12}, e^{16}, e^{17} + e^{26}, e^{27} + e^{18} + e^{34}$                                    | 25679    |
| 94321:20    | $0, 0, 0, 0, 0, -e^{12}, e^{16}, e^{23} + e^{17}, e^{67} + e^{28} + e^{13}$                                   | 34679    |
| 94321:21    | $0, 0, 0, 0, 0, -e^{12}, e^{16}, e^{17} + e^{23}, e^{28} + e^{14} + e^{67}$                                   | 24679    |
| 94321:22    | $0, 0, 0, 0, 0, -e^{12}, e^{16}, e^{26} + e^{17}, e^{67} + e^{34} + e^{28}$                                   | 25679    |
| 94321:23    | $0, 0, 0, 0, 0, -e^{12}, e^{16}, e^{17} + e^{23}, e^{28} + e^{67} + e^{45} + e^{13}$                          | 14679    |
| 94321:24    | $0, 0, 0, 0, 0, -e^{12}, e^{16}, e^{17} + e^{23}, e^{67} + e^{28} + e^{35} + e^{14}$                          | 14679    |
| 94321:25    | $0, 0, 0, 0, 0, -e^{12}, e^{16}, e^{17} + e^{26}, e^{28} + e^{13} + e^{67}$                                   | 35679    |
| 94321:26    | $0, 0, 0, 0, 0, -e^{12}, e^{23} + e^{16}, e^{36} + e^{17}, e^{37} + e^{18}$                                   | 34579    |
| 94321:27    | $0, 0, 0, 0, 0, -e^{12}, e^{16}, e^{26} + e^{17}, e^{28} + e^{13} + e^{45} + e^{67}$                          | 15679    |
| 94321:28    | $0, 0, 0, 0, 0, -e^{12}, e^{16} + e^{23}, e^{17} + e^{36}, e^{45} + e^{37} + e^{18}$                          | 14579    |
| 94321:30    | $0, 0, 0, 0, 0, -e^{12}, e^{16} + e^{23}, e^{17} + e^{36}, e^{24} + e^{37} + e^{18}$                          | 24579    |
| 94321:36    | $0, 0, 0, 0, 0, -e^{12}, e^{16} + e^{23}, e^{36} + e^{17}, e^{18} + e^{37} + e^{26}$                          | 34579    |
| 94321:39    | $0, 0, 0, 0, 0, -e^{12}, e^{16} + e^{23}, e^{24} + e^{36} + e^{17}, e^{18} + e^{46} + e^{37}$                 | 23579    |
| 94321:43    | $0, 0, 0, 0, 0, -e^{12}, e^{16} + e^{23}, e^{36} + e^{17}, e^{37} + e^{26} + e^{18} + e^{45}$                 | 14579    |
| 94321:47    | $0, 0, 0, 0, 0, e^{12}, e^{26} + e^{13}, e^{27} + e^{36} + e^{14}, e^{15} + e^{28} + e^{37} + e^{46}$         | 13579    |
| Type: 5121  |                                                                                                               |          |
| 9431:1      | $0, 0, 0, 0, 0, e^{12}, e^{16}, e^{26}, e^{17}$                                                               | 5679     |
| 9431:2      | $0, 0, 0, 0, 0, e^{12}, e^{16}, e^{26} + e^{34}, e^{17}$                                                      | 3679     |
| 9431:3      | $0, 0, 0, 0, 0, e^{12}, e^{16}, e^{13} + e^{26}, e^{17}$                                                      | 4679     |
| 9431:4      | $0, 0, 0, 0, 0, e^{12}, e^{16}, e^{26}, e^{34} + e^{17}$                                                      | 3679     |
| 9431:5      | $0, 0, 0, 0, 0, e^{12}, e^{16}, e^{26} + e^{34}, e^{17} + e^{35}$                                             | 2679     |
| 9431:6      | $0, 0, 0, 0, 0, e^{12}, e^{16}, e^{45} + e^{26} + e^{13}, e^{17}$                                             | 2679     |

Table 2 – Continued to next page

Table 2 – Continued from previous page

| Name     | $\mathfrak{g}$                                                                                 | UCS Dim. |
|----------|------------------------------------------------------------------------------------------------|----------|
| 9431:7   | $0, 0, 0, 0, 0, e^{12}, e^{16}, e^{26}, e^{17} + e^{23}$                                       | 4679     |
| 9431:8   | $0, 0, 0, 0, 0, e^{12}, e^{16}, e^{13} + e^{26}, e^{17} + e^{34}$                              | 3679     |
| 9431:9   | $0, 0, 0, 0, 0, e^{12}, e^{16}, e^{26} + e^{34}, e^{23} + e^{17}$                              | 3679     |
| 9431:10  | $0, 0, 0, 0, 0, e^{12}, e^{16}, e^{13} + e^{26}, e^{45} + e^{17}$                              | 2679     |
| 9431:11  | $0, 0, 0, 0, 0, e^{12}, e^{16}, e^{26} + e^{34}, e^{25} + e^{17}$                              | 2679     |
| 9431:12  | $0, 0, 0, 0, 0, e^{12}, e^{16}, e^{26} + e^{45} + e^{13}, e^{17} + e^{34}$                     | 2679     |
| 9431:13  | $0, 0, 0, 0, 0, e^{12}, e^{16}, e^{26} + e^{13}, e^{17} + e^{23}$                              | 4679     |
| 9431:14  | $0, 0, 0, 0, 0, e^{12}, e^{16}, e^{26} + e^{13}, e^{17} + e^{24}$                              | 3679     |
| 9431:15  | $0, 0, 0, 0, 0, e^{12}, e^{16}, e^{26}, e^{17} + e^{23} + e^{45}$                              | 2679     |
| 9431:16  | $0, 0, 0, 0, 0, e^{12}, e^{16}, e^{34} + e^{26}, e^{23} + e^{45} + e^{17}$                     | 2679     |
| 9431:17  | $0, 0, 0, 0, 0, e^{12}, e^{16}, e^{13} + e^{45} + e^{26}, e^{23} + e^{17}$                     | 2679     |
| 9431:18  | $0, 0, 0, 0, 0, e^{12}, e^{16}, e^{26} + e^{35} + e^{14}, e^{17} + e^{23}$                     | 2679     |
| 9431:19  | $0, 0, 0, 0, 0, e^{12}, e^{16}, e^{13} + e^{26}, e^{17} + e^{45} + e^{23}$                     | 2679     |
| 9431:20  | $0, 0, 0, 0, 0, e^{12}, e^{16}, e^{26} + e^{13}, e^{35} + e^{24} + e^{17}$                     | 2679     |
| 9431:21  | $0, 0, 0, 0, 0, e^{12}, e^{16}, e^{26} + e^{35} + e^{14}, e^{17} + e^{45} + e^{23}$            | 2679     |
| 9431:22  | $0, 0, 0, 0, 0, e^{12}, e^{26} + e^{13}, e^{16}, e^{36} + e^{27}$                              | 4579     |
| 9431:23  | $0, 0, 0, 0, 0, e^{12}, e^{26} + e^{13}, e^{34} + e^{16}, e^{27} + e^{36}$                     | 3579     |
| 9431:24  | $0, 0, 0, 0, 0, e^{12}, e^{13} + e^{26}, e^{45} + e^{16}, e^{36} + e^{27}$                     | 2579     |
| 9431:25a | $0, 0, 0, 0, 0, -e^{12}, e^{16} + e^{23}, e^{26} + e^{13}, e^{17} + e^{36}$                    | 4579     |
| 9431:25b | $0, 0, 0, 0, 0, -e^{12}, e^{23} - e^{16}, e^{13} + e^{26}, e^{36} + e^{17}$                    | 4579     |
| 9431:26  | $0, 0, 0, 0, 0, -e^{12}, e^{23} + e^{16}, e^{14} + e^{26}, e^{36} + e^{17}$                    | 3579     |
| 9431:27  | $0, 0, 0, 0, 0, e^{12}, e^{13} + e^{26}, e^{16}, e^{36} + e^{27} + e^{45}$                     | 2579     |
| 9431:28  | $0, 0, 0, 0, 0, e^{12}, e^{26} + e^{13}, e^{34} + e^{16}, e^{27} + e^{36} + e^{45}$            | 2579     |
| 9431:29a | $0, 0, 0, 0, 0, -e^{12}, e^{23} + e^{16}, e^{45} + e^{13} + e^{26}, e^{36} + e^{17}$           | 2579     |
| 9431:29b | $0, 0, 0, 0, 0, -e^{12}, e^{23} - e^{16}, e^{13} + e^{45} + e^{26}, e^{36} + e^{17}$           | 2579     |
| 9431:30  | $0, 0, 0, 0, 0, -e^{12}, e^{23} + e^{16}, e^{14} + e^{26} + e^{35}, e^{17} + e^{36}$           | 2579     |
| 9431:31  | $0, 0, 0, 0, 0, e^{12}, e^{26} + e^{13}, e^{16}, e^{27} + e^{36} + e^{14}$                     | 3579     |
| 9431:32a | $0, 0, 0, 0, 0, e^{12}, e^{26} + e^{13}, e^{16} + e^{34}, e^{14} + e^{36} + e^{27}$            | 3579     |
| 9431:32b | $0, 0, 0, 0, 0, e^{12}, e^{13} + e^{26}, -e^{16} + e^{34}, e^{14} + e^{27} + e^{36}$           | 3579     |
| 9431:33  | $0, 0, 0, 0, 0, -e^{12}, e^{23} + e^{16}, e^{14} + e^{26}, e^{17} + e^{45} + e^{36}$           | 2579     |
| 9431:34  | $0, 0, 0, 0, 0, e^{12}, e^{26} + e^{13}, e^{45} + e^{16}, e^{14} + e^{27} + e^{36}$            | 2579     |
| 9431:35a | $0, 0, 0, 0, 0, -e^{12}, e^{23} + e^{16}, e^{13} + e^{26}, e^{17} + e^{45} + e^{36}$           | 2579     |
| 9431:35b | $0, 0, 0, 0, 0, -e^{12}, e^{23} - e^{16}, e^{13} + e^{26}, e^{36} + e^{45} + e^{17}$           | 2579     |
| 9431:36  | $0, 0, 0, 0, 0, e^{12}, e^{13} + e^{26}, e^{34} + e^{16}, e^{36} + e^{27} + e^{15}$            | 2579     |
| 9431:37  | $0, 0, 0, 0, 0, -e^{12}, e^{16} + e^{23}, e^{26} + e^{35} + e^{14}, e^{17} + e^{36} + e^{45}$  | 2579     |
| 9431:38  | $0, 0, 0, 0, 0, -e^{12}, e^{23} + e^{16}, e^{14} + e^{26}, e^{36} + e^{17} + e^{24}$           | 3579     |
| 9431:39a | $0, 0, 0, 0, 0, -e^{12}, e^{23} + e^{16}, e^{13} + e^{26}, e^{24} + e^{36} + e^{17}$           | 3579     |
| 9431:39b | $0, 0, 0, 0, 0, -e^{12}, e^{23} - e^{16}, e^{13} + e^{26}, e^{17} + e^{36} + e^{24}$           | 3579     |
| 9431:40  | $0, 0, 0, 0, 0, -e^{12}, e^{16} + e^{23}, e^{26} + e^{14}, e^{17} + e^{25} + e^{36}$           | 2579     |
| 9431:41a | $0, 0, 0, 0, 0, e^{12}, e^{26} + e^{13}, e^{45} + e^{16} + e^{23}, e^{14} + e^{36} + e^{27}$   | 2579     |
| 9431:41b | $0, 0, 0, 0, 0, -e^{12}, -e^{13} + e^{26}, e^{23} + e^{45} + e^{16}, e^{36} + e^{14} + e^{27}$ | 2579     |
| 9431:42  | $0, 0, 0, 0, 0, e^{12}, e^{13} + e^{26}, e^{24} + e^{35} + e^{16}, e^{36} + e^{27} + e^{14}$   | 2579     |
| 9431:43a | $0, 0, 0, 0, 0, e^{12}, e^{26} + e^{13}, e^{16} + e^{34} + e^{25}, e^{27} + e^{36} + e^{14}$   | 2579     |
| 9431:43b | $0, 0, 0, 0, 0, e^{12}, e^{26} + e^{13}, -e^{16} + e^{25} + e^{34}, e^{14} + e^{36} + e^{27}$  | 2579     |
| 9431:44a | $0, 0, 0, 0, 0, e^{12}, e^{16}, e^{26}, e^{28} + e^{17}$                                       | 4679     |
| 9431:44b | $0, 0, 0, 0, 0, e^{12}, -e^{16}, e^{26}, e^{28} + e^{17}$                                      | 4679     |
| 9431:45  | $0, 0, 0, 0, 0, e^{12}, e^{16}, e^{26}, e^{27} + e^{18}$                                       | 4679     |
| 9431:46a | $0, 0, 0, 0, 0, e^{12}, e^{16}, e^{26}, e^{28} + e^{34} + e^{17}$                              | 2679     |
| 9431:46b | $0, 0, 0, 0, 0, e^{12}, -e^{16}, e^{26}, e^{28} + e^{17} + e^{34}$                             | 2679     |
| 9431:47  | $0, 0, 0, 0, 0, e^{12}, e^{16}, e^{26}, e^{18} + e^{34} + e^{27}$                              | 2679     |
| 9431:48  | $0, 0, 0, 0, 0, e^{12}, e^{16}, e^{26} + e^{13}, e^{27} + e^{18}$                              | 3579     |
| 9431:49  | $0, 0, 0, 0, 0, e^{12}, e^{16}, e^{13} + e^{26}, e^{18} + e^{34} + e^{27}$                     | 2579     |
| 9431:50  | $0, 0, 0, 0, 0, e^{12}, e^{16}, e^{26} + e^{13}, e^{18} + e^{27} + e^{45}$                     | 1579     |
| 9431:51a | $0, 0, 0, 0, 0, e^{12}, e^{16} + e^{23}, e^{26} + e^{13}, e^{28} + e^{17}$                     | 3579     |
| 9431:51b | $0, 0, 0, 0, 0, e^{12}, e^{23} - e^{16}, e^{26} + e^{13}, e^{28} + e^{17}$                     | 3579     |
| 9431:52a | $0, 0, 0, 0, 0, e^{12}, e^{13} + e^{26}, e^{16} + e^{23}, e^{17} + e^{28}$                     | 3579     |
| 9431:52b | $0, 0, 0, 0, 0, e^{12}, e^{26} - e^{13}, e^{23} + e^{16}, e^{28} + e^{17}$                     | 3579     |
| 9431:53a | $0, 0, 0, 0, 0, e^{12}, e^{16}, e^{26} + e^{13}, e^{28} + e^{17} + e^{36}$                     | 3579     |

Table 2 – Continued to next page

Table 2 – Continued from previous page

| Name       | $\mathfrak{g}$                                                                                            | UCS Dim. |
|------------|-----------------------------------------------------------------------------------------------------------|----------|
| 9431:53b   | $0, 0, 0, 0, 0, e^{12}, -e^{16}, e^{13} + e^{26}, e^{17} + e^{28} + e^{36}$                               | 3579     |
| 9431:54a   | $0, 0, 0, 0, 0, e^{12}, e^{16} + e^{23}, e^{13} + e^{26}, e^{28} + e^{34} + e^{17}$                       | 2579     |
| 9431:54b   | $0, 0, 0, 0, 0, e^{12}, -e^{16} + e^{23}, e^{26} + e^{13}, e^{17} + e^{28} + e^{34}$                      | 2579     |
| 9431:55a   | $0, 0, 0, 0, 0, e^{12}, e^{16} + e^{23}, e^{26} + e^{13}, e^{18} + e^{34} + e^{27}$                       | 2579     |
| 9431:55b   | $0, 0, 0, 0, 0, e^{12}, e^{16} + e^{23}, -e^{13} + e^{26}, e^{18} + e^{34} + e^{27}$                      | 2579     |
| 9431:56a   | $0, 0, 0, 0, 0, e^{12}, e^{16} + e^{23}, e^{13} + e^{26}, e^{17} + e^{28} + e^{45}$                       | 1579     |
| 9431:56b   | $0, 0, 0, 0, 0, e^{12}, e^{23} - e^{16}, e^{26} + e^{13}, e^{28} + e^{45} + e^{17}$                       | 1579     |
| 9431:57a   | $0, 0, 0, 0, 0, e^{12}, e^{16} + e^{23}, e^{26} + e^{13}, e^{18} + e^{27} + e^{45}$                       | 1579     |
| 9431:57b   | $0, 0, 0, 0, 0, e^{12}, e^{23} + e^{16}, e^{26} - e^{13}, e^{27} + e^{45} + e^{18}$                       | 1579     |
| 9431:58    | $0, 0, 0, 0, 0, e^{12}, e^{13} + e^{26}, e^{24} + e^{16}, e^{28} + e^{17}$                                | 2479     |
| 9431:59a   | $0, 0, 0, 0, 0, e^{12}, e^{16}, e^{26} + e^{13}, e^{17} + e^{28} + e^{36} + e^{45}$                       | 1579     |
| 9431:59b   | $0, 0, 0, 0, 0, e^{12}, -e^{16}, e^{26} + e^{13}, e^{28} + e^{17} + e^{36} + e^{45}$                      | 1579     |
| 9431:60a   | $0, 0, 0, 0, 0, (-1 + a_2)e^{12}, e^{23} + e^{16}, a_2e^{13} + e^{26}, e^{28} + e^{36} + e^{17}$          | 3579     |
| 9431:60b   | $0, 0, 0, 0, 0, (-1 + a_2)e^{12}, e^{23} - e^{16}, a_2e^{13} + e^{26}, e^{17} + e^{28} + e^{36}$          | 3579     |
| 9431:61    | $0, 0, 0, 0, 0, a_1e^{12}, e^{16} + e^{23}, e^{14} + e^{26}, e^{18} + e^{34} + e^{27}$                    | 2479     |
| 9431:62    | $0, 0, 0, 0, 0, e^{12}, e^{23} + e^{16}, e^{14} + e^{26}, e^{35} + e^{27} + e^{18}$                       | 1479     |
| 9431:63a   | $0, 0, 0, 0, 0, e^{12}a_1, e^{23} + e^{16}, e^{26} + e^{13}(1 + a_1), e^{17} + e^{45} + e^{28} + e^{36}$  | 1579     |
| 9431:63b   | $0, 0, 0, 0, 0, e^{12}a_1, -e^{16} + e^{23}, e^{26} + e^{13}(1 + a_1), e^{45} + e^{28} + e^{17} + e^{36}$ | 1579     |
| Type: 5211 |                                                                                                           |          |
| 9421:1     | $0, 0, 0, 0, 0, e^{12}, e^{34}, e^{16}, e^{18}$                                                           | 3679     |
| 9421:2     | $0, 0, 0, 0, 0, e^{12}, e^{13}, e^{16}, e^{18}$                                                           | 4679     |
| 9421:3     | $0, 0, 0, 0, 0, e^{12}, e^{13}, e^{26}, e^{28}$                                                           | 4679     |
| 9421:4     | $0, 0, 0, 0, 0, e^{12}, e^{34}, e^{16}, e^{18} + e^{35}$                                                  | 2679     |
| 9421:5     | $0, 0, 0, 0, 0, e^{12}, e^{45} + e^{13}, e^{16}, e^{18}$                                                  | 2679     |
| 9421:6     | $0, 0, 0, 0, 0, e^{12}, e^{13} + e^{45}, e^{26}, e^{28}$                                                  | 2679     |
| 9421:7     | $0, 0, 0, 0, 0, e^{12}, e^{13}, e^{16}, e^{34} + e^{18}$                                                  | 3679     |
| 9421:8     | $0, 0, 0, 0, 0, e^{12}, e^{13}, e^{26}, e^{34} + e^{28}$                                                  | 3679     |
| 9421:9     | $0, 0, 0, 0, 0, e^{12}, e^{24} + e^{13}, e^{16}, e^{18}$                                                  | 3679     |
| 9421:10    | $0, 0, 0, 0, 0, e^{12}, e^{34}, e^{16}, e^{18} + e^{23}$                                                  | 3679     |
| 9421:11    | $0, 0, 0, 0, 0, e^{12}, e^{13}, e^{16}, e^{45} + e^{18}$                                                  | 2679     |
| 9421:12    | $0, 0, 0, 0, 0, e^{12}, e^{13}, e^{26}, e^{28} + e^{45}$                                                  | 2679     |
| 9421:13    | $0, 0, 0, 0, 0, e^{12}, e^{34}, e^{16}, e^{25} + e^{18}$                                                  | 2679     |
| 9421:14    | $0, 0, 0, 0, 0, e^{12}, e^{45} + e^{13}, e^{16}, e^{18} + e^{34}$                                         | 2679     |
| 9421:15    | $0, 0, 0, 0, 0, e^{12}, e^{45} + e^{13}, e^{26}, e^{34} + e^{28}$                                         | 2679     |
| 9421:16    | $0, 0, 0, 0, 0, e^{12}, e^{13}, e^{16}, e^{23} + e^{18}$                                                  | 4679     |
| 9421:17    | $0, 0, 0, 0, 0, e^{12}, e^{13}, e^{16}, e^{24} + e^{18}$                                                  | 3679     |
| 9421:18    | $0, 0, 0, 0, 0, e^{12}, e^{13}, e^{26}, e^{14} + e^{28}$                                                  | 3679     |
| 9421:19a   | $0, 0, 0, 0, 0, e^{12}, e^{13} + e^{24}, e^{16}, e^{18} + e^{34}$                                         | 3679     |
| 9421:19b   | $0, 0, 0, 0, 0, -e^{12}, e^{13} + e^{24}, e^{16}, e^{18} + e^{34}$                                        | 3679     |
| 9421:20    | $0, 0, 0, 0, 0, e^{12}, e^{24} + e^{13}, e^{16}, e^{18} + e^{35}$                                         | 2679     |
| 9421:21    | $0, 0, 0, 0, 0, e^{12}, e^{14} + e^{23}, e^{16}, e^{18} + e^{35}$                                         | 2679     |
| 9421:22    | $0, 0, 0, 0, 0, e^{12}, e^{34}, e^{16}, e^{18} + e^{23} + e^{45}$                                         | 2679     |
| 9421:23    | $0, 0, 0, 0, 0, e^{12}, e^{13} + e^{45}, e^{16}, e^{18} + e^{23}$                                         | 2679     |
| 9421:24    | $0, 0, 0, 0, 0, e^{12}, e^{35} + e^{14}, e^{16}, e^{23} + e^{18}$                                         | 2679     |
| 9421:25    | $0, 0, 0, 0, 0, e^{12}, e^{35} + e^{14}, e^{26}, e^{28} + e^{13}$                                         | 2679     |
| 9421:26    | $0, 0, 0, 0, 0, e^{12}, e^{34}, e^{16}, e^{26} + e^{18}$                                                  | 3679     |
| 9421:27    | $0, 0, 0, 0, 0, e^{12}, e^{24} + e^{13}, e^{16}, e^{18} + e^{23}$                                         | 3679     |
| 9421:28    | $0, 0, 0, 0, 0, e^{12}, e^{13}, e^{16}, e^{18} + e^{45} + e^{23}$                                         | 2679     |
| 9421:29    | $0, 0, 0, 0, 0, e^{12}, e^{13}, e^{16}, e^{24} + e^{18} + e^{35}$                                         | 2679     |
| 9421:30    | $0, 0, 0, 0, 0, e^{12}, e^{13}, e^{26}, e^{28} + e^{14} + e^{35}$                                         | 2679     |
| 9421:31    | $0, 0, 0, 0, 0, e^{12}, e^{13} + e^{24}, e^{16}, e^{18} + e^{25}$                                         | 2679     |
| 9421:32    | $0, 0, 0, 0, 0, e^{12}, e^{13} + e^{45}, e^{16}, e^{35} + e^{24} + e^{18}$                                | 2679     |
| 9421:33a   | $0, 0, 0, 0, 0, e^{12}, e^{13} + e^{45}, e^{26}, e^{35} + e^{14} + e^{28}$                                | 2679     |
| 9421:33b   | $0, 0, 0, 0, 0, e^{12}, e^{45} - e^{13}, e^{26}, e^{28} + e^{35} + e^{14}$                                | 2679     |
| 9421:34    | $0, 0, 0, 0, 0, e^{12}, e^{13}, e^{16}, e^{26} + e^{18}$                                                  | 4679     |
| 9421:35    | $0, 0, 0, 0, 0, e^{12}, e^{13}, e^{26}, e^{16} + e^{28}$                                                  | 4679     |
| 9421:36    | $0, 0, 0, 0, 0, e^{12}, e^{34}, e^{16}, e^{18} + e^{26} + e^{35}$                                         | 2679     |
| 9421:37    | $0, 0, 0, 0, 0, e^{12}, e^{13} + e^{45}, e^{16}, e^{18} + e^{26}$                                         | 2679     |

Table 2 – Continued to next page

Table 2 – Continued from previous page

| Name     | $\mathfrak{g}$                                                                       | UCS Dim. |
|----------|--------------------------------------------------------------------------------------|----------|
| 9421:38  | $0, 0, 0, 0, 0, e^{12}, e^{45} + e^{13}, e^{26}, e^{28} + e^{16}$                    | 2679     |
| 9421:39  | $0, 0, 0, 0, 0, e^{12}, e^{24} + e^{13}, e^{16}, e^{23} + e^{45} + e^{18}$           | 2679     |
| 9421:40a | $0, 0, 0, 0, 0, e^{12}, e^{24} + e^{13}, e^{16}, e^{18} + e^{25} + e^{34}$           | 2679     |
| 9421:40b | $0, 0, 0, 0, 0, -e^{12}, e^{13} + e^{24}, e^{16}, e^{25} + e^{18} + e^{34}$          | 2679     |
| 9421:41  | $0, 0, 0, 0, 0, e^{12}, e^{13}, e^{16}, e^{18} + e^{37}$                             | 3579     |
| 9421:42  | $0, 0, 0, 0, 0, e^{12}, e^{13}, e^{26}, e^{28} + e^{37}$                             | 3579     |
| 9421:43  | $0, 0, 0, 0, 0, e^{12}, e^{13}, e^{16}, e^{18} + e^{26} + e^{34}$                    | 3679     |
| 9421:44  | $0, 0, 0, 0, 0, e^{12}, e^{13}, e^{26}, e^{34} + e^{28} + e^{16}$                    | 3679     |
| 9421:45  | $0, 0, 0, 0, 0, e^{12}, e^{13} + e^{24}, e^{16}, e^{18} + e^{26}$                    | 3679     |
| 9421:46  | $0, 0, 0, 0, 0, e^{12}, e^{13}, e^{16}, e^{45} + e^{18} + e^{26}$                    | 2679     |
| 9421:47  | $0, 0, 0, 0, 0, e^{12}, e^{13}, e^{26}, e^{16} + e^{28} + e^{45}$                    | 2679     |
| 9421:48  | $0, 0, 0, 0, 0, e^{12}, e^{45} + e^{13}, e^{16}, e^{18} + e^{34} + e^{26}$           | 2679     |
| 9421:49  | $0, 0, 0, 0, 0, e^{12}, e^{13} + e^{45}, e^{26}, e^{28} + e^{34} + e^{16}$           | 2679     |
| 9421:50  | $0, 0, 0, 0, 0, -e^{12}, e^{34}, e^{16} + e^{23}, e^{36} + e^{18}$                   | 3579     |
| 9421:51  | $0, 0, 0, 0, 0, -e^{12}, e^{34}, e^{16} + e^{25}, e^{18} + e^{56}$                   | 2579     |
| 9421:52  | $0, 0, 0, 0, 0, e^{12}, e^{13}, e^{26}, e^{28} + e^{17}$                             | 3579     |
| 9421:53  | $0, 0, 0, 0, 0, e^{12}, e^{34}, e^{16}, e^{18} + e^{37}$                             | 2479     |
| 9421:54a | $0, 0, 0, 0, 0, e^{12}, e^{13} + e^{24}, e^{16}, e^{26} + e^{18} + e^{34}$           | 3679     |
| 9421:54b | $0, 0, 0, 0, 0, -e^{12}, e^{24} + e^{13}, e^{16}, e^{18} + e^{26} + e^{34}$          | 3679     |
| 9421:55  | $0, 0, 0, 0, 0, e^{12}, e^{24} + e^{13}, e^{16}, e^{18} + e^{26} + e^{35}$           | 2679     |
| 9421:56  | $0, 0, 0, 0, 0, e^{12}, e^{14} + e^{23}, e^{16}, e^{18} + e^{26} + e^{35}$           | 2679     |
| 9421:57  | $0, 0, 0, 0, 0, e^{12}, e^{13}, e^{16}, e^{18} + e^{45} + e^{37}$                    | 1579     |
| 9421:58  | $0, 0, 0, 0, 0, e^{12}, e^{13}, e^{26}, e^{28} + e^{37} + e^{45}$                    | 1579     |
| 9421:59  | $0, 0, 0, 0, 0, -e^{12}, e^{13}, e^{16} + e^{23}, e^{36} + e^{18}$                   | 4579     |
| 9421:60  | $0, 0, 0, 0, 0, -e^{12}, e^{13}, e^{16} + e^{24}, e^{46} + e^{18}$                   | 3579     |
| 9421:61  | $0, 0, 0, 0, 0, e^{12}, e^{13}, e^{26} + e^{14}, e^{28} + e^{46}$                    | 3579     |
| 9421:62  | $0, 0, 0, 0, 0, -e^{12}, e^{34}, e^{23} + e^{16}, e^{36} + e^{45} + e^{18}$          | 2579     |
| 9421:63  | $0, 0, 0, 0, 0, -e^{12}, e^{45} + e^{13}, e^{16} + e^{23}, e^{18} + e^{36}$          | 2579     |
| 9421:64  | $0, 0, 0, 0, 0, -e^{12}, e^{35} + e^{14}, e^{16} + e^{23}, e^{18} + e^{36}$          | 2579     |
| 9421:65  | $0, 0, 0, 0, 0, e^{12}, e^{35} + e^{14}, e^{26} + e^{13}, e^{28} + e^{36}$           | 2579     |
| 9421:66  | $0, 0, 0, 0, 0, e^{12}, e^{13}, e^{16}, e^{37} + e^{18} + e^{24}$                    | 2579     |
| 9421:67  | $0, 0, 0, 0, 0, e^{12}, e^{13}, e^{26}, e^{14} + e^{28} + e^{37}$                    | 2579     |
| 9421:68  | $0, 0, 0, 0, 0, e^{12}, e^{13}, e^{26}, e^{28} + e^{17} + e^{34}$                    | 2579     |
| 9421:69  | $0, 0, 0, 0, 0, e^{12}, e^{13}, e^{26}, e^{17} + e^{28} + e^{45}$                    | 1579     |
| 9421:70  | $0, 0, 0, 0, 0, e^{12}, e^{34}, e^{16}, e^{18} + e^{47} + e^{35}$                    | 1479     |
| 9421:71  | $0, 0, 0, 0, 0, e^{12}, e^{13}, e^{23} + e^{16}, e^{27} + e^{18}$                    | 3579     |
| 9421:72  | $0, 0, 0, 0, 0, e^{12}, -e^{13}, e^{16} + e^{34}, e^{18} + e^{47}$                   | 2479     |
| 9421:73  | $0, 0, 0, 0, 0, -e^{12}, e^{24} + e^{13}, e^{23} + e^{16}, e^{36} + e^{18}$          | 3579     |
| 9421:74  | $0, 0, 0, 0, 0, e^{12}, e^{34}, e^{13} + e^{26}, e^{28} + e^{36} + e^{14}$           | 3579     |
| 9421:75  | $0, 0, 0, 0, 0, -e^{12}, e^{13}, e^{16} + e^{24}, e^{18} + e^{35} + e^{46}$          | 2579     |
| 9421:76  | $0, 0, 0, 0, 0, e^{12}, e^{13}, e^{14} + e^{26}, e^{46} + e^{28} + e^{35}$           | 2579     |
| 9421:77  | $0, 0, 0, 0, 0, -e^{12}, e^{24} + e^{13}, e^{16} + e^{25}, e^{56} + e^{18}$          | 2579     |
| 9421:78  | $0, 0, 0, 0, 0, e^{12}, e^{34}, e^{26} + e^{15}, e^{13} + e^{28} + e^{56}$           | 2579     |
| 9421:79  | $0, 0, 0, 0, 0, -e^{12}, e^{13}, e^{16} + e^{23}, e^{18} + e^{36} + e^{45}$          | 2579     |
| 9421:80  | $0, 0, 0, 0, 0, e^{12}, e^{34}, e^{26} + e^{13}, e^{28} + e^{15} + e^{36}$           | 2579     |
| 9421:81  | $0, 0, 0, 0, 0, -e^{12}, e^{35} + e^{14}, e^{23} + e^{16}, e^{36} + e^{45} + e^{18}$ | 2579     |
| 9421:82  | $0, 0, 0, 0, 0, e^{12}, e^{35} + e^{14}, e^{13} + e^{26}, e^{28} + e^{45} + e^{36}$  | 2579     |
| 9421:83  | $0, 0, 0, 0, 0, e^{12}, e^{34}, e^{16}, e^{18} + e^{47} + e^{23}$                    | 2479     |
| 9421:84  | $0, 0, 0, 0, 0, e^{12}, e^{34}, e^{16}, e^{25} + e^{18} + e^{37}$                    | 1479     |
| 9421:85a | $0, 0, 0, 0, 0, e^{12}, e^{13}, e^{16}, e^{37} + e^{18} + e^{26}$                    | 3579     |
| 9421:85b | $0, 0, 0, 0, 0, -e^{12}, e^{13}, e^{16}, e^{37} + e^{18} + e^{26}$                   | 3579     |
| 9421:86  | $0, 0, 0, 0, 0, e^{12}, e^{13}, e^{16}, e^{27} + e^{36} + e^{18}$                    | 3579     |
| 9421:87  | $0, 0, 0, 0, 0, e^{12}, e^{13}, e^{26}, e^{37} + e^{16} + e^{28}$                    | 3579     |
| 9421:88  | $0, 0, 0, 0, 0, -e^{12}, e^{13}, e^{16} + e^{24}, e^{46} + e^{18} + e^{23}$          | 3579     |
| 9421:89  | $0, 0, 0, 0, 0, -e^{12}, e^{13}, e^{16} + e^{23}, e^{24} + e^{36} + e^{18}$          | 3579     |
| 9421:90  | $0, 0, 0, 0, 0, e^{12}, e^{13}, e^{14} + e^{26}, e^{28} + e^{15} + e^{46}$           | 2579     |
| 9421:91  | $0, 0, 0, 0, 0, -e^{12}, e^{13}, e^{24} + e^{16}, e^{18} + e^{46} + e^{25}$          | 2579     |
| 9421:92  | $0, 0, 0, 0, 0, e^{12}, e^{13}, e^{23} + e^{16}, e^{18} + e^{34} + e^{27}$           | 2579     |

Table 2 – Continued to next page

Table 2 – Continued from previous page

| Name      | $\mathfrak{g}$                                                                                            | UCS Dim. |
|-----------|-----------------------------------------------------------------------------------------------------------|----------|
| 9421:93   | $0, 0, 0, 0, 0, e^{12}, e^{13}, e^{16} + e^{23}, e^{27} + e^{18} + e^{45}$                                | 1579     |
| 9421:94a  | $0, 0, 0, 0, 0, -e^{12}, e^{24} + e^{13}, e^{25} + e^{16}, e^{34} + e^{56} + e^{18}$                      | 2579     |
| 9421:94b  | $0, 0, 0, 0, 0, -e^{12}, e^{24} - e^{13}, e^{25} + e^{16}, e^{34} + e^{18} + e^{56}$                      | 2579     |
| 9421:95   | $0, 0, 0, 0, 0, e^{12}, -e^{13}, e^{34} + e^{16}, e^{47} + e^{18} + e^{35}$                               | 1479     |
| 9421:96   | $0, 0, 0, 0, 0, -e^{12}, e^{24} + e^{13}, e^{16} + e^{23}, e^{36} + e^{18} + e^{45}$                      | 2579     |
| 9421:97   | $0, 0, 0, 0, 0, e^{12}, e^{34} + e^{15}, e^{13} + e^{26}, e^{36} + e^{28} + e^{14}$                       | 2579     |
| 9421:98   | $0, 0, 0, 0, 0, -e^{12}, e^{45} + e^{13}, e^{16} + e^{23}, e^{18} + e^{24} + e^{36}$                      | 2579     |
| 9421:99   | $0, 0, 0, 0, 0, -e^{12}, e^{35} + e^{14}, e^{16} + e^{23}, e^{18} + e^{36} + e^{24}$                      | 2579     |
| 9421:100  | $0, 0, 0, 0, 0, -e^{12}, e^{15} + e^{34}, e^{16} + e^{23}, e^{24} + e^{36} + e^{18}$                      | 2579     |
| 9421:101  | $0, 0, 0, 0, 0, e^{12}, e^{14} + e^{23}, e^{34} + e^{16}, e^{37} + e^{18}$                                | 2479     |
| 9421:102  | $0, 0, 0, 0, 0, e^{12}, e^{34}, e^{16}, e^{37} + e^{18} + e^{26}$                                         | 2479     |
| 9421:103  | $0, 0, 0, 0, 0, e^{12}, -e^{13}, e^{34} + e^{16}, e^{18} + e^{47} + e^{23}$                               | 2479     |
| 9421:104a | $0, 0, 0, 0, 0, e^{12}, e^{13}, e^{16}, e^{26} + e^{37} + e^{45} + e^{18}$                                | 1579     |
| 9421:104b | $0, 0, 0, 0, 0, -e^{12}, e^{13}, e^{16}, e^{18} + e^{26} + e^{37} + e^{45}$                               | 1579     |
| 9421:105  | $0, 0, 0, 0, 0, e^{12}, e^{13}, e^{16}, e^{45} + e^{36} + e^{18} + e^{27}$                                | 1579     |
| 9421:106  | $0, 0, 0, 0, 0, e^{12}, e^{13}, e^{26}, e^{16} + e^{28} + e^{37} + e^{45}$                                | 1579     |
| 9421:107  | $0, 0, 0, 0, 0, e^{12}, -e^{13}, e^{34} + e^{16}, e^{18} + e^{47} + e^{25}$                               | 1479     |
| 9421:108  | $0, 0, 0, 0, 0, e^{12}, e^{14} + e^{23}, e^{26} + e^{15}, e^{13} + e^{56} + e^{28}$                       | 2579     |
| 9421:109  | $0, 0, 0, 0, 0, e^{12}, e^{23} + e^{14}, e^{26} + e^{13}, e^{15} + e^{28} + e^{36}$                       | 2579     |
| 9421:110  | $0, 0, 0, 0, 0, (-1 + a_2)e^{12}, e^{13}a_2, e^{23} + e^{16}, e^{18} + e^{27} + e^{36}$                   | 3579     |
| 9421:111  | $0, 0, 0, 0, 0, e^{12}, e^{35} + e^{14}, e^{34} + e^{16}, e^{18} + e^{37}$                                | 1379     |
| 9421:112  | $0, 0, 0, 0, 0, -e^{12}, e^{34}, e^{16} + e^{23}, e^{36} + e^{18} + e^{47}$                               | 2479     |
| 9421:113  | $0, 0, 0, 0, 0, e^{12}, e^{24} - e^{13}, e^{34} + e^{16}, e^{35} + e^{47} + e^{18}$                       | 1479     |
| 9421:114  | $0, 0, 0, 0, 0, e^{12}, e^{34}, e^{16}, e^{35} + e^{47} + e^{18} + e^{26}$                                | 1479     |
| 9421:115  | $0, 0, 0, 0, 0, e^{12}, e^{14} + e^{23}, e^{13} + e^{26}, e^{28} + e^{17}$                                | 2479     |
| 9421:116  | $0, 0, 0, 0, 0, e^{12}, -e^{13}, e^{16} + e^{34}, e^{18} + e^{26} + e^{47}$                               | 2479     |
| 9421:117  | $0, 0, 0, 0, 0, -e^{12}, e^{13}, e^{16} + e^{24}, e^{46} + e^{37} + e^{18}$                               | 2479     |
| 9421:118  | $0, 0, 0, 0, 0, e^{12}, e^{13}, e^{14} + e^{26}, e^{46} + e^{28} + e^{37}$                                | 2479     |
| 9421:119  | $0, 0, 0, 0, 0, e^{12}, -e^{13} + e^{24}, e^{34} + e^{16}, e^{18} + e^{47} + e^{23}$                      | 2479     |
| 9421:120  | $0, 0, 0, 0, 0, e^{12}, e^{14} + e^{23}, e^{34} + e^{16}, e^{37} + e^{18} + e^{25}$                       | 1479     |
| 9421:121  | $0, 0, 0, 0, 0, e^{12}(-1 + a_2), e^{13}a_2, e^{16} + e^{23}, e^{45} + e^{36} + e^{18} + e^{27}$          | 1579     |
| 9421:122  | $0, 0, 0, 0, 0, e^{12}, -e^{13} + e^{45}, e^{16} + e^{34}, e^{47} + e^{18} + e^{35}$                      | 1379     |
| 9421:123  | $0, 0, 0, 0, 0, e^{12}, e^{24} + e^{13}, e^{16}, e^{18} + e^{27} + e^{36}$                                | 2479     |
| 9421:124  | $0, 0, 0, 0, 0, e^{12}, e^{13}, e^{14} + e^{26}, e^{28} + e^{17} + e^{46}$                                | 2479     |
| 9421:125  | $0, 0, 0, 0, 0, -e^{12}, e^{34}, e^{16} + e^{25}, e^{56} + e^{37} + e^{18}$                               | 1379     |
| 9421:126a | $0, 0, 0, 0, 0, e^{12}, e^{14} + e^{23}, e^{13} + e^{26}, e^{34} + e^{17} + e^{28}$                       | 2479     |
| 9421:126b | $0, 0, 0, 0, 0, -e^{12}, e^{14} + e^{23}, e^{26} + e^{13}, e^{28} + e^{34} + e^{17}$                      | 2479     |
| 9421:127  | $0, 0, 0, 0, 0, e^{12}, e^{14} + e^{23}, e^{26} + e^{13}, e^{28} + e^{17} + e^{35}$                       | 1479     |
| 9421:128  | $0, 0, 0, 0, 0, e^{12}, e^{23} + e^{14}, e^{26} + e^{13}, e^{28} + e^{45} + e^{17}$                       | 1479     |
| 9421:129  | $0, 0, 0, 0, 0, e^{12}, -e^{13} + e^{45}, e^{16} + e^{34}, e^{23} + e^{47} + e^{18}$                      | 1379     |
| 9421:130  | $0, 0, 0, 0, 0, e^{12}, e^{35} + e^{14}, e^{16} + e^{34}, e^{18} + e^{37} + e^{25}$                       | 1379     |
| 9421:131  | $0, 0, 0, 0, 0, e^{12}, -e^{13}, e^{34} + e^{16}, e^{35} + e^{47} + e^{18} + e^{26}$                      | 1479     |
| 9421:132  | $0, 0, 0, 0, 0, e^{12}, e^{34}, e^{26} + e^{13}, e^{47} + e^{28} + e^{36} + e^{15}$                       | 1479     |
| 9421:133  | $0, 0, 0, 0, 0, e^{12}, e^{14} + e^{23}, e^{34} + e^{16}, e^{37} + e^{26} + e^{18}$                       | 2479     |
| 9421:134  | $0, 0, 0, 0, 0, e^{12}, e^{13} + e^{24}, e^{16}, e^{27} + e^{36} + e^{45} + e^{18}$                       | 1479     |
| 9421:135  | $0, 0, 0, 0, 0, e^{12}, e^{13}, e^{14} + e^{26}, e^{46} + e^{28} + e^{15} + e^{37}$                       | 1479     |
| 9421:136  | $0, 0, 0, 0, 0, e^{12}, e^{13}, e^{14} + e^{26}, e^{17} + e^{46} + e^{35} + e^{28}$                       | 1479     |
| 9421:137  | $0, 0, 0, 0, 0, -e^{12}, e^{13}, e^{16} + e^{24}, e^{25} + e^{37} + e^{18} + e^{46}$                      | 1479     |
| 9421:138  | $0, 0, 0, 0, 0, e^{12}(-1 + a_2), e^{23} + e^{14}, e^{26} + a_2e^{13}, e^{17} + e^{28} + e^{36}$          | 2479     |
| 9421:139  | $0, 0, 0, 0, 0, e^{12}, e^{14} + e^{35}, e^{16} + e^{34}, e^{18} + e^{26} + e^{37}$                       | 1379     |
| 9421:140  | $0, 0, 0, 0, 0, -e^{12}, -e^{13}, e^{16} + e^{35} + e^{24}, e^{57} + e^{18} + e^{46}$                     | 1379     |
| 9421:141  | $0, 0, 0, 0, 0, e^{12}, -e^{13} + e^{24}, e^{16} + e^{34}, e^{18} + e^{26} + e^{35} + e^{47}$             | 1479     |
| 9421:142  | $0, 0, 0, 0, 0, -e^{12}, e^{15} + e^{34}, e^{23} + e^{45} + e^{16}, e^{47} + e^{36} + e^{18}$             | 1379     |
| 9421:143  | $0, 0, 0, 0, 0, e^{12}, e^{34}, e^{26} + e^{15}, e^{28} + e^{47} + e^{56} + e^{13}$                       | 1379     |
| 9421:144  | $0, 0, 0, 0, 0, (-1 + a_2)e^{12}, e^{14} + e^{23}, e^{26} + e^{13}a_2, e^{28} + e^{17} + e^{36} + e^{45}$ | 1479     |
| 9421:145  | $0, 0, 0, 0, 0, e^{12}, e^{45} - e^{13}, e^{34} + e^{16}, e^{18} + e^{47} + e^{35} + e^{26}$              | 1379     |
| 9421:146  | $0, 0, 0, 0, 0, -e^{12}, e^{23} + e^{14}, e^{16} + e^{25} + e^{34}, e^{18} + e^{37} + e^{56}$             | 1379     |
| 9421:147  | $0, 0, 0, 0, 0, -e^{12}, -e^{13}, e^{16} + e^{24} + e^{35}, e^{23} + e^{57} + e^{18} + e^{46}$            | 1379     |

Table 2 – Continued to next page

Table 2 – Continued from previous page

| Name     | $\mathfrak{g}$                                                                                          | UCS Dim. |
|----------|---------------------------------------------------------------------------------------------------------|----------|
| 9421:148 | $0, 0, 0, 0, 0, -e^{12}, -e^{13} + e^{45}, e^{16} + e^{24} + e^{35}, e^{18} + e^{23} + e^{57} + e^{46}$ | 1379     |
| 9421:149 | $0, 0, 0, 0, 0, e^{12}, e^{24} + e^{13}, e^{34} + e^{26} + e^{15}, e^{56} + e^{28} + e^{37} + e^{14}$   | 1379     |
|          | Type: 522                                                                                               |          |
| 942:1    | $0, 0, 0, 0, 0, e^{12}, e^{13}, e^{16}, e^{26}$                                                         | 579      |
| 942:2    | $0, 0, 0, 0, 0, e^{12}, e^{34}, e^{16}, e^{26}$                                                         | 479      |
| 942:3    | $0, 0, 0, 0, 0, e^{12}, e^{13}, e^{26}, e^{16} + e^{23}$                                                | 579      |
| 942:4    | $0, 0, 0, 0, 0, e^{12}, e^{13}, e^{16}, e^{26} + e^{34}$                                                | 479      |
| 942:5    | $0, 0, 0, 0, 0, e^{12}, e^{13}, e^{26}, e^{16} + e^{34}$                                                | 479      |
| 942:6    | $0, 0, 0, 0, 0, e^{12}, e^{24} + e^{13}, e^{16}, e^{26}$                                                | 479      |
| 942:7    | $0, 0, 0, 0, 0, e^{12}, e^{34}, e^{16}, e^{13} + e^{26}$                                                | 479      |
| 942:8    | $0, 0, 0, 0, 0, e^{12}, e^{34}, e^{16}, e^{26} + e^{35}$                                                | 379      |
| 942:9    | $0, 0, 0, 0, 0, e^{12}, e^{45} + e^{13}, e^{16}, e^{26}$                                                | 379      |
| 942:10   | $0, 0, 0, 0, 0, e^{12}, e^{13}, e^{16}, e^{14} + e^{26}$                                                | 479      |
| 942:11   | $0, 0, 0, 0, 0, e^{12}, e^{13}, e^{26}, e^{16} + e^{24}$                                                | 479      |
| 942:12   | $0, 0, 0, 0, 0, e^{12}, e^{13}, e^{16}, e^{26} + e^{45}$                                                | 379      |
| 942:13   | $0, 0, 0, 0, 0, e^{12}, e^{13}, e^{26}, e^{45} + e^{16}$                                                | 379      |
| 942:14   | $0, 0, 0, 0, 0, e^{12}, e^{34}, e^{16}, e^{26} + e^{15}$                                                | 379      |
| 942:15   | $0, 0, 0, 0, 0, e^{12}, e^{24} + e^{13}, e^{16}, e^{26} + e^{34}$                                       | 479      |
| 942:16   | $0, 0, 0, 0, 0, e^{12}, e^{34}, e^{35} + e^{16}, e^{45} + e^{26}$                                       | 379      |
| 942:17   | $0, 0, 0, 0, 0, e^{12}, e^{13} + e^{45}, e^{16}, e^{26} + e^{34}$                                       | 379      |
| 942:18   | $0, 0, 0, 0, 0, e^{12}, e^{45} + e^{13}, e^{26}, e^{16} + e^{34}$                                       | 379      |
| 942:19   | $0, 0, 0, 0, 0, e^{12}, e^{13}, e^{16} + e^{23}, e^{26} + e^{34}$                                       | 479      |
| 942:20   | $0, 0, 0, 0, 0, e^{12}, e^{13}, e^{14} + e^{26}, e^{16} + e^{34}$                                       | 479      |
| 942:21   | $0, 0, 0, 0, 0, e^{12}, e^{13}, e^{16} + e^{24}, e^{34} + e^{26}$                                       | 479      |
| 942:22   | $0, 0, 0, 0, 0, e^{12}, e^{14} + e^{23}, e^{16}, e^{13} + e^{26}$                                       | 479      |
| 942:23a  | $0, 0, 0, 0, 0, e^{12}, e^{34}, e^{23} + e^{16}, e^{13} + e^{26}$                                       | 479      |
| 942:23b  | $0, 0, 0, 0, 0, e^{12}, e^{34}, -e^{16} + e^{23}, e^{13} + e^{26}$                                      | 479      |
| 942:24   | $0, 0, 0, 0, 0, e^{12}, e^{34}, e^{23} + e^{16}, e^{14} + e^{26}$                                       | 479      |
| 942:25   | $0, 0, 0, 0, 0, e^{12}, e^{13}, e^{34} + e^{16}, e^{26} + e^{35}$                                       | 379      |
| 942:26   | $0, 0, 0, 0, 0, e^{12}, e^{13}, e^{16} + e^{34}, e^{26} + e^{45}$                                       | 379      |
| 942:27   | $0, 0, 0, 0, 0, e^{12}, e^{13}, e^{26} + e^{34}, e^{45} + e^{16}$                                       | 379      |
| 942:28   | $0, 0, 0, 0, 0, e^{12}, e^{13} + e^{24}, e^{16}, e^{35} + e^{26}$                                       | 379      |
| 942:29   | $0, 0, 0, 0, 0, e^{12}, e^{14} + e^{23}, e^{16}, e^{35} + e^{26}$                                       | 379      |
| 942:30   | $0, 0, 0, 0, 0, e^{12}, e^{34}, e^{13} + e^{26}, e^{35} + e^{16}$                                       | 379      |
| 942:31   | $0, 0, 0, 0, 0, e^{12}, e^{34}, e^{16}, e^{45} + e^{13} + e^{26}$                                       | 379      |
| 942:32   | $0, 0, 0, 0, 0, e^{12}, e^{34}, e^{13} + e^{26}, e^{16} + e^{45}$                                       | 379      |
| 942:33   | $0, 0, 0, 0, 0, e^{12}, e^{34}, e^{26} + e^{15}, e^{16} + e^{35}$                                       | 379      |
| 942:34   | $0, 0, 0, 0, 0, e^{12}, e^{35} + e^{14}, e^{16}, e^{26} + e^{13}$                                       | 379      |
| 942:35   | $0, 0, 0, 0, 0, e^{12}, e^{45} + e^{13}, e^{26}, e^{16} + e^{23}$                                       | 379      |
| 942:36   | $0, 0, 0, 0, 0, e^{12}, e^{14} + e^{35}, e^{26}, e^{23} + e^{16}$                                       | 379      |
| 942:37   | $0, 0, 0, 0, 0, e^{12}, e^{13} + e^{45}, e^{16} + e^{34}, e^{35} + e^{26}$                              | 379      |
| 942:38   | $0, 0, 0, 0, 0, e^{12}, e^{13}, e^{23} + e^{16}, e^{14} + e^{26}$                                       | 479      |
| 942:39a  | $0, 0, 0, 0, 0, e^{12}, e^{13}, e^{24} + e^{16}, e^{26} + e^{14}$                                       | 479      |
| 942:39b  | $0, 0, 0, 0, 0, e^{12}, e^{13}, -e^{16} + e^{24}, e^{14} + e^{26}$                                      | 479      |
| 942:40   | $0, 0, 0, 0, 0, e^{12}, e^{13}, e^{16}, e^{14} + e^{26} + e^{35}$                                       | 379      |
| 942:41   | $0, 0, 0, 0, 0, e^{12}, e^{13}, e^{26}, e^{16} + e^{45} + e^{23}$                                       | 379      |
| 942:42   | $0, 0, 0, 0, 0, e^{12}, e^{13}, e^{26}, e^{16} + e^{24} + e^{35}$                                       | 379      |
| 942:43   | $0, 0, 0, 0, 0, e^{12}, e^{13}, e^{23} + e^{16}, e^{26} + e^{45}$                                       | 379      |
| 942:44   | $0, 0, 0, 0, 0, e^{12}, e^{13}, e^{26} + e^{14}, e^{35} + e^{16}$                                       | 379      |
| 942:45   | $0, 0, 0, 0, 0, e^{12}, e^{13}, e^{24} + e^{16}, e^{35} + e^{26}$                                       | 379      |
| 942:46   | $0, 0, 0, 0, 0, e^{12}, e^{13}, e^{26} + e^{14}, e^{45} + e^{16}$                                       | 379      |
| 942:47   | $0, 0, 0, 0, 0, e^{12}, e^{13}, e^{16} + e^{24}, e^{26} + e^{45}$                                       | 379      |
| 942:48   | $0, 0, 0, 0, 0, e^{12}, e^{24} + e^{13}, e^{16}, e^{26} + e^{15}$                                       | 379      |
| 942:49   | $0, 0, 0, 0, 0, e^{12}, e^{34}, e^{16} + e^{23}, e^{15} + e^{26}$                                       | 379      |
| 942:50a  | $0, 0, 0, 0, 0, e^{12}, e^{34}, e^{16} + e^{25}, e^{15} + e^{26}$                                       | 379      |
| 942:50b  | $0, 0, 0, 0, 0, e^{12}, e^{34}, e^{25} - e^{16}, e^{26} + e^{15}$                                       | 379      |
| 942:51   | $0, 0, 0, 0, 0, e^{12}, e^{23} + e^{14}, e^{26} + e^{13}, e^{34} + e^{16}$                              | 479      |
| 942:52   | $0, 0, 0, 0, 0, e^{12}, e^{24} + e^{13}, e^{16} + e^{34}, e^{35} + e^{26}$                              | 379      |

Table 2 – Continued to next page

Table 2 – Continued from previous page

| Name    | $\mathfrak{g}$                                                                          | UCS Dim. |
|---------|-----------------------------------------------------------------------------------------|----------|
| 942:53  | $0, 0, 0, 0, 0, e^{12}, e^{14} + e^{23}, e^{34} + e^{16}, e^{26} + e^{35}$              | 379      |
| 942:54a | $0, 0, 0, 0, 0, e^{12}, e^{13} + e^{24}, e^{35} + e^{16}, e^{45} + e^{26}$              | 379      |
| 942:54b | $0, 0, 0, 0, 0, e^{12}, -e^{13} + e^{24}, e^{35} + e^{16}, e^{26} + e^{45}$             | 379      |
| 942:55  | $0, 0, 0, 0, 0, e^{12}, e^{23} + e^{14}, a_1, e^{16} + e^{35}, e^{26} + e^{45}$         | 379      |
| 942:56  | $0, 0, 0, 0, 0, e^{12}, e^{34}, e^{16} + e^{35}, e^{13} + e^{26} + e^{45}$              | 379      |
| 942:57  | $0, 0, 0, 0, 0, e^{12}, e^{14} + e^{35}, e^{13} + e^{26}, e^{16} + e^{34}$              | 379      |
| 942:58  | $0, 0, 0, 0, 0, e^{12}, e^{13} + e^{45}, e^{23} + e^{16}, e^{26} + e^{34}$              | 379      |
| 942:59  | $0, 0, 0, 0, 0, e^{12}, e^{35} + e^{14}, e^{16} + e^{23}, e^{26} + e^{34}$              | 379      |
| 942:60a | $0, 0, 0, 0, 0, e^{12}, e^{13} + e^{45}, e^{16}, e^{14} + e^{26} + e^{35}$              | 379      |
| 942:60b | $0, 0, 0, 0, 0, e^{12}, e^{45} - e^{13}, e^{16}, e^{26} + e^{35} + e^{14}$              | 379      |
| 942:61  | $0, 0, 0, 0, 0, e^{12}, e^{45} + e^{13}, e^{26}, e^{16} + e^{35} + e^{24}$              | 379      |
| 942:62  | $0, 0, 0, 0, 0, e^{12}, e^{14} + e^{35}, e^{26} + e^{13}, e^{45} + e^{16}$              | 379      |
| 942:63a | $0, 0, 0, 0, 0, e^{12}, e^{14} + e^{35}, e^{23} + e^{16}, e^{26} + e^{45}$              | 379      |
| 942:63b | $0, 0, 0, 0, 0, e^{12}, e^{35} - e^{14}, e^{23} + e^{16}, e^{26} + e^{45}$              | 379      |
| 942:64  | $0, 0, 0, 0, 0, e^{12}, e^{13}, e^{24} + e^{16}, e^{15} + e^{26}$                       | 379      |
| 942:65  | $0, 0, 0, 0, 0, e^{12}, e^{24} + e^{13}, e^{16} + e^{23}, e^{26} + e^{14}$              | 479      |
| 942:66  | $0, 0, 0, 0, 0, e^{12}, e^{13}, e^{34} + e^{16}, e^{35} + e^{14} + e^{26}$              | 379      |
| 942:67  | $0, 0, 0, 0, 0, e^{12}, e^{13}, e^{26} + e^{34}, e^{45} + e^{23} + e^{16}$              | 379      |
| 942:68  | $0, 0, 0, 0, 0, e^{12}, e^{13}, e^{26} + e^{34}, e^{16} + e^{35} + e^{24}$              | 379      |
| 942:69  | $0, 0, 0, 0, 0, e^{12}, e^{14} + e^{23}, e^{26} + e^{13}, e^{16} + e^{35}$              | 379      |
| 942:70  | $0, 0, 0, 0, 0, e^{12}, e^{13} + e^{24}, e^{16}, e^{35} + e^{14} + e^{26}$              | 379      |
| 942:71  | $0, 0, 0, 0, 0, e^{12}, e^{24} + e^{13}, e^{16}, e^{34} + e^{26} + e^{15}$              | 379      |
| 942:72  | $0, 0, 0, 0, 0, e^{12}, e^{23} + e^{14}, e^{13} + e^{26}, e^{45} + e^{16}$              | 379      |
| 942:73a | $0, 0, 0, 0, 0, e^{12}, e^{34}, e^{13} + e^{26}, e^{45} + e^{16} + e^{23}$              | 379      |
| 942:73b | $0, 0, 0, 0, 0, e^{12}, e^{34}, -e^{13} + e^{26}, e^{23} + e^{16} + e^{45}$             | 379      |
| 942:74  | $0, 0, 0, 0, 0, e^{12}, e^{34}, e^{26} + e^{13}, e^{16} + e^{35} + e^{24}$              | 379      |
| 942:75  | $0, 0, 0, 0, 0, e^{12}, e^{24} + e^{13}, e^{16} + e^{34}, e^{15} + e^{26}$              | 379      |
| 942:76  | $0, 0, 0, 0, 0, e^{12}, e^{13}, e^{45} + e^{16}, e^{14} + e^{26} + e^{35}$              | 379      |
| 942:77  | $0, 0, 0, 0, 0, e^{12}, e^{13}, e^{45} + e^{26}, e^{35} + e^{16} + e^{24}$              | 379      |
| 942:78  | $0, 0, 0, 0, 0, e^{12}, e^{24} + e^{13}, e^{26} + e^{15}, e^{35} + e^{16}$              | 379      |
| 942:79  | $0, 0, 0, 0, 0, e^{12}, e^{23} + e^{14}, e^{15} + e^{26}, e^{35} + e^{16}$              | 379      |
| 942:80  | $0, 0, 0, 0, 0, e^{12}, e^{34}, e^{26} + e^{15}, e^{16} + e^{23} + e^{45}$              | 379      |
| 942:81a | $0, 0, 0, 0, 0, e^{12}, e^{35} + e^{14}, e^{23} + e^{16}, e^{13} + e^{26}$              | 379      |
| 942:81b | $0, 0, 0, 0, 0, e^{12}, e^{14} + e^{35}, e^{23} - e^{16}, e^{26} + e^{13}$              | 379      |
| 942:82  | $0, 0, 0, 0, 0, e^{12}, e^{45} + e^{13}, e^{16} + e^{23}, e^{26} + e^{14}$              | 379      |
| 942:83  | $0, 0, 0, 0, 0, e^{12}, e^{15} + e^{34}, e^{16} + e^{23}, e^{14} + e^{26}$              | 379      |
| 942:84a | $0, 0, 0, 0, 0, e^{12}, e^{45} + e^{13}, e^{34} + e^{16}, e^{35} + e^{14} + e^{26}$     | 379      |
| 942:84b | $0, 0, 0, 0, 0, e^{12}, -e^{13} + e^{45}, e^{16} + e^{34}, e^{14} + e^{35} + e^{26}$    | 379      |
| 942:85  | $0, 0, 0, 0, 0, e^{12}, e^{13} + e^{45}, e^{26} + e^{34}, e^{35} + e^{24} + e^{16}$     | 379      |
| 942:86  | $0, 0, 0, 0, 0, e^{12}, e^{13}, e^{16} + e^{23}, e^{26} + e^{35} + e^{14}$              | 379      |
| 942:87  | $0, 0, 0, 0, 0, e^{12}, e^{13}, e^{14} + e^{26}, e^{23} + e^{16} + e^{45}$              | 379      |
| 942:88a | $0, 0, 0, 0, 0, e^{12}, e^{13}, e^{26} + e^{14}, e^{16} + e^{35} + e^{24}$              | 379      |
| 942:88b | $0, 0, 0, 0, 0, e^{12}, e^{13}, e^{26} - e^{14}, e^{16} + e^{35} + e^{24}$              | 379      |
| 942:89  | $0, 0, 0, 0, 0, e^{12}, e^{13}, e^{14} + e^{26}, e^{16} + e^{25} + e^{34}$              | 379      |
| 942:90a | $0, 0, 0, 0, 0, e^{12}, e^{13}, e^{16} + e^{24}, e^{14} + e^{26} + e^{35}$              | 379      |
| 942:90b | $0, 0, 0, 0, 0, e^{12}, e^{13}, -e^{16} + e^{24}, e^{14} + e^{35} + e^{26}$             | 379      |
| 942:91  | $0, 0, 0, 0, 0, e^{12}, e^{13}, e^{24} + e^{16}, e^{15} + e^{26} + e^{34}$              | 379      |
| 942:92  | $0, 0, 0, 0, 0, e^{12}, e^{24} + e^{13}, e^{16} + e^{23}, e^{26} + e^{15}$              | 379      |
| 942:93a | $0, 0, 0, 0, 0, e^{12}, e^{13} + e^{24}, e^{25} + e^{16}, e^{26} + e^{15}$              | 379      |
| 942:93b | $0, 0, 0, 0, 0, e^{12}, e^{13} + e^{24}, -e^{16} + e^{25}, e^{26} + e^{15}$             | 379      |
| 942:94  | $0, 0, 0, 0, 0, e^{12}, e^{24} + e^{13}, e^{16} + e^{34}, e^{26} + e^{35} + e^{14}$     | 379      |
| 942:95  | $0, 0, 0, 0, 0, e^{12}, e^{24} + e^{13}, e^{16} + e^{35}, e^{15} + e^{26} + e^{34}$     | 379      |
| 942:96  | $0, 0, 0, 0, 0, e^{12}, a_1 e^{14} + e^{23}, e^{16} + e^{35}, e^{13} + e^{26} + e^{45}$ | 379      |
| 942:97  | $0, 0, 0, 0, 0, e^{12}, e^{23} + e^{14}, e^{35} + e^{16}, e^{15} + e^{26} + e^{34}$     | 379      |
| 942:98  | $0, 0, 0, 0, 0, e^{12}, e^{34}, e^{24} + e^{35} + e^{16}, e^{45} + e^{13} + e^{26}$     | 379      |
| 942:99a | $0, 0, 0, 0, 0, e^{12}, e^{14} + e^{35}, e^{13} + e^{26}, e^{23} + e^{16} + e^{45}$     | 379      |
| 942:99b | $0, 0, 0, 0, 0, e^{12}, e^{35} + e^{14}, e^{26} - e^{13}, e^{16} + e^{45} + e^{23}$     | 379      |
| 942:100 | $0, 0, 0, 0, 0, e^{12}, e^{35} + e^{14}, e^{26} + e^{13}, e^{16} + e^{25} + e^{34}$     | 379      |

Table 2 – Continued to next page



Table 2 – Continued from previous page

| Name     | $\mathfrak{g}$                                                                                   | UCS Dim. |
|----------|--------------------------------------------------------------------------------------------------|----------|
| 942:101a | $0, 0, 0, 0, 0, e^{12}, e^{13} + e^{45}, e^{16} + e^{23}, e^{14} + e^{26} + e^{35}$              | 379      |
| 942:101b | $0, 0, 0, 0, 0, e^{12}, e^{45} - e^{13}, e^{23} + e^{16}, e^{35} + e^{14} + e^{26}$              | 379      |
| 942:102a | $0, 0, 0, 0, 0, e^{12}, e^{14} + e^{35}, e^{16} + e^{23}, e^{13} + e^{26} + e^{45}$              | 379      |
| 942:102b | $0, 0, 0, 0, 0, e^{12}, e^{35} + e^{14}, e^{23} - e^{16}, e^{13} + e^{45} + e^{26}$              | 379      |
| 942:102c | $0, 0, 0, 0, 0, e^{12}, e^{35} - e^{14}, e^{16} + e^{23}, e^{13} + e^{26} + e^{45}$              | 379      |
| 942:102d | $0, 0, 0, 0, 0, e^{12}, e^{35} - e^{14}, e^{23} - e^{16}, e^{45} + e^{13} + e^{26}$              | 379      |
| 942:103a | $0, 0, 0, 0, 0, e^{12}, e^{14} + e^{35}, e^{23} + e^{16}, e^{26} + e^{15} + e^{34}$              | 379      |
| 942:103b | $0, 0, 0, 0, 0, e^{12}, e^{35} - e^{14}, e^{16} + e^{23}, e^{15} + e^{26} + e^{34}$              | 379      |
| 942:104  | $0, 0, 0, 0, 0, e^{12}, e^{14} + e^{23}, e^{26} + e^{13}, e^{16} + e^{24} + e^{35}$              | 379      |
| 942:105  | $0, 0, 0, 0, 0, e^{12}, e^{14} + e^{23}, e^{13} + e^{26}, e^{34} + e^{25} + e^{16}$              | 379      |
| 942:106  | $0, 0, 0, 0, 0, e^{12}, e^{13}, e^{16} + e^{23} + e^{45}, e^{14} + e^{35} + e^{26}$              | 379      |
| 942:107  | $0, 0, 0, 0, 0, e^{12}, e^{13}, e^{16} + e^{25} + e^{34}, e^{35} + e^{14} + e^{26}$              | 379      |
| 942:108  | $0, 0, 0, 0, 0, e^{12}, e^{24} + e^{13}, e^{26} + e^{15}, e^{45} + e^{16} + e^{23}$              | 379      |
| 942:109a | $0, 0, 0, 0, 0, e^{12}, e^{13} + e^{24}, e^{26} + e^{15}, e^{25} + e^{16} + e^{34}$              | 379      |
| 942:109b | $0, 0, 0, 0, 0, e^{12}, e^{24} + e^{13}, e^{26} - e^{15}, e^{16} + e^{34} + e^{25}$              | 379      |
| 942:110a | $0, 0, 0, 0, 0, e^{12}, e^{45} + e^{13}, e^{16} + e^{25} + e^{34}, e^{26} + e^{35} + e^{14}$     | 379      |
| 942:110b | $0, 0, 0, 0, 0, e^{12}, -e^{13} + e^{45}, e^{16} + e^{25} + e^{34}, e^{14} + e^{26} + e^{35}$    | 379      |
| 942:111  | $0, 0, 0, 0, 0, e^{12}, a_1 e^{13} + e^{24}, e^{23} + e^{16} + e^{45}, e^{14} + e^{26} + e^{35}$ | 379      |
| 942:112  | $0, 0, 0, 0, 0, e^{12}, e^{24} + e^{13}, e^{16} + e^{25} + e^{34}, e^{35} + e^{14} + e^{26}$     | 379      |
| 942:113  | $0, 0, 0, 0, 0, e^{12}, e^{13}, e^{16}, e^{17}$                                                  | 469      |
| 942:114  | $0, 0, 0, 0, 0, e^{12}, e^{13}, e^{26}, e^{17}$                                                  | 469      |
| 942:115  | $0, 0, 0, 0, 0, e^{12}, e^{13}, e^{26}, e^{37}$                                                  | 469      |
| 942:116  | $0, 0, 0, 0, 0, e^{12}, e^{13}, e^{16}, e^{17} + e^{23}$                                         | 469      |
| 942:117  | $0, 0, 0, 0, 0, e^{12}, e^{13}, e^{26}, e^{17} + e^{23}$                                         | 469      |
| 942:118  | $0, 0, 0, 0, 0, e^{12}, e^{13}, e^{16}, e^{17} + e^{24}$                                         | 369      |
| 942:119  | $0, 0, 0, 0, 0, e^{12}, e^{13}, e^{26}, e^{24} + e^{17}$                                         | 369      |
| 942:120  | $0, 0, 0, 0, 0, e^{12}, e^{13}, e^{16}, e^{37} + e^{14}$                                         | 369      |
| 942:121  | $0, 0, 0, 0, 0, e^{12}, e^{13}, e^{16}, e^{34} + e^{17}$                                         | 369      |
| 942:122  | $0, 0, 0, 0, 0, e^{12}, e^{13}, e^{16}, e^{37} + e^{24}$                                         | 369      |
| 942:123  | $0, 0, 0, 0, 0, e^{12}, e^{13}, e^{26}, e^{37} + e^{14}$                                         | 369      |
| 942:124  | $0, 0, 0, 0, 0, e^{12}, e^{13}, e^{26}, e^{17} + e^{34}$                                         | 369      |
| 942:125  | $0, 0, 0, 0, 0, e^{12}, e^{13}, e^{26}, e^{24} + e^{37}$                                         | 369      |
| 942:126  | $0, 0, 0, 0, 0, e^{12}, e^{13}, e^{16}, e^{45} + e^{17}$                                         | 269      |
| 942:127  | $0, 0, 0, 0, 0, e^{12}, e^{13}, e^{26}, e^{45} + e^{17}$                                         | 269      |
| 942:128  | $0, 0, 0, 0, 0, e^{12}, e^{13}, e^{16}, e^{37} + e^{45}$                                         | 269      |
| 942:129  | $0, 0, 0, 0, 0, e^{12}, e^{13}, e^{26}, e^{37} + e^{45}$                                         | 269      |
| 942:130  | $0, 0, 0, 0, 0, e^{12}, e^{13}, e^{16}, e^{17} + e^{26}$                                         | 469      |
| 942:131a | $0, 0, 0, 0, 0, e^{12}, e^{13}, e^{16}, e^{26} + e^{37}$                                         | 469      |
| 942:131b | $0, 0, 0, 0, 0, -e^{12}, e^{13}, e^{16}, e^{26} + e^{37}$                                        | 469      |
| 942:132  | $0, 0, 0, 0, 0, e^{12}, e^{13}, e^{16}, e^{36} + e^{27}$                                         | 469      |
| 942:133  | $0, 0, 0, 0, 0, e^{12}, e^{13}, e^{26}, e^{16} + e^{37}$                                         | 469      |
| 942:134  | $0, 0, 0, 0, 0, e^{12}, e^{13}, e^{26}, e^{36} + e^{27}$                                         | 469      |
| 942:135  | $0, 0, 0, 0, 0, e^{12}, e^{13}, e^{14} + e^{26}, e^{24} + e^{17}$                                | 369      |
| 942:136a | $0, 0, 0, 0, 0, e^{12}, e^{13}, e^{16} + e^{24}, e^{37} + e^{14}$                                | 369      |
| 942:136b | $0, 0, 0, 0, 0, -e^{12}, e^{13}, e^{16} + e^{24}, e^{37} + e^{14}$                               | 369      |
| 942:137  | $0, 0, 0, 0, 0, e^{12}, a_1 e^{13}, e^{16} + e^{24}, e^{17} + e^{34}$                            | 369      |
| 942:138  | $0, 0, 0, 0, 0, e^{12}, e^{13}, e^{14} + e^{26}, e^{24} + e^{37}$                                | 369      |
| 942:139a | $0, 0, 0, 0, 0, e^{12}, e^{13}, e^{16} + e^{34}, e^{24} + e^{17}$                                | 369      |
| 942:139b | $0, 0, 0, 0, 0, -e^{12}, e^{13}, e^{34} + e^{16}, e^{24} + e^{17}$                               | 369      |
| 942:140  | $0, 0, 0, 0, 0, e^{12}, e^{13}, e^{34} + e^{26}, e^{17} + e^{24}$                                | 369      |
| 942:141  | $0, 0, 0, 0, 0, e^{12}, e^{13}, e^{26} + e^{34}, e^{37} + e^{24}$                                | 369      |
| 942:142  | $0, 0, 0, 0, 0, e^{12}, e^{13}, e^{26} + e^{14}, e^{17} + e^{45}$                                | 269      |
| 942:143  | $0, 0, 0, 0, 0, e^{12}, e^{13}, e^{16} + e^{24}, e^{17} + e^{45}$                                | 269      |
| 942:144  | $0, 0, 0, 0, 0, e^{12}, e^{13}, e^{14} + e^{26}, e^{45} + e^{37}$                                | 269      |
| 942:145  | $0, 0, 0, 0, 0, e^{12}, e^{13}, e^{24} + e^{16}, e^{37} + e^{45}$                                | 269      |
| 942:146  | $0, 0, 0, 0, 0, e^{12}, e^{13}, e^{16} + e^{34}, e^{45} + e^{17}$                                | 269      |
| 942:147  | $0, 0, 0, 0, 0, e^{12}, e^{13}, e^{26} + e^{34}, e^{45} + e^{17}$                                | 269      |
| 942:148  | $0, 0, 0, 0, 0, e^{12}, e^{13}, e^{16} + e^{34}, e^{37} + e^{45}$                                | 269      |

Table 2 – Continued to next page

Table 2 – Continued from previous page

| Name     | $\mathfrak{g}$                                                     | UCS Dim. |
|----------|--------------------------------------------------------------------|----------|
| 942:149  | $0, 0, 0, 0, 0, e^{12}, e^{13}, e^{26} + e^{34}, e^{37} + e^{45}$  | 269      |
| 942:150  | $0, 0, 0, 0, 0, e^{12}, e^{13}, e^{16} + e^{23}, e^{17} + e^{24}$  | 369      |
| 942:151  | $0, 0, 0, 0, 0, e^{12}, e^{13}, e^{16} + e^{23}, e^{14} + e^{37}$  | 369      |
| 942:152  | $0, 0, 0, 0, 0, e^{12}, e^{13}, e^{23} + e^{16}, e^{34} + e^{17}$  | 369      |
| 942:153  | $0, 0, 0, 0, 0, e^{12}, e^{13}, e^{23} + e^{16}, e^{24} + e^{37}$  | 369      |
| 942:154  | $0, 0, 0, 0, 0, e^{12}, e^{13}, e^{16}, e^{37} + e^{14} + e^{25}$  | 269      |
| 942:155  | $0, 0, 0, 0, 0, e^{12}, e^{13}, e^{16}, e^{17} + e^{23} + e^{45}$  | 269      |
| 942:156  | $0, 0, 0, 0, 0, e^{12}, e^{13}, e^{16}, e^{17} + e^{35} + e^{24}$  | 269      |
| 942:157  | $0, 0, 0, 0, 0, e^{12}, e^{13}, e^{26}, e^{14} + e^{37} + e^{25}$  | 269      |
| 942:158  | $0, 0, 0, 0, 0, e^{12}, e^{13}, e^{26}, e^{17} + e^{45} + e^{23}$  | 269      |
| 942:159  | $0, 0, 0, 0, 0, e^{12}, e^{13}, e^{26}, e^{17} + e^{24} + e^{35}$  | 269      |
| 942:160  | $0, 0, 0, 0, 0, e^{12}, e^{13}, e^{23} + e^{16}, e^{17} + e^{45}$  | 269      |
| 942:161  | $0, 0, 0, 0, 0, e^{12}, e^{13}, e^{16} + e^{23}, e^{37} + e^{45}$  | 269      |
| 942:162  | $0, 0, 0, 0, 0, e^{12}, e^{13}, e^{14} + e^{26}, e^{17} + e^{25}$  | 269      |
| 942:163  | $0, 0, 0, 0, 0, e^{12}, e^{13}, e^{24} + e^{16}, e^{25} + e^{17}$  | 269      |
| 942:164  | $0, 0, 0, 0, 0, e^{12}, e^{13}, e^{14} + e^{26}, e^{37} + e^{15}$  | 269      |
| 942:165  | $0, 0, 0, 0, 0, e^{12}, e^{13}, e^{16} + e^{24}, e^{37} + e^{15}$  | 269      |
| 942:166  | $0, 0, 0, 0, 0, e^{12}, e^{13}, e^{16} + e^{24}, e^{17} + e^{35}$  | 269      |
| 942:167  | $0, 0, 0, 0, 0, e^{12}, e^{13}, e^{14} + e^{26}, e^{25} + e^{37}$  | 269      |
| 942:168  | $0, 0, 0, 0, 0, e^{12}, e^{13}, e^{16} + e^{24}, e^{25} + e^{37}$  | 269      |
| 942:169  | $0, 0, 0, 0, 0, e^{12}, e^{13}, e^{34} + e^{16}, e^{25} + e^{17}$  | 269      |
| 942:170  | $0, 0, 0, 0, 0, e^{12}, e^{13}, e^{26} + e^{34}, e^{17} + e^{25}$  | 269      |
| 942:171  | $0, 0, 0, 0, 0, e^{12}, e^{13}, e^{26} + e^{34}, e^{25} + e^{37}$  | 269      |
| 942:172  | $0, 0, 0, 0, 0, e^{12}, e^{13}, e^{23} + e^{16}, e^{17} + e^{26}$  | 469      |
| 942:173a | $0, 0, 0, 0, 0, e^{12}, e^{13}, e^{23} + e^{16}, e^{26} + e^{37}$  | 469      |
| 942:173b | $0, 0, 0, 0, 0, -e^{12}, e^{13}, e^{16} + e^{23}, e^{26} + e^{37}$ | 469      |
| 942:174  | $0, 0, 0, 0, 0, e^{12}, e^{13}, e^{16} + e^{23}, e^{36} + e^{27}$  | 469      |
| 942:175a | $0, 0, 0, 0, 0, e^{12}, e^{13}, e^{16}, e^{26} + e^{37} + e^{14}$  | 369      |
| 942:175b | $0, 0, 0, 0, 0, -e^{12}, e^{13}, e^{16}, e^{37} + e^{14} + e^{26}$ | 369      |
| 942:176  | $0, 0, 0, 0, 0, e^{12}, e^{13}, e^{16}, e^{36} + e^{27} + e^{14}$  | 369      |
| 942:177  | $0, 0, 0, 0, 0, e^{12}, e^{13}, e^{16}, e^{17} + e^{26} + e^{34}$  | 369      |
| 942:178  | $0, 0, 0, 0, 0, e^{12}, e^{13}, e^{26}, e^{16} + e^{37} + e^{24}$  | 369      |
| 942:179  | $0, 0, 0, 0, 0, e^{12}, e^{13}, e^{26}, e^{14} + e^{36} + e^{27}$  | 369      |
| 942:180  | $0, 0, 0, 0, 0, e^{12}, e^{13}, e^{16} + e^{24}, e^{17} + e^{26}$  | 369      |
| 942:181  | $0, 0, 0, 0, 0, e^{12}, e^{13}, e^{14} + e^{26}, e^{37} + e^{16}$  | 369      |
| 942:182a | $0, 0, 0, 0, 0, e^{12}, e^{13}, e^{24} + e^{16}, e^{37} + e^{26}$  | 369      |
| 942:182b | $0, 0, 0, 0, 0, -e^{12}, e^{13}, e^{16} + e^{24}, e^{37} + e^{26}$ | 369      |
| 942:183  | $0, 0, 0, 0, 0, e^{12}, e^{13}, e^{14} + e^{26}, e^{27} + e^{36}$  | 369      |
| 942:184  | $0, 0, 0, 0, 0, e^{12}, e^{13}, e^{16} + e^{24}, e^{36} + e^{27}$  | 369      |
| 942:185  | $0, 0, 0, 0, 0, e^{12}, e^{13}, e^{16} + e^{34}, e^{17} + e^{26}$  | 369      |
| 942:186a | $0, 0, 0, 0, 0, e^{12}, e^{13}, e^{16} + e^{34}, e^{37} + e^{26}$  | 369      |
| 942:186b | $0, 0, 0, 0, 0, -e^{12}, e^{13}, e^{34} + e^{16}, e^{37} + e^{26}$ | 369      |
| 942:187  | $0, 0, 0, 0, 0, e^{12}, e^{13}, e^{16} + e^{34}, e^{27} + e^{36}$  | 369      |
| 942:188  | $0, 0, 0, 0, 0, e^{12}, e^{13}, e^{26} + e^{34}, e^{16} + e^{37}$  | 369      |
| 942:189  | $0, 0, 0, 0, 0, e^{12}, e^{13}, e^{26} + e^{34}, e^{36} + e^{27}$  | 369      |
| 942:190  | $0, 0, 0, 0, 0, e^{12}, e^{13}, e^{16}, e^{17} + e^{26} + e^{45}$  | 269      |
| 942:191a | $0, 0, 0, 0, 0, e^{12}, e^{13}, e^{16}, e^{37} + e^{45} + e^{26}$  | 269      |
| 942:191b | $0, 0, 0, 0, 0, -e^{12}, e^{13}, e^{16}, e^{37} + e^{26} + e^{45}$ | 269      |
| 942:192  | $0, 0, 0, 0, 0, e^{12}, e^{13}, e^{16}, e^{27} + e^{45} + e^{36}$  | 269      |
| 942:193  | $0, 0, 0, 0, 0, e^{12}, e^{13}, e^{26}, e^{16} + e^{37} + e^{45}$  | 269      |
| 942:194  | $0, 0, 0, 0, 0, e^{12}, e^{13}, e^{26}, e^{36} + e^{27} + e^{45}$  | 269      |
| 942:195  | $0, 0, 0, 0, 0, e^{12}, e^{13}, e^{45} + e^{16}, e^{26} + e^{17}$  | 269      |
| 942:196a | $0, 0, 0, 0, 0, e^{12}, e^{13}, e^{45} + e^{16}, e^{37} + e^{26}$  | 269      |
| 942:196b | $0, 0, 0, 0, 0, -e^{12}, e^{13}, e^{45} + e^{16}, e^{37} + e^{26}$ | 269      |
| 942:197  | $0, 0, 0, 0, 0, e^{12}, e^{13}, e^{16} + e^{45}, e^{27} + e^{36}$  | 269      |
| 942:198  | $0, 0, 0, 0, 0, e^{12}, e^{13}, e^{26} + e^{45}, e^{16} + e^{37}$  | 269      |
| 942:199  | $0, 0, 0, 0, 0, e^{12}, e^{13}, e^{26} + e^{45}, e^{36} + e^{27}$  | 269      |
| 942:200  | $0, 0, 0, 0, 0, e^{12}, e^{13}, e^{17} + e^{26}, e^{16} + e^{37}$  | 469      |

Table 2 – Continued to next page

Table 2 – Continued from previous page

| Name     | $\mathfrak{g}$                                                                | UCS Dim. |
|----------|-------------------------------------------------------------------------------|----------|
| 942:201  | $0, 0, 0, 0, 0, e^{12}, e^{13}, e^{17} + e^{26}, e^{36} + e^{27}$             | 469      |
| 942:202a | $0, 0, 0, 0, 0, e^{12}, e^{13}, e^{27} + e^{36}, e^{37} + e^{26}$             | 469      |
| 942:202b | $0, 0, 0, 0, 0, -e^{12}, e^{13}, e^{36} - e^{27}, e^{37} + e^{26}$            | 469      |
| 942:203  | $0, 0, 0, 0, 0, e^{12}, e^{13}, e^{45} + e^{16}, e^{37} + e^{25} + e^{14}$    | 269      |
| 942:204  | $0, 0, 0, 0, 0, e^{12}, e^{13}, e^{16} + e^{45}, e^{17} + e^{35} + e^{24}$    | 269      |
| 942:205  | $0, 0, 0, 0, 0, e^{12}, e^{13}, e^{45} + e^{26}, e^{37} + e^{14} + e^{25}$    | 269      |
| 942:206  | $0, 0, 0, 0, 0, e^{12}, e^{13}, e^{45} + e^{26}, e^{24} + e^{35} + e^{17}$    | 269      |
| 942:207  | $0, 0, 0, 0, 0, e^{12}, e^{13}, e^{14} + e^{26}, e^{37} + e^{15} + e^{24}$    | 269      |
| 942:208  | $0, 0, 0, 0, 0, e^{12}, e^{13}, e^{26} + e^{14}, e^{17} + e^{45} + e^{23}$    | 269      |
| 942:209  | $0, 0, 0, 0, 0, e^{12}, e^{13}, e^{26} + e^{14}, e^{17} + e^{35} + e^{24}$    | 269      |
| 942:210a | $0, 0, 0, 0, 0, e^{12}, e^{13}, e^{14} + e^{26}, e^{17} + e^{25} + e^{34}$    | 269      |
| 942:210b | $0, 0, 0, 0, 0, -e^{12}, e^{13}, e^{14} + e^{26}, e^{17} + e^{25} + e^{34}$   | 269      |
| 942:211a | $0, 0, 0, 0, 0, e^{12}, e^{13}, e^{24} + e^{16}, e^{25} + e^{37} + e^{14}$    | 269      |
| 942:211b | $0, 0, 0, 0, 0, -e^{12}, e^{13}, e^{24} + e^{16}, e^{37} + e^{14} + e^{25}$   | 269      |
| 942:212  | $0, 0, 0, 0, 0, e^{12}, e^{13}, e^{24} + e^{16}, e^{17} + e^{23} + e^{45}$    | 269      |
| 942:213  | $0, 0, 0, 0, 0, e^{12}a_1, e^{13}, e^{16} + e^{24}, e^{17} + e^{34} + e^{25}$ | 269      |
| 942:214  | $0, 0, 0, 0, 0, e^{12}, e^{13}, e^{16} + e^{34}, e^{25} + e^{37} + e^{14}$    | 269      |
| 942:215  | $0, 0, 0, 0, 0, e^{12}, e^{13}, e^{16} + e^{34}, e^{15} + e^{24} + e^{37}$    | 269      |
| 942:216  | $0, 0, 0, 0, 0, e^{12}, e^{13}, e^{34} + e^{16}, e^{45} + e^{17} + e^{23}$    | 269      |
| 942:217a | $0, 0, 0, 0, 0, e^{12}, e^{13}, e^{34} + e^{16}, e^{35} + e^{24} + e^{17}$    | 269      |
| 942:217b | $0, 0, 0, 0, 0, -e^{12}, e^{13}, e^{16} + e^{34}, e^{35} + e^{24} + e^{17}$   | 269      |
| 942:218  | $0, 0, 0, 0, 0, e^{12}, e^{13}, e^{26} + e^{34}, e^{25} + e^{37} + e^{14}$    | 269      |
| 942:219  | $0, 0, 0, 0, 0, e^{12}, e^{13}, e^{26} + e^{34}, e^{37} + e^{15} + e^{24}$    | 269      |
| 942:220  | $0, 0, 0, 0, 0, e^{12}, e^{13}, e^{26} + e^{34}, e^{17} + e^{45} + e^{23}$    | 269      |
| 942:221  | $0, 0, 0, 0, 0, e^{12}, e^{13}, e^{26} + e^{34}, e^{17} + e^{35} + e^{24}$    | 269      |
| 942:222a | $0, 0, 0, 0, 0, e^{12}, e^{13}, e^{14} + e^{26}, e^{16} + e^{24} + e^{37}$    | 369      |
| 942:222b | $0, 0, 0, 0, 0, e^{12}, e^{13}, -e^{14} + e^{26}, e^{37} + e^{16} + e^{24}$   | 369      |
| 942:223a | $0, 0, 0, 0, 0, e^{12}, e^{13}, e^{16} + e^{24}, e^{14} + e^{26} + e^{37}$    | 369      |
| 942:223b | $0, 0, 0, 0, 0, e^{12}, e^{13}, e^{24} - e^{16}, e^{37} + e^{14} + e^{26}$    | 369      |
| 942:223c | $0, 0, 0, 0, 0, -e^{12}, e^{13}, e^{24} + e^{16}, e^{37} + e^{26} + e^{14}$   | 369      |
| 942:223d | $0, 0, 0, 0, 0, -e^{12}, e^{13}, -e^{16} + e^{24}, e^{37} + e^{14} + e^{26}$  | 369      |
| 942:224  | $0, 0, 0, 0, 0, e^{12}, e^{13}, e^{16} + e^{24}, e^{14} + e^{27} + e^{36}$    | 369      |
| 942:225  | $0, 0, 0, 0, 0, a_1e^{12}, e^{13}, e^{16} + e^{24}, e^{17} + e^{26} + e^{34}$ | 369      |
| 942:226a | $0, 0, 0, 0, 0, e^{12}, e^{13}, e^{16} + e^{34}, e^{14} + e^{26} + e^{37}$    | 369      |
| 942:226b | $0, 0, 0, 0, 0, -e^{12}, e^{13}, e^{16} + e^{34}, e^{37} + e^{14} + e^{26}$   | 369      |
| 942:227a | $0, 0, 0, 0, 0, e^{12}, e^{13}, e^{34} + e^{16}, e^{36} + e^{27} + e^{14}$    | 369      |
| 942:227b | $0, 0, 0, 0, 0, e^{12}, e^{13}, -e^{16} + e^{34}, e^{27} + e^{36} + e^{14}$   | 369      |
| 942:228  | $0, 0, 0, 0, 0, e^{12}, e^{13}, e^{26} + e^{34}, e^{16} + e^{24} + e^{37}$    | 369      |
| 942:229  | $0, 0, 0, 0, 0, e^{12}, e^{13}, e^{26} + e^{34}, e^{27} + e^{14} + e^{36}$    | 369      |
| 942:230  | $0, 0, 0, 0, 0, e^{12}, e^{13}, e^{24} + e^{16}, e^{45} + e^{17} + e^{26}$    | 269      |
| 942:231  | $0, 0, 0, 0, 0, e^{12}, e^{13}, e^{26} + e^{14}, e^{37} + e^{16} + e^{45}$    | 269      |
| 942:232  | $0, 0, 0, 0, 0, e^{12}, e^{13}, e^{14} + e^{26}, e^{27} + e^{45} + e^{36}$    | 269      |
| 942:233a | $0, 0, 0, 0, 0, e^{12}, e^{13}, e^{16} + e^{24}, e^{26} + e^{37} + e^{45}$    | 269      |
| 942:233b | $0, 0, 0, 0, 0, -e^{12}, e^{13}, e^{16} + e^{24}, e^{37} + e^{26} + e^{45}$   | 269      |
| 942:234  | $0, 0, 0, 0, 0, e^{12}, e^{13}, e^{16} + e^{24}, e^{27} + e^{45} + e^{36}$    | 269      |
| 942:235  | $0, 0, 0, 0, 0, e^{12}, e^{13}, e^{16} + e^{34}, e^{45} + e^{17} + e^{26}$    | 269      |
| 942:236a | $0, 0, 0, 0, 0, e^{12}, e^{13}, e^{34} + e^{16}, e^{45} + e^{37} + e^{26}$    | 269      |
| 942:236b | $0, 0, 0, 0, 0, -e^{12}, e^{13}, e^{16} + e^{34}, e^{37} + e^{26} + e^{45}$   | 269      |
| 942:237  | $0, 0, 0, 0, 0, e^{12}, e^{13}, e^{16} + e^{34}, e^{27} + e^{36} + e^{45}$    | 269      |
| 942:238  | $0, 0, 0, 0, 0, e^{12}, e^{13}, e^{26} + e^{34}, e^{16} + e^{37} + e^{45}$    | 269      |
| 942:239  | $0, 0, 0, 0, 0, e^{12}, e^{13}, e^{34} + e^{26}, e^{45} + e^{36} + e^{27}$    | 269      |
| 942:240a | $0, 0, 0, 0, 0, e^{12}, e^{13}, e^{45} + e^{16}, e^{37} + e^{14} + e^{26}$    | 269      |
| 942:240b | $0, 0, 0, 0, 0, -e^{12}, e^{13}, e^{16} + e^{45}, e^{37} + e^{26} + e^{14}$   | 269      |
| 942:241  | $0, 0, 0, 0, 0, e^{12}, e^{13}, e^{45} + e^{16}, e^{27} + e^{36} + e^{14}$    | 269      |
| 942:242  | $0, 0, 0, 0, 0, e^{12}, e^{13}, e^{16} + e^{45}, e^{17} + e^{26} + e^{34}$    | 269      |
| 942:243  | $0, 0, 0, 0, 0, e^{12}, e^{13}, e^{45} + e^{26}, e^{16} + e^{24} + e^{37}$    | 269      |
| 942:244  | $0, 0, 0, 0, 0, e^{12}, e^{13}, e^{26} + e^{45}, e^{27} + e^{14} + e^{36}$    | 269      |
| 942:245  | $0, 0, 0, 0, 0, e^{12}, e^{13}, e^{23} + e^{16}, e^{37} + e^{14} + e^{25}$    | 269      |

Table 2 – Continued to next page

Table 2 – Continued from previous page

| Name     | $\mathfrak{g}$                                                                            | UCS Dim. |
|----------|-------------------------------------------------------------------------------------------|----------|
| 942:246  | $0, 0, 0, 0, 0, e^{12}, e^{13}, e^{16} + e^{23}, e^{24} + e^{35} + e^{17}$                | 269      |
| 942:247a | $0, 0, 0, 0, 0, e^{12}, e^{13}, e^{23} + e^{16}, e^{37} + e^{14} + e^{26}$                | 369      |
| 942:247b | $0, 0, 0, 0, 0, -e^{12}, e^{13}, e^{16} + e^{23}, e^{26} + e^{37} + e^{14}$               | 369      |
| 942:248  | $0, 0, 0, 0, 0, e^{12}, e^{13}, e^{16} + e^{23}, e^{27} + e^{36} + e^{14}$                | 369      |
| 942:249  | $0, 0, 0, 0, 0, e^{12}, e^{13}, e^{23} + e^{16}, e^{17} + e^{26} + e^{34}$                | 369      |
| 942:250  | $0, 0, 0, 0, 0, e^{12}, e^{13}, e^{23} + e^{16}, e^{26} + e^{45} + e^{17}$                | 269      |
| 942:251a | $0, 0, 0, 0, 0, e^{12}, e^{13}, e^{23} + e^{16}, e^{37} + e^{45} + e^{26}$                | 269      |
| 942:251b | $0, 0, 0, 0, 0, -e^{12}, e^{13}, e^{16} + e^{23}, e^{37} + e^{26} + e^{45}$               | 269      |
| 942:252  | $0, 0, 0, 0, 0, e^{12}, e^{13}, e^{23} + e^{16}, e^{27} + e^{45} + e^{36}$                | 269      |
| 942:253  | $0, 0, 0, 0, 0, e^{12}, e^{13}, e^{26} + e^{14}, e^{16} + e^{25} + e^{37}$                | 269      |
| 942:254  | $0, 0, 0, 0, 0, e^{12}, e^{13}, e^{14} + e^{26}, e^{15} + e^{36} + e^{27}$                | 269      |
| 942:255a | $0, 0, 0, 0, 0, e^{12}, e^{13}, e^{24} + e^{16}, e^{26} + e^{37} + e^{15}$                | 269      |
| 942:255b | $0, 0, 0, 0, 0, -e^{12}, e^{13}, e^{24} + e^{16}, e^{37} + e^{15} + e^{26}$               | 269      |
| 942:256  | $0, 0, 0, 0, 0, e^{12}, e^{13}, e^{24} + e^{16}, e^{36} + e^{27} + e^{15}$                | 269      |
| 942:257  | $0, 0, 0, 0, 0, e^{12}, e^{13}, e^{16} + e^{24}, e^{17} + e^{26} + e^{35}$                | 269      |
| 942:258a | $0, 0, 0, 0, 0, e^{12}, e^{13}, e^{16} + e^{34}, e^{15} + e^{26} + e^{37}$                | 269      |
| 942:258b | $0, 0, 0, 0, 0, -e^{12}, e^{13}, e^{16} + e^{34}, e^{15} + e^{37} + e^{26}$               | 269      |
| 942:259  | $0, 0, 0, 0, 0, e^{12}, e^{13}, e^{34} + e^{16}, e^{36} + e^{27} + e^{15}$                | 269      |
| 942:260  | $0, 0, 0, 0, 0, e^{12}, e^{13}, e^{16} + e^{34}, e^{35} + e^{17} + e^{26}$                | 269      |
| 942:261  | $0, 0, 0, 0, 0, e^{12}, e^{13}, e^{26} + e^{34}, e^{25} + e^{37} + e^{16}$                | 269      |
| 942:262  | $0, 0, 0, 0, 0, e^{12}, e^{13}, e^{34} + e^{26}, e^{27} + e^{36} + e^{15}$                | 269      |
| 942:263  | $0, 0, 0, 0, 0, e^{12}, e^{13}, e^{16} + e^{45} + e^{23}, e^{17} + e^{26}$                | 269      |
| 942:264  | $0, 0, 0, 0, 0, e^{12}, e^{13}, e^{16} + e^{24} + e^{35}, e^{17} + e^{26}$                | 269      |
| 942:265  | $0, 0, 0, 0, 0, e^{12}, e^{13}, e^{35} + e^{14} + e^{26}, e^{37} + e^{16}$                | 269      |
| 942:266a | $0, 0, 0, 0, 0, e^{12}, e^{13}, e^{16} + e^{23} + e^{45}, e^{26} + e^{37}$                | 269      |
| 942:266b | $0, 0, 0, 0, 0, -e^{12}, e^{13}, e^{23} + e^{45} + e^{16}, e^{37} + e^{26}$               | 269      |
| 942:267a | $0, 0, 0, 0, 0, e^{12}, e^{13}, e^{24} + e^{35} + e^{16}, e^{37} + e^{26}$                | 269      |
| 942:267b | $0, 0, 0, 0, 0, -e^{12}, e^{13}, e^{16} + e^{24} + e^{35}, e^{37} + e^{26}$               | 269      |
| 942:268  | $0, 0, 0, 0, 0, e^{12}, e^{13}, e^{26} + e^{35} + e^{14}, e^{27} + e^{36}$                | 269      |
| 942:269  | $0, 0, 0, 0, 0, e^{12}, e^{13}, e^{16} + e^{23} + e^{45}, e^{36} + e^{27}$                | 269      |
| 942:270  | $0, 0, 0, 0, 0, e^{12}, e^{13}, e^{16} + e^{35} + e^{24}, e^{27} + e^{36}$                | 269      |
| 942:271  | $0, 0, 0, 0, 0, e^{12}, e^{13}, e^{26} + e^{17}, e^{24} + e^{37} + e^{16}$                | 369      |
| 942:272  | $0, 0, 0, 0, 0, e^{12}, e^{13}, e^{17} + e^{26}, e^{27} + e^{36} + e^{14}$                | 369      |
| 942:273a | $0, 0, 0, 0, 0, e^{12}, e^{13}, e^{26} + e^{37}, e^{27} + e^{36} + e^{14}$                | 369      |
| 942:273b | $0, 0, 0, 0, 0, e^{12}, e^{13}, -e^{26} + e^{37}, e^{27} + e^{14} + e^{36}$               | 369      |
| 942:274a | $0, 0, 0, 0, 0, e^{12}, e^{13}, e^{36} + e^{27}, e^{37} + e^{14} + e^{26}$                | 369      |
| 942:274b | $0, 0, 0, 0, 0, -e^{12}, e^{13}, -e^{27} + e^{36}, e^{26} + e^{37} + e^{14}$              | 369      |
| 942:275  | $0, 0, 0, 0, 0, e^{12}, e^{13}, e^{27} + e^{36}, e^{16} + e^{37} + e^{24}$                | 369      |
| 942:276  | $0, 0, 0, 0, 0, e^{12}, e^{13}, e^{17} + e^{26}, e^{45} + e^{37} + e^{16}$                | 269      |
| 942:277  | $0, 0, 0, 0, 0, e^{12}, e^{13}, e^{17} + e^{26}, e^{27} + e^{36} + e^{45}$                | 269      |
| 942:278  | $0, 0, 0, 0, 0, e^{12}, e^{13}, e^{36} + e^{27}, e^{26} + e^{17} + e^{45}$                | 269      |
| 942:279a | $0, 0, 0, 0, 0, e^{12}, e^{13}, e^{26} + e^{37}, e^{27} + e^{36} + e^{45}$                | 269      |
| 942:279b | $0, 0, 0, 0, 0, e^{12}, e^{13}, e^{37} - e^{26}, e^{45} + e^{36} + e^{27}$                | 269      |
| 942:280a | $0, 0, 0, 0, 0, e^{12}, e^{13}, e^{27} + e^{36}, e^{26} + e^{37} + e^{45}$                | 269      |
| 942:280b | $0, 0, 0, 0, 0, -e^{12}, e^{13}, -e^{27} + e^{36}, e^{37} + e^{26} + e^{45}$              | 269      |
| 942:281  | $0, 0, 0, 0, 0, e^{12}, e^{13}, e^{26} + e^{34} + e^{15}, e^{37} + e^{25} + e^{14}$       | 269      |
| 942:282  | $0, 0, 0, 0, 0, e^{12}, e^{13}, e^{16} + e^{45} + e^{23}, e^{25} + e^{37} + e^{14}$       | 269      |
| 942:283a | $0, 0, 0, 0, 0, e^{12}, e^{13}, e^{16} + e^{24} + e^{35}, e^{14} + e^{25} + e^{37}$       | 269      |
| 942:283b | $0, 0, 0, 0, 0, -e^{12}, e^{13}, e^{16} + e^{24} + e^{35}, e^{25} + e^{14} + e^{37}$      | 269      |
| 942:284a | $0, 0, 0, 0, 0, e^{12}, e^{13}, e^{35} + e^{24} + e^{16}, e^{23} + e^{45} + e^{17}$       | 269      |
| 942:284b | $0, 0, 0, 0, 0, e^{12}, e^{13}, e^{35} - e^{24} + e^{16}, e^{23} + e^{45} + e^{17}$       | 269      |
| 942:285a | $0, 0, 0, 0, 0, e^{12}, e^{13}, e^{34} + e^{16} + e^{25}, a_1, e^{24} + e^{35} + e^{17}$  | 269      |
| 942:285b | $0, 0, 0, 0, 0, -e^{12}, e^{13}, e^{34} + e^{16} + e^{25}, a_1, e^{35} + e^{24} + e^{17}$ | 269      |
| 942:286  | $0, 0, 0, 0, 0, e^{12}, e^{13}, e^{16} + e^{24} + e^{35}, e^{17} + e^{26} + e^{45}$       | 269      |
| 942:287  | $0, 0, 0, 0, 0, e^{12}, e^{13}, e^{35} + e^{14} + e^{26}, e^{45} + e^{37} + e^{16}$       | 269      |
| 942:288a | $0, 0, 0, 0, 0, e^{12}, e^{13}, e^{35} + e^{24} + e^{16}, e^{26} + e^{37} + e^{45}$       | 269      |
| 942:288b | $0, 0, 0, 0, 0, -e^{12}, e^{13}, e^{35} + e^{24} + e^{16}, e^{37} + e^{45} + e^{26}$      | 269      |
| 942:289  | $0, 0, 0, 0, 0, e^{12}, e^{13}, e^{26} + e^{35} + e^{14}, e^{45} + e^{36} + e^{27}$       | 269      |

Table 2 – Continued to next page

Table 2 – Continued from previous page

| Name     | $\mathfrak{g}$                                                                          | UCS Dim. |
|----------|-----------------------------------------------------------------------------------------|----------|
| 942:290  | $0, 0, 0, 0, 0, e^{12}, e^{13}, e^{16} + e^{35} + e^{24}, e^{27} + e^{36} + e^{45}$     | 269      |
| 942:291a | $0, 0, 0, 0, 0, e^{12}, e^{13}, e^{45} + e^{16} + e^{23}, e^{14} + e^{37} + e^{26}$     | 269      |
| 942:291b | $0, 0, 0, 0, 0, -e^{12}, e^{13}, e^{45} + e^{23} + e^{16}, e^{37} + e^{14} + e^{26}$    | 269      |
| 942:292a | $0, 0, 0, 0, 0, e^{12}, e^{13}, e^{35} + e^{24} + e^{16}, e^{26} + e^{37} + e^{14}$     | 269      |
| 942:292b | $0, 0, 0, 0, 0, e^{12}, e^{13}, e^{35} + e^{24} - e^{16}, e^{37} + e^{14} + e^{26}$     | 269      |
| 942:292c | $0, 0, 0, 0, 0, -e^{12}, e^{13}, e^{24} + e^{35} + e^{16}, e^{37} + e^{26} + e^{14}$    | 269      |
| 942:292d | $0, 0, 0, 0, 0, -e^{12}, e^{13}, e^{35} - e^{16} + e^{24}, e^{37} + e^{14} + e^{26}$    | 269      |
| 942:293a | $0, 0, 0, 0, 0, e^{12}, e^{13}, e^{34} + e^{16} + e^{25}, e^{14} + e^{26} + e^{37}$     | 269      |
| 942:293b | $0, 0, 0, 0, 0, -e^{12}, e^{13}, e^{16} + e^{25} + e^{34}, e^{26} + e^{37} + e^{14}$    | 269      |
| 942:294a | $0, 0, 0, 0, 0, e^{12}, e^{13}, e^{14} + e^{26} + e^{35}, e^{16} + e^{24} + e^{37}$     | 269      |
| 942:294b | $0, 0, 0, 0, 0, e^{12}, e^{13}, e^{35} - e^{14} + e^{26}, e^{37} + e^{16} + e^{24}$     | 269      |
| 942:295  | $0, 0, 0, 0, 0, e^{12}, e^{13}, e^{15} + e^{34} + e^{26}, e^{16} + e^{24} + e^{37}$     | 269      |
| 942:296  | $0, 0, 0, 0, 0, e^{12}, e^{13}, e^{15} + e^{26} + e^{34}, e^{36} + e^{14} + e^{27}$     | 269      |
| 942:297  | $0, 0, 0, 0, 0, e^{12}, e^{13}, e^{23} + e^{16} + e^{45}, e^{14} + e^{27} + e^{36}$     | 269      |
| 942:298  | $0, 0, 0, 0, 0, e^{12}, e^{13}, e^{16} + e^{35} + e^{24}, e^{27} + e^{36} + e^{14}$     | 269      |
| 942:299a | $0, 0, 0, 0, 0, e^{12}, e^{13}, e^{25} + e^{16} + e^{34}, e^{27} + e^{14} + e^{36}$     | 269      |
| 942:299b | $0, 0, 0, 0, 0, e^{12}, e^{13}, -e^{16} + e^{25} + e^{34}, e^{36} + e^{14} + e^{27}$    | 269      |
| 942:300  | $0, 0, 0, 0, 0, e^{12}, e^{13}, e^{45} + e^{23} + e^{16}, e^{17} + e^{34} + e^{26}$     | 269      |
| 942:301  | $0, 0, 0, 0, 0, a_1 e^{12}, e^{13}, e^{35} + e^{16} + e^{24}, e^{26} + e^{34} + e^{17}$ | 269      |
| 942:302  | $0, 0, 0, 0, 0, e^{12}, e^{13}, e^{14} + e^{36} + e^{27}, e^{16} + e^{24} + e^{37}$     | 369      |
| 942:303  | $0, 0, 0, 0, 0, a_1 e^{12}, e^{13}, e^{34} + e^{26} + e^{17}, e^{24} + e^{37} + e^{16}$ | 369      |
| 942:304  | $0, 0, 0, 0, 0, e^{12}, e^{13}, e^{24} + e^{37} + e^{16}, e^{45} + e^{26} + e^{17}$     | 269      |
| 942:305  | $0, 0, 0, 0, 0, e^{12}, e^{13}, e^{14} + e^{27} + e^{36}, e^{26} + e^{17} + e^{45}$     | 269      |
| 942:306a | $0, 0, 0, 0, 0, e^{12}, e^{13}, e^{27} + e^{36} + e^{14}, e^{26} + e^{37} + e^{45}$     | 269      |
| 942:306b | $0, 0, 0, 0, 0, -e^{12}, e^{13}, -e^{27} + e^{36} + e^{14}, e^{26} + e^{37} + e^{45}$   | 269      |
| 942:307a | $0, 0, 0, 0, 0, e^{12}, e^{13}, e^{37} + e^{14} + e^{26}, e^{36} + e^{45} + e^{27}$     | 269      |
| 942:307b | $0, 0, 0, 0, 0, e^{12}, e^{13}, e^{37} + e^{14} - e^{26}, e^{27} + e^{45} + e^{36}$     | 269      |
| 942:308  | $0, 0, 0, 0, 0, e^{12}, e^{13}, e^{16} + e^{37} + e^{24}, e^{27} + e^{36} + e^{45}$     | 269      |
| 942:309a | $0, 0, 0, 0, 0, e^{12}, e^{13}, e^{27} + e^{14} + e^{36}, e^{26} + e^{15} + e^{37}$     | 269      |
| 942:309b | $0, 0, 0, 0, 0, -e^{12}, e^{13}, e^{36} - e^{27} + e^{14}, e^{37} + e^{26} + e^{15}$    | 269      |
| 942:310  | $0, 0, 0, 0, 0, e^{12}, e^{13}, e^{14} + e^{27} + e^{36}, e^{25} + e^{37} + e^{16}$     | 269      |
| 942:311  | $0, 0, 0, 0, 0, e^{12}, e^{13}, e^{17} + e^{26} + e^{34}, e^{16} + e^{25} + e^{37}$     | 269      |
| 942:312  | $0, 0, 0, 0, 0, e^{12}, e^{34}, e^{16}, e^{37}$                                         | 359      |
| 942:313  | $0, 0, 0, 0, 0, e^{12}, e^{34}, e^{13} + e^{26}, e^{37}$                                | 359      |
| 942:314  | $0, 0, 0, 0, 0, e^{12}, e^{34}, e^{16}, e^{23} + e^{47}$                                | 359      |
| 942:315  | $0, 0, 0, 0, 0, e^{12}, e^{34}, e^{16}, e^{37} + e^{15}$                                | 259      |
| 942:316  | $0, 0, 0, 0, 0, e^{12}, e^{34}, e^{16}, e^{25} + e^{37}$                                | 259      |
| 942:317  | $0, 0, 0, 0, 0, e^{12}, e^{34}, e^{16}, e^{47} + e^{35}$                                | 259      |
| 942:318  | $0, 0, 0, 0, 0, e^{12}, e^{34}, e^{16}, e^{26} + e^{37}$                                | 359      |
| 942:319  | $0, 0, 0, 0, 0, e^{12}, e^{34}, e^{16} + e^{25}, e^{15} + e^{37}$                       | 259      |
| 942:320  | $0, 0, 0, 0, 0, e^{12}, e^{34}, e^{16} + e^{35}, e^{15} + e^{37}$                       | 259      |
| 942:321  | $0, 0, 0, 0, 0, e^{12}, e^{34}, e^{35} + e^{16}, e^{37} + e^{25}$                       | 259      |
| 942:322a | $0, 0, 0, 0, 0, e^{12}, e^{34}, e^{26} + e^{15}, e^{35} + e^{47}$                       | 259      |
| 942:322b | $0, 0, 0, 0, 0, -e^{12}, e^{34}, e^{15} + e^{26}, e^{35} + e^{47}$                      | 259      |
| 942:323a | $0, 0, 0, 0, 0, e^{12}, e^{34}, e^{35} + e^{16}, e^{47} + e^{25}$                       | 259      |
| 942:323b | $0, 0, 0, 0, 0, -e^{12}, e^{34}, e^{16} + e^{35}, e^{25} + e^{47}$                      | 259      |
| 942:324  | $0, 0, 0, 0, 0, -e^{12}, e^{23} + e^{14}, e^{16}, e^{17} + e^{36}$                      | 359      |
| 942:325  | $0, 0, 0, 0, 0, e^{12}, e^{24} + e^{13}, e^{16}, e^{36} + e^{27}$                       | 359      |
| 942:326  | $0, 0, 0, 0, 0, e^{12}, e^{34}, e^{16} + e^{23}, e^{13} + e^{47}$                       | 359      |
| 942:327  | $0, 0, 0, 0, 0, e^{12}, e^{34}, e^{23} + e^{16}, e^{37} + e^{14}$                       | 359      |
| 942:328  | $0, 0, 0, 0, 0, e^{12}, e^{34}, e^{13} + e^{26}, e^{37} + e^{15}$                       | 259      |
| 942:329  | $0, 0, 0, 0, 0, e^{12}, e^{34}, e^{23} + e^{16}, e^{37} + e^{15}$                       | 259      |
| 942:330  | $0, 0, 0, 0, 0, e^{12}, e^{34}, e^{16}, e^{13} + e^{47} + e^{25}$                       | 259      |
| 942:331  | $0, 0, 0, 0, 0, e^{12}, e^{34}, e^{16}, e^{15} + e^{47} + e^{23}$                       | 259      |
| 942:332  | $0, 0, 0, 0, 0, e^{12}, e^{34}, e^{26} + e^{13}, e^{47} + e^{15}$                       | 259      |
| 942:333  | $0, 0, 0, 0, 0, e^{12}, e^{34}, e^{23} + e^{16}, e^{15} + e^{47}$                       | 259      |
| 942:334  | $0, 0, 0, 0, 0, e^{12}, e^{34}, e^{13} + e^{26}, e^{35} + e^{47}$                       | 259      |
| 942:335  | $0, 0, 0, 0, 0, e^{12}, e^{34}, e^{13} + e^{26}, e^{37} + e^{45}$                       | 259      |

Table 2 – Continued to next page

Table 2 – Continued from previous page

| Name     | $\mathfrak{g}$                                                                       | UCS Dim. |
|----------|--------------------------------------------------------------------------------------|----------|
| 942:336  | $0, 0, 0, 0, 0, e^{12}, e^{34}, e^{13} + e^{26}, e^{37} + e^{16}$                    | 359      |
| 942:337  | $0, 0, 0, 0, 0, e^{12}, e^{34}, e^{16}, e^{13} + e^{26} + e^{47}$                    | 359      |
| 942:338  | $0, 0, 0, 0, 0, e^{12}, e^{34}, e^{26} + e^{13}, e^{16} + e^{47}$                    | 359      |
| 942:339  | $0, 0, 0, 0, 0, e^{12}, e^{34}, e^{16}, e^{15} + e^{26} + e^{37}$                    | 259      |
| 942:340  | $0, 0, 0, 0, 0, e^{12}, e^{34}, e^{16}, e^{47} + e^{26} + e^{35}$                    | 259      |
| 942:341  | $0, 0, 0, 0, 0, e^{12}, e^{34}, e^{26} + e^{15}, e^{16} + e^{37}$                    | 259      |
| 942:342  | $0, 0, 0, 0, 0, e^{12}, e^{34}, e^{16} + e^{35}, e^{26} + e^{37}$                    | 259      |
| 942:343  | $0, 0, 0, 0, 0, e^{12}, e^{34}, e^{35} + e^{16}, e^{47} + e^{26}$                    | 259      |
| 942:344  | $0, 0, 0, 0, 0, e^{12}, e^{34}, e^{37} + e^{16}, e^{26} + e^{47}$                    | 359      |
| 942:345  | $0, 0, 0, 0, 0, e^{12}, e^{34}, e^{26} + e^{15}, e^{47} + e^{13} + e^{25}$           | 259      |
| 942:346a | $0, 0, 0, 0, 0, e^{12}, e^{34}, e^{35} + e^{16}, e^{13} + e^{47} + e^{25}$           | 259      |
| 942:346b | $0, 0, 0, 0, 0, -e^{12}, e^{34}, e^{16} + e^{35}, e^{25} + e^{47} + e^{13}$          | 259      |
| 942:347  | $0, 0, 0, 0, 0, e^{12}, e^{34}, e^{16} + e^{35}, e^{15} + e^{23} + e^{47}$           | 259      |
| 942:348  | $0, 0, 0, 0, 0, e^{12}, e^{34}, e^{16} + e^{35}, e^{25} + e^{14} + e^{37}$           | 259      |
| 942:349  | $0, 0, 0, 0, 0, e^{12}, e^{34}, e^{35} + e^{16}, e^{24} + e^{37} + e^{15}$           | 259      |
| 942:350a | $0, 0, 0, 0, 0, e^{12}, e^{34}, e^{15} + e^{26}, e^{37} + e^{16} + e^{25}$           | 259      |
| 942:350b | $0, 0, 0, 0, 0, e^{12}, e^{34}, e^{26} - e^{15}, e^{25} + e^{37} + e^{16}$           | 259      |
| 942:351  | $0, 0, 0, 0, 0, e^{12}, e^{34}, e^{16} + e^{35}, e^{37} + e^{26} + e^{15}$           | 259      |
| 942:352a | $0, 0, 0, 0, 0, e^{12}, e^{34}, e^{26} + e^{15}, e^{16} + e^{47} + e^{35}$           | 259      |
| 942:352b | $0, 0, 0, 0, 0, -e^{12}, e^{34}, e^{15} + e^{26}, e^{16} + e^{35} + e^{47}$          | 259      |
| 942:353  | $0, 0, 0, 0, 0, e^{12}, e^{34}, e^{16} + e^{35}, e^{15} + e^{26} + e^{47}$           | 259      |
| 942:354  | $0, 0, 0, 0, 0, e^{12}, e^{34}, e^{35} + e^{16}, e^{45} + e^{37} + e^{26}$           | 259      |
| 942:355  | $0, 0, 0, 0, 0, -e^{12}, e^{23} + e^{14}, e^{13} + e^{26}, e^{36} + e^{17}$          | 359      |
| 942:356  | $0, 0, 0, 0, 0, e^{12}, e^{24} + e^{13}, e^{16}, e^{36} + e^{27} + e^{14}$           | 359      |
| 942:357  | $0, 0, 0, 0, 0, -e^{12}, e^{24} + e^{13}, e^{16}, e^{17} + e^{46} + e^{23}$          | 359      |
| 942:358  | $0, 0, 0, 0, 0, -e^{12}, e^{13} + e^{24}, e^{23} + e^{16}, e^{46} + e^{17}$          | 359      |
| 942:359  | $0, 0, 0, 0, 0, -e^{12}, e^{23} + e^{14}, e^{16} + e^{34}, e^{36} + e^{17}$          | 359      |
| 942:360  | $0, 0, 0, 0, 0, e^{12}, e^{24} + e^{13}, e^{34} + e^{16}, e^{36} + e^{27}$           | 359      |
| 942:361  | $0, 0, 0, 0, 0, e^{12}, e^{24} + e^{13}, e^{16}, e^{27} + e^{36} + e^{15}$           | 259      |
| 942:362  | $0, 0, 0, 0, 0, -e^{12}, e^{14} + e^{23}, e^{16}, e^{17} + e^{25} + e^{36}$          | 259      |
| 942:363  | $0, 0, 0, 0, 0, -e^{12}, e^{24} + e^{13}, e^{16}, e^{35} + e^{46} + e^{17}$          | 259      |
| 942:364  | $0, 0, 0, 0, 0, e^{12}, e^{24} + e^{13}, e^{16}, e^{36} + e^{27} + e^{45}$           | 259      |
| 942:365  | $0, 0, 0, 0, 0, -e^{12}, e^{23} + e^{14}, e^{15} + e^{26}, e^{17} + e^{36}$          | 259      |
| 942:366  | $0, 0, 0, 0, 0, -e^{12}, e^{14} + e^{23}, e^{25} + e^{16}, e^{36} + e^{17}$          | 259      |
| 942:367  | $0, 0, 0, 0, 0, -e^{12}, e^{23} + e^{14}, e^{35} + e^{16}, e^{36} + e^{17}$          | 259      |
| 942:368  | $0, 0, 0, 0, 0, e^{12}, e^{24} + e^{13}, e^{35} + e^{16}, e^{36} + e^{27}$           | 259      |
| 942:369  | $0, 0, 0, 0, 0, -e^{12}, e^{24} + e^{13}, e^{16} + e^{35}, e^{17} + e^{46}$          | 259      |
| 942:370  | $0, 0, 0, 0, 0, e^{12}, e^{14} + e^{23}, e^{16} + e^{35}, e^{46} + e^{27}$           | 259      |
| 942:371  | $0, 0, 0, 0, 0, -e^{12}, -e^{14} + e^{23}, e^{36} + e^{17}, e^{27} + e^{46}$         | 359      |
| 942:372  | $0, 0, 0, 0, 0, e^{12}, e^{34}, e^{13} + e^{26}, e^{47} + e^{15} + e^{23}$           | 259      |
| 942:373  | $0, 0, 0, 0, 0, e^{12}, e^{34}, e^{26} + e^{13}, e^{14} + e^{37} + e^{25}$           | 259      |
| 942:374  | $0, 0, 0, 0, 0, e^{12}, e^{34}, e^{26} + e^{13}, e^{15} + e^{37} + e^{24}$           | 259      |
| 942:375a | $0, 0, 0, 0, 0, e^{12}, e^{34}, e^{26} + e^{13}, e^{47} + e^{16} + e^{23}$           | 359      |
| 942:375b | $0, 0, 0, 0, 0, e^{12}, e^{34}, -e^{13} + e^{26}, e^{47} + e^{23} + e^{16}$          | 359      |
| 942:376  | $0, 0, 0, 0, 0, e^{12}, e^{34}, e^{13} + e^{26}, e^{16} + e^{24} + e^{37}$           | 359      |
| 942:377  | $0, 0, 0, 0, 0, e^{12}, e^{34}, e^{13} + e^{26}, e^{37} + e^{16} + e^{25}$           | 259      |
| 942:378  | $0, 0, 0, 0, 0, e^{12}, e^{34}, e^{13} + e^{26}, e^{47} + e^{25} + e^{16}$           | 259      |
| 942:379  | $0, 0, 0, 0, 0, e^{12}, e^{34}, e^{13} + e^{26}, e^{47} + e^{16} + e^{35}$           | 259      |
| 942:380  | $0, 0, 0, 0, 0, e^{12}, e^{34}, e^{26} + e^{13}, e^{16} + e^{37} + e^{45}$           | 259      |
| 942:381  | $0, 0, 0, 0, 0, e^{12}, e^{34}, e^{15} + e^{26}, e^{16} + e^{47} + e^{23}$           | 259      |
| 942:382  | $0, 0, 0, 0, 0, e^{12}, e^{34}, e^{16} + e^{35}, e^{47} + e^{26} + e^{13}$           | 259      |
| 942:383  | $0, 0, 0, 0, 0, e^{12}, e^{34}, e^{16} + e^{35}, e^{14} + e^{26} + e^{37}$           | 259      |
| 942:384  | $0, 0, 0, 0, 0, e^{12}, e^{34}, e^{13} + e^{26} + e^{45}, e^{16} + e^{37}$           | 259      |
| 942:385  | $0, 0, 0, 0, 0, e^{12}, e^{34}, e^{35} + e^{14} + e^{26}, e^{37} + e^{16}$           | 259      |
| 942:386  | $0, 0, 0, 0, 0, e^{12}, e^{34}, e^{37} + e^{16}, e^{13} + e^{26} + e^{47}$           | 359      |
| 942:387  | $0, 0, 0, 0, 0, e^{12}, e^{34}, e^{37} + e^{16}, e^{47} + e^{26} + e^{15}$           | 259      |
| 942:388  | $0, 0, 0, 0, 0, -e^{12}, e^{23} + e^{14}, e^{15} + e^{26}, e^{17} + e^{25} + e^{36}$ | 259      |
| 942:389a | $0, 0, 0, 0, 0, e^{12}, e^{24} + e^{13}, e^{16} + e^{35}, e^{15} + e^{36} + e^{27}$  | 259      |

Table 2 – Continued to next page

Table 2 – Continued from previous page

| Name     | $\mathfrak{g}$                                                                                | UCS Dim. |
|----------|-----------------------------------------------------------------------------------------------|----------|
| 942:389b | $0, 0, 0, 0, 0, e^{12}, e^{24} + e^{13}, e^{35} - e^{16}, e^{27} + e^{36} + e^{15}$           | 259      |
| 942:390  | $0, 0, 0, 0, 0, -e^{12}, e^{14} + e^{23}, e^{16} + e^{35}, e^{25} + e^{17} + e^{36}$          | 259      |
| 942:391a | $0, 0, 0, 0, 0, -e^{12}, e^{24} + e^{13}, e^{15} + e^{26}, e^{17} + e^{35} + e^{46}$          | 259      |
| 942:391b | $0, 0, 0, 0, 0, -e^{12}, -e^{13} + e^{24}, e^{26} + e^{15}, e^{46} + e^{35} + e^{17}$         | 259      |
| 942:392  | $0, 0, 0, 0, 0, -e^{12}, e^{24} + a_2 e^{13}, e^{16} + e^{25}, e^{35} + e^{46} + e^{17}$      | 259      |
| 942:393a | $0, 0, 0, 0, 0, -e^{12}, e^{24} + e^{13}, e^{16} + e^{35}, e^{17} + e^{25} + e^{46}$          | 259      |
| 942:393b | $0, 0, 0, 0, 0, -e^{12}, -e^{13} + e^{24}, e^{16} + e^{35}, e^{17} + e^{25} + e^{46}$         | 259      |
| 942:394  | $0, 0, 0, 0, 0, e^{12}, e^{14} + e^{23}, e^{16} + e^{35}, e^{15} + e^{46} + e^{27}$           | 259      |
| 942:395  | $0, 0, 0, 0, 0, -e^{12}, e^{14} + e^{23}, e^{16} + e^{35}, e^{17} + e^{45} + e^{36}$          | 259      |
| 942:396  | $0, 0, 0, 0, 0, e^{12}, e^{24} + e^{13}, e^{16} + e^{35}, e^{27} + e^{36} + e^{45}$           | 259      |
| 942:397  | $0, 0, 0, 0, 0, e^{12}, e^{34}, e^{14} + e^{26} + e^{35}, e^{47} + e^{25} + e^{13}$           | 259      |
| 942:398a | $0, 0, 0, 0, 0, e^{12}, e^{34}, e^{16} + e^{24} + e^{35}, e^{13} + e^{25} + e^{47}$           | 259      |
| 942:398b | $0, 0, 0, 0, 0, -e^{12}, e^{34}, e^{35} + e^{24} + e^{16}, e^{47} + e^{25} + e^{13}$          | 259      |
| 942:399a | $0, 0, 0, 0, 0, e^{23} + e^{14}, e^{24} + e^{13}, e^{17} + e^{26}, e^{27} + e^{16}$           | 359      |
| 942:399b | $0, 0, 0, 0, 0, -e^{14} + e^{23}, e^{24} + e^{13}, -e^{17} + e^{26}, e^{16} + e^{27}$         | 359      |
| 942:400a | $0, 0, 0, 0, 0, e^{14} + e^{23}, e^{13} + e^{24}, e^{27} + e^{16}, e^{36} + e^{47}$           | 359      |
| 942:400b | $0, 0, 0, 0, 0, -e^{23} - e^{14}, e^{24} - e^{13}, e^{16} + e^{27}, e^{36} + e^{47}$          | 359      |
| 942:401  | $0, 0, 0, 0, 0, e^{12}, e^{34}, e^{16} + e^{45} + e^{23}, e^{15} + e^{26} + e^{37}$           | 259      |
| 942:402  | $0, 0, 0, 0, 0, e^{12}, e^{34}, e^{16} + e^{24} + e^{35}, e^{15} + e^{37} + e^{26}$           | 259      |
| 942:403  | $0, 0, 0, 0, 0, e^{12}, e^{34}, e^{45} + e^{13} + e^{26}, e^{35} + e^{47} + e^{16}$           | 259      |
| 942:404  | $0, 0, 0, 0, 0, -e^{12}, e^{23} + e^{14}, e^{13} + e^{26}, e^{24} + e^{36} + e^{17}$          | 359      |
| 942:405a | $0, 0, 0, 0, 0, e^{12}, e^{24} + e^{13}, e^{34} + e^{16}, e^{36} + e^{27} + e^{14}$           | 359      |
| 942:405b | $0, 0, 0, 0, 0, e^{12}, e^{13} + e^{24}, e^{34} - e^{16}, e^{14} + e^{27} + e^{36}$           | 359      |
| 942:406  | $0, 0, 0, 0, 0, -e^{12}, e^{13} + e^{24}, e^{34} + e^{16}, e^{46} + e^{17} + e^{23}$          | 359      |
| 942:407  | $0, 0, 0, 0, 0, -e^{12}, e^{23} + e^{14}, e^{13} + e^{26}, e^{36} + e^{17} + e^{25}$          | 259      |
| 942:408  | $0, 0, 0, 0, 0, e^{12}, e^{14} + e^{23}, e^{13} + e^{26}, e^{46} + e^{27} + e^{15}$           | 259      |
| 942:409  | $0, 0, 0, 0, 0, -e^{12}, e^{23} + e^{14}, e^{26} + e^{13}, e^{17} + e^{36} + e^{45}$          | 259      |
| 942:410  | $0, 0, 0, 0, 0, -e^{12}, e^{13} + e^{24}, e^{23} + e^{16}, e^{17} + e^{46} + e^{35}$          | 259      |
| 942:411  | $0, 0, 0, 0, 0, e^{12}, e^{13} + e^{24}, e^{16} + e^{34}, e^{15} + e^{27} + e^{36}$           | 259      |
| 942:412  | $0, 0, 0, 0, 0, -e^{12}, e^{14} + e^{23}, e^{34} + e^{16}, e^{17} + e^{36} + e^{25}$          | 259      |
| 942:413  | $0, 0, 0, 0, 0, -e^{12}, e^{24} + e^{13}, e^{16} + e^{34}, e^{17} + e^{35} + e^{46}$          | 259      |
| 942:414  | $0, 0, 0, 0, 0, e^{12}, e^{24} + e^{13}, e^{16} + e^{34}, e^{36} + e^{27} + e^{45}$           | 259      |
| 942:415  | $0, 0, 0, 0, 0, e^{12}, e^{24} + e^{13}, e^{26} + e^{15}, e^{27} + e^{36} + e^{14}$           | 259      |
| 942:416  | $0, 0, 0, 0, 0, -e^{12}, e^{13} + e^{24}, e^{26} + e^{15}, e^{23} + e^{17} + e^{46}$          | 259      |
| 942:417  | $0, 0, 0, 0, 0, e^{12}, e^{24} + e^{13}, e^{16} + e^{35}, e^{27} + e^{36} + e^{14}$           | 259      |
| 942:418  | $0, 0, 0, 0, 0, -e^{12}, e^{13} + e^{24}, e^{35} + e^{16}, e^{46} + e^{17} + e^{23}$          | 259      |
| 942:419  | $0, 0, 0, 0, 0, e^{12}, e^{14} + e^{23}, e^{16} + e^{35}, e^{13} + e^{46} + e^{27}$           | 259      |
| 942:420  | $0, 0, 0, 0, 0, -e^{12}, e^{14} + e^{23}, e^{35} + e^{16}, e^{17} + e^{36} + e^{24}$          | 259      |
| 942:421  | $0, 0, 0, 0, 0, -e^{12}, e^{23} + e^{14}, e^{26} + e^{45} + e^{13}, e^{17} + e^{36}$          | 259      |
| 942:422  | $0, 0, 0, 0, 0, -e^{12}, e^{14} + e^{23}, e^{34} + e^{26} + e^{15}, e^{36} + e^{17}$          | 259      |
| 942:423  | $0, 0, 0, 0, 0, -e^{12}, e^{23} + e^{14}, e^{35} + e^{24} + e^{16}, e^{36} + e^{17}$          | 259      |
| 942:424  | $0, 0, 0, 0, 0, -e^{12}, e^{14} + e^{23}, e^{25} + e^{16} + e^{34}, e^{17} + e^{36}$          | 259      |
| 942:425a | $0, 0, 0, 0, 0, e^{12}, e^{34}, e^{16} + e^{37} + e^{25}, e^{26} + e^{47} + e^{15}$           | 259      |
| 942:425b | $0, 0, 0, 0, 0, e^{12}, e^{34}, -e^{16} + e^{25} + e^{37}, e^{15} + e^{26} + e^{47}$          | 259      |
| 942:426a | $0, 0, 0, 0, 0, e^{12}, e^{34}, e^{15} + e^{37} + e^{26}, e^{16} + e^{35} + e^{47}$           | 259      |
| 942:426b | $0, 0, 0, 0, 0, -e^{12}, e^{34}, e^{26} + e^{15} + e^{37}, e^{16} + e^{35} + e^{47}$          | 259      |
| 942:427  | $0, 0, 0, 0, 0, -e^{12}, -e^{14} + e^{23}, e^{17} + e^{36}, e^{27} + e^{46} + e^{13}$         | 359      |
| 942:428  | $0, 0, 0, 0, 0, -e^{12}, -e^{14} + e^{23}, e^{36} + e^{17}, e^{46} + e^{27} + e^{15}$         | 259      |
| 942:429  | $0, 0, 0, 0, 0, -e^{12}, -e^{14} + e^{23}, e^{17} + e^{36}, e^{46} + e^{27} + e^{35}$         | 259      |
| 942:430a | $0, 0, 0, 0, 0, e^{12}, e^{34}, e^{16} + e^{45} + e^{23}, e^{26} + e^{47} + e^{13}$           | 259      |
| 942:430b | $0, 0, 0, 0, 0, e^{12}, e^{34}, -e^{16} + e^{45} + e^{23}, e^{26} + e^{47} + e^{13}$          | 259      |
| 942:431  | $0, 0, 0, 0, 0, e^{12}, e^{34}, e^{16} + e^{24} + e^{35}, e^{47} + e^{26} + e^{13}$           | 259      |
| 942:432  | $0, 0, 0, 0, 0, e^{12}, e^{34}, e^{37} + e^{16} + e^{24}, e^{47} + e^{13} + e^{26}$           | 359      |
| 942:433  | $0, 0, 0, 0, 0, e^{12}, e^{34}, e^{23} + e^{47} + e^{16}, e^{26} + e^{37} + e^{15}$           | 259      |
| 942:434  | $0, 0, 0, 0, 0, e^{12}, e^{24} + e^{13}, e^{35} + e^{14} + e^{26}, e^{36} + e^{15} + e^{27}$  | 259      |
| 942:435  | $0, 0, 0, 0, 0, e^{12}, e^{13} + e^{24}, e^{45} + e^{23} + e^{16}, e^{27} + e^{36} + e^{15}$  | 259      |
| 942:436  | $0, 0, 0, 0, 0, e^{12}, e^{24} + e^{13}, e^{16} + e^{25} + e^{34}, e^{15} + e^{27} + e^{36}$  | 259      |
| 942:437a | $0, 0, 0, 0, 0, -e^{12}, e^{13} + e^{24}, e^{15} + e^{34} + e^{26}, e^{17} + e^{46} + e^{35}$ | 259      |

Table 2 – Continued to next page

Table 2 – Continued from previous page

| Name      | $\mathfrak{g}$                                                                                               | UCS Dim. |
|-----------|--------------------------------------------------------------------------------------------------------------|----------|
| 942:437b  | $0, 0, 0, 0, 0, -e^{12}, e^{24} - e^{13}, e^{26} + e^{34} + e^{15}, e^{46} + e^{35} + e^{17}$                | 259      |
| 942:438   | $0, 0, 0, 0, 0, -e^{12}, e^{24} + e^{13}, e^{16} + e^{45} + e^{23}, e^{17} + e^{46} + e^{35}$                | 259      |
| 942:439   | $0, 0, 0, 0, 0, -e^{12}, e^{13}a_2 + e^{24}, e^{16} + e^{25} + e^{34}, e^{17} + e^{35} + e^{46}$             | 259      |
| 942:440a  | $0, 0, 0, 0, 0, -e^{12}, -e^{13} + e^{24}, e^{27} + e^{36} + e^{15}, e^{17} + e^{46} + e^{25}$               | 259      |
| 942:440b  | $0, 0, 0, 0, 0, -e^{12}, e^{24} - e^{13}, -e^{15} + e^{36} + e^{27}, e^{17} + e^{25} + e^{46}$               | 259      |
| 942:441   | $0, 0, 0, 0, 0, -e^{12}, e^{24} - e^{13}, e^{36} + e^{27} + e^{15}, e^{46} + e^{35} + e^{17}$                | 259      |
| 942:442a  | $0, 0, 0, 0, 0, -e^{12}, e^{24} - e^{13}, e^{17} + e^{35} + e^{46}, e^{27} + e^{36} + e^{45}$                | 259      |
| 942:442b  | $0, 0, 0, 0, 0, -e^{12}, e^{24} - e^{13}, e^{46} - e^{35} + e^{17}, e^{27} + e^{36} + e^{45}$                | 259      |
| 942:443a  | $0, 0, 0, 0, 0, e^{23} + e^{14}, e^{24} + e^{13}, e^{27} + e^{16}, e^{47} + e^{12} + e^{36}$                 | 359      |
| 942:443b  | $0, 0, 0, 0, 0, -e^{14} - e^{23}, -e^{13} + e^{24}, e^{16} + e^{27}, e^{12} + e^{47} + e^{36}$               | 359      |
| 942:444a  | $0, 0, 0, 0, 0, e^{23} + e^{14}, e^{24} + e^{13}, e^{27} + e^{16}, e^{17} + e^{26} + e^{34}$                 | 359      |
| 942:444b  | $0, 0, 0, 0, 0, e^{14} + e^{23}, -e^{13} + e^{24}, e^{27} - e^{16}, e^{17} + e^{26} + e^{34}$                | 359      |
| 942:445a  | $0, 0, 0, 0, 0, e^{23} + e^{14}, e^{24} + e^{13}, e^{27} + e^{16}, e^{35} + e^{17} + e^{26}$                 | 259      |
| 942:445b  | $0, 0, 0, 0, 0, e^{14} + e^{23}, -e^{13} + e^{24}, e^{27} - e^{16}, e^{35} + e^{17} + e^{26}$                | 259      |
| 942:446a  | $0, 0, 0, 0, 0, e^{24} + e^{13}, e^{23} + e^{14}, e^{27} + e^{16}, e^{35} + e^{17} + e^{26}$                 | 259      |
| 942:446b  | $0, 0, 0, 0, 0, e^{13} + e^{24}, -e^{14} + e^{23}, e^{27} - e^{16}, e^{35} + e^{17} + e^{26}$                | 259      |
| 942:447a  | $0, 0, 0, 0, 0, e^{23} + e^{14}, e^{24} + e^{13}, e^{27} + e^{16}, e^{47} + e^{36} + e^{15}$                 | 259      |
| 942:447b  | $0, 0, 0, 0, 0, -e^{14} - e^{23}, -e^{13} + e^{24}, e^{16} + e^{27}, e^{15} + e^{47} + e^{36}$               | 259      |
| 942:448a  | $0, 0, 0, 0, 0, e^{23} + e^{14}, e^{24} + e^{13}, e^{27} + e^{16}, e^{37} + e^{46} + e^{15}$                 | 259      |
| 942:448b  | $0, 0, 0, 0, 0, e^{23} - e^{14}, e^{24} + e^{13}, e^{27} + e^{16}, e^{15} + e^{37} + e^{46}$                 | 259      |
| 942:449   | $0, 0, 0, 0, 0, e^{12}, e^{24} + e^{13}, e^{15} + e^{26} + e^{34}, e^{36} + e^{14} + e^{27}$                 | 259      |
| 942:450   | $0, 0, 0, 0, 0, e^{12}, e^{13} + e^{24}, e^{45} + e^{23} + e^{16}, e^{27} + e^{36} + e^{14}$                 | 259      |
| 942:451a  | $0, 0, 0, 0, 0, e^{12}, e^{24} + e^{13}, e^{16} + e^{25} + e^{34}, e^{27} + e^{36} + e^{14}$                 | 259      |
| 942:451b  | $0, 0, 0, 0, 0, e^{12}, e^{13} + e^{24}, e^{25} - e^{16} + e^{34}, e^{27} + e^{14} + e^{36}$                 | 259      |
| 942:452   | $0, 0, 0, 0, 0, -e^{12}, -e^{13} + e^{24}, e^{23} + e^{17} + e^{46}, e^{14} + e^{27} + e^{36}$               | 359      |
| 942:453   | $0, 0, 0, 0, 0, -e^{12}, -e^{13} + e^{24}, e^{46} + e^{17} + e^{23}, e^{36} + e^{27} + e^{15}$               | 259      |
| 942:454   | $0, 0, 0, 0, 0, -e^{12}, -e^{13} + e^{24}, e^{27} + e^{36} + e^{14}, e^{17} + e^{46} + e^{35}$               | 259      |
| 942:455a  | $0, 0, 0, 0, 0, -e^{24} + e^{13}, e^{34} + e^{12}, e^{15} + e^{37} + e^{26}, e^{47} + e^{16} + e^{25}$       | 259      |
| 942:455b  | $0, 0, 0, 0, 0, -e^{24} + e^{13}, e^{12} + e^{34}, e^{37} + e^{26} - e^{15}, e^{47} + e^{25} + e^{16}$       | 259      |
| 942:455c  | $0, 0, 0, 0, 0, -e^{13}, e^{34} - e^{12}, e^{15} + e^{26} + e^{37}, e^{16} + e^{25} + e^{47}$                | 259      |
| 942:455d  | $0, 0, 0, 0, 0, -e^{13} + e^{24}, -e^{12} + e^{34}, e^{26} - e^{15} + e^{37}, e^{25} + e^{16} + e^{47}$      | 259      |
| 942:456a  | $0, 0, 0, 0, 0, e^{24} + e^{13}, -e^{12} + e^{34}, e^{36} + e^{15} + e^{27}, e^{47} + e^{16} + e^{25}$       | 259      |
| 942:456b  | $0, 0, 0, 0, 0, e^{24} - e^{13}, e^{34} - e^{12}, e^{15} + e^{27} + e^{36}, e^{16} + e^{25} + e^{47}$        | 259      |
| 942:457a  | $0, 0, 0, 0, 0, e^{24} - e^{13}, e^{12} + e^{34}, e^{36} + e^{15} + e^{27}, e^{46} + e^{17} + e^{25}$        | 259      |
| 942:457b  | $0, 0, 0, 0, 0, e^{24} - e^{13}, e^{34} + e^{12}, e^{27} + e^{36} - e^{15}, e^{17} + e^{46} + e^{25}$        | 259      |
| 942:457c  | $0, 0, 0, 0, 0, -e^{13} + e^{24}, e^{34} - e^{12}, e^{36} + e^{27} + e^{15}, e^{46} + e^{17} + e^{25}$       | 259      |
| 942:457d  | $0, 0, 0, 0, 0, e^{24} - e^{13}, -e^{12} + e^{34}, e^{36} + e^{27} - e^{15}, e^{25} + e^{17} + e^{46}$       | 259      |
| 942:458a  | $0, 0, 0, 0, 0, e^{23}a_1 + e^{14}, e^{13}a_1 + e^{24}, e^{26} + e^{35} + e^{17}, e^{27} + e^{45} + e^{16}$  | 259      |
| 942:458b  | $0, 0, 0, 0, 0, e^{23}a_1 - e^{14}, e^{13}a_1 + e^{24}, e^{26} - e^{17} + e^{35}, e^{16} + e^{45} + e^{27}$  | 259      |
| 942:459a  | $0, 0, 0, 0, 0, a_3e^{23} + e^{14}, a_3e^{13} + e^{24}, e^{16} + e^{27} + e^{35}, e^{45} + e^{17} + e^{26}$  | 259      |
| 942:459b  | $0, 0, 0, 0, 0, a_3e^{23} + e^{14}, -a_3e^{13} + e^{24}, e^{27} - e^{16} + e^{35}, e^{17} + e^{26} + e^{45}$ | 259      |
| 942:460a  | $0, 0, 0, 0, 0, -e^{24} + e^{13}, e^{12} + e^{34}, e^{37} + e^{26} + e^{14}, e^{47} + e^{16} + e^{23}$       | 359      |
| 942:460b  | $0, 0, 0, 0, 0, e^{24} - e^{13}, e^{34} - e^{12}, e^{26} + e^{37} + e^{14}, e^{16} + e^{47} + e^{23}$        | 359      |
| 942:461a  | $0, 0, 0, 0, 0, -e^{24} + e^{13}, e^{34} + e^{12}, e^{23} + e^{47} + e^{16}, e^{26} + e^{37} + e^{15}$       | 259      |
| 942:461b  | $0, 0, 0, 0, 0, -e^{13} + e^{24}, e^{34} - e^{12}, e^{47} + e^{23} + e^{16}, e^{37} + e^{26} + e^{15}$       | 259      |
| 942:462a  | $0, 0, 0, 0, 0, e^{24} + e^{13}, e^{34} + e^{12}, e^{14} + e^{36} + e^{27}, e^{15} + e^{37} + e^{26}$        | 259      |
| 942:462b  | $0, 0, 0, 0, 0, -e^{24} + e^{13}, e^{34} + e^{12}, -e^{27} + e^{36} + e^{14}, e^{26} + e^{37} + e^{15}$      | 259      |
| 942:463a  | $0, 0, 0, 0, 0, e^{13} + e^{24}, -e^{12} + e^{34}, e^{23} + e^{16} + e^{47}, e^{27} + e^{15} + e^{36}$       | 259      |
| 942:463b  | $0, 0, 0, 0, 0, -e^{13} + e^{24}, e^{34} - e^{12}, e^{47} + e^{23} + e^{16}, e^{27} + e^{36} + e^{15}$       | 259      |
| 942:464a  | $0, 0, 0, 0, 0, e^{24} + e^{13}, e^{34} + e^{12}, e^{14} + e^{37} + e^{26}, e^{15} + e^{36} + e^{27}$        | 259      |
| 942:464b  | $0, 0, 0, 0, 0, e^{24} - e^{13}, e^{34} + e^{12}, -e^{26} + e^{37} + e^{14}, e^{27} + e^{36} + e^{15}$       | 259      |
| Type: 531 |                                                                                                              |          |
| 941:1     | $0, 0, 0, 0, 0, e^{12}, e^{13}, e^{23}, e^{16}$                                                              | 579      |
| 941:2     | $0, 0, 0, 0, 0, e^{12}, e^{13}, e^{34}, e^{16}$                                                              | 479      |
| 941:3     | $0, 0, 0, 0, 0, e^{12}, e^{13}, e^{34}, e^{26}$                                                              | 479      |
| 941:4     | $0, 0, 0, 0, 0, e^{12}, e^{34}, e^{35}, e^{16}$                                                              | 379      |
| 941:5     | $0, 0, 0, 0, 0, e^{12}, e^{13}, e^{14}, e^{16}$                                                              | 479      |
| 941:6     | $0, 0, 0, 0, 0, e^{12}, e^{13}, e^{14}, e^{26}$                                                              | 479      |

Table 2 – Continued to next page



Table 2 – Continued from previous page

| Name    | $\mathfrak{g}$                                                    | UCS Dim. |
|---------|-------------------------------------------------------------------|----------|
| 941:7   | $0, 0, 0, 0, 0, e^{12}, e^{13}, e^{24}, e^{16}$                   | 479      |
| 941:8   | $0, 0, 0, 0, 0, e^{12}, e^{13}, e^{45}, e^{16}$                   | 379      |
| 941:9   | $0, 0, 0, 0, 0, e^{12}, e^{13}, e^{45}, e^{26}$                   | 379      |
| 941:10  | $0, 0, 0, 0, 0, e^{12}, e^{34}, e^{13} + e^{24}, e^{16}$          | 479      |
| 941:11  | $0, 0, 0, 0, 0, e^{12}, e^{34}, e^{13} + e^{45}, e^{16}$          | 379      |
| 941:12  | $0, 0, 0, 0, 0, e^{12}, e^{34}, e^{13} + e^{45}, e^{26}$          | 379      |
| 941:13  | $0, 0, 0, 0, 0, e^{12}, e^{34}, e^{35}, e^{45} + e^{16}$          | 379      |
| 941:14  | $0, 0, 0, 0, 0, e^{12}, e^{13}, e^{23}, e^{16} + e^{34}$          | 479      |
| 941:15  | $0, 0, 0, 0, 0, e^{12}, e^{13}, e^{23} + e^{14}, e^{16}$          | 479      |
| 941:16  | $0, 0, 0, 0, 0, e^{12}, e^{13}, e^{23} + e^{14}, e^{26}$          | 479      |
| 941:17  | $0, 0, 0, 0, 0, e^{12}, e^{13}, e^{34}, e^{16} + e^{23}$          | 479      |
| 941:18  | $0, 0, 0, 0, 0, e^{12}, e^{13}, e^{14}, e^{16} + e^{34}$          | 479      |
| 941:19  | $0, 0, 0, 0, 0, e^{12}, e^{13}, e^{14}, e^{34} + e^{26}$          | 479      |
| 941:20  | $0, 0, 0, 0, 0, e^{12}, e^{13}, e^{24}, e^{16} + e^{34}$          | 479      |
| 941:21  | $0, 0, 0, 0, 0, e^{12}, e^{13}, e^{34}, e^{26} + e^{14}$          | 479      |
| 941:22  | $0, 0, 0, 0, 0, e^{12}, e^{13}, e^{34}, e^{16} + e^{24}$          | 479      |
| 941:23  | $0, 0, 0, 0, 0, e^{12}, e^{13}, e^{34}, e^{35} + e^{16}$          | 379      |
| 941:24  | $0, 0, 0, 0, 0, e^{12}, e^{13}, e^{34}, e^{26} + e^{35}$          | 379      |
| 941:25  | $0, 0, 0, 0, 0, e^{12}, e^{13}, e^{34}, e^{16} + e^{45}$          | 379      |
| 941:26  | $0, 0, 0, 0, 0, e^{12}, e^{13}, e^{34}, e^{26} + e^{45}$          | 379      |
| 941:27  | $0, 0, 0, 0, 0, e^{12}, e^{13}, e^{35} + e^{14}, e^{16}$          | 379      |
| 941:28  | $0, 0, 0, 0, 0, e^{12}, e^{13}, e^{35} + e^{14}, e^{26}$          | 379      |
| 941:29  | $0, 0, 0, 0, 0, e^{12}, e^{13}, e^{45} + e^{23}, e^{16}$          | 379      |
| 941:30  | $0, 0, 0, 0, 0, e^{12}, e^{13}, e^{24} + e^{35}, e^{16}$          | 379      |
| 941:31  | $0, 0, 0, 0, 0, e^{12}, e^{13}, e^{45} + e^{23}, e^{26}$          | 379      |
| 941:32  | $0, 0, 0, 0, 0, e^{12}, e^{13}, e^{35} + e^{24}, e^{26}$          | 379      |
| 941:33  | $0, 0, 0, 0, 0, e^{12}, e^{13}, e^{45}, e^{16} + e^{34}$          | 379      |
| 941:34  | $0, 0, 0, 0, 0, e^{12}, e^{13}, e^{45}, e^{34} + e^{26}$          | 379      |
| 941:35  | $0, 0, 0, 0, 0, e^{12}, e^{34}, e^{13} + e^{25}, e^{16}$          | 379      |
| 941:36  | $0, 0, 0, 0, 0, e^{12}, e^{34}, e^{23} + e^{15}, e^{16}$          | 379      |
| 941:37  | $0, 0, 0, 0, 0, e^{12}, e^{34}, e^{35}, e^{13} + e^{26}$          | 379      |
| 941:38  | $0, 0, 0, 0, 0, e^{12}, e^{34}, e^{35}, e^{14} + e^{26}$          | 379      |
| 941:39  | $0, 0, 0, 0, 0, e^{12}, e^{34}, e^{13} + e^{45}, e^{35} + e^{16}$ | 379      |
| 941:40  | $0, 0, 0, 0, 0, e^{12}, e^{34}, e^{45} + e^{13}, e^{26} + e^{35}$ | 379      |
| 941:41a | $0, 0, 0, 0, 0, e^{12}, e^{14} + e^{35}, e^{45} + e^{13}, e^{16}$ | 379      |
| 941:41b | $0, 0, 0, 0, 0, e^{12}, e^{35} - e^{14}, e^{45} + e^{13}, e^{16}$ | 379      |
| 941:42a | $0, 0, 0, 0, 0, e^{12}, e^{14} + e^{35}, e^{13} + e^{45}, e^{26}$ | 379      |
| 941:42b | $0, 0, 0, 0, 0, e^{12}, e^{35} - e^{14}, e^{13} + e^{45}, e^{26}$ | 379      |
| 941:43  | $0, 0, 0, 0, 0, e^{12}, e^{35} + e^{14}, e^{45} + e^{23}, e^{16}$ | 379      |
| 941:44  | $0, 0, 0, 0, 0, e^{12}, e^{13}, e^{23}, e^{14} + e^{26}$          | 479      |
| 941:45  | $0, 0, 0, 0, 0, e^{12}, e^{13}, e^{14}, e^{16} + e^{23}$          | 479      |
| 941:46  | $0, 0, 0, 0, 0, e^{12}, e^{13}, e^{24}, e^{16} + e^{23}$          | 479      |
| 941:47  | $0, 0, 0, 0, 0, e^{12}, e^{13}, e^{23}, e^{16} + e^{45}$          | 379      |
| 941:48  | $0, 0, 0, 0, 0, e^{12}, e^{13}, e^{14}, e^{16} + e^{35}$          | 379      |
| 941:49  | $0, 0, 0, 0, 0, e^{12}, e^{13}, e^{14}, e^{35} + e^{26}$          | 379      |
| 941:50  | $0, 0, 0, 0, 0, e^{12}, e^{13}, e^{24}, e^{35} + e^{16}$          | 379      |
| 941:51  | $0, 0, 0, 0, 0, e^{12}, e^{13}, e^{24}, e^{26} + e^{35}$          | 379      |
| 941:52  | $0, 0, 0, 0, 0, e^{12}, e^{13}, e^{34}, e^{26} + e^{15}$          | 379      |
| 941:53  | $0, 0, 0, 0, 0, e^{12}, e^{13}, e^{34}, e^{16} + e^{25}$          | 379      |
| 941:54  | $0, 0, 0, 0, 0, e^{12}, e^{13}, e^{25} + e^{14}, e^{16}$          | 379      |
| 941:55  | $0, 0, 0, 0, 0, e^{12}, e^{13}, e^{14} + e^{25}, e^{26}$          | 379      |
| 941:56  | $0, 0, 0, 0, 0, e^{12}, e^{13}, e^{45}, e^{23} + e^{16}$          | 379      |
| 941:57  | $0, 0, 0, 0, 0, e^{12}, e^{13}, e^{45}, e^{26} + e^{14}$          | 379      |
| 941:58  | $0, 0, 0, 0, 0, e^{12}, e^{13}, e^{45}, e^{24} + e^{16}$          | 379      |
| 941:59  | $0, 0, 0, 0, 0, e^{12}, e^{13}, e^{14} + e^{23}, e^{34} + e^{16}$ | 479      |
| 941:60  | $0, 0, 0, 0, 0, e^{12}, e^{13}, e^{14} + e^{23}, e^{26} + e^{34}$ | 479      |
| 941:61a | $0, 0, 0, 0, 0, e^{12}, e^{23} + e^{14}, e^{24} + e^{13}, e^{16}$ | 479      |
| 941:61b | $0, 0, 0, 0, 0, e^{12}, e^{23} - e^{14}, e^{24} + e^{13}, e^{16}$ | 479      |

Table 2 – Continued to next page

Table 2 – Continued from previous page

| Name    | $\mathfrak{g}$                                                             | UCS Dim. |
|---------|----------------------------------------------------------------------------|----------|
| 941:62  | $0, 0, 0, 0, 0, e^{12}, e^{34}, e^{14} + e^{23}, e^{26} + e^{13}$          | 479      |
| 941:63  | $0, 0, 0, 0, 0, e^{12}, e^{34}, e^{13} + e^{24}, e^{35} + e^{16}$          | 379      |
| 941:64  | $0, 0, 0, 0, 0, e^{12}, e^{34}, e^{23} + e^{14}, e^{35} + e^{16}$          | 379      |
| 941:65  | $0, 0, 0, 0, 0, e^{12}, e^{13}, e^{35} + e^{14}, e^{16} + e^{34}$          | 379      |
| 941:66  | $0, 0, 0, 0, 0, e^{12}, e^{13}, e^{35} + e^{14}, e^{26} + e^{34}$          | 379      |
| 941:67  | $0, 0, 0, 0, 0, e^{12}, e^{13}, e^{45} + e^{23}, e^{34} + e^{16}$          | 379      |
| 941:68  | $0, 0, 0, 0, 0, e^{12}, e^{13}, e^{35} + e^{24}, e^{34} + e^{16}$          | 379      |
| 941:69  | $0, 0, 0, 0, 0, e^{12}, e^{13}, e^{45} + e^{23}, e^{26} + e^{34}$          | 379      |
| 941:70  | $0, 0, 0, 0, 0, e^{12}, e^{13}, e^{24} + e^{35}, e^{26} + e^{34}$          | 379      |
| 941:71  | $0, 0, 0, 0, 0, e^{12}, e^{13} + e^{24}, e^{35}, e^{16} + e^{34}$          | 379      |
| 941:72  | $0, 0, 0, 0, 0, e^{12}, e^{14} + e^{23}, e^{35}, e^{16} + e^{34}$          | 379      |
| 941:73  | $0, 0, 0, 0, 0, e^{12}, e^{23} + e^{14}, e^{13} + e^{45}, e^{16}$          | 379      |
| 941:74  | $0, 0, 0, 0, 0, e^{12}, e^{24} + e^{13}, e^{34} + e^{15}, e^{16}$          | 379      |
| 941:75  | $0, 0, 0, 0, 0, e^{12}, e^{14} + e^{23}, e^{13} + e^{45}, e^{26}$          | 379      |
| 941:76  | $0, 0, 0, 0, 0, e^{12}, e^{24} + e^{13}, e^{34} + e^{15}, e^{26}$          | 379      |
| 941:77  | $0, 0, 0, 0, 0, e^{12}, e^{34}, e^{35} + e^{14}, e^{26} + e^{13}$          | 379      |
| 941:78  | $0, 0, 0, 0, 0, e^{12}, e^{34}, e^{13} + e^{45}, e^{16} + e^{23}$          | 379      |
| 941:79  | $0, 0, 0, 0, 0, e^{12}, e^{34}, e^{14} + e^{35}, e^{23} + e^{16}$          | 379      |
| 941:80  | $0, 0, 0, 0, 0, e^{12}, e^{13}, e^{14} + e^{35}, e^{16} + e^{45}$          | 379      |
| 941:81  | $0, 0, 0, 0, 0, e^{12}, e^{13}, e^{35} + e^{14}, e^{45} + e^{26}$          | 379      |
| 941:82  | $0, 0, 0, 0, 0, e^{12}, e^{13}, e^{24} + e^{35}, e^{16} + e^{45}$          | 379      |
| 941:83  | $0, 0, 0, 0, 0, e^{12}, e^{13}, e^{35} + e^{24}, e^{45} + e^{26}$          | 379      |
| 941:84  | $0, 0, 0, 0, 0, e^{12}, e^{34}, e^{13} + e^{25}, e^{45} + e^{16}$          | 379      |
| 941:85  | $0, 0, 0, 0, 0, e^{12}, e^{34}, e^{15} + e^{23}, e^{16} + e^{45}$          | 379      |
| 941:86  | $0, 0, 0, 0, 0, e^{12}, e^{34}, e^{35}, e^{26} + e^{13} + e^{45}$          | 379      |
| 941:87  | $0, 0, 0, 0, 0, e^{12}, e^{34}, e^{13} + e^{45}, e^{26} + e^{15}$          | 379      |
| 941:88  | $0, 0, 0, 0, 0, e^{12}, e^{34}, e^{45} + e^{13}, e^{25} + e^{16}$          | 379      |
| 941:89a | $0, 0, 0, 0, 0, e^{12}, e^{35} + e^{14}, e^{13} + e^{45}, e^{16} + e^{34}$ | 379      |
| 941:89b | $0, 0, 0, 0, 0, e^{12}, e^{35} - e^{14}, e^{45} + e^{13}, e^{34} + e^{16}$ | 379      |
| 941:90a | $0, 0, 0, 0, 0, e^{12}, e^{14} + e^{35}, e^{13} + e^{45}, e^{26} + e^{34}$ | 379      |
| 941:90b | $0, 0, 0, 0, 0, e^{12}, e^{35} - e^{14}, e^{45} + e^{13}, e^{26} + e^{34}$ | 379      |
| 941:91  | $0, 0, 0, 0, 0, e^{12}, e^{35} + e^{14}, e^{45} + e^{23}, e^{16} + e^{34}$ | 379      |
| 941:92  | $0, 0, 0, 0, 0, e^{12}, e^{13}, e^{14}, e^{15} + e^{26}$                   | 379      |
| 941:93  | $0, 0, 0, 0, 0, e^{12}, e^{13}, e^{14}, e^{25} + e^{16}$                   | 379      |
| 941:94  | $0, 0, 0, 0, 0, e^{12}, e^{13}, e^{24}, e^{26} + e^{15}$                   | 379      |
| 941:95  | $0, 0, 0, 0, 0, e^{12}, e^{13}, e^{23} + e^{14}, e^{24} + e^{16}$          | 479      |
| 941:96  | $0, 0, 0, 0, 0, e^{12}, e^{13}, e^{14} + e^{23}, e^{35} + e^{16}$          | 379      |
| 941:97  | $0, 0, 0, 0, 0, e^{12}, e^{13}, e^{14} + e^{23}, e^{35} + e^{26}$          | 379      |
| 941:98  | $0, 0, 0, 0, 0, e^{12}, e^{13}, e^{14} + e^{23}, e^{45} + e^{16}$          | 379      |
| 941:99  | $0, 0, 0, 0, 0, e^{12}, e^{13}, e^{23} + e^{14}, e^{26} + e^{45}$          | 379      |
| 941:100 | $0, 0, 0, 0, 0, e^{12}, e^{13}, e^{34}, e^{14} + e^{26} + e^{35}$          | 379      |
| 941:101 | $0, 0, 0, 0, 0, e^{12}, e^{13}, e^{34}, e^{23} + e^{16} + e^{45}$          | 379      |
| 941:102 | $0, 0, 0, 0, 0, e^{12}, e^{13}, e^{34}, e^{16} + e^{35} + e^{24}$          | 379      |
| 941:103 | $0, 0, 0, 0, 0, e^{12}, e^{34}, e^{24} + e^{13}, e^{15} + e^{26}$          | 379      |
| 941:104 | $0, 0, 0, 0, 0, e^{12}, e^{13}, e^{35} + e^{14}, e^{16} + e^{23}$          | 379      |
| 941:105 | $0, 0, 0, 0, 0, e^{12}, e^{13}, e^{24} + e^{35}, e^{23} + e^{16}$          | 379      |
| 941:106 | $0, 0, 0, 0, 0, e^{12}, e^{13}, e^{25} + e^{14}, e^{16} + e^{34}$          | 379      |
| 941:107 | $0, 0, 0, 0, 0, e^{12}, e^{13}, e^{15} + e^{24}, e^{16} + e^{34}$          | 379      |
| 941:108 | $0, 0, 0, 0, 0, e^{12}, e^{13}, e^{14} + e^{25}, e^{26} + e^{34}$          | 379      |
| 941:109 | $0, 0, 0, 0, 0, e^{12}, e^{13}, e^{15} + e^{24}, e^{26} + e^{34}$          | 379      |
| 941:110 | $0, 0, 0, 0, 0, e^{12}, e^{13}, e^{34} + e^{15}, e^{26} + e^{14}$          | 379      |
| 941:111 | $0, 0, 0, 0, 0, e^{12}, e^{13}, e^{35} + e^{14}, e^{24} + e^{16}$          | 379      |
| 941:112 | $0, 0, 0, 0, 0, e^{12}, e^{13}, e^{34} + e^{15}, e^{24} + e^{16}$          | 379      |
| 941:113 | $0, 0, 0, 0, 0, e^{12}, e^{13}, e^{45} + e^{23}, e^{14} + e^{26}$          | 379      |
| 941:114 | $0, 0, 0, 0, 0, e^{12}, e^{13}, e^{35} + e^{24}, e^{14} + e^{26}$          | 379      |
| 941:115 | $0, 0, 0, 0, 0, e^{12}, e^{13}, e^{25} + e^{34}, e^{26} + e^{14}$          | 379      |
| 941:116 | $0, 0, 0, 0, 0, e^{12}, e^{13}, e^{23} + e^{45}, e^{16} + e^{24}$          | 379      |
| 941:117 | $0, 0, 0, 0, 0, e^{12}, e^{13}, e^{34} + e^{25}, e^{16} + e^{24}$          | 379      |

Table 2 – Continued to next page

Table 2 – Continued from previous page

| Name     | $\mathfrak{g}$                                                              | UCS Dim. |
|----------|-----------------------------------------------------------------------------|----------|
| 941:118  | $0, 0, 0, 0, 0, e^{12}, e^{23} + e^{14}, e^{25} + e^{13}, e^{16}$           | 379      |
| 941:119  | $0, 0, 0, 0, 0, e^{12}, e^{34}, e^{23} + e^{15}, e^{13} + e^{26}$           | 379      |
| 941:120  | $0, 0, 0, 0, 0, e^{12}, e^{24} + e^{13}, e^{15}, e^{34} + e^{16}$           | 379      |
| 941:121  | $0, 0, 0, 0, 0, e^{12}, e^{13} + e^{24}, e^{15}, e^{26} + e^{34}$           | 379      |
| 941:122  | $0, 0, 0, 0, 0, e^{12}, e^{34}, e^{25} + e^{13}, e^{26} + e^{14}$           | 379      |
| 941:123  | $0, 0, 0, 0, 0, e^{12}, e^{34}, e^{15} + e^{23}, e^{26} + e^{14}$           | 379      |
| 941:124  | $0, 0, 0, 0, 0, e^{12}, e^{24} + e^{13}, e^{35}, e^{14} + e^{26}$           | 379      |
| 941:125  | $0, 0, 0, 0, 0, e^{12}, e^{13}, e^{45}, e^{35} + e^{14} + e^{26}$           | 379      |
| 941:126  | $0, 0, 0, 0, 0, e^{12}, e^{13}, e^{45}, e^{35} + e^{24} + e^{16}$           | 379      |
| 941:127a | $0, 0, 0, 0, 0, e^{12}, e^{23} + e^{14}, e^{24} + e^{13}, e^{16} + e^{34}$  | 479      |
| 941:127b | $0, 0, 0, 0, 0, e^{12}, -e^{14} + e^{23}, e^{24} + e^{13}, e^{34} + e^{16}$ | 479      |
| 941:128  | $0, 0, 0, 0, 0, e^{12}, e^{14} + e^{23}, e^{45} + e^{13}, e^{34} + e^{16}$  | 379      |
| 941:129  | $0, 0, 0, 0, 0, e^{12}, e^{14} + e^{23}, e^{13} + e^{45}, e^{26} + e^{34}$  | 379      |
| 941:130  | $0, 0, 0, 0, 0, e^{12}, e^{23} + e^{14}, e^{45} + e^{13}, e^{16} + e^{35}$  | 379      |
| 941:131  | $0, 0, 0, 0, 0, e^{12}, e^{24} + e^{13}, e^{15} + e^{34}, e^{16} + e^{35}$  | 379      |
| 941:132  | $0, 0, 0, 0, 0, e^{12}, e^{14} + e^{23}, e^{15} + e^{34}, e^{16} + e^{35}$  | 379      |
| 941:133  | $0, 0, 0, 0, 0, e^{12}, e^{14} + e^{23}, e^{13} + e^{45}, e^{35} + e^{26}$  | 379      |
| 941:134  | $0, 0, 0, 0, 0, e^{12}, e^{24} + e^{13}, e^{15} + e^{34}, e^{35} + e^{26}$  | 379      |
| 941:135  | $0, 0, 0, 0, 0, e^{12}, e^{14} + e^{23}, e^{34} + e^{15}, e^{26} + e^{35}$  | 379      |
| 941:136a | $0, 0, 0, 0, 0, e^{12}, e^{34}, e^{13} + e^{45}, e^{14} + e^{26} + e^{35}$  | 379      |
| 941:136b | $0, 0, 0, 0, 0, e^{12}, e^{34}, e^{45} - e^{13}, e^{26} + e^{35} + e^{14}$  | 379      |
| 941:137  | $0, 0, 0, 0, 0, e^{12}, e^{34}, e^{45} + e^{13}, e^{16} + e^{35} + e^{24}$  | 379      |
| 941:138a | $0, 0, 0, 0, 0, e^{12}, e^{15} + e^{34}, e^{14} + e^{35}, e^{26} + e^{13}$  | 379      |
| 941:138b | $0, 0, 0, 0, 0, e^{12}, -e^{15} + e^{34}, e^{14} + e^{35}, e^{13} + e^{26}$ | 379      |
| 941:139a | $0, 0, 0, 0, 0, e^{12}, e^{14} + e^{35}, e^{13} + e^{45}, e^{16} + e^{23}$  | 379      |
| 941:139b | $0, 0, 0, 0, 0, e^{12}, e^{35} - e^{14}, e^{13} + e^{45}, e^{23} + e^{16}$  | 379      |
| 941:140a | $0, 0, 0, 0, 0, e^{12}, e^{34} + e^{15}, e^{35} + e^{14}, e^{16} + e^{23}$  | 379      |
| 941:140b | $0, 0, 0, 0, 0, e^{12}, e^{34} - e^{15}, e^{35} + e^{14}, e^{23} + e^{16}$  | 379      |
| 941:141  | $0, 0, 0, 0, 0, e^{12}, e^{14} + e^{35}, e^{45} + e^{23}, e^{26} + e^{13}$  | 379      |
| 941:142  | $0, 0, 0, 0, 0, e^{12}, e^{15} + e^{34}, e^{35} + e^{24}, e^{26} + e^{13}$  | 379      |
| 941:143  | $0, 0, 0, 0, 0, e^{12}, e^{13}, e^{23}, e^{14} + e^{26} + e^{35}$           | 379      |
| 941:144  | $0, 0, 0, 0, 0, e^{12}, e^{13}, e^{14} + e^{23}, e^{26} + e^{15}$           | 379      |
| 941:145  | $0, 0, 0, 0, 0, e^{12}, e^{13}, e^{23} + e^{14}, e^{25} + e^{16}$           | 379      |
| 941:146  | $0, 0, 0, 0, 0, e^{12}, e^{13}, e^{14}, e^{15} + e^{26} + e^{34}$           | 379      |
| 941:147  | $0, 0, 0, 0, 0, e^{12}, e^{13}, e^{14}, e^{45} + e^{16} + e^{23}$           | 379      |
| 941:148  | $0, 0, 0, 0, 0, e^{12}, e^{13}, e^{14}, e^{25} + e^{16} + e^{34}$           | 379      |
| 941:149  | $0, 0, 0, 0, 0, e^{12}, e^{13}, e^{24}, e^{26} + e^{35} + e^{14}$           | 379      |
| 941:150  | $0, 0, 0, 0, 0, e^{12}, e^{13}, e^{24}, e^{15} + e^{26} + e^{34}$           | 379      |
| 941:151  | $0, 0, 0, 0, 0, e^{12}, e^{13}, e^{14} + e^{25}, e^{16} + e^{23}$           | 379      |
| 941:152  | $0, 0, 0, 0, 0, e^{12}, e^{13}, e^{15} + e^{24}, e^{14} + e^{26}$           | 379      |
| 941:153  | $0, 0, 0, 0, 0, e^{12}, e^{13}, e^{14} + e^{25}, e^{16} + e^{24}$           | 379      |
| 941:154a | $0, 0, 0, 0, 0, e^{12}, e^{23} + e^{14}, e^{24} + e^{13}, e^{35} + e^{16}$  | 379      |
| 941:154b | $0, 0, 0, 0, 0, e^{12}, -e^{14} + e^{23}, e^{24} + e^{13}, e^{35} + e^{16}$ | 379      |
| 941:155  | $0, 0, 0, 0, 0, e^{12}, e^{34}, e^{13} + e^{24}, e^{35} + e^{14} + e^{26}$  | 379      |
| 941:156  | $0, 0, 0, 0, 0, e^{12}, e^{14} + e^{23}, e^{13} + e^{25}, e^{34} + e^{16}$  | 379      |
| 941:157  | $0, 0, 0, 0, 0, e^{12}, e^{24} + e^{13}, e^{15} + e^{23}, e^{16} + e^{34}$  | 379      |
| 941:158  | $0, 0, 0, 0, 0, e^{12}, e^{14} + e^{23}, e^{15} + e^{34}, e^{26} + e^{13}$  | 379      |
| 941:159  | $0, 0, 0, 0, 0, e^{12}, e^{13} + e^{24}, e^{35} + e^{14}, e^{23} + e^{16}$  | 379      |
| 941:160  | $0, 0, 0, 0, 0, e^{12}, e^{13} + e^{24}, e^{15} + e^{34}, e^{16} + e^{23}$  | 379      |
| 941:161a | $0, 0, 0, 0, 0, e^{12}, e^{13}, e^{35} + e^{14}, e^{15} + e^{26} + e^{34}$  | 379      |
| 941:161b | $0, 0, 0, 0, 0, e^{12}, e^{13}, e^{35} - e^{14}, e^{26} + e^{34} + e^{15}$  | 379      |
| 941:162  | $0, 0, 0, 0, 0, e^{12}, e^{13}, e^{14} + e^{35}, e^{23} + e^{16} + e^{45}$  | 379      |
| 941:163  | $0, 0, 0, 0, 0, e^{12}, e^{13}, e^{35} + e^{14}, e^{16} + e^{34} + e^{25}$  | 379      |
| 941:164  | $0, 0, 0, 0, 0, e^{12}, e^{13}, e^{45} + e^{23}, e^{26} + e^{35} + e^{14}$  | 379      |
| 941:165a | $0, 0, 0, 0, 0, e^{12}, e^{13}, e^{23} + e^{45}, e^{16} + e^{24} + e^{35}$  | 379      |
| 941:165b | $0, 0, 0, 0, 0, e^{12}, e^{13}, -e^{23} + e^{45}, e^{16} + e^{24} + e^{35}$ | 379      |
| 941:166  | $0, 0, 0, 0, 0, e^{12}, e^{13}, e^{35} + e^{24}, e^{34} + e^{26} + e^{15}$  | 379      |
| 941:167a | $0, 0, 0, 0, 0, e^{12}, e^{13}, e^{35} + e^{24}, e^{23} + e^{45} + e^{16}$  | 379      |

Table 2 – Continued to next page

Table 2 – Continued from previous page

| Name     | $\mathfrak{g}$                                                                       | UCS Dim. |
|----------|--------------------------------------------------------------------------------------|----------|
| 941:167b | $0, 0, 0, 0, 0, e^{12}, e^{13}, -e^{24} + e^{35}, e^{16} + e^{23} + e^{45}$          | 379      |
| 941:168a | $0, 0, 0, 0, 0, e^{12}, e^{13}, e^{35} + e^{24}, e^{34} + e^{25} + e^{16}$           | 379      |
| 941:168b | $0, 0, 0, 0, 0, e^{12}, e^{13}, e^{35} - e^{24}, e^{34} + e^{16} + e^{25}$           | 379      |
| 941:169  | $0, 0, 0, 0, 0, e^{12}, e^{23} + e^{14}, e^{25} + e^{13}, e^{16} + e^{45}$           | 379      |
| 941:170  | $0, 0, 0, 0, 0, e^{12}, e^{34}, e^{25} + e^{13}, e^{14} + e^{26} + e^{35}$           | 379      |
| 941:171  | $0, 0, 0, 0, 0, e^{12}, e^{34}, e^{13} + e^{25}, e^{45} + e^{23} + e^{16}$           | 379      |
| 941:172  | $0, 0, 0, 0, 0, e^{12}, e^{34}, e^{25} + e^{13}, e^{35} + e^{24} + e^{16}$           | 379      |
| 941:173  | $0, 0, 0, 0, 0, e^{12}, e^{23} + e^{14}, e^{13} + e^{45}, e^{15} + e^{26}$           | 379      |
| 941:174  | $0, 0, 0, 0, 0, e^{12}, e^{14} + e^{23}, e^{45} + e^{13}, e^{25} + e^{16}$           | 379      |
| 941:175  | $0, 0, 0, 0, 0, e^{12}, e^{13} + e^{24}, e^{15} + e^{34}, e^{25} + e^{16}$           | 379      |
| 941:176a | $0, 0, 0, 0, 0, e^{12}, e^{35} + e^{14}, e^{45} + e^{13}, e^{26} + e^{34} + e^{15}$  | 379      |
| 941:176b | $0, 0, 0, 0, 0, e^{12}, e^{35} + e^{14}, e^{45} - e^{13}, e^{15} + e^{26} + e^{34}$  | 379      |
| 941:176c | $0, 0, 0, 0, 0, e^{12}, -e^{14} + e^{35}, e^{45} + e^{13}, e^{15} + e^{26} + e^{34}$ | 379      |
| 941:177a | $0, 0, 0, 0, 0, e^{12}, e^{35} + e^{14}, e^{45} + e^{13}, e^{34} + e^{25} + e^{16}$  | 379      |
| 941:177b | $0, 0, 0, 0, 0, e^{12}, -e^{14} + e^{35}, e^{13} + e^{45}, e^{16} + e^{34} + e^{25}$ | 379      |
| 941:178a | $0, 0, 0, 0, 0, e^{12}, e^{35} + e^{14}, e^{23} + e^{45}, e^{15} + e^{26} + e^{34}$  | 379      |
| 941:178b | $0, 0, 0, 0, 0, e^{12}, e^{35} - e^{14}, e^{23} + e^{45}, e^{26} + e^{34} + e^{15}$  | 379      |
| 941:179  | $0, 0, 0, 0, 0, e^{12}, e^{13}, e^{14} + e^{23}, e^{34} + e^{26} + e^{15}$           | 379      |
| 941:180  | $0, 0, 0, 0, 0, e^{12}, e^{13}, e^{14} + e^{23}, e^{35} + e^{16} + e^{24}$           | 379      |
| 941:181  | $0, 0, 0, 0, 0, e^{12}, e^{13}, e^{23} + e^{14}, e^{16} + e^{25} + e^{34}$           | 379      |
| 941:182a | $0, 0, 0, 0, 0, e^{12}, e^{14} + e^{23}, e^{24} + e^{13}, e^{15} + e^{26}$           | 379      |
| 941:182b | $0, 0, 0, 0, 0, e^{12}, -e^{14} + e^{23}, e^{13} + e^{24}, e^{26} + e^{15}$          | 379      |
| 941:183  | $0, 0, 0, 0, 0, e^{12}, e^{13} + e^{24}, e^{15} + e^{23}, e^{14} + e^{26}$           | 379      |
| 941:184  | $0, 0, 0, 0, 0, e^{12}, e^{13}, e^{14} + e^{25}, e^{15} + e^{26} + e^{34}$           | 379      |
| 941:185  | $0, 0, 0, 0, 0, e^{12}, e^{13}, e^{25} + e^{14}, e^{45} + e^{16} + e^{23}$           | 379      |
| 941:186  | $0, 0, 0, 0, 0, e^{12}, e^{13}, e^{25} + e^{14}, e^{16} + e^{24} + e^{35}$           | 379      |
| 941:187a | $0, 0, 0, 0, 0, e^{12}, e^{23} + e^{14}, e^{45} + e^{13}, e^{26} + e^{34} + e^{15}$  | 379      |
| 941:187b | $0, 0, 0, 0, 0, e^{12}, e^{23} + e^{14}, e^{45} - e^{13}, e^{15} + e^{26} + e^{34}$  | 379      |
| 941:188  | $0, 0, 0, 0, 0, e^{12}, e^{14} + e^{23}, e^{45} + e^{13}, e^{16} + e^{24} + e^{35}$  | 379      |
| 941:189  | $0, 0, 0, 0, 0, e^{12}, e^{14} + e^{23}, e^{13} + e^{45}, e^{25} + e^{16} + e^{34}$  | 379      |
| 941:190a | $0, 0, 0, 0, 0, e^{12}, e^{13} + e^{24}, e^{15} + e^{34}, e^{14} + e^{35} + e^{26}$  | 379      |
| 941:190b | $0, 0, 0, 0, 0, e^{12}, e^{24} + e^{13}, -e^{15} + e^{34}, e^{35} + e^{14} + e^{26}$ | 379      |
| 941:191  | $0, 0, 0, 0, 0, e^{12}, e^{24} + e^{13}, e^{34} + e^{15}, e^{16} + e^{23} + e^{45}$  | 379      |
| 941:192a | $0, 0, 0, 0, 0, e^{12}, e^{14} + e^{23}, e^{13} + e^{24}, e^{34} + e^{26} + e^{15}$  | 379      |
| 941:192b | $0, 0, 0, 0, 0, e^{12}, -e^{14} + e^{23}, e^{13} + e^{24}, e^{26} + e^{15} + e^{34}$ | 379      |
| 941:193  | $0, 0, 0, 0, 0, e^{12}, e^{23} + e^{14}, e^{25} + e^{13}, e^{15} + e^{26} + e^{34}$  | 379      |
| 941:194  | $0, 0, 0, 0, 0, e^{12}, e^{13}, e^{23}, e^{17} + e^{26}$                             | 469      |
| 941:195a | $0, 0, 0, 0, 0, e^{12}, e^{13}, e^{23}, e^{26} + e^{37}$                             | 469      |
| 941:195b | $0, 0, 0, 0, 0, -e^{12}, e^{13}, e^{23}, e^{26} + e^{37}$                            | 469      |
| 941:196  | $0, 0, 0, 0, 0, e^{12}, e^{13}, e^{23}, e^{36} + e^{27}$                             | 469      |
| 941:197  | $0, 0, 0, 0, 0, e^{12}, e^{13}, e^{14}, e^{26} + e^{17}$                             | 369      |
| 941:198  | $0, 0, 0, 0, 0, e^{12}, e^{13}, e^{24}, e^{17} + e^{26}$                             | 369      |
| 941:199a | $0, 0, 0, 0, 0, e^{12}, e^{13}, e^{14}, e^{26} + e^{37}$                             | 369      |
| 941:199b | $0, 0, 0, 0, 0, -e^{12}, e^{13}, e^{14}, e^{37} + e^{26}$                            | 369      |
| 941:200  | $0, 0, 0, 0, 0, e^{12}, e^{13}, e^{14}, e^{36} + e^{27}$                             | 369      |
| 941:201  | $0, 0, 0, 0, 0, e^{12}, e^{13}, e^{24}, e^{37} + e^{16}$                             | 369      |
| 941:202a | $0, 0, 0, 0, 0, e^{12}, e^{13}, e^{24}, e^{37} + e^{26}$                             | 369      |
| 941:202b | $0, 0, 0, 0, 0, -e^{12}, e^{13}, e^{24}, e^{37} + e^{26}$                            | 369      |
| 941:203  | $0, 0, 0, 0, 0, e^{12}, e^{13}, e^{24}, e^{27} + e^{36}$                             | 369      |
| 941:204  | $0, 0, 0, 0, 0, e^{12}, e^{13}, e^{45}, e^{17} + e^{26}$                             | 269      |
| 941:205a | $0, 0, 0, 0, 0, e^{12}, e^{13}, e^{45}, e^{26} + e^{37}$                             | 269      |
| 941:205b | $0, 0, 0, 0, 0, -e^{12}, e^{13}, e^{45}, e^{26} + e^{37}$                            | 269      |
| 941:206  | $0, 0, 0, 0, 0, e^{12}, e^{13}, e^{45}, e^{36} + e^{27}$                             | 269      |
| 941:207  | $0, 0, 0, 0, 0, e^{12}, e^{13}, e^{14} + e^{23}, e^{26} + e^{17}$                    | 369      |
| 941:208a | $0, 0, 0, 0, 0, e^{12}, e^{13}, e^{23} + e^{14}, e^{26} + e^{37}$                    | 369      |
| 941:208b | $0, 0, 0, 0, 0, -e^{12}, e^{13}, e^{23} + e^{14}, e^{26} + e^{37}$                   | 369      |
| 941:209  | $0, 0, 0, 0, 0, e^{12}, e^{13}, e^{14} + e^{23}, e^{36} + e^{27}$                    | 369      |
| 941:210  | $0, 0, 0, 0, 0, e^{12}, e^{13}, e^{14}, e^{24} + e^{37} + e^{16}$                    | 369      |

Table 2 – Continued to next page

Table 2 – Continued from previous page

| Name     | $\mathfrak{g}$                                                              | UCS Dim. |
|----------|-----------------------------------------------------------------------------|----------|
| 941:211a | $0, 0, 0, 0, 0, e^{12}, e^{13}, e^{24}, e^{37} + e^{14} + e^{26}$           | 369      |
| 941:211b | $0, 0, 0, 0, 0, -e^{12}, e^{13}, e^{24}, e^{37} + e^{26} + e^{14}$          | 369      |
| 941:212  | $0, 0, 0, 0, 0, e^{12}, e^{13}, e^{24}, e^{27} + e^{36} + e^{14}$           | 369      |
| 941:213  | $0, 0, 0, 0, 0, e^{12}, e^{13}, e^{24}, e^{17} + e^{26} + e^{34}$           | 369      |
| 941:214  | $0, 0, 0, 0, 0, e^{12}, e^{13}, e^{14}, e^{17} + e^{26} + e^{45}$           | 269      |
| 941:215  | $0, 0, 0, 0, 0, e^{12}, e^{13}, e^{24}, e^{45} + e^{17} + e^{26}$           | 269      |
| 941:216a | $0, 0, 0, 0, 0, e^{12}, e^{13}, e^{14}, e^{26} + e^{37} + e^{45}$           | 269      |
| 941:216b | $0, 0, 0, 0, 0, -e^{12}, e^{13}, e^{14}, e^{37} + e^{45} + e^{26}$          | 269      |
| 941:217  | $0, 0, 0, 0, 0, e^{12}, e^{13}, e^{14}, e^{45} + e^{36} + e^{27}$           | 269      |
| 941:218  | $0, 0, 0, 0, 0, e^{12}, e^{13}, e^{24}, e^{16} + e^{37} + e^{45}$           | 269      |
| 941:219a | $0, 0, 0, 0, 0, e^{12}, e^{13}, e^{24}, e^{26} + e^{37} + e^{45}$           | 269      |
| 941:219b | $0, 0, 0, 0, 0, -e^{12}, e^{13}, e^{24}, e^{45} + e^{37} + e^{26}$          | 269      |
| 941:220  | $0, 0, 0, 0, 0, e^{12}, e^{13}, e^{24}, e^{45} + e^{36} + e^{27}$           | 269      |
| 941:221  | $0, 0, 0, 0, 0, e^{12}, e^{13}, e^{14} + e^{25}, e^{17} + e^{26}$           | 269      |
| 941:222  | $0, 0, 0, 0, 0, e^{12}, e^{13}, e^{25} + e^{14}, e^{37} + e^{16}$           | 269      |
| 941:223a | $0, 0, 0, 0, 0, e^{12}, e^{13}, e^{25} + e^{14}, e^{37} + e^{26}$           | 269      |
| 941:223b | $0, 0, 0, 0, 0, -e^{12}, e^{13}, e^{14} + e^{25}, e^{26} + e^{37}$          | 269      |
| 941:224  | $0, 0, 0, 0, 0, e^{12}, e^{13}, e^{25} + e^{14}, e^{27} + e^{36}$           | 269      |
| 941:225  | $0, 0, 0, 0, 0, e^{12}, e^{13}, e^{45} + e^{23}, e^{17} + e^{26}$           | 269      |
| 941:226  | $0, 0, 0, 0, 0, e^{12}, e^{13}, e^{35} + e^{24}, e^{17} + e^{26}$           | 269      |
| 941:227a | $0, 0, 0, 0, 0, e^{12}, e^{13}, e^{23} + e^{45}, e^{37} + e^{26}$           | 269      |
| 941:227b | $0, 0, 0, 0, 0, -e^{12}, e^{13}, e^{45} + e^{23}, e^{37} + e^{26}$          | 269      |
| 941:228a | $0, 0, 0, 0, 0, e^{12}, e^{13}, e^{24} + e^{35}, e^{37} + e^{26}$           | 269      |
| 941:228b | $0, 0, 0, 0, 0, -e^{12}, e^{13}, e^{35} + e^{24}, e^{26} + e^{37}$          | 269      |
| 941:229  | $0, 0, 0, 0, 0, e^{12}, e^{13}, e^{45} + e^{23}, e^{27} + e^{36}$           | 269      |
| 941:230  | $0, 0, 0, 0, 0, e^{12}, e^{13}, e^{24} + e^{35}, e^{27} + e^{36}$           | 269      |
| 941:231a | $0, 0, 0, 0, 0, e^{12}, e^{13}, e^{45}, e^{37} + e^{14} + e^{26}$           | 269      |
| 941:231b | $0, 0, 0, 0, 0, -e^{12}, e^{13}, e^{45}, e^{37} + e^{26} + e^{14}$          | 269      |
| 941:232  | $0, 0, 0, 0, 0, e^{12}, e^{13}, e^{45}, e^{37} + e^{16} + e^{24}$           | 269      |
| 941:233  | $0, 0, 0, 0, 0, e^{12}, e^{13}, e^{45}, e^{14} + e^{27} + e^{36}$           | 269      |
| 941:234a | $0, 0, 0, 0, 0, e^{12}, e^{13}, e^{23}, e^{14} + e^{37} + e^{26}$           | 369      |
| 941:234b | $0, 0, 0, 0, 0, -e^{12}, e^{13}, e^{23}, e^{14} + e^{26} + e^{37}$          | 369      |
| 941:235  | $0, 0, 0, 0, 0, e^{12}, e^{13}, e^{23}, e^{24} + e^{37} + e^{16}$           | 369      |
| 941:236  | $0, 0, 0, 0, 0, e^{12}, e^{13}, e^{23}, e^{36} + e^{14} + e^{27}$           | 369      |
| 941:237  | $0, 0, 0, 0, 0, e^{12}, e^{13}, e^{23}, e^{26} + e^{17} + e^{45}$           | 269      |
| 941:238a | $0, 0, 0, 0, 0, e^{12}, e^{13}, e^{23}, e^{26} + e^{37} + e^{45}$           | 269      |
| 941:238b | $0, 0, 0, 0, 0, -e^{12}, e^{13}, e^{23}, e^{26} + e^{37} + e^{45}$          | 269      |
| 941:239  | $0, 0, 0, 0, 0, e^{12}, e^{13}, e^{23}, e^{36} + e^{27} + e^{45}$           | 269      |
| 941:240a | $0, 0, 0, 0, 0, e^{12}, e^{13}, e^{14}, e^{15} + e^{26} + e^{37}$           | 269      |
| 941:240b | $0, 0, 0, 0, 0, -e^{12}, e^{13}, e^{14}, e^{37} + e^{15} + e^{26}$          | 269      |
| 941:241  | $0, 0, 0, 0, 0, e^{12}, e^{13}, e^{14}, e^{25} + e^{37} + e^{16}$           | 269      |
| 941:242  | $0, 0, 0, 0, 0, e^{12}, e^{13}, e^{14}, e^{27} + e^{36} + e^{15}$           | 269      |
| 941:243a | $0, 0, 0, 0, 0, e^{12}, e^{13}, e^{24}, e^{15} + e^{26} + e^{37}$           | 269      |
| 941:243b | $0, 0, 0, 0, 0, -e^{12}, e^{13}, e^{24}, e^{15} + e^{37} + e^{26}$          | 269      |
| 941:244  | $0, 0, 0, 0, 0, e^{12}, e^{13}, e^{24}, e^{37} + e^{25} + e^{16}$           | 269      |
| 941:245  | $0, 0, 0, 0, 0, e^{12}, e^{13}, e^{24}, e^{15} + e^{27} + e^{36}$           | 269      |
| 941:246  | $0, 0, 0, 0, 0, e^{12}, e^{13}, e^{24}, e^{26} + e^{35} + e^{17}$           | 269      |
| 941:247  | $0, 0, 0, 0, 0, e^{12}, e^{13}, e^{25} + e^{14}, e^{26} + e^{17} + e^{45}$  | 269      |
| 941:248  | $0, 0, 0, 0, 0, e^{12}, e^{13}, e^{25} + e^{14}, e^{16} + e^{37} + e^{45}$  | 269      |
| 941:249a | $0, 0, 0, 0, 0, e^{12}, e^{13}, e^{25} + e^{14}, e^{26} + e^{37} + e^{45}$  | 269      |
| 941:249b | $0, 0, 0, 0, 0, -e^{12}, e^{13}, e^{14} + e^{25}, e^{37} + e^{26} + e^{45}$ | 269      |
| 941:250  | $0, 0, 0, 0, 0, e^{12}, e^{13}, e^{25} + e^{14}, e^{27} + e^{45} + e^{36}$  | 269      |
| 941:251  | $0, 0, 0, 0, 0, e^{12}, e^{13}, e^{35} + e^{24}, e^{45} + e^{17} + e^{26}$  | 269      |
| 941:252a | $0, 0, 0, 0, 0, e^{12}, e^{13}, e^{24} + e^{35}, e^{37} + e^{26} + e^{45}$  | 269      |
| 941:252b | $0, 0, 0, 0, 0, -e^{12}, e^{13}, e^{35} + e^{24}, e^{37} + e^{45} + e^{26}$ | 269      |
| 941:253  | $0, 0, 0, 0, 0, e^{12}, e^{13}, e^{35} + e^{24}, e^{27} + e^{36} + e^{45}$  | 269      |
| 941:254  | $0, 0, 0, 0, 0, e^{12}, e^{13}, e^{14} + e^{23}, e^{16} + e^{24} + e^{37}$  | 369      |
| 941:255  | $0, 0, 0, 0, 0, e^{12}, e^{13}, e^{14} + e^{23}, e^{45} + e^{17} + e^{26}$  | 269      |

Table 2 – Continued to next page

Table 2 – Continued from previous page

| Name     | $\mathfrak{g}$                                                                          | UCS Dim. |
|----------|-----------------------------------------------------------------------------------------|----------|
| 941:256a | $0, 0, 0, 0, 0, e^{12}, e^{13}, e^{23} + e^{14}, e^{26} + e^{37} + e^{45}$              | 269      |
| 941:256b | $0, 0, 0, 0, 0, -e^{12}, e^{13}, e^{23} + e^{14}, e^{37} + e^{45} + e^{26}$             | 269      |
| 941:257  | $0, 0, 0, 0, 0, e^{12}, e^{13}, e^{14} + e^{23}, e^{45} + e^{36} + e^{27}$              | 269      |
| 941:258  | $0, 0, 0, 0, 0, e^{12}, e^{13}, e^{25} + e^{14}, e^{16} + e^{37} + e^{24}$              | 269      |
| 941:259  | $0, 0, 0, 0, 0, e^{12}, e^{13}, e^{25} + e^{14}, e^{17} + e^{26} + e^{34}$              | 269      |
| 941:260a | $0, 0, 0, 0, 0, e^{12}, e^{13}, e^{15} + e^{24}, e^{14} + e^{37} + e^{26}$              | 269      |
| 941:260b | $0, 0, 0, 0, 0, -e^{12}, e^{13}, e^{15} + e^{24}, e^{37} + e^{14} + e^{26}$             | 269      |
| 941:261  | $0, 0, 0, 0, 0, e^{12}, e^{13}, e^{24} + e^{15}, e^{27} + e^{36} + e^{14}$              | 269      |
| 941:262  | $0, 0, 0, 0, 0, e^{12}, e^{13}, e^{24} + e^{15}, e^{26} + e^{34} + e^{17}$              | 269      |
| 941:263a | $0, 0, 0, 0, 0, e^{12}, e^{13}, e^{45} + e^{23}, e^{37} + e^{14} + e^{26}$              | 269      |
| 941:263b | $0, 0, 0, 0, 0, -e^{12}, e^{13}, e^{45} + e^{23}, e^{14} + e^{26} + e^{37}$             | 269      |
| 941:264  | $0, 0, 0, 0, 0, e^{12}, e^{13}, e^{45} + e^{23}, e^{16} + e^{37} + e^{24}$              | 269      |
| 941:265  | $0, 0, 0, 0, 0, e^{12}, e^{13}, e^{45} + e^{23}, e^{14} + e^{36} + e^{27}$              | 269      |
| 941:266a | $0, 0, 0, 0, 0, e^{12}, e^{13}, e^{35} + e^{24}, e^{14} + e^{26} + e^{37}$              | 269      |
| 941:266b | $0, 0, 0, 0, 0, -e^{12}, e^{13}, e^{35} + e^{24}, e^{37} + e^{14} + e^{26}$             | 269      |
| 941:267  | $0, 0, 0, 0, 0, e^{12}, e^{13}, e^{24} + e^{35}, e^{36} + e^{27} + e^{14}$              | 269      |
| 941:268  | $0, 0, 0, 0, 0, e^{12}, e^{13}, e^{35} + e^{24}, e^{17} + e^{26} + e^{34}$              | 269      |
| 941:269a | $0, 0, 0, 0, 0, e^{12}, e^{13}, e^{23} + e^{14}, e^{15} + e^{26} + e^{37}$              | 269      |
| 941:269b | $0, 0, 0, 0, 0, -e^{12}, e^{13}, e^{14} + e^{23}, e^{15} + e^{37} + e^{26}$             | 269      |
| 941:270  | $0, 0, 0, 0, 0, e^{12}, e^{13}, e^{14} + e^{23}, e^{25} + e^{16} + e^{37}$              | 269      |
| 941:271  | $0, 0, 0, 0, 0, e^{12}, e^{13}, e^{14} + e^{23}, e^{15} + e^{27} + e^{36}$              | 269      |
| 941:272  | $0, 0, 0, 0, 0, e^{12}, e^{13}, e^{23}, e^{26} + e^{17} + e^{38}$                       | 369      |
| 941:273  | $0, 0, 0, 0, 0, e^{12}a_1, e^{13}(1 + a_1), e^{23}, e^{18} + e^{27} + e^{36}$           | 369      |
| 941:274  | $0, 0, 0, 0, 0, e^{12}, e^{13}, e^{23}, e^{17} + e^{26} + e^{45} + e^{38}$              | 169      |
| 941:275  | $0, 0, 0, 0, 0, e^{12}(-1 + a_2), a_2e^{13}, e^{23}, e^{36} + e^{18} + e^{27} + e^{45}$ | 169      |
| 941:276  | $0, 0, 0, 0, 0, e^{12}, e^{34}, e^{13}, e^{37} + e^{16}$                                | 359      |
| 941:277  | $0, 0, 0, 0, 0, e^{12}, e^{34}, e^{13}, e^{37} + e^{26}$                                | 359      |
| 941:278  | $0, 0, 0, 0, 0, e^{12}, e^{34}, e^{13}, e^{47} + e^{26}$                                | 359      |
| 941:279  | $0, 0, 0, 0, 0, e^{12}, e^{34}, e^{15}, e^{37} + e^{16}$                                | 259      |
| 941:280  | $0, 0, 0, 0, 0, e^{12}, e^{34}, e^{15}, e^{26} + e^{37}$                                | 259      |
| 941:281  | $0, 0, 0, 0, 0, e^{12}, e^{34}, e^{24} + e^{13}, e^{16} + e^{37}$                       | 359      |
| 941:282  | $0, 0, 0, 0, 0, e^{12}, e^{34}, e^{14} + e^{23}, e^{16} + e^{37}$                       | 359      |
| 941:283  | $0, 0, 0, 0, 0, e^{12}, e^{34}, e^{13} + e^{25}, e^{37} + e^{16}$                       | 259      |
| 941:284  | $0, 0, 0, 0, 0, e^{12}, e^{34}, e^{23} + e^{15}, e^{37} + e^{16}$                       | 259      |
| 941:285  | $0, 0, 0, 0, 0, e^{12}, e^{34}, e^{13} + e^{25}, e^{47} + e^{16}$                       | 259      |
| 941:286  | $0, 0, 0, 0, 0, e^{12}, e^{34}, e^{15} + e^{23}, e^{16} + e^{47}$                       | 259      |
| 941:287  | $0, 0, 0, 0, 0, e^{12}, e^{34}, e^{15}, e^{37} + e^{25} + e^{16}$                       | 259      |
| 941:288  | $0, 0, 0, 0, 0, e^{12}, e^{34}, e^{35}, e^{26} + e^{15} + e^{37}$                       | 259      |
| 941:289  | $0, 0, 0, 0, 0, e^{12}, e^{34}, e^{15}, e^{26} + e^{35} + e^{47}$                       | 259      |
| 941:290  | $0, 0, 0, 0, 0, -e^{12}, e^{14} + e^{23}, e^{13}, e^{17} + e^{36}$                      | 359      |
| 941:291  | $0, 0, 0, 0, 0, e^{12}, e^{14} + e^{23}, e^{13}, e^{46} + e^{27}$                       | 359      |
| 941:292  | $0, 0, 0, 0, 0, -e^{12}, e^{14} + e^{23}, e^{34}, e^{17} + e^{36}$                      | 359      |
| 941:293  | $0, 0, 0, 0, 0, -e^{12}, e^{23} + e^{14}, e^{15}, e^{17} + e^{36}$                      | 259      |
| 941:294  | $0, 0, 0, 0, 0, e^{12}, e^{24} + e^{13}, e^{15}, e^{36} + e^{27}$                       | 259      |
| 941:295  | $0, 0, 0, 0, 0, -e^{12}, e^{23} + e^{14}, e^{35}, e^{36} + e^{17}$                      | 259      |
| 941:296  | $0, 0, 0, 0, 0, -e^{12}, e^{13} + e^{24}, e^{35}, e^{17} + e^{46}$                      | 259      |
| 941:297  | $0, 0, 0, 0, 0, e^{12}, e^{34}, e^{13}, e^{47} + e^{23} + e^{16}$                       | 359      |
| 941:298  | $0, 0, 0, 0, 0, e^{12}, e^{34}, e^{13}, e^{16} + e^{37} + e^{24}$                       | 359      |
| 941:299  | $0, 0, 0, 0, 0, e^{12}, e^{34}, e^{13}, e^{15} + e^{37} + e^{26}$                       | 259      |
| 941:300  | $0, 0, 0, 0, 0, e^{12}, e^{34}, e^{13}, e^{37} + e^{25} + e^{16}$                       | 259      |
| 941:301  | $0, 0, 0, 0, 0, e^{12}, e^{34}, e^{13}, e^{47} + e^{26} + e^{15}$                       | 259      |
| 941:302  | $0, 0, 0, 0, 0, e^{12}, e^{34}, e^{13}, e^{47} + e^{16} + e^{25}$                       | 259      |
| 941:303  | $0, 0, 0, 0, 0, e^{12}, e^{34}, e^{15}, e^{47} + e^{13} + e^{26}$                       | 259      |
| 941:304  | $0, 0, 0, 0, 0, e^{12}, e^{34}, e^{15}, e^{23} + e^{47} + e^{16}$                       | 259      |
| 941:305  | $0, 0, 0, 0, 0, e^{12}, e^{34}, e^{25} + e^{13}, e^{26} + e^{37} + e^{15}$              | 259      |
| 941:306  | $0, 0, 0, 0, 0, e^{12}, e^{34}, e^{25} + e^{13}, e^{15} + e^{26} + e^{47}$              | 259      |
| 941:307  | $0, 0, 0, 0, 0, e^{12}, e^{34}, e^{25} + e^{13}, e^{47} + e^{16} + e^{35}$              | 259      |
| 941:308  | $0, 0, 0, 0, 0, e^{12}, e^{34}, e^{13} + e^{25}, e^{45} + e^{37} + e^{16}$              | 259      |

Table 2 – Continued to next page

Table 2 – Continued from previous page

| Name     | $\mathfrak{g}$                                                                        | UCS Dim. |
|----------|---------------------------------------------------------------------------------------|----------|
| 941:309  | $0, 0, 0, 0, 0, e^{12}, e^{34}, e^{15} + e^{23}, e^{16} + e^{35} + e^{47}$            | 259      |
| 941:310  | $0, 0, 0, 0, 0, e^{12}, e^{34}, e^{23} + e^{15}, e^{37} + e^{45} + e^{16}$            | 259      |
| 941:311a | $0, 0, 0, 0, 0, -e^{12}, e^{14} + e^{23}, e^{13} + e^{24}, e^{17} + e^{36}$           | 359      |
| 941:311b | $0, 0, 0, 0, 0, -e^{12}, e^{23} - e^{14}, e^{24} + e^{13}, e^{17} + e^{36}$           | 359      |
| 941:312  | $0, 0, 0, 0, 0, -e^{12}, e^{14} + e^{23}, e^{13} + e^{25}, e^{17} + e^{36}$           | 259      |
| 941:313  | $0, 0, 0, 0, 0, -e^{12}, e^{24} + e^{13}, e^{23} + e^{15}, e^{46} + e^{17}$           | 259      |
| 941:314  | $0, 0, 0, 0, 0, -e^{12}, e^{14} + e^{23}, e^{13} + e^{45}, e^{17} + e^{36}$           | 259      |
| 941:315  | $0, 0, 0, 0, 0, -e^{12}, e^{23} + e^{14}, e^{15} + e^{34}, e^{17} + e^{36}$           | 259      |
| 941:316  | $0, 0, 0, 0, 0, e^{12}, e^{24} + e^{13}, e^{14} + e^{35}, e^{36} + e^{27}$            | 259      |
| 941:317  | $0, 0, 0, 0, 0, e^{12}, e^{13} + e^{24}, e^{15} + e^{34}, e^{27} + e^{36}$            | 259      |
| 941:318  | $0, 0, 0, 0, 0, -e^{12}, e^{14} + e^{23}, e^{15}, e^{17} + e^{36} + e^{25}$           | 259      |
| 941:319  | $0, 0, 0, 0, 0, e^{12}, e^{13} + e^{24}, e^{35}, e^{15} + e^{27} + e^{36}$            | 259      |
| 941:320  | $0, 0, 0, 0, 0, -e^{12}, e^{13} + e^{24}, e^{15}, e^{17} + e^{46} + e^{35}$           | 259      |
| 941:321  | $0, 0, 0, 0, 0, e^{12}, e^{24} + e^{13}, e^{15}, e^{27} + e^{36} + e^{45}$            | 259      |
| 941:322  | $0, 0, 0, 0, 0, -e^{12}, e^{13} + e^{24}, e^{35}, e^{25} + e^{17} + e^{46}$           | 259      |
| 941:323  | $0, 0, 0, 0, 0, -e^{12}, e^{23} + e^{14}, e^{35}, e^{17} + e^{36} + e^{45}$           | 259      |
| 941:324a | $0, 0, 0, 0, 0, e^{14} + e^{23}, e^{24} + e^{13}, e^{12}, e^{16} + e^{27}$            | 359      |
| 941:324b | $0, 0, 0, 0, 0, -e^{14} + e^{23}, e^{13} + e^{24}, e^{12}, e^{16} + e^{27}$           | 359      |
| 941:325a | $0, 0, 0, 0, 0, e^{14} + e^{23}, e^{24} + e^{13}, e^{12}, e^{36} + e^{47}$            | 359      |
| 941:325b | $0, 0, 0, 0, 0, e^{14} - e^{23}, e^{13} + e^{24}, e^{12}, e^{36} + e^{47}$            | 359      |
| 941:326a | $0, 0, 0, 0, 0, e^{14} + e^{23}, e^{24} + e^{13}, e^{15}, e^{16} + e^{27}$            | 259      |
| 941:326b | $0, 0, 0, 0, 0, -e^{14} + e^{23}, e^{13} + e^{24}, e^{15}, e^{16} + e^{27}$           | 259      |
| 941:327a | $0, 0, 0, 0, 0, e^{24} + e^{13}, e^{12} + e^{34}, e^{15}, e^{37} + e^{26}$            | 259      |
| 941:327b | $0, 0, 0, 0, 0, -e^{24} + e^{13}, e^{34} + e^{12}, e^{15}, e^{26} + e^{37}$           | 259      |
| 941:328a | $0, 0, 0, 0, 0, e^{34} + e^{12}, e^{24} + e^{13}, e^{15}, e^{37} + e^{26}$            | 259      |
| 941:328b | $0, 0, 0, 0, 0, e^{34} - e^{12}, e^{24} + e^{13}, e^{15}, e^{26} + e^{37}$            | 259      |
| 941:329  | $0, 0, 0, 0, 0, e^{12}, e^{34}, e^{24} + e^{13}, e^{16} + e^{23} + e^{47}$            | 359      |
| 941:330  | $0, 0, 0, 0, 0, e^{12}, e^{34}, e^{13} + e^{24}, e^{37} + e^{26} + e^{15}$            | 259      |
| 941:331  | $0, 0, 0, 0, 0, e^{12}, e^{34}, e^{13} + e^{24}, e^{37} + e^{16} + e^{25}$            | 259      |
| 941:332  | $0, 0, 0, 0, 0, e^{12}, e^{34}, e^{25} + e^{13}, e^{16} + e^{47} + e^{23}$            | 259      |
| 941:333  | $0, 0, 0, 0, 0, e^{12}, e^{34}, e^{25} + e^{13}, e^{14} + e^{37} + e^{26}$            | 259      |
| 941:334  | $0, 0, 0, 0, 0, e^{12}, e^{34}, e^{13} + e^{25}, e^{37} + e^{16} + e^{24}$            | 259      |
| 941:335  | $0, 0, 0, 0, 0, -e^{12}, e^{23} + e^{14}, e^{13}, e^{24} + e^{36} + e^{17}$           | 359      |
| 941:336  | $0, 0, 0, 0, 0, e^{12}, e^{24} + e^{13}, e^{34}, e^{36} + e^{27} + e^{14}$            | 359      |
| 941:337  | $0, 0, 0, 0, 0, -e^{12}, e^{23} + e^{14}, e^{13}, e^{17} + e^{25} + e^{36}$           | 259      |
| 941:338  | $0, 0, 0, 0, 0, e^{12}, e^{14} + e^{23}, e^{13}, e^{46} + e^{15} + e^{27}$            | 259      |
| 941:339  | $0, 0, 0, 0, 0, -e^{12}, e^{23} + e^{14}, e^{13}, e^{36} + e^{45} + e^{17}$           | 259      |
| 941:340  | $0, 0, 0, 0, 0, e^{12}, e^{14} + e^{23}, e^{13}, e^{27} + e^{35} + e^{46}$            | 259      |
| 941:341  | $0, 0, 0, 0, 0, e^{12}, e^{13} + e^{24}, e^{34}, e^{15} + e^{27} + e^{36}$            | 259      |
| 941:342  | $0, 0, 0, 0, 0, -e^{12}, e^{13} + e^{24}, e^{34}, e^{17} + e^{46} + e^{35}$           | 259      |
| 941:343  | $0, 0, 0, 0, 0, e^{12}, e^{13} + e^{24}, e^{15}, e^{14} + e^{27} + e^{36}$            | 259      |
| 941:344  | $0, 0, 0, 0, 0, -e^{12}, e^{13} + e^{24}, e^{15}, e^{23} + e^{17} + e^{46}$           | 259      |
| 941:345  | $0, 0, 0, 0, 0, e^{12}, e^{24} + e^{13}, e^{35}, e^{27} + e^{36} + e^{14}$            | 259      |
| 941:346  | $0, 0, 0, 0, 0, -e^{12}, e^{13} + e^{24}, e^{35}, e^{17} + e^{23} + e^{46}$           | 259      |
| 941:347  | $0, 0, 0, 0, 0, e^{12}, e^{14} + e^{23}, e^{13} + e^{25}, e^{15} + e^{46} + e^{27}$   | 259      |
| 941:348  | $0, 0, 0, 0, 0, -e^{12}, e^{14} + e^{23}, e^{13} + e^{25}, e^{17} + e^{45} + e^{36}$  | 259      |
| 941:349  | $0, 0, 0, 0, 0, -e^{12}, e^{24} + e^{13}, e^{15} + e^{23}, e^{17} + e^{35} + e^{46}$  | 259      |
| 941:350  | $0, 0, 0, 0, 0, -e^{12}, e^{14} + e^{23}, e^{13} + e^{45}, e^{17} + e^{25} + e^{36}$  | 259      |
| 941:351  | $0, 0, 0, 0, 0, e^{12}, e^{24} + e^{13}, e^{35} + e^{14}, e^{27} + e^{36} + e^{15}$   | 259      |
| 941:352  | $0, 0, 0, 0, 0, -e^{12}, e^{14} + e^{23}, e^{15} + e^{34}, e^{25} + e^{17} + e^{36}$  | 259      |
| 941:353  | $0, 0, 0, 0, 0, -e^{12}, e^{24} + e^{13}, e^{15} + e^{34}, e^{17} + e^{35} + e^{46}$  | 259      |
| 941:354  | $0, 0, 0, 0, 0, e^{12}, e^{14} + e^{23}, e^{13} + e^{45}, e^{27} + e^{35} + e^{46}$   | 259      |
| 941:355  | $0, 0, 0, 0, 0, e^{12}, e^{24} + e^{13}, e^{34}, e^{27} + e^{36} + e^{45}$            | 259      |
| 941:356a | $0, 0, 0, 0, 0, e^{14} + e^{23}, e^{24} + e^{13}, e^{12} + e^{34}, e^{27} + e^{16}$   | 359      |
| 941:356b | $0, 0, 0, 0, 0, e^{23} - e^{14}, e^{24} + e^{13}, e^{34} + e^{12}, e^{27} + e^{16}$   | 359      |
| 941:356c | $0, 0, 0, 0, 0, -e^{14} + e^{23}, e^{13} + e^{24}, -e^{12} + e^{34}, e^{27} + e^{16}$ | 359      |
| 941:357a | $0, 0, 0, 0, 0, e^{14} + e^{23}, e^{13} + e^{24}, e^{12} + e^{35}, e^{16} + e^{27}$   | 259      |
| 941:357b | $0, 0, 0, 0, 0, -e^{14} + e^{23}, e^{24} + e^{13}, e^{12} + e^{35}, e^{27} + e^{16}$  | 259      |

Table 2 – Continued to next page

Table 2 – Continued from previous page

| Name     | $\mathfrak{g}$                                                                                 | UCS Dim. |
|----------|------------------------------------------------------------------------------------------------|----------|
| 941:358a | $0, 0, 0, 0, 0, e^{24} + e^{13}, e^{23} + e^{14}, e^{35} + e^{12}, e^{16} + e^{27}$            | 259      |
| 941:358b | $0, 0, 0, 0, 0, e^{24} - e^{13}, e^{14} + e^{23}, e^{35} + e^{12}, e^{16} + e^{27}$            | 259      |
| 941:359a | $0, 0, 0, 0, 0, e^{24} + e^{13}, -e^{12} + e^{34}, e^{23} + e^{15}, e^{47} + e^{16}$           | 259      |
| 941:359b | $0, 0, 0, 0, 0, -e^{13} + e^{24}, e^{34} - e^{12}, e^{15} + e^{23}, e^{47} + e^{16}$           | 259      |
| 941:360a | $0, 0, 0, 0, 0, e^{23} + e^{14}, e^{34} - e^{12}, e^{15}, e^{16} + e^{25} + e^{37}$            | 259      |
| 941:360b | $0, 0, 0, 0, 0, -e^{14} + e^{23}, e^{34} - e^{12}, e^{15}, e^{37} + e^{25} + e^{16}$           | 259      |
| 941:361a | $0, 0, 0, 0, 0, e^{23} + e^{14}, e^{34} + e^{12}, e^{15}, e^{25} + e^{36} + e^{17}$            | 259      |
| 941:361b | $0, 0, 0, 0, 0, e^{14} + e^{23}, -e^{12} + e^{34}, e^{15}, e^{36} + e^{25} + e^{17}$           | 259      |
| 941:362a | $0, 0, 0, 0, 0, e^{24} + e^{13}, e^{34} + e^{12}, e^{15}, e^{26} + e^{37} + e^{45}$            | 259      |
| 941:362b | $0, 0, 0, 0, 0, -e^{24} + e^{13}, e^{34} + e^{12}, e^{15}, e^{45} + e^{37} + e^{26}$           | 259      |
| 941:363a | $0, 0, 0, 0, 0, e^{13} + e^{24}, e^{12} + e^{34}, e^{15}, e^{27} + e^{36} + e^{45}$            | 259      |
| 941:363b | $0, 0, 0, 0, 0, e^{24} - e^{13}, e^{12} + e^{34}, e^{15}, e^{36} + e^{27} + e^{45}$            | 259      |
| 941:364a | $0, 0, 0, 0, 0, -e^{12}, e^{23} + e^{14}, e^{24} + e^{13}, e^{17} + e^{25} + e^{36}$           | 259      |
| 941:364b | $0, 0, 0, 0, 0, -e^{12}, -e^{14} + e^{23}, e^{13} + e^{24}, e^{36} + e^{17} + e^{25}$          | 259      |
| 941:365a | $0, 0, 0, 0, 0, -e^{12}, e^{23} + e^{14}, e^{24} + e^{13}, e^{36} + e^{45} + e^{17}$           | 259      |
| 941:365b | $0, 0, 0, 0, 0, -e^{12}, -e^{14} + e^{23}, e^{13} + e^{24}, e^{17} + e^{45} + e^{36}$          | 259      |
| 941:366  | $0, 0, 0, 0, 0, -e^{12}, e^{23} + e^{14}, e^{25} + e^{13}, e^{17} + e^{36} + e^{24}$           | 259      |
| 941:367  | $0, 0, 0, 0, 0, -e^{12}, e^{14} + e^{23}, e^{13} + e^{45}, e^{17} + e^{24} + e^{36}$           | 259      |
| 941:368  | $0, 0, 0, 0, 0, e^{12}, e^{13} + e^{24}, e^{15} + e^{34}, e^{14} + e^{27} + e^{36}$            | 259      |
| 941:369  | $0, 0, 0, 0, 0, -e^{12}, e^{13} + e^{24}, e^{34} + e^{15}, e^{17} + e^{46} + e^{23}$           | 259      |
| 941:370a | $0, 0, 0, 0, 0, e^{14} + e^{23}, e^{13} + e^{24}, e^{12}, e^{27} + e^{34} + e^{16}$            | 359      |
| 941:370b | $0, 0, 0, 0, 0, -e^{14} + e^{23}, e^{24} + e^{13}, e^{12}, e^{16} + e^{34} + e^{27}$           | 359      |
| 941:371a | $0, 0, 0, 0, 0, e^{23} + e^{14}, e^{24} + e^{13}, e^{12}, e^{35} + e^{27} + e^{16}$            | 259      |
| 941:371b | $0, 0, 0, 0, 0, -e^{14} + e^{23}, e^{24} + e^{13}, e^{12}, e^{27} + e^{35} + e^{16}$           | 259      |
| 941:372a | $0, 0, 0, 0, 0, e^{23} + e^{14}, e^{24} + e^{13}, e^{12}, e^{17} + e^{26} + e^{35}$            | 259      |
| 941:372b | $0, 0, 0, 0, 0, e^{14} + e^{23}, e^{24} - e^{13}, e^{12}, e^{17} + e^{26} + e^{35}$            | 259      |
| 941:373a | $0, 0, 0, 0, 0, e^{14} + e^{23}, e^{13} + e^{24}, e^{12}, e^{15} + e^{47} + e^{36}$            | 259      |
| 941:373b | $0, 0, 0, 0, 0, e^{14} - e^{23}, e^{24} + e^{13}, e^{12}, e^{36} + e^{15} + e^{47}$            | 259      |
| 941:374a | $0, 0, 0, 0, 0, e^{14} + e^{23}, e^{13} + e^{24}, e^{12}, e^{15} + e^{37} + e^{46}$            | 259      |
| 941:374b | $0, 0, 0, 0, 0, -e^{14} + e^{23}, e^{24} + e^{13}, e^{12}, e^{46} + e^{15} + e^{37}$           | 259      |
| 941:375a | $0, 0, 0, 0, 0, e^{24} + e^{13}, -e^{12} + e^{34}, e^{15}, e^{23} + e^{47} + e^{16}$           | 259      |
| 941:375b | $0, 0, 0, 0, 0, -e^{13} + e^{24}, -e^{12} + e^{34}, e^{15}, e^{23} + e^{47} + e^{16}$          | 259      |
| 941:376a | $0, 0, 0, 0, 0, e^{24} + e^{13}, e^{34} + e^{12}, e^{15}, e^{26} + e^{37} + e^{14}$            | 259      |
| 941:376b | $0, 0, 0, 0, 0, -e^{24} + e^{13}, e^{34} + e^{12}, e^{15}, e^{14} + e^{37} + e^{26}$           | 259      |
| 941:377a | $0, 0, 0, 0, 0, e^{24} + e^{13}, e^{34} + e^{12}, e^{15}, e^{27} + e^{36} + e^{14}$            | 259      |
| 941:377b | $0, 0, 0, 0, 0, e^{24} - e^{13}, e^{12} + e^{34}, e^{15}, e^{36} + e^{27} + e^{14}$            | 259      |
| 941:378a | $0, 0, 0, 0, 0, e^{14} + e^{23}, e^{13} + e^{24}, e^{12} + e^{35}, e^{27} + e^{45} + e^{16}$   | 259      |
| 941:378b | $0, 0, 0, 0, 0, -e^{14} + e^{23}, e^{24} + e^{13}, e^{35} + e^{12}, e^{16} + e^{27} + e^{45}$  | 259      |
| 941:379a | $0, 0, 0, 0, 0, e^{23} + e^{14}, e^{24} + e^{13}, e^{35} + e^{12}, e^{26} + e^{45} + e^{17}$   | 259      |
| 941:379b | $0, 0, 0, 0, 0, e^{14} + e^{23}, e^{24} - e^{13}, e^{12} + e^{35}, e^{45} + e^{26} + e^{17}$   | 259      |
| 941:380a | $0, 0, 0, 0, 0, e^{23} + e^{14}, e^{34} + e^{12}, e^{25} + e^{13}, e^{26} + e^{47} + e^{15}$   | 259      |
| 941:380b | $0, 0, 0, 0, 0, e^{14} - e^{23}, e^{34} + e^{12}, e^{25} + e^{13}, e^{47} + e^{15} + e^{26}$   | 259      |
| 941:381a | $0, 0, 0, 0, 0, -e^{23} + e^{14}, e^{12} + e^{34}, e^{13} + e^{25}, e^{46} + e^{15} + e^{27}$  | 259      |
| 941:381b | $0, 0, 0, 0, 0, -e^{14} - e^{23}, e^{34} + e^{12}, e^{13} + e^{25}, e^{27} + e^{46} + e^{15}$  | 259      |
| 941:382a | $0, 0, 0, 0, 0, e^{14} + e^{23}, e^{13} + e^{24}, e^{12} + e^{34}, e^{27} + e^{35} + e^{16}$   | 259      |
| 941:382b | $0, 0, 0, 0, 0, -e^{14} + e^{23}, e^{13} + e^{24}, e^{34} + e^{12}, e^{35} + e^{27} + e^{16}$  | 259      |
| 941:382c | $0, 0, 0, 0, 0, e^{23} - e^{14}, e^{24} + e^{13}, -e^{12} + e^{34}, e^{35} + e^{27} + e^{16}$  | 259      |
| 941:383a | $0, 0, 0, 0, 0, e^{14} + e^{23}, e^{24} + e^{13}, e^{12} + e^{34}, e^{26} + e^{35} + e^{17}$   | 259      |
| 941:383b | $0, 0, 0, 0, 0, e^{23} + e^{14}, e^{24} - e^{13}, e^{34} + e^{12}, e^{17} + e^{26} + e^{35}$   | 259      |
| 941:383c | $0, 0, 0, 0, 0, e^{14} + e^{23}, -e^{13} + e^{24}, -e^{12} + e^{34}, e^{17} + e^{26} + e^{35}$ | 259      |
| 941:384a | $0, 0, 0, 0, 0, e^{14} + e^{23}, e^{13} + e^{24}, e^{12} + e^{35}, e^{16} + e^{34} + e^{27}$   | 259      |
| 941:384b | $0, 0, 0, 0, 0, -e^{14} + e^{23}, e^{24} + e^{13}, e^{12} + e^{35}, e^{34} + e^{27} + e^{16}$  | 259      |
| 941:385a | $0, 0, 0, 0, 0, e^{14} + e^{23}, e^{13} + e^{24}, e^{12} + e^{35}, e^{26} + e^{34} + e^{17}$   | 259      |
| 941:385b | $0, 0, 0, 0, 0, e^{14} + e^{23}, e^{24} - e^{13}, e^{35} + e^{12}, e^{17} + e^{26} + e^{34}$   | 259      |
| 941:386a | $0, 0, 0, 0, 0, e^{12}, e^{13}, e^{14}, e^{26} + e^{37} + e^{18}$                              | 259      |
| 941:386b | $0, 0, 0, 0, 0, -e^{12}, e^{13}, e^{14}, e^{37} + e^{18} + e^{26}$                             | 259      |
| 941:387  | $0, 0, 0, 0, 0, e^{12}, e^{13}, e^{14}, e^{18} + e^{36} + e^{27}$                              | 259      |
| 941:388  | $0, 0, 0, 0, 0, e^{12}, e^{13}, e^{24}, e^{16} + e^{28} + e^{37}$                              | 259      |

Table 2 – Continued to next page



Table 2 – Continued from previous page

| Name     | $\mathfrak{g}$                                                                                                    | UCS Dim. |
|----------|-------------------------------------------------------------------------------------------------------------------|----------|
| 941:389a | $0, 0, 0, 0, 0, e^{12}, e^{13}, e^{14}, e^{26} + e^{48} + e^{37}$                                                 | 259      |
| 941:389b | $0, 0, 0, 0, 0, e^{12}, -e^{13}, e^{14}, e^{37} + e^{26} + e^{48}$                                                | 259      |
| 941:390  | $0, 0, 0, 0, 0, e^{12}, e^{13}, e^{14}, e^{36} + e^{48} + e^{27}$                                                 | 259      |
| 941:391a | $0, 0, 0, 0, 0, e^{12}, e^{13}, e^{24}, e^{48} + e^{37} + e^{16}$                                                 | 259      |
| 941:391b | $0, 0, 0, 0, 0, -e^{12}, e^{13}, e^{24}, e^{48} + e^{37} + e^{16}$                                                | 259      |
| 941:392  | $0, 0, 0, 0, 0, -e^{12}, e^{13}, e^{24}, e^{37} + e^{46} + e^{18}$                                                | 259      |
| 941:393  | $0, 0, 0, 0, 0, e^{12}a_1, e^{13}(1 + a_1), e^{23} + e^{14}, e^{27} + e^{18} + e^{36}$                            | 259      |
| 941:394a | $0, 0, 0, 0, 0, e^{12}, e^{13}, e^{14} + e^{23}, e^{17} + e^{46} + e^{28}$                                        | 259      |
| 941:394b | $0, 0, 0, 0, 0, e^{12}, -e^{13}, e^{14} + e^{23}, e^{28} + e^{46} + e^{17}$                                       | 259      |
| 941:395  | $0, 0, 0, 0, 0, e^{12}, e^{13}, e^{23} + e^{14}, e^{26} + e^{38} + e^{47}$                                        | 259      |
| 941:396  | $0, 0, 0, 0, 0, e^{12}, e^{34}, e^{24} + e^{13}, e^{16} + e^{38} + e^{27}$                                        | 259      |
| 941:397a | $0, 0, 0, 0, 0, e^{12}, e^{13}, e^{14}, e^{48} + e^{26} + e^{37} + e^{15}$                                        | 159      |
| 941:397b | $0, 0, 0, 0, 0, e^{12}, -e^{13}, e^{14}, e^{48} + e^{37} + e^{15} + e^{26}$                                       | 159      |
| 941:398a | $0, 0, 0, 0, 0, e^{12}, e^{13}, e^{14}, e^{48} + e^{25} + e^{37} + e^{16}$                                        | 159      |
| 941:398b | $0, 0, 0, 0, 0, e^{12}, -e^{13}, e^{14}, e^{37} + e^{48} + e^{25} + e^{16}$                                       | 159      |
| 941:399  | $0, 0, 0, 0, 0, e^{12}, e^{13}, e^{14}, e^{15} + e^{27} + e^{36} + e^{48}$                                        | 159      |
| 941:400  | $0, 0, 0, 0, 0, e^{12}, e^{13}, e^{14}, e^{16} + e^{38} + e^{25} + e^{47}$                                        | 159      |
| 941:401a | $0, 0, 0, 0, 0, e^{12}, e^{13}, e^{24}, e^{48} + e^{26} + e^{37} + e^{15}$                                        | 159      |
| 941:401b | $0, 0, 0, 0, 0, -e^{12}, e^{13}, e^{24}, e^{48} + e^{37} + e^{15} + e^{26}$                                       | 159      |
| 941:402  | $0, 0, 0, 0, 0, e^{12}, e^{13}, e^{24}, e^{48} + e^{36} + e^{27} + e^{15}$                                        | 159      |
| 941:403  | $0, 0, 0, 0, 0, e^{12}, e^{13}, e^{24}, e^{17} + e^{26} + e^{48} + e^{35}$                                        | 159      |
| 941:404a | $0, 0, 0, 0, 0, e^{12}(-1 + a_2), e^{23} + e^{14}, a_2e^{13} + e^{24}, e^{28} + e^{17} + e^{36}$                  | 259      |
| 941:404b | $0, 0, 0, 0, 0, e^{12}(-1 + a_2), -e^{14} + e^{23}, a_2e^{13} + e^{24}, e^{17} + e^{28} + e^{36}$                 | 259      |
| 941:405a | $0, 0, 0, 0, 0, e^{12}, e^{14} + e^{23}, e^{13} + e^{24}, e^{37} + e^{48} + e^{16}$                               | 259      |
| 941:405b | $0, 0, 0, 0, 0, e^{12}, -e^{23} + e^{14}, e^{24} + e^{13}, e^{16} + e^{48} + e^{37}$                              | 259      |
| 941:405c | $0, 0, 0, 0, 0, -e^{12}, e^{14} + e^{23}, e^{13} + e^{24}, e^{16} + e^{37} + e^{48}$                              | 259      |
| 941:406a | $0, 0, 0, 0, 0, e^{12}, e^{23} + e^{14}, e^{24} + e^{13}, e^{47} + e^{38} + e^{16}$                               | 259      |
| 941:406b | $0, 0, 0, 0, 0, e^{12}, -e^{14} + e^{23}, e^{13} + e^{24}, e^{38} + e^{47} + e^{16}$                              | 259      |
| 941:407  | $0, 0, 0, 0, 0, e^{12}, e^{13}, e^{23} + e^{14}, e^{15} + e^{26} + e^{47} + e^{38}$                               | 159      |
| 941:408a | $0, 0, 0, 0, 0, e^{12}, e^{13}, e^{14} + e^{23}, e^{25} + e^{16} + e^{38} + e^{47}$                               | 159      |
| 941:408b | $0, 0, 0, 0, 0, -e^{12}, e^{13}, e^{23} + e^{14}, e^{47} + e^{38} + e^{16} + e^{25}$                              | 159      |
| 941:409  | $0, 0, 0, 0, 0, (-1 + a_2)e^{12}, a_2e^{13}, e^{14} + e^{23}, e^{18} + e^{27} + e^{45} + e^{36}$                  | 159      |
| 941:410  | $0, 0, 0, 0, 0, e^{12}, e^{34}, -e^{13} + e^{24}, e^{17} + e^{26} + e^{35} + e^{48}$                              | 159      |
| 941:411a | $0, 0, 0, 0, 0, e^{23} + e^{14}, e^{24} + e^{13}(1 + a_2), e^{34} + e^{12}a_2, e^{38} + e^{27} + e^{16}$          | 259      |
| 941:411b | $0, 0, 0, 0, 0, e^{14} + e^{23}, -e^{24} + e^{13}(1 + a_2), e^{34} + e^{12}a_2, e^{38} + e^{27} + e^{16}$         | 259      |
| 941:412a | $0, 0, 0, 0, 0, e^{12}, e^{23} + e^{14}, e^{24} + e^{13}, e^{15} + e^{26} + e^{48} + e^{37}$                      | 159      |
| 941:412b | $0, 0, 0, 0, 0, e^{12}, e^{14} - e^{23}, e^{13} + e^{24}, e^{37} + e^{48} + e^{26} + e^{15}$                      | 159      |
| 941:413a | $0, 0, 0, 0, 0, e^{12}, e^{23} + e^{14}, e^{24} + e^{13}, e^{48} + e^{37} + e^{16} + e^{25}$                      | 159      |
| 941:413b | $0, 0, 0, 0, 0, e^{12}, e^{14} - e^{23}, e^{13} + e^{24}, e^{37} + e^{48} + e^{25} + e^{16}$                      | 159      |
| 941:413c | $0, 0, 0, 0, 0, -e^{12}, e^{23} + e^{14}, e^{24} + e^{13}, e^{16} + e^{25} + e^{48} + e^{37}$                     | 159      |
| 941:414a | $0, 0, 0, 0, 0, (-1 + a_2)e^{12}, e^{14} + e^{23}, e^{13}a_2 + e^{24}, e^{45} + e^{36} + e^{17} + e^{28}$         | 159      |
| 941:414b | $0, 0, 0, 0, 0, (-1 + a_2)e^{12}, -e^{14} + e^{23}, e^{13}a_2 + e^{24}, e^{28} + e^{45} + e^{36} + e^{17}$        | 159      |
| 941:415a | $0, 0, 0, 0, 0, (1 + a_2)e^{14} + e^{23}, e^{24} + e^{13}, e^{34} + e^{12}a_2, e^{17} + e^{26} + e^{35} + e^{48}$ | 159      |
| 941:415b | $0, 0, 0, 0, 0, (1 + a_2)e^{14} - e^{23}, e^{24} - e^{13}, e^{34} + e^{12}a_2, e^{35} + e^{48} + e^{26} + e^{17}$ | 159      |
| 941:416  | $0, 0, 0, 0, 0, e^{14} + e^{23}, e^{13} + e^{25}, e^{12}, e^{27} + e^{16}$                                        | 249      |
| 941:417  | $0, 0, 0, 0, 0, e^{13} + e^{24}, e^{15} + e^{23}, e^{14}, e^{26} + e^{17}$                                        | 249      |
| 941:418  | $0, 0, 0, 0, 0, e^{24} + e^{13}, e^{35} + e^{12}, e^{14}, e^{37} + e^{26}$                                        | 249      |
| 941:419  | $0, 0, 0, 0, 0, e^{23} + e^{14}, e^{25} + e^{13}, e^{45}, e^{27} + e^{16}$                                        | 249      |
| 941:420a | $0, 0, 0, 0, 0, e^{14} + e^{23}, e^{13} + e^{25}, e^{12} + e^{34}, e^{27} + e^{16}$                               | 249      |
| 941:420b | $0, 0, 0, 0, 0, e^{23} - e^{14}, e^{25} + e^{13}, e^{34} + e^{12}, e^{16} + e^{27}$                               | 249      |
| 941:421  | $0, 0, 0, 0, 0, e^{14} + e^{23}, e^{25} + e^{13}, e^{45} + e^{12}, e^{16} + e^{27}$                               | 249      |
| 941:422  | $0, 0, 0, 0, 0, e^{14} + e^{23}, e^{13} + e^{25}, e^{15} + e^{24}, e^{16} + e^{27}$                               | 249      |
| 941:423  | $0, 0, 0, 0, 0, e^{14} + e^{23}, e^{35} - e^{12}, e^{15} + e^{24}, e^{37} + e^{16}$                               | 249      |
| 941:424  | $0, 0, 0, 0, 0, e^{14} + e^{23}, e^{13} + e^{25}, e^{12}, e^{27} + e^{34} + e^{16}$                               | 249      |
| 941:425  | $0, 0, 0, 0, 0, e^{34} - e^{12}, e^{15} + e^{23}, e^{14}, e^{36} + e^{17} + e^{24}$                               | 249      |
| 941:426  | $0, 0, 0, 0, 0, e^{14} + e^{23}, e^{13} + e^{25}, e^{12}, e^{16} + e^{27} + e^{45}$                               | 249      |
| 941:427  | $0, 0, 0, 0, 0, e^{24} + e^{13}, e^{12} + e^{35}, e^{14}, e^{37} + e^{26} + e^{15}$                               | 249      |
| 941:428  | $0, 0, 0, 0, 0, e^{34} - e^{12}, e^{15} + e^{23}, e^{14}, e^{17} + e^{25} + e^{36}$                               | 249      |

Table 2 – Continued to next page

Table 2 – Continued from previous page

| Name     | $\mathfrak{g}$                                                                                            | UCS Dim. |
|----------|-----------------------------------------------------------------------------------------------------------|----------|
| 941:429  | $0, 0, 0, 0, 0, e^{24} + e^{13}, e^{15} + e^{23}, e^{14}, e^{45} + e^{17} + e^{26}$                       | 249      |
| 941:430  | $0, 0, 0, 0, 0, e^{13} + e^{24}, e^{12} + e^{35}, e^{14}, e^{26} + e^{37} + e^{45}$                       | 249      |
| 941:431  | $0, 0, 0, 0, 0, e^{24} + e^{13}, e^{12} + e^{35}, e^{45}, e^{37} + e^{26} + e^{14}$                       | 249      |
| 941:432a | $0, 0, 0, 0, 0, e^{14} + e^{23}, e^{13} + e^{25}, e^{12} + e^{34}, e^{27} + e^{35} + e^{16}$              | 249      |
| 941:432b | $0, 0, 0, 0, 0, -e^{14} + e^{23}, e^{25} + e^{13}, e^{34} + e^{12}, e^{16} + e^{27} + e^{35}$             | 249      |
| 941:433a | $0, 0, 0, 0, 0, e^{23} + e^{14}, e^{25} + e^{13}, e^{34} + e^{12}, e^{27} + e^{45} + e^{16}$              | 249      |
| 941:433b | $0, 0, 0, 0, 0, -e^{14} + e^{23}, e^{13} + e^{25}, e^{12} + e^{34}, e^{45} + e^{27} + e^{16}$             | 249      |
| 941:434  | $0, 0, 0, 0, 0, e^{23} + e^{14}, e^{25} + e^{13}, e^{45} + e^{12}, e^{16} + e^{27} + e^{34}$              | 249      |
| 941:435  | $0, 0, 0, 0, 0, e^{34} - e^{12}, e^{15} + e^{23}, e^{25} + e^{14}, e^{36} + e^{17} + e^{24}$              | 249      |
| 941:436  | $0, 0, 0, 0, 0, e^{24} + e^{13}, e^{23} + e^{15}, e^{25} + e^{14}, e^{34} + e^{26} + e^{17}$              | 249      |
| 941:437  | $0, 0, 0, 0, 0, e^{24} + e^{13}, e^{15} + e^{23}, e^{25} + e^{14}, e^{26} + e^{17} + e^{45}$              | 249      |
| 941:438  | $0, 0, 0, 0, 0, e^{34} - e^{12}, e^{15} + e^{23}, e^{25} + e^{14}, e^{17} + e^{36} + e^{45}$              | 249      |
| 941:439  | $0, 0, 0, 0, 0, e^{12}, e^{13}, e^{45}, e^{48} + e^{17} + e^{26}$                                         | 149      |
| 941:440a | $0, 0, 0, 0, 0, e^{12}, e^{13}, e^{45}, e^{26} + e^{37} + e^{48}$                                         | 149      |
| 941:440b | $0, 0, 0, 0, 0, -e^{12}, e^{13}, e^{45}, e^{48} + e^{26} + e^{37}$                                        | 149      |
| 941:441  | $0, 0, 0, 0, 0, e^{12}, e^{13}, e^{45}, e^{36} + e^{48} + e^{27}$                                         | 149      |
| 941:442  | $0, 0, 0, 0, 0, e^{12}, e^{13}, e^{25} + e^{14}, e^{17} + e^{46} + e^{28}$                                | 149      |
| 941:443  | $0, 0, 0, 0, 0, -e^{12}, e^{13}, e^{15} + e^{24}, e^{46} + e^{37} + e^{18}$                               | 149      |
| 941:444  | $0, 0, 0, 0, 0, e^{12}, e^{13}, e^{25} + e^{14}, e^{28} + e^{46} + e^{37}$                                | 149      |
| 941:445  | $0, 0, 0, 0, 0, -e^{12}, e^{34}, e^{15} + e^{23}, e^{36} + e^{18} + e^{47}$                               | 149      |
| 941:446  | $0, 0, 0, 0, 0, -e^{12}, e^{13} + e^{24}, e^{35}, e^{38} + e^{46} + e^{17}$                               | 149      |
| 941:447  | $0, 0, 0, 0, 0, -e^{12}, -e^{13}, e^{35} + e^{24}, e^{57} + e^{46} + e^{18}$                              | 149      |
| 941:448a | $0, 0, 0, 0, 0, -e^{12}, e^{34}, e^{13} + e^{25}, e^{47} + e^{18} + e^{56}$                               | 149      |
| 941:448b | $0, 0, 0, 0, 0, -e^{12}, e^{34}, -e^{13} + e^{25}, e^{47} + e^{56} + e^{18}$                              | 149      |
| 941:449a | $0, 0, 0, 0, 0, e^{12}, e^{13}, e^{45}, e^{26} + e^{37} + e^{58} + e^{14}$                                | 149      |
| 941:449b | $0, 0, 0, 0, 0, -e^{12}, e^{13}, e^{45}, e^{26} + e^{37} + e^{14} + e^{58}$                               | 149      |
| 941:450  | $0, 0, 0, 0, 0, e^{12}, e^{13}, e^{45}, e^{58} + e^{16} + e^{24} + e^{37}$                                | 149      |
| 941:451  | $0, 0, 0, 0, 0, e^{12}, e^{13}, e^{45}, e^{58} + e^{36} + e^{27} + e^{14}$                                | 149      |
| 941:452  | $0, 0, 0, 0, 0, (-1 + a_2)e^{12}, e^{23} + e^{14}, e^{25} + e^{13}a_2, e^{36} + e^{28} + e^{17}$          | 149      |
| 941:453  | $0, 0, 0, 0, 0, e^{12}, e^{14} + e^{23}, e^{15} + e^{34}, e^{26} + e^{37} + e^{18}$                       | 149      |
| 941:454a | $0, 0, 0, 0, 0, e^{12}, e^{14} + e^{23}, e^{45} + e^{13}, e^{48} + e^{16} + e^{37}$                       | 149      |
| 941:454b | $0, 0, 0, 0, 0, -e^{12}, e^{14} + e^{23}, e^{13} + e^{45}, e^{16} + e^{48} + e^{37}$                      | 149      |
| 941:455  | $0, 0, 0, 0, 0, e^{12}, e^{14} + e^{23}, e^{45} + e^{13}, e^{48} + e^{37} + e^{26}$                       | 149      |
| 941:456a | $0, 0, 0, 0, 0, e^{24} + e^{13}, e^{34} + e^{12}, e^{15}, e^{18} + e^{26} + e^{37}$                       | 149      |
| 941:456b | $0, 0, 0, 0, 0, -e^{24} + e^{13}, e^{34} + e^{12}, e^{15}, e^{37} + e^{18} + e^{26}$                      | 149      |
| 941:457a | $0, 0, 0, 0, 0, e^{13} + e^{24}, e^{12} + e^{34}, e^{15}, e^{18} + e^{27} + e^{36}$                       | 149      |
| 941:457b | $0, 0, 0, 0, 0, e^{24} - e^{13}, e^{12} + e^{34}, e^{15}, e^{36} + e^{27} + e^{18}$                       | 149      |
| 941:458  | $0, 0, 0, 0, 0, e^{12}, e^{13} + e^{24}, e^{15} + e^{34}, e^{28} + e^{37} + e^{56}$                       | 149      |
| 941:459a | $0, 0, 0, 0, 0, e^{23} + e^{14}, e^{24} + e^{13}, e^{15}, e^{58} + e^{27} + e^{16}$                       | 149      |
| 941:459b | $0, 0, 0, 0, 0, -e^{14} + e^{23}, e^{24} + e^{13}, e^{15}, e^{58} + e^{27} + e^{16}$                      | 149      |
| 941:460a | $0, 0, 0, 0, 0, e^{24} + e^{13}, e^{34} + e^{12}, e^{15}, e^{26} + e^{37} + e^{58}$                       | 149      |
| 941:460b | $0, 0, 0, 0, 0, -e^{24} + e^{13}, e^{34} + e^{12}, e^{15}, e^{37} + e^{26} + e^{58}$                      | 149      |
| 941:461a | $0, 0, 0, 0, 0, e^{13} + e^{24}, e^{12} + e^{34}, e^{15}, e^{58} + e^{27} + e^{36}$                       | 149      |
| 941:461b | $0, 0, 0, 0, 0, e^{24} + e^{13}, -e^{12} + e^{34}, e^{15}, e^{36} + e^{58} + e^{27}$                      | 149      |
| 941:461c | $0, 0, 0, 0, 0, -e^{13} + e^{24}, -e^{12} + e^{34}, e^{15}, e^{27} + e^{36} + e^{58}$                     | 149      |
| 941:462a | $0, 0, 0, 0, 0, e^{12}, e^{14} + e^{35}, e^{45} + e^{23}, e^{47} + e^{16} + e^{38}$                       | 149      |
| 941:462b | $0, 0, 0, 0, 0, -e^{12}, e^{14} + e^{35}, e^{23} + e^{45}, e^{16} + e^{47} + e^{38}$                      | 149      |
| 941:463  | $0, 0, 0, 0, 0, -e^{12}, e^{15} + e^{34}, e^{23} + e^{45}, e^{47} + e^{18} + e^{36}$                      | 149      |
| 941:464  | $0, 0, 0, 0, 0, e^{12}, e^{13}, e^{14} + e^{25}, e^{28} + e^{15} + e^{37} + e^{46}$                       | 149      |
| 941:465  | $0, 0, 0, 0, 0, e^{12}, e^{13}, e^{25} + e^{14}, e^{46} + e^{35} + e^{28} + e^{17}$                       | 149      |
| 941:466  | $0, 0, 0, 0, 0, -e^{12}, e^{13}, e^{25} + e^{14}, e^{18} + e^{37} + e^{56} + e^{24}$                      | 149      |
| 941:467  | $0, 0, 0, 0, 0, -e^{12}, -e^{13}, e^{24} + e^{35}, e^{18} + e^{23} + e^{57} + e^{46}$                     | 149      |
| 941:468  | $0, 0, 0, 0, 0, e^{12}, e^{34}, e^{13} + e^{25}, e^{36} + e^{47} + e^{28} + e^{15}$                       | 149      |
| 941:469a | $0, 0, 0, 0, 0, -e^{12}, e^{34}, e^{13} + e^{25}, e^{18} + e^{56} + e^{47} + e^{23}$                      | 149      |
| 941:469b | $0, 0, 0, 0, 0, -e^{12}, e^{34}, e^{25} - e^{13}, e^{18} + e^{47} + e^{56} + e^{23}$                      | 149      |
| 941:470  | $0, 0, 0, 0, 0, -e^{12}, e^{34}, e^{25} + e^{13}, e^{56} + e^{24} + e^{37} + e^{18}$                      | 149      |
| 941:471a | $0, 0, 0, 0, 0, e^{14} + e^{23}, e^{13}(1 + a_2) + e^{24}, e^{35} + e^{12}a_2, e^{38} + e^{27} + e^{16}$  | 149      |
| 941:471b | $0, 0, 0, 0, 0, -e^{14} + e^{23}, e^{13}(1 + a_2) + e^{24}, e^{35} + e^{12}a_2, e^{27} + e^{16} + e^{38}$ | 149      |

Table 2 – Continued to next page

Table 2 – Continued from previous page

| Name     | $\mathfrak{g}$                                                                                                     | UCS Dim. |
|----------|--------------------------------------------------------------------------------------------------------------------|----------|
| 941:472  | $0, 0, 0, 0, 0, e^{24} + e^{13}, e^{15} + e^{23}, e^{45} + e^{12}, e^{18} + e^{47} + e^{36}$                       | 149      |
| 941:473  | $0, 0, 0, 0, 0, e^{24} + e^{13}, e^{23} + e^{15}, e^{14} + e^{25}, e^{47} + e^{36} + e^{58}$                       | 149      |
| 941:474  | $0, 0, 0, 0, 0, e^{12}a_1, e^{23} + e^{14}, e^{25} + (1 + a_1)e^{13}, e^{17} + e^{28} + e^{36} + e^{45}$           | 149      |
| 941:475  | $0, 0, 0, 0, 0, e^{12}, e^{14} + e^{23}, e^{13} + e^{45}, e^{26} + e^{15} + e^{37} + e^{48}$                       | 149      |
| 941:476a | $0, 0, 0, 0, 0, e^{12}, e^{23} + e^{14}, e^{13} + e^{45}, e^{48} + e^{37} + e^{16} + e^{25}$                       | 149      |
| 941:476b | $0, 0, 0, 0, 0, -e^{12}, e^{14} + e^{23}, e^{45} + e^{13}, e^{37} + e^{48} + e^{25} + e^{16}$                      | 149      |
| 941:477  | $0, 0, 0, 0, 0, e^{12}, e^{24} + e^{13}, e^{15} + e^{34}, e^{28} + e^{37} + e^{14} + e^{56}$                       | 149      |
| 941:478  | $0, 0, 0, 0, 0, e^{12}, e^{24} - e^{13}, e^{34} + e^{15}, e^{18} + e^{47} + e^{26} + e^{35}$                       | 149      |
| 941:479a | $0, 0, 0, 0, 0, e^{24} + e^{13}, e^{34} - e^{12}, e^{15}, e^{16} + e^{58} + e^{47} + e^{23}$                       | 149      |
| 941:479b | $0, 0, 0, 0, 0, e^{24} - e^{13}, e^{34} - e^{12}, e^{15}, e^{16} + e^{23} + e^{47} + e^{58}$                       | 149      |
| 941:480a | $0, 0, 0, 0, 0, e^{13} + e^{24}, e^{34} + e^{12}, e^{15}, e^{58} + e^{37} + e^{14} + e^{26}$                       | 149      |
| 941:480b | $0, 0, 0, 0, 0, -e^{24} + e^{13}, e^{12} + e^{34}, e^{15}, e^{58} + e^{37} + e^{14} + e^{26}$                      | 149      |
| 941:481a | $0, 0, 0, 0, 0, e^{13} + e^{24}, e^{34} + e^{12}, e^{15}, e^{27} + e^{58} + e^{36} + e^{14}$                       | 149      |
| 941:481b | $0, 0, 0, 0, 0, e^{24} + e^{13}, e^{34} - e^{12}, e^{15}, e^{27} + e^{36} + e^{14} + e^{58}$                       | 149      |
| 941:481c | $0, 0, 0, 0, 0, -e^{13} + e^{24}, -e^{12} + e^{34}, e^{15}, e^{27} + e^{14} + e^{58} + e^{36}$                     | 149      |
| 941:482a | $0, 0, 0, 0, 0, e^{24} + e^{13}, e^{12} + e^{34}, e^{15}, e^{37} + e^{45} + e^{18} + e^{26}$                       | 149      |
| 941:482b | $0, 0, 0, 0, 0, e^{13} - e^{24}, e^{12} + e^{34}, e^{15}, e^{37} + e^{26} + e^{45} + e^{18}$                       | 149      |
| 941:483a | $0, 0, 0, 0, 0, e^{24} + e^{13}, e^{34} + e^{12}, e^{15}, e^{27} + e^{18} + e^{36} + e^{45}$                       | 149      |
| 941:483b | $0, 0, 0, 0, 0, -e^{13} + e^{24}, e^{12} + e^{34}, e^{15}, e^{18} + e^{27} + e^{45} + e^{36}$                      | 149      |
| 941:484  | $0, 0, 0, 0, 0, e^{12}, e^{35} + e^{14}, e^{45} - e^{23}, e^{27} + e^{58} + e^{46} + e^{13}$                       | 149      |
| 941:485a | $0, 0, 0, 0, 0, e^{12}, e^{35} + e^{14}, e^{45} + e^{23}, e^{15} + e^{26} + e^{47} + e^{38}$                       | 149      |
| 941:485b | $0, 0, 0, 0, 0, -e^{12}, e^{35} + e^{14}, e^{45} + e^{23}, e^{38} + e^{47} + e^{26} + e^{15}$                      | 149      |
| 941:486a | $0, 0, 0, 0, 0, e^{23} + e^{14}, e^{13}a_1 + e^{24}, (-1 + a_1)e^{12} + e^{35}, e^{45} + e^{38} + e^{27} + e^{16}$ | 149      |
| 941:486b | $0, 0, 0, 0, 0, e^{23} - e^{14}, e^{13}a_1 + e^{24}, (-1 + a_1)e^{12} + e^{35}, e^{16} + e^{38} + e^{27} + e^{45}$ | 149      |
| 941:487  | $0, 0, 0, 0, 0, e^{14} + e^{23}, e^{13} + e^{25}, e^{45} + e^{12}, e^{36} + e^{47} + e^{28} + e^{15}$              | 149      |
| 941:488  | $0, 0, 0, 0, 0, e^{13} + e^{24}, e^{15} + e^{23}, e^{25} + e^{14}, e^{47} + e^{58} + e^{36} + e^{12}$              | 149      |
| Type: 45 |                                                                                                                    |          |
| 95:1     | $0, 0, 0, 0, 0, e^{12}, e^{13}, e^{23}, e^{14}, e^{24}$                                                            | 59       |
| 95:2     | $0, 0, 0, 0, 0, e^{12}, e^{13}, e^{24}, e^{34}, e^{14} + e^{23}$                                                   | 59       |
| Type: 54 |                                                                                                                    |          |
| 94:1     | $0, 0, 0, 0, 0, 0, e^{12}, e^{13}, e^{23}, e^{14}$                                                                 | 59       |
| 94:2     | $0, 0, 0, 0, 0, 0, e^{12}, e^{13}, e^{24}, e^{34}$                                                                 | 59       |
| 94:3     | $0, 0, 0, 0, 0, 0, e^{12}, e^{13}, e^{24}, e^{14} + e^{23}$                                                        | 59       |
| 94:4a    | $0, 0, 0, 0, 0, 0, e^{12}, e^{34}, e^{14} + e^{23}, e^{13} + e^{24}$                                               | 59       |
| 94:4b    | $0, 0, 0, 0, 0, 0, e^{12}, e^{34}, e^{23} - e^{14}, e^{24} + e^{13}$                                               | 59       |
| 94:5     | $0, 0, 0, 0, 0, 0, e^{12}, e^{13}, e^{23}, e^{45}$                                                                 | 49       |
| 94:6     | $0, 0, 0, 0, 0, 0, e^{12}, e^{13}, e^{14}, e^{15}$                                                                 | 49       |
| 94:7     | $0, 0, 0, 0, 0, 0, e^{12}, e^{13}, e^{14}, e^{25}$                                                                 | 49       |
| 94:8     | $0, 0, 0, 0, 0, 0, e^{12}, e^{13}, e^{24}, e^{35}$                                                                 | 49       |
| 94:9     | $0, 0, 0, 0, 0, 0, e^{12}, e^{13}, e^{23}, e^{14} + e^{25}$                                                        | 49       |
| 94:10    | $0, 0, 0, 0, 0, 0, e^{12}, e^{13}, e^{14}, e^{15} + e^{23}$                                                        | 49       |
| 94:11    | $0, 0, 0, 0, 0, 0, e^{12}, e^{13}, e^{24}, e^{15} + e^{23}$                                                        | 49       |
| 94:12    | $0, 0, 0, 0, 0, 0, e^{12}, e^{13}, e^{14}, e^{45} + e^{23}$                                                        | 49       |
| 94:13    | $0, 0, 0, 0, 0, 0, e^{12}, e^{13}, e^{24}, e^{35} + e^{14}$                                                        | 49       |
| 94:14    | $0, 0, 0, 0, 0, 0, e^{12}, e^{13}, e^{24}, e^{15} + e^{34}$                                                        | 49       |
| 94:15    | $0, 0, 0, 0, 0, 0, e^{12}, e^{13}, e^{14} + e^{23}, e^{45}$                                                        | 49       |
| 94:16    | $0, 0, 0, 0, 0, 0, e^{12}, e^{34}, e^{24} + e^{13}, e^{15}$                                                        | 49       |
| 94:17    | $0, 0, 0, 0, 0, 0, e^{12}, e^{13}, e^{45}, e^{35} + e^{24}$                                                        | 49       |
| 94:18    | $0, 0, 0, 0, 0, 0, e^{12}, e^{13}, e^{14} + e^{23}, e^{24} + e^{15}$                                               | 49       |
| 94:19    | $0, 0, 0, 0, 0, 0, e^{12}, e^{13}, e^{14} + e^{23}, e^{24} + e^{35}$                                               | 49       |
| 94:20a   | $0, 0, 0, 0, 0, 0, e^{12}, e^{23} + e^{14}, e^{24} + e^{13}, e^{15}$                                               | 49       |
| 94:20b   | $0, 0, 0, 0, 0, 0, e^{12}, e^{23} - e^{14}, e^{24} + e^{13}, e^{15}$                                               | 49       |
| 94:21    | $0, 0, 0, 0, 0, 0, e^{12}, e^{34}, e^{14} + e^{23}, e^{25} + e^{13}$                                               | 49       |
| 94:22a   | $0, 0, 0, 0, 0, 0, e^{12}, e^{14} + e^{23}, e^{13} + e^{24}, e^{35}$                                               | 49       |
| 94:22b   | $0, 0, 0, 0, 0, 0, e^{12}, -e^{14} + e^{23}, e^{13} + e^{24}, e^{35}$                                              | 49       |
| 94:23    | $0, 0, 0, 0, 0, 0, e^{12}, e^{13}, e^{24} + e^{15}, e^{35} + e^{14}$                                               | 49       |
| 94:24    | $0, 0, 0, 0, 0, 0, e^{12}, e^{13}, e^{25} + e^{14}, e^{23} + e^{45}$                                               | 49       |
| 94:25    | $0, 0, 0, 0, 0, 0, e^{12}, e^{13}, e^{25} + e^{14}, e^{35} + e^{24}$                                               | 49       |

Table 2 – Continued to next page

Table 2 – Continued from previous page

| Name       | $\mathfrak{g}$                                                                      | UCS Dim. |
|------------|-------------------------------------------------------------------------------------|----------|
| 94:26a     | $0, 0, 0, 0, 0, e^{12}, e^{13}, e^{35} + e^{24}, e^{45} + e^{23}$                   | 49       |
| 94:26b     | $0, 0, 0, 0, 0, e^{12}, e^{13}, e^{35} - e^{24}, e^{45} + e^{23}$                   | 49       |
| 94:27a     | $0, 0, 0, 0, 0, e^{12}, e^{13}, e^{25} + e^{34}, e^{24} + e^{35}$                   | 49       |
| 94:27b     | $0, 0, 0, 0, 0, e^{12}, e^{13}, e^{34} - e^{25}, e^{35} + e^{24}$                   | 49       |
| 94:28      | $0, 0, 0, 0, 0, e^{12}, e^{34}, e^{15} + e^{23}, e^{14} + e^{25}$                   | 49       |
| 94:29      | $0, 0, 0, 0, 0, e^{12}, e^{34}, e^{23} + e^{15}, e^{13} + e^{45}$                   | 49       |
| 94:30      | $0, 0, 0, 0, 0, e^{12}, e^{34}, e^{15} + e^{23}, e^{35} + e^{14}$                   | 49       |
| 94:31a     | $0, 0, 0, 0, 0, e^{12}, e^{14} + e^{23}, e^{13} + e^{24}, e^{15} + e^{34}$          | 49       |
| 94:31b     | $0, 0, 0, 0, 0, e^{12}, e^{23} - e^{14}, e^{24} + e^{13}, e^{34} + e^{15}$          | 49       |
| 94:32a     | $0, 0, 0, 0, 0, e^{23} + e^{14}, e^{24} + e^{13}, e^{34} + e^{12}, e^{15}$          | 49       |
| 94:32b     | $0, 0, 0, 0, 0, e^{14} + e^{23}, e^{24} - e^{13}, e^{34} + e^{12}, e^{15}$          | 49       |
| 94:33      | $0, 0, 0, 0, 0, e^{12}, e^{13} + e^{24}, e^{15} + e^{23}, e^{25} + e^{14}$          | 49       |
| 94:34      | $0, 0, 0, 0, 0, e^{12}, e^{24} + e^{13}, e^{23} + e^{15}, e^{35} + e^{14}$          | 49       |
| 94:35a     | $0, 0, 0, 0, 0, e^{12}, e^{23} + e^{14}, e^{15} + e^{34}, e^{13} + e^{45}$          | 49       |
| 94:35b     | $0, 0, 0, 0, 0, e^{12}, e^{14} + e^{23}, e^{34} - e^{15}, e^{13} + e^{45}$          | 49       |
| 94:36      | $0, 0, 0, 0, 0, e^{12}, e^{13} + e^{24}, e^{35} + e^{14}, e^{45} + e^{23}$          | 49       |
| 94:37      | $0, 0, 0, 0, 0, e^{12}, e^{13} + e^{24}, e^{15} + e^{34}, e^{45} + e^{23}$          | 49       |
| 94:38a     | $0, 0, 0, 0, 0, e^{24} + e^{13}, e^{34} + e^{12}, e^{15}, e^{45} + e^{23}$          | 49       |
| 94:38b     | $0, 0, 0, 0, 0, e^{24} - e^{13}, e^{34} + e^{12}, e^{15}, e^{23} + e^{45}$          | 49       |
| 94:39a     | $0, 0, 0, 0, 0, e^{13} + e^{24}, e^{34} + e^{12}, e^{15} + e^{23}, e^{25} + e^{14}$ | 49       |
| 94:39b     | $0, 0, 0, 0, 0, e^{24} - e^{13}, e^{34} + e^{12}, e^{23} + e^{15}, e^{25} + e^{14}$ | 49       |
| 94:40      | $0, 0, 0, 0, 0, e^{12} + e^{34}, e^{23} + e^{15}, e^{14} + e^{25}, e^{13} + e^{45}$ | 49       |
| Type: 6111 |                                                                                     |          |
| 9321:1     | $0, 0, 0, 0, 0, 0, e^{12}, e^{17}, e^{18}$                                          | 5679     |
| 9321:2     | $0, 0, 0, 0, 0, 0, e^{12}, e^{17}, e^{18} + e^{34}$                                 | 3679     |
| 9321:3     | $0, 0, 0, 0, 0, 0, e^{12}, e^{17}, e^{18} + e^{23}$                                 | 4679     |
| 9321:4     | $0, 0, 0, 0, 0, 0, e^{12}, e^{17}, e^{18} + e^{34} + e^{56}$                        | 1679     |
| 9321:5     | $0, 0, 0, 0, 0, 0, e^{12}, e^{17}, e^{18} + e^{27}$                                 | 5679     |
| 9321:6     | $0, 0, 0, 0, 0, 0, e^{12}, e^{17}, e^{45} + e^{18} + e^{23}$                        | 2679     |
| 9321:7     | $0, 0, 0, 0, 0, 0, e^{12}, e^{17}, e^{18} + e^{34} + e^{27}$                        | 3679     |
| 9321:8     | $0, 0, 0, 0, 0, 0, e^{12}, e^{17}, e^{56} + e^{27} + e^{18} + e^{34}$               | 1679     |
| 9321:9     | $0, 0, 0, 0, 0, 0, -e^{12}, e^{17} + e^{23}, e^{18} + e^{37}$                       | 4579     |
| 9321:10    | $0, 0, 0, 0, 0, 0, -e^{12}, e^{17} + e^{23}, e^{18} + e^{37} + e^{45}$              | 2579     |
| 9321:11    | $0, 0, 0, 0, 0, 0, e^{12}, e^{27} + e^{13}, e^{28} + e^{14} + e^{37}$               | 3579     |
| 9321:12    | $0, 0, 0, 0, 0, 0, e^{12}, e^{13} + e^{27}, e^{14} + e^{56} + e^{28} + e^{37}$      | 1579     |
| Type: 612  |                                                                                     |          |
| 932:1      | $0, 0, 0, 0, 0, 0, e^{12}, e^{17}, e^{27}$                                          | 679      |
| 932:2      | $0, 0, 0, 0, 0, 0, e^{12}, e^{17}, e^{13} + e^{27}$                                 | 579      |
| 932:3      | $0, 0, 0, 0, 0, 0, e^{12}, e^{17}, e^{27} + e^{34}$                                 | 479      |
| 932:4a     | $0, 0, 0, 0, 0, 0, e^{12}, e^{17} + e^{23}, e^{27} + e^{13}$                        | 579      |
| 932:4b     | $0, 0, 0, 0, 0, 0, e^{12}, -e^{17} + e^{23}, e^{27} + e^{13}$                       | 579      |
| 932:5      | $0, 0, 0, 0, 0, 0, e^{12}, e^{27} + e^{13}, e^{17} + e^{34}$                        | 479      |
| 932:6      | $0, 0, 0, 0, 0, 0, e^{12}, e^{17} + e^{34}, e^{35} + e^{27}$                        | 379      |
| 932:7      | $0, 0, 0, 0, 0, 0, e^{12}, e^{23} + e^{17}, e^{14} + e^{27}$                        | 479      |
| 932:8      | $0, 0, 0, 0, 0, 0, e^{12}, e^{17}, e^{13} + e^{27} + e^{45}$                        | 379      |
| 932:9      | $0, 0, 0, 0, 0, 0, e^{12}, e^{27} + e^{13}, e^{17} + e^{45}$                        | 379      |
| 932:10     | $0, 0, 0, 0, 0, 0, e^{12}, e^{17}, e^{27} + e^{56} + e^{34}$                        | 279      |
| 932:11     | $0, 0, 0, 0, 0, 0, e^{12}, e^{17} + e^{34}, e^{27} + e^{56}$                        | 279      |
| 932:12     | $0, 0, 0, 0, 0, 0, e^{12}, e^{17} + e^{34}, e^{27} + e^{13} + e^{45}$               | 379      |
| 932:13     | $0, 0, 0, 0, 0, 0, e^{12}, e^{17} + e^{34}, e^{27} + e^{46} + e^{35}$               | 279      |
| 932:14a    | $0, 0, 0, 0, 0, 0, e^{12}, e^{27} + e^{13}, e^{23} + e^{45} + e^{17}$               | 379      |
| 932:14b    | $0, 0, 0, 0, 0, 0, e^{12}, -e^{13} + e^{27}, e^{23} + e^{45} + e^{17}$              | 379      |
| 932:15     | $0, 0, 0, 0, 0, 0, e^{12}, e^{13} + e^{27}, e^{24} + e^{35} + e^{17}$               | 379      |
| 932:16     | $0, 0, 0, 0, 0, 0, e^{12}, e^{13} + e^{27}, e^{56} + e^{17} + e^{34}$               | 279      |
| 932:17     | $0, 0, 0, 0, 0, 0, e^{12}, e^{17} + e^{34}, e^{27} + e^{56} + e^{13}$               | 279      |
| 932:18     | $0, 0, 0, 0, 0, 0, e^{12}, e^{17} + e^{34}, e^{15} + e^{27} + e^{36}$               | 279      |
| 932:19a    | $0, 0, 0, 0, 0, 0, e^{12}, e^{17} + e^{35} + e^{46}, e^{34} + e^{27} + e^{56}$      | 279      |
| 932:19b    | $0, 0, 0, 0, 0, 0, e^{12}, e^{46} - e^{35} + e^{17}, e^{34} + e^{56} + e^{27}$      | 279      |

Table 2 – Continued to next page

Table 2 – Continued from previous page

| Name      | $\mathfrak{g}$                                                                 | UCS Dim. |
|-----------|--------------------------------------------------------------------------------|----------|
| 932:20    | $0, 0, 0, 0, 0, 0, e^{12}, e^{27} + e^{13}, e^{24} + e^{56} + e^{17}$          | 279      |
| 932:21    | $0, 0, 0, 0, 0, 0, e^{12}, e^{35} + e^{24} + e^{17}, e^{13} + e^{45} + e^{27}$ | 379      |
| 932:22    | $0, 0, 0, 0, 0, 0, e^{12}, e^{13} + e^{27} + e^{45}, e^{34} + e^{17} + e^{56}$ | 279      |
| 932:23a   | $0, 0, 0, 0, 0, 0, e^{12}, e^{17} + e^{45} + e^{23}, e^{27} + e^{46} + e^{13}$ | 279      |
| 932:23b   | $0, 0, 0, 0, 0, 0, e^{12}, e^{45} + e^{23} - e^{17}, e^{27} + e^{13} + e^{46}$ | 279      |
| 932:24    | $0, 0, 0, 0, 0, 0, e^{12}, e^{17} + e^{35} + e^{24}, e^{27} + e^{46} + e^{13}$ | 279      |
| 932:25    | $0, 0, 0, 0, 0, 0, e^{12}, e^{17} + e^{25} + e^{34}, e^{46} + e^{27} + e^{13}$ | 279      |
| Type: 621 |                                                                                |          |
| 931:1     | $0, 0, 0, 0, 0, 0, e^{12}, e^{13}, e^{17}$                                     | 579      |
| 931:2     | $0, 0, 0, 0, 0, 0, e^{12}, e^{13}, e^{27}$                                     | 579      |
| 931:3     | $0, 0, 0, 0, 0, 0, e^{12}, e^{34}, e^{17}$                                     | 479      |
| 931:4     | $0, 0, 0, 0, 0, 0, e^{12}, e^{13}, e^{17} + e^{23}$                            | 579      |
| 931:5     | $0, 0, 0, 0, 0, 0, e^{12}, e^{13}, e^{17} + e^{34}$                            | 479      |
| 931:6     | $0, 0, 0, 0, 0, 0, e^{12}, e^{13}, e^{27} + e^{34}$                            | 479      |
| 931:7     | $0, 0, 0, 0, 0, 0, e^{12}, e^{24} + e^{13}, e^{17}$                            | 479      |
| 931:8     | $0, 0, 0, 0, 0, 0, e^{12}, e^{34}, e^{27} + e^{13}$                            | 479      |
| 931:9     | $0, 0, 0, 0, 0, 0, e^{12}, e^{34}, e^{17} + e^{35}$                            | 379      |
| 931:10    | $0, 0, 0, 0, 0, 0, e^{12}, e^{45} + e^{13}, e^{17}$                            | 379      |
| 931:11    | $0, 0, 0, 0, 0, 0, e^{12}, e^{13} + e^{45}, e^{27}$                            | 379      |
| 931:12    | $0, 0, 0, 0, 0, 0, e^{12}, e^{34} + e^{56}, e^{17}$                            | 279      |
| 931:13    | $0, 0, 0, 0, 0, 0, e^{12}, e^{13}, e^{27} + e^{14}$                            | 479      |
| 931:14    | $0, 0, 0, 0, 0, 0, e^{12}, e^{13}, e^{24} + e^{17}$                            | 479      |
| 931:15    | $0, 0, 0, 0, 0, 0, e^{12}, e^{13}, e^{17} + e^{45}$                            | 379      |
| 931:16    | $0, 0, 0, 0, 0, 0, e^{12}, e^{13}, e^{27} + e^{45}$                            | 379      |
| 931:17    | $0, 0, 0, 0, 0, 0, e^{12}, e^{34}, e^{27} + e^{15}$                            | 379      |
| 931:18    | $0, 0, 0, 0, 0, 0, e^{12}, e^{34}, e^{56} + e^{17}$                            | 279      |
| 931:19    | $0, 0, 0, 0, 0, 0, e^{12}, e^{24} + e^{13}, e^{17} + e^{34}$                   | 479      |
| 931:20    | $0, 0, 0, 0, 0, 0, e^{12}, e^{45} + e^{13}, e^{34} + e^{17}$                   | 379      |
| 931:21    | $0, 0, 0, 0, 0, 0, e^{12}, e^{13} + e^{45}, e^{34} + e^{27}$                   | 379      |
| 931:22    | $0, 0, 0, 0, 0, 0, e^{12}, e^{46} + e^{35}, e^{17} + e^{34}$                   | 279      |
| 931:23    | $0, 0, 0, 0, 0, 0, e^{12}, e^{23} + e^{14}, e^{27} + e^{13}$                   | 479      |
| 931:24    | $0, 0, 0, 0, 0, 0, e^{12}, e^{24} + e^{13}, e^{17} + e^{35}$                   | 379      |
| 931:25    | $0, 0, 0, 0, 0, 0, e^{12}, e^{14} + e^{23}, e^{35} + e^{17}$                   | 379      |
| 931:26    | $0, 0, 0, 0, 0, 0, e^{12}, e^{34}, e^{13} + e^{27} + e^{45}$                   | 379      |
| 931:27    | $0, 0, 0, 0, 0, 0, e^{12}, e^{35} + e^{14}, e^{13} + e^{27}$                   | 379      |
| 931:28    | $0, 0, 0, 0, 0, 0, e^{12}, e^{13} + e^{45}, e^{17} + e^{23}$                   | 379      |
| 931:29    | $0, 0, 0, 0, 0, 0, e^{12}, e^{35} + e^{14}, e^{17} + e^{23}$                   | 379      |
| 931:30    | $0, 0, 0, 0, 0, 0, e^{12}, e^{34}, e^{46} + e^{35} + e^{17}$                   | 279      |
| 931:31    | $0, 0, 0, 0, 0, 0, e^{12}, e^{45} + e^{13}, e^{17} + e^{36}$                   | 279      |
| 931:32    | $0, 0, 0, 0, 0, 0, e^{12}, e^{14} + e^{35}, e^{17} + e^{36}$                   | 279      |
| 931:33    | $0, 0, 0, 0, 0, 0, e^{12}, e^{45} + e^{13}, e^{36} + e^{27}$                   | 279      |
| 931:34    | $0, 0, 0, 0, 0, 0, e^{12}, e^{14} + e^{35}, e^{27} + e^{36}$                   | 279      |
| 931:35    | $0, 0, 0, 0, 0, 0, e^{12}, e^{24} + e^{13} + e^{56}, e^{17}$                   | 279      |
| 931:36    | $0, 0, 0, 0, 0, 0, e^{12}, e^{56} + e^{34}, e^{13} + e^{27}$                   | 279      |
| 931:37a   | $0, 0, 0, 0, 0, 0, e^{12}, e^{56} + e^{34}, e^{17} + e^{46} + e^{35}$          | 279      |
| 931:37b   | $0, 0, 0, 0, 0, 0, e^{12}, e^{56} - e^{34}, e^{17} + e^{46} + e^{35}$          | 279      |
| 931:38    | $0, 0, 0, 0, 0, 0, e^{12}, e^{13}, e^{27} + e^{35} + e^{14}$                   | 379      |
| 931:39    | $0, 0, 0, 0, 0, 0, e^{12}, e^{13}, e^{45} + e^{17} + e^{23}$                   | 379      |
| 931:40    | $0, 0, 0, 0, 0, 0, e^{12}, e^{13}, e^{17} + e^{24} + e^{35}$                   | 379      |
| 931:41    | $0, 0, 0, 0, 0, 0, e^{12}, e^{13} + e^{24}, e^{15} + e^{27}$                   | 379      |
| 931:42    | $0, 0, 0, 0, 0, 0, e^{12}, e^{13}, e^{56} + e^{17} + e^{34}$                   | 279      |
| 931:43    | $0, 0, 0, 0, 0, 0, e^{12}, e^{13}, e^{34} + e^{27} + e^{56}$                   | 279      |
| 931:44    | $0, 0, 0, 0, 0, 0, e^{12}, e^{13} + e^{24}, e^{17} + e^{56}$                   | 279      |
| 931:45    | $0, 0, 0, 0, 0, 0, e^{12}, e^{34}, e^{27} + e^{13} + e^{56}$                   | 279      |
| 931:46    | $0, 0, 0, 0, 0, 0, e^{12}, e^{34}, e^{15} + e^{27} + e^{36}$                   | 279      |
| 931:47    | $0, 0, 0, 0, 0, 0, e^{12}, e^{13} + e^{45}, e^{16} + e^{27}$                   | 279      |
| 931:48    | $0, 0, 0, 0, 0, 0, e^{12}, e^{13} + e^{45}, e^{17} + e^{26}$                   | 279      |
| 931:49a   | $0, 0, 0, 0, 0, 0, e^{12}, e^{45} + e^{13}, e^{35} + e^{27} + e^{14}$          | 379      |

Table 2 – Continued to next page

Table 2 – Continued from previous page

| Name    | $\mathfrak{g}$                                                                 | UCS Dim. |
|---------|--------------------------------------------------------------------------------|----------|
| 931:49b | $0, 0, 0, 0, 0, 0, e^{12}, -e^{13} + e^{45}, e^{35} + e^{14} + e^{27}$         | 379      |
| 931:50  | $0, 0, 0, 0, 0, 0, e^{12}, e^{45} + e^{13}, e^{24} + e^{35} + e^{17}$          | 379      |
| 931:51  | $0, 0, 0, 0, 0, 0, e^{12}, e^{13} + e^{45}, e^{56} + e^{17} + e^{34}$          | 279      |
| 931:52  | $0, 0, 0, 0, 0, 0, e^{12}, e^{45} + e^{13}, e^{27} + e^{56} + e^{34}$          | 279      |
| 931:53  | $0, 0, 0, 0, 0, 0, e^{12}, e^{24} + e^{13} + e^{56}, e^{17} + e^{34}$          | 279      |
| 931:54  | $0, 0, 0, 0, 0, 0, e^{12}, e^{25} + e^{13} + e^{46}, e^{17} + e^{34}$          | 279      |
| 931:55  | $0, 0, 0, 0, 0, 0, e^{12}, e^{46} + e^{15} + e^{23}, e^{34} + e^{17}$          | 279      |
| 931:56  | $0, 0, 0, 0, 0, 0, e^{12}, e^{34} + e^{56}, e^{13} + e^{27} + e^{45}$          | 279      |
| 931:57  | $0, 0, 0, 0, 0, 0, e^{12}, e^{13}, e^{56} + e^{14} + e^{27}$                   | 279      |
| 931:58  | $0, 0, 0, 0, 0, 0, e^{12}, e^{13}, e^{24} + e^{17} + e^{56}$                   | 279      |
| 931:59  | $0, 0, 0, 0, 0, 0, e^{12}, e^{13} + e^{24}, e^{27} + e^{35} + e^{14}$          | 379      |
| 931:60  | $0, 0, 0, 0, 0, 0, e^{12}, e^{13} + e^{24}, e^{15} + e^{27} + e^{34}$          | 379      |
| 931:61  | $0, 0, 0, 0, 0, 0, e^{12}, e^{24} + e^{13}, e^{17} + e^{34} + e^{56}$          | 279      |
| 931:62  | $0, 0, 0, 0, 0, 0, e^{12}, e^{24} + e^{13}, e^{46} + e^{17} + e^{35}$          | 279      |
| 931:63  | $0, 0, 0, 0, 0, 0, e^{12}, e^{45} + e^{13}, e^{36} + e^{27} + e^{14}$          | 279      |
| 931:64  | $0, 0, 0, 0, 0, 0, e^{12}, e^{13} + e^{45}, e^{16} + e^{34} + e^{27}$          | 279      |
| 931:65  | $0, 0, 0, 0, 0, 0, e^{12}, e^{13} + e^{45}, e^{23} + e^{46} + e^{17}$          | 279      |
| 931:66  | $0, 0, 0, 0, 0, 0, e^{12}, e^{45} + e^{13}, e^{24} + e^{36} + e^{17}$          | 279      |
| 931:67  | $0, 0, 0, 0, 0, 0, e^{12}, e^{13} + e^{45}, e^{26} + e^{17} + e^{34}$          | 279      |
| 931:68  | $0, 0, 0, 0, 0, 0, e^{12}, e^{34} + e^{15}, e^{27} + e^{46} + e^{13}$          | 279      |
| 931:69  | $0, 0, 0, 0, 0, 0, e^{12}, e^{15} + e^{34}, e^{17} + e^{46} + e^{23}$          | 279      |
| 931:70  | $0, 0, 0, 0, 0, 0, e^{12}, e^{14} + e^{23} + e^{56}, e^{27} + e^{13}$          | 279      |
| 931:71  | $0, 0, 0, 0, 0, 0, e^{12}, e^{25} + e^{14} + e^{36}, e^{27} + e^{13}$          | 279      |
| 931:72  | $0, 0, 0, 0, 0, 0, e^{12}, e^{46} + e^{25} + e^{13}, e^{34} + e^{56} + e^{17}$ | 279      |
| 931:73  | $0, 0, 0, 0, 0, 0, e^{12}, e^{24} + e^{13}, e^{36} + e^{15} + e^{27}$          | 279      |
| 931:74  | $0, 0, 0, 0, 0, 0, e^{12}, e^{24} + e^{13}, e^{17} + e^{23} + e^{56}$          | 279      |
| 931:75  | $0, 0, 0, 0, 0, 0, e^{12}, e^{13} + e^{24}, e^{17} + e^{36} + e^{25}$          | 279      |
| 931:76  | $0, 0, 0, 0, 0, 0, e^{12}, e^{14} + e^{56} + e^{23}, e^{27} + e^{13} + e^{45}$ | 279      |
| 931:77  | $0, 0, 0, 0, 0, 0, e^{12}, e^{25} + e^{36} + e^{14}, e^{27} + e^{45} + e^{13}$ | 279      |
| 931:78a | $0, 0, 0, 0, 0, 0, e^{12}, e^{14} + e^{26} + e^{35}, e^{27} + e^{13} + e^{45}$ | 279      |
| 931:78b | $0, 0, 0, 0, 0, 0, e^{12}, e^{35} - e^{14} + e^{26}, e^{45} + e^{27} + e^{13}$ | 279      |
| 931:79  | $0, 0, 0, 0, 0, 0, e^{12}, e^{35} + e^{24} + e^{16}, e^{27} + e^{45} + e^{13}$ | 279      |
| 931:80  | $0, 0, 0, 0, 0, 0, e^{12}, e^{13}, e^{27} + e^{18}$                            | 469      |
| 931:81a | $0, 0, 0, 0, 0, 0, e^{12}, e^{13}, e^{38} + e^{27}$                            | 469      |
| 931:81b | $0, 0, 0, 0, 0, 0, -e^{12}, e^{13}, e^{38} + e^{27}$                           | 469      |
| 931:82  | $0, 0, 0, 0, 0, 0, e^{12}, e^{13}, e^{28} + e^{37}$                            | 469      |
| 931:83a | $0, 0, 0, 0, 0, 0, e^{12}, e^{13}, e^{14} + e^{38} + e^{27}$                   | 369      |
| 931:83b | $0, 0, 0, 0, 0, 0, -e^{12}, e^{13}, e^{38} + e^{27} + e^{14}$                  | 369      |
| 931:84  | $0, 0, 0, 0, 0, 0, e^{12}, e^{13}, e^{24} + e^{38} + e^{17}$                   | 369      |
| 931:85  | $0, 0, 0, 0, 0, 0, e^{12}, e^{13}, e^{37} + e^{14} + e^{28}$                   | 369      |
| 931:86  | $0, 0, 0, 0, 0, 0, e^{12}, e^{13}, e^{18} + e^{27} + e^{45}$                   | 269      |
| 931:87a | $0, 0, 0, 0, 0, 0, e^{12}, e^{13}, e^{38} + e^{27} + e^{45}$                   | 269      |
| 931:87b | $0, 0, 0, 0, 0, 0, -e^{12}, e^{13}, e^{27} + e^{45} + e^{38}$                  | 269      |
| 931:88  | $0, 0, 0, 0, 0, 0, e^{12}, e^{13}, e^{45} + e^{28} + e^{37}$                   | 269      |
| 931:89a | $0, 0, 0, 0, 0, 0, e^{12}, e^{13}, e^{14} + e^{56} + e^{38} + e^{27}$          | 169      |
| 931:89b | $0, 0, 0, 0, 0, 0, -e^{12}, e^{13}, e^{14} + e^{38} + e^{27} + e^{56}$         | 169      |
| 931:90  | $0, 0, 0, 0, 0, 0, e^{12}, e^{13}, e^{38} + e^{56} + e^{24} + e^{17}$          | 169      |
| 931:91  | $0, 0, 0, 0, 0, 0, e^{12}, e^{13}, e^{37} + e^{14} + e^{56} + e^{28}$          | 169      |
| 931:92  | $0, 0, 0, 0, 0, 0, e^{12}, e^{34}, e^{17} + e^{38}$                            | 359      |
| 931:93  | $0, 0, 0, 0, 0, 0, -e^{12}, e^{14} + e^{23}, e^{18} + e^{37}$                  | 359      |
| 931:94  | $0, 0, 0, 0, 0, 0, e^{12}, e^{34}, e^{13} + e^{48} + e^{27}$                   | 359      |
| 931:95  | $0, 0, 0, 0, 0, 0, e^{12}, e^{34}, e^{38} + e^{15} + e^{27}$                   | 259      |
| 931:96  | $0, 0, 0, 0, 0, 0, e^{12}, e^{34}, e^{17} + e^{56} + e^{38}$                   | 159      |
| 931:97a | $0, 0, 0, 0, 0, 0, e^{14} + e^{23}, e^{13} + e^{24}, e^{17} + e^{28}$          | 359      |
| 931:97b | $0, 0, 0, 0, 0, 0, e^{23} - e^{14}, e^{24} + e^{13}, e^{28} + e^{17}$          | 359      |
| 931:98  | $0, 0, 0, 0, 0, 0, e^{12}, e^{13} + e^{24}, e^{28} + e^{14} + e^{37}$          | 359      |
| 931:99  | $0, 0, 0, 0, 0, 0, e^{12}, e^{24} + e^{13}, e^{37} + e^{15} + e^{28}$          | 259      |
| 931:100 | $0, 0, 0, 0, 0, 0, -e^{12}, e^{24} + e^{13}, e^{18} + e^{47} + e^{35}$         | 259      |

Table 2 – Continued to next page

Table 2 – Continued from previous page

| Name     | $\mathfrak{g}$                                                                           | UCS Dim. |
|----------|------------------------------------------------------------------------------------------|----------|
| 931:101  | $0, 0, 0, 0, 0, 0, -e^{12}, e^{14} + e^{23}, e^{37} + e^{18} + e^{56}$                   | 159      |
| 931:102  | $0, 0, 0, 0, 0, 0, e^{12}, e^{34}, e^{48} + e^{56} + e^{27} + e^{13}$                    | 159      |
| 931:103  | $0, 0, 0, 0, 0, 0, e^{12}, e^{34}, e^{48} + e^{27} + e^{36} + e^{15}$                    | 159      |
| 931:104a | $0, 0, 0, 0, 0, 0, e^{24} + e^{13}, -e^{12} + e^{34}, e^{48} + e^{17} + e^{23}$          | 359      |
| 931:104b | $0, 0, 0, 0, 0, 0, -e^{13} + e^{24}, -e^{12} + e^{34}, e^{48} + e^{23} + e^{17}$         | 359      |
| 931:105a | $0, 0, 0, 0, 0, 0, e^{24} + e^{13}, e^{34} + e^{12}, e^{15} + e^{27} + e^{38}$           | 259      |
| 931:105b | $0, 0, 0, 0, 0, 0, e^{13} - e^{24}, e^{12} + e^{34}, e^{27} + e^{15} + e^{38}$           | 259      |
| 931:106a | $0, 0, 0, 0, 0, 0, e^{24} + e^{13}, e^{12} + e^{34}, e^{37} + e^{15} + e^{28}$           | 259      |
| 931:106b | $0, 0, 0, 0, 0, 0, -e^{13} + e^{24}, e^{12} + e^{34}, e^{37} + e^{15} + e^{28}$          | 259      |
| 931:107a | $0, 0, 0, 0, 0, 0, e^{23} + e^{14}, e^{24} + e^{13}, e^{56} + e^{28} + e^{17}$           | 159      |
| 931:107b | $0, 0, 0, 0, 0, 0, -e^{14} + e^{23}, e^{13} + e^{24}, e^{17} + e^{28} + e^{56}$          | 159      |
| 931:108  | $0, 0, 0, 0, 0, 0, e^{12}, e^{24} + e^{13}, e^{56} + e^{37} + e^{14} + e^{28}$           | 159      |
| 931:109  | $0, 0, 0, 0, 0, 0, e^{12}, e^{13} + e^{24}, e^{28} + e^{37} + e^{46} + e^{15}$           | 159      |
| 931:110a | $0, 0, 0, 0, 0, 0, e^{24} + e^{13}, e^{34} - e^{12}, e^{17} + e^{23} + e^{56} + e^{48}$  | 159      |
| 931:110b | $0, 0, 0, 0, 0, 0, e^{24} - e^{13}, e^{34} - e^{12}, e^{23} + e^{48} + e^{56} + e^{17}$  | 159      |
| 931:111a | $0, 0, 0, 0, 0, 0, e^{24} + e^{13}, -e^{12} + e^{34}, e^{48} + e^{36} + e^{25} + e^{17}$ | 159      |
| 931:111b | $0, 0, 0, 0, 0, 0, e^{24} - e^{13}, e^{34} - e^{12}, e^{17} + e^{36} + e^{48} + e^{25}$  | 159      |
| 931:112  | $0, 0, 0, 0, 0, 0, e^{23} + e^{14}, e^{25} + e^{13}, e^{28} + e^{17}$                    | 249      |
| 931:113  | $0, 0, 0, 0, 0, 0, e^{13} + e^{24}, e^{35} + e^{12}, e^{38} + e^{27} + e^{14}$           | 249      |
| 931:114  | $0, 0, 0, 0, 0, 0, e^{23} + e^{14}, e^{13} + e^{25}, e^{45} + e^{28} + e^{17}$           | 249      |
| 931:115  | $0, 0, 0, 0, 0, 0, e^{13} + e^{24}, e^{35} + e^{12}, e^{27} + e^{38} + e^{16}$           | 149      |
| 931:116  | $0, 0, 0, 0, 0, 0, e^{23} + e^{14}, e^{25} + e^{13}, e^{28} + e^{17} + e^{46}$           | 149      |
| 931:117  | $0, 0, 0, 0, 0, 0, e^{13} + e^{24}, e^{12} + e^{35}, e^{27} + e^{14} + e^{38} + e^{56}$  | 149      |
| 931:118  | $0, 0, 0, 0, 0, 0, e^{24} + e^{13}, e^{35} + e^{12}, e^{45} + e^{38} + e^{27} + e^{16}$  | 149      |
| Type: 63 |                                                                                          |          |
| 93:1     | $0, 0, 0, 0, 0, 0, e^{12}, e^{13}, e^{23}$                                               | 69       |
| 93:2     | $0, 0, 0, 0, 0, 0, e^{12}, e^{13}, e^{14}$                                               | 59       |
| 93:3     | $0, 0, 0, 0, 0, 0, e^{12}, e^{13}, e^{24}$                                               | 59       |
| 93:4     | $0, 0, 0, 0, 0, 0, e^{12}, e^{13}, e^{14} + e^{23}$                                      | 59       |
| 93:5     | $0, 0, 0, 0, 0, 0, e^{12}, e^{34}, e^{13} + e^{24}$                                      | 59       |
| 93:6a    | $0, 0, 0, 0, 0, 0, e^{12}, e^{14} + e^{23}, e^{13} + e^{24}$                             | 59       |
| 93:6b    | $0, 0, 0, 0, 0, 0, e^{12}, e^{23} - e^{14}, e^{24} + e^{13}$                             | 59       |
| 93:7a    | $0, 0, 0, 0, 0, 0, e^{14} + e^{23}, e^{24} + e^{13}, e^{12} + e^{34}$                    | 59       |
| 93:7b    | $0, 0, 0, 0, 0, 0, e^{14} + e^{23}, -e^{13} + e^{24}, e^{34} + e^{12}$                   | 59       |
| 93:8     | $0, 0, 0, 0, 0, 0, e^{12}, e^{13}, e^{45}$                                               | 49       |
| 93:9     | $0, 0, 0, 0, 0, 0, e^{12}, e^{13}, e^{25} + e^{14}$                                      | 49       |
| 93:10    | $0, 0, 0, 0, 0, 0, e^{12}, e^{13}, e^{23} + e^{45}$                                      | 49       |
| 93:11    | $0, 0, 0, 0, 0, 0, e^{12}, e^{13}, e^{24} + e^{35}$                                      | 49       |
| 93:12    | $0, 0, 0, 0, 0, 0, e^{12}, e^{34}, e^{25} + e^{13}$                                      | 49       |
| 93:13    | $0, 0, 0, 0, 0, 0, e^{12}, e^{23} + e^{14}, e^{13} + e^{25}$                             | 49       |
| 93:14    | $0, 0, 0, 0, 0, 0, e^{12}, e^{14} + e^{23}, e^{45} + e^{13}$                             | 49       |
| 93:15    | $0, 0, 0, 0, 0, 0, e^{12}, e^{13} + e^{24}, e^{15} + e^{34}$                             | 49       |
| 93:16a   | $0, 0, 0, 0, 0, 0, e^{24} + e^{13}, e^{34} + e^{12}, e^{15}$                             | 49       |
| 93:16b   | $0, 0, 0, 0, 0, 0, e^{24} - e^{13}, e^{34} + e^{12}, e^{15}$                             | 49       |
| 93:17    | $0, 0, 0, 0, 0, 0, e^{12}, e^{14} + e^{35}, e^{23} + e^{45}$                             | 49       |
| 93:18a   | $0, 0, 0, 0, 0, 0, e^{14} + e^{23}, e^{13} + e^{24}, e^{35} + e^{12}$                    | 49       |
| 93:18b   | $0, 0, 0, 0, 0, 0, -e^{14} + e^{23}, e^{13} + e^{24}, e^{12} + e^{35}$                   | 49       |
| 93:19    | $0, 0, 0, 0, 0, 0, e^{23} + e^{14}, e^{13} + e^{25}, e^{12} + e^{45}$                    | 49       |
| 93:20    | $0, 0, 0, 0, 0, 0, e^{24} + e^{13}, e^{15} + e^{23}, e^{25} + e^{14}$                    | 49       |
| 93:21    | $0, 0, 0, 0, 0, 0, e^{12}, e^{34}, e^{56}$                                               | 39       |
| 93:22    | $0, 0, 0, 0, 0, 0, e^{12}, e^{13}, e^{14} + e^{56}$                                      | 39       |
| 93:23    | $0, 0, 0, 0, 0, 0, e^{12}, e^{13}, e^{24} + e^{56}$                                      | 39       |
| 93:24    | $0, 0, 0, 0, 0, 0, e^{12}, e^{34}, e^{15} + e^{26}$                                      | 39       |
| 93:25    | $0, 0, 0, 0, 0, 0, e^{12}, e^{34}, e^{56} + e^{13}$                                      | 39       |
| 93:26    | $0, 0, 0, 0, 0, 0, e^{12}, e^{34}, e^{15} + e^{36}$                                      | 39       |
| 93:27    | $0, 0, 0, 0, 0, 0, e^{12}, e^{13}, e^{23} + e^{14} + e^{56}$                             | 39       |
| 93:28    | $0, 0, 0, 0, 0, 0, e^{12}, e^{13}, e^{36} + e^{25} + e^{14}$                             | 39       |
| 93:29    | $0, 0, 0, 0, 0, 0, e^{12}, e^{13} + e^{24}, e^{26} + e^{15}$                             | 39       |

Table 2 – Continued to next page

Table 2 – Continued from previous page

| Name   | $\mathfrak{g}$                                                                  | UCS Dim. |
|--------|---------------------------------------------------------------------------------|----------|
| 93:30  | $0, 0, 0, 0, 0, 0, e^{12}, e^{23} + e^{14}, e^{56} + e^{13}$                    | 39       |
| 93:31  | $0, 0, 0, 0, 0, 0, e^{12}, e^{24} + e^{13}, e^{15} + e^{36}$                    | 39       |
| 93:32  | $0, 0, 0, 0, 0, 0, e^{12}, e^{14} + e^{23}, e^{15} + e^{36}$                    | 39       |
| 93:33  | $0, 0, 0, 0, 0, 0, e^{12}, e^{34}, e^{13} + e^{24} + e^{56}$                    | 39       |
| 93:34  | $0, 0, 0, 0, 0, 0, e^{12}, e^{34}, e^{46} + e^{25} + e^{13}$                    | 39       |
| 93:35  | $0, 0, 0, 0, 0, 0, e^{12}, e^{24} + e^{13}, e^{56} + e^{34}$                    | 39       |
| 93:36  | $0, 0, 0, 0, 0, 0, e^{12}, e^{24} + e^{13}, e^{35} + e^{46}$                    | 39       |
| 93:37a | $0, 0, 0, 0, 0, 0, e^{13} + e^{24}, e^{34} + e^{12}, e^{56}$                    | 39       |
| 93:37b | $0, 0, 0, 0, 0, 0, -e^{13} + e^{24}, e^{12} + e^{34}, e^{56}$                   | 39       |
| 93:38  | $0, 0, 0, 0, 0, 0, e^{12}, e^{35} + e^{14}, e^{46} + e^{13}$                    | 39       |
| 93:39  | $0, 0, 0, 0, 0, 0, e^{12}, e^{15} + e^{34}, e^{13} + e^{46}$                    | 39       |
| 93:40  | $0, 0, 0, 0, 0, 0, e^{12}, e^{45} + e^{13}, e^{46} + e^{23}$                    | 39       |
| 93:41  | $0, 0, 0, 0, 0, 0, e^{12}, e^{35} + e^{14}, e^{46} + e^{23}$                    | 39       |
| 93:42  | $0, 0, 0, 0, 0, 0, e^{12}, e^{15} + e^{34}, e^{23} + e^{46}$                    | 39       |
| 93:43  | $0, 0, 0, 0, 0, 0, e^{12} + e^{34}, e^{15}, e^{46} + e^{23}$                    | 39       |
| 93:44a | $0, 0, 0, 0, 0, 0, e^{12}, e^{13} + e^{24}, e^{14} + e^{23} + e^{56}$           | 39       |
| 93:44b | $0, 0, 0, 0, 0, 0, e^{12}, e^{24} - e^{13}, e^{56} + e^{23} + e^{14}$           | 39       |
| 93:45  | $0, 0, 0, 0, 0, 0, e^{12}, e^{24} + e^{13}, e^{15} + e^{46} + e^{23}$           | 39       |
| 93:46  | $0, 0, 0, 0, 0, 0, e^{12}, e^{24} + e^{13}, e^{15} + e^{26} + e^{34}$           | 39       |
| 93:47a | $0, 0, 0, 0, 0, 0, e^{14} + e^{23}, e^{13} + e^{24}, e^{56} + e^{12}$           | 39       |
| 93:47b | $0, 0, 0, 0, 0, 0, -e^{14} + e^{23}, e^{13} + e^{24}, e^{12} + e^{56}$          | 39       |
| 93:48a | $0, 0, 0, 0, 0, 0, e^{24} + e^{13}, e^{12} + e^{34}, e^{15} + e^{26}$           | 39       |
| 93:48b | $0, 0, 0, 0, 0, 0, e^{24} - e^{13}, e^{12} + e^{34}, e^{26} + e^{15}$           | 39       |
| 93:49a | $0, 0, 0, 0, 0, 0, e^{14} + e^{23}, e^{13} + e^{24}, e^{26} + e^{15}$           | 39       |
| 93:49b | $0, 0, 0, 0, 0, 0, -e^{14} + e^{23}, e^{13} + e^{24}, e^{26} + e^{15}$          | 39       |
| 93:50  | $0, 0, 0, 0, 0, 0, e^{23} + e^{14}, e^{25} + e^{13}, e^{36} + e^{12}$           | 39       |
| 93:51  | $0, 0, 0, 0, 0, 0, e^{14} + e^{23}, e^{25} + e^{13}, e^{46} + e^{12}$           | 39       |
| 93:52  | $0, 0, 0, 0, 0, 0, e^{34} + e^{12}, e^{13} + e^{25}, e^{14} + e^{26}$           | 39       |
| 93:53  | $0, 0, 0, 0, 0, 0, e^{12} + e^{34}, e^{15} + e^{23}, e^{14} + e^{26}$           | 39       |
| 93:54  | $0, 0, 0, 0, 0, 0, e^{24} + e^{13}, e^{23} + e^{15}, e^{14} + e^{26}$           | 39       |
| 93:55  | $0, 0, 0, 0, 0, 0, e^{12}, e^{45} + e^{13}, e^{56} + e^{14} + e^{23}$           | 39       |
| 93:56  | $0, 0, 0, 0, 0, 0, e^{12}, e^{13} + e^{45}, e^{25} + e^{14} + e^{36}$           | 39       |
| 93:57a | $0, 0, 0, 0, 0, 0, e^{12}, e^{45} + e^{13}, e^{26} + e^{35} + e^{14}$           | 39       |
| 93:57b | $0, 0, 0, 0, 0, 0, e^{12}, e^{45} - e^{13}, e^{26} + e^{35} + e^{14}$           | 39       |
| 93:58  | $0, 0, 0, 0, 0, 0, e^{12}, e^{45} + e^{13}, e^{16} + e^{24} + e^{35}$           | 39       |
| 93:59  | $0, 0, 0, 0, 0, 0, e^{13} + e^{24}, e^{12} + e^{35}, e^{14} + e^{56}$           | 39       |
| 93:60  | $0, 0, 0, 0, 0, 0, e^{12} + e^{34}, e^{15} + e^{23}, e^{14} + e^{56}$           | 39       |
| 93:61  | $0, 0, 0, 0, 0, 0, e^{24} + e^{13}, e^{35} + e^{12}, e^{45} + e^{16}$           | 39       |
| 93:62  | $0, 0, 0, 0, 0, 0, e^{14} + e^{23}, e^{12} + e^{35}, e^{16} + e^{45}$           | 39       |
| 93:63  | $0, 0, 0, 0, 0, 0, e^{12}, e^{56} + e^{34}, e^{46} + e^{13} + e^{25}$           | 39       |
| 93:64a | $0, 0, 0, 0, 0, 0, e^{13} + e^{24}, e^{26} + e^{15}, e^{56} + e^{34}$           | 39       |
| 93:64b | $0, 0, 0, 0, 0, 0, e^{24} - e^{13}, e^{15} + e^{26}, e^{34} + e^{56}$           | 39       |
| 93:65a | $0, 0, 0, 0, 0, 0, e^{24} + e^{13}, e^{15} + e^{26}, e^{35} + e^{46}$           | 39       |
| 93:65b | $0, 0, 0, 0, 0, 0, -e^{13} + e^{24}, e^{26} + e^{15}, e^{46} + e^{35}$          | 39       |
| 93:66  | $0, 0, 0, 0, 0, 0, a_1 e^{14} + e^{23}, e^{26} + e^{15}, e^{46} + e^{35}$       | 39       |
| 93:67a | $0, 0, 0, 0, 0, 0, e^{24} + e^{13}, e^{12} + e^{34}, e^{56} + e^{14} + e^{23}$  | 39       |
| 93:67b | $0, 0, 0, 0, 0, 0, e^{13} + e^{24}, -e^{12} + e^{34}, e^{14} + e^{23} + e^{56}$ | 39       |
| 93:67c | $0, 0, 0, 0, 0, 0, e^{24} - e^{13}, e^{34} + e^{12}, e^{56} + e^{23} + e^{14}$  | 39       |
| 93:68a | $0, 0, 0, 0, 0, 0, e^{24} + e^{13}, e^{34} + e^{12}, e^{15} + e^{46} + e^{23}$  | 39       |
| 93:68b | $0, 0, 0, 0, 0, 0, e^{24} - e^{13}, e^{34} + e^{12}, e^{15} + e^{23} + e^{46}$  | 39       |
| 93:69a | $0, 0, 0, 0, 0, 0, e^{13} + e^{24}, e^{35} + e^{12}, e^{56} + e^{14} + e^{23}$  | 39       |
| 93:69b | $0, 0, 0, 0, 0, 0, e^{24} - e^{13}, e^{35} + e^{12}, e^{23} + e^{56} + e^{14}$  | 39       |
| 93:70  | $0, 0, 0, 0, 0, 0, e^{24} + e^{13}, e^{35} + e^{12}, e^{36} + e^{14} + e^{25}$  | 39       |
| 93:71  | $0, 0, 0, 0, 0, 0, e^{24} + e^{13}, e^{12} + e^{35}, e^{16} + e^{23} + e^{45}$  | 39       |
| 93:72  | $0, 0, 0, 0, 0, 0, e^{13} + e^{24}, e^{35} + e^{12}, e^{34} + e^{25} + e^{16}$  | 39       |
| 93:73  | $0, 0, 0, 0, 0, 0, e^{12}, e^{15} + e^{46} + e^{23}, e^{13} + e^{56} + e^{24}$  | 39       |
| 93:74  | $0, 0, 0, 0, 0, 0, e^{12}, e^{15} + e^{26} + e^{34}, e^{24} + e^{13} + e^{56}$  | 39       |
| 93:75  | $0, 0, 0, 0, 0, 0, e^{24} + e^{13}, e^{56} + e^{12}, e^{46} + e^{15} + e^{23}$  | 39       |

Table 2 – Continued to next page



Table 2 – Continued from previous page

| Name      | $\mathfrak{g}$                                                                                           | UCS Dim. |
|-----------|----------------------------------------------------------------------------------------------------------|----------|
| 93:76a    | $0, 0, 0, 0, 0, 0, e^{13} + e^{24}, e^{12} + e^{56}, e^{26} + e^{15} + e^{34}$                           | 39       |
| 93:76b    | $0, 0, 0, 0, 0, 0, e^{13} + e^{24}, -e^{12} + e^{56}, e^{15} + e^{34} + e^{26}$                          | 39       |
| 93:77a    | $0, 0, 0, 0, 0, 0, e^{24} + e^{13}, e^{15} + e^{26}, e^{12} + e^{34} + e^{56}$                           | 39       |
| 93:77b    | $0, 0, 0, 0, 0, 0, e^{24} + e^{13}, e^{26} - e^{15}, e^{56} + e^{12} + e^{34}$                           | 39       |
| 93:77c    | $0, 0, 0, 0, 0, 0, -e^{13} + e^{24}, e^{26} - e^{15}, e^{12} + e^{56} + e^{34}$                          | 39       |
| 93:78a    | $0, 0, 0, 0, 0, 0, e^{24} + e^{13}, e^{26} + e^{15}, e^{56} + e^{23} + e^{14}$                           | 39       |
| 93:78b    | $0, 0, 0, 0, 0, 0, e^{24} - e^{13}, e^{15} + e^{26}, e^{56} + e^{23} + e^{14}$                           | 39       |
| 93:79a    | $0, 0, 0, 0, 0, 0, e^{24} + e^{13}, e^{15} + e^{26}, e^{46} + e^{35} + e^{12}$                           | 39       |
| 93:79b    | $0, 0, 0, 0, 0, 0, -e^{13} + e^{24}, e^{26} + e^{15}, e^{12} + e^{46} + e^{35}$                          | 39       |
| 93:80     | $0, 0, 0, 0, 0, 0, e^{24} + a_1 e^{13}, e^{26} + e^{15}, e^{36} + e^{45} + e^{12}$                       | 39       |
| 93:81     | $0, 0, 0, 0, 0, 0, e^{24} + e^{13}, e^{26} + e^{15}, e^{36} + e^{25} + e^{14}$                           | 39       |
| 93:82a    | $0, 0, 0, 0, 0, 0, e^{34} + e^{12}, e^{46} + e^{15} + e^{23}, e^{56} + e^{13} + e^{24}$                  | 39       |
| 93:82b    | $0, 0, 0, 0, 0, 0, -e^{12} + e^{34}, e^{15} + e^{46} + e^{23}, e^{13} + e^{56} + e^{24}$                 | 39       |
| 93:83a    | $0, 0, 0, 0, 0, 0, e^{34} + e^{12}, e^{15} + e^{36} + e^{24}, e^{25} + e^{46} + e^{13}$                  | 39       |
| 93:83b    | $0, 0, 0, 0, 0, 0, e^{34} - e^{12}, e^{15} + e^{24} + e^{36}, e^{25} + e^{13} + e^{46}$                  | 39       |
| 93:84     | $0, 0, 0, 0, 0, 0, e^{34} + e^{12}, e^{35} + e^{14} + e^{26}, e^{46} + e^{13} + e^{25}$                  | 39       |
| 93:85     | $0, 0, 0, 0, 0, 0, e^{34} + a_1 e^{12}, e^{35} + e^{24} + e^{16}, e^{46} + e^{25} + e^{13}$              | 39       |
| 93:86     | $0, 0, 0, 0, 0, 0, e^{24} + e^{36} + e^{15} a_1, e^{46} + e^{13} + e^{25}, e^{56} + e^{12} + e^{34}$     | 39       |
| 93:87     | $0, 0, 0, 0, 0, 0, e^{16} a_1 + e^{35} + e^{24}, e^{46} + e^{25} + e^{13} a_2, e^{56} + e^{34} + e^{12}$ | 39       |
| Type: 711 |                                                                                                          |          |
| 921:1     | $0, 0, 0, 0, 0, 0, 0, e^{12}, e^{18}$                                                                    | 679      |
| 921:2     | $0, 0, 0, 0, 0, 0, 0, e^{12}, e^{28} + e^{13}$                                                           | 579      |
| 921:3     | $0, 0, 0, 0, 0, 0, 0, e^{12}, e^{34} + e^{18}$                                                           | 479      |
| 921:4     | $0, 0, 0, 0, 0, 0, 0, e^{12}, e^{13} + e^{45} + e^{28}$                                                  | 379      |
| 921:5     | $0, 0, 0, 0, 0, 0, 0, e^{12}, e^{34} + e^{18} + e^{56}$                                                  | 279      |
| 921:6     | $0, 0, 0, 0, 0, 0, 0, e^{12}, e^{28} + e^{67} + e^{45} + e^{13}$                                         | 179      |
| Type: 72  |                                                                                                          |          |
| 92:1      | $0, 0, 0, 0, 0, 0, 0, e^{12}, e^{13}$                                                                    | 69       |
| 92:2      | $0, 0, 0, 0, 0, 0, 0, e^{12}, e^{34}$                                                                    | 59       |
| 92:3      | $0, 0, 0, 0, 0, 0, 0, e^{12}, e^{24} + e^{13}$                                                           | 59       |
| 92:4a     | $0, 0, 0, 0, 0, 0, 0, e^{13} + e^{24}, e^{34} + e^{12}$                                                  | 59       |
| 92:4b     | $0, 0, 0, 0, 0, 0, 0, -e^{13} + e^{24}, e^{12} + e^{34}$                                                 | 59       |
| 92:5      | $0, 0, 0, 0, 0, 0, 0, e^{12}, e^{13} + e^{45}$                                                           | 49       |
| 92:6      | $0, 0, 0, 0, 0, 0, 0, e^{24} + e^{13}, e^{12} + e^{35}$                                                  | 49       |
| 92:7      | $0, 0, 0, 0, 0, 0, 0, e^{12}, e^{56} + e^{34}$                                                           | 39       |
| 92:8      | $0, 0, 0, 0, 0, 0, 0, e^{12}, e^{56} + e^{24} + e^{13}$                                                  | 39       |
| 92:9      | $0, 0, 0, 0, 0, 0, 0, e^{24} + e^{13}, e^{56} + e^{12}$                                                  | 39       |
| 92:10     | $0, 0, 0, 0, 0, 0, 0, e^{24} + e^{13}, e^{15} + e^{26}$                                                  | 39       |
| 92:11a    | $0, 0, 0, 0, 0, 0, 0, e^{12} + e^{34}, e^{13} + e^{24} + e^{56}$                                         | 39       |
| 92:11b    | $0, 0, 0, 0, 0, 0, 0, -e^{12} + e^{34}, e^{13} + e^{24} + e^{56}$                                        | 39       |
| 92:12     | $0, 0, 0, 0, 0, 0, 0, e^{12} + e^{34}, e^{13} + e^{46} + e^{25}$                                         | 39       |
| 92:13     | $0, 0, 0, 0, 0, 0, 0, e^{13} + e^{25} + e^{46}, e^{12} + e^{34} + e^{56}$                                | 39       |
| 92:14     | $0, 0, 0, 0, 0, 0, 0, e^{12}, e^{67} + e^{45} + e^{13}$                                                  | 29       |
| 92:15     | $0, 0, 0, 0, 0, 0, 0, e^{12} + e^{34}, e^{67} + e^{15}$                                                  | 29       |
| 92:16     | $0, 0, 0, 0, 0, 0, 0, e^{34} + e^{12}, e^{25} + e^{13} + e^{67}$                                         | 29       |
| 92:17     | $0, 0, 0, 0, 0, 0, 0, e^{34} + e^{12}, e^{15} + e^{37} + e^{26}$                                         | 29       |
| 92:18a    | $0, 0, 0, 0, 0, 0, 0, e^{13} + e^{24} + e^{56}, e^{12} + e^{57} + e^{34}$                                | 29       |
| 92:18b    | $0, 0, 0, 0, 0, 0, 0, e^{24} + e^{56} - e^{13}, e^{34} + e^{57} + e^{12}$                                | 29       |
| 92:19     | $0, 0, 0, 0, 0, 0, 0, e^{13} + e^{46} + e^{25}, e^{12} + e^{34} + e^{57}$                                | 29       |
| Type: 81  |                                                                                                          |          |
| 91:1      | $0, 0, 0, 0, 0, 0, 0, 0, e^{12}$                                                                         | 79       |
| 91:2      | $0, 0, 0, 0, 0, 0, 0, 0, e^{12} + e^{34}$                                                                | 59       |
| 91:3      | $0, 0, 0, 0, 0, 0, 0, 0, e^{56} + e^{34} + e^{12}$                                                       | 39       |
| 91:4      | $0, 0, 0, 0, 0, 0, 0, 0, e^{34} + e^{12} + e^{56} + e^{78}$                                              | 19       |
| Type: 9   |                                                                                                          |          |
| 9:1       | $0, 0, 0, 0, 0, 0, 0, 0, 0$                                                                              | 9        |

End of Table 2
